# Supplementary material for: Four-component relativistic range-separated density-functional theory: Short-range exchange local-density approximation
Source: arXiv:1812.02024 source file (2018-12-05)
Supplement: Supplementary file 1 [file supplementary.pdf]

# Supplementary Information to Four-component relativistic range-separated density-functional theory: Short-range exchange local-density approximation

Julien Paquier\* and Julien Toulouse†

*Laboratoire de Chimie Théorique (LCT), Sorbonne Université and CNRS, F-75005 Paris, France*

(Dated: July 25, 2018)

| CONTENTS                                                    |    |                                                                 |    |
|-------------------------------------------------------------|----|-----------------------------------------------------------------|----|
| <b>I Sums over spin combinations</b>                        | 1  |                                                                 |    |
| I. Coulomb contribution                                     | 1  |                                                                 |    |
| II. Breit contribution                                      | 2  |                                                                 |    |
| <b>II Large-<math>\tilde{c}</math> asymptotic expansion</b> | 4  |                                                                 |    |
| I. First part of the exchange energy ( $I$ )                | 5  |                                                                 |    |
| A. First integral of the first part ( $I_1$ )               | 5  |                                                                 |    |
| B. Second integral of the first part ( $I_2$ )              | 6  |                                                                 |    |
| 1. Integration over $k$ in $I_2$                            | 6  |                                                                 |    |
| 2. Integration over $k_1$ in $I_2$                          | 7  |                                                                 |    |
| 3. Expression of integral $I_2$                             | 10 |                                                                 |    |
| C. Third integral of the first part ( $I_3$ )               | 10 |                                                                 |    |
| 1. Integration over $k$ in $I_3$                            | 11 |                                                                 |    |
| 2. Integration over $k_1$ in $I_3$                          | 11 |                                                                 |    |
|                                                             |    | 3. Expression of integral $I_3$                                 | 14 |
|                                                             |    | <b>II. Second part of the exchange energy (<math>II</math>)</b> | 14 |
|                                                             |    | A. First integral of the second part ( $II_1$ )                 | 14 |
|                                                             |    | 1. Integration over $k$ in $II_1$                               | 15 |
|                                                             |    | 2. Integration over $k_1$ in $II_1$                             | 15 |
|                                                             |    | 3. Expression of integral $II_1$                                | 16 |
|                                                             |    | B. Second integral of the second part ( $II_2$ )                | 16 |
|                                                             |    | 1. Integration over $k$ in $II_2$                               | 16 |
|                                                             |    | 2. Integration over $k_1$ in $II_2$                             | 16 |
|                                                             |    | 3. Expression of integral $II_2$                                | 17 |
|                                                             |    | C. Third integral of the second part ( $II_3$ )                 | 17 |
|                                                             |    | 1. Integration over $k$ in $II_3$                               | 17 |
|                                                             |    | 2. Integration over $k_1$ in $II_3$                             | 18 |
|                                                             |    | 3. Expression of integral $II_3$                                | 20 |
|                                                             |    | D. Fourth integral of the second part ( $II_4$ )                | 20 |
|                                                             |    | 1. Integration over $k$ in $II_4$                               | 20 |
|                                                             |    | 2. Integration over $k_1$ in $II_4$                             | 21 |
|                                                             |    | 3. Expression of integral $II_4$                                | 22 |
|                                                             |    | References                                                      | 22 |

## Part I

## Sums over spin combinations

We give here the expressions of the sums over the “spin” combinations that are needed to calculate the exchange energy per particle of the relativistic homogeneous electron gas for the Coulomb-Breit electron-electron interaction [Eq. (A1) of the main paper]. The notations used here are the same as in the main paper [see in particular Section III A]. We first consider the Coulomb contribution, and then the Breit contribution which contains the  $\alpha$  matrices and is thus slightly more complex to calculate.

### I. COULOMB CONTRIBUTION

We wish to calculate the expression

$$\sum_{\sigma_1, \sigma_2 = \downarrow, \uparrow} \psi_{\mathbf{k}_1, \sigma_1}^\dagger(\mathbf{r}_1) \psi_{\mathbf{k}_2, \sigma_2}(\mathbf{r}_1) \psi_{\mathbf{k}_2, \sigma_2}^\dagger(\mathbf{r}_2) \psi_{\mathbf{k}_1, \sigma_1}(\mathbf{r}_2), \quad (1)$$

which means that we have to consider four spin combinations, and contrary to the non-relativistic case none of these combinations is zero.

---

\* julien.paquier@lct.jussieu.fr

† toulouse@lct.jussieu.fr

*a. Calculation of the  $\uparrow/\uparrow/\uparrow/\uparrow$  and  $\downarrow/\downarrow/\downarrow/\downarrow$  terms for the Coulomb interaction*

We consider the expression of the product of two  $\uparrow$ -spinors

$$\begin{aligned}\psi_{\mathbf{k}_1,\uparrow}^\dagger(\mathbf{r}_1)\psi_{\mathbf{k}_2,\uparrow}(\mathbf{r}_1) &= \begin{pmatrix} \varphi_{\mathbf{k}_1,\uparrow}^\dagger(\mathbf{r}_1) & \chi_{\mathbf{k}_1,\uparrow}^\dagger(\mathbf{r}_1) \end{pmatrix} \begin{pmatrix} \varphi_{\mathbf{k}_2,\uparrow}(\mathbf{r}_1) \\ \chi_{\mathbf{k}_2,\uparrow}(\mathbf{r}_1) \end{pmatrix} \\ &= (\varphi_{\mathbf{k}_1,\uparrow}^\dagger(\mathbf{r}_1)\varphi_{\mathbf{k}_2,\uparrow}(\mathbf{r}_1) + \chi_{\mathbf{k}_1,\uparrow}^\dagger(\mathbf{r}_1)\chi_{\mathbf{k}_2,\uparrow}(\mathbf{r}_1)) \\ &= \frac{1}{V} \sqrt{\frac{E_{k_1} + c^2}{2E_{k_1}}} \sqrt{\frac{E_{k_2} + c^2}{2E_{k_2}}} e^{-i(\mathbf{k}_2 - \mathbf{k}_1) \cdot \mathbf{r}_1} \left( 1 + \frac{c^2(\mathbf{k}_1 \cdot \mathbf{k}_2 + i(\mathbf{k}_1 \times \mathbf{k}_2)_z)}{(E_{k_1} + c^2)(E_{k_2} + c^2)} \right)\end{aligned}\quad (2)$$

so that

$$\psi_{\mathbf{k}_1,\uparrow}^\dagger(\mathbf{r}_1)\psi_{\mathbf{k}_2,\uparrow}(\mathbf{r}_1)\psi_{\mathbf{k}_2,\uparrow}^\dagger(\mathbf{r}_2)\psi_{\mathbf{k}_1,\uparrow}(\mathbf{r}_2) = \frac{1}{V^2} e^{-i(\mathbf{k}_2 - \mathbf{k}_1) \cdot (\mathbf{r}_1 - \mathbf{r}_2)} \left( \frac{(E_{k_1} + c^2)(E_{k_2} + c^2)}{4E_{k_1}E_{k_2}} + \frac{c^2(\mathbf{k}_1 \cdot \mathbf{k}_2)}{2E_{k_1}E_{k_2}} + \frac{c^4((\mathbf{k}_1 \cdot \mathbf{k}_2)^2 + (\mathbf{k}_1 \times \mathbf{k}_2)_z^2)}{4(E_{k_1} + c^2)(E_{k_2} + c^2)E_{k_1}E_{k_2}} \right) \quad (3)$$

with the  $\downarrow/\downarrow/\downarrow/\downarrow$  term being equal to this one.

*b. Calculation of the  $\uparrow/\downarrow/\downarrow/\uparrow$  and  $\downarrow/\uparrow/\uparrow/\downarrow$  terms for the Coulomb interaction*

We consider the expression of the product of a  $\uparrow$ -spinor and a  $\downarrow$ -spinor

$$\begin{aligned}\psi_{\mathbf{k}_1,\uparrow}^\dagger(\mathbf{r}_1)\psi_{\mathbf{k}_2,\downarrow}(\mathbf{r}_1) &= \begin{pmatrix} \varphi_{\mathbf{k}_1,\uparrow}^\dagger(\mathbf{r}_1) & \chi_{\mathbf{k}_1,\uparrow}^\dagger(\mathbf{r}_1) \end{pmatrix} \begin{pmatrix} \varphi_{\mathbf{k}_2,\downarrow}(\mathbf{r}_1) \\ \chi_{\mathbf{k}_2,\downarrow}(\mathbf{r}_1) \end{pmatrix} \\ &= (\varphi_{\mathbf{k}_1,\uparrow}^\dagger(\mathbf{r}_1)\varphi_{\mathbf{k}_2,\downarrow}(\mathbf{r}_1) + \chi_{\mathbf{k}_1,\uparrow}^\dagger(\mathbf{r}_1)\chi_{\mathbf{k}_2,\downarrow}(\mathbf{r}_1)) \\ &= \frac{1}{V} \sqrt{\frac{E_{k_1} + c^2}{2E_{k_1}}} \sqrt{\frac{E_{k_2} + c^2}{2E_{k_2}}} e^{-i(\mathbf{k}_2 - \mathbf{k}_1) \cdot \mathbf{r}_1} \frac{c^2 i((\mathbf{k}_1 \times \mathbf{k}_2)_x - i(\mathbf{k}_1 \times \mathbf{k}_2)_y)}{(E_{k_1} + c^2)(E_{k_2} + c^2)}\end{aligned}\quad (4)$$

thus giving us

$$\psi_{\mathbf{k}_1,\uparrow}^\dagger(\mathbf{r}_1)\psi_{\mathbf{k}_2,\downarrow}(\mathbf{r}_1)\psi_{\mathbf{k}_2,\downarrow}^\dagger(\mathbf{r}_2)\psi_{\mathbf{k}_1,\uparrow}(\mathbf{r}_2) = \frac{1}{V^2} e^{-i(\mathbf{k}_2 - \mathbf{k}_1) \cdot (\mathbf{r}_1 - \mathbf{r}_2)} \left( \frac{c^4((\mathbf{k}_1 \times \mathbf{k}_2)_x^2 + (\mathbf{k}_1 \times \mathbf{k}_2)_y^2)}{4(E_{k_1} + mc^2)(E_{k_2} + mc^2)E_{k_1}E_{k_2}} \right) \quad (5)$$

with the  $\downarrow/\uparrow/\uparrow/\downarrow$  term being equal to this one.

*c. Sum of the four Coulomb spin combinations*

The sum of the four spin combinations previously determined is, using the relative variables  $\mathbf{k}_{12} = \mathbf{k}_1 - \mathbf{k}_2$  and  $\mathbf{r}_{12} = \mathbf{r}_1 - \mathbf{r}_2$ ,

$$\begin{aligned}\sum_{\sigma_1, \sigma_2 = \uparrow, \downarrow} \psi_{\mathbf{k}_1, \sigma_1}^\dagger(\mathbf{r}_1)\psi_{\mathbf{k}_2, \sigma_2}(\mathbf{r}_1)\psi_{\mathbf{k}_2, \sigma_2}^\dagger(\mathbf{r}_2)\psi_{\mathbf{k}_1, \sigma_1}(\mathbf{r}_2) &= \frac{1}{V^2} e^{-i\mathbf{k}_{12} \cdot \mathbf{r}_{12}} \left( \frac{(E_{k_1} + c^2)(E_{k_2} + c^2)}{4E_{k_1}E_{k_2}} + \frac{c^2(\mathbf{k}_1 \cdot \mathbf{k}_2)}{2E_{k_1}E_{k_2}} + \frac{c^4((\mathbf{k}_1 \cdot \mathbf{k}_2)^2 + (\mathbf{k}_1 \times \mathbf{k}_2)_z^2)}{4(E_{k_1} + c^2)(E_{k_2} + c^2)E_{k_1}E_{k_2}} \right) \\ &= \frac{1}{V^2} e^{-i\mathbf{k}_{12} \cdot \mathbf{r}_{12}} \frac{E_{k_1}E_{k_2} + (\mathbf{k}_1 \cdot \mathbf{k}_2)c^2 + c^4}{E_{k_1}E_{k_2}}.\end{aligned}\quad (6)$$

## II. BREIT CONTRIBUTION

We wish to calculate the expression

$$\sum_{\sigma_1, \sigma_2 = \uparrow, \downarrow} \left( \psi_{\mathbf{k}_1, \sigma_1}^\dagger(\mathbf{r}_1)\alpha_1\psi_{\mathbf{k}_2, \sigma_2}(\mathbf{r}_1) \cdot \psi_{\mathbf{k}_2, \sigma_2}^\dagger(\mathbf{r}_2)\alpha_2\psi_{\mathbf{k}_1, \sigma_1}(\mathbf{r}_2) + \frac{\psi_{\mathbf{k}_1, \sigma_1}^\dagger(\mathbf{r}_1)(\alpha_1 \cdot \mathbf{r}_{12})\psi_{\mathbf{k}_2, \sigma_2}(\mathbf{r}_1) \psi_{\mathbf{k}_2, \sigma_2}^\dagger(\mathbf{r}_2)(\alpha_2 \cdot \mathbf{r}_{12})\psi_{\mathbf{k}_1, \sigma_1}(\mathbf{r}_2)}{r_{12}^2} \right). \quad (7)$$

We work in two steps: first, we calculate the four spin combinations for the first Gaunt-type part (which we shall simply refer to as Gaunt in the following), and then we calculate the four spin combinations for the Gauge retardation part (which we shall simply refer to as Gauge in the following).

*a. Calculation of the  $\uparrow/\uparrow/\uparrow/\uparrow$  and  $\downarrow/\downarrow/\downarrow/\downarrow$  terms for the Gaunt part of the Breit interaction:*

We consider the expression of the product of two  $\uparrow$ -spinors

$$\begin{aligned}\psi_{\mathbf{k}_1,\uparrow}^\dagger(\mathbf{r}_1)\alpha_1\psi_{\mathbf{k}_2,\uparrow}(\mathbf{r}_1) &= \begin{pmatrix} \varphi_{\mathbf{k}_1,\uparrow}^\dagger(\mathbf{r}_1) & \chi_{\mathbf{k}_1,\uparrow}^\dagger(\mathbf{r}_1) \end{pmatrix} \begin{pmatrix} 0 & \sigma \\ \sigma & 0 \end{pmatrix} \begin{pmatrix} \varphi_{\mathbf{k}_2,\uparrow}(\mathbf{r}_1) \\ \chi_{\mathbf{k}_2,\uparrow}(\mathbf{r}_1) \end{pmatrix} \\ &= (\chi_{\mathbf{k}_1,\uparrow}^\dagger(\mathbf{r}_1)\sigma\varphi_{\mathbf{k}_2,\uparrow}(\mathbf{r}_1) + \varphi_{\mathbf{k}_1,\uparrow}^\dagger(\mathbf{r}_1)\sigma\chi_{\mathbf{k}_2,\uparrow}(\mathbf{r}_1)) \\ &= \frac{1}{V} \sqrt{\frac{E_{k_1} + c^2}{2E_{k_1}}} \sqrt{\frac{E_{k_2} + c^2}{2E_{k_2}}} e^{-i(\mathbf{k}_2 - \mathbf{k}_1) \cdot \mathbf{r}_1} \left[ \frac{c}{E_{k_1} + c^2} \begin{pmatrix} (k_1)_x - i(k_1)_y \\ i(k_1)_x + (k_1)_y \\ (k_1)_z \end{pmatrix} + \frac{c}{E_{k_2} + c^2} \begin{pmatrix} (k_2)_x + i(k_2)_y \\ -i(k_2)_x + (k_2)_y \\ (k_2)_z \end{pmatrix} \right] \quad (8)\end{aligned}$$

thus we have

$$\begin{aligned}\psi_{\mathbf{k}_1,\uparrow}^\dagger(\mathbf{r}_1)\alpha_1\psi_{\mathbf{k}_2,\uparrow}(\mathbf{r}_1) \cdot \psi_{\mathbf{k}_2,\uparrow}^\dagger(\mathbf{r}_2)\alpha_2\psi_{\mathbf{k}_1,\uparrow}(\mathbf{r}_2) &= \frac{1}{V^2} \frac{e^{-i\mathbf{k}_{12} \cdot \mathbf{r}_{12}}}{4E_{k_1}E_{k_2}} \left( \frac{c^2(E_{k_2} + c^2)}{(E_{k_1} + c^2)} (2k_1^2 - (k_1)_z^2) + \frac{c^2(E_{k_1} + c^2)}{(E_{k_2} + c^2)} (2k_2^2 - (k_2)_z^2) \right. \\ &\quad \left. + 2c^2(k_1)_z(k_2)_z \right) \quad (9)\end{aligned}$$

with the  $\downarrow\downarrow/\downarrow\downarrow$  term equal to this one.

*b. Calculation of the  $\uparrow\downarrow/\downarrow\uparrow$  and  $\downarrow\uparrow/\uparrow\downarrow$  terms for the Gaunt part of the Breit interaction*

We consider the expression of the product of a  $\uparrow$ -spinor and a  $\downarrow$ -spinor

$$\begin{aligned}\psi_{\mathbf{k}_1,\uparrow}^\dagger(\mathbf{r}_1)\alpha_1\psi_{\mathbf{k}_2,\downarrow}(\mathbf{r}_1) &= \begin{pmatrix} \varphi_{\mathbf{k}_1,\uparrow}^\dagger(\mathbf{r}_1) & \chi_{\mathbf{k}_1,\uparrow}^\dagger(\mathbf{r}_1) \end{pmatrix} \begin{pmatrix} 0 & \sigma \\ \sigma & 0 \end{pmatrix} \begin{pmatrix} \varphi_{\mathbf{k}_2,\downarrow}(\mathbf{r}_1) \\ \chi_{\mathbf{k}_2,\downarrow}(\mathbf{r}_1) \end{pmatrix} \\ &= (\chi_{\mathbf{k}_1,\uparrow}^\dagger(\mathbf{r}_1)\sigma\varphi_{\mathbf{k}_2,\downarrow}(\mathbf{r}_1) + \varphi_{\mathbf{k}_1,\uparrow}^\dagger(\mathbf{r}_1)\sigma\chi_{\mathbf{k}_2,\downarrow}(\mathbf{r}_1)) \\ &= \frac{1}{V} \sqrt{\frac{E_{k_1} + c^2}{2E_{k_1}}} \sqrt{\frac{E_{k_2} + c^2}{2E_{k_2}}} e^{-i(\mathbf{k}_2 - \mathbf{k}_1) \cdot \mathbf{r}_1} \left[ \frac{c}{E_{k_1} + c^2} \begin{pmatrix} (k_1)_z \\ -i(k_1)_z \\ -(k_1)_x + i(k_1)_y \end{pmatrix} + \frac{c}{E_{k_2} + c^2} \begin{pmatrix} -(k_2)_z \\ i(k_2)_z \\ (k_2)_x - i(k_2)_y \end{pmatrix} \right] \quad (10)\end{aligned}$$

so that

$$\begin{aligned}\psi_{\mathbf{k}_1,\uparrow}^\dagger(\mathbf{r}_1)\alpha_1\psi_{\mathbf{k}_2,\downarrow}(\mathbf{r}_1) \cdot \psi_{\mathbf{k}_2,\downarrow}^\dagger(\mathbf{r}_2)\alpha_2\psi_{\mathbf{k}_1,\uparrow}(\mathbf{r}_2) &= \frac{1}{V^2} \frac{e^{-i\mathbf{k}_{12} \cdot \mathbf{r}_{12}}}{4E_{k_1}E_{k_2}} \left( \frac{c^2(E_{k_1} + c^2)}{(E_{k_1} + c^2)} (k_1^2 + (k_1)_z^2) + \frac{c^2(E_{k_2} + c^2)}{(E_{k_2} + c^2)} (k_2^2 + (k_2)_z^2) \right. \\ &\quad \left. - 2c^2(\mathbf{k}_1 \cdot \mathbf{k}_2 + (k_1)_z(k_2)_z) \right) \quad (11)\end{aligned}$$

with the  $\downarrow\uparrow/\uparrow\downarrow$  term equal to this one.

*c. Calculation of the  $\uparrow\uparrow/\uparrow\uparrow$  and  $\downarrow\downarrow/\downarrow\downarrow$  term for the Gauge part of the Breit interaction*

We consider the expression of the product of two  $\uparrow$ -spinors

$$\begin{aligned}\psi_{\mathbf{k}_1,\uparrow}^\dagger(\mathbf{r}_1)(\alpha_1 \cdot \mathbf{r})\psi_{\mathbf{k}_2,\uparrow}(\mathbf{r}_1) &= \begin{pmatrix} \varphi_{\mathbf{k}_1,\uparrow}^\dagger(\mathbf{r}_1) & \chi_{\mathbf{k}_1,\uparrow}^\dagger(\mathbf{r}_1) \end{pmatrix} \begin{pmatrix} 0 & \sigma \cdot \mathbf{r} \\ \sigma \cdot \mathbf{r} & 0 \end{pmatrix} \begin{pmatrix} \varphi_{\mathbf{k}_2,\uparrow}(\mathbf{r}_1) \\ \chi_{\mathbf{k}_2,\uparrow}(\mathbf{r}_1) \end{pmatrix} \\ &= (\chi_{\mathbf{k}_1,\uparrow}^\dagger(\mathbf{r}_1)(\sigma \cdot \mathbf{r})\varphi_{\mathbf{k}_2,\uparrow}(\mathbf{r}_1) + \varphi_{\mathbf{k}_1,\uparrow}^\dagger(\mathbf{r}_1)(\sigma \cdot \mathbf{r})\chi_{\mathbf{k}_2,\uparrow}(\mathbf{r}_1)) \\ &= \frac{1}{V} \sqrt{\frac{E_{k_1} + c^2}{2E_{k_1}}} \sqrt{\frac{E_{k_2} + c^2}{2E_{k_2}}} e^{-i(\mathbf{k}_2 - \mathbf{k}_1) \cdot \mathbf{r}_1} \left( \frac{c}{E_{k_1} + c^2} (\mathbf{k}_1 \cdot \mathbf{r} + i(\mathbf{k}_1 \times \mathbf{r})_z) + \frac{c}{E_{k_2} + c^2} (\mathbf{k}_2 \cdot \mathbf{r} - i(\mathbf{k}_2 \times \mathbf{r})_z) \right) \quad (12)\end{aligned}$$

so that

$$\begin{aligned}\psi_{\mathbf{k}_1,\uparrow}^\dagger(\mathbf{r}_1)(\alpha_1 \cdot \mathbf{r})\psi_{\mathbf{k}_2,\uparrow}(\mathbf{r}_1) \cdot \psi_{\mathbf{k}_2,\uparrow}^\dagger(\mathbf{r}_2)(\alpha_2 \cdot \mathbf{r})\psi_{\mathbf{k}_1,\uparrow}(\mathbf{r}_2) &= \frac{1}{V^2} \frac{e^{-i\mathbf{k}_{12} \cdot \mathbf{r}_{12}}}{4E_{k_1}E_{k_2}} \left( \frac{c^2(E_{k_2} + c^2)}{(E_{k_1} + c^2)} ((\mathbf{k}_1 \cdot \mathbf{r})^2 + (\mathbf{k}_1 \times \mathbf{r})_z^2) \right. \\ &\quad \left. + \frac{c^2(E_{k_1} + c^2)}{(E_{k_2} + c^2)} ((\mathbf{k}_2 \cdot \mathbf{r})^2 + (\mathbf{k}_2 \times \mathbf{r})_z^2) + 2c^2((\mathbf{k}_1 \cdot \mathbf{r})(\mathbf{k}_2 \cdot \mathbf{r}) - (\mathbf{k}_1 \times \mathbf{r})_z(\mathbf{k}_2 \times \mathbf{r})_z) \right) \quad (13)\end{aligned}$$

with the  $\downarrow\downarrow/\downarrow\downarrow$  term being equal to this one.

*d. Calculation of the  $\uparrow\downarrow/\downarrow\uparrow$  and  $\downarrow\uparrow/\uparrow\downarrow$  term for the Gauge part of the Breit interaction*

We consider the expression of the product of a  $\uparrow$ -spinor and a  $\downarrow$ -spinor

$$\begin{aligned}
\psi_{\mathbf{k}_1,\uparrow}^\dagger(\mathbf{r}_1)(\boldsymbol{\alpha}_1 \cdot \mathbf{r})\psi_{\mathbf{k}_2,\downarrow}(\mathbf{r}_1) &= \begin{pmatrix} \varphi_{\mathbf{k}_1,\uparrow}^\dagger(\mathbf{r}_1) & \chi_{\mathbf{k}_1,\uparrow}^\dagger(\mathbf{r}_1) \end{pmatrix} \begin{pmatrix} 0 & \boldsymbol{\sigma} \cdot \mathbf{r} \\ \boldsymbol{\sigma} \cdot \mathbf{r} & 0 \end{pmatrix} \begin{pmatrix} \varphi_{\mathbf{k}_2,\downarrow}(\mathbf{r}_1) \\ \chi_{\mathbf{k}_2,\downarrow}(\mathbf{r}_1) \end{pmatrix} \\
&= \left( \chi_{\mathbf{k}_1,\uparrow}^\dagger(\mathbf{r}_1)(\boldsymbol{\sigma} \cdot \mathbf{r})\varphi_{\mathbf{k}_2,\downarrow}(\mathbf{r}_1) + \varphi_{\mathbf{k}_1,\uparrow}^\dagger(\mathbf{r}_1)(\boldsymbol{\sigma} \cdot \mathbf{r})\chi_{\mathbf{k}_2,\downarrow}(\mathbf{r}_1) \right) \\
&= \frac{1}{V} \sqrt{\frac{E_{k_1} + c^2}{2E_{k_1}}} \sqrt{\frac{E_{k_2} + c^2}{2E_{k_2}}} e^{-i(\mathbf{k}_2 - \mathbf{k}_1) \cdot \mathbf{r}_1} \left( \frac{c}{E_{k_1} + c^2} \left( i(\mathbf{k}_1 \times \mathbf{r})_x + (\mathbf{k}_1 \times \mathbf{r})_y \right) \right. \\
&\quad \left. + \frac{c}{E_{k_2} + c^2} \left( -i(\mathbf{k}_2 \times \mathbf{r})_x - (\mathbf{k}_2 \times \mathbf{r})_y \right) \right) \quad (14)
\end{aligned}$$

so that

$$\begin{aligned}
\psi_{\mathbf{k}_1,\uparrow}^\dagger(\mathbf{r}_1)(\boldsymbol{\alpha}_1 \cdot \mathbf{r})\psi_{\mathbf{k}_2,\downarrow}(\mathbf{r}_1)\psi_{\mathbf{k}_2,\downarrow}^\dagger(\mathbf{r}_2)(\boldsymbol{\alpha}_2 \cdot \mathbf{r})\psi_{\mathbf{k}_1,\uparrow}(\mathbf{r}_2) &= \frac{1}{V^2} \frac{e^{-i\mathbf{k}_{12} \cdot \mathbf{r}_{12}}}{4E_{k_1}E_{k_2}} \left( \frac{c^2(E_{k_2} + c^2)}{(E_{k_1} + c^2)} \left( (\mathbf{k}_1 \times \mathbf{r})_x^2 + (\mathbf{k}_1 \times \mathbf{r})_y^2 \right) \right. \\
&\quad \left. + \frac{c^2(E_{k_1} + c^2)}{(E_{k_2} + c^2)} \left( (\mathbf{k}_2 \times \mathbf{r})_x^2 + (\mathbf{k}_2 \times \mathbf{r})_y^2 \right) - 2c^2 \left( (\mathbf{k}_1 \times \mathbf{r})_x(\mathbf{k}_2 \times \mathbf{r})_x + (\mathbf{k}_1 \times \mathbf{r})_y(\mathbf{k}_2 \times \mathbf{r})_y \right) \right) \quad (15)
\end{aligned}$$

with the  $\downarrow/\uparrow/\downarrow$  term equal to this one.

#### e. Sum of the four Gaunt and four Gauge terms

The sum of the eight spins combinations previously determined is

$$\begin{aligned}
\sum_{\sigma_1, \sigma_2 = \downarrow, \uparrow} &\left( \psi_{\mathbf{k}_1, \sigma_1}^\dagger(\mathbf{r}_1)\boldsymbol{\alpha}_1\psi_{\mathbf{k}_2, \sigma_2}(\mathbf{r}_1) \cdot \psi_{\mathbf{k}_2, \sigma_2}^\dagger(\mathbf{r}_2)\boldsymbol{\alpha}_2\psi_{\mathbf{k}_1, \sigma_1}(\mathbf{r}_2) + \frac{\psi_{\mathbf{k}_1, \sigma_1}^\dagger(\mathbf{r}_1)(\boldsymbol{\alpha}_1 \cdot \mathbf{r}_{12})\psi_{\mathbf{k}_2, \sigma_2}(\mathbf{r}_1) \psi_{\mathbf{k}_2, \sigma_2}^\dagger(\mathbf{r}_2)(\boldsymbol{\alpha}_2 \cdot \mathbf{r}_{12})\psi_{\mathbf{k}_1, \sigma_1}(\mathbf{r}_2)}{r_{12}^2} \right) \\
&= 2 \frac{e^{-i\mathbf{k}_{12} \cdot \mathbf{r}_{12}}}{V^2} \frac{c^2}{4E_{k_1}E_{k_2}} \left( \frac{E_{k_2} + c^2}{E_{k_1} + c^2} \left( 3k_1^2 + \frac{(\mathbf{k}_1 \cdot \mathbf{r})^2 + (\mathbf{k}_1 \times \mathbf{r})^2}{r^2} \right) + \frac{E_{k_1} + c^2}{E_{k_2} + c^2} \left( 3k_2^2 + \frac{(\mathbf{k}_2 \cdot \mathbf{r})^2 + (\mathbf{k}_2 \times \mathbf{r})^2}{r^2} \right) \right. \\
&\quad \left. + 2 \left( -\mathbf{k}_1 \cdot \mathbf{k}_2 + \frac{(\mathbf{k}_1 \cdot \mathbf{r})(\mathbf{k}_2 \cdot \mathbf{r})}{r^2} - \frac{(\mathbf{k}_1 \times \mathbf{r})(\mathbf{k}_2 \times \mathbf{r})}{r^2} \right) \right) \\
&= 2 \frac{e^{-i\mathbf{k}_{12} \cdot \mathbf{r}_{12}}}{V^2} \frac{c^2}{E_{k_1}E_{k_2}} \left( \frac{E_{k_2} + c^2}{E_{k_1} + c^2} k_1^2 + \frac{E_{k_1} + c^2}{E_{k_2} + c^2} k_2^2 \right) \quad (16)
\end{aligned}$$

where the last expression has been simplified considering that

$$\left( -\mathbf{k}_1 \cdot \mathbf{k}_2 + \frac{(\mathbf{k}_1 \cdot \mathbf{r})(\mathbf{k}_2 \cdot \mathbf{r})}{r^2} - \frac{(\mathbf{k}_1 \times \mathbf{r})(\mathbf{k}_2 \times \mathbf{r})}{r^2} \right) = -2k_1k_2 \sin(\theta_1) \sin(\theta_2) \cos(\phi_1 - \phi_2) \quad (17)$$

is zero once integrated over  $\phi_1$  or  $\phi_2$  on  $[0, 2\pi]$ , and therefore this term can be removed with the understanding that the expression must always be used in an integral over  $\phi_1$  or  $\phi_2$ .

## Part II

# Large- $\tilde{c}$ asymptotic expansion

We explain here the key steps involved in the analytical calculation of the coefficients of the large- $\tilde{c}$  asymptotic expansions of the short-range Coulomb and Breit exchange energies per particle [Eqs. (36) and (41) of the main paper]. The Coulomb and Breit terms being of similar forms, we only explicitly consider the short-range Coulomb exchange energy per particle. We start

from its expression in Eq. (35) of the main paper

$$\begin{aligned} \epsilon_x^{C, sr, \mu} = & \frac{3k_F}{4\pi} \int_{\tilde{k}_1=0}^1 \int_{\tilde{k}_2=0}^1 d\tilde{k}_1 d\tilde{k}_2 \tilde{k}_1 \tilde{k}_2 \left( \frac{1}{\sqrt{\tilde{c}^2 + \tilde{k}_1^2} \sqrt{\tilde{c}^2 + \tilde{k}_2^2}} \left[ \tilde{k}_1 \tilde{k}_2 + \left( e^{-\left(\frac{\tilde{k}_1 + \tilde{k}_2}{2\tilde{\mu}}\right)^2} - e^{-\left(\frac{\tilde{k}_1 - \tilde{k}_2}{2\tilde{\mu}}\right)^2} \right) \tilde{\mu}^2 \right] \right. \\ & \left. + \frac{2\tilde{c}^2 + \tilde{k}_1^2 + \tilde{k}_2^2 + 2\sqrt{\tilde{c}^2 + \tilde{k}_1^2} \sqrt{\tilde{c}^2 + \tilde{k}_2^2}}{4\sqrt{\tilde{c}^2 + \tilde{k}_1^2} \sqrt{\tilde{c}^2 + \tilde{k}_2^2}} \left[ \text{Ei}\left(-\left(\frac{\tilde{k}_1 + \tilde{k}_2}{2\tilde{\mu}}\right)^2\right) - \text{Ei}\left(-\left(\frac{\tilde{k}_1 - \tilde{k}_2}{2\tilde{\mu}}\right)^2\right) + \ln((\tilde{k}_1 - \tilde{k}_2)^2) - \ln((\tilde{k}_1 + \tilde{k}_2)^2) \right] \right). \end{aligned} \quad (18)$$

From now on, for simplicity, we drop the tilde notation and it will be implicit that  $k_1, k_2, c$ , and  $\mu$  are in units of  $k_F$ . We want to find the expansion for  $c \rightarrow \infty$ . The expansion of the first part of the integrand is

$$\frac{\frac{1}{c^2}}{\sqrt{1 + \frac{k_1^2}{c^2}} \sqrt{1 + \frac{k_2^2}{c^2}}} = \frac{1}{c^2} - \left( \frac{k_1^2}{2} + \frac{k_2^2}{2} \right) \frac{1}{c^4} + \left( \frac{3k_1^4}{8} + \frac{k_1^2 k_2^2}{4} + \frac{3k_2^4}{8} \right) \frac{1}{c^6} + O\left(\frac{1}{c^8}\right), \quad (19)$$

and the expansion of the second part of the integrand is

$$\frac{2 + (k_1^2 + k_2^2) \frac{1}{c^2} + 2\sqrt{1 + \frac{k_1^2}{c^2}} \sqrt{1 + \frac{k_2^2}{c^2}}}{4\sqrt{1 + \frac{k_1^2}{c^2}} \sqrt{1 + \frac{k_2^2}{c^2}}} = 1 + \left( \frac{k_1^4}{16} - \frac{k_1^2 k_2^2}{8} + \frac{k_2^4}{16} \right) \frac{1}{c^4} + O\left(\frac{1}{c^6}\right). \quad (20)$$

Permuting the sum and the integrals, we integrate the general term of the large- $\tilde{c}$  expansion. For the first part of the exchange energy, we need to calculate the general term

$$\frac{a_{m,n}}{c^{2m+2n+2}} \int_{k_1=0}^1 \int_{k_2=0}^1 k_1^{1+2m} k_2^{1+2n} \left[ k_1 k_2 + \left( e^{-\left(\frac{k_1 + k_2}{2\mu}\right)^2} - e^{-\left(\frac{k_1 - k_2}{2\mu}\right)^2} \right) \mu^2 \right] dk_2 dk_1, \quad (21)$$

and for the second part of the exchange energy, we need to calculate the general term

$$\frac{b_{m,n}}{c^{2m+2n}} \int_{k_1=0}^1 \int_{k_2=0}^1 k_1^{1+2m} k_2^{1+2n} \left[ \text{Ei}\left(-\left(\frac{k_1 + k_2}{2\mu}\right)^2\right) - \text{Ei}\left(-\left(\frac{k_1 - k_2}{2\mu}\right)^2\right) + \ln((k_1 - k_2)^2) - \ln((k_1 + k_2)^2) \right] dk_2 dk_1, \quad (22)$$

with  $m$  and  $n$  positive integers,  $a_{m,n}$  and  $b_{m,n}$  being expressed using the coefficients of Eqs. (19) and (20) and are determined uniquely by the pair  $\{m, n\}$ . We observe a symmetry in  $m$  and  $n$ , so that only half the terms needs to be calculated.

These integrals are analytically calculated in the following pages because, although they can be calculated using the program Wolfram Mathematica [1] for a given value of  $2m + 2n$ , the general term for an unspecified value of  $2m + 2n$  cannot be directly integrated by the program. It is convenient to have the analytical expression of the general term in order to calculate the expansion for large orders. The final complete expressions of the large- $c$  expansions and their associated Padé approximants are explicitly given up to an arbitrary order in the accompanying Mathematica notebook.

## I. FIRST PART OF THE EXCHANGE ENERGY ( $I$ )

$$I = \int_{k_1=0}^1 \int_{k_2=0}^1 k_1^{1+2m} k_2^{1+2n} \left[ k_1 k_2 + \left( e^{-\left(\frac{k_1 + k_2}{2\mu}\right)^2} - e^{-\left(\frac{k_1 - k_2}{2\mu}\right)^2} \right) \mu^2 \right] dk_2 dk_1. \quad (23)$$

### A. First integral of the first part ( $I_1$ )

The first integral of the first part gives

$$I_1 = \int_{k_1=0}^1 \int_{k_2=0}^1 k_1^{2+2m} k_2^{2+2n} dk_2 dk_1 = \frac{1}{9 + 6m + 6n + 4mn}. \quad (24)$$

## B. Second integral of the first part ( $I_2$ )

The second integral of the first part is

$$I_2 = \int_{k_1=0}^1 \int_{k_2=0}^1 k_1^{1+2m} k_2^{1+2n} e^{-\left(\frac{k_1+k_2}{2\mu}\right)^2} dk_2 dk_1, \quad (25)$$

which can be calculated using changes of variables, binomial expansions, and integrations by parts. It will be more or less the same procedure for all the following integral calculations, we shall do it once in full.

We start with a change of variable,  $k_2 = 2\mu k - k_1$ , so that we have

$$I_2 = 2\mu \int_{k_1=0}^1 \int_{k=\frac{k_1}{2\mu}}^{\frac{1+k_1}{2\mu}} k_1^{1+2m} (2\mu k - k_1)^{1+2n} e^{-k^2} dk dk_1, \quad (26)$$

then we use a binomial expansion to express our integral as

$$I_2 = \sum_{i=0}^{1+2n} \binom{1+2n}{i} (-1)^{1-i} (2\mu)^{1+i} \int_{k_1=0}^1 k_1^{2+2(m+n)-i} \left( \int_{k=\frac{k_1}{2\mu}}^{\frac{1+k_1}{2\mu}} k^i e^{-k^2} dk \right) dk_1. \quad (27)$$

We now consider the two last integrals successively, first the one over  $k$  and then the one over  $k_1$ .

### 1. Integration over $k$ in $I_2$

We calculate the integral over  $k$  with repeated integrations by parts using at each step

$$\frac{d}{dk} k^{i-1} = (i-1)k^{i-2} \quad \text{and} \quad \int^k x e^{-x^2} dx = -\frac{1}{2} e^{-k^2}. \quad (28)$$

For the first step of the integration by parts, we have

$$\int_{k=\frac{k_1}{2\mu}}^{\frac{1+k_1}{2\mu}} k^{i-1} k e^{-k^2} dk = -\frac{1}{2} \left[ \left( \frac{1+k_1}{2\mu} \right)^{i-1} e^{-\left(\frac{1+k_1}{2\mu}\right)^2} - \left( \frac{k_1}{2\mu} \right)^{i-1} e^{-\left(\frac{k_1}{2\mu}\right)^2} \right] + \frac{i-1}{2} \int_{k=\frac{k_1}{2\mu}}^{\frac{1+k_1}{2\mu}} k^{i-3} k e^{-k^2} dk. \quad (29)$$

The repeated integrations by parts lead to two different cases for the last integral, depending on the parity of the integer  $i$ .

If  $i$  is even, the final integral obtained is

$$\int_{k=\frac{k_1}{2\mu}}^{\frac{1+k_1}{2\mu}} e^{-k^2} dk = \frac{\sqrt{\pi}}{2} \left[ \operatorname{erf}\left(\frac{1+k_1}{2\mu}\right) - \operatorname{erf}\left(\frac{k_1}{2\mu}\right) \right] \quad (30)$$

so that we have

$$\begin{aligned} \int_{k=\frac{k_1}{2\mu}}^{\frac{1+k_1}{2\mu}} k^i e^{-k^2} dk = & - \sum_{l_p=0}^{\frac{i}{2}-1} \frac{1}{2^{l_p+1}} \frac{(i-1)!!}{(i-1-2l_p)!!} \left[ \left( \frac{1+k_1}{2\mu} \right)^{i-1-2l_p} e^{-\left(\frac{1+k_1}{2\mu}\right)^2} - \left( \frac{k_1}{2\mu} \right)^{i-1-2l_p} e^{-\left(\frac{k_1}{2\mu}\right)^2} \right] \\ & + \frac{(i-1)!!}{2^{\frac{i}{2}}} \frac{\sqrt{\pi}}{2} \left[ \operatorname{erf}\left(\frac{1+k_1}{2\mu}\right) - \operatorname{erf}\left(\frac{k_1}{2\mu}\right) \right]. \end{aligned} \quad (31)$$

If  $i$  is odd, the final integral obtained is

$$\int_{k=\frac{k_1}{2\mu}}^{\frac{1+k_1}{2\mu}} k e^{-k^2} dk = \frac{-1}{2} \left[ e^{-\left(\frac{1+k_1}{2\mu}\right)^2} - e^{-\left(\frac{k_1}{2\mu}\right)^2} \right] \quad (32)$$

so that we have

$$\int_{k=\frac{k_1}{2\mu}}^{\frac{1+k_1}{2\mu}} k^i e^{-k^2} dk = - \sum_{l_i=0}^{\frac{i-1}{2}-1} \frac{1}{2^{l_i+1}} \frac{(i-1)!!}{(i-1-2l_i)!!} \left[ \left( \frac{1+k_1}{2\mu} \right)^{i-1-2l_i} e^{-\left(\frac{1+k_1}{2\mu}\right)^2} - \left( \frac{k_1}{2\mu} \right)^{i-1-2l_i} e^{-\left(\frac{k_1}{2\mu}\right)^2} \right] + \frac{(i-1)!!}{2^{\frac{i-1}{2}}} \frac{-1}{2} \left[ e^{-\left(\frac{1+k_1}{2\mu}\right)^2} - e^{-\left(\frac{k_1}{2\mu}\right)^2} \right]. \quad (33)$$

## 2. Integration over $k_1$ in $I_2$

We calculate the remaining integral as the sum of two sums over two different indices,  $i_p$  and  $i_i$  with  $i = 2i_p$  if  $i$  is even and  $i = 2i_i + 1$  if  $i$  is odd, which both run between 0 and  $n$  so that we have indeed  $2 + 2n$  terms

$$\begin{aligned} I_2 &= \sum_{i=0}^{1+2n} \binom{1+2n}{i} (-1)^{1-i} (2\mu)^{1+i} \int_{k_1=0}^1 k_1^{2+2(m+n)-i} \left( \int_{k=\frac{k_1}{2\mu}}^{\frac{1+k_1}{2\mu}} k^i e^{-k^2} dk \right) dk_1 \\ &= - \sum_{i_p=0}^n \binom{1+2n}{2i_p} (2\mu)^{1+2i_p} \int_{k_1=0}^1 k_1^{2+2(m+n)-2i_p} \left( \frac{(2i_p-1)!!}{2^{i_p}} \frac{\sqrt{\pi}}{2} \left[ \operatorname{erf}\left(\frac{1+k_1}{2\mu}\right) - \operatorname{erf}\left(\frac{k_1}{2\mu}\right) \right] \right. \\ &\quad \left. - \sum_{l_p=0}^{i_p-1} \frac{1}{2^{l_p+1}} \frac{(2i_p-1)!!}{(2i_p-1-2l_p)!!} \frac{1}{(2\mu)^{2i_p-1-2l_p}} \left[ (1+k_1)^{2i_p-1-2l_p} e^{-\left(\frac{1+k_1}{2\mu}\right)^2} - k_1^{2i_p-1-2l_p} e^{-\left(\frac{k_1}{2\mu}\right)^2} \right] \right) dk_1 \\ &\quad + \sum_{i_i=0}^n \binom{1+2n}{2i_i+1} (2\mu)^{2+2i_i} \int_{k_1=0}^1 k_1^{1+2(m+n)-2i_i} \left( \frac{(2i_i)!!}{2^{i_i}} \frac{-1}{2} \left[ e^{-\left(\frac{1+k_1}{2\mu}\right)^2} - e^{-\left(\frac{k_1}{2\mu}\right)^2} \right] \right. \\ &\quad \left. - \sum_{l_i=0}^{i_i-1} \frac{1}{2^{l_i+1}} \frac{(2i_i)!!}{(2i_i-2l_i)!!} \frac{1}{(2\mu)^{2i_i-2l_i}} \left[ (1+k_1)^{2i_i-2l_i} e^{-\left(\frac{1+k_1}{2\mu}\right)^2} - k_1^{2i_i-2l_i} e^{-\left(\frac{k_1}{2\mu}\right)^2} \right] \right) dk_1 \quad (34) \end{aligned}$$

### a. Sum over $i_p$

There are four sub-integrals in the sum over  $i_p$ .

### First sub-integral

$$\begin{aligned} & - \frac{\sqrt{\pi}}{2} \int_{k_1=0}^1 k_1^{2+2(m+n-i_p)} \operatorname{erf}\left(\frac{k_1}{2\mu}\right) dk_1 \\ &= - \int_{k_1=0}^1 k_1^{2+2(m+n-i_p)} \int_{t=0}^{\frac{k_1}{2\mu}} e^{-t^2} dt dk_1 \\ &= - \int_{k_1=0}^1 k_1^{2+2(m+n-i_p)} \int_{k=0}^{k_1} e^{-\left(\frac{k}{2\mu}\right)^2} \frac{1}{2\mu} dk dk_1 \\ &= \frac{1}{3+2(m+n-i_p)} \left( - \frac{\sqrt{\pi}}{2} \operatorname{erf}\left(\frac{1}{2\mu}\right) + \frac{1}{2\mu} \int_{k_1=0}^1 k_1^{2+2(m+n-i_p)} k_1 e^{-\left(\frac{k_1}{2\mu}\right)^2} dk_1 \right) \\ &= \frac{1}{3+2(m+n-i_p)} \left( - \frac{\sqrt{\pi}}{2} \operatorname{erf}\left(\frac{1}{2\mu}\right) + \frac{1}{2\mu} \left( (2\mu^2)^{1+m+n-i_p} (2+2(m+n-i_p))!! (-2\mu^2) \left[ e^{-\left(\frac{1}{2\mu}\right)^2} - 1 \right] \right. \right. \\ &\quad \left. \left. - \sum_{\lambda_i=0}^{m+n-i_p} (2\mu^2)^{\lambda_i+1} \frac{(2+2(m+n-i_p))!!}{(2+2(m+n-i_p)-2\lambda_i)!!} e^{-\left(\frac{1}{2\mu}\right)^2} \right) \right) \\ &= \frac{1}{3+2(m+n-i_p)} \left( - \frac{\sqrt{\pi}}{2} \operatorname{erf}\left(\frac{1}{2\mu}\right) + \frac{1}{2\mu} S_i[1+m+n-i_p] \right) \quad (35) \end{aligned}$$

where we used first the change of variable  $t = \frac{k}{2\mu}$ , then an integration by parts with

$$\frac{d}{dk_1} \frac{\sqrt{\pi}}{2} \operatorname{erf}\left(\frac{k_1}{2\mu}\right) = \frac{d}{dk_1} \int_{k=0}^{k_1} e^{-\left(\frac{k}{2\mu}\right)^2} \frac{1}{2\mu} dk = \frac{e^{-\left(\frac{k_1}{2\mu}\right)^2}}{2\mu} \text{ and } \int^{k_1} x^{2+2(m+n-i_p)} dx = \frac{k_1^{3+2(m+n-i_p)}}{3+2(m+n-i_p)}, \quad (36)$$

to get rid of the error function. We then used repeated integrations by parts with the first step being

$$\frac{d}{dk} k^{2+2(m+n-i_p)} = (2+2(m+n-i_p))k^{1+2(m+n-i_p)} \text{ and } \int^{k_1} x e^{-\left(\frac{x}{2\mu}\right)^2} dx = -2\mu^2 e^{-\left(\frac{k_1}{2\mu}\right)^2} \quad (37)$$

and the final step is

$$\int_{k_1=0}^1 k_1 e^{-\left(\frac{k_1}{2\mu}\right)^2} dk_1 = (-2\mu^2) \left[ e^{-\left(\frac{1}{2\mu}\right)^2} - 1 \right]. \quad (38)$$

We also define a convenient notation for the result of the repeated integrations by parts over  $k_1$  as

$$\int_{k_1=0}^1 k_1^{2N} e^{-\left(\frac{k_1}{2\mu}\right)^2} dk_1 = S_p[N] \text{ and } \int_{k_1=0}^1 k_1^{2N+1} e^{-\left(\frac{k_1}{2\mu}\right)^2} dk_1 = S_i[N]. \quad (39)$$

### Second sub-integral

$$\begin{aligned} & \frac{\sqrt{\pi}}{2} \int_{k_1=0}^1 k_1^{2+2(m+n-i_p)} \operatorname{erf}\left(\frac{1+k_1}{2\mu}\right) dk_1 \\ &= \int_{k_1=0}^1 k_1^{2+2(m+n-i_p)} \int_{t=0}^{\frac{1+k_1}{2\mu}} e^{-t^2} dt dk_1 \\ &= \int_{k_1=0}^1 k_1^{2+2(m+n-i_p)} \int_{k=0}^{k_1} e^{-\left(\frac{1+k}{2\mu}\right)^2} \frac{1}{2\mu} dk dk_1 \\ &= \frac{1}{3+2(m+n-i_p)} \left( \frac{\sqrt{\pi}}{2} \operatorname{erf}\left(\frac{1}{\mu}\right) - \frac{1}{2\mu} \int_{k_1=0}^1 k_1^{3+2(m+n-i_p)} e^{-\left(\frac{1+k_1}{2\mu}\right)^2} dk_1 \right) \\ &= \frac{1}{3+2(m+n-i_p)} \left( \frac{\sqrt{\pi}}{2} \operatorname{erf}\left(\frac{1}{\mu}\right) - \frac{1}{2\mu} \sum_{j=0}^{3+2(m+n-i_p)} \binom{3+2(m+n-i_p)}{j} (-1)^{3-j} \int_{k_1=0}^1 (1+k_1)^j e^{-\left(\frac{1+k_1}{2\mu}\right)^2} dk_1 \right) \\ &= \frac{1}{3+2(m+n-i_p)} \left( \frac{\sqrt{\pi}}{2} \operatorname{erf}\left(\frac{1}{\mu}\right) + \frac{1}{2\mu} \sum_{j_p=0}^{1+m+n-i_p} \binom{3+2(m+n-i_p)}{2j_p} \left[ (2\mu^2)^{j_p} (2j_p-1)!! \frac{\sqrt{\pi}}{2} \left[ \operatorname{erf}\left(\frac{1}{\mu}\right) - \operatorname{erf}\left(\frac{1}{2\mu}\right) \right] \right. \right. \\ &\quad \left. \left. - \sum_{\lambda_p=0}^{j_p-1} [(2\mu^2)^{\lambda_p+1} \frac{(2j_p-1)!!}{(2j_p-1-2\lambda_p)!!} \left[ 2^{2j_p-1-2\lambda_p} e^{-\left(\frac{1}{\mu}\right)^2} - e^{-\left(\frac{1}{2\mu}\right)^2} \right] \right] \right. \right. \\ &\quad \left. \left. - \frac{1}{2\mu} \sum_{j_i=0}^{1+m+n-i_p} \binom{3+2(m+n-i_p)}{2j_i+1} \left[ (2\mu^2)^{j_i} (2j_i)!! (-2\mu^2) \left[ e^{-\left(\frac{1}{\mu}\right)^2} - e^{-\left(\frac{1}{2\mu}\right)^2} \right] \right. \right. \right. \\ &\quad \left. \left. \left. - \sum_{\lambda_i=0}^{j_i-1} [(2\mu^2)^{\lambda_i+1} \frac{(2j_i)!!}{(2j_i-2\lambda_i)!!} \left[ 2^{2j_i-2\lambda_i} e^{-\left(\frac{1}{\mu}\right)^2} - e^{-\left(\frac{1}{2\mu}\right)^2} \right] \right] \right] \right) \right) \\ &= \frac{1}{3+2(m+n-i_p)} \left( \frac{\sqrt{\pi}}{2} \operatorname{erf}\left(\frac{1}{\mu}\right) + \frac{1}{2\mu} \sum_{j_p=0}^{1+m+n-i_p} \binom{3+2(m+n-i_p)}{2j_p} S_p^+[j_p] - \frac{1}{2\mu} \sum_{j_i=0}^{1+m+n-i_p} \binom{3+2(m+n-i_p)}{2j_i+1} S_i^+[j_i] \right) \end{aligned} \quad (40)$$

where we used the binomial expansion

$$k_1^{3+2(m+n-i_p)} = \sum_{j=0}^{3+2(m+n-i_p)} \binom{3+2(m+n-i_p)}{j} (-1)^{3-j} (1+k_1)^j \quad (41)$$

and split the sum over  $j$  into two sums over  $j_p$  and  $j_i$ . We also introduced the definitions

$$\int_{k_1=0}^1 (1+k_1)^{2N} e^{-\left(\frac{1+k_1}{2\mu}\right)^2} dk_1 = S_p^+[N] \quad \text{and} \quad \int_{k_1=0}^1 (1+k_1)^{2N+1} e^{-\left(\frac{1+k_1}{2\mu}\right)^2} dk_1 = S_i^+[N]. \quad (42)$$

### Third sub-integral

$$- \int_{k_1=0}^1 k_1^{1+2(m+n-l_p)} e^{-\left(\frac{k_1}{2\mu}\right)^2} dk_1 = -S_i[m+n-l_p] \quad (43)$$

### Fourth sub-integral

$$\begin{aligned} & \int_{k_1=0}^1 k_1^{2+2(m+n-i_p)} (1+k_1)^{2i_p-1-2l_p} e^{-\left(\frac{1+k_1}{2\mu}\right)^2} dk_1 \\ &= \sum_{j=0}^{2+2(m+n-i_p)} \binom{2+2(m+n-i_p)}{j} (-1)^j \int_{k_1=0}^1 (1+k_1)^{j+2(i_p-l_p)-1} e^{-\left(\frac{1+k_1}{2\mu}\right)^2} dk_1 \\ &= \sum_{j_p=0}^{1+m+n-i_p} \binom{2+2(m+n-i_p)}{2j_p} \int_{k_1=0}^1 (1+k_1)^{2(j_p+i_p-l_p)-1} e^{-\left(\frac{1+k_1}{2\mu}\right)^2} dk_1 - \sum_{j_i=0}^{m+n-i_p} \binom{2+2(m+n-i_p)}{2j_i+1} \int_{k_1=0}^1 (1+k_1)^{2(j_i+i_p-l_p)} e^{-\left(\frac{1+k_1}{2\mu}\right)^2} dk_1 \\ &= \sum_{j_p=0}^{1+m+n-i_p} \binom{2+2(m+n-i_p)}{2j_p} S_i^+[j_p+i_p-l_p-1] - \sum_{j_i=0}^{m+n-i_p} \binom{2+2(m+n-i_p)}{2j_i+1} S_p^+[j_i+i_p-l_p] \end{aligned} \quad (44)$$

### b. Sum over $i_i$

There are also four sub-integrals in the sum over  $i_i$ .

### First sub-integral

$$- \int_{k_1=0}^1 k_1^{1+2(m+n-i_i)} e^{-\left(\frac{k_1}{2\mu}\right)^2} dk_1 = -S_i[m+n+i_i] \quad (45)$$

### Second sub-integral

$$\begin{aligned} \int_{k_1=0}^1 k_1^{1+2(m+n-i_i)} e^{-\left(\frac{1+k_1}{2\mu}\right)^2} dk_1 &= \sum_{j=0}^{1+2(m+n-i_i)} \binom{1+2(m+n-i_i)}{j} (-1)^{1-j} \int_{k_1=0}^1 (1+k_1)^j e^{-\left(\frac{1+k_1}{2\mu}\right)^2} dk_1 \\ &= - \sum_{j_p=0}^{m+n-i_i} \binom{1+2(m+n-i_i)}{2j_p} S_p^+[j_p] + \sum_{j_i=0}^{m+n-i_i} \binom{1+2(m+n-i_i)}{2j_i+1} S_i^+[j_i] \end{aligned} \quad (46)$$

### Third sub-integral

$$- \int_{k_1=0}^1 k_1^{1+2(m+n-l_i)} e^{-\left(\frac{k_1}{2\mu}\right)^2} dk_1 = -S_i[m+n-l_i] \quad (47)$$

### Fourth sub-integral

$$\begin{aligned}
& \int_{k_1=0}^1 k_1^{1+2(m+n-i_i)} (1+k_1)^{2(i_i-l_i)} e^{-\left(\frac{1+k_1}{2\mu}\right)^2} dk_1 \\
&= \sum_{j=0}^{1+2(m+n-i_i)} \binom{1+2(m+n-i_i)}{j} (-1)^{1-j} \int_{k_1=0}^1 (1+k_1)^j e^{-\left(\frac{1+k_1}{2\mu}\right)^2} dk_1 \\
&= - \sum_{j_p=0}^{m+n-i_i} \binom{1+2(m+n-i_i)}{2j_p} S_p^+[j_p+i_i-l_i] + \sum_{j_i=0}^{m+n-i_i} \binom{1+2(m+n-i_i)}{2j_i+1} S_i^+[j_i+i_i-l_i]
\end{aligned} \tag{48}$$

### 3. Expression of integral $I_2$

We have found each sub-integral of the second integral  $I_2$  of the first part of the exchange energy. The expression of  $I_2$  is thus

$$\begin{aligned}
I_2 &= \int_{k_1=0}^1 \int_{k_2=0}^1 k_1^{1+2m} k_2^{1+2n} e^{-\left(\frac{k_1+k_2}{2\mu}\right)^2} dk_2 dk_1 \\
&= - \sum_{i_p=0}^n \binom{1+2n}{2i_p} (2\mu)^{1+2i_p} \left\{ \frac{(2i_p-1)!!}{2^{i_p}} \frac{1}{3+2(m+n-i_p)} \left( \frac{\sqrt{\pi}}{2} \left[ \operatorname{erf}\left(\frac{1}{\mu}\right) - \operatorname{erf}\left(\frac{1}{2\mu}\right) \right] \right) \right. \\
&\quad + \frac{1}{2\mu} \left[ S_i[1+m+n-i_p] + \sum_{j_p=0}^{1+m+n-i_p} \binom{3+2(m+n-i_p)}{2j_p} S_p^+[j_p] - \sum_{j_i=0}^{1+m+n-i_p} \binom{3+2(m+n-i_p)}{2j_i+1} S_i^+[j_i] \right] \\
&\quad - \sum_{l_p=0}^{i_p-1} \frac{1}{2^{l_p+1}} \frac{(2i_p-1)!!}{(2i_p-1-2l_p)!!} \frac{1}{(2\mu)^{2i_p-1-2l_p}} \left( -S_i[m+n-l_p] \right. \\
&\quad \left. + \sum_{j_p=0}^{1+m+n-i_p} \binom{2+2(m+n-i_p)}{2j_p} S_i^+[j_p+i_p-l_p-1] - \sum_{j_i=0}^{m+n-i_p} \binom{2+2(m+n-i_p)}{2j_i+1} S_p^+[j_i+i_p-l_p] \right) \Big\} \\
&\quad + \sum_{i_i=0}^n \binom{1+2n}{2i_i+1} (2\mu)^{2+2i_i} \left\{ \frac{(2i_i)!!}{2^{i_i}} \frac{-1}{2} \left( -S_i[m+n-i_i] \right. \right. \\
&\quad \left. - \sum_{j_p=0}^{m+n-i_i} \binom{1+2(m+n-i_i)}{2j_p} S_p^+[j_p] + \sum_{j_i=0}^{m+n-i_i} \binom{1+2(m+n-i_i)}{2j_i+1} S_i^+[j_i] \right) \\
&\quad - \sum_{l_i=0}^{i_i-1} \frac{1}{2^{l_i+1}} \frac{(2i_i)!!}{(2i_i-2l_i)!!} \frac{1}{(2\mu)^{2i_i-2l_i}} \left( -S_i[m+n-l_i] \right. \\
&\quad \left. + \sum_{j_p=0}^{m+n-i_i} \binom{1+2(m+n-i_p)}{2j_p} S_p^+[j_p+i_i-l_i] - \sum_{j_i=0}^{m+n-i_i} \binom{1+2(m+n-i_i)}{2j_i+1} S_i^+[j_i+i_i-l_i] \right) \Big\}.
\end{aligned} \tag{49}$$

Most of the following calculations use exactly the same steps. They are written now with less details.

### C. Third integral of the first part ( $I_3$ )

$$I_3 = \int_{k_1=0}^1 \int_{k_2=0}^1 k_1^{1+2m} k_2^{1+2n} e^{-\left(\frac{k_1+k_2}{2\mu}\right)^2} dk_2 dk_1 = \sum_{i=0}^{1+2n} \binom{1+2n}{i} (-1)^{1+i} (2\mu)^{1+i} \int_{k_1=0}^1 k_1^{2+2(m+n-i)} \left( \int_{k=\frac{k_1}{2\mu}}^{\frac{k_1-1}{2\mu}} k^i e^{-k^2} dk \right) dk_1. \tag{50}$$

where we used the change of variable  $k_2 = 2\mu k + k_1$ .

### 1. Integration over $k$ in $I_3$

Once again, we can calculate the integral over  $k$  with repeated integrations by parts, with two different cases depending on the parity of  $i$ . If  $i$  is even we have

$$\begin{aligned} & \int_{k=\frac{k_1}{2\mu}}^{\frac{k_1-1}{2\mu}} k^i e^{-k^2} dk \\ &= - \sum_{l_p=0}^{\frac{i}{2}-1} \frac{1}{2^{l_p+1}} \frac{(i-1)!!}{(i-1-2l_p)!!} \left[ \left( \frac{k_1-1}{2\mu} \right)^{i-1-2l_p} e^{-\left( \frac{k_1-1}{2\mu} \right)^2} - \left( \frac{k_1}{2\mu} \right)^{i-1-2l_p} e^{-\left( \frac{k_1}{2\mu} \right)^2} \right] + \frac{(i-1)!!}{2^{\frac{i}{2}}} \frac{\sqrt{\pi}}{2} \left[ \operatorname{erf}\left( \frac{k_1-1}{2\mu} \right) - \operatorname{erf}\left( \frac{k_1}{2\mu} \right) \right], \quad (51) \end{aligned}$$

while if  $i$  is odd we have

$$\begin{aligned} & \int_{k=\frac{k_1}{2\mu}}^{\frac{k_1+1}{2\mu}} k^i e^{-k^2} dk \\ &= - \sum_{l_i=0}^{\frac{i-1}{2}-1} \frac{1}{2^{l_i+1}} \frac{(i-1)!!}{(i-1-2l_i)!!} \left[ \left( \frac{k_1-1}{2\mu} \right)^{i-1-2l_i} e^{-\left( \frac{k_1-1}{2\mu} \right)^2} - \left( \frac{k_1}{2\mu} \right)^{i-1-2l_i} e^{-\left( \frac{k_1}{2\mu} \right)^2} \right] + \frac{(i-1)!!}{2^{\frac{i-1}{2}}} \frac{-1}{2} \left[ e^{-\left( \frac{k_1-1}{2\mu} \right)^2} - e^{-\left( \frac{k_1}{2\mu} \right)^2} \right]. \quad (52) \end{aligned}$$

### 2. Integration over $k_1$ in $I_3$

We write the integral  $I_3$  as the sum of two sums over two indices,  $i_p$  and  $i_i$  with  $i = 2i_p$  if  $i$  is even and  $i = 2i_i + 1$  if  $i$  is odd, which both run between 0 and  $n$  so that we have indeed  $2 + 2n$  terms. We have

$$\begin{aligned} I_3 &= \sum_{i=0}^{1+2n} \binom{1+2n}{i} (-1)^{1+i} (2\mu)^{1+i} \int_{k_1=0}^1 k_1^{2+2(m+n)-i} \left( \int_{k=\frac{k_1}{2\mu}}^{\frac{k_1-1}{2\mu}} k^i e^{-k^2} dk \right) dk_1 \\ &= - \sum_{i_p=0}^n \binom{1+2n}{2i_p} (2\mu)^{1+2i_p} \int_{k_1=0}^1 k_1^{2+2(m+n)-2i_p} \left( \frac{(2i_p-1)!!}{2^{i_p}} \frac{\sqrt{\pi}}{2} \left[ \operatorname{erf}\left( \frac{k_1-1}{2\mu} \right) - \operatorname{erf}\left( \frac{k_1}{2\mu} \right) \right] \right. \\ &\quad \left. - \sum_{l_p=0}^{i_p-1} \frac{1}{2^{l_p+1}} \frac{(2i_p-1)!!}{(2i_p-1-2l_p)!!} \frac{1}{(2\mu)^{2i_p-1-2l_p}} \left[ (k_1-1)^{2i_p-1-2l_p} e^{-\left( \frac{k_1-1}{2\mu} \right)^2} - k_1^{2i_p-1-2l_p} e^{-\left( \frac{k_1}{2\mu} \right)^2} \right] \right) dk_1 \\ &\quad + \sum_{i_i=0}^n \binom{1+2n}{2i_i+1} (2\mu)^{2+2i_i} \int_{k_1=0}^1 k_1^{1+2(m+n)-2i_i} \left( \frac{(2i_i)!!}{2^{i_i}} \frac{-1}{2} \left[ e^{-\left( \frac{k_1-1}{2\mu} \right)^2} - e^{-\left( \frac{k_1}{2\mu} \right)^2} \right] \right. \\ &\quad \left. - \sum_{l_i=0}^{i_i-1} \frac{1}{2^{l_i+1}} \frac{(2i_i)!!}{(2i_i-2l_i)!!} \frac{1}{(2\mu)^{2i_i-2l_i}} \left[ (k_1-1)^{2i_i-2l_i} e^{-\left( \frac{k_1-1}{2\mu} \right)^2} - k_1^{2i_i-2l_i} e^{-\left( \frac{k_1}{2\mu} \right)^2} \right] \right) dk_1. \quad (53) \end{aligned}$$

#### a. Sum over $i_p$

There are four sub-integrals in the sum over  $i_p$ .

#### First sub-integral

$$-\frac{\sqrt{\pi}}{2} \int_{k_1=0}^1 k_1^{2+2(m+n-i_p)} \operatorname{erf}\left( \frac{k_1}{2\mu} \right) dk_1 = \frac{1}{3+2(m+n-i_p)} \left( -\frac{\sqrt{\pi}}{2} \operatorname{erf}\left( \frac{1}{2\mu} \right) + \frac{1}{2\mu} S_i[1+m+n-i_p] \right) \quad (54)$$

#### Second sub-integral

$$\begin{aligned}
& \frac{\sqrt{\pi}}{2} \int_{k_1=0}^1 k_1^{2+2(m+n-i_p)} \operatorname{erf}\left(\frac{k_1-1}{2\mu}\right) dk_1 \\
&= \int_{k_1=0}^1 k_1^{2+2(m+n-i_p)} \int_{t=0}^{\frac{k_1-1}{2\mu}} e^{-t^2} dt dk_1 \\
&= \int_{k_1=0}^1 k_1^{2+2(m+n-i_p)} \int_{k=0}^{k_1} e^{-\left(\frac{k-1}{2\mu}\right)^2} \frac{1}{2\mu} dk dk_1 \\
&= \frac{1}{3+2(m+n-i_p)} \left( 0 - \frac{1}{2\mu} \int_{k_1=0}^1 k_1^{3+2(m+n-i_p)} e^{-\left(\frac{k_1-1}{2\mu}\right)^2} dk_1 \right) \\
&= \frac{1}{3+2(m+n-i_p)} \left( 0 - \frac{1}{2\mu} \sum_{j=0}^{3+2(m+n-i_p)} \binom{3+2(m+n-i_p)}{j} \int_{k_1=0}^1 (k_1-1)^j e^{-\left(\frac{k_1-1}{2\mu}\right)^2} dk_1 \right) \\
&= \frac{1}{3+2(m+n-i_p)} \frac{-1}{2\mu} \left( \sum_{j_p=0}^{1+m+n-i_p} \binom{3+2(m+n-i_p)}{2j_p} \left[ (2\mu^2)^{j_p} (2j_p-1)!! \frac{\sqrt{\pi}}{2} \left[ 0 - \operatorname{erf}\left(\frac{-1}{2\mu}\right) \right] \right. \right. \\
&\quad \left. \left. - \sum_{\lambda_p=0}^{j_p-1} [(2\mu^2)^{\lambda_p+1} \frac{(2j_p-1)!!}{(2j_p-1-2\lambda_p)!!} \left[ 0 - (-1)^{2j_p-1-2\lambda_p} e^{-\left(\frac{-1}{2\mu}\right)^2} \right] \right] \right. \right. \\
&\quad \left. \left. + \sum_{j_i=0}^{1+m+n-i_p} \binom{3+2(m+n-i_p)}{2j_i+1} \left[ (2\mu^2)^{j_i} (2j_i)!! (-2\mu^2) \left[ 1 - e^{-\left(\frac{-1}{2\mu}\right)^2} \right] \right. \right. \right. \\
&\quad \left. \left. \left. - \sum_{\lambda_i=0}^{j_i-1} [(2\mu^2)^{\lambda_i+1} \frac{(2j_i)!!}{(2j_i-2\lambda_i)!!} \left[ 0 - (-1)^{2j_i-2\lambda_i} e^{-\left(\frac{-1}{2\mu}\right)^2} \right] \right] \right] \right] \right) \\
&= \frac{1}{3+2(m+n-i_p)} \frac{-1}{2\mu} \left( \sum_{j_p=0}^{1+m+n-i_p} \binom{3+2(m+n-i_p)}{2j_p} S_p^-[j_p] + \sum_{j_i=0}^{1+m+n-i_p} \binom{3+2(m+n-i_p)}{2j_i+1} S_i^-[j_i] \right) \tag{55}
\end{aligned}$$

where we used the binomial expansion

$$k_1^{3+2(m+n-i_p)} = \sum_{j=0}^{3+2(m+n-i_p)} \binom{3+2(m+n-i_p)}{j} (k_1-1)^j \tag{56}$$

and split the sum over  $j$  into two sums over  $j_p$  and  $j_i$ . We also introduced the notations

$$\int_{k_1=0}^1 (k_1-1)^{2N} e^{-\left(\frac{k_1-1}{2\mu}\right)^2} dk_1 = S_p^-[N] \quad \text{and} \quad \int_{k_1=0}^1 (k_1-1)^{2N+1} e^{-\left(\frac{k_1-1}{2\mu}\right)^2} dk_1 = S_i^-[N]. \tag{57}$$

### Third sub-integral

$$- \int_{k_1=0}^1 k_1^{1+2(m+n-l_p)} e^{-\left(\frac{k_1}{2\mu}\right)^2} dk_1 = -S_i^-[m+n-l_p] \tag{58}$$

### Fourth sub-integral

$$\begin{aligned}
& \int_{k_1=0}^1 k_1^{2+2(m+n-i_p)} (k_1-1)^{2i_p-1-2l_p} e^{-\left(\frac{k_1-1}{2\mu}\right)^2} dk_1 \\
&= \sum_{j=0}^{2+2(m+n-i_p)} \binom{2+2(m+n-i_p)}{j} \int_{k_1=0}^1 (k_1-1)^{j+2(i_p-l_p)-1} e^{-\left(\frac{k_1-1}{2\mu}\right)^2} dk_1 \\
&= \sum_{j_p=0}^{1+m+n-i_p} \binom{2+2(m+n-i_p)}{2j_p} S_i^-[j_p+i_p-l_p-1] + \sum_{j_i=0}^{m+n-i_p} \binom{2+2(m+n-i_p)}{2j_i+1} S_p^-[j_i+i_p-l_p] \tag{59}
\end{aligned}$$

*b. Sum over  $i_i$*

There are four sub-integrals in the sum over  $i_i$ .

### First sub-integral

$$- \int_{k_1=0}^1 k_1^{1+2(m+n-i_i)} e^{-\left(\frac{k_1-1}{2\mu}\right)^2} dk_1 = -S_i[m+n+i_i] \quad (60)$$

### Second sub-integral

$$\begin{aligned} & \int_{k_1=0}^1 k_1^{1+2(m+n-i_i)} e^{-\left(\frac{k_1-1}{2\mu}\right)^2} dk_1 \\ &= \sum_{j=0}^{1+2(m+n-i_i)} \binom{1+2(m+n-i_i)}{j} \int_{k_1=0}^1 (k_1-1)^j e^{-\left(\frac{k_1-1}{2\mu}\right)^2} dk_1 \\ &= \sum_{j_p=0}^{m+n-i_i} \binom{1+2(m+n-i_i)}{2j_p} S_p^-[j_p] + \sum_{j_i=0}^{m+n-i_i} \binom{1+2(m+n-i_i)}{2j_i+1} S_i^-[j_i] \end{aligned} \quad (61)$$

### Third sub-integral

$$- \int_{k_1=0}^1 k_1^{1+2(m+n-l_i)} e^{-\left(\frac{k_1-1}{2\mu}\right)^2} dk_1 = -S_i[m+n-l_i] \quad (62)$$

### Fourth sub-integral

$$\begin{aligned} & \int_{k_1=0}^1 k_1^{1+2(m+n-i_i)} (k_1-1)^{2(i_i-l_i)} e^{-\left(\frac{k_1-1}{2\mu}\right)^2} dk_1 \\ &= \sum_{j=0}^{1+2(m+n-i_i)} \binom{1+2(m+n-i_i)}{j} \int_{k_1=0}^1 (k_1-1)^j e^{-\left(\frac{k_1-1}{2\mu}\right)^2} dk_1 \\ &= \sum_{j_p=0}^{m+n-i_i} \binom{1+2(m+n-i_i)}{2j_p} S_p^-[j_p+i_i-l_i] + \sum_{j_i=0}^{m+n-i_i} \binom{1+2(m+n-i_i)}{2j_i+1} S_i^-[j_i+i_i-l_i] \end{aligned} \quad (63)$$

### 3. Expression of integral $I_3$

We have found each sub-integral of the third integral  $I_3$  of the first part of the exchange energy. The expression of  $I_3$  is thus

$$\begin{aligned}
I_3 &= \int_{k_1=0}^1 \int_{k_2=0}^1 k_1^{1+2m} k_2^{1+2n} e^{-\left(\frac{k_1-k_2}{2\mu}\right)^2} dk_2 dk_1 \\
&= - \sum_{i_p=0}^n \binom{1+2n}{2i_p} (2\mu)^{1+2i_p} \left\{ \frac{(2i_p-1)!!}{2^{i_p}} \frac{1}{3+2(m+n-i_p)} \left( \frac{\sqrt{\pi}}{2} \left[ 0 - \operatorname{erf}\left(\frac{1}{2\mu}\right) \right] \right. \right. \\
&\quad + \frac{1}{2\mu} \left[ S_i[1+m+n-i_p] - \sum_{j_p=0}^{1+m+n-i_p} \binom{3+2(m+n-i_p)}{2j_p} S_p^-[j_p] - \sum_{j_i=0}^{1+m+n-i_p} \binom{3+2(m+n-i_p)}{2j_i+1} S_i^-[j_i] \right] \Big) \\
&\quad - \sum_{l_p=0}^{i_p-1} \frac{1}{2^{l_p+1}} \frac{(2i_p-1)!!}{(2i_p-1-2l_p)!!} \frac{1}{(2\mu)^{2i_p-1-2l_p}} \left( -S_i[m+n-l_p] \right. \\
&\quad \left. + \sum_{j_p=0}^{1+m+n-i_p} \binom{2+2(m+n-i_p)}{2j_p} S_i^-[j_p+i_p-l_p-1] + \sum_{j_i=0}^{m+n-i_p} \binom{2+2(m+n-i_p)}{2j_i+1} S_p^-[j_i+i_p-l_p] \right) \Big\} \\
&\quad + \sum_{i_i=0}^n \binom{1+2n}{2i_i+1} (2\mu)^{2+2i_i} \left\{ \frac{(2i_i)!!}{2^{i_i}} \frac{-1}{2} \left( -S_i[m+n-i_i] \right. \right. \\
&\quad + \sum_{j_p=0}^{m+n-i_i} \binom{1+2(m+n-i_i)}{2j_p} S_p^-[j_p] + \sum_{j_i=0}^{m+n-i_i} \binom{1+2(m+n-i_i)}{2j_i+1} S_i^-[j_i] \Big) \\
&\quad - \sum_{l_i=0}^{i_i-1} \frac{1}{2^{l_i+1}} \frac{(2i_i)!!}{(2i_i-2l_i)!!} \frac{1}{(2\mu)^{2i_i-2l_i}} \left( -S_i[m+n-l_i] \right. \\
&\quad \left. + \sum_{j_p=0}^{m+n-i_i} \binom{1+2(m+n-i_p)}{2j_p} S_p^-[j_p+i_i-l_i] + \sum_{j_i=0}^{m+n-i_i} \binom{1+2(m+n-i_i)}{2j_i+1} S_i^-[j_i+i_i-l_i] \right) \Big\}. \tag{64}
\end{aligned}$$

This expression has to be subtracted from the one of the second integral  $I_2$ , many terms in fact cancel each other.

## II. SECOND PART OF THE EXCHANGE ENERGY ( $II$ )

$$II = \int_{k_1=0}^1 \int_{k_2=0}^1 k_1^{1+2m} k_2^{1+2n} \left[ \operatorname{Ei}\left(-\left(\frac{k_1+k_2}{2\mu}\right)^2\right) - \operatorname{Ei}\left(-\left(\frac{k_1-k_2}{2\mu}\right)^2\right) + \ln((k_1-k_2)^2) - \ln((k_1+k_2)^2) \right] dk_2 dk_1 \tag{65}$$

### A. First integral of the second part ( $II_1$ )

$$II_1 = \int_{k_1=0}^1 \int_{k_2=0}^1 k_1^{1+2m} k_2^{1+2n} \ln((k_1+k_2)^2) dk_2 dk_1 = \sum_{i=0}^{1+2n} \binom{1+2n}{i} (-1)^{1-i} \int_{k_1=0}^1 k_1^{1+2(m+n)-i} \left( \int_{k=k_1}^{1+k_1} k^i 2 \ln(k) dk \right) dk_1 \tag{66}$$

where we used the change of variable  $k_2 = k - k_1$ .

1. Integration over  $k$  in  $II_1$

$$\int_{k=k_1}^{1+k_1} k^i 2 \ln(k) dk = 2 \frac{1}{(1+i)^2} \left( k_1^{1+i} - (1+k_1)^{1+i} - (1+i)k_1^{1+i} \ln(k_1) + (1+i)(1+k_1)^{1+i} \ln(1+k_1) \right) \quad (67)$$

2. Integration over  $k_1$  in  $II_1$

$$\begin{aligned} II_1 &= \sum_{i=0}^{1+2n} \binom{1+2n}{i} (-1)^{1-i} \int_{k_1=0}^1 k_1^{1+2(m+n)-i} \left( \int_{k=k_1}^{1+k_1} k^i 2 \ln(k) dk \right) dk_1 \\ &= \sum_{i=0}^{1+2n} \binom{1+2n}{i} \frac{2(-1)^{1-i}}{(1+i)^2} \int_{k_1=0}^1 k_1^{1+2(m+n)-i} \left( k_1^{1+i} - (1+k_1)^{1+i} - (1+i)k_1^{1+i} \ln(k_1) + (1+i)(1+k_1)^{1+i} \ln(1+k_1) \right) dk_1, \end{aligned} \quad (68)$$

which we will integrate term by term over  $k_1$ .

**First sub-integral**

$$\int_{k_1=0}^1 k_1^{2+2(m+n)+1} dk_1 = \frac{1}{4+2(m+n)} \quad (69)$$

**Second sub-integral**

$$\begin{aligned} - \int_{k_1=0}^1 k_1^{2+2(m+n)-i} (1+k_1)^{i+1} dk_1 &= - \sum_{j=0}^{1+i} \binom{1+i}{j} \int_{k_1=0}^1 k_1^{2+2(m+n)-i+j} dk_1 \\ &= - \sum_{j=0}^{1+i} \binom{1+i}{j} \frac{1}{3+2(m+n)-i+j} \end{aligned} \quad (70)$$

**Third sub-integral**

$$-(1+i) \int_{k_1=0}^1 k_1^{2+2(m+n)+1} \ln(k_1) dk_1 = (1+i) \frac{1}{4(2+m+n)^2} \quad (71)$$

**Fourth sub-integral**

$$\begin{aligned} &(1+i) \int_{k_1=0}^1 k_1^{2+2(m+n)-i} (1+k_1)^{i+1} \ln(1+k_1) dk_1 \\ &= (1+i) \sum_{j=0}^{2+2(m+n)-i} \binom{2+2(m+n)-i}{j} (-1)^{-i-j} \int_{k_1=0}^1 (1+k_1)^{1+i+j} \ln(1+k_1) dk_1 \\ &= (1+i) \sum_{j=0}^{2+2(m+n)-i} \binom{2+2(m+n)-i}{j} \frac{(-1)^{-i-j}}{(2+i+j)^2} \left( 1 + 2^{2+i+j} (-1 + (i+j) \ln(2) + \ln(4)) \right) \end{aligned} \quad (72)$$

where we used the binomial relation in Eq. (41).

### 3. Expression of integral $II_1$

We have found each sub-integral of the first integral  $II_1$  of the second part of the exchange energy. The expression of  $II_1$  is thus

$$\begin{aligned}
 II_1 &= \int_{k_1=0}^1 \int_{k_2=0}^1 k_1^{1+2m} k_2^{1+2n} \ln((k_1 + k_2)^2) dk_2 dk_1 \\
 &= \sum_{i=0}^{1+2n} \binom{1+2n}{i} \frac{2(-1)^{1-i}}{(1+i)^2} \left\{ \frac{1}{4+2(m+n)} - \sum_{j=0}^{1+i} \binom{1+i}{j} \frac{1}{3+2(m+n)-i+j} + (1+i) \frac{1}{4(2+m+n)^2} \right. \\
 &\quad \left. + (1+i) \sum_{j=0}^{2+2(m+n)-i} \binom{2+2(m+n)-i}{j} \frac{(-1)^{-i-j}}{(2+i+j)^2} \left( 1 + 2^{2+i+j} (-1 + (i+j) \ln(2) + \ln(4)) \right) \right\}. \quad (73)
 \end{aligned}$$

### B. Second integral of the second part ( $II_2$ )

$$II_2 = \int_{k_1=0}^1 \int_{k_2=0}^1 k_1^{1+2m} k_2^{1+2n} \ln((k_1 - k_2)^2) dk_2 dk_1 = \sum_{i=0}^{1+2n} \binom{1+2n}{i} (-1)^{1+i} \int_{k_1=0}^1 k_1^{1+2(m+n)-i} \left( \int_{k=k_1}^{k_1-1} k^i 2 \ln(k) dk \right) dk_1 \quad (74)$$

where we used the change of variable  $k_2 = k_1 - k$  and a binomial expansion.

#### 1. Integration over $k$ in $II_2$

$$\int_{k=k_1}^{k_1-1} k^i 2 \ln(k) dk_1 = 2 \frac{1}{(1+i)^2} \left( k_1^{1+i} - (k_1 - 1)^{1+i} - (1+i) k_1^{1+i} \ln(k_1) + (1+i)(k_1 - 1)^{1+i} \ln(k_1 - 1) \right) \quad (75)$$

#### 2. Integration over $k_1$ in $II_2$

$$\begin{aligned}
 II_2 &= \sum_{i=0}^{1+2n} \binom{1+2n}{i} (-1)^{1+i} \int_{k_1=0}^1 k_1^{1+2(m+n)-i} \left( \int_{k=k_1}^{k_1-1} k^i 2 \ln(k) dk \right) dk_1 \\
 &= \sum_{i=0}^{1+2n} \binom{1+2n}{i} \frac{2(-1)^{1-i}}{(1+i)^2} \int_{k_1=0}^1 k_1^{1+2(m+n)-i} \left( k_1^{1+i} - (k_1 - 1)^{1+i} - (1+i) k_1^{1+i} \ln(k_1) + (1+i)(k_1 - 1)^{1+i} \ln(1 - k_1) \right) dk_1 \quad (76)
 \end{aligned}$$

which we integrate term by term over  $k_1$ .

#### First sub-integral

$$\int_{k_1=0}^1 k_1^{2+2(m+n)+1} dk_1 = \frac{1}{4+2(m+n)} \quad (77)$$

#### Second sub-integral

$$\begin{aligned}
 - \int_{k_1=0}^1 k_1^{2+2(m+n)-i} (k_1 - 1)^{i+1} dk_1 &= - \sum_{j=0}^{1+i} \binom{1+i}{j} (-1)^{1+i-j} \int_{k_1=0}^1 k_1^{2+2(m+n)-i+j} dk_1 \\
 &= - \sum_{j=0}^{1+i} \binom{1+i}{j} (-1)^{1+i-j} \frac{1}{3+2(m+n)-i+j} \quad (78)
 \end{aligned}$$

### Third sub-integral

$$-(1+i) \int_{k_1=0}^1 k_1^{2+2(m+n)+1} \ln(k_1) dk_1 = (1+i) \frac{1}{4(2+m+n)^2} \quad (79)$$

### Fourth sub-integral

$$\begin{aligned} (1+i) \int_{k_1=0}^1 k_1^{2+2(m+n)-i} (k_1-1)^{i+1} \ln(1-k_1) dk_1 &= (1+i) \sum_{j=0}^{2+2(m+n)-i} \binom{2+2(m+n)-i}{j} \int_{k_1=0}^1 (k_1-1)^{1+i+j} \ln(1-k_1) dk_1 \\ &= (1+i) \sum_{j=0}^{2+2(m+n)-i} \binom{2+2(m+n)-i}{j} \frac{(-1)^{i+j}}{(2+i+j)^2} \end{aligned} \quad (80)$$

where we used the binomial relation in Eq. (56).

### 3. Expression of integral $II_2$

We have found each sub-integral of the second integral  $II_2$  of the second part of the exchange energy. The expression of  $II_2$  is thus

$$\begin{aligned} II_2 &= \int_{k_1=0}^1 \int_{k_2=0}^1 k_1^{1+2m} k_2^{1+2n} \ln((k_1-k_2)^2) dk_2 dk_1 \\ &= \sum_{i=0}^{1+2n} \binom{1+2n}{i} \frac{2(-1)^{1-i}}{(1+i)^2} \left\{ \frac{1}{4+2(m+n)} - \sum_{j=0}^{1+i} \binom{1+i}{j} (-1)^{1+i-j} \frac{1}{3+2(m+n)-i+j} \right. \\ &\quad \left. + (1+i) \frac{1}{4(2+m+n)^2} + (1+i) \sum_{j=0}^{2+2(m+n)-i} \binom{2+2(m+n)-i}{j} \frac{(-1)^{i+j}}{(2+i+j)^2} \right\}. \end{aligned} \quad (81)$$

### C. Third integral of the second part ( $II_3$ )

$$\begin{aligned} II_3 &= \int_{k_1=0}^1 \int_{k_2=0}^1 k_1^{1+2m} k_2^{1+2n} \text{Ei}\left(-\left(\frac{k_1+k_2}{2\mu}\right)^2\right) dk_1 dk_2 \\ &= \int_{k_1=0}^1 \int_{k_2=0}^1 k_1^{1+2m} k_2^{1+2n} \left( - \int_{\left(\frac{k_1+k_2}{2\mu}\right)^2}^{\infty} \frac{e^{-t}}{t} dt \right) dk_1 dk_2 \\ &= \sum_{i=0}^{1+2n} \binom{1+2n}{i} (-1)^{1-i} (2\mu)^{1+i} \int_{k_1=0}^1 k_1^{2+2(m+n)-i} \left( \int_{k=\frac{k_1}{2\mu}}^{\frac{1+k_1}{2\mu}} k^i \left( - \int_{k^2}^{\infty} \frac{e^{-t}}{t} dt \right) dk \right) dk_1 \end{aligned} \quad (82)$$

where we used the change of variable  $k_2 = 2\mu k - k_1$ .

#### 1. Integration over $k$ in $II_3$

We calculate the integral over  $k$  with an integration by parts using

$$\frac{d}{dk} \text{Ei}(-k^2) = \frac{2e^{-k^2}}{k} \quad \text{and} \quad \int^k x^i dx = \frac{k^{i+1}}{i+1} \quad (83)$$

so that we have

$$\int_{k=\frac{k_1}{2\mu}}^{\frac{1+k_1}{2\mu}} k^i \left( - \int_{k^2}^{\infty} \frac{e^{-t}}{t} dt \right) dk = \frac{1}{i+1} \frac{1}{(2\mu)^{i+1}} \left[ (1+k_1)^{i+1} \text{Ei} \left( - \left( \frac{1+k_1}{2\mu} \right)^2 \right) - (k_1)^{i+1} \text{Ei} \left( - \left( \frac{k_1}{2\mu} \right)^2 \right) \right] - \frac{2}{i+1} \int_{k=\frac{k_1}{2\mu}}^{\frac{1+k_1}{2\mu}} k^i e^{-k^2} dk. \quad (84)$$

We can observe that the integral over  $k$  is now exactly the integral that has been calculated for the second integral of the first part of the exchange energy but for a  $-2/(1+i)$  factor. We introduce the notation

$$\binom{1+2n}{i} (-1)^{1-i} (2\mu)^{1+i} \int_{k_1=0}^1 k_1^{2+2(m+n)-i} \int_{k=\frac{k_1}{2\mu}}^{\frac{1+k_1}{2\mu}} k^i e^{-k^2} dk dk_1 = \{I_{2,i}\} \quad (85)$$

for the following calculations.

## 2. Integration over $k_1$ in $I_3$

We now can split the sum over  $i_p$  and  $i_i$

$$\begin{aligned} I_3 &= \sum_{i=0}^{1+2n} \binom{1+2n}{i} (-1)^{1-i} (2\mu)^{1+i} \int_{k_1=0}^1 k_1^{2+2(m+n)-i} \left( \int_{k=\frac{k_1}{2\mu}}^{\frac{1+k_1}{2\mu}} k^i \left( - \int_{k^2}^{\infty} \frac{e^{-t}}{t} dt \right) dk \right) dk_1 \\ &= \sum_{i_p=0}^n \left( \frac{-2}{2i_p+1} \{I_{2,2i_p}\} - \binom{1+2n}{2i_p} \int_{k_1=0}^1 \frac{k_1^{2+2(m+n)-2i_p}}{2i_p+1} \left[ (1+k_1)^{2i_p+1} \text{Ei} \left( - \left( \frac{1+k_1}{2\mu} \right)^2 \right) - (k_1)^{2i_p+1} \text{Ei} \left( - \left( \frac{k_1}{2\mu} \right)^2 \right) \right] dk_1 \right) \\ &\quad + \sum_{i_i=0}^n \left( \frac{-2}{2i_i+2} \{I_{2,2i_i+1}\} + \binom{1+2n}{2i_i+1} \int_{k_1=0}^1 \frac{k_1^{1+2(m+n)-2i_i}}{2i_i+2} \left[ (1+k_1)^{2i_i+2} \text{Ei} \left( - \left( \frac{1+k_1}{2\mu} \right)^2 \right) - (k_1)^{2i_i+2} \text{Ei} \left( - \left( \frac{k_1}{2\mu} \right)^2 \right) \right] dk_1 \right). \quad (86) \end{aligned}$$

### a. Sum over $i_p$

There are two sub-integrals in the sum over  $i_p$ .

#### First sub-integral

We calculate this integral over  $k_1$  with an integration by parts using

$$\frac{d}{dk} \text{Ei} \left( - \left( \frac{k_1}{2\mu} \right)^2 \right) = \frac{2 e^{-\left(\frac{k_1}{2\mu}\right)^2}}{k_1} \quad \text{and} \quad \int^k x^{3+2(m+n)} dx = \frac{k^{4+2(m+n)}}{4+2(m+n)} \quad (87)$$

so that we have

$$\begin{aligned} - \int_{k_1=0}^1 k_1^{2+2(m+n)+1} \text{Ei} \left( - \left( \frac{k_1}{2\mu} \right)^2 \right) dk_1 &= - \frac{\text{Ei} \left( - \left( \frac{1}{2\mu} \right)^2 \right)}{4+2(m+n)} + \frac{2}{4+2(m+n)} \int_{k_1=0}^1 k_1^{3+2(m+n)} e^{-\left(\frac{k_1}{2\mu}\right)^2} dk_1 \\ &= - \frac{\text{Ei} \left( - \left( \frac{1}{2\mu} \right)^2 \right)}{4+2(m+n)} + \frac{2}{4+2(m+n)} S_i[m+n+1]. \quad (88) \end{aligned}$$

#### Second sub-integral

$$\begin{aligned}
\int_{k_1=0}^1 k_1^{2+2(m+n-i_p)} (1+k_1)^{2i_p+1} \text{Ei}\left(-\left(\frac{1+k_1}{2\mu}\right)^2\right) dk_1 &= \sum_{j=0}^{2+2(m+n-i_p)} \binom{2+2(m+n-i_p)}{j} (-1)^{-j} \int_{k_1=0}^1 (1+k_1)^{j+2i_p+1} \text{Ei}\left(-\left(\frac{1+k_1}{2\mu}\right)^2\right) dk_1 \\
&= \sum_{j=0}^{2+2(m+n-i_p)} \binom{2+2(m+n-i_p)}{j} \frac{(-1)^{-j}}{j+2i_p+2} \left[ 2^{j+2i_p+2} \text{Ei}\left(-\left(\frac{1}{\mu}\right)^2\right) - \text{Ei}\left(-\left(\frac{1}{2\mu}\right)^2\right) \right] \\
&\quad - \sum_{j_p=0}^{1+m+n-i_p} \binom{2+2(m+n-i_p)}{2j_p} \frac{1}{2j_p+2i_p+2} S_i^+[j_p+i_p] \\
&\quad + \sum_{j_i=0}^{m+n-i_p} \binom{2+2(m+n-i_p)}{2j_i+1} \frac{1}{2j_i+2i_p+3} S_p^+[j_i+i_p+1] \tag{89}
\end{aligned}$$

where we used a binomial expansion, the same integration by parts as before, and then split the sum over  $j$ .

*b. Sum over  $i_i$*

There are two sub-integrals in the sum over  $i_i$ .

### First sub-integral

$$-\int_{k_1=0}^1 k_1^{2+2(m+n)+1} \text{Ei}\left(-\left(\frac{k_1}{2\mu}\right)^2\right) dk_1 = -\frac{\text{Ei}\left(-\left(\frac{1}{2\mu}\right)^2\right)}{4+2(m+n)} + \frac{2}{4+2(m+n)} S_i[m+n+1] \tag{90}$$

### Second sub-integral

$$\begin{aligned}
\int_{k_1=0}^1 k_1^{1+2(m+n-i_i)} (1+k_1)^{2i_i+2} \text{Ei}\left(-\left(\frac{1+k_1}{2\mu}\right)^2\right) dk_1 &= \sum_{j=0}^{1+2(m+n-i_i)} \binom{1+2(m+n-i_i)}{j} (-1)^{-j} \int_{k_1=0}^1 (1+k_1)^{j+2i_i+2} \text{Ei}\left(-\left(\frac{1+k_1}{2\mu}\right)^2\right) dk_1 \\
&= \sum_{j=0}^{1+2(m+n-i_i)} \binom{1+2(m+n-i_i)}{j} \frac{(-1)^{1-j}}{j+2i_i+3} \left[ 2^{j+2i_i+3} \text{Ei}\left(-\left(\frac{1}{\mu}\right)^2\right) - \text{Ei}\left(-\left(\frac{1}{2\mu}\right)^2\right) \right] \\
&\quad + \sum_{j_p=0}^{m+n-i_i} \binom{1+2(m+n-i_i)}{2j_p} \frac{1}{2j_p+2i_i+3} S_p^+[j_p+i_i+1] \\
&\quad - \sum_{j_i=0}^{m+n-i_i} \binom{1+2(m+n-i_i)}{2j_i+1} \frac{1}{2j_i+2i_i+4} S_i^+[j_i+i_i+1] \tag{91}
\end{aligned}$$

### 3. Expression of integral $II_3$

We have found each sub-integral of the third integral  $II_3$  of the second part of the exchange energy. The expression of  $II_3$  is thus

$$\begin{aligned}
II_3 &= \int_{k_1=0}^1 \int_{k_2=0}^1 k_1^{1+2m} k_2^{1+2n} \text{Ei} \left( - \left( \frac{k_1 + k_2}{2\mu} \right)^2 \right) dk_2 dk_1 \\
&= \sum_{i_p=0}^n \left\{ \frac{-2}{2i_p+1} \{I_{2,2i_p}\} - \frac{1}{2i_p+1} \left( \frac{1+2n}{2i_p} \right) \left[ - \frac{\text{Ei} \left( - \left( \frac{1}{2\mu} \right)^2 \right)}{4+2(m+n)} + \frac{2}{4+2(m+n)} S_i[m+n+1] \right. \right. \\
&\quad + \sum_{j=0}^{2+2(m+n-i_p)} \binom{2+2(m+n-i_p)}{j} \frac{(-1)^{-j}}{j+2i_p+2} \left[ 2^{j+2i_p+2} \text{Ei} \left( - \left( \frac{1}{\mu} \right)^2 \right) - \text{Ei} \left( - \left( \frac{1}{2\mu} \right)^2 \right) \right] \\
&\quad + \sum_{j_p=0}^{m+n-i_p+1} \binom{2+2(m+n-i_p)}{2j_p} \frac{1}{2j_p+2i_p+2} S_i^+[j_p+i_p] \\
&\quad \left. - \sum_{j_i=0}^{m+n-i_p} \binom{2+2(m+n-i_p)}{2j_i+1} \frac{1}{2j_i+2i_p+3} S_p^+[j_i+i_p+1] \right] \Big\} \\
&\quad + \sum_{i_i=0}^n \left\{ \frac{-2}{2i_i+2} \{I_{2,2i_i+1}\} - \frac{1}{2i_i+2} \left( \frac{1+2n}{2i_i+1} \right) \left[ - \frac{\text{Ei} \left( - \left( \frac{1}{2\mu} \right)^2 \right)}{4+2(m+n)} + \frac{2}{4+2(m+n)} S_i[m+n+1] \right. \right. \\
&\quad + \sum_{j=0}^{1+2(m+n-i_i)} \binom{1+2(m+n-i_i)}{j} \frac{(-1)^{1-j}}{j+2i_i+3} \left[ 2^{j+2i_i+3} \text{Ei} \left( - \left( \frac{1}{\mu} \right)^2 \right) - \text{Ei} \left( - \left( \frac{1}{2\mu} \right)^2 \right) \right] \\
&\quad + \sum_{j_p=0}^{m+n-i_i} \binom{1+2(m+n-i_i)}{2j_p} \frac{1}{2j_p+2i_i+3} S_p^+[j_p+i_i+1] \\
&\quad \left. - \sum_{j_i=0}^{m+n-i_i} \binom{1+2(m+n-i_i)}{2j_i+1} \frac{1}{2j_i+2i_i+4} S_i^+[j_i+i_i+1] \right] \Big\}. \tag{92}
\end{aligned}$$

### D. Fourth integral of the second part ( $II_4$ )

$$\begin{aligned}
II_4 &= \int_{k_1=0}^1 \int_{k_2=0}^1 k_1^{1+2m} k_2^{1+2n} \text{Ei} \left( - \left( \frac{k_1 - k_2}{2\mu} \right)^2 \right) dk_2 dk_1 = \int_{k_1=0}^1 \int_{k_2=0}^1 k_1^{1+2m} k_2^{1+2n} \left( - \int_{\left(\frac{k_1-k_2}{2\mu}\right)^2}^{\infty} \frac{e^{-t}}{t} dt \right) dk_2 dk_1 \\
&= \sum_{i=0}^{1+2n} \binom{1+2n}{i} (-1)^{1+i} (2\mu)^{1+i} \int_{k_1=0}^1 k_1^{2+2(m+n)-i} \left( \int_{k=\frac{k_1}{2\mu}}^{\frac{k_1-1}{2\mu}} k^i \left( - \int_{k^2}^{\infty} \frac{e^{-t}}{t} dt \right) dk \right) dk_1 \tag{93}
\end{aligned}$$

where we used the change of variable  $k_2 = -2\mu k + k_1$ .

#### 1. Integration over $k$ in $II_4$

We calculate the integral over  $k$  using the usual integration by parts

$$\int_{k=\frac{k_1}{2\mu}}^{\frac{k_1-1}{2\mu}} k^i \left( - \int_{k^2}^{\infty} \frac{e^{-t}}{t} dt \right) dk = \frac{1}{i+1} \frac{1}{(2\mu)^{i+1}} \left[ (k_1-1)^{i+1} \text{Ei} \left( - \left( \frac{k_1-1}{2\mu} \right)^2 \right) - (k_1)^{i+1} \text{Ei} \left( - \left( \frac{k_1}{2\mu} \right)^2 \right) \right] - \frac{2}{i+1} \int_{k=\frac{k_1}{2\mu}}^{\frac{k_1-1}{2\mu}} k^i e^{-k^2} dk. \tag{94}$$

We observe that the integral on  $k$  is now exactly the integral that has been calculated for the third integral of the first part of the exchange energy but for a  $-2/(1+i)$  factor. We introduce the notation

$$\binom{1+2n}{i} (-1)^{1-i} (2\mu)^{1+i} \int_{k_1=0}^1 k_1^{2+2(m+n)-i} \int_{k=\frac{k_1}{2\mu}}^{\frac{k_1-1}{2\mu}} k^i e^{-k^2} dk dk_1 = \{I_{3,i}\} \quad (95)$$

for the following calculations.

## 2. Integration over $k_1$ in $II_4$

We split the sum over  $i_p$  and  $i_i$

$$\begin{aligned} II_4 &= \sum_{i=0}^{1+2n} \binom{1+2n}{i} (-1)^{1+i} (2\mu)^{1+i} \int_{k_1=0}^1 k_1^{2+2(m+n)-i} \left( \int_{k=\frac{k_1}{2\mu}}^{\frac{k_1-1}{2\mu}} k^i \left( - \int_{k^2}^{\infty} \frac{e^{-t}}{t} dt \right) dk \right) dk_1 \\ &= \sum_{i_p=0}^n \left( \frac{-2}{2i_p+1} \{I_{3,2i_p}\} - \binom{1+2n}{2i_p} \int_{k_1=0}^1 \frac{k_1^{2+2(m+n)-2i_p}}{2i_p+1} \left[ (k_1-1)^{2i_p+1} \text{Ei} \left( -\left(\frac{k_1-1}{2\mu}\right)^2 \right) - (k_1)^{2i_p+1} \text{Ei} \left( -\left(\frac{k_1}{2\mu}\right)^2 \right) \right] dk_1 \right) \\ &\quad + \sum_{i_i=0}^n \left( \frac{-2}{2i_i+2} \{I_{3,2i_i+1}\} + \binom{1+2n}{2i_i+1} \int_{k_1=0}^1 \frac{k_1^{1+2(m+n)-2i_i}}{2i_i+2} \left[ (k_1-1)^{2i_i+2} \text{Ei} \left( -\left(\frac{k_1-1}{2\mu}\right)^2 \right) - (k_1)^{2i_i+2} \text{Ei} \left( -\left(\frac{k_1}{2\mu}\right)^2 \right) \right] dk_1 \right). \end{aligned} \quad (96)$$

### a. Sum over $i_p$

There are two sub-integrals in the sum over  $i_p$ .

#### First sub-integral

$$- \int_{k_1=0}^1 k_1^{2+2(m+n)+1} \text{Ei} \left( -\left(\frac{k_1}{2\mu}\right)^2 \right) dk_1 = - \frac{\text{Ei} \left( -\left(\frac{1}{2\mu}\right)^2 \right)}{4+2(m+n)} + \frac{2}{4+2(m+n)} S_1[m+n+1] \quad (97)$$

#### Second sub-integral

$$\begin{aligned} \int_{k_1=0}^1 k_1^{2+2(m+n-i_p)} (k_1-1)^{2i_p+1} \text{Ei} \left( -\left(\frac{k_1-1}{2\mu}\right)^2 \right) dk_1 &= \sum_{j=0}^{2+2(m+n-i_p)} \binom{2+2(m+n-i_p)}{j} \int_{k_1=0}^1 (k_1-1)^{j+2i_p+1} \text{Ei} \left( -\left(\frac{k_1-1}{2\mu}\right)^2 \right) dk_1 \\ &= \sum_{j=0}^{2+2(m+n-i_p)} \binom{2+2(m+n-i_p)}{j} \frac{1}{j+2i_p+2} \left[ 0 - (-1)^{j+2i_p+2} \text{Ei} \left( -\left(\frac{-1}{2\mu}\right)^2 \right) \right] \\ &\quad - \sum_{j_p=0}^{1+m+n-i_p} \binom{2+2(m+n-i_p)}{2j_p} \frac{1}{2j_p+2i_p+2} S_1^-[j_p+i_p] \\ &\quad - \sum_{j_i=0}^{m+n-i_p} \binom{2+2(m+n-i_p)}{2j_i+1} \frac{1}{2j_i+2i_p+3} S_1^-[j_i+i_p+1]. \end{aligned} \quad (98)$$

### b. Sum over $i_i$

There are two sub-integrals in the sum over  $i_i$ .

#### First sub-integral

$$- \int_{k_1=0}^1 k_1^{2+2(m+n)+1} \text{Ei} \left( -\left(\frac{k_1}{2\mu}\right)^2 \right) dk_1 = - \frac{\text{Ei} \left( -\left(\frac{1}{2\mu}\right)^2 \right)}{4+2(m+n)} + \frac{2}{4+2(m+n)} S_1[m+n+1] \quad (99)$$

### Second sub-integral

$$\begin{aligned}
\int_{k_1=0}^1 k_1^{1+2(m+n-i_i)} (k_1-1)^{2i_i+2} \text{Ei}\left(-\left(\frac{k_1-1}{2\mu}\right)^2\right) dk_1 &= \sum_{j=0}^{1+2(m+n-i_i)} \binom{1+2(m+n-i_i)}{j} \int_{k_1=0}^1 (k_1-1)^{j+2i_i+2} \text{Ei}\left(-\left(\frac{k_1-1}{2\mu}\right)^2\right) dk_1 \\
&= \sum_{j=0}^{1+2(m+n-i_i)} \binom{1+2(m+n-i_i)}{j} \frac{1}{j+2i_i+3} \left[ 0 - (-1)^{j+i_i+3} \text{Ei}\left(-\left(\frac{-1}{2\mu}\right)^2\right) \right] \\
&\quad - \sum_{j_p=0}^{m+n-i_i} \binom{1+2(m+n-i_i)}{2j_p} \frac{1}{2j_p+2i_i+3} S_p^+[j_p+i_i+1] \\
&\quad - \sum_{j_i=0}^{m+n-i_i} \binom{1+2(m+n-i_i)}{2j_i+1} \frac{1}{2j_i+2i_i+4} S_i^+[j_i+i_i+1] \quad (100)
\end{aligned}$$

### 3. Expression of integral $II_4$

We have found each sub-integral of the fourth integral  $II_4$  of the second part of the exchange energy. The expression of  $II_4$  is thus

$$\begin{aligned}
II_4 &= \int_{k_1=0}^1 \int_{k_2=0}^1 k_1^{1+2m} k_2^{1+2n} \text{Ei}\left(-\left(\frac{k_1-k_2}{2\mu}\right)^2\right) dk_2 dk_1 \\
&= \sum_{i_p=0}^n \left\{ \frac{-2}{2i_p+1} \{I_{3,2i_p}\} - \frac{1}{2i_p+1} \binom{1+2n}{2i_p} \left[ -\frac{\text{Ei}\left(-\left(\frac{1}{2\mu}\right)^2\right)}{4+2(m+n)} + \frac{2}{4+2(m+n)} S_i[m+n+1] \right. \right. \\
&\quad + \sum_{j=0}^{2+2(m+n-i_p)} \binom{2+2(m+n-i_p)}{j} \frac{1}{j+2i_p+2} \left[ 0 - \text{Ei}\left(-\left(\frac{-1}{2\mu}\right)^2\right) \right] \\
&\quad - \sum_{j_p=0}^{m+n-i_p+1} \binom{2+2(m+n-i_p)}{2j_p} \frac{1}{2j_p+2i_p+2} S_i^-[j_p+i_p] \\
&\quad \left. \left. - \sum_{j_i=0}^{m+n-i_p} \binom{2+2(m+n-i_p)}{2j_i+1} \frac{1}{2j_i+2i_p+3} S_p^-[j_i+i_p+1] \right] \right\} \\
&+ \sum_{i_i=0}^n \left\{ \frac{-2}{2i_i+2} \{I_{3,2i_i+1}\} - \frac{1}{2i_i+2} \binom{1+2n}{2i_i+1} \left[ -\frac{\text{Ei}\left(-\left(\frac{1}{2\mu}\right)^2\right)}{4+2(m+n)} + \frac{2}{4+2(m+n)} S_i[m+n+1] \right. \right. \\
&\quad + \sum_{j=0}^{1+2(m+n-i_i)} \binom{1+2(m+n-i_i)}{j} \frac{1}{j+2i_i+3} \left[ 0 - \text{Ei}\left(-\left(\frac{-1}{2\mu}\right)^2\right) \right] \\
&\quad + \sum_{j_p=0}^{m+n-i_i} \binom{1+2(m+n-i_i)}{2j_p} \frac{1}{2j_p+2i_i+3} S_p^-[j_p+i_i+1] \\
&\quad \left. \left. - \sum_{j_i=0}^{m+n-i_i} \binom{1+2(m+n-i_i)}{2j_i+1} \frac{1}{2j_i+2i_i+4} S_i^-[j_i+i_i+1] \right] \right\}. \quad (101)
\end{aligned}$$
