# Supplementary material for: Four-component relativistic range-separated density-functional theory: Short-range exchange local-density approximation
Source: arXiv:1812.02024 source file (2018-12-05)
Supplement: Supplementary file 2 [file supplementary_mathematica.tex]

(* Content-type: application/vnd.wolfram.mathematica *)

(*** Wolfram Notebook File ***)
(* http://www.wolfram.com/nb *)

(* CreatedBy='Mathematica 11.0' *)

(*CacheID: 234*)
(* Internal cache information:
NotebookFileLineBreakTest
NotebookFileLineBreakTest
NotebookDataPosition[       158,          7]
NotebookDataLength[    621816,      12385]
NotebookOptionsPosition[    599104,      12043]
NotebookOutlinePosition[    599509,      12059]
CellTagsIndexPosition[    599466,      12056]
WindowFrame->Normal*)

(* Beginning of Notebook Content *)
Notebook[{

Cell[CellGroupData[{
Cell["\<\
Supplementary Information to 
Four-component relativistic range-separated density-functional theory: 
\tShort-range exchange local-density approximation                  \
\>", "Chapter",
 CellChangeTimes->{{3.741404290596384*^9, 3.741404373922989*^9}, {
   3.741404454230689*^9, 3.7414044603298407`*^9}, {3.741487232155581*^9, 
   3.741487234218924*^9}, {3.741487272560252*^9, 3.7414872878844976`*^9}, 
   3.741487339979101*^9, 3.7414963985987453`*^9},
 TextAlignment->Center,ExpressionUUID->"3ecf45d0-c07a-46d3-9913-4e3a72c6e449"],

Cell["\<\
                           
Julien Paquier (\:2217) and Julien Toulouse (\[Dagger])
Laboratoire de Chimie Th\[EAcute]orique (LCT), Sorbonne Universit\[EAcute] \
and CNRS, F-75005 Paris, France
(Dated: July 25, 2018)
\
\>", "Subtitle",
 CellChangeTimes->{
  3.741404357532297*^9, {3.741404415994296*^9, 3.7414044632933073`*^9}, {
   3.741404781164523*^9, 3.741404800110065*^9}, {3.74140483612987*^9, 
   3.741404909008362*^9}, {3.741407439145772*^9, 3.7414074421546717`*^9}, {
   3.7414873081337013`*^9, 3.7414873142832747`*^9}, {3.741496437110674*^9, 
   3.7414964373504744`*^9}},
 TextAlignment->Center,ExpressionUUID->"e546b7da-b0f3-4494-8292-4519e1a30d74"],

Cell["", "Text",
 CellChangeTimes->{{3.7414048511854753`*^9, 
  3.7414048555474*^9}},ExpressionUUID->"93278e3d-662c-41eb-9dc8-fe7a8e9c8693"],

Cell[BoxData[{
 FormBox[
  RowBox[{
   RowBox[{
    RowBox[{
     RowBox[{
     "This", " ", "notebook", " ", "contains", " ", "calculations", " ", "of",
       " ", "the", " ", "relativistic", " ", "short"}], "-", 
     RowBox[{
     "range", " ", "exchange", " ", "energies", " ", "per", " ", "particle", 
      " ", "of", " ", "the", " ", "relativistic", " ", "homogeneous", " ", 
      "electron", " ", "gas", "  ", 
      RowBox[{"(", "RHEG", ")"}], "for", " ", "several", "  ", "electron"}], 
     "-", 
     RowBox[{"electron", " ", "interaction", " ", "potentials", " ", 
      RowBox[{
       RowBox[{"(", 
        RowBox[{"Coulomb", ",", " ", "Breit", ",", " ", 
         RowBox[{
          RowBox[{"and", " ", "Coulomb"}], "-", "Breit"}]}], ")"}], ".", " ", 
       "\[IndentingNewLine]", "\[LineSeparator]", "We"}], " ", "consider", 
      " ", "the", " ", "variables", " ", "in", " ", "unit", " ", "of", " ", 
      "kF"}]}], ",", " ", 
    RowBox[{
    "meaning", " ", "that", " ", "the", " ", "present", " ", "c", " ", "and", 
     " ", "\[Mu]", " ", "must", " ", "be", " ", "understood", " ", "as", " ", 
     "the", " ", 
     OverscriptBox["c", "~"], " ", "and", " ", 
     OverscriptBox["\[Mu]", "~"], " ", "of", " ", "the", " ", "main", " ", 
     RowBox[{"article", ".", "  ", "\[LineSeparator]", "The"}], " ", 
     "\[Alpha]", " ", "and", " ", "\[Beta]", "  ", "coefficients", " ", 
     "expressed", " ", "respectively", " ", "in", " ", 
     RowBox[{"Eq", ".", "  ", 
      RowBox[{"(", "37", ")"}]}], " ", "and", " ", 
     RowBox[{"Eq", ".", "  ", 
      RowBox[{"(", "42", ")"}]}], " ", "of", " ", "the", " ", "main", " ", 
     "article", " ", "have", " ", "been", " ", "obtained", " ", "using", " ", 
     "the", " ", "present", " ", "mathematica", " ", "calculations"}], ",", 
    RowBox[{
     RowBox[{"the", "  ", "large"}], "-", 
     RowBox[{
     "c", " ", "expansion", " ", "of", "  ", "the", " ", "relativistic", "  ",
       "short"}], "-", 
     RowBox[{
     "range", " ", "exchange", " ", "energies", " ", "per", " ", "particle", 
      " ", "is", " ", "expressed"}]}]}], " "}], 
  TraditionalForm], "\[LineSeparator]", 
 FormBox[
  RowBox[{
   RowBox[{
    RowBox[{"as", " ", 
     StyleBox["a",
      FontSlant->"Plain"], " ", "function", " ", "of", " ", "the", " ", 
     "order", " ", "N", " ", "of", " ", "the", " ", 
     RowBox[{"expansion", ".", "\[LineSeparator]", "The"}], " ", 
     "Pad\[EAcute]", " ", "approximants", " ", "illustrated", " ", "in", " ", 
     
     RowBox[{"Fig", ".", " ", "3"}], " ", "of", " ", "the", " ", "main", " ", 
     "article", " ", "have", " ", "been", " ", "obtained", " ", "using", " ", 
     "the", " ", "present", " ", "mathematica", " ", "calculations"}], ",", 
    RowBox[{
     RowBox[{
     "the", " ", "diagonal", " ", "Pad\[EAcute]", " ", "approximants", " ", 
      "of", "  ", "the", " ", "relativistic", "  ", "full"}], "-", 
     RowBox[{"range", " ", "and", " ", "short"}], "-", 
     RowBox[{
     "range", " ", "exchange", " ", "energies", " ", "per", " ", "particle", 
      " ", "are", " ", "expressed"}]}]}], " "}], 
  TraditionalForm], "\[LineSeparator]", 
 FormBox[
  RowBox[{
  "as", " ", "functions", " ", "of", " ", "the", " ", "order", " ", "N", " ", 
   "of", " ", "the", " ", 
   RowBox[{
   "approximants", ".", "\[LineSeparator]", "\[LineSeparator]", 
    "\[LineSeparator]", "One"}], " ", "should", " ", "first", " ", "run", " ",
    "the", " ", "\"\<General preliminary calculations\>\"", " ", 
   RowBox[{"section", ".", "  ", "The"}], " ", "final", " ", "expressions", 
   " ", "are", " ", "in", " ", "the", 
   "\"\<Calculation of the large-c expansion and Pad\[EAcute] \
approximant\>\"", " ", 
   RowBox[{"subsections", ".", "\[IndentingNewLine]"}]}], 
  TraditionalForm]}], "Text",
 CellChangeTimes->{{3.741312350472324*^9, 3.7413123690967083`*^9}, {
   3.741312410375852*^9, 3.741312557625122*^9}, {3.741325692446144*^9, 
   3.7413257825250053`*^9}, {3.741325866893469*^9, 3.74132592228545*^9}, 
   3.741332102041424*^9, 3.741404903525641*^9, {3.74140496847904*^9, 
   3.741405118017108*^9}, {3.741405744988945*^9, 3.74140586708692*^9}, {
   3.741405897301285*^9, 3.741405926984535*^9}, {3.741406031338621*^9, 
   3.741406053547368*^9}, {3.7414060892714853`*^9, 3.741406281292914*^9}, {
   3.7414063117459173`*^9, 3.741406405059928*^9}, {3.741406939330653*^9, 
   3.741406940643499*^9}, {3.741406976321501*^9, 3.741406982394936*^9}, {
   3.741407021313044*^9, 3.7414071180558853`*^9}, {3.7414071572254877`*^9, 
   3.741407191542362*^9}, {3.741407561959086*^9, 3.741407575901327*^9}, {
   3.741487350124145*^9, 3.741487368767684*^9}, {3.741505907982675*^9, 
   3.741506082895246*^9}, {3.741506144015271*^9, 
   3.741506175823838*^9}},ExpressionUUID->"f8dabe74-5bba-4406-82a0-\
464dc32821f0"],

Cell[CellGroupData[{

Cell["\<\
(\:2217) julien.paquier@lct.jussieu.fr \t(\[Dagger]) toulouse@lct.jussieu.fr\
\>", "Subsubtitle",
 CellChangeTimes->{
  3.741404901814217*^9, {3.741404936644725*^9, 
   3.7414049586961184`*^9}},ExpressionUUID->"cd72ad39-209c-4743-a995-\
1bc6c760601a"],

Cell[CellGroupData[{

Cell["General preliminary calculations", "Section",
 CellChangeTimes->{{3.741319870976974*^9, 3.741319874769227*^9}, 
   3.7413257351831512`*^9, {3.7413350820752153`*^9, 3.741335087819014*^9}},
 ExpressionUUID -> "a087474c-de1e-4a3b-8d4f-b56f42fdf834"],

Cell[CellGroupData[{

Cell["\<\
Tables of the integrated expressions of the general term of the large-c \
expansion \
\>", "Subsection",
 CellChangeTimes->{
  3.741312160234782*^9, {3.741315121356236*^9, 3.741315129548183*^9}, {
   3.741334737770865*^9, 3.7413347433531227`*^9}},
 ExpressionUUID -> "f6fe979e-a9d6-4ad6-bbdc-7f019076ef4e"],

Cell[CellGroupData[{

Cell["Sums from repeated integrations by part", "Subsubsection",
 CellChangeTimes->{{3.741314336794527*^9, 3.741314344585115*^9}, {
   3.7413346715301533`*^9, 3.741334672377591*^9}, {3.74133470936985*^9, 
   3.741334711497727*^9}, 
   3.741334765145706*^9},ExpressionUUID->"0c0573a7-6809-493a-a553-\
d5438add8965"],

Cell[TextData[{
 "We need to consider and stock in matrix form the sums coming from the \
repeated integrations by parts. First we have the sum for an even index ",
 Cell[BoxData[
  FormBox[
   SubscriptBox["j", "p"], TraditionalForm]],ExpressionUUID->
  "4b903f20-c8b8-4097-9b4d-91c7a3482334"]
}], "Text",
 CellChangeTimes->{{3.72215848038514*^9, 3.722158490240019*^9}, {
  3.7413133809378967`*^9, 3.741313471225456*^9}, {3.7413135084897118`*^9, 
  3.741313539721591*^9}, {3.741313593497574*^9, 3.741313605151305*^9}, {
  3.741313667337452*^9, 3.7413136674340973`*^9}, {3.7413347745061207`*^9, 
  3.741334809066297*^9}},ExpressionUUID->"33af9183-bbc9-4d43-b33d-\
c33e4c164cf4"],

Cell[BoxData[
 RowBox[{
  RowBox[{
   SubscriptBox["S", "even"], "[", "jp_", "]"}], ":=", 
  RowBox[{"Simplify", "[", 
   RowBox[{
    RowBox[{
     SuperscriptBox[
      RowBox[{"(", 
       RowBox[{"2", 
        SuperscriptBox["\[Mu]", "2"]}], ")"}], "jp"], 
     RowBox[{
      RowBox[{"(", 
       RowBox[{
        RowBox[{"2", "jp"}], "-", "1"}], ")"}], "!!"}], 
     RowBox[{"(", 
      RowBox[{"2", "\[Mu]"}], ")"}], 
     FractionBox[
      SqrtBox["\[Pi]"], "2"], 
     RowBox[{"(", 
      RowBox[{"Erf", "[", 
       FractionBox["1", "\[Mu]"], "]"}], ")"}]}], " ", "-", 
    RowBox[{"Sum", "[", 
     RowBox[{
      RowBox[{
       SuperscriptBox[
        RowBox[{"(", 
         RowBox[{"2", 
          SuperscriptBox["\[Mu]", "2"]}], ")"}], 
        RowBox[{"\[Lambda]p", "+", "1"}]], 
       FractionBox[
        RowBox[{
         RowBox[{"(", 
          RowBox[{
           RowBox[{"2", "jp"}], "-", "1"}], ")"}], "!!"}], 
        RowBox[{
         RowBox[{"(", 
          RowBox[{
           RowBox[{"2", "jp"}], "-", 
           RowBox[{"(", 
            RowBox[{"1", "+", 
             RowBox[{"2", "\[Lambda]p"}]}], ")"}]}], ")"}], "!!"}]], 
       RowBox[{"(", 
        RowBox[{
         SuperscriptBox[
          RowBox[{"(", "2", ")"}], 
          RowBox[{
           RowBox[{"2", "jp"}], "-", 
           RowBox[{"(", 
            RowBox[{"1", "+", 
             RowBox[{"2", "\[Lambda]p"}]}], ")"}]}]], 
         RowBox[{"Exp", "[", 
          RowBox[{"-", 
           SuperscriptBox[
            RowBox[{"(", 
             FractionBox["1", "\[Mu]"], ")"}], "2"]}], "]"}]}], ")"}]}], ",", 
      
      RowBox[{"{", 
       RowBox[{"\[Lambda]p", ",", "0", ",", 
        RowBox[{"jp", "-", "1"}]}], "}"}]}], "]"}]}], "]"}]}]], "Input",
 CellChangeTimes->{{3.722145850982307*^9, 3.722145926980988*^9}, {
   3.72214653341287*^9, 3.722146545042983*^9}, {3.722146717392494*^9, 
   3.722146718623077*^9}, 3.722147760547078*^9, {3.7221485399057627`*^9, 
   3.722148540399416*^9}, 3.722148628112403*^9, 3.74116478586759*^9, {
   3.741404137586298*^9, 3.7414041407826967`*^9}},
 ExpressionUUID -> "6e8fe0f7-bd5a-44da-ac3e-5795deda50df"],

Cell[BoxData[
 RowBox[{
  RowBox[{
   SubscriptBox["TableS", "even"], "=", 
   RowBox[{"Table", "[", 
    RowBox[{
     RowBox[{
      SubscriptBox["S", "even"], "[", "i", "]"}], ",", 
     RowBox[{"{", 
      RowBox[{"i", ",", "0", ",", "20"}], "}"}]}], "]"}]}], ";"}]], "Input",
 CellChangeTimes->{{3.72214598334976*^9, 3.722145986564417*^9}, {
   3.722146721892762*^9, 3.722146725541695*^9}, {3.722147467422069*^9, 
   3.722147467757551*^9}, 3.7221485463200502`*^9, 3.7221486306683598`*^9, 
   3.7221587254879007`*^9, 3.722158782767756*^9, {3.740299028150506*^9, 
   3.740299028246863*^9}, {3.740300004168995*^9, 3.740300004296165*^9}, {
   3.740363781710928*^9, 3.7403637864321957`*^9}},
 ExpressionUUID -> "a9168a14-3b0c-4487-ba58-1bd5ab5e3e8f"],

Cell[TextData[{
 "We have also the sums for an odd index ",
 Cell[BoxData[
  FormBox[
   SubscriptBox["j", "i"], TraditionalForm]],ExpressionUUID->
  "566897b3-0995-42d8-bf4c-85000dc673c8"]
}], "Text",
 CellChangeTimes->{{3.720685696087637*^9, 3.720685706319282*^9}, {
  3.7206868782729797`*^9, 3.720686878835619*^9}, {3.720695340799407*^9, 
  3.720695346668665*^9}, {3.72214602544331*^9, 3.722146031360856*^9}, {
  3.741313610873383*^9, 3.741313622700389*^9}, {3.741334839209894*^9, 
  3.741334839514122*^9}},ExpressionUUID->"2b48ce9f-8763-4a59-bd98-\
c18a18f551a6"],

Cell[BoxData[
 RowBox[{
  RowBox[{
   SubscriptBox["S", "odd"], "[", "ji_", "]"}], ":=", 
  RowBox[{"Simplify", "[", 
   RowBox[{
    RowBox[{
     SuperscriptBox[
      RowBox[{"(", 
       RowBox[{"2", 
        SuperscriptBox["\[Mu]", "2"]}], ")"}], "ji"], 
     RowBox[{
      RowBox[{"(", 
       RowBox[{"2", "ji"}], ")"}], "!!"}], 
     RowBox[{"(", 
      RowBox[{
       RowBox[{"-", "2"}], 
       SuperscriptBox["\[Mu]", "2"]}], ")"}], 
     RowBox[{"(", 
      RowBox[{
       RowBox[{"Exp", "[", 
        RowBox[{"-", 
         SuperscriptBox[
          RowBox[{"(", 
           FractionBox[
            RowBox[{"1", "+", "1"}], 
            RowBox[{"2", "\[Mu]"}]], ")"}], "2"]}], "]"}], "-", "1"}], 
      ")"}]}], " ", "-", 
    RowBox[{"Sum", "[", 
     RowBox[{
      RowBox[{
       SuperscriptBox[
        RowBox[{"(", 
         RowBox[{"2", 
          SuperscriptBox["\[Mu]", "2"]}], ")"}], 
        RowBox[{"\[Lambda]i", "+", "1"}]], 
       FractionBox[
        RowBox[{
         RowBox[{"(", 
          RowBox[{"2", "ji"}], ")"}], "!!"}], 
        RowBox[{
         RowBox[{"(", 
          RowBox[{
           RowBox[{"2", "ji"}], "-", 
           RowBox[{"2", "\[Lambda]i"}]}], ")"}], "!!"}]], 
       RowBox[{"(", 
        RowBox[{
         SuperscriptBox[
          RowBox[{"(", "2", ")"}], 
          RowBox[{
           RowBox[{"2", "ji"}], "-", 
           RowBox[{"2", "\[Lambda]i"}]}]], 
         RowBox[{"Exp", "[", 
          RowBox[{"-", 
           SuperscriptBox[
            RowBox[{"(", 
             FractionBox[
              RowBox[{"1", "+", "1"}], 
              RowBox[{"2", "\[Mu]"}]], ")"}], "2"]}], "]"}]}], ")"}]}], ",", 
      RowBox[{"{", 
       RowBox[{"\[Lambda]i", ",", "0", ",", 
        RowBox[{"ji", "-", "1"}]}], "}"}]}], "]"}]}], "]"}]}]], "Input",
 CellChangeTimes->{{3.720683748649046*^9, 3.7206837593057203`*^9}, {
   3.7206856790646963`*^9, 3.720685679459322*^9}, {3.720685740214123*^9, 
   3.720685768707493*^9}, {3.720685802202055*^9, 3.720685833057756*^9}, {
   3.720685879846085*^9, 3.7206859214901323`*^9}, {3.720685965142241*^9, 
   3.720686042779799*^9}, {3.720686321254796*^9, 3.720686323495965*^9}, {
   3.720686884119032*^9, 3.720686940757525*^9}, {3.720705129030883*^9, 
   3.720705136409897*^9}, {3.720705271624501*^9, 3.720705274737891*^9}, {
   3.720707116509796*^9, 3.720707128840559*^9}, {3.7207071634184713`*^9, 
   3.72070718451825*^9}, {3.720764876967244*^9, 3.72076488777966*^9}, {
   3.7207658811435003`*^9, 3.720765884776372*^9}, {3.7207785473716908`*^9, 
   3.720778549337688*^9}, {3.721448294610702*^9, 3.721448354643697*^9}, 
   3.721448710113863*^9, {3.7221461055725927`*^9, 3.7221461115258703`*^9}, {
   3.7221461449006977`*^9, 3.722146166179097*^9}, {3.7221465808032627`*^9, 
   3.722146594757306*^9}, 3.722146633540729*^9, {3.722146700402128*^9, 
   3.7221467009153147`*^9}, {3.7221477524666986`*^9, 3.722147752591444*^9}, {
   3.722148543009444*^9, 3.7221485436923656`*^9}, 3.722148633391795*^9, {
   3.741404151099427*^9, 3.741404157002962*^9}},
 ExpressionUUID -> "8b8964af-abbe-474c-a7ca-5b5b099e5fff"],

Cell[BoxData[
 RowBox[{
  RowBox[{
   SubscriptBox["TableS", "odd"], "=", 
   RowBox[{"Table", "[", 
    RowBox[{
     RowBox[{
      SubscriptBox["S", "odd"], "[", "i", "]"}], ",", 
     RowBox[{"{", 
      RowBox[{"i", ",", "0", ",", "20"}], "}"}]}], "]"}]}], ";"}]], "Input",
 CellChangeTimes->{{3.7214690643865013`*^9, 3.7214690673947077`*^9}, {
   3.7220600269291897`*^9, 3.722060027201326*^9}, {3.722146202370328*^9, 
   3.722146205239731*^9}, {3.722146657906699*^9, 3.722146709489509*^9}, 
   3.722147470397524*^9, {3.722147698547394*^9, 3.722147717395541*^9}, {
   3.72214776584096*^9, 3.7221477660789957`*^9}, 3.722148552894147*^9, 
   3.72214863548717*^9, 3.7221587304320087`*^9, 3.722158785888052*^9, {
   3.740299033942544*^9, 3.740299034038559*^9}, {3.740300007639592*^9, 
   3.74030000775134*^9}, {3.7403637838083153`*^9, 3.740363784304389*^9}},
 ExpressionUUID -> "43d481f5-8d4a-44b1-800c-0bc62b04edac"]
}, Closed]],

Cell[CellGroupData[{

Cell["Analytical integrals of the general term", "Subsubsection",
 CellChangeTimes->{{3.741314356602261*^9, 
  3.741314368266243*^9}},ExpressionUUID->"c3b2621d-5f51-4c39-9370-\
521d59221e49"],

Cell["\<\
Having expressed the sums coming from the repeated integrations by parts we \
can express the general expressions of the different parts of the analytical \
integrals of the general term. We start with the First integral of the First \
Part of the exchange energy\
\>", "Text",
 CellChangeTimes->{{3.7221584940672083`*^9, 3.722158505682335*^9}, {
  3.7413136503776712`*^9, 3.741313721337852*^9}, {3.741313832026993*^9, 
  3.741313833515273*^9}, {3.7413141721710176`*^9, 3.7413141776742163`*^9}, {
  3.741314372522131*^9, 3.741314375530726*^9}, {3.7413348719950457`*^9, 
  3.74133487642655*^9}, {3.7413349836591473`*^9, 3.741334984714993*^9}},
 ExpressionUUID -> "25cd696f-46f9-4ebd-97f3-f191097f1483"],

Cell[BoxData[
 RowBox[{
  RowBox[{"Part1First", "[", 
   RowBox[{"m_", ",", "n_"}], "]"}], ":=", 
  FractionBox["1", 
   RowBox[{"9", "+", 
    RowBox[{"6", " ", "m"}], "+", 
    RowBox[{"6", " ", "n"}], "+", 
    RowBox[{"4", " ", "m", " ", "n"}]}]]}]], "Input",
 CellChangeTimes->{{3.7220584461219063`*^9, 3.722058454466215*^9}, {
   3.741313732922333*^9, 3.7413137334822807`*^9}, 3.7413137879465227`*^9},
 ExpressionUUID -> "84733fba-0f2c-49a1-9c9f-acf6ec228a6b"],

Cell["\<\
We express the subtraction of the Third integral of the First Part from the \
Second integral of the First Part\
\>", "Text",
 CellChangeTimes->{{3.741313827545678*^9, 3.741313925002655*^9}, {
  3.741314149226349*^9, 3.741314166525208*^9}},
 ExpressionUUID -> "1a333e23-d307-41b9-bb5f-7b866d32ef3c"],

Cell[BoxData[
 RowBox[{
  RowBox[{"Part1SecondminusThird", "[", 
   RowBox[{"m_", ",", "n_"}], "]"}], ":=", " ", 
  RowBox[{
   RowBox[{"-", 
    RowBox[{"Sum", "[", 
     RowBox[{
      RowBox[{
       RowBox[{"Binomial", "[", 
        RowBox[{
         RowBox[{"1", "+", 
          RowBox[{"2", "n"}]}], ",", 
         RowBox[{"2", "ip"}]}], "]"}], 
       SuperscriptBox[
        RowBox[{"(", 
         RowBox[{"2", "\[Mu]"}], ")"}], 
        RowBox[{"1", "+", 
         RowBox[{"2", "ip"}]}]], 
       RowBox[{"(", 
        RowBox[{
         RowBox[{
          FractionBox[
           RowBox[{
            RowBox[{"(", 
             RowBox[{
              RowBox[{"2", "ip"}], "-", "1"}], ")"}], "!!"}], 
           SuperscriptBox["2", "ip"]], 
          FractionBox["1", 
           RowBox[{"3", "+", 
            RowBox[{"2", 
             RowBox[{"(", 
              RowBox[{"m", "+", "n", "-", "ip"}], ")"}]}]}]], 
          RowBox[{"(", 
           RowBox[{
            RowBox[{
             FractionBox[
              SqrtBox["\[Pi]"], "2"], 
             RowBox[{"(", 
              RowBox[{"Erf", "[", 
               FractionBox["1", "\[Mu]"], "]"}], ")"}]}], "+", 
            RowBox[{
             FractionBox["1", 
              RowBox[{"2", "\[Mu]"}]], 
             RowBox[{"(", 
              RowBox[{
               RowBox[{"Sum", "[", 
                RowBox[{
                 RowBox[{
                  RowBox[{"Binomial", "[", 
                   RowBox[{
                    RowBox[{"3", "+", 
                    RowBox[{"2", 
                    RowBox[{"(", 
                    RowBox[{"m", "+", "n", "-", "ip"}], ")"}]}]}], ",", 
                    RowBox[{"2", "jp"}]}], "]"}], 
                  RowBox[{"Part", "[", 
                   RowBox[{
                    SubscriptBox["TableS", "even"], ",", 
                    RowBox[{"jp", "+", "1"}]}], "]"}]}], ",", 
                 RowBox[{"{", 
                  RowBox[{"jp", ",", "0", ",", 
                   RowBox[{"m", "+", "n", "-", "ip", "+", "1"}]}], "}"}]}], 
                "]"}], "-", 
               RowBox[{"Sum", "[", 
                RowBox[{
                 RowBox[{
                  RowBox[{"Binomial", "[", 
                   RowBox[{
                    RowBox[{"3", "+", 
                    RowBox[{"2", 
                    RowBox[{"(", 
                    RowBox[{"m", "+", "n", "-", "ip"}], ")"}]}]}], ",", 
                    RowBox[{
                    RowBox[{"2", "ji"}], "+", "1"}]}], "]"}], 
                  RowBox[{"Part", "[", 
                   RowBox[{
                    SubscriptBox["TableS", "odd"], ",", 
                    RowBox[{"ji", "+", "1"}]}], "]"}]}], ",", 
                 RowBox[{"{", 
                  RowBox[{"ji", ",", "0", ",", 
                   RowBox[{"m", "+", "n", "-", "ip", "+", "1"}]}], "}"}]}], 
                "]"}]}], ")"}]}]}], ")"}]}], "-", 
         RowBox[{"(", 
          RowBox[{"Sum", "[", 
           RowBox[{
            RowBox[{
             FractionBox["1", 
              SuperscriptBox["2", 
               RowBox[{"lp", "+", "1"}]]], 
             FractionBox[
              RowBox[{
               RowBox[{"(", 
                RowBox[{
                 RowBox[{"2", "ip"}], "-", "1"}], ")"}], "!!"}], 
              RowBox[{
               RowBox[{"(", 
                RowBox[{
                 RowBox[{"2", "ip"}], "-", "1", "-", 
                 RowBox[{"2", "lp"}]}], ")"}], "!!"}]], 
             FractionBox["1", 
              SuperscriptBox[
               RowBox[{"(", 
                RowBox[{"2", "\[Mu]"}], ")"}], 
               RowBox[{
                RowBox[{"2", "ip"}], "-", "1", "-", 
                RowBox[{"2", "lp"}]}]]], 
             RowBox[{"(", 
              RowBox[{
               RowBox[{"Sum", "[", 
                RowBox[{
                 RowBox[{
                  RowBox[{"Binomial", "[", 
                   RowBox[{
                    RowBox[{"2", "+", 
                    RowBox[{"2", 
                    RowBox[{"(", 
                    RowBox[{"m", "+", "n", "-", "ip"}], ")"}]}]}], ",", 
                    RowBox[{"2", "jp"}]}], "]"}], 
                  RowBox[{"Part", "[", 
                   RowBox[{
                    SubscriptBox["TableS", "odd"], ",", 
                    RowBox[{
                    "jp", "+", "ip", "-", "lp", "-", "1", "+", "1"}]}], 
                   "]"}]}], ",", 
                 RowBox[{"{", 
                  RowBox[{"jp", ",", "0", ",", 
                   RowBox[{"m", "+", "n", "-", "ip", "+", "1"}]}], "}"}]}], 
                "]"}], "-", 
               RowBox[{"Sum", "[", 
                RowBox[{
                 RowBox[{
                  RowBox[{"Binomial", "[", 
                   RowBox[{
                    RowBox[{"2", "+", 
                    RowBox[{"2", 
                    RowBox[{"(", 
                    RowBox[{"m", "+", "n", "-", "ip"}], ")"}]}]}], ",", 
                    RowBox[{
                    RowBox[{"2", "ji"}], "+", "1"}]}], "]"}], 
                  RowBox[{"Part", "[", 
                   RowBox[{
                    SubscriptBox["TableS", "even"], ",", 
                    RowBox[{"ji", "+", "ip", "-", "lp", "+", "1"}]}], "]"}]}],
                  ",", 
                 RowBox[{"{", 
                  RowBox[{"ji", ",", "0", ",", 
                   RowBox[{"m", "+", "n", "-", "ip"}]}], "}"}]}], "]"}]}], 
              ")"}]}], ",", 
            RowBox[{"{", 
             RowBox[{"lp", ",", "0", ",", 
              RowBox[{"ip", "-", "1"}]}], "}"}]}], "]"}], ")"}]}], ")"}]}], 
      ",", " ", 
      RowBox[{"{", 
       RowBox[{"ip", ",", "0", ",", "n"}], "}"}]}], "]"}]}], "+", 
   RowBox[{"Sum", "[", 
    RowBox[{
     RowBox[{
      RowBox[{"Binomial", "[", 
       RowBox[{
        RowBox[{"1", "+", 
         RowBox[{"2", "n"}]}], ",", 
        RowBox[{
         RowBox[{"2", "ii"}], "+", "1"}]}], "]"}], 
      SuperscriptBox[
       RowBox[{"(", 
        RowBox[{"2", "\[Mu]"}], ")"}], 
       RowBox[{"2", "+", 
        RowBox[{"2", "ii"}]}]], 
      RowBox[{"(", 
       RowBox[{
        RowBox[{
         FractionBox[
          RowBox[{
           RowBox[{"(", 
            RowBox[{"2", "ii"}], ")"}], "!!"}], 
          SuperscriptBox["2", "ii"]], 
         RowBox[{"(", 
          RowBox[{"-", 
           FractionBox["1", "2"]}], ")"}], 
         RowBox[{"(", 
          RowBox[{
           RowBox[{"Sum", "[", 
            RowBox[{
             RowBox[{
              RowBox[{"-", 
               RowBox[{"Binomial", "[", 
                RowBox[{
                 RowBox[{"1", "+", 
                  RowBox[{"2", 
                   RowBox[{"(", 
                    RowBox[{"m", "+", "n", "-", "ii"}], ")"}]}]}], ",", 
                 RowBox[{"2", "jp"}]}], "]"}]}], 
              RowBox[{"Part", "[", 
               RowBox[{
                SubscriptBox["TableS", "even"], ",", 
                RowBox[{"jp", "+", "1"}]}], "]"}]}], ",", 
             RowBox[{"{", 
              RowBox[{"jp", ",", "0", ",", 
               RowBox[{"m", "+", "n", "-", "ii"}]}], "}"}]}], "]"}], "+", 
           RowBox[{"Sum", "[", 
            RowBox[{
             RowBox[{
              RowBox[{"Binomial", "[", 
               RowBox[{
                RowBox[{"1", "+", 
                 RowBox[{"2", 
                  RowBox[{"(", 
                   RowBox[{"m", "+", "n", "-", "ii"}], ")"}]}]}], ",", 
                RowBox[{
                 RowBox[{"2", "ji"}], "+", "1"}]}], "]"}], 
              RowBox[{"Part", "[", 
               RowBox[{
                SubscriptBox["TableS", "odd"], ",", 
                RowBox[{"ji", "+", "1"}]}], "]"}]}], ",", 
             RowBox[{"{", 
              RowBox[{"ji", ",", "0", ",", 
               RowBox[{"m", "+", "n", "-", "ii"}]}], "}"}]}], "]"}]}], 
          ")"}]}], "-", "                            ", 
        RowBox[{"(", 
         RowBox[{"Sum", "[", 
          RowBox[{
           RowBox[{
            FractionBox["1", 
             SuperscriptBox["2", 
              RowBox[{"li", "+", "1"}]]], 
            FractionBox[
             RowBox[{
              RowBox[{"(", 
               RowBox[{"2", "ii"}], ")"}], "!!"}], 
             RowBox[{
              RowBox[{"(", 
               RowBox[{
                RowBox[{"2", "ii"}], "-", 
                RowBox[{"2", "li"}]}], ")"}], "!!"}]], 
            FractionBox["1", 
             SuperscriptBox[
              RowBox[{"(", 
               RowBox[{"2", "\[Mu]"}], ")"}], 
              RowBox[{
               RowBox[{"2", "ii"}], "-", 
               RowBox[{"2", "li"}]}]]], 
            RowBox[{"(", 
             RowBox[{
              RowBox[{"-", 
               RowBox[{"Sum", "[", 
                RowBox[{
                 RowBox[{
                  RowBox[{"Binomial", "[", 
                   RowBox[{
                    RowBox[{"1", "+", 
                    RowBox[{"2", 
                    RowBox[{"(", 
                    RowBox[{"m", "+", "n", "-", "ii"}], ")"}]}]}], ",", 
                    RowBox[{"2", "jp"}]}], "]"}], 
                  RowBox[{"Part", "[", 
                   RowBox[{
                    SubscriptBox["TableS", "even"], ",", 
                    RowBox[{"jp", "+", "ii", "-", "li", "+", "1"}]}], "]"}]}],
                  ",", 
                 RowBox[{"{", 
                  RowBox[{"jp", ",", "0", ",", 
                   RowBox[{"m", "+", "n", "-", "ii", "+", "1"}]}], "}"}]}], 
                "]"}]}], "+", 
              RowBox[{"Sum", "[", 
               RowBox[{
                RowBox[{
                 RowBox[{"Binomial", "[", 
                  RowBox[{
                   RowBox[{"1", "+", 
                    RowBox[{"2", 
                    RowBox[{"(", 
                    RowBox[{"m", "+", "n", "-", "ii"}], ")"}]}]}], ",", 
                   RowBox[{
                    RowBox[{"2", "ji"}], "+", "1"}]}], "]"}], 
                 RowBox[{"Part", "[", 
                  RowBox[{
                   SubscriptBox["TableS", "odd"], ",", 
                   RowBox[{"ji", "+", "ii", "-", "li", "+", "1"}]}], "]"}]}], 
                ",", 
                RowBox[{"{", 
                 RowBox[{"ji", ",", "0", ",", 
                  RowBox[{"m", "+", "n", "-", "ii"}]}], "}"}]}], "]"}]}], 
             ")"}]}], ",", 
           RowBox[{"{", 
            RowBox[{"li", ",", "0", ",", 
             RowBox[{"ii", "-", "1"}]}], "}"}]}], "]"}], ")"}]}], ")"}]}], 
     ",", 
     RowBox[{"{", 
      RowBox[{"ii", ",", "0", ",", "n"}], "}"}]}], "]"}]}]}]], "Input",
 CellChangeTimes->{{3.72145188313299*^9, 3.7214520293125153`*^9}, {
   3.721452654409964*^9, 3.7214529262030888`*^9}, {3.721452960218816*^9, 
   3.721453146313904*^9}, {3.721454186648013*^9, 3.721454195180797*^9}, 
   3.721455566973351*^9, {3.721462432203248*^9, 3.721462439802164*^9}, {
   3.721464046137562*^9, 3.7214640462360353`*^9}, {3.7221462711475163`*^9, 
   3.7221462755090218`*^9}, {3.722146828552949*^9, 3.722146854639701*^9}, {
   3.722146886490834*^9, 3.722146954399622*^9}, {3.722148664639679*^9, 
   3.722148807924111*^9}, {3.7221488611351557`*^9, 3.722148885694502*^9}, {
   3.7413137762894506`*^9, 3.74131379242767*^9}},
 ExpressionUUID -> "d8f71f73-3795-4d27-ac64-93c7ccc2e9c6"],

Cell["\<\
We then express the subtraction of the First integral of the Second part from \
the Second integral of the Second Part\
\>", "Text",
 CellChangeTimes->{{3.741313827545678*^9, 3.741313925002655*^9}, {
  3.741313991098235*^9, 3.741314006729919*^9}, {3.741314119338253*^9, 
  3.7413141361862392`*^9}, {3.741314186928789*^9, 
  3.7413141874189262`*^9}},ExpressionUUID->"1b686033-8371-4109-a22d-\
c8001602254c"],

Cell[BoxData[
 RowBox[{
  RowBox[{"Part2SecondminusFirst", "[", 
   RowBox[{"m_", ",", "n_"}], "]"}], ":=", 
  RowBox[{"2", 
   RowBox[{"Sum", "[", 
    RowBox[{
     RowBox[{"FullSimplify", "[", 
      RowBox[{
       RowBox[{"Binomial", "[", 
        RowBox[{
         RowBox[{"1", "+", 
          RowBox[{"2", "n"}]}], ",", "i"}], "]"}], 
       FractionBox[
        SuperscriptBox[
         RowBox[{"(", 
          RowBox[{"-", "1"}], ")"}], 
         RowBox[{"1", "-", "i"}]], 
        SuperscriptBox[
         RowBox[{"(", 
          RowBox[{"1", "+", "i"}], ")"}], "2"]], 
       RowBox[{"(", 
        RowBox[{"0", "-", 
         RowBox[{"Sum", "[", 
          RowBox[{
           RowBox[{
            RowBox[{"Binomial", "[", 
             RowBox[{
              RowBox[{"1", "+", "i"}], ",", "j"}], "]"}], 
            FractionBox[
             RowBox[{"1", "-", 
              SuperscriptBox[
               RowBox[{"(", 
                RowBox[{"-", "1"}], ")"}], 
               RowBox[{"1", "+", "i", "-", "j"}]]}], 
             RowBox[{"3", "+", 
              RowBox[{"2", 
               RowBox[{"(", 
                RowBox[{"m", "+", "n"}], ")"}]}], "-", "i", "+", "j"}]]}], 
           ",", 
           RowBox[{"{", 
            RowBox[{"j", ",", "0", ",", 
             RowBox[{"1", "+", "i"}]}], "}"}]}], "]"}], "+", 
         RowBox[{
          RowBox[{"(", 
           RowBox[{"1", "+", "i"}], ")"}], 
          RowBox[{"Sum", "[", 
           RowBox[{
            RowBox[{
             RowBox[{"Binomial", "[", 
              RowBox[{
               RowBox[{"2", "+", 
                RowBox[{"2", 
                 RowBox[{"(", 
                  RowBox[{"m", "+", "n"}], ")"}]}], "-", "i"}], ",", "j"}], 
              "]"}], 
             FractionBox[
              SuperscriptBox[
               RowBox[{"(", 
                RowBox[{"-", "1"}], ")"}], 
               RowBox[{
                RowBox[{"-", "i"}], "-", "j"}]], 
              SuperscriptBox[
               RowBox[{"(", 
                RowBox[{"2", "+", "i", "+", "j"}], ")"}], "2"]], 
             RowBox[{"(", 
              RowBox[{"0", "+", 
               RowBox[{
                SuperscriptBox["2", 
                 RowBox[{"2", "+", "i", "+", "j"}]], 
                RowBox[{"(", 
                 RowBox[{
                  RowBox[{"-", "1"}], "+", 
                  RowBox[{
                   RowBox[{"(", 
                    RowBox[{"i", "+", "j"}], ")"}], 
                   RowBox[{"Log", "[", "2", "]"}]}], "+", 
                  RowBox[{"Log", "[", "4", "]"}]}], ")"}]}]}], ")"}]}], ",", 
            RowBox[{"{", 
             RowBox[{"j", ",", "0", ",", 
              RowBox[{"2", "+", 
               RowBox[{"2", 
                RowBox[{"(", 
                 RowBox[{"m", "+", "n"}], ")"}]}], "-", "i"}]}], "}"}]}], 
           "]"}]}]}], ")"}]}], "]"}], ",", 
     RowBox[{"{", 
      RowBox[{"i", ",", "0", ",", 
       RowBox[{"1", "+", 
        RowBox[{"2", "n"}]}]}], "}"}]}], "]"}]}]}]], "Input",
 CellChangeTimes->{{3.722157391038197*^9, 3.7221574051564903`*^9}, {
  3.7221575539556417`*^9, 3.72215758174837*^9}, {3.722157691669528*^9, 
  3.7221577008553753`*^9}, {3.741314010027947*^9, 3.741314016125527*^9}},
 ExpressionUUID -> "bdab91bc-fbbb-4f53-95f4-a2edbf3be5c3"],

Cell["\<\
We then express the subtraction of the Fourth integral of the Second part \
from the Third integral of the Second Part\
\>", "Text",
 CellChangeTimes->{{3.741313827545678*^9, 3.741313925002655*^9}, {
  3.741314097156006*^9, 3.741314117770349*^9}, {3.74131419129032*^9, 
  3.741314191802169*^9}},ExpressionUUID->"39f8ce22-a906-480d-8790-\
c31a42632c49"],

Cell[BoxData[
 RowBox[{
  RowBox[{"Part2ThirdminusFourth", "[", 
   RowBox[{"m_", ",", "n_"}], "]"}], ":=", " ", 
  RowBox[{
   RowBox[{"Sum", "[", 
    RowBox[{
     RowBox[{
      FractionBox["1", 
       RowBox[{
        RowBox[{"2", "ip"}], "+", "1"}]], " ", 
      RowBox[{"Binomial", "[", 
       RowBox[{
        RowBox[{"1", "+", 
         RowBox[{"2", "n"}]}], ",", 
        RowBox[{"2", "ip"}]}], "]"}], 
      RowBox[{"(", 
       RowBox[{
        RowBox[{"2", 
         SuperscriptBox[
          RowBox[{"(", 
           RowBox[{"2", "\[Mu]"}], ")"}], 
          RowBox[{"1", "+", 
           RowBox[{"2", "ip"}]}]], 
         RowBox[{"(", 
          RowBox[{
           RowBox[{
            FractionBox[
             RowBox[{
              RowBox[{"(", 
               RowBox[{
                RowBox[{"2", "ip"}], "-", "1"}], ")"}], "!!"}], 
             SuperscriptBox["2", "ip"]], 
            FractionBox["1", 
             RowBox[{"3", "+", 
              RowBox[{"2", 
               RowBox[{"(", 
                RowBox[{"m", "+", "n", "-", "ip"}], ")"}]}]}]], 
            RowBox[{"(", 
             RowBox[{
              RowBox[{
               FractionBox[
                SqrtBox["\[Pi]"], "2"], 
               RowBox[{"(", 
                RowBox[{"Erf", "[", 
                 FractionBox["1", "\[Mu]"], "]"}], ")"}]}], "+", 
              RowBox[{
               FractionBox["1", 
                RowBox[{"2", "\[Mu]"}]], 
               RowBox[{"(", 
                RowBox[{
                 RowBox[{"Sum", "[", 
                  RowBox[{
                   RowBox[{
                    RowBox[{"Binomial", "[", 
                    RowBox[{
                    RowBox[{"3", "+", 
                    RowBox[{"2", 
                    RowBox[{"(", 
                    RowBox[{"m", "+", "n", "-", "ip"}], ")"}]}]}], ",", 
                    RowBox[{"2", "jp"}]}], "]"}], 
                    RowBox[{"Part", "[", 
                    RowBox[{
                    SubscriptBox["TableS", "even"], ",", 
                    RowBox[{"jp", "+", "1"}]}], "]"}]}], ",", 
                   RowBox[{"{", 
                    RowBox[{"jp", ",", "0", ",", 
                    RowBox[{"m", "+", "n", "-", "ip", "+", "1"}]}], "}"}]}], 
                  "]"}], "-", 
                 RowBox[{"Sum", "[", 
                  RowBox[{
                   RowBox[{
                    RowBox[{"Binomial", "[", 
                    RowBox[{
                    RowBox[{"3", "+", 
                    RowBox[{"2", 
                    RowBox[{"(", 
                    RowBox[{"m", "+", "n", "-", "ip"}], ")"}]}]}], ",", 
                    RowBox[{
                    RowBox[{"2", "ji"}], "+", "1"}]}], "]"}], 
                    RowBox[{"Part", "[", 
                    RowBox[{
                    SubscriptBox["TableS", "odd"], ",", 
                    RowBox[{"ji", "+", "1"}]}], "]"}]}], ",", 
                   RowBox[{"{", 
                    RowBox[{"ji", ",", "0", ",", 
                    RowBox[{"m", "+", "n", "-", "ip", "+", "1"}]}], "}"}]}], 
                  "]"}]}], ")"}]}]}], ")"}]}], "-", 
           RowBox[{"(", 
            RowBox[{"Sum", "[", 
             RowBox[{
              RowBox[{
               FractionBox["1", 
                SuperscriptBox["2", 
                 RowBox[{"lp", "+", "1"}]]], 
               FractionBox[
                RowBox[{
                 RowBox[{"(", 
                  RowBox[{
                   RowBox[{"2", "ip"}], "-", "1"}], ")"}], "!!"}], 
                RowBox[{
                 RowBox[{"(", 
                  RowBox[{
                   RowBox[{"2", "ip"}], "-", "1", "-", 
                   RowBox[{"2", "lp"}]}], ")"}], "!!"}]], 
               FractionBox["1", 
                SuperscriptBox[
                 RowBox[{"(", 
                  RowBox[{"2", "\[Mu]"}], ")"}], 
                 RowBox[{
                  RowBox[{"2", "ip"}], "-", "1", "-", 
                  RowBox[{"2", "lp"}]}]]], 
               RowBox[{"(", 
                RowBox[{
                 RowBox[{"Sum", "[", 
                  RowBox[{
                   RowBox[{
                    RowBox[{"Binomial", "[", 
                    RowBox[{
                    RowBox[{"2", "+", 
                    RowBox[{"2", 
                    RowBox[{"(", 
                    RowBox[{"m", "+", "n", "-", "ip"}], ")"}]}]}], ",", 
                    RowBox[{"2", "jp"}]}], "]"}], 
                    RowBox[{"Part", "[", 
                    RowBox[{
                    SubscriptBox["TableS", "odd"], ",", 
                    RowBox[{
                    "jp", "+", "ip", "-", "lp", "-", "1", "+", "1"}]}], 
                    "]"}]}], ",", 
                   RowBox[{"{", 
                    RowBox[{"jp", ",", "0", ",", 
                    RowBox[{"m", "+", "n", "-", "ip", "+", "1"}]}], "}"}]}], 
                  "]"}], "-", 
                 RowBox[{"Sum", "[", 
                  RowBox[{
                   RowBox[{
                    RowBox[{"Binomial", "[", 
                    RowBox[{
                    RowBox[{"2", "+", 
                    RowBox[{"2", 
                    RowBox[{"(", 
                    RowBox[{"m", "+", "n", "-", "ip"}], ")"}]}]}], ",", 
                    RowBox[{
                    RowBox[{"2", "ji"}], "+", "1"}]}], "]"}], 
                    RowBox[{"Part", "[", 
                    RowBox[{
                    SubscriptBox["TableS", "even"], ",", 
                    RowBox[{"ji", "+", "ip", "-", "lp", "+", "1"}]}], "]"}]}],
                    ",", 
                   RowBox[{"{", 
                    RowBox[{"ji", ",", "0", ",", 
                    RowBox[{"m", "+", "n", "-", "ip"}]}], "}"}]}], "]"}]}], 
                ")"}]}], ",", 
              RowBox[{"{", 
               RowBox[{"lp", ",", "0", ",", 
                RowBox[{"ip", "-", "1"}]}], "}"}]}], "]"}], ")"}]}], ")"}]}], 
        "-", 
        RowBox[{"(", 
         RowBox[{
          RowBox[{"Sum", "[", 
           RowBox[{
            RowBox[{
             RowBox[{"Binomial", "[", 
              RowBox[{
               RowBox[{"2", "+", 
                RowBox[{"2", 
                 RowBox[{"(", 
                  RowBox[{"m", "+", "n", "-", "ip"}], ")"}]}]}], ",", "j"}], 
              "]"}], 
             FractionBox[
              SuperscriptBox[
               RowBox[{"(", 
                RowBox[{"-", "1"}], ")"}], "j"], 
              RowBox[{"j", "+", 
               RowBox[{"2", "ip"}], "+", "2"}]], 
             RowBox[{"(", 
              RowBox[{
               SuperscriptBox["2", 
                RowBox[{"j", "+", 
                 RowBox[{"2", "ip"}], "+", "2"}]], 
               RowBox[{"ExpIntegralEi", "[", 
                RowBox[{"-", 
                 FractionBox["1", 
                  RowBox[{" ", 
                   SuperscriptBox["\[Mu]", "2"]}]]}], "]"}]}], ")"}]}], " ", 
            ",", 
            RowBox[{"{", 
             RowBox[{"j", ",", "0", ",", 
              RowBox[{"2", "+", 
               RowBox[{"2", 
                RowBox[{"(", 
                 RowBox[{"m", "+", "n", "-", "ip"}], ")"}]}]}]}], "}"}]}], 
           "]"}], "-", 
          RowBox[{"Sum", "[", 
           RowBox[{
            RowBox[{
             RowBox[{"Binomial", "[", 
              RowBox[{
               RowBox[{"2", "+", 
                RowBox[{"2", 
                 RowBox[{"(", 
                  RowBox[{"m", "+", "n", "-", "ip"}], ")"}]}]}], ",", 
               RowBox[{"2", "jp"}]}], "]"}], 
             FractionBox["2", 
              RowBox[{
               RowBox[{"2", "jp"}], "+", 
               RowBox[{"2", "ip"}], "+", "2"}]], 
             RowBox[{"Part", "[", 
              RowBox[{
               SubscriptBox["TableS", "odd"], ",", 
               RowBox[{"jp", "+", "ip", "+", "1"}]}], "]"}]}], ",", 
            RowBox[{"{", 
             RowBox[{"jp", ",", "0", ",", 
              RowBox[{"1", "+", "m", "+", "n", "-", "ip"}]}], "}"}]}], "]"}], 
          "+", 
          RowBox[{"Sum", "[", 
           RowBox[{
            RowBox[{
             RowBox[{"Binomial", "[", 
              RowBox[{
               RowBox[{"2", "+", 
                RowBox[{"2", 
                 RowBox[{"(", 
                  RowBox[{"m", "+", "n", "-", "ip"}], ")"}]}]}], ",", 
               RowBox[{
                RowBox[{"2", "ji"}], "+", "1"}]}], "]"}], 
             FractionBox["2", 
              RowBox[{
               RowBox[{"2", "ji"}], "+", 
               RowBox[{"2", "ip"}], "+", "3"}]], 
             RowBox[{"Part", "[", 
              RowBox[{
               SubscriptBox["TableS", "even"], ",", 
               RowBox[{"ji", "+", "ip", " ", "+", "1", "+", "1"}]}], "]"}]}], 
            ",", 
            RowBox[{"{", 
             RowBox[{"ji", ",", "0", ",", 
              RowBox[{"m", "+", "n", "-", "ip"}]}], "}"}]}], "]"}]}], ")"}]}],
        ")"}]}], ",", " ", 
     RowBox[{"{", 
      RowBox[{"ip", ",", "0", ",", "n"}], "}"}]}], "]"}], "-", 
   "                                                                          \
                         ", 
   RowBox[{"Sum", "[", 
    RowBox[{
     RowBox[{
      FractionBox["1", 
       RowBox[{
        RowBox[{"2", "ii"}], "+", "2"}]], 
      RowBox[{"Binomial", "[", 
       RowBox[{
        RowBox[{"1", "+", 
         RowBox[{"2", "n"}]}], ",", 
        RowBox[{
         RowBox[{"2", "ii"}], "+", "1"}]}], "]"}], 
      RowBox[{"(", 
       RowBox[{
        RowBox[{"2", 
         SuperscriptBox[
          RowBox[{"(", 
           RowBox[{"2", "\[Mu]"}], ")"}], 
          RowBox[{"2", "+", 
           RowBox[{"2", "ii"}]}]], 
         RowBox[{"(", 
          RowBox[{
           RowBox[{
            FractionBox[
             RowBox[{
              RowBox[{"(", 
               RowBox[{"2", "ii"}], ")"}], "!!"}], 
             SuperscriptBox["2", "ii"]], 
            RowBox[{"(", 
             RowBox[{"-", 
              FractionBox["1", "2"]}], ")"}], 
            RowBox[{"(", 
             RowBox[{
              RowBox[{"Sum", "[", 
               RowBox[{
                RowBox[{
                 RowBox[{"-", 
                  RowBox[{"Binomial", "[", 
                   RowBox[{
                    RowBox[{"1", "+", 
                    RowBox[{"2", 
                    RowBox[{"(", 
                    RowBox[{"m", "+", "n", "-", "ii"}], ")"}]}]}], ",", 
                    RowBox[{"2", "jp"}]}], "]"}]}], 
                 RowBox[{"Part", "[", 
                  RowBox[{
                   SubscriptBox["TableS", "even"], ",", 
                   RowBox[{"jp", "+", "1"}]}], "]"}]}], ",", 
                RowBox[{"{", 
                 RowBox[{"jp", ",", "0", ",", 
                  RowBox[{"m", "+", "n", "-", "ii"}]}], "}"}]}], "]"}], "+", 
              RowBox[{"Sum", "[", 
               RowBox[{
                RowBox[{
                 RowBox[{"Binomial", "[", 
                  RowBox[{
                   RowBox[{"1", "+", 
                    RowBox[{"2", 
                    RowBox[{"(", 
                    RowBox[{"m", "+", "n", "-", "ii"}], ")"}]}]}], ",", 
                   RowBox[{
                    RowBox[{"2", "ji"}], "+", "1"}]}], "]"}], 
                 RowBox[{"Part", "[", 
                  RowBox[{
                   SubscriptBox["TableS", "odd"], ",", 
                   RowBox[{"ji", "+", "1"}]}], "]"}]}], ",", 
                RowBox[{"{", 
                 RowBox[{"ji", ",", "0", ",", 
                  RowBox[{"m", "+", "n", "-", "ii"}]}], "}"}]}], "]"}]}], 
             ")"}]}], "-", "                            ", 
           RowBox[{"(", 
            RowBox[{"Sum", "[", 
             RowBox[{
              RowBox[{
               FractionBox["1", 
                SuperscriptBox["2", 
                 RowBox[{"li", "+", "1"}]]], 
               FractionBox[
                RowBox[{
                 RowBox[{"(", 
                  RowBox[{"2", "ii"}], ")"}], "!!"}], 
                RowBox[{
                 RowBox[{"(", 
                  RowBox[{
                   RowBox[{"2", "ii"}], "-", 
                   RowBox[{"2", "li"}]}], ")"}], "!!"}]], 
               FractionBox["1", 
                SuperscriptBox[
                 RowBox[{"(", 
                  RowBox[{"2", "\[Mu]"}], ")"}], 
                 RowBox[{
                  RowBox[{"2", "ii"}], "-", 
                  RowBox[{"2", "li"}]}]]], 
               RowBox[{"(", 
                RowBox[{
                 RowBox[{"-", 
                  RowBox[{"Sum", "[", 
                   RowBox[{
                    RowBox[{
                    RowBox[{"Binomial", "[", 
                    RowBox[{
                    RowBox[{"1", "+", 
                    RowBox[{"2", 
                    RowBox[{"(", 
                    RowBox[{"m", "+", "n", "-", "ii"}], ")"}]}]}], ",", 
                    RowBox[{"2", "jp"}]}], "]"}], 
                    RowBox[{"Part", "[", 
                    RowBox[{
                    SubscriptBox["TableS", "even"], ",", 
                    RowBox[{"jp", "+", "ii", "-", "li", "+", "1"}]}], "]"}]}],
                     ",", 
                    RowBox[{"{", 
                    RowBox[{"jp", ",", "0", ",", 
                    RowBox[{"m", "+", "n", "-", "ii", "+", "1"}]}], "}"}]}], 
                   "]"}]}], "+", 
                 RowBox[{"Sum", "[", 
                  RowBox[{
                   RowBox[{
                    RowBox[{"Binomial", "[", 
                    RowBox[{
                    RowBox[{"1", "+", 
                    RowBox[{"2", 
                    RowBox[{"(", 
                    RowBox[{"m", "+", "n", "-", "ii"}], ")"}]}]}], ",", 
                    RowBox[{
                    RowBox[{"2", "ji"}], "+", "1"}]}], "]"}], 
                    RowBox[{"Part", "[", 
                    RowBox[{
                    SubscriptBox["TableS", "odd"], ",", 
                    RowBox[{"ji", "+", "ii", "-", "li", "+", "1"}]}], "]"}]}],
                    ",", 
                   RowBox[{"{", 
                    RowBox[{"ji", ",", "0", ",", 
                    RowBox[{"m", "+", "n", "-", "ii"}]}], "}"}]}], "]"}]}], 
                ")"}]}], ",", 
              RowBox[{"{", 
               RowBox[{"li", ",", "0", ",", 
                RowBox[{"ii", "-", "1"}]}], "}"}]}], "]"}], ")"}]}], ")"}]}], 
        "-", 
        RowBox[{"(", 
         RowBox[{
          RowBox[{"Sum", "[", 
           RowBox[{
            RowBox[{
             RowBox[{"Binomial", "[", 
              RowBox[{
               RowBox[{"1", "+", 
                RowBox[{"2", 
                 RowBox[{"(", 
                  RowBox[{"m", "+", "n", "-", "ii"}], ")"}]}]}], ",", "j"}], 
              "]"}], 
             FractionBox[
              SuperscriptBox[
               RowBox[{"(", 
                RowBox[{"-", "1"}], ")"}], 
               RowBox[{"1", "-", "j"}]], 
              RowBox[{"j", "+", 
               RowBox[{"2", "ii"}], "+", "3"}]], 
             RowBox[{"(", 
              RowBox[{
               SuperscriptBox["2", 
                RowBox[{"j", "+", 
                 RowBox[{"2", "ii"}], "+", "3"}]], 
               RowBox[{"ExpIntegralEi", "[", 
                RowBox[{"-", 
                 FractionBox["1", 
                  RowBox[{" ", 
                   SuperscriptBox["\[Mu]", "2"]}]]}], "]"}]}], ")"}]}], " ", 
            ",", 
            RowBox[{"{", 
             RowBox[{"j", ",", "0", ",", 
              RowBox[{"1", "+", 
               RowBox[{"2", 
                RowBox[{"(", 
                 RowBox[{"m", "+", "n", "-", "ii"}], ")"}]}]}]}], "}"}]}], 
           "]"}], "+", 
          RowBox[{"Sum", "[", 
           RowBox[{
            RowBox[{
             RowBox[{"Binomial", "[", 
              RowBox[{
               RowBox[{"1", "+", 
                RowBox[{"2", 
                 RowBox[{"(", 
                  RowBox[{"m", "+", "n", "-", "ii"}], ")"}]}]}], ",", 
               RowBox[{"2", "jp"}]}], "]"}], 
             FractionBox["2", 
              RowBox[{
               RowBox[{"2", "jp"}], "+", 
               RowBox[{"2", "ii"}], "+", "3"}]], 
             RowBox[{"Part", "[", 
              RowBox[{
               SubscriptBox["TableS", "even"], ",", 
               RowBox[{"jp", "+", "ii", "+", "1", "+", "1"}]}], "]"}]}], ",", 
            
            RowBox[{"{", 
             RowBox[{"jp", ",", "0", ",", 
              RowBox[{"m", "+", "n", "-", "ii"}]}], "}"}]}], "]"}], "-", 
          RowBox[{"Sum", "[", 
           RowBox[{
            RowBox[{
             RowBox[{"Binomial", "[", 
              RowBox[{
               RowBox[{"1", "+", 
                RowBox[{"2", 
                 RowBox[{"(", 
                  RowBox[{"m", "+", "n", "-", "ii"}], ")"}]}]}], ",", 
               RowBox[{
                RowBox[{"2", "ji"}], "+", "1"}]}], "]"}], 
             FractionBox["2", 
              RowBox[{
               RowBox[{"2", "ji"}], "+", 
               RowBox[{"2", "ii"}], "+", "4"}]], 
             RowBox[{"Part", "[", 
              RowBox[{
               SubscriptBox["TableS", "odd"], ",", 
               RowBox[{"ji", "+", "ii", "+", "1", "+", "1"}]}], "]"}]}], ",", 
            
            RowBox[{"{", 
             RowBox[{"ji", ",", "0", ",", 
              RowBox[{"m", "+", "n", "-", "ii"}]}], "}"}]}], "]"}]}], ")"}]}],
        ")"}]}], ",", 
     RowBox[{"{", 
      RowBox[{"ii", ",", "0", ",", "n"}], "}"}]}], "]"}]}]}]], "Input",
 CellChangeTimes->{{3.72145188313299*^9, 3.7214520293125153`*^9}, {
   3.721452654409964*^9, 3.7214529262030888`*^9}, {3.721452960218816*^9, 
   3.721453146313904*^9}, {3.721454186648013*^9, 3.721454195180797*^9}, 
   3.721455566973351*^9, {3.721462432203248*^9, 3.721462439802164*^9}, {
   3.721464046137562*^9, 3.7214640462360353`*^9}, {3.721643928199654*^9, 
   3.72164392827938*^9}, {3.721646193972369*^9, 3.721646194758437*^9}, {
   3.7216462276590443`*^9, 3.721646264752104*^9}, {3.721646355483562*^9, 
   3.7216463567537537`*^9}, {3.721646440560555*^9, 3.721646674633954*^9}, {
   3.721646706831491*^9, 3.721646801874136*^9}, {3.721646866739175*^9, 
   3.721647092732327*^9}, {3.72170676848381*^9, 3.721706771429459*^9}, {
   3.721706827179264*^9, 3.7217068299965067`*^9}, {3.7217119098933687`*^9, 
   3.721712042282798*^9}, 3.7217121637007093`*^9, {3.7217121958564863`*^9, 
   3.721712330674097*^9}, {3.721713638480556*^9, 3.721713650143136*^9}, {
   3.72171371859853*^9, 3.7217137802952213`*^9}, {3.721713816381413*^9, 
   3.721713829652701*^9}, 3.72171681034828*^9, 3.721718191953271*^9, {
   3.722155926764591*^9, 3.7221559720503883`*^9}, {3.7221560348537493`*^9, 
   3.7221560559049797`*^9}, {3.7221561169198027`*^9, 
   3.7221561252616873`*^9}, {3.722156167070784*^9, 3.7221562509153976`*^9}, {
   3.722156569925638*^9, 3.722156651593007*^9}, {3.722156707587171*^9, 
   3.72215671754095*^9}, {3.741314083792276*^9, 3.7413140911476107`*^9}},
 ExpressionUUID -> "b35aed36-3a1d-44c7-b6fa-32102d91f4dc"]
}, Closed]]
}, Closed]],

Cell[CellGroupData[{

Cell["Tables of the general coefficients of the Pad\[EAcute] approximant ", \
"Subsection",
 CellChangeTimes->{
  3.741315111053999*^9, {3.7413153603955517`*^9, 3.741315376811513*^9}, 
   3.741318588576071*^9, {3.741335007211803*^9, 
   3.741335011546761*^9}},ExpressionUUID->"bd68f630-76bb-4a25-9644-\
9fc7f10c4e93"],

Cell["\<\
We prepare the general resolution of the diagonal Pad\[EAcute] approximant\
\>", "Text",
 CellChangeTimes->{{3.7227556865784073`*^9, 3.722755701562633*^9}, {
  3.741165367529112*^9, 3.741165369883627*^9}, {3.741315385483111*^9, 
  3.741315385644908*^9}},ExpressionUUID->"7c42b86e-26e9-47a6-92ec-\
f5ece51c6f10"],

Cell[BoxData[
 RowBox[{
  RowBox[{"MatrixPad\[EAcute]", "[", "M_", "]"}], ":=", 
  RowBox[{"Table", "[", 
   RowBox[{
    RowBox[{"If", "[", 
     RowBox[{
      RowBox[{
       RowBox[{"Mod", "[", 
        RowBox[{
         RowBox[{"M", "+", "i", "-", "j"}], ",", "2"}], "]"}], "==", "0"}], 
      ",", 
      SubscriptBox["T", 
       RowBox[{"M", "+", "i", "-", "j"}]], ",", "0"}], "]"}], ",", 
    RowBox[{"{", 
     RowBox[{"i", ",", "1", ",", "M"}], "}"}], ",", 
    RowBox[{"{", 
     RowBox[{"j", ",", "1", ",", "M"}], "}"}]}], "]"}]}]], "Input",
 CellChangeTimes->{{3.72267953909367*^9, 3.722679542375702*^9}, {
  3.722679765368495*^9, 3.7226797807266893`*^9}, {3.7226798516544647`*^9, 
  3.722679851774665*^9}, {3.7227500097990103`*^9, 3.7227500156697617`*^9}, {
  3.722750055416525*^9, 3.7227500943256207`*^9}, {3.741315195900532*^9, 
  3.741315200764884*^9}},
 ExpressionUUID -> "c813af06-04bc-4770-b7b2-921ac560ee97"],

Cell[BoxData[
 RowBox[{
  RowBox[{"ColumnPad\[EAcute]", "[", "M_", "]"}], ":=", 
  RowBox[{"Table", "[", 
   RowBox[{
    RowBox[{"If", "[", 
     RowBox[{
      RowBox[{
       RowBox[{"Mod", "[", 
        RowBox[{
         RowBox[{"M", "+", "i"}], ",", "2"}], "]"}], "==", "0"}], ",", 
      SubscriptBox["T", 
       RowBox[{"M", "+", "i"}]], ",", "0"}], "]"}], ",", 
    RowBox[{"{", 
     RowBox[{"i", ",", "1", ",", "M"}], "}"}]}], "]"}]}]], "Input",
 CellChangeTimes->{{3.722676136666432*^9, 3.722676173595167*^9}, {
  3.722750173053117*^9, 3.722750186917301*^9}, {3.741315203677578*^9, 
  3.741315205723914*^9}},
 ExpressionUUID -> "fd2294a4-4954-4e86-9d56-7f1938dc4e7f"],

Cell[BoxData[
 RowBox[{
  RowBox[{"SolutionBPad\[EAcute]", "[", "M_", "]"}], ":=", 
  RowBox[{"-", 
   RowBox[{"Simplify", "[", 
    RowBox[{
     RowBox[{"Inverse", " ", "[", 
      RowBox[{"MatrixPad\[EAcute]", "[", "M", "]"}], "]"}], ".", 
     RowBox[{"ColumnPad\[EAcute]", "[", "M", "]"}]}], "]"}]}]}]], "Input",
 CellChangeTimes->{
  3.722755923324892*^9, {3.741315215068181*^9, 3.741315224011672*^9}, {
   3.741315676923102*^9, 3.7413156774846373`*^9}},
 ExpressionUUID -> "8d1fa17a-1a32-4f76-bf07-8de145f4eecf"],

Cell[BoxData[
 RowBox[{
  RowBox[{"CoefBPad\[EAcute]", "[", "M_", "]"}], ":=", 
  RowBox[{"Table", "[", 
   RowBox[{
    RowBox[{"If", "[", 
     RowBox[{
      RowBox[{
       RowBox[{"Mod", "[", 
        RowBox[{"i", ",", "2"}], "]"}], "\[Equal]", "0"}], ",", 
      RowBox[{"SolutionBPad\[EAcute]", "[", "i", "]"}], ",", "0"}], "]"}], 
    ",", 
    RowBox[{"{", 
     RowBox[{"i", ",", "1", ",", "M"}], "}"}]}], "]"}]}]], "Input",
 CellChangeTimes->{{3.722676592891827*^9, 3.722676593115856*^9}, 
   3.722750266723699*^9, {3.7227503637187366`*^9, 3.7227504461137543`*^9}, {
   3.7227508889799843`*^9, 3.722750889735475*^9}, {3.722751743028767*^9, 
   3.722751763715478*^9}, {3.722751829730443*^9, 3.7227518388336906`*^9}, {
   3.722752280737562*^9, 3.7227523110731087`*^9}, {3.722752871566914*^9, 
   3.722752901967402*^9}, {3.722753077680962*^9, 3.722753151149047*^9}, {
   3.722753643391568*^9, 3.722753645790571*^9}, {3.7227538118255043`*^9, 
   3.7227538536789837`*^9}, {3.741315232540187*^9, 3.741315235355875*^9}, {
   3.741315666716778*^9, 3.7413156848773947`*^9}},
 ExpressionUUID -> "502dab36-1868-456e-a408-57afd53c357a"],

Cell[BoxData[
 RowBox[{
  RowBox[{"SolutionAPad\[EAcute]", "[", "M_", "]"}], ":=", 
  RowBox[{"Table", "[", 
   RowBox[{
    RowBox[{"Simplify", "[", 
     RowBox[{"(", 
      RowBox[{
       SubscriptBox["T", "k"], "+", 
       RowBox[{"Sum", "[", 
        RowBox[{
         RowBox[{
          SubscriptBox["T", 
           RowBox[{"k", "-", "j"}]], 
          RowBox[{"Part", "[", 
           RowBox[{
            RowBox[{"CoefBPad\[EAcute]", "[", "M", "]"}], ",", "M", ",", 
            "j"}], "]"}]}], ",", 
         RowBox[{"{", 
          RowBox[{"j", ",", "1", ",", "k"}], "}"}]}], "]"}]}], ")"}], "]"}], 
    ",", 
    RowBox[{"{", 
     RowBox[{"k", ",", "0", ",", "M"}], "}"}]}], "]"}]}]], "Input",
 CellChangeTimes->{{3.722753262897891*^9, 3.722753297665489*^9}, {
  3.722753341808571*^9, 3.722753342094528*^9}, {3.722753431694509*^9, 
  3.72275343278249*^9}, {3.722753931647711*^9, 3.722753955296125*^9}, {
  3.722754227039239*^9, 3.722754229887331*^9}, {3.722756015485976*^9, 
  3.7227560180426693`*^9}, {3.722768908946848*^9, 3.7227689104316797`*^9}, {
  3.741315245516918*^9, 3.7413152472129097`*^9}, {3.741315679453515*^9, 
  3.7413156897584467`*^9}},
 ExpressionUUID -> "0e49ba41-0291-4592-8c5b-a2fdd1e831c7"],

Cell[BoxData[
 RowBox[{
  RowBox[{"CoefAPad\[EAcute]", "[", "M_", "]"}], ":=", 
  RowBox[{"Table", "[", 
   RowBox[{
    RowBox[{"If", "[", 
     RowBox[{
      RowBox[{
       RowBox[{"Mod", "[", 
        RowBox[{"i", ",", "2"}], "]"}], "\[Equal]", "0"}], ",", 
      RowBox[{"SolutionAPad\[EAcute]", "[", "i", "]"}], ",", "0"}], "]"}], 
    ",", 
    RowBox[{"{", 
     RowBox[{"i", ",", "1", ",", "M"}], "}"}]}], "]"}]}]], "Input",
 CellChangeTimes->{{3.722753998174238*^9, 3.722754024926609*^9}, {
  3.722766550502486*^9, 3.722766551306336*^9}, {3.7413152497408752`*^9, 
  3.7413152504446793`*^9}, {3.741315670284986*^9, 3.7413156933408213`*^9}},
 ExpressionUUID -> "90358802-4407-459e-be13-fea2102244ce"]
}, Closed]]
}, Closed]],

Cell[CellGroupData[{

Cell["\<\
Relativistic short-range Coulomb exchange energy per particle\
\>", "Section",
 CellChangeTimes->{{3.741163258537374*^9, 3.741163260080551*^9}, {
  3.741164011085541*^9, 3.741164011830337*^9}, {3.7413127114487133`*^9, 
  3.741312714344654*^9}, {3.741318634512967*^9, 3.7413186346724453`*^9}, {
  3.741335105035335*^9, 
  3.741335111803047*^9}},ExpressionUUID->"42c72d06-0525-46d6-89f8-\
9b91f3b11cf2"],

Cell[CellGroupData[{

Cell["General expressions of the energy", "Subsection",
 CellChangeTimes->{{3.74116431193472*^9, 3.741164315937715*^9}, {
  3.7413126994963493`*^9, 3.7413127203925047`*^9}},
 ExpressionUUID -> "cb4602cb-e1a4-4a24-82d8-495045542c07"],

Cell["\<\
The expression of the relativistic full-range exchange energy per particle \
for the Coulomb interaction potential is\
\>", "Text",
 CellChangeTimes->{{3.741312221879962*^9, 3.741312269736453*^9}, {
  3.741335132523316*^9, 3.741335134171356*^9}, {3.741407812800604*^9, 
  3.741407817135066*^9}},
 ExpressionUUID -> "86a7ecd8-b29a-45f5-9d90-7ff2593b7558"],

Cell[BoxData[
 RowBox[{
  RowBox[{"ExRC", "=", 
   RowBox[{
    RowBox[{"-", 
     FractionBox[
      RowBox[{"3", " ", "kF", " "}], 
      RowBox[{"4", " ", "\[Pi]"}]]}], 
    RowBox[{"(", 
     RowBox[{
      FractionBox["5", "6"], "+", 
      FractionBox[
       SuperscriptBox["c", "2"], "3"], "+", 
      RowBox[{
       FractionBox["2", "3"], " ", 
       SqrtBox[
        RowBox[{"1", "+", 
         FractionBox["1", 
          SuperscriptBox["c", "2"]]}]], " ", "c", " ", 
       RowBox[{"ArcSinh", "[", 
        FractionBox["1", "c"], "]"}]}], "-", 
      RowBox[{
       FractionBox["1", "2"], " ", 
       SuperscriptBox[
        RowBox[{"(", 
         RowBox[{
          RowBox[{
           SqrtBox[
            RowBox[{"1", "+", 
             FractionBox["1", 
              SuperscriptBox["c", "2"]]}]], " ", "c"}], "-", 
          RowBox[{
           SuperscriptBox["c", "2"], " ", 
           RowBox[{"ArcSinh", "[", 
            FractionBox["1", "c"], "]"}]}]}], ")"}], "2"]}], "-", 
      RowBox[{
       FractionBox["2", "3"], " ", 
       SuperscriptBox[
        RowBox[{"(", 
         RowBox[{"1", "+", 
          FractionBox["1", 
           SuperscriptBox["c", "2"]]}], ")"}], "2"], " ", 
       SuperscriptBox["c", "4"], " ", 
       RowBox[{"Log", "[", 
        SqrtBox[
         RowBox[{"1", "+", 
          FractionBox["1", 
           SuperscriptBox["c", "2"]]}]], "]"}]}]}], ")"}]}]}], ";"}]], "Input",\

 CellChangeTimes->{{3.7191233323485947`*^9, 3.719123354257957*^9}, {
   3.7191333462516327`*^9, 3.719133346586507*^9}, 3.719206123103397*^9, {
   3.741163278291253*^9, 3.741163297605877*^9}, 3.741164059325994*^9, {
   3.741312056731365*^9, 3.7413120923784237`*^9}, 3.74131220922822*^9, {
   3.7413122954352703`*^9, 3.741312295818676*^9}, 3.741313073294773*^9},
 ExpressionUUID -> "818b68b6-8af9-49b8-9533-7898a84d3459"],

Cell["\<\
The relativistic short-range exchange energy per particle for the Coulomb \
interaction potential can be calculated through numerical integration using\
\>", "Text",
 CellChangeTimes->{{3.741312281128374*^9, 3.741312335545431*^9}, {
   3.741312671624989*^9, 3.7413126773038692`*^9}, {3.741407822295622*^9, 
   3.741407826103919*^9}, 3.741407867392549*^9}],

Cell[BoxData[
 RowBox[{
  RowBox[{"ExRCsr", "[", 
   RowBox[{"\[Mu]_", ",", "c_"}], "]"}], ":=", " ", 
  RowBox[{
   RowBox[{"NIntegrate", "[", 
    RowBox[{
     RowBox[{
      FractionBox["1", 
       RowBox[{"16", " ", 
        SqrtBox[
         RowBox[{
          RowBox[{"(", 
           RowBox[{
            SuperscriptBox["c", "2"], "+", 
            SuperscriptBox["k1", "2"]}], ")"}], " ", 
          RowBox[{"(", 
           RowBox[{
            SuperscriptBox["c", "2"], "+", 
            SuperscriptBox["k2", "2"]}], ")"}]}]], " ", "\[Pi]"}]], "3", " ", 
      "k1", " ", "k2", " ", "kF", " ", 
      RowBox[{"(", 
       RowBox[{
        RowBox[{"4", " ", "k1", " ", "k2"}], "+", 
        RowBox[{"4", " ", 
         RowBox[{"(", 
          RowBox[{
           RowBox[{"-", 
            SuperscriptBox["\[ExponentialE]", 
             RowBox[{"-", 
              FractionBox[
               SuperscriptBox[
                RowBox[{"(", 
                 RowBox[{"k1", "-", "k2"}], ")"}], "2"], 
               RowBox[{"4", " ", 
                SuperscriptBox["\[Mu]", "2"]}]]}]]}], "+", 
           SuperscriptBox["\[ExponentialE]", 
            RowBox[{"-", 
             FractionBox[
              SuperscriptBox[
               RowBox[{"(", 
                RowBox[{"k1", "+", "k2"}], ")"}], "2"], 
              RowBox[{"4", " ", 
               SuperscriptBox["\[Mu]", "2"]}]]}]]}], ")"}], " ", 
         SuperscriptBox["\[Mu]", "2"]}], "-", 
        RowBox[{
         RowBox[{"(", 
          RowBox[{
           RowBox[{"2", " ", 
            SuperscriptBox["c", "2"]}], "+", 
           SuperscriptBox["k1", "2"], "+", 
           SuperscriptBox["k2", "2"], "+", 
           RowBox[{"2", " ", 
            SqrtBox[
             RowBox[{
              RowBox[{"(", 
               RowBox[{
                SuperscriptBox["c", "2"], "+", 
                SuperscriptBox["k1", "2"]}], ")"}], " ", 
              RowBox[{"(", 
               RowBox[{
                SuperscriptBox["c", "2"], "+", 
                SuperscriptBox["k2", "2"]}], ")"}]}]]}]}], ")"}], " ", 
         RowBox[{"(", 
          RowBox[{
           RowBox[{"ExpIntegralEi", "[", 
            RowBox[{"-", 
             FractionBox[
              SuperscriptBox[
               RowBox[{"(", 
                RowBox[{"k1", "-", "k2"}], ")"}], "2"], 
              RowBox[{"4", " ", 
               SuperscriptBox["\[Mu]", "2"]}]]}], "]"}], "-", 
           RowBox[{"ExpIntegralEi", "[", 
            RowBox[{"-", 
             FractionBox[
              SuperscriptBox[
               RowBox[{"(", 
                RowBox[{"k1", "+", "k2"}], ")"}], "2"], 
              RowBox[{"4", " ", 
               SuperscriptBox["\[Mu]", "2"]}]]}], "]"}], "-", 
           RowBox[{"Log", "[", 
            SuperscriptBox[
             RowBox[{"(", 
              RowBox[{"k1", "-", "k2"}], ")"}], "2"], "]"}], "+", 
           RowBox[{"2", " ", 
            RowBox[{"Log", "[", 
             RowBox[{"k1", "+", "k2"}], "]"}]}]}], ")"}]}]}], ")"}]}], ",", 
     RowBox[{"{", 
      RowBox[{"k1", ",", "0", ",", "1"}], "}"}], ",", 
     RowBox[{"{", 
      RowBox[{"k2", ",", "0", ",", "1"}], "}"}], ",", 
     RowBox[{"Method", "\[Rule]", 
      RowBox[{"{", 
       RowBox[{"\"\<GlobalAdaptive\>\"", ",", 
        RowBox[{"\"\<MaxErrorIncreases\>\"", "\[Rule]", "2000"}]}], "}"}]}], 
     ",", 
     RowBox[{"WorkingPrecision", "\[Rule]", "8"}]}], "]"}], "//", 
   "Quiet"}]}]], "Input",
 CellChangeTimes->{{3.701145681788294*^9, 3.7011457077245607`*^9}, {
   3.7011457387970448`*^9, 3.701145742715835*^9}, {3.701145838955688*^9, 
   3.701145864971176*^9}, {3.701145973723259*^9, 3.701145997658729*^9}, 
   3.701146056572063*^9, {3.701146107515278*^9, 3.701146121611495*^9}, {
   3.701146196843637*^9, 3.701146247866346*^9}, {3.701146312635221*^9, 
   3.701146375081807*^9}, {3.7011464264741697`*^9, 3.701146477657305*^9}, {
   3.701146583432921*^9, 3.7011465958422613`*^9}, {3.701146635256982*^9, 
   3.701146673336335*^9}, {3.7011471055597353`*^9, 3.70114712658249*^9}, {
   3.701147399749424*^9, 3.701147402949328*^9}, {3.701147490165003*^9, 
   3.701147559316208*^9}, {3.701147589652295*^9, 3.70114760658006*^9}, {
   3.701147762259828*^9, 3.701147764355604*^9}, {3.701148064721983*^9, 
   3.701148067649757*^9}, {3.701148188946526*^9, 3.7011482124492397`*^9}, {
   3.7011483018407917`*^9, 3.701148396496244*^9}, {3.7011484538239727`*^9, 
   3.7011484901597433`*^9}, 3.7011485487194843`*^9, 3.701148617247799*^9, {
   3.701148653359206*^9, 3.70114865593461*^9}, {3.701148686398691*^9, 
   3.701148686638567*^9}, {3.7011492174203663`*^9, 3.701149217484399*^9}, 
   3.703923968822303*^9, 3.70392400506175*^9, {3.7039240660390387`*^9, 
   3.703924077057626*^9}, 3.703924120324793*^9, 3.7039244524507217`*^9, {
   3.703924650531103*^9, 3.7039246519228373`*^9}, {3.706590014367525*^9, 
   3.706590016210148*^9}, {3.714289166465165*^9, 3.714289168351822*^9}, {
   3.7177498205374203`*^9, 3.717749842137086*^9}, {3.717751156491482*^9, 
   3.717751186824505*^9}, {3.717751246744615*^9, 3.717751480920171*^9}, {
   3.717751518361574*^9, 3.7177515280449133`*^9}, {3.717751613705089*^9, 
   3.7177516876773376`*^9}, 3.7177517201526127`*^9, {3.717751803459509*^9, 
   3.7177518054711514`*^9}, {3.717752264568583*^9, 3.7177522695631037`*^9}, 
   3.717753253914151*^9, 3.717821459452956*^9, {3.7181908060799026`*^9, 
   3.718190806213161*^9}, 3.718190982122443*^9, {3.718191793953211*^9, 
   3.718191819001253*^9}, 3.718193884654935*^9, {3.718194736362905*^9, 
   3.718194737316622*^9}, 3.718779040850235*^9, {3.719032398425578*^9, 
   3.719032400770814*^9}, {3.719118906710697*^9, 3.719118917476943*^9}, 
   3.719121597767376*^9, {3.719121653871307*^9, 3.719121682857985*^9}, {
   3.719121726918955*^9, 3.719121730672037*^9}, 3.741163512479328*^9, 
   3.741163642224904*^9, {3.741312059418722*^9, 3.741312060146904*^9}, {
   3.741312287467168*^9, 3.741312298541902*^9}, 3.741313077581509*^9},
 ExpressionUUID -> "1ac1fba6-f4b4-446b-90bb-31468fe3fb76"]
}, Closed]],

Cell[CellGroupData[{

Cell["Calculation of the large-c expansion and Pad\[EAcute] approximant", \
"Subsection",
 CellChangeTimes->{{3.722158370784416*^9, 3.722158376544992*^9}, 
   3.740375873100111*^9, {3.741335552412428*^9, 
   3.7413355615003557`*^9}},ExpressionUUID->"4f889624-928f-4ed6-a4d6-\
4754ad1645ed"],

Cell[CellGroupData[{

Cell["Tables of the expansion coefficients", "Subsubsection",
 CellChangeTimes->{{3.741164766995187*^9, 3.741164769226877*^9}, {
  3.741164800614396*^9, 3.741164808695251*^9}, {3.7411649271723413`*^9, 
  3.741164931300631*^9}},
 ExpressionUUID -> "e1261da4-e649-4ce6-b540-e1b98bee379c"],

Cell["\<\
We need first to consider and stock in matrix forms the coefficients which \
take part in the First Part of the exchange energy \
\>", "Text",
 CellChangeTimes->{{3.722158424609398*^9, 3.722158432240468*^9}, {
  3.741312800410178*^9, 3.741312967528989*^9}, {3.7413130008901443`*^9, 
  3.741313016467299*^9}, {3.741315945243114*^9, 
  3.741315948620363*^9}},ExpressionUUID->"9b328790-2cfb-4c9c-8e45-\
4bbed356410a"],

Cell[BoxData[
 RowBox[{
  RowBox[{"Coef1Csr", "[", 
   RowBox[{"M_", ",", "n_"}], "]"}], ":=", 
  RowBox[{"FullSimplify", "[", 
   RowBox[{"Coefficient", "[", 
    RowBox[{
     RowBox[{"(", 
      RowBox[{
       RowBox[{"Coefficient", "[", 
        RowBox[{
         RowBox[{"Series", "[", 
          RowBox[{
           FractionBox[
            SuperscriptBox["x", "2"], 
            RowBox[{" ", 
             RowBox[{
              SqrtBox[
               RowBox[{
                RowBox[{"(", 
                 RowBox[{"1", "+", 
                  RowBox[{
                   SuperscriptBox["x", "2"], " ", 
                   SuperscriptBox["k1", "2"]}]}], ")"}], " "}]], 
              SqrtBox[
               RowBox[{
                RowBox[{"(", 
                 RowBox[{"1", "+", 
                  RowBox[{
                   SuperscriptBox["x", "2"], " ", 
                   SuperscriptBox["k2", "2"]}]}], ")"}], " "}]], " "}]}]], 
           ",", 
           RowBox[{"{", 
            RowBox[{"x", ",", "0", ",", "M"}], "}"}]}], "]"}], ",", "x", ",", 
         "M"}], "]"}], "/.", 
       RowBox[{"{", 
        RowBox[{"k2", "\[Rule]", "1"}], "}"}]}], ")"}], ",", "k1", ",", "n"}],
     "]"}], "]"}]}]], "Input",
 CellChangeTimes->{{3.741067468632078*^9, 3.741067469775463*^9}, {
   3.741164676901334*^9, 3.741164680855814*^9}, {3.7411651769392443`*^9, 
   3.7411651785144653`*^9}, 3.741165729269765*^9, {3.741312742954957*^9, 
   3.7413127678181543`*^9}},
 ExpressionUUID -> "49516a0d-7570-49f3-8f6f-cc49b839e270"],

Cell[BoxData[
 RowBox[{
  RowBox[{"Coef1Csr", "=", 
   RowBox[{"Table", "[", 
    RowBox[{
     RowBox[{"Coef1Csr", "[", 
      RowBox[{
       RowBox[{"2", "i"}], ",", 
       RowBox[{"2", "j"}]}], "]"}], ",", 
     RowBox[{"{", 
      RowBox[{"i", ",", "0", ",", "10"}], "}"}], ",", 
     RowBox[{"{", 
      RowBox[{"j", ",", "0", ",", "10"}], "}"}]}], "]"}]}], ";"}]], "Input",
 CellChangeTimes->{{3.7220573274031277`*^9, 3.722057411958555*^9}, {
   3.722057553909235*^9, 3.722057558258687*^9}, 3.722058361827209*^9, {
   3.722059020563114*^9, 3.722059036001809*^9}, {3.722064043326339*^9, 
   3.7220640436134567`*^9}, {3.722068938617219*^9, 3.7220689488567133`*^9}, 
   3.7220690691792727`*^9, {3.722069129642337*^9, 3.722069129865574*^9}, {
   3.72207100528871*^9, 3.7220711073354273`*^9}, {3.72207151536589*^9, 
   3.722071516470203*^9}, {3.722071548694812*^9, 3.7220715507900457`*^9}, {
   3.722158613895567*^9, 3.7221586159691896`*^9}, {3.72215876562182*^9, 
   3.722158767779505*^9}, {3.740299010870399*^9, 3.740299012550469*^9}, {
   3.740299522922635*^9, 3.740299529194179*^9}, {3.740299573786133*^9, 
   3.7402995759288683`*^9}, {3.7402999926019487`*^9, 3.7402999947622147`*^9}, 
   3.740363775166651*^9, {3.74036395318329*^9, 3.740363953270483*^9}, {
   3.7410679449531727`*^9, 3.741067948530664*^9}, {3.7411646834503117`*^9, 
   3.74116468587321*^9}, {3.741165179680643*^9, 3.741165181922716*^9}, {
   3.74116573241179*^9, 3.741165736966127*^9}, {3.741312754730145*^9, 
   3.741312771899719*^9}},
 ExpressionUUID -> "52408072-9114-4f50-97c0-7b4856233421"],

Cell["\<\
and then consider and stock in matrix forms the coefficients which take part \
in the Second Part of the exchange energy \
\>", "Text",
 CellChangeTimes->{{3.7221584371697073`*^9, 3.7221584415565367`*^9}, {
  3.741313026071665*^9, 3.7413130337851467`*^9}, {3.7413159401083517`*^9, 
  3.741315942972286*^9}}],

Cell[BoxData[
 RowBox[{
  RowBox[{"Coef2Csr", "[", 
   RowBox[{"M_", ",", "n_"}], "]"}], ":=", 
  RowBox[{"FullSimplify", "[", 
   RowBox[{"Coefficient", "[", 
    RowBox[{
     RowBox[{"(", 
      RowBox[{
       RowBox[{"Coefficient", "[", 
        RowBox[{
         RowBox[{"Series", "[", 
          RowBox[{
           RowBox[{
            FractionBox[
             RowBox[{"2", " ", "+", 
              RowBox[{
               SuperscriptBox["x", "2"], 
               RowBox[{"(", 
                RowBox[{
                 SuperscriptBox["k1", "2"], "+", 
                 SuperscriptBox["k2", "2"]}], ")"}]}]}], 
             RowBox[{" ", 
              SqrtBox[
               RowBox[{
                RowBox[{"(", 
                 RowBox[{"1", "+", " ", 
                  RowBox[{
                   SuperscriptBox["x", "2"], 
                   SuperscriptBox["k1", "2"]}]}], ")"}], " ", 
                RowBox[{"(", 
                 RowBox[{"1", "+", 
                  RowBox[{
                   SuperscriptBox["x", "2"], 
                   SuperscriptBox["k2", "2"]}]}], ")"}]}]], " "}]], "+", 
            "2"}], ",", 
           RowBox[{"{", 
            RowBox[{"x", ",", "0", ",", "M"}], "}"}]}], "]"}], ",", "x", ",", 
         "M"}], "]"}], "/.", 
       RowBox[{"{", 
        RowBox[{"k2", "\[Rule]", "1"}], "}"}]}], ")"}], ",", "k1", ",", "n"}],
     "]"}], "]"}]}]], "Input",
 CellChangeTimes->{{3.741067884946085*^9, 3.741067885275538*^9}, {
  3.741164679322756*^9, 3.7411646796226387`*^9}, {3.741165183607019*^9, 
  3.741165185606667*^9}, {3.74116570682456*^9, 3.7411657305145693`*^9}, {
  3.74131277413778*^9, 3.741312777544195*^9}},
 ExpressionUUID -> "d0800c20-1e76-438b-8757-2502969f7326"],

Cell[BoxData[
 RowBox[{
  RowBox[{"Coef2Csr", "=", 
   RowBox[{"Table", "[", 
    RowBox[{
     RowBox[{"Coef2Csr", "[", 
      RowBox[{
       RowBox[{"2", "i"}], ",", 
       RowBox[{"2", "j"}]}], "]"}], ",", 
     RowBox[{"{", 
      RowBox[{"i", ",", "0", ",", "10"}], "}"}], ",", 
     RowBox[{"{", 
      RowBox[{"j", ",", "0", ",", "10"}], "}"}]}], "]"}]}], ";"}]], "Input",
 CellChangeTimes->{{3.7220573274031277`*^9, 3.722057411958555*^9}, {
   3.722057553909235*^9, 3.722057558258687*^9}, 3.722058361827209*^9, {
   3.722059020563114*^9, 3.722059036001809*^9}, {3.722064043326339*^9, 
   3.7220640436134567`*^9}, {3.722068938617219*^9, 3.7220689488567133`*^9}, 
   3.7220690691792727`*^9, {3.722069129642337*^9, 3.722069129865574*^9}, {
   3.72207100528871*^9, 3.7220711073354273`*^9}, {3.72207151536589*^9, 
   3.722071516470203*^9}, {3.722071548694812*^9, 3.7220715507900457`*^9}, {
   3.722071640791222*^9, 3.7220716428698053`*^9}, {3.722158642706012*^9, 
   3.722158647632127*^9}, {3.7221587753440323`*^9, 3.722158777071834*^9}, {
   3.740299016390862*^9, 3.740299018742794*^9}, {3.740299562999009*^9, 
   3.740299566134993*^9}, {3.740299998439867*^9, 3.740300000263646*^9}, {
   3.7403637773136587`*^9, 3.7403637775028477`*^9}, {3.74036395662405*^9, 
   3.740363957136101*^9}, {3.741067949563488*^9, 3.741067953791477*^9}, {
   3.741164687935804*^9, 3.741164690479032*^9}, {3.741165187387107*^9, 
   3.741165189310234*^9}, {3.741165739048711*^9, 3.741165741896358*^9}, {
   3.741312779166647*^9, 3.7413127880905457`*^9}, {3.741315865935526*^9, 
   3.741315866604557*^9}},
 ExpressionUUID -> "e92ccd43-fa50-45d6-b546-7af5ee4c333d"]
}, Closed]],

Cell[CellGroupData[{

Cell["Large-c expansion", "Subsubsection",
 CellChangeTimes->{{3.741164836522542*^9, 3.741164866842805*^9}, {
  3.741335292923712*^9, 3.741335293435851*^9}},
 ExpressionUUID -> "275360dd-05f5-49d2-ad65-189b5f73105e"],

Cell["We have the large-c expansion expression", "Text",
 CellChangeTimes->{{3.724470606233453*^9, 3.724470623578065*^9}, {
  3.7411648516469088`*^9, 3.741164855153366*^9}, {3.741335296939602*^9, 
  3.741335297467857*^9}, {3.7414078769598*^9, 3.741407891772097*^9}},
 ExpressionUUID -> "42cbd2e3-37c9-4aeb-b39b-51d35fbe42ad"],

Cell[BoxData[
 RowBox[{
  RowBox[{"ExRCsrExpansion", "[", "N_", " ", "]"}], ":=", 
  RowBox[{"Simplify", "[", 
   RowBox[{"Sum", "[", 
    RowBox[{
     RowBox[{
      FractionBox["1", 
       SuperscriptBox["c", 
        RowBox[{"2", "n"}]]], 
      RowBox[{"Simplify", "[", 
       RowBox[{"(", 
        RowBox[{
         RowBox[{
          FractionBox[
           RowBox[{"3", "kF"}], 
           RowBox[{"4", "\[Pi]"}]], 
          RowBox[{"Simplify", "[", 
           RowBox[{"(", 
            RowBox[{
             RowBox[{"If", "[", 
              RowBox[{
               RowBox[{
                RowBox[{"Mod", "[", 
                 RowBox[{"n", ",", "2"}], "]"}], "==", "0"}], ",", 
               RowBox[{"Sum", "[", 
                RowBox[{
                 RowBox[{"2", " ", 
                  RowBox[{"Part", "[", 
                   RowBox[{"Coef1Csr", ",", 
                    RowBox[{"n", "+", "1"}], ",", 
                    RowBox[{"\[Nu]", "+", "1"}]}], "]"}], 
                  RowBox[{"Simplify", "[", 
                   RowBox[{"(", 
                    RowBox[{
                    RowBox[{"Part1First", "[", 
                    RowBox[{
                    RowBox[{"n", "-", "1", "-", "\[NoBreak]", "\[Nu]"}], ",", 
                    "\[Nu]"}], "]"}], "+", 
                    RowBox[{
                    SuperscriptBox["\[Mu]", "2"], 
                    RowBox[{"Part1SecondminusThird", "[", 
                    RowBox[{
                    RowBox[{"n", "-", "1", "-", "\[NoBreak]", "\[Nu]"}], ",", 
                    "\[NoBreak]", "\[Nu]"}], "]"}]}]}], ")"}], "]"}]}], ",", 
                 RowBox[{"{", 
                  RowBox[{"\[Nu]", ",", "0", ",", 
                   RowBox[{
                    RowBox[{"(", 
                    RowBox[{"n", "-", "2"}], ")"}], "/", "2"}]}], "}"}]}], 
                "]"}], ",", "0"}], "]"}], "+", 
             RowBox[{"If", "[", 
              RowBox[{
               RowBox[{
                RowBox[{"Mod", "[", 
                 RowBox[{"n", ",", "2"}], "]"}], "\[Equal]", "1"}], ",", " ", 
               
               RowBox[{
                RowBox[{
                 RowBox[{"Part", "[", 
                  RowBox[{"Coef1Csr", ",", 
                   RowBox[{"n", "+", "1"}], ",", 
                   RowBox[{
                    RowBox[{
                    RowBox[{"(", 
                    RowBox[{"n", "-", "1"}], ")"}], "/", "2"}], "+", "1"}]}], 
                  "]"}], 
                 RowBox[{"Simplify", "[", 
                  RowBox[{"(", 
                   RowBox[{
                    RowBox[{"Part1First", "[", 
                    RowBox[{
                    RowBox[{"n", "-", "1", "-", "\[NoBreak]", 
                    RowBox[{
                    RowBox[{"(", 
                    RowBox[{"n", "-", "1"}], ")"}], "/", "2"}]}], ",", 
                    RowBox[{
                    RowBox[{"(", 
                    RowBox[{"n", "-", "1"}], ")"}], "/", "2"}]}], "]"}], "+", 
                    
                    RowBox[{
                    SuperscriptBox["\[Mu]", "2"], 
                    RowBox[{"Part1SecondminusThird", "[", 
                    RowBox[{
                    RowBox[{"n", "-", "1", "-", "\[NoBreak]", 
                    RowBox[{
                    RowBox[{"(", 
                    RowBox[{"n", "-", "1"}], ")"}], "/", "2"}]}], ",", 
                    "\[NoBreak]", 
                    RowBox[{
                    RowBox[{"(", 
                    RowBox[{"n", "-", "1"}], ")"}], "/", "2"}]}], "]"}]}]}], 
                   ")"}], "]"}]}], "+", 
                RowBox[{"Sum", "[", 
                 RowBox[{
                  RowBox[{"2", 
                   RowBox[{"Part", "[", 
                    RowBox[{"Coef1Csr", ",", 
                    RowBox[{"n", "+", "1"}], ",", 
                    RowBox[{"\[Nu]", "+", "1"}]}], "]"}], 
                   RowBox[{"Simplify", "[", 
                    RowBox[{"(", 
                    RowBox[{
                    RowBox[{"Part1First", "[", 
                    RowBox[{
                    RowBox[{"n", "-", "1", "-", "\[NoBreak]", "\[Nu]"}], ",", 
                    "\[Nu]"}], "]"}], "+", 
                    RowBox[{
                    SuperscriptBox["\[Mu]", "2"], 
                    RowBox[{"Part1SecondminusThird", "[", 
                    RowBox[{
                    RowBox[{"n", "-", "1", "-", "\[NoBreak]", "\[Nu]"}], ",", 
                    "\[NoBreak]", "\[Nu]"}], "]"}]}]}], ")"}], "]"}]}], ",", 
                  RowBox[{"{", 
                   RowBox[{"\[Nu]", ",", "0", ",", 
                    RowBox[{
                    RowBox[{"(", 
                    RowBox[{"n", "-", "3"}], ")"}], "/", "2"}]}], "}"}]}], 
                 "]"}]}], ",", "0"}], "]"}]}], ")"}], "]"}]}], "+", 
         RowBox[{
          FractionBox[
           RowBox[{"3", "kF"}], 
           RowBox[{"16", " ", "\[Pi]"}]], 
          RowBox[{"Simplify", "[", 
           RowBox[{"(", 
            RowBox[{
             RowBox[{"If", "[", 
              RowBox[{
               RowBox[{
                RowBox[{"Mod", "[", 
                 RowBox[{"n", ",", "2"}], "]"}], "\[Equal]", "1"}], ",", 
               RowBox[{"Sum", "[", 
                RowBox[{
                 RowBox[{"2", " ", 
                  RowBox[{"Part", "[", 
                   RowBox[{"Coef2Csr", ",", 
                    RowBox[{"n", "+", "1"}], ",", 
                    RowBox[{"\[Nu]", "+", "1"}]}], "]"}], 
                  RowBox[{"Simplify", "[", 
                   RowBox[{"(", 
                    RowBox[{
                    RowBox[{"Part2ThirdminusFourth", "[", 
                    RowBox[{
                    RowBox[{"n", "-", "\[NoBreak]", "\[Nu]"}], ",", "\[Nu]"}],
                     "]"}], "-", 
                    RowBox[{"Part2SecondminusFirst", "[", 
                    RowBox[{
                    RowBox[{"n", "-", "\[NoBreak]", "\[Nu]"}], ",", "\[Nu]"}],
                     "]"}]}], ")"}], "]"}]}], ",", 
                 RowBox[{"{", 
                  RowBox[{"\[Nu]", ",", "0", ",", 
                   RowBox[{
                    RowBox[{"(", 
                    RowBox[{"n", "-", "1"}], ")"}], "/", "2"}]}], "}"}]}], 
                "]"}], ",", "0"}], "]"}], "+", 
             RowBox[{"If", "[", 
              RowBox[{
               RowBox[{
                RowBox[{"Mod", "[", 
                 RowBox[{"n", ",", "2"}], "]"}], "\[Equal]", "0"}], ",", " ", 
               
               RowBox[{
                RowBox[{
                 RowBox[{"Part", "[", 
                  RowBox[{"Coef2Csr", ",", 
                   RowBox[{"n", "+", "1"}], ",", 
                   RowBox[{
                    RowBox[{"n", "/", "2"}], "+", "1"}]}], "]"}], 
                 RowBox[{"Simplify", "[", 
                  RowBox[{"(", 
                   RowBox[{
                    RowBox[{"Part2ThirdminusFourth", "[", 
                    RowBox[{
                    RowBox[{"n", "-", "\[NoBreak]", 
                    RowBox[{"n", "/", "2"}]}], ",", 
                    RowBox[{"n", "/", "2"}]}], "]"}], "-", 
                    RowBox[{"Part2SecondminusFirst", "[", 
                    RowBox[{
                    RowBox[{"n", "-", "\[NoBreak]", 
                    RowBox[{"n", "/", "2"}]}], ",", 
                    RowBox[{"n", "/", "2"}]}], "]"}]}], ")"}], "]"}]}], "+", 
                RowBox[{"Sum", "[", 
                 RowBox[{
                  RowBox[{"2", 
                   RowBox[{"Part", "[", 
                    RowBox[{"Coef2Csr", ",", 
                    RowBox[{"n", "+", "1"}], ",", 
                    RowBox[{"\[Nu]", "+", "1"}]}], "]"}], 
                   RowBox[{"Simplify", "[", 
                    RowBox[{"(", 
                    RowBox[{
                    RowBox[{"Part2ThirdminusFourth", "[", 
                    RowBox[{
                    RowBox[{"n", "-", "\[NoBreak]", "\[Nu]"}], ",", "\[Nu]"}],
                     "]"}], "-", 
                    RowBox[{"Part2SecondminusFirst", "[", 
                    RowBox[{
                    RowBox[{"n", "-", "\[NoBreak]", "\[Nu]"}], ",", "\[Nu]"}],
                     "]"}]}], ")"}], "]"}]}], ",", 
                  RowBox[{"{", 
                   RowBox[{"\[Nu]", ",", "0", ",", 
                    RowBox[{
                    RowBox[{"(", 
                    RowBox[{"n", "-", "2"}], ")"}], "/", "2"}]}], "}"}]}], 
                 "]"}]}], ",", "0"}], "]"}]}], ")"}], "]"}]}]}], ")"}], 
       "]"}]}], ",", " ", 
     RowBox[{"{", 
      RowBox[{"n", ",", "0", ",", 
       RowBox[{"N", "/", "2"}]}], "}"}]}], "]"}], "]"}]}]], "Input",
 CellChangeTimes->{{3.722754572486408*^9, 3.7227546129606533`*^9}, {
   3.741165015141117*^9, 3.741165045250079*^9}, {3.741165197810758*^9, 
   3.741165254957601*^9}, {3.741165773814*^9, 3.741165787768862*^9}, {
   3.741313113248271*^9, 3.741313144590747*^9}, {3.741313741742466*^9, 
   3.741313747071333*^9}, {3.7413138069750032`*^9, 3.74131381753027*^9}, {
   3.7413142649963427`*^9, 3.741314277224654*^9}, 3.741317053590225*^9, {
   3.741318788621028*^9, 3.741318790515428*^9}},
 ExpressionUUID -> "505fa03b-bcf8-4e3e-95dc-50418acd2030"],

Cell["\<\
We first calculate the large-c expansion to a satisfying order, let\
\[CloseCurlyQuote]s say 20.\
\>", "Text",
 CellChangeTimes->{{3.722658255655129*^9, 3.722658274741214*^9}, {
  3.741313268936226*^9, 
  3.741313280568243*^9}},ExpressionUUID->"7424e152-80a6-4099-b04c-\
62d5086ae49f"],

Cell[BoxData[
 RowBox[{
  RowBox[{"ExRCsrOrder20", "=", 
   RowBox[{"ExRCsrExpansion", "[", "20", "]"}]}], ";"}]], "Input",
 CellChangeTimes->{{3.722657885346245*^9, 3.722657905194455*^9}, {
   3.72265917006719*^9, 3.722659250932714*^9}, {3.722763920069398*^9, 
   3.722763928880912*^9}, {3.740299051015119*^9, 3.740299051080347*^9}, {
   3.740363795247789*^9, 3.740363796239716*^9}, {3.7411652585174932`*^9, 
   3.7411652633781548`*^9}, {3.741165795859723*^9, 3.7411657984422483`*^9}, {
   3.741313222841453*^9, 3.741313257225306*^9}, {3.741315481468864*^9, 
   3.741315506042829*^9}, 3.7413170548330317`*^9, {3.7413187966294327`*^9, 
   3.741318808432065*^9}},
 ExpressionUUID -> "82a23dc9-5948-4081-b410-add8e4510fb2"],

Cell[BoxData[
 RowBox[{
  RowBox[{"ExRCOrder20", "=", 
   RowBox[{"Limit", "[", 
    RowBox[{"ExRCsrOrder20", ",", 
     RowBox[{"\[Mu]", "\[Rule]", "0"}]}], "]"}]}], ";"}]], "Input",
 CellChangeTimes->{
  3.7227558995802526`*^9, {3.7411657967815123`*^9, 3.7411657994598923`*^9}, 
   3.741313225929617*^9, {3.741313263481997*^9, 3.741313264425818*^9}, {
   3.741315509596798*^9, 3.741315510780417*^9}, {3.741316041485497*^9, 
   3.741316043549305*^9}},
 ExpressionUUID -> "03b2a6ef-b326-417c-b67e-e404b10e056c"]
}, Closed]],

Cell[CellGroupData[{

Cell["Pad\[EAcute] approximants", "Subsubsection",
 CellChangeTimes->{{3.7411649136217203`*^9, 3.741164917030664*^9}, {
  3.741164959746048*^9, 3.741164964829475*^9}, {3.7413353542841578`*^9, 
  3.741335356283766*^9}},
 ExpressionUUID -> "4c21d97d-33d1-4287-8364-88baa46d5f2b"],

Cell["\<\
We prepare the coefficient of the large-c expansion for the short-range \
exchange energy per particle and for the \[Mu] \[RightArrow] 0 limit\
\>", "Text",
 CellChangeTimes->{{3.7227553188603687`*^9, 3.722755371373106*^9}, {
   3.72275562759557*^9, 3.7227556515776443`*^9}, {3.724470657833439*^9, 
   3.72447066020118*^9}, {3.741315414203617*^9, 3.741315470363694*^9}, {
   3.7413353707158623`*^9, 3.741335374955949*^9}, 3.7414079334623833`*^9},
 ExpressionUUID -> "2c374c70-8b7b-4d91-8791-a25f833f520c"],

Cell[BoxData[
 RowBox[{
  RowBox[{"CoefficientCsr", "[", 
   RowBox[{"M_", ",", "n_"}], "]"}], ":=", 
  RowBox[{"Simplify", "[", 
   RowBox[{"Coefficient", "[", 
    RowBox[{
     RowBox[{"ExRCsrOrder20", "/.", 
      RowBox[{"{", 
       RowBox[{"c", "\[Rule]", 
        RowBox[{"1", "/", "x"}]}], "}"}]}], ",", "x", ",", "n"}], "]"}], 
   "]"}]}]], "Input",
 CellChangeTimes->{{3.7226678420237913`*^9, 3.722667861528064*^9}, {
   3.72266815372162*^9, 3.7226681849194813`*^9}, {3.7226721981498747`*^9, 
   3.722672207155808*^9}, 3.7227550567672377`*^9, {3.722755656577574*^9, 
   3.7227556642370653`*^9}, {3.741165279910945*^9, 3.741165280303294*^9}, {
   3.741165801108734*^9, 3.741165802557379*^9}, {3.741314586153861*^9, 
   3.741314586281663*^9}, {3.7413148850075493`*^9, 3.741314885241417*^9}, {
   3.741315516652811*^9, 3.7413155175013733`*^9}},
 ExpressionUUID -> "3458de6d-dc55-4eee-8f68-47cc595316a0"],

Cell[BoxData[
 RowBox[{
  RowBox[{"CoefficientC", "[", 
   RowBox[{"M_", ",", "n_"}], "]"}], ":=", 
  RowBox[{"Simplify", "[", 
   RowBox[{"Coefficient", "[", 
    RowBox[{
     RowBox[{"ExRCOrder20", "/.", 
      RowBox[{"{", 
       RowBox[{"c", "\[Rule]", 
        RowBox[{"1", "/", "x"}]}], "}"}]}], ",", "x", ",", "n"}], "]"}], 
   "]"}]}]], "Input",
 CellChangeTimes->{{3.7227556735963917`*^9, 3.7227556754363728`*^9}, {
   3.741165291318172*^9, 3.7411653095641212`*^9}, {3.7411658075165567`*^9, 
   3.741165809802228*^9}, {3.741314633492703*^9, 3.741314634757943*^9}, 
   3.741314919610902*^9, {3.741315520381742*^9, 3.741315521149824*^9}},
 ExpressionUUID -> "64b73a86-5875-4097-8a07-6d52f2a444f1"],

Cell[BoxData[
 RowBox[{
  RowBox[{"CoefCsr", "[", "M_", "]"}], ":=", 
  RowBox[{"Table", "[", 
   RowBox[{
    RowBox[{
     SubscriptBox["T", "i"], "->", 
     RowBox[{"CoefficientCsr", "[", 
      RowBox[{"M", ",", "i"}], "]"}]}], ",", 
    RowBox[{"{", 
     RowBox[{"i", ",", "0", ",", "M"}], "}"}]}], "]"}]}]], "Input",
 CellChangeTimes->{{3.722749765088842*^9, 3.722749844950129*^9}, {
   3.72275111355685*^9, 3.7227511736510963`*^9}, {3.7227512675099688`*^9, 
   3.722751272325121*^9}, 3.722752713870413*^9, {3.7227542354300613`*^9, 
   3.722754236382597*^9}, {3.722755666317625*^9, 3.7227556680165157`*^9}, {
   3.7411652856659613`*^9, 3.741165288839732*^9}, {3.741165803964905*^9, 
   3.741165805816494*^9}, {3.741314890229391*^9, 3.741314893738743*^9}, {
   3.7413149288437023`*^9, 3.741314934843973*^9}},
 ExpressionUUID -> "449c22ee-b6b0-4c67-9180-b8f7bf1e2975"],

Cell[BoxData[
 RowBox[{
  RowBox[{"CoefC", "[", "M_", "]"}], ":=", 
  RowBox[{"Table", "[", 
   RowBox[{
    RowBox[{
     SubscriptBox["T", "i"], "->", 
     RowBox[{"CoefficientC", "[", 
      RowBox[{"M", ",", "i"}], "]"}]}], ",", 
    RowBox[{"{", 
     RowBox[{"i", ",", "0", ",", "M"}], "}"}]}], "]"}]}]], "Input",
 CellChangeTimes->{{3.722755679643105*^9, 3.722755680670816*^9}, {
   3.7411652967818327`*^9, 3.7411652992974167`*^9}, 3.7411658123477707`*^9, 
   3.7411662521890163`*^9, {3.741314937994246*^9, 3.741314954859644*^9}},
 ExpressionUUID -> "98571266-4a62-450a-903b-31e985157417"],

Cell["\<\
We now express the specific coefficients for our Pad\[EAcute] approximant \
using the order-20  large-c expansion\
\>", "Text",
 CellChangeTimes->{{3.722763848195755*^9, 3.722763880899667*^9}, {
  3.741315729450776*^9, 3.7413157473068323`*^9}, {3.741335389932165*^9, 
  3.741335421420309*^9}, {3.741335452204438*^9, 
  3.741335452956361*^9}},ExpressionUUID->"97a36114-4b5f-4269-8150-\
3df4a4ae776d"],

Cell[BoxData[
 RowBox[{
  RowBox[{"CoefBPad\[EAcute]C", "=", 
   RowBox[{
    RowBox[{"CoefBPad\[EAcute]", "[", "10", "]"}], "/.", 
    RowBox[{"CoefC", "[", "20", "]"}]}]}], ";"}]], "Input",
 CellChangeTimes->{{3.722753594171132*^9, 3.722753620589405*^9}, 
   3.722753773971465*^9, 3.722753896092773*^9, {3.722754258580085*^9, 
   3.7227542587988586`*^9}, {3.722754465761252*^9, 3.722754485745597*^9}, {
   3.72275541074507*^9, 3.722755440462531*^9}, {3.722755709305892*^9, 
   3.7227557107485*^9}, {3.7227560316951523`*^9, 3.722756055026368*^9}, {
   3.722756395457559*^9, 3.722756409823081*^9}, {3.741165336843622*^9, 
   3.741165357183463*^9}, {3.741165825467124*^9, 3.7411658299082203`*^9}, {
   3.7413149650996237`*^9, 3.7413149699957933`*^9}, {3.741315265420334*^9, 
   3.741315266187937*^9}, {3.741315550782506*^9, 3.7413155823186483`*^9}, {
   3.741315643371585*^9, 3.741315647437683*^9}},
 ExpressionUUID -> "12765f75-bf12-4a8e-bc21-043278e419ab"],

Cell[BoxData[
 RowBox[{
  RowBox[{"CoefBPad\[EAcute]Csr", "=", 
   RowBox[{
    RowBox[{"CoefBPad\[EAcute]", "[", "10", "]"}], "/.", 
    RowBox[{"CoefCsr", "[", "20", "]"}]}]}], ";"}]], "Input",
 CellChangeTimes->{{3.7227563927641907`*^9, 3.722756424828418*^9}, {
  3.722756470028845*^9, 3.722756471262659*^9}, {3.741165338166099*^9, 
  3.74116535636982*^9}, {3.741165826280868*^9, 3.741165830758252*^9}, {
  3.741314982347934*^9, 3.7413149848775673`*^9}, {3.741315268045794*^9, 
  3.74131526958106*^9}, {3.741315564238062*^9, 3.741315585069827*^9}, {
  3.741315648332552*^9, 3.741315649151641*^9}},
 ExpressionUUID -> "714600a4-53dd-4aca-af71-5ed1e99c7226"],

Cell[BoxData[
 RowBox[{
  RowBox[{"CoefAPad\[EAcute]C", "=", 
   RowBox[{
    RowBox[{"CoefAPad\[EAcute]", "[", "10", "]"}], "/.", 
    RowBox[{"CoefC", "[", "20", "]"}]}]}], ";"}]], "Input",
 CellChangeTimes->{{3.722754029546383*^9, 3.722754044308186*^9}, {
   3.722754301982415*^9, 3.722754302035227*^9}, {3.7227544718864326`*^9, 
   3.722754488205662*^9}, {3.722755452684111*^9, 3.722755452924046*^9}, 
   3.7227557289252*^9, {3.722756027149149*^9, 3.722756058413001*^9}, 
   3.722756119853417*^9, 3.722756296716875*^9, {3.722756447367597*^9, 
   3.722756450307869*^9}, {3.741165339561618*^9, 3.741165355379118*^9}, {
   3.741165827109076*^9, 3.741165832083321*^9}, {3.741314987228261*^9, 
   3.7413149885234613`*^9}, {3.741315271836527*^9, 3.741315272429305*^9}, {
   3.7413155708925943`*^9, 3.741315586204362*^9}, {3.741315650300768*^9, 
   3.741315651546886*^9}},
 ExpressionUUID -> "dafc6fff-5fa3-4323-a7a6-3db969c4b656"],

Cell[BoxData[
 RowBox[{
  RowBox[{"CoefAPad\[EAcute]Csr", "=", 
   RowBox[{
    RowBox[{"CoefAPad\[EAcute]", "[", "10", "]"}], "/.", 
    RowBox[{"CoefCsr", "[", "20", "]"}]}]}], ";"}]], "Input",
 CellChangeTimes->{{3.722756457980381*^9, 3.722756467531996*^9}, {
  3.741165343013163*^9, 3.741165354109902*^9}, {3.741165828153932*^9, 
  3.741165833829134*^9}, {3.741314992123789*^9, 3.741314992987317*^9}, {
  3.741315274700562*^9, 3.741315280252084*^9}, {3.74131558898942*^9, 
  3.741315591501307*^9}, {3.741315652989523*^9, 3.7413156541452312`*^9}},
 ExpressionUUID -> "6447cd9c-f64a-48c9-a24e-d0dde32446d1"],

Cell["\<\
We can now define our  Pad\[EAcute] approximants for the full-range and the \
short-range Coulomb exchange energies per particle\
\>", "Text",
 CellChangeTimes->{{3.7227640074737988`*^9, 3.722764017491691*^9}, {
  3.741335490778098*^9, 
  3.741335513211927*^9}},ExpressionUUID->"064c57d7-1569-4b7d-af88-\
cad4f23b52df"],

Cell[BoxData[
 RowBox[{
  RowBox[{"ExRCPad\[EAcute]", "[", "M_", "]"}], ":=", 
  RowBox[{
   RowBox[{"(", 
    RowBox[{"Sum", "[", 
     RowBox[{
      FractionBox[
       RowBox[{"Part", "[", 
        RowBox[{"CoefAPad\[EAcute]C", ",", "M", ",", 
         RowBox[{"k", "+", "1"}]}], "]"}], 
       SuperscriptBox["c", "k"]], ",", 
      RowBox[{"{", 
       RowBox[{"k", ",", "0", ",", "M"}], "}"}]}], "]"}], ")"}], "/", 
   RowBox[{"(", 
    RowBox[{"1", "+", 
     RowBox[{"Sum", "[", 
      RowBox[{
       FractionBox[
        RowBox[{"Part", "[", 
         RowBox[{"CoefBPad\[EAcute]C", ",", "M", ",", "k"}], "]"}], 
        SuperscriptBox["c", "k"]], ",", 
       RowBox[{"{", 
        RowBox[{"k", ",", "1", ",", "M"}], "}"}]}], "]"}]}], 
    ")"}]}]}]], "Input",
 CellChangeTimes->{{3.7227562198866377`*^9, 3.722756223232061*^9}, {
   3.722756344477265*^9, 3.722756374429248*^9}, {3.724472328737096*^9, 
   3.7244723404597588`*^9}, {3.7244725391989813`*^9, 3.724472541421919*^9}, {
   3.7244732518101883`*^9, 3.724473255736369*^9}, {3.7411651613833103`*^9, 
   3.741165167052189*^9}, {3.7411653461762133`*^9, 3.7411653497927322`*^9}, {
   3.741165839085773*^9, 3.741165845925786*^9}, {3.7413156004345922`*^9, 
   3.7413156087854156`*^9}, {3.741316207389226*^9, 3.7413162096777487`*^9}, {
   3.741318767108757*^9, 3.741318773618332*^9}, 3.7413194469795*^9},
 ExpressionUUID -> "7ea81c99-1e1c-44c3-a5f3-92ba46f3d003"],

Cell[BoxData[
 RowBox[{
  RowBox[{"ExRCsrPad\[EAcute]", "[", "M_", "]"}], ":=", 
  RowBox[{
   RowBox[{"(", 
    RowBox[{"Sum", "[", 
     RowBox[{
      FractionBox[
       RowBox[{"Part", "[", 
        RowBox[{"CoefAPad\[EAcute]Csr", ",", "M", ",", 
         RowBox[{"k", "+", "1"}]}], "]"}], 
       SuperscriptBox["c", "k"]], ",", 
      RowBox[{"{", 
       RowBox[{"k", ",", "0", ",", "M"}], "}"}]}], "]"}], ")"}], "/", 
   RowBox[{"(", 
    RowBox[{"1", "+", 
     RowBox[{"Sum", "[", 
      RowBox[{
       FractionBox[
        RowBox[{"Part", "[", 
         RowBox[{"CoefBPad\[EAcute]Csr", ",", "M", ",", "k"}], "]"}], 
        SuperscriptBox["c", "k"]], ",", 
       RowBox[{"{", 
        RowBox[{"k", ",", "1", ",", "M"}], "}"}]}], "]"}]}], 
    ")"}]}]}]], "Input",
 CellChangeTimes->{{3.722754133946948*^9, 3.722754168197061*^9}, 
   3.722755764286047*^9, {3.722755795648616*^9, 3.7227557972443647`*^9}, {
   3.722756165936594*^9, 3.7227562108616667`*^9}, {3.722756481371945*^9, 
   3.722756490285556*^9}, {3.724472343389707*^9, 3.724472353121357*^9}, {
   3.724473258746921*^9, 3.724473263323648*^9}, {3.741165168482983*^9, 
   3.741165168762787*^9}, {3.7411653511334343`*^9, 3.741165353067666*^9}, {
   3.7411658422331877`*^9, 3.741165847801704*^9}, {3.741315603778873*^9, 
   3.741315606040073*^9}, {3.741316210380775*^9, 3.741316213918049*^9}, {
   3.741318775359991*^9, 3.741318780850219*^9}},
 ExpressionUUID -> "d8ccd518-5236-4a0b-9bce-cf5d56e4d059"]
}, Closed]]
}, Closed]],

Cell[CellGroupData[{

Cell["Tests", "Subsection",
 CellChangeTimes->{{3.7411646556876497`*^9, 3.741164658735076*^9}},
 ExpressionUUID -> "623a936f-92cc-4236-91b4-25f2f70700c3"],

Cell[CellGroupData[{

Cell["Full-range Coulomb exchange energy per particle", "Subsubsection",
 CellChangeTimes->{{3.741166404504117*^9, 3.74116641070641*^9}, 
   3.74131965313426*^9, {3.741335575996008*^9, 3.7413355923644743`*^9}},
 ExpressionUUID -> "8d35845f-7f80-46e8-808b-7f7f87394988"],

Cell[CellGroupData[{

Cell[BoxData[
 RowBox[{"ExRCPad\[EAcute]2", "=", 
  RowBox[{"Simplify", "[", 
   RowBox[{"ExRCPad\[EAcute]", "[", "2", "]"}], "]"}]}]], "Input",
 ExpressionUUID -> "9df73f38-04ca-4221-8f34-4aaa88b382c8"],

Cell[BoxData[
 RowBox[{"-", 
  FractionBox[
   RowBox[{
    RowBox[{"97", " ", "kF"}], "+", 
    RowBox[{"180", " ", 
     SuperscriptBox["c", "2"], " ", "kF"}]}], 
   RowBox[{
    RowBox[{"156", " ", "\[Pi]"}], "+", 
    RowBox[{"240", " ", 
     SuperscriptBox["c", "2"], " ", "\[Pi]"}]}]]}]], "Output",
 CellChangeTimes->{3.741319797998054*^9, 3.7413200901848373`*^9, 
  3.741320587749445*^9, 3.7413218763825417`*^9, 3.741335626371447*^9, 
  3.7414085507549*^9, 3.74140923104434*^9, 3.741409430154316*^9, 
  3.741409975685452*^9},
 ExpressionUUID -> "91a4722e-059a-4232-ba24-de99b20b23f0"]
}, Open  ]],

Cell[CellGroupData[{

Cell[BoxData[
 RowBox[{"ExRCPad\[EAcute]4", "=", 
  RowBox[{"Simplify", "[", 
   RowBox[{"ExRCPad\[EAcute]", "[", "4", "]"}], "]"}]}]], "Input",
 ExpressionUUID -> "8bf298f8-d170-49ad-badc-15fc77cf9e9e"],

Cell[BoxData[
 RowBox[{"-", 
  FractionBox[
   RowBox[{
    RowBox[{"(", 
     RowBox[{"584417", "+", 
      RowBox[{"2500260", " ", 
       SuperscriptBox["c", "2"]}], "+", 
      RowBox[{"2286900", " ", 
       SuperscriptBox["c", "4"]}]}], ")"}], " ", "kF"}], 
   RowBox[{"48", " ", 
    RowBox[{"(", 
     RowBox[{"20147", "+", 
      RowBox[{"76510", " ", 
       SuperscriptBox["c", "2"]}], "+", 
      RowBox[{"63525", " ", 
       SuperscriptBox["c", "4"]}]}], ")"}], " ", "\[Pi]"}]]}]], "Output",
 CellChangeTimes->{3.741319800239278*^9, 3.741320094376034*^9, 
  3.74132187648322*^9, 3.741335628737815*^9, 3.741408550896235*^9, 
  3.741409231169609*^9, 3.7414094302991962`*^9, 3.7414099758179398`*^9},
 ExpressionUUID -> "82c14e9d-eabf-4ed8-a218-c5ee6663846f"]
}, Open  ]],

Cell[CellGroupData[{

Cell[BoxData[
 RowBox[{"ExRCPad\[EAcute]6", "=", 
  RowBox[{"Simplify", "[", 
   RowBox[{"ExRCPad\[EAcute]", "[", "6", "]"}], "]"}]}]], "Input",
 ExpressionUUID -> "784a75bc-a185-4077-83a2-a9566d665d32"],

Cell[BoxData[
 RowBox[{"-", 
  FractionBox[
   RowBox[{
    RowBox[{"(", 
     RowBox[{"647533920739", "+", 
      RowBox[{"4750712757380", " ", 
       SuperscriptBox["c", "2"]}], "+", 
      RowBox[{"9877792994300", " ", 
       SuperscriptBox["c", "4"]}], "+", 
      RowBox[{"6090941656800", " ", 
       SuperscriptBox["c", "6"]}]}], ")"}], " ", "kF"}], 
   RowBox[{"400", " ", 
    RowBox[{"(", 
     RowBox[{"2699080675", "+", 
      RowBox[{"18278469270", " ", 
       SuperscriptBox["c", "2"]}], "+", 
      RowBox[{"35181880965", " ", 
       SuperscriptBox["c", "4"]}], "+", 
      RowBox[{"20303138856", " ", 
       SuperscriptBox["c", "6"]}]}], ")"}], " ", "\[Pi]"}]]}]], "Output",
 CellChangeTimes->{3.741319838419587*^9, 3.741320097292377*^9, 
  3.741321876535376*^9, 3.741335630854007*^9, 3.7414085509715347`*^9, 
  3.741409231290845*^9, 3.741409430431424*^9, 3.741409975955346*^9, 
  3.74141076653083*^9},
 ExpressionUUID -> "c9ad8416-79af-41ad-95a7-3d2ae6d4a06f"]
}, Open  ]],

Cell[BoxData[
 RowBox[{
  RowBox[{"ExRCPad\[EAcute]8", "=", 
   RowBox[{"Simplify", "[", 
    RowBox[{"ExRCPad\[EAcute]", "[", "8", "]"}], "]"}]}], ";"}]], "Input",
 CellChangeTimes->{{3.7414106641241713`*^9, 3.741410680947584*^9}, {
  3.74141076836687*^9, 3.7414107685613194`*^9}}],

Cell[CellGroupData[{

Cell[BoxData[
 RowBox[{"Plot", "[", 
  RowBox[{
   RowBox[{"{", 
    RowBox[{
     RowBox[{"ExRC", "/.", 
      RowBox[{"{", 
       RowBox[{"c", "\[Rule]", 
        RowBox[{"137.036", "/", "kF"}]}], "}"}]}], ",", 
     RowBox[{"ExRCOrder20", "/.", 
      RowBox[{"{", 
       RowBox[{"c", "\[Rule]", 
        RowBox[{"137.036", "/", "kF"}]}], "}"}]}], ",", 
     RowBox[{"ExRCPad\[EAcute]2", "/.", 
      RowBox[{"{", 
       RowBox[{"c", "\[Rule]", 
        RowBox[{"137.036", "/", "kF"}]}], "}"}]}], ",", 
     RowBox[{"ExRCPad\[EAcute]4", "/.", 
      RowBox[{"{", 
       RowBox[{"c", "\[Rule]", 
        RowBox[{"137.036", "/", "kF"}]}], "}"}]}], ",", 
     RowBox[{"ExRCPad\[EAcute]6", "/.", 
      RowBox[{"{", 
       RowBox[{"c", "\[Rule]", 
        RowBox[{"137.036", "/", "kF"}]}], "}"}]}]}], "}"}], ",", 
   RowBox[{"{", 
    RowBox[{"kF", ",", "0", ",", "300"}], "}"}], ",", 
   RowBox[{"PlotStyle", "\[Rule]", 
    RowBox[{"{", 
     RowBox[{"Blue", ",", "Red", ",", "Green", ",", "Purple", ",", "White"}], 
     "}"}]}], ",", 
   RowBox[{"PlotRange", "\[Rule]", 
    RowBox[{"{", 
     RowBox[{
      RowBox[{"{", 
       RowBox[{"0", ",", "300"}], "}"}], ",", 
      RowBox[{"{", 
       RowBox[{
        RowBox[{"-", "65"}], ",", "0"}], "}"}]}], "}"}]}]}], "]"}]], "Input",
 CellChangeTimes->{{3.725790426404578*^9, 3.725790453840857*^9}, {
   3.725790502785564*^9, 3.725790550992629*^9}, {3.726898837998486*^9, 
   3.726898847052638*^9}, {3.741165900638431*^9, 3.7411659400545387`*^9}, {
   3.741166056629149*^9, 3.741166057200569*^9}, 3.7413162488297863`*^9, {
   3.741318686271461*^9, 3.741318713551878*^9}, {3.7413187477294397`*^9, 
   3.741318749185649*^9}, {3.741320129814933*^9, 3.741320147957473*^9}},
 ExpressionUUID -> "0ceba4c0-8e5b-4a64-b27f-206e85f1f4cf"],

Cell[BoxData[
 GraphicsBox[{{{}, {}, 
    TagBox[
     {RGBColor[0, 0, 1], AbsoluteThickness[1.6], Opacity[1.], 
      LineBox[CompressedData["
1:eJwVkHs01AkfxnEozbrUsjQxTtpa6TVNsjEamS8ybvltal0iYZIXscyv0vam
mU1FyNCYpavFukTRFNO8uf2+3fQqCudMtogupEHua5DdXvuc85znfP57nseS
n7DrgJaGhgZ/0f9ktY3CjBAruBr/CHZievO+Lr9F5lsNZSUI86icVynHLcSP
uRmXo+0dhGXU6PrrOhmVHVwPH3KvoldGSfulbdriLq7dd+frOcI71NZC4a8i
wWvuq+hV5s2MBmqcWbvxROVb7kBD6sOyXqTyVFdn1FmDXI5WxxGmsJmKeSwJ
louGuIFe+WvHfVsop9K0JlLwiRt4f8b/NqOVEsjYD5IqJ7iXK4zOXeptp0zj
1mROZKm57wtLzejCF5RGt/m29iVz3MiQvFr1QBc15GU6Vi2a57YadyuVvi+p
Biu93XGCv7htjz5m5zB6qFsT/8k6VKkJ+s6iX0W9b6jAqkj/0aylcGL2Wsjr
Ex+o1v6I6lBvXXj4+Trnse0gBeZhS9uWLIPL1zTLZQOD1IbMPXevi2gQp5pc
nuKrohaiCUaMQB/ufxX43IIxQvl9fWVSULkCTJVGiRa945S67UzdSJYpdJ78
OWAueYaK5NLYK6ZNoZC3Sn6od4bqlInlW4JXQtpE3blPXDVVnZsvE35HB3qa
WUGf1iwVuaeibDm1CmrOvKE1np2jOvtbJd+PM8Dgk2BViHSB6vorfYuz9RrQ
ftHqkeGviTXGHfqpmeuhs8lmSOPgUkz81/ftjZzNMOYc73E7fAWaeKilLUZs
KBsfpTYNmeBUo2lscawzGLDmjjr3m+OZMIuV+RtcIbAq1Oi5gyXeyAo75Rbm
DqqbCxNpdmvR7NjeuNnTnpBXdW+Hp5kVlld0t6Ue9gEnr+5Sx6fW+CwtXXH8
dwKKfsz7/WS1DWYoe/TWPdsJG+ztD1gHs7D9UWfycrddcOgJS994bhP2673Z
dLNrN/xtad7cGroZ05I2Fm318wfXqzO9/HI7VNtL/Y8NBYCNIsR67bIt+NWL
Lk+n5CCgh90oUofbY3X+3tnhyT0w7euSXVTggBay2WEiPQR06/iOutNsZAwr
Lxdoh8KSqmVOvaytOJT8JLvot31gdUHVwzzFwaokIkJKDwcWrzvqdJsTMuGP
oGfKcLhQU3An4Ms2NJLHT74tioCSJxM/nPTkokv9t0MHw/kgdU/60O0EeE/m
qck22w+h7WclGR2A5X7H6l4P7Ada8hT0CVxQeepJx1xxJNxqi24pXeKKsRFW
mWMJByDqvvduWrkr+m2c2m/lGAXFIrqL3M0NRef6Limno0AS9uApU+mGxnld
h0Lx30Cvf5DBI7fj+KbxyhBhNDw2mHAP1nZHi/qjmlfYMVA+6FBkmOuONeO0
eblWLLD7TRKimTzMVjTt5FGxcEeron++gYed1kIvWeZBkA/sy2MFeeBe5r7C
HO84uKq4H9n40QPZq6tManTiwVWy4e9vkzzxeNNS1s32eKgtTjGwNfRCndGU
UkvxT3CpJF9676oXzvxvWVN8SAKsNqyennXwxistX+ZPfJ0I4brZequfe2OE
msb7JTER9E30+4ZDfPDlvBk/4UUieB5YTfGnffBP3raqi1sE4Gdbt1GcsgPr
aCa6AxIBMB728Fr0fXFzybQdY1YAEju+YU2JLxKp78U5ASQ8f1e1MsqWQA9v
8Q77IBJy6Rn0V3YEgoEjrWcPCQUBP6wk7Am0zROfsQolIXHFRUN7DoHGZY7J
TftJmJHzBnTcCex+lB0zkkjCy55JZmkQgdE6Tts9M0kYtWjgvBMRGNHyQXP0
HAkCl/9+9k8hMDjrPJUrJkG1puluy2kCd3wzuLXvPAlsy2HWrXQCWesktkkX
SBgYHtD+JZfAme0fLUpKSRDnOO1ilBM4ppvb41VOgl2tz1ROBYEfW7ddGrtG
QlPUYYn2DQJf/pj7DecGCbNhJk+HZQQ2RDrrdd5e3PNesa6ujkD5elXL0VoS
ou9VK5iNBFaP5KYx7pDQPtXsUUQRWHhYpRVzlwRqcxj/7EMCL7KlaFBPwhGb
tyOfmwmULDgLaxsW+/qfPZLQQmAGqjjBTYt/FvsvvHtK4KnT0rkvFAmpNO+T
Ac8I/D9oRQwH
       "]]},
     Annotation[#, "Charting`Private`Tag$16400#1"]& ], 
    TagBox[
     {RGBColor[1, 0, 0], AbsoluteThickness[1.6], Opacity[1.], 
      LineBox[CompressedData["
1:eJwVxQk41AkfwHG6TFGKXNnmXZWUO9VQMvMzM8w0MUhUmpj5//9jC6FNjs1K
B9M1XSvHa7OJbdQmo9aRyC+hSKJybRTpcrZGDJXtfff7PJ/na0ZEbJZO09DQ
2P9///6W/9exofwOZpCqti8nqfTu8drANp/TJSw3o3dvZAmplWf/OnyAfvoB
q0H84ZJ/wpXKlDcpj2ecbmMJTSOcXBKKK1P7Lo6r5e9ZJte8QmwSaiuNwpac
HJGrWROPJ01NElort+ZTfsNyLRCtK97R9fO7SvXjpLJBuRH4SWP9J+PHK28t
bJ6bfHIFqBTW/RqhWhhptaapwtkBnjnv4d0UL0BDnjqlTt8JjEeGK+37DXG0
wijkcggTuuwmY5hvvsOkILpxmiUbAvJ36j9xNMPr8qAjnCA3GC38OiJbvQxN
40RhE0f5oNNxz4NvaoGKqy8eJ0dtgvDkrt/XPVqJjbLjJQdyhBAaWphz6IY1
nmjp1DFv9IbEVfrBKwPssKnmafx8zmZYBzPmL5y0xzc63fYFbb5gPvtYe8NO
B5RF22av9/GDiJwEZ1KxGtWMFL+4fn8Ypz39x3z2WtRubeNviN8GRxzsSr+J
GXgjTTQxoNoOnvtfrazMckS6cmJAeHwHlE+nDsR8csLFAy2ZWTN2wpMcfRfO
qvXYH19/Jvu3QEjXzz1eJ3PG/GihJMVEDKZ54cKkFxvQBtq3NbaIgfdn0JwP
y5iokcpU/NMuBmeXFR0Flkx8PpA7ZtsphuhP/Z/j7JkYn7b3/JnXYmg+FbPT
YAMT64fnNHh/FEMW7b1yty8Tgy+6sJ7RJMCbSc84d5iJlz5fNm93lkDw4cE/
bXuZGOU9O4rGkkDmmiq6fx8TeVciqpzYEqgTvPc/9JGJwz4bgjL4ElDzvPb0
fmGiy9WW9AA/CfQvCuhsW8jCv7bSdLrCJcDRvlp9hsdC/aI9qp5sCYzmSwZL
lCy0lnss6syVwOoXbTpaJSzkSq3YrQoJTDaHxe+oYGG0Qd+5+nwJPN41dH5h
PQvb91Orbt2WQLrKVlnXy8Isxo7Io80SALqpbIUOoGUpf3i5JgHjgoZTDA4g
56yFodkMAu6JlAEP3AFFu2YxTbUImDK64CgSAMqNq+W6cwl4OmXrd94H8O9Y
ls2EMQEPXTFvlRiweB0jrM6eAHVwonxjAqDrnaX9oWICZNp1el53AY28Ehdt
JQnwtGnPCqkCHHrdKWAHE/B9c+u8U7WAGXNS/zAOIyBB8fO77kbAke20PTUx
BOw5+u2X568AsycGP9LPEBB17YRibJorajKKx5orCNDcp7x3W+iKbXV6yyuQ
gB951cZ3fF0xf2eEf959AmqVhtY121xxe9KKkoQ6Algy5tgo4YqFz/8ba9VC
wDmzrqWVMa4o2Xfwy9FBAn5t1M4wz3HFe0q+ppMpCa3T89L0prGRu88mnaCT
0EU42I7Q2PhwrZ6d3IwEkYXgzUtdNjaVvRC9tiBhXlBT7IfFbHxZHV56ag0J
0ZFP+m6vZ+Pn9pSIHk8SMuSezKQYNiZkxs3S8SFh1har++EH2agZGHiRsYWE
H+jlHSEyNtJ6LR6dDCBhzLVQmZnGRqOhsuWMH0jQtnjS/a6UjWs0e7pOJJJw
dxrnD9E3Npber4kqOkJCMWPqjJzGQefka9rdySTUKJ+sblnAQbZ21Lq1chK2
Fxn1XF3GQR8DrQuvMkho8a6g793EwfCVNh5rbpHALfC8UH6RgwqfuLKutyQw
BJamiq1cjExttXz6gYS9vYvGYkguOr1YnVk7QIL37E5hcAQX66nhAwUjJCyt
Fnf/KuPiYAzpcmiKBKY6lnfgNhcdsjxxmQEFvtPNG4RL3fDL62v2JsYU5Gq2
Vy9Z5YbVFrTsuaYURKUvt17EckO/wqpD499TsDU37H3UDjeMrXbkPLSmwGAZ
vfjtBTe8229WG8qloP7llTIDPXeU2R1kiHkUWG7qfeW7xB29ozqvbBFQYJ7m
nFju4I49U6kyF28KFDPnm+lucccZC3Q26ooo+KpoLHqQ7o4Cx/FHN/dRkF24
ljdpycOWI/XNk5cpYK4t0+VG89FDXZBnc4UCK4vr9fdP87Eq5MJByVUKBpu6
/z6h4OMNH7FNXQEFU6qmUVUHH4/9Z/xYejkFybW7f2GzN+L6O2bg2ErB0wG7
jhtmAlTaahmFdlDQNTMyUI8lQIvLg0NZnRToCkP8GkQCXHi8JHNWLwXTVFQ5
L0OAQ/6e6paPFDy4bKf3k+EmvKSKvRE1WwpnP4U4Vi/xQMPgwKQ8HSlwT/bs
W+Dugac6OKJOXSlIWK8WP9jtgXE4bw7XUAq83PL8yJseuPl0rlR/qRR+3zVq
1c33xJmWTd/d3CAFE99UxraTQoy/WDT6liWFRDxLPiwSomp+Zr0JRwqi5P0/
FXcL8aVaGntooxTUl64L9Zy8sLTmyzNvfync31zVoRr0wv193XNoYilo/Bt4
4/8A/YSAlA==
       "]]},
     Annotation[#, "Charting`Private`Tag$16400#2"]& ], 
    TagBox[
     {RGBColor[0, 1, 0], AbsoluteThickness[1.6], Opacity[1.], 
      LineBox[CompressedData["
1:eJwVznk41AkYwHE6NkkXhZ7JPFtY1AopOccr14z4jaNsMW6Ve8ZvQy2Nzbka
hjKPjpVMKV0jGyIx87Y9KYXF07CWrs01iCkxZratbf/4Pp9/v5si2f4HF6mp
qfl87X/rAj/NvRMN0MI+tMku5zaJC9pC+/34jc5ueqPD+dwySclfWelU/mPn
rvDxykDuVYlgWNC5hN/v7E1h2zpx70rKZBfmFUVjzpQbzDhzbptEL2Ez732R
wtmkS0nZwO2T/CCK3jddtAw03O8Gvzg+KlF05jZPFelBPJEeqMyYl9St61mZ
xzOF7tDNk2rxy5CzdUd3q8N2iLk9R9wJX4u6ngpBu44tlDcmzFpO6OJsq17c
pTga6BeK05yHN2JuGFX/zJbdoHgmFXfv2oS3isKyXcPcYTxpTFZobYSUY6yE
hRw6dKZqC/dSTLD6+mBn3pE9sFr7ZmzAMzPsyi9oTL9MQAiN/VtDzfd4Ujqk
ZdzlCw36jpfzgiyw+1FvxhpXfzB5EP0lQmmJw1qvLW/3BwDZnF/rE7od81O3
Ce399sHkCTNz02vWqLAR7Ds2EQitMuZRX82duKKvn+6YsR/qz6oWiyJtsOYM
a2HywwGw/vu91b+Vu5BauzBJFASDdKVqI0NhiwaT0l8rloSArLUq02yHPU5k
PC0WXgwFVWnF1MAvDihKJSIEG8LhnU9STu9zRzSHP/d3ScMhRe6QwtGgoU5D
4oc3wgjoa2I8fxngjC73DSfiwyOhqsqm44Er4INaurotJQqChiagfQCw2u9Y
84uRKOgYcTf7Pd0FpdlPe5SXomEgqSnFSXs3xkWY8GbYB8Ho8NwaUf1u9Ns2
G2VidwhGNIW5hQGumFn46rz04yH47DOR4zLmiuvK+n8MwcNQlpVMU+a5odxS
fiOYGwMzI0JGDcUdqffT1MttY2FCazTUUOSOdXJNVcOiOEhrUlKveXlgcaPY
10MSB/9UGj5jvfDAXjMuo5YXD+V2Vq++y/BElnloZYlXApyrtDSyW0NH229F
unVLE+HR5OIL9kI6pouXWdzuToStR3l+LBoDl05nXdnETwL7ISL3bTcD558s
FycGs+FSyk3fErYXlrd/UR3X5oCoIOANrNiDEQpNj585HGDnPibiy/fggIoS
ye7jwE8ONu8f2nnjnIeT6NzOZAh6Phd9scMbmzV1NUZOJ4NLi7yrhOWD26s+
WhssJMNVmkVK44IPEnlv+SWBJLwE+om4kwR6evG9bfaTgBmT2nOFBMIqO82h
AyRk+RdUZRYTaFXGzzUJIUHu1/hYICBw3VW7DHEUCcN20yslFQQOPiqOneKQ
YBQWcF6njsCYpY5udB4Jnzd4NrYMEhjRPqo+XUjC6r0chudLAoOKTklK+SRk
N1UP9rwm0Hv9mP2rUyRIWa5qYyMEWhiftko9S0JPHs1rrZzAebdxatUVEqpn
294cXMLEGY3SIUY1CZkq/RT5N0wc73A6P3Pt609alkb6ciYO7C1d73CLBBa1
wqJkFRNbomlavXdI2Kiukdmsz8QGU1l7Wj0JOVeMddwpTKyZKs03uEtCPj2s
+g8DJlYekS2KvUcC74lp9/BmJp6zFeCq+yS8fngvmm3MxNOfaNz6FhI4qhil
0oSJJ1HmECQm4brKhp+zhYnZOQLlFwkJQn8jw9XmTPwPojhn/A==
       "]]},
     Annotation[#, "Charting`Private`Tag$16400#3"]& ], 
    TagBox[
     {RGBColor[0.5, 0, 0.5], AbsoluteThickness[1.6], Opacity[1.], 
      LineBox[CompressedData["
1:eJwVx3k41HkcwHE8WWVp25w1Gx0rtUsminGM+WQGY/CVipV7TDocS79KCbNK
8jCMa1LpQknXlM1Vrt+nZ7eDbYTNVXmsJym0SBjkeWz7x/t5P681YTE7wtVU
VFQ8v/b/K3znp/6V9ziGTDwZupr6oDH9SXCXt7SGwzUYHEgTF9A5r04mGEmf
chShH4p8xddp2YBMsUjaxfFgxLDY4mq6YOjStDLrPYdxyyvCXPyENohaK/mU
peTMKWYZK8Sd9C/yPT6jWRoQYFsd0Js0SCsVqbUfswxgV/gx39nEabpCt037
tGQDmN4wG1aJ1MDYn7e0Nthbwgg32vV+6Peo76qUNemwYLJgjGYO6+PnBoOI
kghHGLNVPeY48AOmhhgZnv3JCbpjj+m8sFmDd7JCUrghznDGIHcizepHZMQH
Rs2c4kOPl5kXn2GKZTdfK04fdgchLZHb/rURW9LSaxKuErCMbqo9cdcMMzre
aJm0bIfa9SZXNvpbYOvj9sRl3B2g81mf6M4ycUDrH+a9rp3gm77URxFkiWlx
m4rtvH0gOVg+JSqzQqW1zCd+2BcurfzCXb9kK37b2cV3SPSDqP7+qC+h1nj3
bODMyMRuOHJub3fZZRs0Kp8ZIekBsCJmunj5JAtXjXRcuLwoCKi0ejJqYYfD
ic3ZxVeCwV7YU+WSYo/yOCKUrQiFhyufet1UOKA5dPu1dISCMtUEMxbYqFMV
PdFfLIR1fXqfmvkc3Fa3bjgyNAy2PPijRpsN+Kicr8piiGBC0BD4vA2wzDu+
tvedCGzq+jOtqW3YkdLcNluyB+zf2RXpaThhhNBUMhYTDlE7ZbzCMif03vRZ
ZGq7F44fWTQSwePib5l9hR2Te8Esp6lBq5OLugVdh4JwHygMa37bfYiH48zx
WwHi/eAmYjNK1Z3RqO6o6kXWAdAw9Ms9J3PGinHNuSq1CPAPLDrMtnDB7JrG
7S50BHi/8k8wpl2wfaPYrVwSCQsXamwq/V0x0Dy4KEcQBRzPYigdcUXWarl+
hXo0OAjYwrh4PiY0aljca40Gun5/kaqOG6qPnixdI/0VpoQlxstL3HD62ZLG
6IAYaLiQdLLPQYAXmxbmkpbHAq3y7ETpSwEKlZouybGxwMpZr70szB175hhh
MZ2xwNv1VuL4xR2nXNjy81sPwjYrU6fVGR5Yq6m/+F3eQWgNPm5jqO+Jltcm
rVbNHATpn2LeK7knktNvpTm+FCyea6kR2hN0FUg9rP0o4Fa4n+phE4Sltppv
dlOwZW2ilzcQ3FwgTTUNooDHnO8HZ4K6120TG0UU3A45ozT2Ivj6cfaBj7EU
zPO1B3vDCO5Xd+DxJRQkTWl0+WUQFDYNqo5mfrX6SEJrJkH/rFw6X0qBs7jY
mJ9N0EPvvV1fLgWvUzNFNjKCFiZ5m+POUdDdfaRX7zLBad4Ho2ulFOheiyxs
/53g2OL8N25lFFyymDETVBL88JxdOHaDAlH4vsZH1QR7duXr2d/56rxPveV1
BOv3OGq136cgmfniu+zHBKs2DDUdraSgmkjOf/OM4N2P+Wmrqiloydu8VtxM
sOjwkNqBhxQAF5jRLwieZ8lwaR0Fo+m3qgbaCObNO4or6ylg3lazC3xJMAOH
7P0bKXDId2v4u5NgyinZ7AJNwbh5Mse9h+B/gKdcEg==
       "]]},
     Annotation[#, "Charting`Private`Tag$16400#4"]& ], 
    TagBox[
     {GrayLevel[1], AbsoluteThickness[1.6], Opacity[1.], 
      LineBox[CompressedData["
1:eJwVzXk41AkYwHE8Wle6iLXDlE1JNYgwcr05x/Ur0iRMDKlMZPw21xNTGccj
jGserbZrSFqlelKm7Zh582wjNufTZDVZbSFXimJMebLtH9/n8+fXPDY5NF5D
TU0t+Hv/28RcmH3f2O8ePSMbq827JymU7e8LEYg9fI1Hhgp4VdKylznHqYJW
j2cxo5eYvCtS4ZCwQ1PQ5xFMSaa78ZqlVWPn55Ql7zwoDTs5NJ5Mapz4c9F0
idJD1aGimPBeSPc2HtgzVaIFLOfmyIHsEamyI+/+ZIkxhMVnMFVZc9Imwx79
/KKNMF2/ZVztiBZyN2/rfuRiB89dkvxux6xEIz+lsM2ADqbTU1LbcSP89MiY
U8NxBwtbVbr7kCnmRVN/PLPJE366yTLocjLH6yXRfK9oH2hsWZgusLdASmZU
4nwuA6ZtWoIYFEus/13RkX8sEAJbBuqc/7LCzoJC8fFaAsyzRbWnbmzB0/JX
S9d37oJMU1a8VYQNdj/pzVrhFQo8P46+ocoWh5a+tr3ZtxukylbZM5YdFqRZ
i7aH7AHOhprXsfX2qHQU7skcZwJXlkaz0HFAvRd9DNescPBmKhqUMY5440zU
/MTMPlgjFIhEF5yQemt+giiMhLAncpb2ZzqaTch/u6DJgqpN2rx/bLbjeFZ7
qejifmgrqwqz5rtgYxrBFprEwHBt7La8Dlekwd/hnfIY2PDef3Hvohsa3E2a
+VfEBsW2jTF8hgfueLBu/EhMLAhP9qQOuAI+vsVQp1PiQL9F9LK4B7A+JPP+
wHAcTNTIz71J2YFyfnuPquYA/Nm1eKLhB0/ksC2LPiTHA0Nm8HVFvSeGWH+K
s3Q+CAmjgYckXl54onjwrPzzQSjvFI84y73QsKrvFxYeAoVaaQOT9MaPth8b
InmHwVSvQCdZ0wepD9LVz9ETIG/Np2GrSh9s+qj75a4GB5zW6A0V0nyxVCzZ
5SvlQHVLLtPikS/2WvH8bxUdAX67FsSF+2EUbf+lsoBEMAxNdVwY9UP62kaj
piVJQO0dP5ScxsDjEi2bm91JkNHLtShe7o9LpnLqzAVHoTxaPYx2wR/nnupI
kiKTIdTAf10mPQDPtS1+yV7FBdqUq6K5KwDZSl3fk1wubC4OcTgbFYj9Xyix
yS+4sGrOh02bDcRZX7fGaocUmEl9o0zlB+F9XSPt4YoUMNFR7OxeFox2lz/b
m82ngNG3dJPBumAk8t8KypgknKlpvSa2I9AvQBDkGE5CN6mM2OJAICxz1n21
j4S3ikBtkROBW6sEeZYsEqxbDrJOuxJoeMU5SxJHwvKOnOkoXwIVT0oTJrkk
DGp4tqhHEHh4ias3o4iE52PO+gGnCGS3jahPFZNQsVWHL+ETGFFSLq0UkLC+
lqq0yycwaPW77YPlJCSarn1JKSLQZn3F1rRfSaAuVhe9FxI45z1KvVxHgp92
8PmyqwR+0K585V9PwqSuSql5jcDRZ25nP1wlQXb0667MRgL7wypXu1wnYTZC
6xv7NoEPD7gv7b39/Sfe623/kMC7G8fa0u+QIBX3ltdLCLwxWVlg1kyCfOX1
AcpjAi8dG9NI+IOEi63ZXE0ZgdV0IS57QIKeWYY44ymBFQvuvDsPSdgtfb4w
2U7gaRxziZCQwGkQAruDQH6uULUoJWGs/16OvIvA/wCl9mJf
       "]]},
     Annotation[#, "Charting`Private`Tag$16400#5"]& ]}, {}, {}},
  AspectRatio->NCache[GoldenRatio^(-1), 0.6180339887498948],
  Axes->{True, True},
  AxesLabel->{None, None},
  AxesOrigin->{0, 0},
  BaseStyle->{FontFamily -> "Arial"},
  DisplayFunction->Identity,
  Frame->{{False, False}, {False, False}},
  FrameLabel->{{None, None}, {None, None}},
  FrameTicks->{{Automatic, 
     Charting`ScaledFrameTicks[{Identity, Identity}]}, {Automatic, 
     Charting`ScaledFrameTicks[{Identity, Identity}]}},
  GridLines->{None, None},
  GridLinesStyle->Directive[
    GrayLevel[0.5, 0.4]],
  ImagePadding->All,
  ImageSize->{608., Automatic},
  Method->{
   "DefaultBoundaryStyle" -> Automatic, "DefaultMeshStyle" -> 
    AbsolutePointSize[6], "ScalingFunctions" -> None, 
    "CoordinatesToolOptions" -> {"DisplayFunction" -> ({
        (Identity[#]& )[
         Part[#, 1]], 
        (Identity[#]& )[
         Part[#, 2]]}& ), "CopiedValueFunction" -> ({
        (Identity[#]& )[
         Part[#, 1]], 
        (Identity[#]& )[
         Part[#, 2]]}& )}},
  PlotRange->{{0, 300}, {-65, 0}},
  PlotRangeClipping->True,
  PlotRangePadding->{{0, 0}, {0, 0}},
  Ticks->{Automatic, Automatic}]], "Output",
 CellChangeTimes->{
  3.725790454653599*^9, 3.725790514460441*^9, 3.725790551700067*^9, 
   3.725790631266589*^9, 3.7403738145650263`*^9, 3.741166057760421*^9, 
   3.7411663256639023`*^9, 3.741166397999399*^9, 3.741318749767981*^9, {
   3.741320125263187*^9, 3.7413201485063477`*^9}, 3.741335633507371*^9},
 ExpressionUUID -> "f66d83f0-4e88-4251-87b7-7ce26bde884f"]
}, Open  ]]
}, Closed]],

Cell[CellGroupData[{

Cell["Short-range Coulomb exchange energy per particle", "Subsubsection",
 CellChangeTimes->{{3.741166418018155*^9, 3.7411664232849703`*^9}, {
  3.74133560418407*^9, 
  3.7413356053245087`*^9}},ExpressionUUID->"0714bd96-a8d1-4935-bf60-\
0f69d80f8aa2"],

Cell[BoxData[
 RowBox[{
  RowBox[{"ExRCsrPad\[EAcute]2", "=", 
   RowBox[{"ExRCsrPad\[EAcute]", "[", "2", "]"}]}], ";"}]], "Input",
 CellChangeTimes->{{3.722676673170491*^9, 3.7226766840788517`*^9}, {
   3.7226769607964897`*^9, 3.722676964008954*^9}, {3.722677058507019*^9, 
   3.72267715175624*^9}, 3.722750488409705*^9, 3.722750909349684*^9, 
   3.722751650069563*^9, {3.722751697031013*^9, 3.722751701925248*^9}, 
   3.722751733156549*^9, {3.722751776660254*^9, 3.722751780232744*^9}, {
   3.722752400242813*^9, 3.722752400432448*^9}, {3.722752467679291*^9, 
   3.72275252014501*^9}, {3.722752952275763*^9, 3.722752969101005*^9}, {
   3.72275303435499*^9, 3.7227530345334883`*^9}, {3.722754156545463*^9, 
   3.722754156795789*^9}, {3.722754188112558*^9, 3.722754208304021*^9}, 
   3.72275432057234*^9, {3.722754402080971*^9, 3.722754454383902*^9}, 
   3.7227544955051527`*^9, {3.722755499949471*^9, 3.722755529084709*^9}, {
   3.722755602590743*^9, 3.72275561222154*^9}, {3.722755806077857*^9, 
   3.722755808828918*^9}, {3.7227562912298307`*^9, 3.7227563187455587`*^9}, {
   3.722756509642661*^9, 3.722756533689232*^9}, {3.722756667772307*^9, 
   3.722756667930399*^9}, 3.722763826327332*^9, {3.7227640337205467`*^9, 
   3.722764094101956*^9}, {3.722764391670136*^9, 3.7227644061291647`*^9}, {
   3.722765493776552*^9, 3.722765494139145*^9}, 3.7227690116290216`*^9, {
   3.724470727309154*^9, 3.724470739564727*^9}, {3.724470771805664*^9, 
   3.724470785724593*^9}, {3.726898654440785*^9, 3.726898654805393*^9}, {
   3.740374409484497*^9, 3.7403744097069387`*^9}, 3.7403846191115026`*^9, {
   3.741164665136079*^9, 3.741164665361087*^9}, {3.741165865704812*^9, 
   3.74116586682211*^9}, {3.741166428171543*^9, 3.741166438232815*^9}, {
   3.741166673009337*^9, 3.741166673879197*^9}, {3.741320180328374*^9, 
   3.7413202006602716`*^9}},
 ExpressionUUID -> "3dfb4948-85d8-4c57-9320-7d6d626e2f6d"],

Cell[BoxData[
 RowBox[{
  RowBox[{"ExRCsrPad\[EAcute]4", "=", 
   RowBox[{"ExRCsrPad\[EAcute]", "[", "4", "]"}]}], ";"}]], "Input",
 CellChangeTimes->{{3.74116594537556*^9, 3.7411659505081453`*^9}, {
  3.7411664420165*^9, 3.741166448399979*^9}, {3.741166669555909*^9, 
  3.7411666717409487`*^9}, {3.7413201851879263`*^9, 3.7413202036193867`*^9}},
 ExpressionUUID -> "a842e2ea-d338-487c-8cca-f8d86a10332b"],

Cell[BoxData[
 RowBox[{
  RowBox[{"ExRCsrPad\[EAcute]6", "=", 
   RowBox[{"ExRCsrPad\[EAcute]", "[", "6", "]"}]}], ";"}]], "Input",
 CellChangeTimes->{{3.741165952141227*^9, 3.741165955289587*^9}, {
  3.7411664557837667`*^9, 3.741166458935994*^9}, {3.7411666649928627`*^9, 
  3.741166668197682*^9}, {3.74132018654982*^9, 3.741320205987595*^9}, {
  3.741320411380327*^9, 3.741320433555772*^9}},
 ExpressionUUID -> "1f141737-2b25-4ae9-a85a-2339e370a95d"],

Cell[CellGroupData[{

Cell[BoxData[
 RowBox[{"Plot", "[", 
  RowBox[{
   RowBox[{"{", 
    RowBox[{
     RowBox[{
      RowBox[{"ExRCsr", "[", 
       RowBox[{"\[Mu]", ",", "c"}], "]"}], "/.", 
      RowBox[{"{", 
       RowBox[{
        RowBox[{"c", "\[Rule]", 
         RowBox[{"137.036", "/", "kF"}]}], ",", 
        RowBox[{"\[Mu]", "\[Rule]", "0.6"}]}], "}"}]}], ",", 
     RowBox[{"ExRCsrOrder20", "/.", 
      RowBox[{"{", 
       RowBox[{
        RowBox[{"c", "\[Rule]", 
         RowBox[{"137.036", "/", "kF"}]}], ",", 
        RowBox[{"\[Mu]", "\[Rule]", "0.6"}]}], "}"}]}], ",", 
     RowBox[{"ExRCsrPad\[EAcute]2", "/.", 
      RowBox[{"{", 
       RowBox[{
        RowBox[{"c", "\[Rule]", 
         RowBox[{"137.036", "/", "kF"}]}], ",", 
        RowBox[{"\[Mu]", "\[Rule]", "0.6"}]}], "}"}]}], ",", 
     RowBox[{"ExRCsrPad\[EAcute]4", "/.", 
      RowBox[{"{", 
       RowBox[{
        RowBox[{"c", "\[Rule]", 
         RowBox[{"137.036", "/", "kF"}]}], ",", 
        RowBox[{"\[Mu]", "\[Rule]", "0.6"}]}], "}"}]}], ",", 
     RowBox[{"ExRCsrPad\[EAcute]6", "/.", 
      RowBox[{"{", 
       RowBox[{
        RowBox[{"c", "\[Rule]", 
         RowBox[{"137.036", "/", "kF"}]}], ",", 
        RowBox[{"\[Mu]", "\[Rule]", "0.6"}]}], "}"}]}]}], "}"}], ",", 
   RowBox[{"{", 
    RowBox[{"kF", ",", "0", ",", "300"}], "}"}], ",", 
   RowBox[{"PlotStyle", "\[Rule]", 
    RowBox[{"{", 
     RowBox[{"Blue", ",", "Red", ",", "Green", ",", "Purple", ",", "White"}], 
     "}"}]}], ",", 
   RowBox[{"PlotRange", "\[Rule]", 
    RowBox[{"{", 
     RowBox[{
      RowBox[{"{", 
       RowBox[{"0", ",", "300"}], "}"}], ",", 
      RowBox[{"{", 
       RowBox[{
        RowBox[{"-", "12"}], ",", "0"}], "}"}]}], "}"}]}]}], "]"}]], "Input",
 CellChangeTimes->{{3.725790426404578*^9, 3.725790453840857*^9}, {
  3.725790502785564*^9, 3.725790550992629*^9}, {3.726898837998486*^9, 
  3.726898847052638*^9}, {3.741165900638431*^9, 3.7411659400545387`*^9}, {
  3.741166056629149*^9, 3.741166057200569*^9}, {3.741166464014175*^9, 
  3.7411666068642197`*^9}, {3.741166645830902*^9, 3.741166658462842*^9}, {
  3.74132019589301*^9, 3.7413202316535683`*^9}, {3.741320284775901*^9, 
  3.741320289842805*^9}},
 ExpressionUUID -> "e952e9b7-c710-4f8c-a078-a46854ace494"],

Cell[BoxData[
 GraphicsBox[{{{}, {}, 
    TagBox[
     {RGBColor[0, 0, 1], AbsoluteThickness[1.6], Opacity[1.], 
      LineBox[CompressedData["
1:eJwVjWs0lAkYgBulNMlRGHLL7RO7oaaSu3eFhp1cc0nkmiIWXw5HJlmKZGbc
JopqXSM1kSGnaL63lS0VRxcNpa1EqFCUoaNs++M5z6/nPLphcV77ZZYsWbLr
J/9b5LvwdUI4YFdrabPTxOO0OOeffRJPfqv9SETJox/cw1T+84xUbf5deyan
U/yEm0kJhgXdy/gS+01WVHU7t4gqHj8/K+WN2nt/3d1Xz62iVGP0cj/zpPZr
cwqHT3JFlJ8wwmeStwLilrJ7lbgdlLT7xM2PPFUg2zUCXE49oUTKj1Zn5RrB
8TOH66J2D1Pxv27tvWXNhIW3DMNtupMUY6dU0KVkAY5HTIckT2aomVuq0ZXR
djAwnyckpuaoE8HaaiW/OIAh44L/bMV36govOHNHsBNo2rkWTnjSUCMlMGbu
OAsK1NxbFNuWYu2lF91Zib9DNZspXjMliz3ZOa2pVW5QnooJzk5yeKpvUJ7o
8YCeppzhO5F07O18zFHc4QX1JTV1pgnyOCz/elODxBuY6cpyeqUKmJ1kWmHl
6QPtVSXTp1mKKDUX+KS894WVT5kLHl5rcNUzCcuG4w8cNW/TCI+1eLUkcO7D
9B5wNh/ecXS7Emo3zn1wy9kLxuN1y2U3KqPWh76yC8uCoMbCweEeXQXfc+7n
Vfy1DyqF08mZsyooTHILFawLgbtbU5YV9jPQBPr9e/pCgBZ7Nm7moioqtcRO
v6kIheY5qxGtDDX8rU3//aGQMHiq5r7ihus6vN3IollohEPAgaGOoVXqWOuZ
cvPlSDjMaBYkdw+oY1/m/UfzlRGgcSRgf0+xBkaHbsiditsPdwxtqdQQTfQ0
nQnfYBkJjYlLx0/qa+Ex7qvSvi+RwBjSEK+WaKFyseRwEB6AN5KH894l2vhp
06f6vWkH4W+vMGeKtR6125Jp5yyiYCDN12n0y3oUfaJ/a5GJhrEXJVUzvjqY
1yr2cKaiwcUmpiv1ig4+Nk5zacw9BLHLhzQT5HQx0GRfeb5rDBhbc1QvBemi
hY6QIZKNhXvHHgTXNepiqniFWUNvLBil+Al16HooO5lRo8v/A+4Uke1GQXo4
e2+lOHZvHMyKMhyE1/XwXNfit6Nr46FMqhNJKOhjqJTunB4fD+5P2byDwfo4
8E0jLO5ZPNyeqPzBbNXHr862wrPbEkDOp4M9LGeAN+kMuZHCBPAuV0m+7W+A
zOovW7TmEiC9odjQrMEA3bLe8vN9SUi0eSu9uGiAO135bHN/EvLWvB5fTSMQ
FCzpg3tIMI7p70+UIXBzMf/EhiAS8k07hA6yBCpftOSIw0nQM2rZ8i+dwBed
eVEf40mw4tZfU2YQeFDWxpGVS8J5q6aMYxsJDO16R5vkkmB+tEn1nQmBAbwC
qohPQtiDsUtsMwLZKqNWrwpIqL/8o3Mdk0AzonBz0pmfP1vaS9F2Amcdx7Sr
a0igx0xkjzoQOCVXNOhSS0LQoN7nXY4Ejj20LZ2qI+EGt96v2YnAgd1FKtZX
SCitbNX8k0Vge4Sd/OMmEr6bzWepuxHYYjTeldxMQhLz8/N0dwKvfizK1rpO
gt8ul42jHgSWJ47LRN0g4cJlnbsibwLPWghQoe1nH1ilqO5DYOGCXVpzOwnX
ZHh+6b4EnsJx6wAxCSu9XpW98yMw87hgfpEioXax7CV7D4H/AaNvVKU=
       "]]},
     Annotation[#, "Charting`Private`Tag$17358#1"]& ], 
    TagBox[
     {RGBColor[1, 0, 0], AbsoluteThickness[1.6], Opacity[1.], 
      LineBox[CompressedData["
1:eJwdkAs01IsWxlHJEQoxL8aMTNNJZMqrh2wkKtVMUSHTzP8/R+eEVB55VSqP
6zEogyTJIw49JJXoaHZSokghUx4VnXvLM3VEKeu691trr72+tfZv7W99bCJw
+28qSkpKETPzv12588f48NVX62LfCteZ8TPuJTwSdgpSquwX3wxpnE4Okqe9
PhnJTGmw9+ktvN2WfEouey9rnp3SaZ9dmnv+r+R0eebH3K8T0v/YD0esbC5L
LpRT/I2TxqQT9o67D3X/K7lSvuuqxGNEOhe0pkwf6yY/kE80x9YMSSmgM6y0
fWNim7xy4XPNuKQlUBfNufiH+3v5QVPL1to1K6A10IVuxR6R67tMyBp1baHT
Q6ers+2L/EstZX/B/nVgYm9azBmdlMfuZVKzljpCi6Fg+9f8n/Ir0r2nnPY6
w7aLqWnDAmVkhO/xn4xxBdWivFsL7s7CktKu5rjgzRD3IwK1R+dgS3xCVWTh
Vrjk6BOywVkNEzu6NTgtfChZEfOh3lcdWx++iFrgtB0cYzRumB/SwPcaby3K
O3dAT8HoRuNzWhgfap6/WuABnfM2Xcl0XYAT1jKP8IGd4G20/I37dm2c97LT
dW3UbnCLvlwWwtfBa1l7Jgc/e4KXg7Cq1kYXmdcnB7cmeIPYMm9sYtlCNBzs
yLkw2wd4R31i2jX1cCCqKTU/Twjph3gNmUr6eDV0q1hGEwHXqncTb0If23KX
bYw1EEFfQlz36Hd9/Favzgs1EsHgZ57W9Wl9dNZtUNrNEUFkVTVppUrBnnL7
iwyeCN6pvqp216Og5keLNwWuIoj+9ihhaCUFA7x1fSqOzNw7hTfcPUzB9JNj
6wsiRPCr743LtaEUrC59tiz9qAiCnmm51UVQcM5k0o/gUyJIae5uajtJwVzZ
7PO2qSJgXWYupaVTsLl5/LW8WARXtn1Ya3OTgmag2N3SIQLZuHMd/RsFlTLX
lUwrRGA1ndYy8JOC7YNF4+bdIjh3o1wFVagYlXXoTGqfCBqcLjEiNKjYNKL+
lD86470cIpezqOiba2ffpiaGzT8YUTdcqXjxewFHsUYMWUPtYY0XqBjM/yVY
zV4MDGvFtF8RFV2KA+tsHcXA9rT8ol9GxRHB2r3ZrjN8apBj3C0q2pV2nPXy
EEODyWXlZ0+p+HqXmkbPATFs8Kfs4/6kou6tgM/v8sXw5+qX7Sq+NFwmdaN3
F4nh0+Nr/JP+NFz/m6njyxIxvCjJ8NUMomGo3sfTTVfFUOOdZecSTUNFiIRX
WS2GW1X6lVtyaHjB2vtgzHMxSF8Ih5600bBKa/XZY+1ieKptU0rromHrv6kY
1imG4Db+m5A+GipnvZwf0COGLp5FhNcYDSUTgnKPj2JgLWCpvZpPx6V3XEcW
KxNwXMtNtWsbHZ3SuPrs2QQMn/i9i7ubjnt+V13HmEuA5KFZZpyIjlJqvXS+
JgF1lomOEYfo+CnM3mySSsCbtEI/Bxkdb6+y9m+0IIDw6z8f30NHh7uLBvxE
M/zCnDlvoxlI2RZN30USsHSqPKQiiYHDfd2bHH0JCJp6q5KbycBs9czLVH8C
Wu//olN3hYFjnmoBD48QYPeoRch/zcD8yaFRZioBg082HW5abYBHkjey1M8Q
UDMdni52McAtrGL+uIwA8o9PMqq7AX5z2Vvx5BwBGxTmwr8DDFCQ9fxwWDEB
7v0NSuqFBqhsfXv8eS0BiQ4WXl26htjZqLO4FglI42S45Rgb4lWfwJ1/PiAg
vZT7NJpniJ6xS6qONRIgiOLW4DZDrGg/F2baQcB0q2c8K8UQxUHHp2KGCNih
KNr8TIeJNnO7TQ+OEqDlsbbFzISJmjm2e7w/E6CnqNtfY8XE6rqxv3iTBCiM
7WzFnkzU1pEc651Fwrw23r7xAibev+6qbMsgIZIeAnftjXB9kNlZgknCmfvf
VdV2GuFjK53lUjYJj2NWfM/0N8LWmq49fVwSKm7OjTh2zgh76w/cSbYk4XTQ
TcOUb0b4XSELfLeFhGpv4UY5wcJjOeGqGgIS0v5pjDQ7yEJloTDX2p0EhnnG
4fqjLFTr5z5J8iKhLDR3/YFsFlKGaxZb7yPBlHb7Hr5goaXyu57EaBIm8xKU
erew8c6Dh8G3Ts38v+TpQhWycU1c2by3cSQEmtLcYg6w0XFe8CorKQns5tkO
/6SyUaA3N+NN9ky+wif1zh1sPPCrmZtlJQl5CVcynPcb4+dB7X7hbRLUeyKc
ho4aY8i1r+EJ1SSUo/k/z04bY9RKLOmVk+A364wLv8YYE+12zEp4OpNvn/dF
N61FWCIIr+n5m4TEXRuWD9YtwoOZL5e++EBCa1HRJ86rRWjbtTLn0SAJoUqx
o3mji7BJMhJZPjbTz/Q1nrehCQ4dIe1O/CSBo6Zomog0wRUXtqCJngQYbSx5
9AYOTvWVWdCoEqhiMKdYYg7Wc9XyNRkSSJIxh7SiOOhRUXfiK0sC/TIbT8UN
DobV2zg9XjbDj5hpW5osxnsD7Ed+6yVw2jog5r0+F+OXH7cWuUhgoqc/q9ma
i/zg7mL3TRJQF+i16e7i4rufmfF2fAmomM1fUn2Wi9cHsgdWeUpA6f9agv8F
RdCYVw==
       "]]},
     Annotation[#, "Charting`Private`Tag$17358#2"]& ], 
    TagBox[
     {RGBColor[0, 1, 0], AbsoluteThickness[1.6], Opacity[1.], 
      LineBox[CompressedData["
1:eJwVxXk4lAkcAGAqm6Q2d7EmQ9/SQYlEGD8bEyXrzq2JckTGR1o5kjOMSUzj
SFtIqs3RSrZovt/qaTOKrp2wKSkl0pBr0FS7+8f7vPR90W77F8jIyOz+z/83
ekmnP9b2MopfBTIMXU4Lcv4K7HblNttYXj8s/MqJpQr+SUukce/ZBLysuvGU
k07xBnmdi7jdNpWXz5a3cooo/vDZGUn+kM3QUZPOK5wqSiNSN+9TvsSG5x3T
d4LTSO2pDfEU5y+GkhUb2lU4dyhJZ+at0XwNKHT6zs0x9ynVqPp4WVaeAUin
RyrCPQYp9nrTR7ctN4NpjZLZFrqYUt8h4QlVzEHZTmrR83SSmrytEVEZwYA9
PONk/bFZKjOItrJ43U8wvkzniLTiC3U1Pyh9e5A9OPVHXptxlUWtBP/I2QwH
yKhjeui3LMSay887s+J2Af8raxLG5LArO6c5scoZzEYTL1bby2OuqE+R6HKB
+8kfadGhCvjo7pOkFdvdYGP1jy07SUUcVHy1qb7bHdK+lPfPnFmO2fFGFdtc
PeGQap+s1HEFSsx4ngkjXjAdRrSxPZRw6bNuB6skb+CziLCj7spYV+w/+2HC
B3RNXPi3LVWQ1jD7wTnHDxgKPnb9xqqo/UF05tdFAUAy4+OTldVwJKnjZMW5
QLB1H5r4TUYda+OdWbxVe2FHXGnVubfqaAg93l2ivVDiMHfBsFkDVZqiJgYq
WPDyfoG1F38l2rbojRzcuw+Gnj0P2xq8Cv9scJA11wqGsjNGuzXXamKNa8Kt
F2+DwdAn9V6bVBNF6R2P5ypDwEpNyb6Z0sIIln7eWPR+CJqwCEst+AFdjSaD
9S0OwL2pUC9TP208xukvE00dgOmQmzHx6jRU5XfHBmAoSK51E8J+Go5vGr/i
lxIGcqETttvLViOt5YhsuXk4mMz1lIn1dbBxXGG+aUEEHFfNtX6Zo4MnmwUu
TCoCDGM617cN6uCTtSmODXkHwVaDf+lvJh39DQPPF+yMhNcnMo8tqaSjuU6t
eqNcFBz8eSDV4DMdEwWLN9Y/igK6l1Nlnp8uyonTquncQ5AQVWLg0KSLM+1L
BFF+0bCSOVrmrq6H5cJv88nKbLC/k5zCPqyHLIkCM5XNBgtfzQLFLj3sndfa
F/2MDbZBSinyRmtwmmldW7olBuTgizIvew3eUlCXf1sYA1l2E6fd+tfg5gtT
JtqzMXDH1OKPFAaBzllvuAVeJLTTl1K7igncsZPrZOZNwuLYaLueEgJhuYVC
nw8JvQulwpAyAo353Ez9ABI25ReKks8SqHrRIkkQTAJ1UySuryLw+d2T4aNs
Eua33Vin2kBgmJyVnUMeCb+0PXjY104gS/hOVswhwfDdIf/wDgJ9809RRVwS
9gcEDE/fJ9BJbWhb/ykSfM/pLfr+IYEbiULj+BISwgSx1rYiAmfs3tMuVJOQ
0a2M1QMEjskX9TnWkFDA+uy6+Q2B7x9Yl41dIsElwHZQMEhgr0eRmuVVEkr7
hpf0DBHYGsJQfPI7CautOnwUxAQ2GQwLj1wnobW0RcwfI7ButChb+wYJ+pRy
ht4nAs/HDS8Iv0mC2/GZeqspAkvNebi8hQTehkymcJrAQikj5XorCXWtyS88
JQTm4rClr4CEyK0Dca9nCUzP4M19o0hYVtmgGD1P4L/d/F/I
       "]]},
     Annotation[#, "Charting`Private`Tag$17358#3"]& ], 
    TagBox[
     {RGBColor[0.5, 0, 0.5], AbsoluteThickness[1.6], Opacity[1.], 
      LineBox[CompressedData["
1:eJwVxXk41HkcAOChPKSplWMUO3J9o5QuFamZTylnzeOIyDmuInbGr2SnaDfn
YgwxRVYtpayeHBnylOP3oaetqahYIXZTK1HuyhG7dveP93kNAgWuIYoMBuPg
f/5f5jH/ZaSsm5Pb58fZ4HyhMfU3v04XSS3Xujpa/o/4BJ31Kv6MnuQh1+fP
a3faxQm0tF/asljSyb1aermgXpxDXxy6PDWd8Z47cHpry03xNVo7wjB9ImOa
y/GM6v1JLKMPlwW7j2YoA3PO7JGG+D493ZJ0bzhDG1aOMFwd0tppmeaLZcnp
pmB2jhSGHeqnhWYWzxustwBPbKezzWCUZtlNS+UaltAq0ujpbP9Ef2rQDr8a
zoHVfKsbZGyGTvLXW5m7bi/YaVS4ThX9Td/K8E+w8d8PjKKc8yMuCqgr8omY
SbSHtRNdd9XqFmFJaU9L8kknqLzS17JiTAlbU1Jrz1zjgVtm/GXb/SqY1tHL
JK3OUJ1o4fQgVBWfP2iLVbNxhfU8YfLGKCb2M/s2VXS6wevysQGj/OWYcsq8
aKeLO9yelzXl2qvh9Hapu+iDBwwfln5/yHUFLn3Zab8r1hMCQhRjwp3VsTzX
Z+bjpBd0mbaWp+zQQL3KmY+8VG+YK1NxZK3XRPbHjp+vLPaFZW+aR96qauGH
2MeZRb/4gVbqQdmtKS0sO8XjS1cFQMxiBudZFws3QJdna0cAVCWmVzqUaKNG
TeTkmyI+eNr2P8mNX4l76ow+HA8IBMb20CZfp1XYVGmvYKkbBAeFvl/qmDpY
4iK698e7INh9zmLVyCsd7Eh4/GL2ajAICqpMOXm6GM43SR8ThEDOTOW8W+C3
6GL+KcjEKhT4Iv24HsLGH8Sv8zs+h8LvD/Oa33WzUfNi5wlfPApCtb609nw9
HN80ftP77DGQDe6wmjywGvXqYhQKLMNgbnBgvG92NcrGVb/WKIZDNZsvH/LS
x8zaRmdbOhxs5Ob+4xX62Lb2rENl+nFwIDZP45gG6LPBrzDLMQJcBJ4hroEG
aKlfxpIpRcIKVpP9bI0BnmlU3ljxPBKE2SaiHWqGqDQaf91A8h0Ua6y9oBxs
iFOPljRGegtgpFTQG91oiAXyha9x6kJYn8J60c8yQv60qu2PQiEoNgQ0s8OM
sPurbqDgpRCsI4qrFjUb4Rfb3WWXtkVBNK8+r0XTGO+pslTeZUeBoINR9TTE
GLcUf97KnomCZ5senUxqMEZe8l+SLA8KjM1uSvZ8Q9DOUXJguycFTl0qjuVq
BGG5lWqvFwWi3uRFuuoEN1+UJJn4UqBrOCj8rElQ84ZVbGMQBUSR2laiQ7Dn
QWbYsJCCJ+lbjzLXEDymtGuffToFyiK5qGMXQb58QGFUTIH524T5PRyCRzLO
0zkSCvwnLsSVcwke0Hq/8/V5Cta9eng6ZS/BjSR786k8CiazsvlW9gSn9g3q
FV+nIHYp922BG8ExlZxehxIKQnO5TkvcCQ4+3Z0/9isFb9qqqqI9CHYfytGy
vkXBnMJMLM+LYH0wh9lWRcH9GrOFBT+CNaZD8phqCpbuHPeOCCBYPpyTwr5D
wZoyi9ouPsHCk0OKYXcpGJuwCbsdTPCSpRSX11FwWlUd2aEEs+c5Z6vrKThR
GKqVdpRgGg5ZH2mkwMLdJmzqGMGEROnsAk3B/seldYHhBP8FSf9UTg==
       "]]},
     Annotation[#, "Charting`Private`Tag$17358#4"]& ], 
    TagBox[
     {GrayLevel[1], AbsoluteThickness[1.6], Opacity[1.], 
      LineBox[CompressedData["
1:eJwVjXk4lAkcgI1jTZMid8kw+HbalC61JDO/kttaM7lyhVEi1swXlUJtE6UZ
Q4hy7GJEelJKsiHfr91VtKsVD5NiS0kkdLg6Vlt/vM/7z/s8Lys8jr9TWUlJ
6YcvfHWt76epsepeTv6TEM5Kr9PN6bdDFDxZPdfuWkLbnHQvlfXw6CGm7A43
+F/59S6pmModzG1XlSm4ZVXFRU3SHCpvpHh6JuMFd+jguvYLUjllEGMmeZMx
w+X6i/pOSGspv+oIn/EMdZj/0bJVR/oHNdOe2vAqwwAMx5T4rie7qFrd+wvS
JMvgryNESZT3ICW0tO64abcWWuKcl6xnjVP6zjO5bTo28NBH+5Gi6x317qZB
dFk0B0q5lhXExCyVuoNpmL98C7Sa8/jTpf9RFzN2iB12OEJvY2bWGI+GRolB
MbPHXMDbrKROq1EFK6setafFu4Oyy0FcNKGG946n1x+Se4Jbv3WCkyMdT3b3
aRD3vKDY7+nQn7sY2NHSmaTlwIdAQVyFlUgDBzWerL6s2AYrXPM+sgoW4vF9
VqUbeT4gSq4aPO2ihTMbcn0SX/qC5l29Z178RTi/R+GyKckf0nxH6BFe2ngp
P2h29O120JS/0E3+XgeZNbOjnumB0G/B71ZdoYvGo92Fv6gGwwGPAWYrQw9f
Jt3NLP01BEyL48XiaT2s3ucZlrs4FL7pppHZD/RxJTzwv9cdCu8Px6VMVhig
Tl3s24HSMPD//bam6VFD3Nxo/nJPaDi06rJvN7ktxls1LjQbIwFsbk5vHJ6/
BCt5iQ39zwXgfmJrR0/vEuwW373/viwCkreYzevLM8LoMLZkIm4nTPGCcjJD
lyLP6p2AbbsLlMMlV8vNjfGw9HFB9+QuSFJwJ9cqjFE3T7E3GCPhXCZtJjWf
ia9Xv74QmLIbhIL4qc8uJshs3E8rsomCQu3CH22nTLD2NeNDnXI0eOg4TLD9
TDGzvtnLiYoGjcMJkqaLptj5XYprjWQPFI8b3bhFZ2HQypCSLLcYoHvuHGGE
sNDGtFq/Vi0WErreiI2vsPBQs/qqyx2xsKAusKGaYYZq40fPsWQ/QcXcFa1/
gs1wunVec2xgHESbHNtD1pthUdvnD8naQjDmDfysoWmOYTMMpyNCIWyyzWkl
Q82x94NReFyPEOqmNkLkb+Y45WRffXa9CETu2+QODAtsYOjTn2eLwJ2T3eIZ
YIFryyfXGc+KoGeuR/62xgI9057JsnxJSOwrsCylEejsJvPY4E+CytNvjeap
EAgLbRl920ngpirRRaoErsmTpbKDSVjOl/eCOoG6FbZJzQIShPb9QU80CHzU
khn1SkhC7ao7g0xDAnerbdrqIiHhTFGyeoEVgWFtQ7RxKQnym77ltNUEBmSc
onJkX346NzhRawj00Hux8fEpEuzZJjE21gSuIrLX7DtDQuYBeVWPLYHTW4eZ
5edI6OdaXNF2JHCCntPnWklC+HAY+6ATgcN/2xdMnCdBTHcsHHAmsNc7R8/u
IgmnYlWSatwIbIrgaHReJcEnUsby9CKwbtlI2/5rJISMLUut4xF46VXOcePr
X3rR/qGl2wgsiR9RjrpBwkfr9WWjPgSetcnFhY0kdArOf+L7EZj9iZNyrYmE
St0e7wZ/Ak/iiF1AMwkPluIFVgCB4mO57z9TJByRRM6dCCTwf7gAS8M=
       "]]},
     Annotation[#, "Charting`Private`Tag$17358#5"]& ]}, {}, {}},
  AspectRatio->NCache[GoldenRatio^(-1), 0.6180339887498948],
  Axes->{True, True},
  AxesLabel->{None, None},
  AxesOrigin->{0, 0},
  BaseStyle->{FontFamily -> "Arial"},
  DisplayFunction->Identity,
  Frame->{{False, False}, {False, False}},
  FrameLabel->{{None, None}, {None, None}},
  FrameTicks->{{Automatic, 
     Charting`ScaledFrameTicks[{Identity, Identity}]}, {Automatic, 
     Charting`ScaledFrameTicks[{Identity, Identity}]}},
  GridLines->{None, None},
  GridLinesStyle->Directive[
    GrayLevel[0.5, 0.4]],
  ImagePadding->All,
  ImageSize->{572., Automatic},
  Method->{
   "DefaultBoundaryStyle" -> Automatic, "DefaultMeshStyle" -> 
    AbsolutePointSize[6], "ScalingFunctions" -> None, 
    "CoordinatesToolOptions" -> {"DisplayFunction" -> ({
        (Identity[#]& )[
         Part[#, 1]], 
        (Identity[#]& )[
         Part[#, 2]]}& ), "CopiedValueFunction" -> ({
        (Identity[#]& )[
         Part[#, 1]], 
        (Identity[#]& )[
         Part[#, 2]]}& )}},
  PlotRange->{{0, 300}, {-12, 0}},
  PlotRangeClipping->True,
  PlotRangePadding->{{0, 0}, {0, 0}},
  Ticks->{Automatic, Automatic}]], "Output",
 CellChangeTimes->{3.725790454653599*^9, 3.725790514460441*^9, 
  3.725790551700067*^9, 3.725790631266589*^9, 3.7403738145650263`*^9, 
  3.741166057760421*^9, 3.7411663256639023`*^9, 3.741166397999399*^9, 
  3.741166542593484*^9, 3.7411665895018*^9, 3.741166622965687*^9, 
  3.741166683533572*^9, 3.741320237523958*^9, 3.741320293440097*^9, 
  3.741335676988141*^9},
 ExpressionUUID -> "f01c5285-5862-4179-af7b-362c93247a22"]
}, Open  ]],

Cell[CellGroupData[{

Cell[BoxData[
 RowBox[{"Plot", "[", 
  RowBox[{
   RowBox[{"{", 
    RowBox[{
     RowBox[{
      RowBox[{"ExRCsr", "[", 
       RowBox[{"\[Mu]", ",", "c"}], "]"}], "/.", 
      RowBox[{"{", 
       RowBox[{
        RowBox[{"c", "\[Rule]", 
         RowBox[{"1", "/", "2"}]}], ",", 
        RowBox[{"kF", "\[Rule]", "274"}]}], "}"}]}], ",", 
     RowBox[{"ExRCsrPad\[EAcute]2", "/.", 
      RowBox[{"{", 
       RowBox[{
        RowBox[{"c", "\[Rule]", 
         RowBox[{"1", "/", "2"}]}], ",", 
        RowBox[{"kF", "\[Rule]", "274"}]}], "}"}]}], ",", 
     RowBox[{"ExRCsrPad\[EAcute]4", "/.", 
      RowBox[{"{", 
       RowBox[{
        RowBox[{"c", "\[Rule]", 
         RowBox[{"1", "/", "2"}]}], ",", 
        RowBox[{"kF", "\[Rule]", "274"}]}], "}"}]}], ",", 
     RowBox[{"ExRCsrPad\[EAcute]6", "/.", 
      RowBox[{"{", 
       RowBox[{
        RowBox[{"c", "\[Rule]", 
         RowBox[{"1", "/", "2"}]}], ",", 
        RowBox[{"kF", "\[Rule]", "274"}]}], "}"}]}]}], "}"}], ",", 
   RowBox[{"{", 
    RowBox[{"\[Mu]", ",", "0.1", ",", "3"}], "}"}], ",", 
   RowBox[{"PlotStyle", "\[Rule]", 
    RowBox[{"{", 
     RowBox[{"Blue", ",", "Green", ",", "Purple", ",", "White"}], "}"}]}], 
   ",", 
   RowBox[{"PlotRange", "\[Rule]", 
    RowBox[{"{", 
     RowBox[{
      RowBox[{"{", 
       RowBox[{"0.1", ",", "3"}], "}"}], ",", 
      RowBox[{"{", 
       RowBox[{
        RowBox[{"-", "60"}], ",", "0"}], "}"}]}], "}"}]}]}], "]"}]], "Input",
 CellChangeTimes->{{3.741166702088785*^9, 3.7411667403449783`*^9}, {
  3.74116711726934*^9, 3.7411671242508717`*^9}, {3.74116715876818*^9, 
  3.7411672068705463`*^9}, {3.741167873686638*^9, 3.741167910298462*^9}, {
  3.7413202993838654`*^9, 3.741320377250519*^9}, {3.741335745391975*^9, 
  3.741335789485965*^9}},
 ExpressionUUID -> "976156bf-7e26-4ad3-8d91-cb7e6b6e311d"],

Cell[BoxData[
 GraphicsBox[{{{}, {}, 
    TagBox[
     {RGBColor[0, 0, 1], AbsoluteThickness[1.6], Opacity[1.], 
      LineBox[CompressedData["
1:eJwVxXk4lGsfAOCJMa9OKEloMcZRpilKFBK/d8o6lqQ9FaZooxLpSoUUkRQq
pOSkhWoqiuw9D9GCCiUzx9I7YxuRNZGxnO/7475uFv+om7ccjUaL/p//n1dc
mZRyswAcXzbcnbPdBpe3x99t+1IAERcn6p462OAalR1PDFUKwSz7nvIGCxss
9ex8XRZeCG8nM8490rbBmgr0jh+Hi6BGK+FVSbs1Dna2NLGwKgFd+rejHies
MbNvm9TPHwMv4Pbw5ZT1WBJaeUFlbjnYMoIeVsu42Ge9i3bGqnJQZgwkO/Ry
cRejLg+2lMN7jVcxnyku7o8V/Th2vRw8L8p8f1dw8eQtqeuX2RXQmc488D2O
i+fnMxYmz3wLP+aSMyT6XLy5f10ua/p7sHIt9M3eReK3nkXtJuNVwOnWq84p
tcTKBVnBuVrVEHk75FK8wBJvVn04c7VpNUwICZWzSZZYUhpnbnq8Gkw1VTeG
+VniSV2fWHNpNYTV5FuYzrPEq9pnrbL6+hGYcVNL+EFr8f2DPhfsBJ8h/sEz
x73mFphbEKVq8KwWwiO3ze3sMsPBDjft7xXXQkv+Ysd/hGY4R/QoVKuqFqQ1
Bi4+78yw/ljlTwVpLWzV2XVf84EZVrZQrmxh1UF2m/SbupcZFhXHh8fdqIOZ
QWanfBtNsT9OGRo68wXusw0d3UWr8d13gvpCx3r42X3Qu3jUBO88qtxwyL0e
hl/5/bTsMsGzNY4I5x2uh3WLs85Wi0xwuM/yxuBL9XDgzZOEWUUmmK/wglrz
oR4eGQXGGYeYYL31ed2Ftt9g25ewriaGCc58XTqtiNsAbsZHzp1lGeOs3G8G
RaYisNe+tW78lBGu1O9f5mErguouqZrLESPcdnP6MvktIlAZMeY94hthzZC1
HMfjImCN2X047WiEQ23TFzcKRJAamcCLW2iEXRr8mDLWvyCXKOT4v1mBf47S
VS2UGiFVkuIvVl+BOWuNfxVSTeDY3zsmyzDAZRW3S5L7m2DV4X09TtcMsPsG
xsUgWjO8C2kZfB5igC/zRVordZqB+sqafLLFAPdFhcIjj2Z44i7mBdMNcE59
1aWklmZIST7x1st7GYaj+1iBTS3wIyPqWa/xUsyp5WXM9aUga+zKgVe0JVgu
ihdOBVBwzrrSwqufjUVWvN2PT1NwSJ9q16LYOErgoGYVQ0Fs5MmYHMTG7Rft
Q70fU7DyZUJ+bCgb/2Nluy1HSoEGvSm1fBobqwu4hJu3GD4b/CnvnamPaRfN
9sfukUDdHgfZQ9dFWPHeHG6ttwTqv5ZnOlkvwrNQ/zx1Pwms2fCuWWa6CLNG
Mj/dPi0Bp6vtxUHMRXjdfq3VgmQJHNv40qe5Vw+ftxujV9VJgKe82Hz/VT3M
UCxOV7RrBS0nXrVJw99YKRpazi9vg7TB7ZHKYbr4a9b61H2mbSC/++/NskBd
fEtot8sG2iDTwUt78KAu5rBd/2VsaIPxUlrk2CZdbP/O81v0kTbosdHLOcHW
xREK4Z+uPm0Dm9BRc5UvLDx5rvz1raXtoIs/EFcNWbgv2CHtpX4H0Ib3nLIe
Y2IpwdmtsrwDIrgB+Vu6mJi6/tf8g6s7YFXZmk0BQiaueVaVqG3TAb4lV459
ecXELyTOV6L5HWDmaLZwcSATB/HcznqkdoDbceuRGQPaeFzL3X2GWicYHq88
Ez+0ECsW+GrsneyE1juTvl5aC7DklJNuTVUXZLorXvjaqYmvc5afDMLdoOp4
MyxwQh2f0V96/va1n3Bf48KnJVlq2GIORySL7QPhw7Atq+JUcXPpoOdl1A8K
XZOFe+Jn4nxmc9bOjAE4dypNxHmphEOH3z+oSB+E6bmJtfunpmMvf27Qsdgh
cMprlf+rmsCG3kXdeTG/IF4nVeN7jgLelXKNsydiGBbdLBJ87JTHD06MWlsf
+Q1+p6iyyENyWPR+D/3doRGwlubL5YzRMLtsY1r01lHIGmdrboqbQsLxdPkn
ln+A4cGWGQRMoMDnw0oHzcbgtYOxZjhfhpYq1g/46MogabvGUY0Hf9BHYe7p
aTrjsECOLafUP4Jqfvz6NKY5AaLohMmUw79RbzqeMJ42CV5d0aUOrGE0Uhdb
O31iEn7p3M8aFQ2h+Y86w5jSKWgKignmlg2iDdTncYf9NPLeFjs9QcUAIjIF
MW5tNDKE7C5x+tCPPpZtUJRtn0Yy1RMNeVQfir4Z0ODfMI3s8F/B32nQi9ze
7L4e5SxHpo1a/07P7UFVyiO5LqVy5GTeCsFcj260Zo4qp9VKnlyZRjtUrPAD
5fkNxGjkyJM6pmo5VSIp4px3I+cZ00lytkZy7+NO5FzA31H9nE4+q1oxxEjs
QGfXmXtq6ymQabFJ5/feb0f3LsYVWKUrkOMuH2fRn7ehBuYz2pQGg/TjR+62
F7aiImGw4EgMg/zokrhPb3YruuH8/rFAkSB3hcy+028nQWfUmxIvnSXIxtOb
OjYlipHcd0/f66EEeftwYN3Ga2IUldnOvXOOINWU2Odd48TomkVfT3YEQXIs
LI1cL4nRYy+59aJYgnx5piV/e4gYNTxl9+nfIcjEAde1V3zEaKXtCbuK1wTp
k7LGKdpUjPJnji34jAnS3L7OMc1EjCxFIYPCMoKs7P5OvDISI3vfqNSetwQZ
EuWZ075UjDwSbg2pfSbI7Ik5QmcdMbrcUprG/06Q6h+uqnGni9HsTNsTvmKC
lITrlfAZYpTsX8ULaiXIG3X2zAh5MbpHrx+O7iTITzo8peoJChVypI7ZfQR5
ISU4nD9IIfKXL6togCA9D33riu6jUEXJwO/yIYKMWi8kXvRQqMZVdlc4QpAB
nEYfeieFts4LOyn5Q5BzFPZmGLZRqKmV7twjI8ik0DupO8QU4j+N1v09QZAt
VhsdIloo1BmkMjo1RZBFNHic3Uih/wBDJFpG
       "]]},
     Annotation[#, "Charting`Private`Tag$128101#1"]& ], 
    TagBox[
     {RGBColor[0, 1, 0], AbsoluteThickness[1.6], Opacity[1.], 
      LineBox[CompressedData["
1:eJwVkGk8lG0fQIfG3CQkbSrbSDSFrBHmf499SUqLSmUr8qRFlp5I1kLSRqko
pdI2tHokcl1EhIrKMoXmHsMgZd/F2/vh/M6n8+WoeR923SdOo9ES//J/5xdV
pV2/VgDOK7Ji2zNtcFn7xdvCLwUQoi56H3HRBtfK7nisI/saikRlmUqxNrjT
U1RcGvMadD/+ngrytcGLJegd3QcKYfq8wblwbRsc5mxhaMZ+A2NyirEjRdZY
pdet82AghrdnpY1vUlZYEFkVJ7uwDGqjAszzOJbY12qD8n2jMuB+LRZoGFri
LsbnfNhaBgI1O7/MFZa4L5nXfSS1DF4Ev2fkSFvi6fTOjV/mlYN9TWyUfgMH
L33FULoq9w6mpUzWtwdw8JY+yzw1qUrIX5G4gH+LxO88C9sNp6rBwcbtbpQN
G8sUPA3LU6wBKps2ZbKGjbfIZ8sZr62B1R2qvTNL2FhQcsF07dEa8L9vfrmg
zwJPM32TTTtr4Cxbcff3DAts1D7XiP31A0QFeGV+HTXHd/194+y4n0BzqZlN
2CszzClIkNfOrQOSlPu008cUhzlcs79TVAeYZxLWtckUv+Q9jFSsroMvszc1
xJGmWHOi6pdEZx08bP2dQCmZYhkzmapWtc/QbGy5Wp9ngnlFF2MuXP4MuQ1+
MyxXExyIrw8OnvgCS7z8bmxwXotvV3DrXzvVQ4hVS3qfrxHeeVim8R/3egjK
f/4S3IzwvEWHmpYcqAf/tU616XZGOMZX93vYmXoQ7enqCdMywt4Sz/nr3teD
p2dMxZduQ7zcKv/na9sGuJRl694ZaIgfFJeIFXIaYcirNd0j0QA/zWvQLlzL
gyLxvZnp3/VwlWbfag9bHsy3+I+NPulh4TWp1bO28iB8+cT6nrd6ePFJc5bT
UR7wpUOve3P1cKRt1orvXB7MmEcZowg9vKHxoMqk2jeIsN3no8/Uw7/G6PJm
c76Dj7v66drANZhlbjD0mt8MouaMbNEWHVxanvHmal8z2FTrtn8HHezuwogP
pbVA31ith4Clg8968xT1VVtAnVB/ryGmg3sTIuGhRwt8tt2UE5erjV/WV59J
a20BbXW19tQ52hgO71ULbm6Fo2NCt0v1qzCrzvH+wgA+KCzW3VyUthKLJzjG
8IP40HtMOXlh/ErMYzvufhTOh8tKjytPhq7ECVwHBXYSH4yvJ8of37oSt8fb
R+57xAd61cxphfkr8S22rdvLTj5Y/2vGqE/Rwgu4HMJ1HwXUlcWnDG9oYlq8
iV/yHgFM6OTTGr9qYMk78zl1+wSgmm6536xSA89FfUsWHBTAruwT4Q8LNbDa
6IOPGeECyJDdEZuVpYEt/RSNuVcFoFtdokMEauBYuwl69WcB1ClfKUyR08AM
yaIsSbs2+HKBtjF683I8JxFaY3WFcPCXQaDYMBN/fWp1Y+9aIWhdcf/xrIuJ
05vsdtmAEMIVco8caGViltbGbwwXIYwUuHwbr2Bi+wrPhsRDQnDRL+bFpDPx
KYmYj+dzhPAye+UKtjUTT0eXFaevagefbTKnVTPUcG+YQ+YLzQ6w+iCMFPio
4k6CtVtWtwOOOd+2X+euivmps5f6G3fAKrukXVddVXFtbvUVZZsOSBofd/Hj
qOLnAudzid4dcK+dqnFRUcWhjq4RHjc6gNsz3XT2lQqeUnR3l1YQgdW3Ln+n
PGUsWRCwyGdaBJSXuLFu7TIsOL6eWVvdBUSr3OngJEWcytI9Fop/grHtgRS9
8wvxCc1VsRkpv8D4p2dxvMF8bDafxZtM7oUZnCyhzJiHW0oGPM+iPoiqQxq6
BnPxK5WWpzvv94NfTk55WogMjhyuvFeeNQDw472u7tPZ2CuQE3okeRD+856M
dzskiXX2Ff7MTxqCcZUza7Y5MPCu6ymsPaeGIS7OFdkdoeN7IWPW1odGIPDD
9rnSXeKYV7mHXvHPKBDrhH6XDothrdJNmYnbxkB5TiRtxJCGm6ayZj22GAeC
fivyBHsaBT8ZnuNvMgEtgyVba1Wm0CrJ+n5f5iRon+NJX9o2gT405YWLqU7B
iIPbtPDyGKrtHvo4sfgP1Dn1li0iRtHvLPzHQGwaNuuj4YEXw2j0c3Kd1J9p
OEkek/zhM4SWPhRFqXTOgFPYMuYD60Hkwv805eBHI78lSA04cgYQ8YCb5Cqk
kf2VRzqY7H70odRFcnK7GLldNFtL3aMPJV4LagxsFCMP0zc8vznzG7m+3Z2a
4CxOLvy9nF0e8QtVy4zmbSgRJ313RL8bV+pB6+bLs9rYs8joC0SbY2E3yj/Y
n7To5Swyf9fJIYv4LsSKdSWXGNDJmTPyH3Q2diLnAu8dNU/oZCRjR1KFgQhF
WJp6Ki+XIA/nCdrSzDrQnfgLBewsCVIt4aD9RWhHjSq5tJlFDPIPb9RC3EeI
CpvCuIeSGGRSSmpIRFobuuxc+YgrSZDFx00HqysE6MSC5itnIgjS80d/q7u8
AIn/8AxIjSTIY2F3WqxlBSjhQTvnZjRBav3LytaRFqAUs96eZ6cIUslhTipd
QoAeeYlb8ZIJcrb+/m8FYxRqzNHq1bxJkEHpEw0OfArp24bYlRcTJC9jrPDP
Ewq9kptY9gkT5EW7jOAZLoUseCcHmkoJMmDS87fYIwrZByTc6HlHkINeCiuk
7lLI41L6oMIngtTuUL6hepVCZ1tLMr1/EGR9A+NIUBSF5j2wDQmgCFIwxVGP
jqDQ1cBqx9A2glzmX5pyPoxCd+j1w4kigiytSuPmBlPoNavT6Vnv3z66I294
P4XIoQC1wn6C7FZav0HKl0Llb/pHygYJ8h4VlKXkQ6HajZO3m0YJckR21gn7
3RTatiTqmGD875+8ODGPnRRqbqM790wSpNTpR5xQNwp55yQyR/787QXI7NwW
ColCZcdmZgjy8fvVfdmbKPQ/WpNS+Q==
       "]]},
     Annotation[#, "Charting`Private`Tag$128101#2"]& ], 
    TagBox[
     {RGBColor[0.5, 0, 0.5], AbsoluteThickness[1.6], Opacity[1.], 
      LineBox[CompressedData["
1:eJwVjGk8lGsfgO2PZE0RnZoo0YwloZT4P2NfjpJWyZo4lZQKHQmRF9UoUWQp
SVFNRYdk6745I4psZZmKZsYYU2TJVtbT++H6XZ+uS8P3hOthMRERkcTf/N+l
lW/TMm6VwffEz8dVvWwwqy/5Lv99GZxlyL4odrHBLfJuj/Xly+FDtmOOm6UN
Fnr3v6qJKYeSlEGPci0bvFxSQvDtWAV0Wrgndw5a43Bnc2Mziyrwq6jxuRBh
jSnD+4THgzF4zY49u3HXCvOi3l6UV2GBQRfJYYlZYn+r7avyTVhAfWOXSE7Q
8VeptlLYw4LRx3uotf10PMJgfzuZygIFz0MuXxvpeD5T6PJ+SS2oPzkpl51G
xyteSq1MV3gNYXU3TIv06Xj3iGWJxqJ6CHESFYs5ROLX3hV9xrMNwCL5Owub
zLFcWWF4iVojVD4hqxLKzPFupQcKmzY3gmsm+e1EnjnmVV/bsvlUI5gq14Yc
DTfH85r+jC3CRniaNVCvoG2OTfoUTSw+vAPIMRlRid2G8474X7RjNoPbXhHu
qI0ZppclKOk9bQW5+JnelAlTHO5wy/5eZSs8zmn2c+Cb4mL2wyi1hlYYuYUf
LX5virWn336XFLYChxEV+KLQFMuZyb3t0WgDmr/K0rxAU8yuTI65dqMNKhuW
OH4UbMbBOGNsLOI9MK581L/I34Tv1jHby53aYY5GUXEVN8EHTsh1HnVvh7P3
U2KaxozxEtWgLvVj7bApRHdyH98Yx/gbfAq/1A6/uhuakmuNsa/kc87WN+0Q
dpbhkJNgjNdalQ6U23ZAkV1/9GolY1zwqlq0gt4JHTX5rCCaES4s6dCr2MyG
QN71DsdYQ/xWe0TXy5YNAlP1mbQwQ8y/tUhXfA8b2v79Ejd0zBAvj9xGdTrF
BoNFVUWluw1xlG3uuk9MNlw54JNVts4Qb+88TpnR+AjjYyPJIY0b8PefEkpm
sp/gwJT+uuxVGzB1m9F4OeczTMqU8A681MM1tVlV6SOfwaQt4mbuPT3svkMq
PlSkG7xWNByaTdLDV3zZahtXd0N1k4OM4LAeHk6Igode3dCYsoZ1dakeLm5v
uJTW0w16vWOT+iG6GE74aZz53AMHk0Nb9a1omNrqmK8SyAGiQ1D/TX49Fktw
jOGc5kAOVvqHMa+D2RaOHo/OccA3vPysxZAOTmA6KFtc5oBstNehN+90cF+8
fdThRxyQcdZxjWXo4BwL233Fwt99aFJ6hIIOXsakE66HuWAfRRnTX6mNReJN
AxiePDiiOqsk6aGFpe8tpbce5sHiLbPH8ly0sCIaUV92nAfhRvY7na21sMZU
QVPWOR68JiyzKmha2DJAbRMznQeBP185LppZi2PtpiUa2ngQYKDK9slci6Wk
K3Ol7XohyGM0t5m3BssmQk+sAR+evvEPGLukiT8UWmX7beaDhWOHy6coTZzZ
ZXfQBvhwzbZga+MZTUzVcfkotYMP1HSj7/Wemti+zrsjMYgP20Jmv+gaaeI4
yZimq0/4IKphV5DWrYHnL7BeZdL64FytUzMy1cDD4Q53/tEWQNfpvReZUqux
kKB6yBsIQLF/cNp7loI5qTIrjmwSQDmldHvIAAW3PG24ucpGACqK8cM1byj4
Oc85KdFXAPeMMoQj/6PgUEfX817ZAuh2FwtKEqfgWTV398XK/bAnpTQ8XnIV
li4LVD003w8Bnk6ntlP/wLy//9RsafgK+opn1/yYXI5TqQZhoXgASJ+rEnwZ
FRyhTYvNSvkOItFyFHqlMjZbSmXPMIahJ9XoyOJMJdxd/cP7ChoBnU9S9QN5
CvglpbvwQP4o+FlNDsyzZHHURP392twf8EAzo/qWggz2CaaHnmSMQUgA7Wrf
RwLrH64YKL08DjUit9mnayTxwYwUqmfcBDTKrn5hNy6O74f8tLYOmoTi/W0G
KqFimF3vKVF3dAreuV36y1tSFOvU7LyTuPcn2HgsO7MhbwF1zeaKPzb/BRJr
VzyoiJtDZ55NyB4xnYa2yU8r607PIJp0+6i/5gzseuRH2JX8Qu+6Ss6Jrp6F
18H7hdSFKdTybbxpevkc8KmGBnV/T6KhXDxnJDoPkUWczfn6E2iqjdG6aG4e
6EUrVRIFY2jFw/5oinAB7B1kDmg2/UA7OM2zDgEiZI/UixNDLaOIKGBeduWL
kOsN/U6MvB9B72p2SM/sFyV3Mc9vjR4fRom3TncGd4qS6XdzGJHkEHL91yM1
wVmMjJjfmP6xbhA1yE2VbK8WIx12GzaGnBxAW5cqUXstxMm9h9JK6CrfUOnx
0cuqxeLkeJOuVupXIaLGupLqRhJkdlqx2M+yfuRc5uvW+EyCbFUyTPDJE6Dz
llu8V62VJMPOOp/Set6H7sVfK7PIlSSLj1np6VTyUSflqciCqhTpsmY2Usjv
RRVd4cygy1LkUaHCNfqqXnTDuf4RU5ogIx/bmKfu4qGIZZ9vXjpPkEomXgNx
d7lI7It3YGoUQTJvkyZRt7kooaCPfvsCQWrmPfe6mMlFKWbDg0VxBOm1bYtW
2A0ueuQjZsVmEGR1qlVVaCIXdT7RGda+TZA2fVbXs4K5aKNtiF3tK4J8nWE9
GmnJRS8Vpv9oxgQ5tAD6qcBF5uzIH101BPnnS7P6/G1cZB+YkD34miATrgrW
N27iIq/rmWPKzQRJoy2wjGlcdKWn+o7vl99/5u1o5aVctKTANiSQS5BJvs8V
aUpclB7c4BjaS5DLMjxhhzwX3ZNon0jsJ0i3ndbHc6S5qJwqdCoaJsjABKbC
ujkOIscDNSpGCVKd0dFpM81BtVWjk6wxgmSdXlF1ZoqDWlxm7nZNEeT+fndR
1igH7VWPDuP9Isj7oVLKA0Mc9LlXwnlwhiAVtZyMVQY5yPdJoubkHEEaq1GT
rL9yUH+o/M+FBYLUPa+f/5eAg/4DBMBUOg==
       "]]},
     Annotation[#, "Charting`Private`Tag$128101#3"]& ], 
    TagBox[
     {GrayLevel[1], AbsoluteThickness[1.6], Opacity[1.], 
      LineBox[CompressedData["
1:eJwVx3k81OkDwPFxfmWjhNBhcrTkWMl9Pg9yp2TTueUo2nKrtMtK2F1Xdp01
7lAR40rkyvPQKIVQxAjNd4xbuW/x298fn9fn9ZZx9XFw46ZQKLT/+v9f1L17
kJpSDUjxlUf0s+aYMRyfzflYDR7etM22sTHHHcLnCn8SrgHXkg+ZzhiY4zHn
0frGsBqQKx5604FqjiX5eEcmPGpBSuiJEv+RozjQzkjTwPgl4JUu55cLOIqp
02fGvPwweHKswcwizQyzQ979KbybASoPbMtP3TDB7mbHpfO0GGDCd+2lxLQJ
Huf/8AI4MkDvZNb7DNIEz8QyJ3yTGKCNj/mZ8doEb6aN2X/c1QTqE4b+vhNv
gvdW8e+n7XgNiG3qglmKJvjUjGmFzLZmcOXRY6foixC/dq4d1txoAbRmVpru
KyMsVF0aWCHVCpYeujWIFRvhUyJPdmjrtAL7Z+WFWzQjzG6I09PxbwXa6Uq1
XD5GeFPWPVZvrBXM3X6rX7nXCGsN79Qy7moDDefELftvG+JH19z/tKS3A57A
Q1tL+gbYpDpSRLW4E7jJSXGkJ3VxoHWKVW5dJ3AEZ1N6mbr4OfNpiFRLJ/A2
WxDLatbFCmvvvvKNdYLii2XmDk90sZCB0LtBmQ/AaEOaae+qi5l18WFxyR+A
4oKd5NN+HeyHU+fn//gI9H4JynvQp42z39C7a2y7geZ50YnpVU183keo5/qF
bvCtronfb0IT75Lw7t3j0Q1cI44rbfVp4jB3tc+B0d2As/zWxbROE7vyPWPp
v+0Ga3IRyZdDNLG82YvJGotP4NZS6o/bBDRxfn0DV61JDyg+YpScLauBSys+
qdbqMMEjlwPNwkHq+J3CjIqTBRM8MCkQdfZRx5yUbSo8jkzQ/kqeUXNZHUve
MVSy9WcCsuc3nXvH1HGIRc6Pn+lM0HZ7+WGmtDo+3uNFXZfpA2357SeDGIfx
1xVeEYPtn0HlPzSzod2HsZKhxkINqx+4aOfzf3mqihub0l/SZvrByLXIoZ+S
VfGFE/wRAZQB8PMgqzvuriq+58qUOnJgAIiNGtZEn1HF05Eh4KnTACgMxvWn
+FXx8+6W6AeDA8Dy+jzWuKqCgc8VmZv9g2DWY1WiVEsZK3Xa5O32ZIHxlF8d
znIfwtyRNmGsGyzwJcJJh3tOETONbS4WBLGAgdzL+WpSEUfSrUWNY1igazQa
OTQo4uEIqxC3AhbY944OFEMV8UNjizPPx1hAC/sNn+FRxOJ0E8LBjQSi0SLL
N0QUMCVC92rsJTbQTljIEXE4iAVyxUw63dggyvOfhErzg3gnmtkj7sUGjUIH
Bd30DmKZ5fz36UFskMZo9hk8cBCbXpXSptPY4Oc9IiqmM/I43HKNt+XDf3bc
qfc6Th7zC9TlCFgOAZrisfuRvXJ4exQYDFfjgJGBlyrHQmVxV6lZxhUdDuhV
jbPRC5DFab2Wv5gDDvDNtXdT85DFSor2ffwnOECVfdFH21EWW71x/hTlzQHb
jbjHig/J4r/4wt7/W8QBEoIHpEy7ZPBmKKM+TXkYPNbNSqpSk8HTgdZZ5Qoj
4CrDkPTdoOIxQumisNoIoFvxbg+dpGJWkuDea9ojgBGnk5jRR8UdxS33pc1H
QOykf8x6FRU/Y9v9E+U6Akrk9ZasA6g4wMYh2CljBBRmWXkpzEvjDakLF34Q
HQU9x/Lo6Yv7sUC1p8TlzVGQNfPDst3efZj9+zHZjpZxwP8pPj1mXBInKand
DsCT4GvEIeW1TXH8h4JyeHriV7Bf41fByDJRbCCmxFyPnQZ9tJTP3vEieKBh
zvkemgGU/ba9iYk7cBV1oPR83iyI4cOdqhXbcchi8+OmnDmwczb4iAGXIHbx
MwnwjZ0Hh243PK5sI/BPbrWTL2IWwCn3C+nulXz4l9REpUt/LQLxsLPOWuM8
+PGtlaNHvZfAxNDD8o8e3JjZfIn3zfVlYOzOsh9fp2DFxpNZUadXwAkOQfk3
YQv1buTwFBqtgo77UhpGt76jmyWL26/prgEXEXqXy5V1pCzQPesuuw4ilec9
Jp6sorbeiiCuAxuAzIgpkppbRh0TC+/XJL8Dw6gP6kmeS+hbDv6uwbUJSuOX
K+ZkF9Hyh9jObd83geANxa2Ovnm09+noXerYFrB26/abZsyhE6z2DeurFBjs
62Vn82YWEfn0GAcOBS4QF55VvJ1BbY0nBNbPcsE4z9MJcGwaRaXc6PHr4YIK
nSoyTzS+IYdXF5Mi7bihdndirFDxFGoRWq443sAN75LBYcqek0hfTERpyJgH
PrpU5vG78AR64TUbI/GcB5akr1/XXRtDSuEOcI8GL/QcMHJ78GYU2VW7nmst
4YV3L+vTPIpGULCpnrO0PB/czGyKiy4fRrkRcdXGOXxwa7yM91wNB/VQiylb
EvywkZR6c2d4CNX2BtK9Y/ihguvpdPf9QyjZrrmALkBA2kHDb8M/s9Ef4v33
o4MJWHCj5Aolm0TcX5w9k0IIuEDtXK3IJFFk/rBJZigBV7pcW1PSSCTsf10i
P5yA5XdOZ1TSSJRoMD1V9hcB6dQqaJJMIkm+m421EQSkPuQLLUwgUeb7lQdN
UQTsf3G+Wfk/y9OCvdpjCBiFD0/ExpKowIXbjBlLQEfbfYsFV0l0WDlCcuhf
AhZWe7W6/E2iioUfvk3FE7CLsnDHM5xE+vVxr5YSCbg+2X8kPoREOEI8hXKf
gJXjkYNTwSSyOJnqLUgjYEyrX+LvgSRq3UM9KpZKQEN/0eSi30jkwMmVkk4n
4OEaD1OZmyTqKVKcVsgk4GZKy2iwH4mOWNyybKonYCa7vDb2KImqdqzta8cE
LLF2KpaHJDJi3pnrbSTg3fykT/OGJGrM4WlmMwjYE2N6JVGfRFaekRlTrwl4
LYJdl61NovdaQjeWmgmY8b1qF9Qk0amteCtKCwG790l0fFIjUV/zbmnBNgJK
2MoyE1RJ5JSQNi/aTsCBYeaPjsokujfYkOX6hYBnBfwr2aIk2pVvccuTJGBp
nkrFXhES0fxabAKGCOj/KK9LTphEubzdi1GjBPQsMjvdJkCiGqUx27JpAg76
ug/LfGchuOApUztLQMmTWwsyayzU9HJ2iTFPwNHHg+LlyyzUYb+e3btMwNrw
ttrKWRY6vefubfYqAZXOZ8s1fmOh/iFeu6l1AvIHBXlwTbGQa1GU7NJ3AoaX
bflcGmeh0QDhla0tAtquVo94DbPQ/wDlQ9t3
       "]]},
     Annotation[#, "Charting`Private`Tag$128101#4"]& ]}, {}, {}},
  AspectRatio->NCache[GoldenRatio^(-1), 0.6180339887498948],
  Axes->{True, True},
  AxesLabel->{None, None},
  AxesOrigin->{0.1, 0},
  BaseStyle->{FontFamily -> "Arial"},
  DisplayFunction->Identity,
  Frame->{{False, False}, {False, False}},
  FrameLabel->{{None, None}, {None, None}},
  FrameTicks->{{Automatic, 
     Charting`ScaledFrameTicks[{Identity, Identity}]}, {Automatic, 
     Charting`ScaledFrameTicks[{Identity, Identity}]}},
  GridLines->{None, None},
  GridLinesStyle->Directive[
    GrayLevel[0.5, 0.4]],
  ImagePadding->All,
  ImageSize->{1514., Automatic},
  Method->{
   "DefaultBoundaryStyle" -> Automatic, "DefaultMeshStyle" -> 
    AbsolutePointSize[6], "ScalingFunctions" -> None, 
    "CoordinatesToolOptions" -> {"DisplayFunction" -> ({
        (Identity[#]& )[
         Part[#, 1]], 
        (Identity[#]& )[
         Part[#, 2]]}& ), "CopiedValueFunction" -> ({
        (Identity[#]& )[
         Part[#, 1]], 
        (Identity[#]& )[
         Part[#, 2]]}& )}},
  PlotRange->{{0.1, 3}, {-60, 0}},
  PlotRangeClipping->True,
  PlotRangePadding->{{0, 0}, {0, 0}},
  Ticks->{Automatic, Automatic}]], "Output",
 CellChangeTimes->{
  3.741166779981697*^9, {3.7411671399470673`*^9, 3.7411671686750097`*^9}, {
   3.741167199651115*^9, 3.74116721940021*^9}, {3.741167884725768*^9, 
   3.741167931427692*^9}, {3.741320315663919*^9, 3.741320386793285*^9}, 
   3.7413356976495733`*^9, {3.741335758898391*^9, 3.741335793265177*^9}},
 ExpressionUUID -> "38594ffa-6779-41cc-911c-2df497f5c59f"]
}, Open  ]]
}, Closed]]
}, Closed]]
}, Closed]],

Cell[CellGroupData[{

Cell["Relativistic short-range Breit exchange energy per particle", "Section",
 CellChangeTimes->{{3.7411632736382093`*^9, 3.741163274226321*^9}, {
  3.741164012603465*^9, 3.741164012810066*^9}, {3.7413186312802887`*^9, 
  3.7413186325287237`*^9}, {3.741335816912109*^9, 3.7413358182364273`*^9}},
 ExpressionUUID -> "4df3c283-bc3d-4c0d-9f21-a98fda0e7e36"],

Cell[CellGroupData[{

Cell["General expressions of the energy", "Subsection",
 CellChangeTimes->{{3.74116431193472*^9, 3.741164315937715*^9}, {
  3.741315833500453*^9, 3.741315835582797*^9}},
 ExpressionUUID -> "b1e4cde8-1b16-4f96-8f5b-c832d1569647"],

Cell["\<\
The expression of the relativistic full-range exchange energy per particle \
for the Breit interaction potential is\
\>", "Text",
 CellChangeTimes->{{3.741312221879962*^9, 3.741312269736453*^9}, {
  3.741315812750471*^9, 3.741315813596662*^9}, {3.7413358369732018`*^9, 
  3.741335838557274*^9}, {3.741407988386943*^9, 3.741407993630865*^9}},
 ExpressionUUID -> "5ab243ca-3a93-46c0-96fa-2ab8df663c1f"],

Cell[BoxData[
 RowBox[{
  RowBox[{"ExRB", "=", 
   RowBox[{
    FractionBox["1", 
     RowBox[{"4", " ", "\[Pi]"}]], 
    RowBox[{"3", " ", "kF", " ", 
     RowBox[{"(", 
      RowBox[{"1", "+", 
       RowBox[{"2", " ", 
        SuperscriptBox["c", "2"], " ", 
        RowBox[{"(", 
         RowBox[{
          RowBox[{
           RowBox[{"-", "2"}], " ", 
           RowBox[{"Log", "[", "c", "]"}]}], "+", 
          RowBox[{"2", " ", 
           SqrtBox[
            RowBox[{"1", "+", 
             SuperscriptBox["c", "2"]}]], " ", 
           RowBox[{"Log", "[", "c", "]"}]}], "+", 
          RowBox[{"Log", "[", 
           RowBox[{"1", "+", 
            SuperscriptBox["c", "2"]}], "]"}], "-", 
          RowBox[{"2", " ", 
           SqrtBox[
            RowBox[{"1", "+", 
             SuperscriptBox["c", "2"]}]], " ", 
           RowBox[{"Log", "[", 
            RowBox[{"1", "+", 
             SqrtBox[
              RowBox[{"1", "+", 
               SuperscriptBox["c", "2"]}]]}], "]"}]}], "+", 
          RowBox[{
           SuperscriptBox["c", "2"], " ", 
           RowBox[{"(", 
            RowBox[{
             SuperscriptBox[
              RowBox[{"Log", "[", "c", "]"}], "2"], "+", 
             RowBox[{"Log", "[", 
              RowBox[{"1", "+", 
               SuperscriptBox["c", "2"]}], "]"}], "+", 
             SuperscriptBox[
              RowBox[{"Log", "[", 
               RowBox[{"1", "+", 
                SqrtBox[
                 RowBox[{"1", "+", 
                  SuperscriptBox["c", "2"]}]]}], "]"}], "2"], "-", 
             RowBox[{"2", " ", 
              RowBox[{"Log", "[", "c", "]"}], " ", 
              RowBox[{"(", 
               RowBox[{"1", "+", 
                RowBox[{"Log", "[", 
                 RowBox[{"1", "+", 
                  SqrtBox[
                   RowBox[{"1", "+", 
                    SuperscriptBox["c", "2"]}]]}], "]"}]}], ")"}]}]}], 
            ")"}]}]}], ")"}]}]}], ")"}]}]}]}], ";"}]], "Input",
 CellChangeTimes->{{3.7191233323485947`*^9, 3.719123354257957*^9}, {
   3.7191333462516327`*^9, 3.719133346586507*^9}, 3.719206123103397*^9, {
   3.719299206450746*^9, 3.719299211261162*^9}, 3.71929961625492*^9, {
   3.719299896739259*^9, 3.719299904721034*^9}, {3.7411632855777817`*^9, 
   3.741163294469509*^9}, 3.7411640647062817`*^9, {3.741316831279217*^9, 
   3.741316833661255*^9}, {3.741320559043417*^9, 3.7413205593793497`*^9}, {
   3.7413222973050756`*^9, 3.741322303558218*^9}, 3.7413366737294683`*^9},
 ExpressionUUID -> "d1ed7912-60ba-45cb-8a7a-f1a23394a45e"],

Cell["\<\
The relativistic short-range exchange energy per particle for the Breit \
interaction potential can be calculated through numerical integration using\
\>", "Text",
 CellChangeTimes->{{3.741312281128374*^9, 3.741312335545431*^9}, {
  3.741312671624989*^9, 3.7413126773038692`*^9}, {3.741315815612306*^9, 
  3.7413158161560907`*^9}, {3.741407997956012*^9, 3.741407998257225*^9}}],

Cell[BoxData[
 RowBox[{
  RowBox[{"ExRBsr", "[", 
   RowBox[{"\[Mu]_", ",", "c_"}], "]"}], ":=", " ", 
  RowBox[{
   RowBox[{"NIntegrate", "[", 
    RowBox[{
     RowBox[{
      FractionBox["1", 
       RowBox[{"4", " ", 
        SqrtBox[
         RowBox[{
          RowBox[{"(", 
           RowBox[{
            SuperscriptBox["c", "2"], "+", 
            SuperscriptBox["k1", "2"]}], ")"}], " ", 
          RowBox[{"(", 
           RowBox[{
            SuperscriptBox["c", "2"], "+", 
            SuperscriptBox["k2", "2"]}], ")"}]}]], " ", "\[Pi]"}]], "3", " ", 
      "k1", " ", "k2", " ", 
      RowBox[{"(", 
       RowBox[{
        RowBox[{"-", 
         SuperscriptBox["c", "2"]}], "+", 
        SqrtBox[
         RowBox[{
          RowBox[{"(", 
           RowBox[{
            SuperscriptBox["c", "2"], "+", 
            SuperscriptBox["k1", "2"]}], ")"}], " ", 
          RowBox[{"(", 
           RowBox[{
            SuperscriptBox["c", "2"], "+", 
            SuperscriptBox["k2", "2"]}], ")"}]}]]}], ")"}], " ", "kF", " ", 
      RowBox[{"(", 
       RowBox[{
        RowBox[{"ExpIntegralEi", "[", 
         RowBox[{"-", 
          FractionBox[
           SuperscriptBox[
            RowBox[{"(", 
             RowBox[{"k1", "-", "k2"}], ")"}], "2"], 
           RowBox[{"4", " ", 
            SuperscriptBox["\[Mu]", "2"]}]]}], "]"}], "-", 
        RowBox[{"ExpIntegralEi", "[", 
         RowBox[{"-", 
          FractionBox[
           RowBox[{
            SuperscriptBox["k1", "2"], "+", 
            SuperscriptBox["k2", "2"]}], 
           RowBox[{"4", " ", 
            SuperscriptBox["\[Mu]", "2"]}]]}], "]"}], "+", 
        RowBox[{"Gamma", "[", 
         RowBox[{"0", ",", 
          FractionBox[
           SuperscriptBox[
            RowBox[{"(", 
             RowBox[{"k1", "+", "k2"}], ")"}], "2"], 
           RowBox[{"4", " ", 
            SuperscriptBox["\[Mu]", "2"]}]]}], "]"}], "-", 
        RowBox[{"Gamma", "[", 
         RowBox[{"0", ",", 
          FractionBox[
           RowBox[{
            SuperscriptBox["k1", "2"], "+", 
            SuperscriptBox["k2", "2"]}], 
           RowBox[{"4", " ", 
            SuperscriptBox["\[Mu]", "2"]}]]}], "]"}], "-", 
        RowBox[{"Log", "[", 
         SuperscriptBox[
          RowBox[{"(", 
           RowBox[{"k1", "-", "k2"}], ")"}], "2"], "]"}], "+", 
        RowBox[{"2", " ", 
         RowBox[{"Log", "[", 
          RowBox[{"k1", "+", "k2"}], "]"}]}]}], ")"}]}], ",", 
     RowBox[{"{", 
      RowBox[{"k1", ",", "0", ",", "1"}], "}"}], ",", 
     RowBox[{"{", 
      RowBox[{"k2", ",", "0", ",", "1"}], "}"}], ",", 
     RowBox[{"Method", "\[Rule]", 
      RowBox[{"{", 
       RowBox[{"\"\<GlobalAdaptive\>\"", ",", 
        RowBox[{"\"\<MaxErrorIncreases\>\"", "\[Rule]", "2000"}]}], "}"}]}], 
     ",", 
     RowBox[{"WorkingPrecision", "\[Rule]", "8"}]}], "]"}], "//", 
   "Quiet"}]}]], "Input",
 CellChangeTimes->{{3.701145681788294*^9, 3.7011457077245607`*^9}, {
   3.7011457387970448`*^9, 3.701145742715835*^9}, {3.701145838955688*^9, 
   3.701145864971176*^9}, {3.701145973723259*^9, 3.701145997658729*^9}, 
   3.701146056572063*^9, {3.701146107515278*^9, 3.701146121611495*^9}, {
   3.701146196843637*^9, 3.701146247866346*^9}, {3.701146312635221*^9, 
   3.701146375081807*^9}, {3.7011464264741697`*^9, 3.701146477657305*^9}, {
   3.701146583432921*^9, 3.7011465958422613`*^9}, {3.701146635256982*^9, 
   3.701146673336335*^9}, {3.7011471055597353`*^9, 3.70114712658249*^9}, {
   3.701147399749424*^9, 3.701147402949328*^9}, {3.701147490165003*^9, 
   3.701147559316208*^9}, {3.701147589652295*^9, 3.70114760658006*^9}, {
   3.701147762259828*^9, 3.701147764355604*^9}, {3.701148064721983*^9, 
   3.701148067649757*^9}, {3.701148188946526*^9, 3.7011482124492397`*^9}, {
   3.7011483018407917`*^9, 3.701148396496244*^9}, {3.7011484538239727`*^9, 
   3.7011484901597433`*^9}, 3.7011485487194843`*^9, 3.701148617247799*^9, {
   3.701148653359206*^9, 3.70114865593461*^9}, {3.701148686398691*^9, 
   3.701148686638567*^9}, {3.7011492174203663`*^9, 3.701149217484399*^9}, 
   3.703923968822303*^9, 3.70392400506175*^9, {3.7039240660390387`*^9, 
   3.703924077057626*^9}, 3.703924120324793*^9, 3.7039244524507217`*^9, {
   3.703924650531103*^9, 3.7039246519228373`*^9}, {3.706590014367525*^9, 
   3.706590016210148*^9}, {3.714289166465165*^9, 3.714289168351822*^9}, {
   3.7177498205374203`*^9, 3.717749842137086*^9}, {3.717751156491482*^9, 
   3.717751186824505*^9}, {3.717751246744615*^9, 3.717751480920171*^9}, {
   3.717751518361574*^9, 3.7177515280449133`*^9}, {3.717751613705089*^9, 
   3.7177516876773376`*^9}, 3.7177517201526127`*^9, {3.717751803459509*^9, 
   3.7177518054711514`*^9}, {3.717752264568583*^9, 3.7177522695631037`*^9}, 
   3.717753253914151*^9, 3.717821459452956*^9, {3.7181908060799026`*^9, 
   3.718190806213161*^9}, 3.718190982122443*^9, {3.718191793953211*^9, 
   3.718191819001253*^9}, 3.718193884654935*^9, {3.718194736362905*^9, 
   3.718194737316622*^9}, 3.718779040850235*^9, {3.719032398425578*^9, 
   3.719032400770814*^9}, {3.719118906710697*^9, 3.719118917476943*^9}, 
   3.719121597767376*^9, {3.719121653871307*^9, 3.719121682857985*^9}, {
   3.719121726918955*^9, 3.719121730672037*^9}, {3.719298214253356*^9, 
   3.719298240031876*^9}, 3.719298300286251*^9, 3.719298398897888*^9, 
   3.741163479074169*^9, 3.741163662608089*^9, 3.741163711657773*^9, 
   3.741316835855143*^9, {3.741320560885421*^9, 3.741320561223034*^9}},
 ExpressionUUID -> "2ef7566e-fcfe-4543-ad25-86dcb0349bb3"]
}, Closed]],

Cell[CellGroupData[{

Cell["Calculation of the large-c expansion and Pad\[EAcute] approximant", \
"Subsection",
 CellChangeTimes->{{3.722158370784416*^9, 3.722158376544992*^9}, 
   3.740375873100111*^9, {3.741335857321227*^9, 3.7413358591010523`*^9}},
 ExpressionUUID -> "5b0c55df-1bfd-415e-a8f7-3c0c17bf0b2a"],

Cell[CellGroupData[{

Cell["Tables of the expansion coefficients", "Subsubsection",
 CellChangeTimes->{{3.741164766995187*^9, 3.741164769226877*^9}, {
  3.741164800614396*^9, 3.741164808695251*^9}, {3.7411649271723413`*^9, 
  3.741164931300631*^9}},
 ExpressionUUID -> "7a64d4ba-15c1-4344-b830-6cbefdb342b5"],

Cell["\<\
We need to consider and stock in matrix forms the coefficients which take \
part in the Second Part of the exchange energy  (There is no \
\[OpenCurlyDoubleQuote]First Part\[CloseCurlyDoubleQuote] in the case of only \
the Breit interaction potential)\
\>", "Text",
 CellChangeTimes->{{3.7221584371697073`*^9, 3.7221584415565367`*^9}, {
  3.741315895680744*^9, 3.741315937740252*^9}}],

Cell[BoxData[
 RowBox[{
  RowBox[{
   RowBox[{"Coef2Bsr", "[", 
    RowBox[{"M_", ",", "n_"}], "]"}], ":=", 
   RowBox[{"FullSimplify", "[", 
    RowBox[{"Coefficient", "[", 
     RowBox[{
      RowBox[{"(", 
       RowBox[{
        RowBox[{"Coefficient", "[", 
         RowBox[{
          RowBox[{"Series", "[", 
           RowBox[{
            RowBox[{
             FractionBox["4", 
              RowBox[{" ", 
               SqrtBox[
                RowBox[{
                 RowBox[{"(", 
                  RowBox[{"1", "+", " ", 
                   RowBox[{
                    SuperscriptBox["x", "2"], 
                    SuperscriptBox["k1", "2"]}]}], ")"}], " ", 
                 RowBox[{"(", 
                  RowBox[{"1", "+", 
                   RowBox[{
                    SuperscriptBox["x", "2"], 
                    SuperscriptBox["k2", "2"]}]}], ")"}]}]], " "}]], "-", 
             "4"}], ",", 
            RowBox[{"{", 
             RowBox[{"x", ",", "0", ",", "M"}], "}"}]}], "]"}], ",", "x", ",",
           "M"}], "]"}], "/.", 
        RowBox[{"{", 
         RowBox[{"k2", "\[Rule]", "1"}], "}"}]}], ")"}], ",", "k1", ",", 
      "n"}], "]"}], "]"}]}], ";"}]], "Input",
 CellChangeTimes->{{3.741067884946085*^9, 3.741067885275538*^9}, {
   3.741164679322756*^9, 3.7411646796226387`*^9}, {3.741165183607019*^9, 
   3.741165185606667*^9}, {3.74116570682456*^9, 3.7411657305145693`*^9}, {
   3.7411673014964323`*^9, 3.7411673211258383`*^9}, {3.7413158602903357`*^9, 
   3.7413158767474117`*^9}, 3.741320699331543*^9},
 ExpressionUUID -> "81f3d099-daa3-42c4-af26-5607545f7e58"],

Cell[BoxData[
 RowBox[{
  RowBox[{"Coef2Bsr", "=", 
   RowBox[{"Table", "[", 
    RowBox[{
     RowBox[{"Coef2Bsr", "[", 
      RowBox[{
       RowBox[{"2", "i"}], ",", 
       RowBox[{"2", "j"}]}], "]"}], ",", 
     RowBox[{"{", 
      RowBox[{"i", ",", "0", ",", "10"}], "}"}], ",", 
     RowBox[{"{", 
      RowBox[{"j", ",", "0", ",", "10"}], "}"}]}], "]"}]}], ";"}]], "Input",
 CellChangeTimes->{{3.7220573274031277`*^9, 3.722057411958555*^9}, {
   3.722057553909235*^9, 3.722057558258687*^9}, 3.722058361827209*^9, {
   3.722059020563114*^9, 3.722059036001809*^9}, {3.722064043326339*^9, 
   3.7220640436134567`*^9}, {3.722068938617219*^9, 3.7220689488567133`*^9}, 
   3.7220690691792727`*^9, {3.722069129642337*^9, 3.722069129865574*^9}, {
   3.72207100528871*^9, 3.7220711073354273`*^9}, {3.72207151536589*^9, 
   3.722071516470203*^9}, {3.722071548694812*^9, 3.7220715507900457`*^9}, {
   3.722071640791222*^9, 3.7220716428698053`*^9}, {3.722158642706012*^9, 
   3.722158647632127*^9}, {3.7221587753440323`*^9, 3.722158777071834*^9}, {
   3.740299016390862*^9, 3.740299018742794*^9}, {3.740299562999009*^9, 
   3.740299566134993*^9}, {3.740299998439867*^9, 3.740300000263646*^9}, {
   3.7403637773136587`*^9, 3.7403637775028477`*^9}, {3.74036395662405*^9, 
   3.740363957136101*^9}, {3.741067949563488*^9, 3.741067953791477*^9}, {
   3.741164687935804*^9, 3.741164690479032*^9}, {3.741165187387107*^9, 
   3.741165189310234*^9}, {3.741165739048711*^9, 3.741165741896358*^9}, {
   3.741167322586659*^9, 3.741167323937245*^9}, {3.741315861125105*^9, 
   3.741315881997106*^9}},
 ExpressionUUID -> "96c6b2e2-e721-46b6-bd9f-4a92af1a35fd"]
}, Closed]],

Cell[CellGroupData[{

Cell["Large-c expansion", "Subsubsection",
 CellChangeTimes->{{3.741164836522542*^9, 3.741164866842805*^9}, {
  3.741335879085162*^9, 3.7413358797092237`*^9}},
 ExpressionUUID -> "ec8ceff6-1b00-4520-85b2-e28ba60c7c18"],

Cell["We have the large-c expansion expression", "Text",
 CellChangeTimes->{{3.724470606233453*^9, 3.724470623578065*^9}, {
  3.7411648516469088`*^9, 3.741164855153366*^9}, {3.741335882966888*^9, 
  3.741335886829115*^9}},
 ExpressionUUID -> "863298f1-c3df-4aeb-9adc-8b1a1d0739f3"],

Cell[BoxData[
 RowBox[{
  RowBox[{"ExRBsrExpansion", "[", "N_", " ", "]"}], ":=", 
  RowBox[{"Simplify", "[", 
   RowBox[{"Sum", "[", 
    RowBox[{
     RowBox[{
      FractionBox["1", 
       SuperscriptBox["c", 
        RowBox[{"2", "n"}]]], 
      RowBox[{"Simplify", "[", 
       RowBox[{"(", 
        RowBox[{
         RowBox[{"+", 
          FractionBox[
           RowBox[{"3", "kF"}], 
           RowBox[{"16", " ", "\[Pi]"}]]}], 
         RowBox[{"Simplify", "[", 
          RowBox[{"(", 
           RowBox[{
            RowBox[{"If", "[", 
             RowBox[{
              RowBox[{
               RowBox[{"Mod", "[", 
                RowBox[{"n", ",", "2"}], "]"}], "\[Equal]", "1"}], ",", 
              RowBox[{"Sum", "[", 
               RowBox[{
                RowBox[{"2", " ", 
                 RowBox[{"Part", "[", 
                  RowBox[{"Coef2Bsr", ",", 
                   RowBox[{"n", "+", "1"}], ",", 
                   RowBox[{"\[Nu]", "+", "1"}]}], "]"}], 
                 RowBox[{"Simplify", "[", 
                  RowBox[{"(", 
                   RowBox[{
                    RowBox[{"Part2ThirdminusFourth", "[", 
                    RowBox[{
                    RowBox[{"n", "-", "\[NoBreak]", "\[Nu]"}], ",", "\[Nu]"}],
                     "]"}], "-", 
                    RowBox[{"Part2SecondminusFirst", "[", 
                    RowBox[{
                    RowBox[{"n", "-", "\[NoBreak]", "\[Nu]"}], ",", "\[Nu]"}],
                     "]"}]}], ")"}], "]"}]}], ",", 
                RowBox[{"{", 
                 RowBox[{"\[Nu]", ",", "0", ",", 
                  RowBox[{
                   RowBox[{"(", 
                    RowBox[{"n", "-", "1"}], ")"}], "/", "2"}]}], "}"}]}], 
               "]"}], ",", "0"}], "]"}], "+", 
            RowBox[{"If", "[", 
             RowBox[{
              RowBox[{
               RowBox[{"Mod", "[", 
                RowBox[{"n", ",", "2"}], "]"}], "\[Equal]", "0"}], ",", " ", 
              RowBox[{
               RowBox[{
                RowBox[{"Part", "[", 
                 RowBox[{"Coef2Bsr", ",", 
                  RowBox[{"n", "+", "1"}], ",", 
                  RowBox[{
                   RowBox[{"n", "/", "2"}], "+", "1"}]}], "]"}], 
                RowBox[{"Simplify", "[", 
                 RowBox[{"(", 
                  RowBox[{
                   RowBox[{"Part2ThirdminusFourth", "[", 
                    RowBox[{
                    RowBox[{"n", "-", "\[NoBreak]", 
                    RowBox[{"n", "/", "2"}]}], ",", 
                    RowBox[{"n", "/", "2"}]}], "]"}], "-", 
                   RowBox[{"Part2SecondminusFirst", "[", 
                    RowBox[{
                    RowBox[{"n", "-", "\[NoBreak]", 
                    RowBox[{"n", "/", "2"}]}], ",", 
                    RowBox[{"n", "/", "2"}]}], "]"}]}], ")"}], "]"}]}], "+", 
               RowBox[{"Sum", "[", 
                RowBox[{
                 RowBox[{"2", 
                  RowBox[{"Part", "[", 
                   RowBox[{"Coef2Bsr", ",", 
                    RowBox[{"n", "+", "1"}], ",", 
                    RowBox[{"\[Nu]", "+", "1"}]}], "]"}], 
                  RowBox[{"Simplify", "[", 
                   RowBox[{"(", 
                    RowBox[{
                    RowBox[{"Part2ThirdminusFourth", "[", 
                    RowBox[{
                    RowBox[{"n", "-", "\[NoBreak]", "\[Nu]"}], ",", "\[Nu]"}],
                     "]"}], "-", 
                    RowBox[{"Part2SecondminusFirst", "[", 
                    RowBox[{
                    RowBox[{"n", "-", "\[NoBreak]", "\[Nu]"}], ",", "\[Nu]"}],
                     "]"}]}], ")"}], "]"}]}], ",", 
                 RowBox[{"{", 
                  RowBox[{"\[Nu]", ",", "0", ",", 
                   RowBox[{
                    RowBox[{"(", 
                    RowBox[{"n", "-", "2"}], ")"}], "/", "2"}]}], "}"}]}], 
                "]"}]}], ",", "0"}], "]"}]}], ")"}], "]"}]}], ")"}], "]"}]}], 
     ",", " ", 
     RowBox[{"{", 
      RowBox[{"n", ",", "0", ",", 
       RowBox[{"N", "/", "2"}]}], "}"}]}], "]"}], "]"}]}]], "Input",
 CellChangeTimes->{{3.722754572486408*^9, 3.7227546129606533`*^9}, {
   3.741165015141117*^9, 3.741165045250079*^9}, {3.741165197810758*^9, 
   3.741165254957601*^9}, {3.741165773814*^9, 3.741165787768862*^9}, {
   3.741167340996427*^9, 3.7411674221001043`*^9}, {3.7411674682156353`*^9, 
   3.741167476614678*^9}, {3.7413142924460087`*^9, 3.741314309866496*^9}, {
   3.7413159856659107`*^9, 3.74131600245077*^9}, 3.741317069053763*^9, {
   3.741319489285994*^9, 3.7413194914003077`*^9}, {3.7413211803131742`*^9, 
   3.741321189643249*^9}},
 ExpressionUUID -> "c631a045-ad99-446b-b9cc-8b657bf23fa8"],

Cell["\<\
We first calculate the large-c expansion to a satisfying order, let\
\[CloseCurlyQuote]s say 20.\
\>", "Text",
 CellChangeTimes->{{3.722658255655129*^9, 3.722658274741214*^9}, {
  3.741335910521679*^9, 
  3.741335912461376*^9}},ExpressionUUID->"aa3105b6-5b01-41de-aacd-\
b8f17e1e59c3"],

Cell[BoxData[
 RowBox[{
  RowBox[{"ExRBsrOrder20", "=", 
   RowBox[{"ExRBsrExpansion", "[", "20", "]"}]}], ";"}]], "Input",
 CellChangeTimes->{{3.722657885346245*^9, 3.722657905194455*^9}, {
   3.72265917006719*^9, 3.722659250932714*^9}, {3.722763920069398*^9, 
   3.722763928880912*^9}, {3.740299051015119*^9, 3.740299051080347*^9}, {
   3.740363795247789*^9, 3.740363796239716*^9}, {3.7411652585174932`*^9, 
   3.7411652633781548`*^9}, {3.741165795859723*^9, 3.7411657984422483`*^9}, {
   3.741313222841453*^9, 3.741313257225306*^9}, {3.741315481468864*^9, 
   3.741315506042829*^9}, {3.741316015949769*^9, 3.741316019244528*^9}, {
   3.7413170707818003`*^9, 3.741317071502873*^9}, 3.741319495220552*^9},
 ExpressionUUID -> "987f9c66-8483-4a9d-bc59-d64a4e9e6fea"],

Cell[BoxData[
 RowBox[{
  RowBox[{"ExRBOrder20", "=", 
   RowBox[{"Limit", "[", 
    RowBox[{"ExRBsrOrder20", ",", 
     RowBox[{"\[Mu]", "\[Rule]", "0"}]}], "]"}]}], ";"}]], "Input",
 CellChangeTimes->{
  3.7227558995802526`*^9, {3.7411657967815123`*^9, 3.7411657994598923`*^9}, 
   3.741313225929617*^9, {3.741313263481997*^9, 3.741313264425818*^9}, {
   3.741315509596798*^9, 3.741315510780417*^9}, {3.741316023900951*^9, 
   3.7413160507329493`*^9}},
 ExpressionUUID -> "c1afbf3c-b5df-46b8-884b-e4431185951a"]
}, Closed]],

Cell[CellGroupData[{

Cell["Pad\[EAcute] approximants", "Subsubsection",
 CellChangeTimes->{{3.7411649136217203`*^9, 3.741164917030664*^9}, {
  3.741164959746048*^9, 3.741164964829475*^9}, {3.741335936109335*^9, 
  3.741335936461323*^9}},
 ExpressionUUID -> "1daa3f19-7fea-4e3a-9d60-00ca91a25d0e"],

Cell["\<\
We prepare the coefficient of the large-c expansion, for the short-range \
exchange energy and for the \[Mu] \[RightArrow] 0 limit\
\>", "Text",
 CellChangeTimes->{{3.7227553188603687`*^9, 3.722755371373106*^9}, {
  3.72275562759557*^9, 3.7227556515776443`*^9}, {3.724470657833439*^9, 
  3.72447066020118*^9}, {3.741315414203617*^9, 3.741315470363694*^9}}],

Cell[BoxData[
 RowBox[{
  RowBox[{"CoefficientBsr", "[", 
   RowBox[{"M_", ",", "n_"}], "]"}], ":=", 
  RowBox[{"Simplify", "[", 
   RowBox[{"Coefficient", "[", 
    RowBox[{
     RowBox[{"ExRBsrOrder20", "/.", 
      RowBox[{"{", 
       RowBox[{"c", "\[Rule]", 
        RowBox[{"1", "/", "x"}]}], "}"}]}], ",", "x", ",", "n"}], "]"}], 
   "]"}]}]], "Input",
 CellChangeTimes->{{3.7226678420237913`*^9, 3.722667861528064*^9}, {
   3.72266815372162*^9, 3.7226681849194813`*^9}, {3.7226721981498747`*^9, 
   3.722672207155808*^9}, 3.7227550567672377`*^9, {3.722755656577574*^9, 
   3.7227556642370653`*^9}, {3.741165279910945*^9, 3.741165280303294*^9}, {
   3.741165801108734*^9, 3.741165802557379*^9}, {3.741314586153861*^9, 
   3.741314586281663*^9}, {3.7413148850075493`*^9, 3.741314885241417*^9}, {
   3.741315516652811*^9, 3.7413155175013733`*^9}, {3.7413161019493837`*^9, 
   3.741316104733344*^9}},
 ExpressionUUID -> "8a7d4bab-2a35-4def-8bce-a73356c6c725"],

Cell[BoxData[
 RowBox[{
  RowBox[{"CoefficientB", "[", 
   RowBox[{"M_", ",", "n_"}], "]"}], ":=", 
  RowBox[{"Simplify", "[", 
   RowBox[{"Coefficient", "[", 
    RowBox[{
     RowBox[{"ExRBOrder20", "/.", 
      RowBox[{"{", 
       RowBox[{"c", "\[Rule]", 
        RowBox[{"1", "/", "x"}]}], "}"}]}], ",", "x", ",", "n"}], "]"}], 
   "]"}]}]], "Input",
 CellChangeTimes->{{3.7227556735963917`*^9, 3.7227556754363728`*^9}, {
   3.741165291318172*^9, 3.7411653095641212`*^9}, {3.7411658075165567`*^9, 
   3.741165809802228*^9}, {3.741314633492703*^9, 3.741314634757943*^9}, 
   3.741314919610902*^9, {3.741315520381742*^9, 3.741315521149824*^9}, {
   3.7413161089280157`*^9, 3.7413161107667713`*^9}},
 ExpressionUUID -> "eebafb90-9827-4bd4-8010-f99bfe8d64a7"],

Cell[BoxData[
 RowBox[{
  RowBox[{"CoefBsr", "[", "M_", "]"}], ":=", 
  RowBox[{"Table", "[", 
   RowBox[{
    RowBox[{
     SubscriptBox["T", "i"], "->", 
     RowBox[{"CoefficientBsr", "[", 
      RowBox[{"M", ",", "i"}], "]"}]}], ",", 
    RowBox[{"{", 
     RowBox[{"i", ",", "0", ",", "M"}], "}"}]}], "]"}]}]], "Input",
 CellChangeTimes->{{3.722749765088842*^9, 3.722749844950129*^9}, {
   3.72275111355685*^9, 3.7227511736510963`*^9}, {3.7227512675099688`*^9, 
   3.722751272325121*^9}, 3.722752713870413*^9, {3.7227542354300613`*^9, 
   3.722754236382597*^9}, {3.722755666317625*^9, 3.7227556680165157`*^9}, {
   3.7411652856659613`*^9, 3.741165288839732*^9}, {3.741165803964905*^9, 
   3.741165805816494*^9}, {3.741314890229391*^9, 3.741314893738743*^9}, {
   3.7413149288437023`*^9, 3.741314934843973*^9}, {3.741316114910597*^9, 
   3.741316117071061*^9}},
 ExpressionUUID -> "7e389313-60d7-458a-8661-49a0901bd7a6"],

Cell[BoxData[
 RowBox[{
  RowBox[{"CoefB", "[", "M_", "]"}], ":=", 
  RowBox[{"Table", "[", 
   RowBox[{
    RowBox[{
     SubscriptBox["T", "i"], "->", 
     RowBox[{"CoefficientB", "[", 
      RowBox[{"M", ",", "i"}], "]"}]}], ",", 
    RowBox[{"{", 
     RowBox[{"i", ",", "0", ",", "M"}], "}"}]}], "]"}]}]], "Input",
 CellChangeTimes->{{3.722755679643105*^9, 3.722755680670816*^9}, {
   3.7411652967818327`*^9, 3.7411652992974167`*^9}, 3.7411658123477707`*^9, 
   3.7411662521890163`*^9, {3.741314937994246*^9, 3.741314954859644*^9}, {
   3.7413161182066517`*^9, 3.741316127084984*^9}},
 ExpressionUUID -> "3a506947-528f-4649-bd86-f4d5b72b8289"],

Cell["\<\
We now express the specific coefficients for our Pad\[EAcute] approximant \
using the order-20 large-c expansion\
\>", "Text",
 CellChangeTimes->{{3.722763848195755*^9, 3.722763880899667*^9}, {
  3.741315729450776*^9, 3.7413157473068323`*^9}, {3.741335949949676*^9, 
  3.741335960541609*^9}},ExpressionUUID->"6ada03bb-338d-440e-92fd-\
f20b4878f40e"],

Cell[BoxData[
 RowBox[{
  RowBox[{"CoefBPad\[EAcute]B", "=", 
   RowBox[{
    RowBox[{"CoefBPad\[EAcute]", "[", "10", "]"}], "/.", 
    RowBox[{"CoefB", "[", "20", "]"}]}]}], ";"}]], "Input",
 CellChangeTimes->{{3.722753594171132*^9, 3.722753620589405*^9}, 
   3.722753773971465*^9, 3.722753896092773*^9, {3.722754258580085*^9, 
   3.7227542587988586`*^9}, {3.722754465761252*^9, 3.722754485745597*^9}, {
   3.72275541074507*^9, 3.722755440462531*^9}, {3.722755709305892*^9, 
   3.7227557107485*^9}, {3.7227560316951523`*^9, 3.722756055026368*^9}, {
   3.722756395457559*^9, 3.722756409823081*^9}, {3.741165336843622*^9, 
   3.741165357183463*^9}, {3.741165825467124*^9, 3.7411658299082203`*^9}, {
   3.7413149650996237`*^9, 3.7413149699957933`*^9}, {3.741315265420334*^9, 
   3.741315266187937*^9}, {3.741315550782506*^9, 3.7413155823186483`*^9}, {
   3.741315643371585*^9, 3.741315647437683*^9}, {3.7413161558032913`*^9, 
   3.741316159532916*^9}},
 ExpressionUUID -> "bf7b8143-ef4b-49f2-a89f-abc0120114fb"],

Cell[BoxData[
 RowBox[{
  RowBox[{"CoefBPad\[EAcute]Bsr", "=", 
   RowBox[{
    RowBox[{"CoefBPad\[EAcute]", "[", "10", "]"}], "/.", 
    RowBox[{"CoefBsr", "[", "20", "]"}]}]}], ";"}]], "Input",
 CellChangeTimes->{{3.7227563927641907`*^9, 3.722756424828418*^9}, {
  3.722756470028845*^9, 3.722756471262659*^9}, {3.741165338166099*^9, 
  3.74116535636982*^9}, {3.741165826280868*^9, 3.741165830758252*^9}, {
  3.741314982347934*^9, 3.7413149848775673`*^9}, {3.741315268045794*^9, 
  3.74131526958106*^9}, {3.741315564238062*^9, 3.741315585069827*^9}, {
  3.741315648332552*^9, 3.741315649151641*^9}, {3.7413161612941227`*^9, 
  3.741316163326283*^9}},
 ExpressionUUID -> "d8937fb1-2e8b-4335-85a2-60dfa103748a"],

Cell[BoxData[
 RowBox[{
  RowBox[{"CoefAPad\[EAcute]B", "=", 
   RowBox[{
    RowBox[{"CoefAPad\[EAcute]", "[", "10", "]"}], "/.", 
    RowBox[{"CoefB", "[", "20", "]"}]}]}], ";"}]], "Input",
 CellChangeTimes->{{3.722754029546383*^9, 3.722754044308186*^9}, {
   3.722754301982415*^9, 3.722754302035227*^9}, {3.7227544718864326`*^9, 
   3.722754488205662*^9}, {3.722755452684111*^9, 3.722755452924046*^9}, 
   3.7227557289252*^9, {3.722756027149149*^9, 3.722756058413001*^9}, 
   3.722756119853417*^9, 3.722756296716875*^9, {3.722756447367597*^9, 
   3.722756450307869*^9}, {3.741165339561618*^9, 3.741165355379118*^9}, {
   3.741165827109076*^9, 3.741165832083321*^9}, {3.741314987228261*^9, 
   3.7413149885234613`*^9}, {3.741315271836527*^9, 3.741315272429305*^9}, {
   3.7413155708925943`*^9, 3.741315586204362*^9}, {3.741315650300768*^9, 
   3.741315651546886*^9}, {3.741316164462429*^9, 3.741316167247802*^9}},
 ExpressionUUID -> "833becab-154e-4061-9bd2-e5410ea49d60"],

Cell[BoxData[
 RowBox[{
  RowBox[{"CoefAPad\[EAcute]Bsr", "=", 
   RowBox[{
    RowBox[{"CoefAPad\[EAcute]", "[", "10", "]"}], "/.", 
    RowBox[{"CoefBsr", "[", "20", "]"}]}]}], ";"}]], "Input",
 CellChangeTimes->{{3.722756457980381*^9, 3.722756467531996*^9}, {
  3.741165343013163*^9, 3.741165354109902*^9}, {3.741165828153932*^9, 
  3.741165833829134*^9}, {3.741314992123789*^9, 3.741314992987317*^9}, {
  3.741315274700562*^9, 3.741315280252084*^9}, {3.74131558898942*^9, 
  3.741315591501307*^9}, {3.741315652989523*^9, 3.7413156541452312`*^9}, {
  3.741316170380205*^9, 3.7413161727343283`*^9}},
 ExpressionUUID -> "8282e9b8-c019-43ff-a14a-1ea64fe8290f"],

Cell["\<\
We can now define our Pad\[EAcute] approximants for the full-range and the \
short-range Breit exchange energies per particle\
\>", "Text",
 CellChangeTimes->{{3.7227640074737988`*^9, 3.722764017491691*^9}, {
  3.7413359698036127`*^9, 
  3.741335998859766*^9}},ExpressionUUID->"bdfaf6df-6ec3-49bb-aaee-\
e11367a46ec2"],

Cell[BoxData[
 RowBox[{
  RowBox[{"ExRBPad\[EAcute]", "[", "M_", "]"}], ":=", 
  RowBox[{
   RowBox[{"(", 
    RowBox[{"Sum", "[", 
     RowBox[{
      FractionBox[
       RowBox[{"Part", "[", 
        RowBox[{"CoefAPad\[EAcute]B", ",", "M", ",", 
         RowBox[{"k", "+", "1"}]}], "]"}], 
       SuperscriptBox["c", "k"]], ",", 
      RowBox[{"{", 
       RowBox[{"k", ",", "0", ",", "M"}], "}"}]}], "]"}], ")"}], "/", 
   RowBox[{"(", 
    RowBox[{"1", "+", 
     RowBox[{"Sum", "[", 
      RowBox[{
       FractionBox[
        RowBox[{"Part", "[", 
         RowBox[{"CoefBPad\[EAcute]B", ",", "M", ",", "k"}], "]"}], 
        SuperscriptBox["c", "k"]], ",", 
       RowBox[{"{", 
        RowBox[{"k", ",", "1", ",", "M"}], "}"}]}], "]"}]}], 
    ")"}]}]}]], "Input",
 CellChangeTimes->{{3.7227562198866377`*^9, 3.722756223232061*^9}, {
  3.722756344477265*^9, 3.722756374429248*^9}, {3.724472328737096*^9, 
  3.7244723404597588`*^9}, {3.7244725391989813`*^9, 3.724472541421919*^9}, {
  3.7244732518101883`*^9, 3.724473255736369*^9}, {3.7411651613833103`*^9, 
  3.741165167052189*^9}, {3.7411653461762133`*^9, 3.7411653497927322`*^9}, {
  3.741165839085773*^9, 3.741165845925786*^9}, {3.7413156004345922`*^9, 
  3.7413156087854156`*^9}, {3.7413161805897408`*^9, 3.741316200798999*^9}, {
  3.741319513007175*^9, 3.7413195147391453`*^9}, {3.741320467171023*^9, 
  3.741320467410928*^9}},
 ExpressionUUID -> "f6ea00f0-ec8d-4051-9788-d630ebc87bce"],

Cell[BoxData[
 RowBox[{
  RowBox[{"ExRBsrPad\[EAcute]", " ", "[", "M_", "]"}], ":=", 
  RowBox[{
   RowBox[{"(", 
    RowBox[{"Sum", "[", 
     RowBox[{
      FractionBox[
       RowBox[{"Part", "[", 
        RowBox[{"CoefAPad\[EAcute]Bsr", ",", "M", ",", 
         RowBox[{"k", "+", "1"}]}], "]"}], 
       SuperscriptBox["c", "k"]], ",", 
      RowBox[{"{", 
       RowBox[{"k", ",", "0", ",", "M"}], "}"}]}], "]"}], ")"}], "/", 
   RowBox[{"(", 
    RowBox[{"1", "+", 
     RowBox[{"Sum", "[", 
      RowBox[{
       FractionBox[
        RowBox[{"Part", "[", 
         RowBox[{"CoefBPad\[EAcute]Bsr", ",", "M", ",", "k"}], "]"}], 
        SuperscriptBox["c", "k"]], ",", 
       RowBox[{"{", 
        RowBox[{"k", ",", "1", ",", "M"}], "}"}]}], "]"}]}], 
    ")"}]}]}]], "Input",
 CellChangeTimes->{{3.722754133946948*^9, 3.722754168197061*^9}, 
   3.722755764286047*^9, {3.722755795648616*^9, 3.7227557972443647`*^9}, {
   3.722756165936594*^9, 3.7227562108616667`*^9}, {3.722756481371945*^9, 
   3.722756490285556*^9}, {3.724472343389707*^9, 3.724472353121357*^9}, {
   3.724473258746921*^9, 3.724473263323648*^9}, {3.741165168482983*^9, 
   3.741165168762787*^9}, {3.7411653511334343`*^9, 3.741165353067666*^9}, {
   3.7411658422331877`*^9, 3.741165847801704*^9}, {3.741315603778873*^9, 
   3.741315606040073*^9}, {3.741316184686599*^9, 3.741316204541964*^9}, 
   3.741319512101202*^9, {3.741320464964718*^9, 3.741320465138805*^9}},
 ExpressionUUID -> "10eb1b52-8df3-49f0-b678-d642cb9904ae"]
}, Closed]]
}, Closed]],

Cell[CellGroupData[{

Cell["Tests", "Subsection",
 CellChangeTimes->{{3.7411646556876497`*^9, 3.741164658735076*^9}}],

Cell[CellGroupData[{

Cell["Full-range Breit exchange energy per particle", "Subsubsection",
 CellChangeTimes->{{3.741166404504117*^9, 3.74116641070641*^9}, 
   3.74131965313426*^9, {3.741320529698434*^9, 3.7413205323543262`*^9}, 
   3.741320618101907*^9, {3.7413360218169127`*^9, 3.7413360255049553`*^9}},
 ExpressionUUID -> "4afc1e85-1253-4af0-8306-16ff736415c1"],

Cell[CellGroupData[{

Cell[BoxData[
 RowBox[{"ExRBPad\[EAcute]2", "=", 
  RowBox[{"Simplify", "[", 
   RowBox[{"ExRBPad\[EAcute]", "[", "2", "]"}], "]"}]}]], "Input",
 CellChangeTimes->{{3.7413206194463654`*^9, 3.7413206194579363`*^9}},
 ExpressionUUID -> "5d1d01b0-9a7a-42b8-912e-b434ed13d982"],

Cell[BoxData[
 FractionBox[
  RowBox[{"125", " ", "kF"}], 
  RowBox[{
   RowBox[{"198", " ", "\[Pi]"}], "+", 
   RowBox[{"300", " ", 
    SuperscriptBox["c", "2"], " ", "\[Pi]"}]}]]], "Output",
 CellChangeTimes->{3.7413206241258087`*^9, 3.7413209218838377`*^9, 
  3.741336042567102*^9, 3.741408558315051*^9, 3.74140863001085*^9, 
  3.74140953315545*^9, 3.7414100831975594`*^9},
 ExpressionUUID -> "b681ce6c-496c-431d-b141-ee58b7180e09"]
}, Open  ]],

Cell[CellGroupData[{

Cell[BoxData[
 RowBox[{"ExRBPad\[EAcute]4", "=", 
  RowBox[{"Simplify", "[", 
   RowBox[{"ExRBPad\[EAcute]", "[", "4", "]"}], "]"}]}]], "Input",
 CellChangeTimes->{{3.741320544979157*^9, 3.741320548322682*^9}},
 ExpressionUUID -> "5995df5b-3eab-4246-b873-5ed84eec6651"],

Cell[BoxData[
 FractionBox[
  RowBox[{"35", " ", 
   RowBox[{"(", 
    RowBox[{"62417", "+", 
     RowBox[{"112050", " ", 
      SuperscriptBox["c", "2"]}]}], ")"}], " ", "kF"}], 
  RowBox[{"24", " ", 
   RowBox[{"(", 
    RowBox[{"127443", "+", 
     RowBox[{"477295", " ", 
      SuperscriptBox["c", "2"]}], "+", 
     RowBox[{"392175", " ", 
      SuperscriptBox["c", "4"]}]}], ")"}], " ", "\[Pi]"}]]], "Output",
 CellChangeTimes->{3.741319800239278*^9, 3.741320094376034*^9, 
  3.741320963957502*^9, 3.7413360426136227`*^9, 3.741408558426804*^9, 
  3.7414086300872507`*^9, 3.7414095332955217`*^9, 3.7414100833248367`*^9},
 ExpressionUUID -> "67d570a9-22f6-4a67-a8b3-95e0f0e98abd"]
}, Open  ]],

Cell[CellGroupData[{

Cell[BoxData[
 RowBox[{"ExRBPad\[EAcute]6", "=", 
  RowBox[{"Simplify", "[", 
   RowBox[{"ExRBPad\[EAcute]", "[", "6", "]"}], "]"}]}]], "Input",
 CellChangeTimes->{{3.741320550338684*^9, 3.741320552564827*^9}},
 ExpressionUUID -> "263ff912-7602-4260-b1c6-47d886514680"],

Cell[BoxData[
 FractionBox[
  RowBox[{
   RowBox[{"(", 
    RowBox[{"6211753183071", "+", 
     RowBox[{"27901124665260", " ", 
      SuperscriptBox["c", "2"]}], "+", 
     RowBox[{"25677653501500", " ", 
      SuperscriptBox["c", "4"]}]}], ")"}], " ", "kF"}], 
  RowBox[{"200", " ", 
   RowBox[{"(", 
    RowBox[{"42232061575", "+", 
     RowBox[{"282365117775", " ", 
      SuperscriptBox["c", "2"]}], "+", 
     RowBox[{"538180511715", " ", 
      SuperscriptBox["c", "4"]}], "+", 
     RowBox[{"308131842018", " ", 
      SuperscriptBox["c", "6"]}]}], ")"}], " ", "\[Pi]"}]]], "Output",
 CellChangeTimes->{3.741319838419587*^9, 3.741320097292377*^9, 
  3.74132096639118*^9, 3.741336042637965*^9, 3.741408558432271*^9, 
  3.741408630171752*^9, 3.74140953333967*^9, 3.7414100834579678`*^9, 
  3.7414107556664047`*^9},
 ExpressionUUID -> "fa46eade-f011-4379-bf87-6bf71bce4948"]
}, Open  ]],

Cell[BoxData[
 RowBox[{
  RowBox[{"ExRBPad\[EAcute]8", "=", 
   RowBox[{"Simplify", "[", 
    RowBox[{"ExRBPad\[EAcute]", "[", "8", "]"}], "]"}]}], ";"}]], "Input",
 CellChangeTimes->{{3.7414106921697483`*^9, 3.7414106941977053`*^9}, {
  3.7414107575751953`*^9, 3.741410757831979*^9}}],

Cell[CellGroupData[{

Cell[BoxData[
 RowBox[{"Plot", "[", 
  RowBox[{
   RowBox[{"{", 
    RowBox[{
     RowBox[{"ExRB", "/.", 
      RowBox[{"{", 
       RowBox[{"c", "\[Rule]", 
        RowBox[{"137.036", "/", "kF"}]}], "}"}]}], ",", 
     RowBox[{"ExRBOrder20", "/.", 
      RowBox[{"{", 
       RowBox[{"c", "\[Rule]", 
        RowBox[{"137.036", "/", "kF"}]}], "}"}]}], ",", 
     RowBox[{"ExRBPad\[EAcute]2", "/.", 
      RowBox[{"{", 
       RowBox[{"c", "\[Rule]", 
        RowBox[{"137.036", "/", "kF"}]}], "}"}]}], ",", 
     RowBox[{"ExRBPad\[EAcute]4", "/.", 
      RowBox[{"{", 
       RowBox[{"c", "\[Rule]", 
        RowBox[{"137.036", "/", "kF"}]}], "}"}]}], ",", 
     RowBox[{"ExRBPad\[EAcute]6", "/.", 
      RowBox[{"{", 
       RowBox[{"c", "\[Rule]", 
        RowBox[{"137.036", "/", "kF"}]}], "}"}]}]}], "}"}], ",", 
   RowBox[{"{", 
    RowBox[{"kF", ",", "0", ",", "300"}], "}"}], ",", 
   RowBox[{"PlotStyle", "\[Rule]", 
    RowBox[{"{", 
     RowBox[{"Blue", ",", "Red", ",", "Green", ",", "Purple", ",", "White"}], 
     "}"}]}]}], "]"}]], "Input",
 CellChangeTimes->{{3.725790426404578*^9, 3.725790453840857*^9}, {
   3.725790502785564*^9, 3.725790550992629*^9}, {3.726898837998486*^9, 
   3.726898847052638*^9}, {3.741165900638431*^9, 3.7411659400545387`*^9}, {
   3.741166056629149*^9, 3.741166057200569*^9}, 3.7413162488297863`*^9, {
   3.741318686271461*^9, 3.741318713551878*^9}, {3.7413187477294397`*^9, 
   3.741318749185649*^9}, {3.741320129814933*^9, 3.741320147957473*^9}, {
   3.7413205551420794`*^9, 3.7413205557639*^9}, {3.741320980068277*^9, 
   3.741320992978437*^9}},
 ExpressionUUID -> "321391df-44fd-4ce9-9fe2-fe784e534efb"],

Cell[BoxData[
 GraphicsBox[{{{}, {}, {}, 
    TagBox[
     {RGBColor[1, 0, 0], AbsoluteThickness[1.6], Opacity[1.], 
      LineBox[CompressedData["
1:eJwVl3k81c0Xx20VQvY93Pu1hULWx3LnZFf0kETW+733tlFZslWWRGUJEcka
EREKTxKVi7JFoVCSLSn7kq2y/O7vr3m9X+c1c875zJmZMwSK15ETLExMTL7M
TEz/HyuPrS/PlH4mmfFfuLCRla0f3eTWZxv/DD3EMi/M5uqQbvVfvSwV34wy
iKphR3JPkWYVH22LKe5Cyp6/1ebnIkjJY8kdbPF9SE7w8uOtnFSSXk5oSpjP
V/Rh5NFNeYFC0vze//aFFI+gpLch/9TMVZIadxYl6WWOoVe0bx/9H9aR7kxk
razG/UCV99VmG3KaSWeak5yehk2ihBvaskrdnSSDBzde+frMoDOahtnj/H2k
qAMkvrvq82j9akDMtqpBks8T3caA4gVkfmEz/NLcN5KTtIa/PfYLOVQtmyU6
TpBM4vcqaGYuISar5qsbhXOkfRsKn/mFVtD3C3IPagJ/kUTOEmMX4laRuEuX
okPOKonpi6Rh5/bfSJFavFh2bJ00aSkyVxb2B8WpfNZ918WEPlTz5cat/UVv
/SRm1ptZ0QsFLruzPhsIvFUTbfh3oII727cdmtxEdh+ct7SecqKWq1e+JKsz
QX4wPif2lAcZ1IRoss0ywbwOfkkzlg+VL1yKu1DMDPFBka+aZwWQ/J6g8dGT
LCCO7/gRfEMYpZP90RGMFViNiCwxDmJo113fu/VDrOCXHcwuh0uiyPdeC2qZ
bPCAxXYgokAa/d5+7mCO4zbAAy1kZ5MJ6DzJI2+X0HbY68nGVBGAIYdSmv1s
3A5oGFx7N5WtgNrH8DLXg+ww3taomfpjDwJJ9x0d2zngxMAF2TdHVZBS7PHn
j8I44alKbkB0pxrKbjjGL2GwE6oPpn/TOLAfCfyx84xZ2wkX5KdTjjZpoPXT
h3ef8eGGSZbD/nt5dZBPzqGAT3t5IMOa59tWjy4a77N4bz7JA1dCxEVCKvTQ
6bxcuK3OC4vEuV+PykmIiGRm2hJ4YWej59taD0AD/dlpLLO8YEea+80bfQDZ
8mcu+hTzgWTuOw1s2hhxlYnfK2Lnh8PTUULn1E1Rk2XaoZGT/FD68RMTRJoh
vfA7+TaYAGgEdJ9Kt7NES5JCtlHhApD8pj6hrPMgelx9e6NuiGG/lSF2wsUK
yc7fOqaaKQhu1W3nunP+RYOxu1hP/RGEyK0LXzhLbVCaQvzjbEchGKrKV41J
tEU87rHsPELCMD8cZFLma4dWO67VTMeJQP3Ptg08zQHREKcu35IIJN4upzt3
OaLuJ/FPtZxEweM/U70RASdUdjv1Sai8GOBLtrkHnrsgyW2S+/JuioH/6tli
f0k3FB2Q86h5UQzqRO1yf8S4I9rxogLeOnHwvrT1SMIUR91te2W15CRAxkJ3
2zNuCgKDitzjsRIwFTNrfnCAgiSkazPvO0hCbM03t/JYGuoea0/SnN8NgqET
HHNapxEcs+U9fkwK+g+8WatSO4PKmnviQl5IgaSKl7rifg8UXTwY1RQlDZ7L
HmtulmeRjG4QKrklAx/e+Bq8PuGN+rz1Ql81ysCAxZVKli1vFF+0/qJzRQba
EpukZjN80Lp4uN6yCwFKrF73rw77or6NaC3SHiKEkoKbONP8Uby2lZ+NCxGu
5nW2jNkEIBMvnkpKAhHYLm/Pb+QKRBXDSWo3lomQa5n/tPZWEIpvzFDurMcg
/kBqYnPbZWS67uoxuoTBqGtY5Z+8YLSuKVO0pCALz+YTpWLCQ5BHQb68WLws
zOdXUycsw5BpdCmB4iQH9RlyhHNR4Wi93ovsFycHz/ZX7eHdcRVV/FG/d50u
B1qBbJ1cUVeRzNkqyUfy8sA5V5mtmBiB1g/XiSwtysPzJc6CcPo1VCnYxX09
VhG6THVbve/GoBc+EmNatYogkHq9i18zFr1+d6Lm+6QiRP/V2sPVHYt6o/6c
ND24B56c+LRXWCgOra1jdDYOJZBUVlFirk5ApO8BvhHXlYGZeR0PrUlC5kb1
FhpVylBqeXWRW/I2srm3U/rbd2VY4e+vnwq9jfDjOW+NTFVgfiWhPN0iGUV2
tMqysO2F9rdOLczTKajtqWTflfB9YJNVX9Xtl4a6+U+VqpXvg0VyR7TZdBr6
4lUeMTy8DyY1ZMqVTqSj6T1magCqoOe+y8vKOQPtyvaK3tpUBf3xwSK141lI
yXhkN3qlBuwGwXJF73JQmc92DpFeNdAcz3tPFc5FGjnKS7MzauBJf3Lqh1su
Mtjwb8verQ7bv8lGWS/mIutnnIGbweow36kYVUHMQ97Kmp0v9ffD4cYWr6bi
B2hQx3xrt91+mG/GhYY3HiBrE6d9oR77IeLO6MM22wKk5HrlJiltP2ylK3gL
rxeg7/HtFnUr+8EprdEqz+khclqk1dPLNcCyZ73gFDxCLZuB8zKtGlDO3V3G
kvsI6eyMlQ4f1oC+deqXEJYSJChbHnJglyZIpyScEG0pQe/sN/5pOMvgi6Nh
a65lyPh5SkWjghYsXsPG0/ufoIo3D0cwpAU29xbyCfzlSKa7ljfymBb8IG79
lD5YjjYnR86bXNMC+kx7X2RtOaqW3Kf8ZlQLpEX9FDbyKpDKlaa8pixtWMtj
quG++R8SNl9NbhXQBdezARO9tdVoseXQmuxeXZB1ArcDHM9Rx8Ec5ytmuqBM
/uRl6fAcRR62JOpc1IUPRiUPNJefo0X7jMf5g7ogoEj4dV23FnXQUFtY0T+w
oGW9cufrSxR59caWFtKH0Jqbc+nd9YjMNkBJdNSHe0Z7RSpYG5D+dbWmaR99
EG+QeSWj1YAWoz/fzMvXhyorsdRtaQ2InKgszsdpAKENBq1LtEZkkPNec/qj
ARAEchzzuN+gXy9FPO57kCC2eYJ7Z34LWrNVS7O6SoLLCdvbIwda0Pp3i5aV
NBKcv8D6wVaoFbHxXJI/1EqCdc/kG+M3WpGw28DoLwUEeZYpokw+bUh3M8fZ
9DuCm7/4fkrbtSMknSK/9Bgg9I25u7ZKJzI6QyC11gIkckkRP1l3IpPKUvvs
ZoC2+xVZBV6dyMK8KdJiCOC8Z9vutspOZOO1OprJcwD+arv27CV1IUrd8Xum
5w7A7Vbn+GDnbnTNXUo0VckIzsRd8e+r/ohItLetZ3SM4CWTek7st49o5XTQ
ZQMTI2jJ0X4UyNODTvt2D464GoHxZ6xrldaDDl67/kAl0QhcMkXIGYK9iOfR
7P6GVSOYszuN3wjtQ3dXXlnPvDaG0wIUq9KQfmTz13OrrssYFt5rFyQ+7kcc
TGLlSYPG4EH7vq98pB9d4rggqLtmDLSEber3zb4gV0mFL1eVTYBfgq/8sMAA
IholnBZNMoGEwsvSP559RSVx7hHG7qbwkjf7nlvqMHIKZ3Xo9zQFRY+J+uTK
YcTuX6jkE2QKNREyn36+H0ZUl7mu7ERTqDuZxTnFPoLElcNk/jSagnFlSalj
8AiKasl++UTRDF787f09cnoU0VgHV3cvmsHBltVtvxzHkMRFl7NrkRYg1Equ
lEn9iQb9Rx9U3bKAimCBY/9V/0Q5vqeH/DItIKbLh5fW/xPJnvU7slBpAUNe
7uMiUhNIxf2m7uSoBbTxZLR3FUwgkukLtgGwBNHxVuHkl5MI55PMqlu3BEku
qZoQphlUWPSl47rfIfi3uqI1aXYeyeBXc43CD4FJUgP7E7YFdFd0j/9m3CH4
StPLGRRfQDE3AiQDCg/BkbnjY17mC+jsCT7PE/2H4P4IhyA1dwGpEczZTcAK
rl3xvRPvuIhq7lYYMXNZQ3fT+mHuj7/QuxvRzy7nHQZop33dz7SKYnoGuOTe
2UCopPBFhdIN1PmmO5jX+AhoW7PXJaaywBjXsNrjPjuoWrAyWtHcATcC9uXq
2dpDbP47jjQ2LljVTra/OHkMHogq6O38xuhrevssDIIdYYcHfQD+CEBZqsva
1OJx2JLs4esWEgGpJ2tTh6OdYcSJVp9VKg67p3oystlcoSfohqO7uhRMBrcl
5N5zA0flLw9jtjHe1aaUkrkHbqDLxYKvchHgPC/ealjiBq57B8ZxQQIs5K2y
9Fe7wd2TLGJqGAHW2mQD+LvdIOmyvfZjIMB2sTCXCDZ3mFDx81a8TADiU409
J864g+m8W0TQDAHGNjdNK73cYbaEePLiEgEKLNoozAHukDLz/oL/XwLsGSBn
Zl11hzLDmXw3DiKoscbv6s1wBw5fTudFWSKQbH8um71zh1MWEve2OROhNOAw
nixGBhvfR4Or9UT4kKVieU2SDMZOkueqm4nw+zWneoA0GWYHRaR9OohgKtDM
5ChHBt6YRmrbJyJ8fYxyJNTJ4ErVvSU6RwTuCbWh+xZk8FWx+MoijoEG767m
24fIECyqdElTGoPjOjNlkYfJ8MOn6rOzLAYPrhWFnjxKhi2B3dqx+zAwJBKl
lMiM+RmiaaeMMDjnLOBaHkgGnqSy6tlTGNy+umBy/xIZisLlTE+dxeB50XuV
2yFkECJcyuv2xmDbWuy6XwQZNtbnWMIvYpCVzJapm0CGAAkCRTsGg8ba0Yg9
SWSIzrJLRfEYTIzSPcVTyKBuZDz+TxIGWuoh+uvpZMhetPjBlI5BR8dyf10B
GUIes411PcTg19KHhidFZCjc7uPkWoKBmGRFcW4JGQyTmFk+PcbghMf5SxEV
ZMhMbR9Oq8JgY/sPMfNXZFCQb0iyaMQA2/eGWbeeDE/0O6zNmjCwtM+bUHxN
BuHUYQn1VgxS8tyfc7aRIWYnS1f7Owz2wifHdz1k+BjjFy34GQOmO6TCzU9k
SJ4z+pb/BYOPU/nL+wbIUJNioiE5iEFwqk9SwigZThpySr0axcBmpm+47jvD
f531xI8xhn9jkur8T4Ze9c93ro5j0DbL2W4zR4Z9doMFjZMYZJv4iIcvksHh
zz8mV6Yx8EnvO12+TAbVXX/CZWYxMJk3fDayRoZTYUmzeXMYiJrlb+NfZ/ib
HhHmXMBgOoPzqNEWGVJsVK4fWcSgbsH7vi8LDk7JQk3BvzBIMu+bv78Nh2N8
mW5RjD7xZJYh+sCOQwybQK/fMgZ6v/LiWLlwuDsrWX5gBQNuS84BjV04MK41
31kGD2d7K9H4cZiq/5pxaRWD/5Z6g5KFcJg+tb/kO4OjDho2vxbFwZduSVBd
w8AlJ09oWQKH2o6/AccYrLbCQZOTZtjTrRScGcxq5V1hT8RBXexksQGDe3N7
ma7L4WA0nxjwh7Fe8arBv1WKOLDv12BKZnCodV7WuDIOGcz05+wMPpLHMS2s
yogPqxVwZMQn/9tLz3w/Dh8vlgaHM/L5fbg3KlALh/qz0ngkI9/2fIO+Ql0c
dAyTlMkMPXL+3Jf7pI9DqvFFE0GGXn42HH7sCIcOUQ3+nHkMzAu8GnSNcJAv
ZvnNwtBbfL2H94wpDg467M4GMxjM2hq4p1ng8EFP7+6hKQwaCu+Xth7CoV/f
jUdtAoM7G+zrvw/jIBTDLDbB2G/Dop67TvY4+G0+Pdw7ggHvlv6PGEccCtiv
y3EMYTB29L5WrTMjnk3jn9wDGNxk8uqWoOBwx07TK6YHA/KxHhmrEzjs6dFq
Z+pmnO8Sfa/g0zjwZ1eamTHqtd+BnevreRxYam8X6zPqu6z0vBO3Lw7oXa/o
JOOfEM7a89DQHwfpZbMy2ksMFB/nmmZfZtTH4Ef92koM1tnYk9+F4uDy/nNe
ShkG753Oj26G4yBb2sL/TxEGAdv1w9yjcPhvRbS5LwuDgy65HQmxOHyt/Pdk
VyoGuyt2SNLjcdjMYaffSsTgtevHapkUHITHmHRcIzEQeHpucSQXh29jx+8K
Mu4TlTgr8YF8hp6W/50scWfU9wllo95CHCqrDunvdGT4E5pIbCtl6LkmPyRu
gcEnf5p65XMc/hKvfvWUw2DB2vh46QscBgdu1chJYsApTwwvrMPhVfCWcg4/
Bvq9Q50Zb3DgZffBP2wSIVvb2TuyC4efOs63xT8S4RmP3t3Qjzhk+ubcp7cQ
oXNclB7Uh4P48V+KMi+JwJzau+vcVxx2TuX07HhABNqq7WP7CRxqzr287+ZD
hJD3an3/TjPOkxzV9ymVCHcKd21ZzuHQRY0bemlPhGaHjsOkZRxiM7+fGdIl
glK1xaw8MwUa9fg9zBnvhfEtBWECGwVc+JJPcU8RwOX0dpLEDgpIuNxyCu4n
QJzo67hd3BRIsDwRa1NNgPkgtHdNlAKtQ5+0y70IwGErZb8oQQEu3d/C2Yx/
JXHPRvC0FAV2eQhRlCwJYPe5pn1YlgIhR+VUJAkEqPpH+2yrGgUoA2/toV0G
3vMJJTdqUODvj7rzbFUy8HPiV+1LbQpw+/z1cr0nA2Lp5TsrDCjQvaGe0eIt
A8F/VB6lW1Ag8+rzJ848MnCgFpv0JFNgsGpg2PqkFIj8e0XcgUqBHy8UpZGK
FMyMDhw0OkmBnHPxnzQWdkMa551HomcpkDjFzyURtBsWjrOfexPIiG+4/8a1
i5LQPEPLenKJAtVr3Qs6OpKQFV7fkRFCgYiisqAPvyTAsujSPt8Ihl4RQXPP
zkhA7tr0nFQCBW773avqNheHwJuWMpxJFJDN2IzwWBcDa5kCm+VkCog7N4W+
eywGv83dy9+mU4CYN/TfFL8Y2KZ2+QYVUCDOQqmEu00EmLWrlrteUuCEUpOs
65og9LXyy7+kU4BVLGZHT6oglLp6HXvYSIH7DloJvVqCcPya4rPQVgoMRPxR
pZ0TgPKP6UHKPRTgexWpKt/GB/iFsL+R0xQ4T5Q1W/bkAp0dA8recxQQUngx
lBi4E7gzdF2cFynA6XXrd24YJzxvWHihvkaBSB6H7PlIduDjp4UOslLhFemV
MheVDeqfWDDrSlDBYMxyduzNCjK5sPcuRYphD8a2m6gsoRYtftU4AhVaH0QZ
RUQtoM6aLy6jClTYCBz30DZh9Kevz1ff1KTCjzXRHsLLYvTnU7LXiDUV0l3Z
npcOrdaFZlzczmXL4IDimi3lv3XMbm5Z2kepIFxvOVAXuVnH/k3hbawTFe4K
ysqIlLHQRWZq5LVPUcElhWOs5AMHXZN55GvMFSrYzjloHH0qSK9ufOP3NIIK
YikCJ9XrhOj614t3Dl+nwodzu9m+tgvTjXb6/aMVRwUl72+CXb9E6bZCO1KG
0qhArcyfTvDZTT+/Z6+VZiUV5lpWxlkyMfriFN83tyoqtKTpa/gbydL9y1Yu
Rj+nwl8/NKk3JUsP1qAXDtZRYfb0x5uDxvL0GEM71uh2KuxJ4Tvqyr+HXmh7
sebrdyqIZu8gGSir0r3v9Cp1/6TCwqhJU+G0Kl33i0ZG0xQj3/wDMaaOavQ2
2uzlxwtUYNYNU5qSVqdPB1INwzeo8Kk5Lfnhq/30/dnWdFkhGuziW1I4ZqhN
/ztarCYmSoMR8f1fUiu16a8V2HO5JWhgLvlx6aiyDt2+vCF8RYYGEvZFrUek
delBr3WMW1RowNpKL/wspkd/NUlo8jShwe3BpXGiK4l+QzVMm2xOA9W7La/R
DIlu4zdQcPQgDfDOplAsDNFHNu7cMLShQeDFfZJKR4HOxsdlucuFBtevOLgG
Rh2gH9RZeVtxgQYc1whS09ImdIFgO4PCABocCqhZDwg0oQ/Qn5RkXKQBP9Gc
k7/ThH7uoGdcZBgNmlaFlyMjTelWlz4TbWNp8JamuML3x4z+PwOJekw=
       "]]},
     Annotation[#, "Charting`Private`Tag$157963#2"]& ], 
    TagBox[
     {RGBColor[0, 1, 0], AbsoluteThickness[1.6], Opacity[1.], 
      LineBox[CompressedData["
1:eJwVlGc4FYz/xmVlJSsys4WyReh8v9ax+6mQWVYeq3CKUmRnnByzROhIWrJT
QmYRTyRPkpEZRXZ25N//xX3db+5Xn+v63GKufifP0dLQ0Mz9zf93hc3WymxR
H0GP6+LF7Zxc7fiWM70nKC8hQCL74lyeBiG5P/KaCKUVtkUUw07m/UOYO1jI
kPD0I7x12FBamI8ipH9L76Cn9MLF/qslO9QMghb1+q2wgK9gYFt4U5r7EWHh
8HOF0KejINQTcrR6voLQzPokVSv7GzxPGvkU+LiecHsqZ3Ut8Ttk7D4810Rt
JXi1ptpXhk3DD28VSbnuLoJOQWwdKWAW7t1Vy53k6iXE6RI47ygvgHPTuQSG
F0OEgFLN5qCni5DINh9xdX6cYH9ANdBa4hcw1/UTU2ynCAaUwzJq2ctwbTsz
cvvRPEFhW6aPa98q+NTSFFRf/kXg8xUnLyauAX9RxsHT1DUCzYDQsS7GDSAf
OblUbLNFmDbhmy8O24S9HhmanR9p4L8qzrzE9d9A9q2Z2Wqlg1oZtlO+Adtw
ZbYg2ZJrNzy8zchgNv0H9E9n/VGvZIF3keED6co06B9vPcdfyQ461aFq9HM0
KGf3NFiNzAlli1cTLz7dhShFed06xw3SslcmxzxoMT6jfiIklheynAPhpAQd
2s6RaBJO88PeO6Q7jcN0qDZpyijlIgTRH/wWlbLpsTM4pC/q4QHYYDxvSrVl
QF37YPG5dDG4QPDO37uPEb+avdouC5KA00Xu1nOJu7GGfObfn7ky8P6bS7GT
KRNG9ZopZXyXBRQ6u7uDkRmtRJdE3lodAjmy3avCMBakFsSQ4ruUILfJhktQ
hxULYqlDqroqwL15yidhnRXJe2eTrFpUYcvzuLBXwB58tr/K9zCHBgRQzYK+
HGZHvf6+Lzs9mjDZa/zBaJodu7UZWUPLtcAzPw/TlDnQlKA+XlhGAHEQnW1P
4sAa4v3GGm+Ewf7cTNo5DtQhxsxxxOvCCa7spYCnnEjR8JOUmNEHtmKBe0+Y
uFD1UwvdeWVDaDHJNBv14MLgDPcZiCaCVsTtB5YS3BgvMmWedcoEloX2nYiL
4MY9l2kDirtMoaQqbbt+mBuNapJX3R3NQXIh2UYxmwePmmdiN/V/METeS/fP
Jg/+nBppZCmyhEwZSkmu7T78UNfElZByAtjPkpnY9/FirffggWLSKVjriKme
SeRDQ0HzNy6Zp8EdWDQ5l/nQ+whTuMNHW+gupVSq2+9Hb+OyxRFueyhOyyi9
Ls2PauWuRN1XjiDEIKSQf5MfMXjKIFDoDMQHUQtbl/hRp09Z6XvCWXC3e/KQ
o14AY8P4PAQNXaC7/bCkupQgylwsfflijyugTnmeHVkQ6U25l0wGXUHwQE32
/dNC2LG4d7WU7A7d396nqi0Io9x+Bf85dU9AmxMcdjYi2FQvbvlCyQuKW3sS
Q2tF8IlI0RUZFW+IfzoU1xJ3AN3cfATPmPiCqOYVeJYsihSrC9Tmc/7Q6691
va5ZFM16h5lpd/yB8mSrtmtVFGN54z1m7wbAlkCE1oqjGIYlsdCujZCgdzte
nSArjoF5gznMmYFAOWJ+ydJRHH1mnsWNWwaBgR97hWuSOMY9aDdtYrsM5SOp
SrEr4nhhW0yqOvkKUJrvync1SqD2/vBrb9uvgeGWk/fYsgTaKt4NWs8PgS01
0SfLMpJI9Q+tio0IBe+HD6T5KZLInJ6dP2kSBobxRWKu9lJo9euHtU9cBGw1
+jlfSpTCp2WlwL47Eso3le/daJDCVbugtyxxkSDq+0KoUFoaTdrDLaRTomDr
eD3f8pI09pObiq83xEAFz8c9N8gH8T79BKvvnQSoDRD8pl5zEAMjb3bvUSPD
m85z1RPTB9HYImWCsZsMn+M2PQxNZbEq2ek0x75EWN+SaKBnlsMdnjv0my+T
gDARRIq6IY+uLSwiwdWpYKTXaKz6Qh7fjTedZxJKA8t7rAfGJ+RR2fvRxsT1
NHCxo/6rZ3gIfUbl7dON0yG6o02Slv4w3k94o7D58xa0Vwr1hkcoIAutyVLr
pUzo5vqnSKlMAbVXJI5rz2TCgF9Z1MiIAjqMTWyInMuCGVmiEqIiGvWwVIDD
Xdib6xe/80cR5Yivn4jZ5YCc/qgw1CnhXoLGQG4nFYoDGJn5PivhTv6UsB1v
HqhS5ZfnZpWQxZTdbPBMHuhsB7bnCitjxJe1BN2lPLB4yXL5T4gycnw+kv1A
PB/85dW6XmurIJNmVG/F0wIY0jDaET6lgqm/rXrebxeAhYG9wnVvFUxsYa59
ceIhyDmF3yRkquA2WVZg19ZDmKC8N65fVcHfkoVjCfaPwX7JvbGhTBUPMYfM
GWEhvPtzeUG0TRWFktjmRqmFoMFKPhAxoooK+9lZHWmfAY9kWajuXjX0qSKf
XW59Bp3W20ebfNWQWTi05INTMei/ulXeLKOOG/+tjIT3l0L528ejEqCOxQLX
PzNylYFodw1HtI06KjUIm9OblsGf6dELBjF/98cPUv6pKYMqIQX5t2Pq6N8R
ozuYXw6HwlvyW3KO4OOKV4HfyM+B12gtvY1bE/XTF50zaqpg6Z3ZuuRhTdwv
60hHw/wKOkypDuFETfQU0ddgPP0Koo+biGsEa2La0hfK7PIrWLK+W/JgSBPl
P48kamjWQIc7tIc9OYqzfS6Bal9fQ3Rk7I46aGPMnvF7lt2N4Ew/6Jpiq42i
xvY/ztE1gfYNpZaZAG28xrtU0K3WBEvxfTfzH2gjKWPyZsWdJnBOkRfgZNHB
vQIvbbPcm0GH+kFt5pMOJpaFfFff8xZ+vebzvu9NwO8dgyfP57+D9RNKmeaR
BPwoc+3N+MA72JowfreaScD77Pv8i3jagJ79qrRZGwFdWk6jdmwb8J4ZHPsl
A1iSGmZO9G8HzT9UB8MJwKyF0DnDk+8BDtySXi5B1H7hxHlfvgv0vMQIbTWI
jW2D9LoWXWBQUWSd24rYIpRfwObXBcZGLdHGw4hxX8Us5Cq6wNJvbSybXRfl
+2ybI459BNd6u3uG53Uxg472dqV9N8ScFdmfIaeHRSuMqx9efgKC+79tXhp6
eNsqXTFs7BOsel65pmOghzTLSeoee3rAk9Q9NOqkh3RZ5TyDbj1gGnOj4FCK
Hj5LZxLy5v4M7IVzKk1renj8VvS0dGgv3Fmts5h9o4/42+vbwLV+sPzts1P/
UR+9V1KMqor6gZmGvyx1SB/zpL1qPwz3w1Xmizya6/p4wIaBUGowAE5CMgOR
8gYYx61hqcU5COJ6SZ77Uw1wgOAyGlv5FZ4lno3SP2uIMw7F/32+NQL2EXSn
+30M8bbryZ+M5SPAFPhILuCKIbrW0Y5bdY6Am+P8x9wUQ6TE0Web7h4FAfkw
0c1mQ9QPf2iVe3UU4t7lvi49SMSQte66eY8xcKcbWhNeIqLGj2L9MJtvIBjs
6LsebYxKev1M1mk/YChwrOBFsjGabYuXDD7/AVSS5/ClbGP0GWmzCP/8AyR9
L51crDBGiQ3nREGBKTh09qbm9JgxcjLov7l/fwoIhrX0g2iCt4cDfTaqpsGF
Uyinfsvkr/8WXxY2Z+DRk4GOG5fM0CSyWi57egFEXSLz9CLMMPWCyLUimkW4
s1828E+iGfZnX2Ts4l2EhNggoaBHZmhMZukz1l8E33OcPuf6zfBCJqmaOWcR
lMSMmAzQHNc69BrbTy1B9Z1yvV1sFsgi3uDh0PkLOmPjX17LP46ur4Ouqqyv
QkLPIJtUpyWW0G4x9eRuQ9fb7hAO/ZP4mD/S7S6ZFr+xjSiV9J5Cxhvik6pi
uzE2SCFP64Q1/pTLk/KdZMW1I+nWwdM2qMgiwKv+ngNZP/ca64TYYvFd7t7g
Pm4sznBc/7lkh18LxkPkpnlRpHT95/F4B9xzaUPA+rIACv/suZtL74RRjMDn
9lsYp0Pak/LunUGzUcGS5B1RLAo67pLO74wqvBSfJg4JPIxfbDt7nLFpxW7y
Py4p5K48vzSa54K3wr9OUq1kULdGYtrH2fUv8ebWighZbCw13qUp6IYN1qLc
k+Xy+OhEcPXXCTd8w4tH2SQUsCeq/ePGfXc8FuO221BbCb1dZMjzfufwRmxj
iWO0Mp5Q+OUmc9QDz1v+l36sQwXDbg5n9Sx74F3frUPZ9GrIc7v3olPDP+gr
d2izwV4dF5QWnjpc98Qs+gnZ4b8/KFJzeVe2phemDIenvvyqgRULLJuVtN7Y
3fGL75P2UUx6WWdJrPfGMlkX0z/RWtgte92klOyD/FVajioz2uh4+Aw12dQX
ifqFW3HHjqGmaBFvBcN5FFwY3+iMJ+C1ut2KJV3n0cLOX6/iFyDDXGSBGOUC
ykx5fflfPuLqO+a68w5+SM6a9b3qoIvZbTuboVz+SEpdr6ni0EOXNRZiuL8/
NrXeyuSv1sO+TUFXv8/+yF4neoqepI8rxGNFmeoBuBLze2pS2ACrWXiZJlID
8GAwBt9oMUCVB8uqwusBKMDnbJoYaojHb4xTkm1IqFjI23Hmr2dGphTzI7Yk
tH9CuWknT0RkP8oyaEdCnitDZlYKRFS+TYmRcSJh+pWNNhM1IvI8PBpS50ZC
2t/vmtWQiANvk7xm/Ekox6hayGJLRE8GHQNjMglnK0vUXsQS0aVtctfcTRLe
Aq+p0gQi2iem1KdRSHjpSE5OYSIRzfd91xpOIaGxrBd9XhoRFaVSlYPukPDD
I71/yfeIuGrwQ+RBAQk9NRO1XV4ScZ4pbdDkEQn113MnHaqJ+OP9saz5xyRU
6PiTbPOaiH1Wafu0n5HwTE/OuFkzEWvdCWzd5SRsStwTfuQDESsPTrVdfk5C
BgEDKeVuIhbPpMUKvyBhtWhFm3wPEamXpmi9XpEwdEaRQ2yAiJma6Q3sNSRs
ddQsFxwiYuoW4frzWhKu5Fw4xTtKxISGKW37OhLaMHf94vhGxKjo9I2dehI+
37BLY/1OxP8D4KHMdw==
       "]]},
     Annotation[#, "Charting`Private`Tag$157963#3"]& ], 
    TagBox[
     {RGBColor[0.5, 0, 0.5], AbsoluteThickness[1.6], Opacity[1.], 
      LineBox[CompressedData["
1:eJwV0/c/FYr/wHGJQpLMbNl7i6LzftsH5VLXzh5ZhWOkm5GRma1kpCMrRCEr
siorCZ+kIZkNyThZucb3fn94PV5/wfO4s+85N2oqKqrF//r/11lsr/2q+kDQ
ZQkI2LlboJHQbT9mltII5cL5AYuFaoS0j1HX+FN6IFdIPuJc4UXCokQlbWLF
MMh4/1FYXoomZM1mvaZJGQMxtmuP9sjZhFPk8FsR/p/hf1OVN8VYywjLsk/k
wiqmIO1V2MmnS3WE54fKM07lz0KL68zboAfthNs/7q5vJH+D+vsKi13kHoJn
T4ZNfcQ8pMSdEJEaGSJolsS1kfx/gYfK6YKvLGOEeC3C0TuKy/BvVHAibcME
wf+x+vPgihUgBuxG/rM0Q7ARUA4yF/4N1g1r+ulWPwi6KbLiKvmrsGvcE7VT
tkSQ2xH/wMK+DtMBoiVPr/wmcPoIJa0kbwDXhWEJS/IGgeoT7+mhA39A3KWC
Um2xTZg35FyqjtiCVJkP6oPDVPC/pqOFyZv/Qn8gz6/tnv3QKs543sd/BzT9
5NNNWQ5C6e0DtMbzu/DX/2z3VOsZoDfq+qcsRSosDXVa4qpnAs2nYSo0i1S4
rOb0j0rSUahZ+Sc5oGIfJofEtPUssoKYZMjXaXdq5HE6+C00jgNyHYPgnPB+
pNMWok605IIjd0h3Or/sx+CCUDpRJ16IeeO7opBPg6XUZuPRpQLw58AlI7IV
LTpcIYosZh2HywSvoiPsB1DWm4aqNlgYLKtczReTD2LHxObgzwJxGJh1qrYz
osOZ/ucq2d8kAXkdDr4+QI8u4wEiL/+WAakk6+bKCAaskykMThhSgIIuCxYe
zUPYYJQ7o6ylBKxb570TNw8hSWzh1t/dyrDtYcLn6X8Y56lNgmSZ1cCfbBz8
XpYJb51lmtkbVYevY8Q3BvNMGBLGzRlWewo8igoxU5EZvwot/a6sIYAQCP7q
T2XG/c+9X7V4IYx/LMihXmRGI8LSH+YELTBjyaf4VxzFQ4WDysILOsBYzX2v
nI4FTy/Es19S1INuwxzjKXcWvPX2PRXG6MOpyNvFpsKsyBE8cjH3vCGs8rKb
xUeyosvLztTqISN41JS50/6FFbdT87jcLpwBkeU0C/l8Njzc1H9phPwXTCQd
2X9xiw3P7QV8YqgyhRzxlEcFVuxY3FAsn5huBkwOSXRM7ByYMxmiW006Dxuv
bzxdSOZE1u/9O045luAKDOpHVzmxPaOmw3bYCkYep9Sr2hxD3zq9U1OsNlCd
mf04XIwLtyhmhVrNF4CXlleu6CYX9q35VATx2kNCMLmyh8KFnRznC78lOoCr
dXkpczs3Ml/dq+TRc4KRflkRVVEevK6vTtt42BlQs7bQOokHaRMWDYzGnYFH
oCX/viUvrjbO2NckucLI7ECGyjIfnr/6g35J1QPQwozZ2oIf7TVfbjYoeEJ1
z2hyWCs/dov6KkooeUFCxUR8d7wA0v7y2rQ39AFB9RB4mCaId9tImi/c/GDM
71R423NBLMXrddR7fpBSvt06tC6IPvHd/It5/rDNHXlq7cJxvI0vPm5MkmBs
J0GVICmEtVKh3Qw5QZBy4kyg6QUhVEwe6p01DQZdX6Y651QhnHU6UPyc8QrU
TmYoxK0J4ZxkcX1LWgikPM+THuoUxsoj2ek9/ddAb9vOa3pVGFXEIuq2ikJh
W0WwfFVcBPNr0/kTI8PAq7RYjCtFBCmWTS4/DCNAL6HquLONKBo6iR6/FB8J
252+joHJovjvSr0k88EoqN1SvBfbIYo58jRDjPFRIOjTwFspJob3susKJNKj
YduknXOVIobzAQylkR03oI5t+HBskgQ2qav1+d1JhFZ/nlnVFglsJt0YZlFJ
gheDbk/n5iVQvE1FknEkCd7Fb7nrGUni+eV3shzsybC5LdxBQy+Fe5JSUvua
UoEwF0yKjpVGkNxyCn+aAQbanUTlBmnsPXudcpg3E0zvHRKYmZPGgOWxzp/h
meBkTX6lrSeDzBHJNbnELIh53SdCTSOLVDGWvfsWbkF/Pe/Y9Ug5DF5paRgJ
zIERlotVCjVyeNKsJ0F/IQc++dZET07KochTrhopt1xYkNRXQJRH152Dvmds
8+BIgW/C3q481lqPlitY3wUpnSk+aFPAgy6BouWDZKj2P0DP+U4Bx1Lz3rhw
FIIyWXp18ZcCFsyVXfxmXwiaO0H9BXyK+Po7d/xZSiGcbWS4shuqiElKvPG1
QkXgJ60y9ExDCYsmn/h2V5TAhJrBHt95JYzsPcM+uVMCZ3Vt5MK9lHDRe+BB
v1kpSNldv0nIUcKgBSY/ju1SmEsZILavK6HVsZIzRTYPwIbi2tlRo4yug4Ol
F7ESenevLAv2KWNZaWE1dWElqB1KEoicVEYXLsVPYdQPgU2kJkzriAoqOli6
Het9CIPmOye7fFSQma0gYtOuGnSab9U+F1fFZZ+VudyPj6H25YMpYVBFYcFn
xcdZakBwpIU5xkIV2YR7vwsY1cDu/NRl3RuquHgnbSympQaaeOWkX06r4kKl
tPhOUS3IXO8u6r57ArM0c5oP33wCHAYbWX2s6tjaWPH9XUsTUHqNN0Vk1bHd
1dtOi74ZXhuRbf+zjex9fy4bWjZDjImhkNpVdSSpNRerrDUDxTzvUfGEOp4+
QEWJVW+B167QH1F+ElWDG1dvf34GMVFxe6qggRHJ9Iu5I53gSDPunG6lga9K
c9lr93eBRqxC94K/BrZKhrcKqnYBJeHDzaJiDaTs/X2LNqcLHNOluY8yaKJK
jmzPqutz0CS/UVl4q4nRze/Niw6/hN/POL3uexFQJ26L7lBxL2yaKeSciSLg
2s1f3THjvbA9R+xdzyHgb7/212bsfUDD9I+YcR8BJ1PWI7/G9QGH/fj0b3FA
L3NlFir/flDfJdvqzQHenvv8ReD8AIDALbHVR4jpbGSrEzJDoO15nNDXgjhr
p8Pz/uwQ6NZVmRf0IGZlF90u9R0CokF3DPEL4jlPE47+uiEw9d2YzmfSQi7b
tQFZwjA4t1vf07ukhT+NBqJDbUfghgP/sWwpbRzXY3cba3oLBNdXfZ5q2hik
YpiaNPMW1j1CrmnqamPIvjc5V5hGwYM0MjFlp41C1rVtG66jYHQjtkQmXRtf
SV00zmN7B0yVi0pdG9oY+uiqQVz4GNxZbzv764UOBqiiSFXYRzD913uvfVgH
1bz2QtMffQR6Kq6ajAkdpO5Kp6mZ+gj/0AewqW/qoEiXK819/U9gxyv+KUpa
F53pIyJMWMdBSDvV41iGLro3xE1/bfwMD5MdonUc9PBihSDJPnsSbCL3W370
1sO/qkwzs+omgS6oTMo/RA/7ie4Pvr+ZBJcLS8MF6Xpogsnv5+mmgFs6QnDr
uR4upxUGW4VOQXxvwbPHEvpo6hDaOOUxDa77Jzb4KPpINssspVjNAs/VCz6b
MUS0mVtcE8j+DhNB0yUNaUR0n6Bk1TV9BzLJ40tgPhEvKWQYu3z8DiI+gedW
6oj4YfUNFyf/D5BxuKk+P03Ey9Gfl4ZKfwBBr5VmHA3xT70GR+azeXA6ynu3
fdsQZWg5nEOpfkFZ+afXsYHGWKL3Oj99cRkEnaIKtSONUeqx8btqmhW4c0wy
aDfZGOMHuD0+c69AYlwwb3CZMar1FJIvG6yAj9tRb7ePxnjk0VajU+EKKBw3
oNPFMxjs8YYm2YoCT+/Uau9jPItjT35rHHr7GwbjEhqvFZng49ZWc3mqDUgc
HWcUHTTFjGq+F/xVOzD0ciSUWeccKujvM43PpsZZxkmFR2Pn8c+0XdKMykGM
C5YrPGVmjuZh60fDaRhx40SW+dV5C7xDVZdEP8OMh96NETVDrVAiL9qxeIsV
q7MvbP6kWONybOTZEU5O5H+8+dMkwRa5y6Y7hRu4ke/naF4BjR2m0zQI05vw
43xof2rhPXtMehlI2lA9jlXBJk5ZXI7Y5WjYlGkhjLL43mpw1BHLmg+1RnqK
Imv9JcpUoRM+7MoYDOoQR60W4XlvR2dskx6r4KGRws7HxH3qPC5YFcHQJWsi
g2VmV59+nnPBMpbIyOBxORyN7h/+c98Vd2Rs0hLLFNDLSTxpydcN5Y6oZ4vv
V0Izud8u4ifd8cT9N7kzDsoYcfNL7uiqO/IPnHTXqVRBtttjAXYdF/FFXTOh
7tgJXFZYrrAN90AJSt4Z+gA15G+5si9f3RMpr17J7ParY90yw1Y9tRfyGpms
t+qewtTGNlP9di8UjL0yQluugSOS4YaPk7xR/fR090H503hB1p6cZuSDIcTG
FPcCAqoLVnHU0V5Cs1yHCjIN4rW2g/KPhi6h29Ur3i/6EWkXo0qOp1zGrBrh
0eEYLVzvpW+7ZOuL/teyGmP/0sb8vr2tMBY/TC2nsY/i1EGnDQb9635+uJal
dXpkRAc/bPE4+77zwxOv7q+VFOjimv7pqhxVf4y/uiQQb6eHTxk46OYy/LGV
OotRhEsflYpXlfk2/fGsjDu96Jw+msTOpKRZkDBk4HrNRJEBGhilnDlhRUIP
z78PKJcZIDKdZBi3JuGUzLpjXIUBKt5OuSFuR0Lq4TRxhRoDZCs9GdrmQkIf
ct6fyDYD/PQy1XPBj4TvLr97KPbBAD1oNXWJSSRkDemQC2QiolPf132LN0lo
SxRU6Tv6n9vk9PbMFBL+ZdRI4Gcn4hn2b6e+pJNQNzbEpZeHiPKiGYrBd0io
1NYzzytJxHXd7/zFJSTsdClY6NYh4hJd5rhhGQk/WJjo8BoQ8fvA6dylByTU
m1ko8Df6z/nfmewaD0n4cmbGldeMiK2uBMaRWhL+fqgpTbInYr3Ej74rT0ho
GDf7oMeJiNULmXF8DSSMcbaU5nMjIjnwB7VnMwlvk24Ser2JmKOe1cHUQsKw
Mb03fL5EzNgmhD9pJaHn3SbXABIREzt+aNi0kfBfx8nd3iAiRsdk/dlrJ2Fp
R9Nd/qtE/D/Zuta7
       "]]},
     Annotation[#, "Charting`Private`Tag$157963#4"]& ], 
    TagBox[
     {GrayLevel[1], AbsoluteThickness[1.6], Opacity[1.], 
      LineBox[CompressedData["
1:eJwVluc/Foofhs3IypbsvTdl9Xy/9mNGHZEVoYQOHiOVEcnMY6SQHamIjEgU
yclKDk5SSHZWVkIO+Z3fi/tzvbiuP+AWOed30pOKgoJi+b/9n7Wnd39+r/hM
0GcPDNzLy9dJaHcZsiE/hydiuYHLRccIqcPR1wTJHZAtqhR5sugCYVm6nDax
rB8UfX4pr67cIGRMZ7ynIQ+BDOe1p/uFmQTtwog7kQFfYHCi/JYkx0PCqsIz
xfCyCUh7F67VuFJLaGN8nK6dOw0vPaY+BD9qIdydz9vcSv4Gz+8rL78p7CBc
7Eh3qItcgOS4o+KyA30E3QdxzaSA7+Clfjx/ln2IEK9HYMtSWYW96JBE2vox
QkCVZltI2RqYBP6OuroyRXAQUgu2FfsBjvU/jdPs5wmGZAUp9dwNoLDoiN57
uEJQ3JP6zM61CZOBEg8aL/8g8PiKJq0lbwG/U7+0XeEWgWKE/3jfgV8g6V62
Xnl6l7BgyrNSGbkDZPnPmr39FPBPA1tR8va/0B3E9323gxpeSjGd8g3Yg+P+
SmnW7HRQevcArfnCb7D+x3Ffo44BOqOvj2SoUODDMLcV3joW0G0MV6dZpsCV
Y25X1ZPYoHrtanJgGSWmhsY0dyxzgKRM6OzkeSrkd6P7FhbHDfdcg+GkGDUy
6ItSJdrxwqEsUlbrV2oMyQ+jl3Djh5i//daUc2mwlMpm9EapEPw6cMms0J4W
XS8TxZczROBPgnfxIa4DqOhDQ1ETIgZ2FR62y8l02Da23buYLwU9026Vzmb0
ON3dpp75TQaQ/yzd+wMH8fxooPjbP+RBNunMi/JIBqyXLwpJ6FOG/Den2fl0
GfGF2b0pNT1V4Ng55ZO4zYjBkkt3/mhXg10vK4GLAcy4RGUVrMB6DAIKzUM+
KbBgriXL1P6gJswOEf82WWDB6PAjPOE12uBVXIS3VVjxp+jKj/JqAoiC8Pfu
FFZkbPN51+SNMDqcn021zIrWhJVfrAl6YMOeux5Qxoa8Rb1qYksGwFR5pOAx
PTtaLsVzXVIxgnbTbPOJ8+xY/uETBcYYg3bU3RJrMQ7UChm4cO+UKWzwc9nE
R3Fg+tvWlMo+M3jacHuv5SsHqqXm8Ho6WYD4aupppVxOdGrovjRQeALGkg5R
X9jhxJj9wBGGCmvIliI/zbfnwrH6EqXENBtgOZtEz8LFjWvjoYaVpFOw9f5m
41IyDzbPde+5ZduBBzBosm3wYPrt6teO/fYwUEWu03A4jL7PjLQnOByg8nZm
VYQkL7ps2BTpvXACflp+xeJbvBi05VsWzO8CCSGF5R3rvNhw+FTRt8Sz4HHm
cSlryxEMuLpfzmfkBgPdCuIaEnwoQNSkfc58DlC3puhMEh9+T1w2MRs9B3xC
Tbn37fgxpXHKpTrJAwame9LVVwWQLWL+4IqGF+BpG9YzpwXxi97b7Xrli1DZ
MZgc/lIQ+eT9VKRVvSGhbCy+PV4IfX96b7uY+oKwZig8SRXGgbck3b88/WHI
XzuiuU0YvxKv11Lt+wP58e7Lvk1h7ElrF1zOCYDdI1HaP51E8KnFX8Nb4yQY
2kvQIMiIYgQhrJ0hOxjIRy2CrJ1EMbq4r3PaOgQM/Vhqz6WIIu21AyVtTJeh
ZjxdOe6nKN43LalrSg0FcluOXF+rGKbqZaZ1dF8Do11n78kNMZxwjqzdKQ6D
XXXhxxtS4tiwmiaYGBUO3qUlkrxkcdwoaXCfN40Eo4QKkXMOEtiSIyFyKT4K
dlv9XIOSJbBBtV6GlS4aanZUCmJfS+DRyzR9TPHRIOxbz18uKYl0K7X50mk3
YNeqhWdjXRJfbjCURr2+CbWc/cyxSdLYa6TZ5Z+VCC8D+KY1mqSRNTO2n109
Cf7q9WycWZDGmH81ZJgGkuBj/M55IzMZrPb8pMDNlQzbu2KvaQ7KooCcvCxl
QwoQZkJIN2LlkIJy1y2iMR1M9FuJavVyWGEavc7MfxusCxiFpmbk8Cf7cOti
xG1wO1P4Tt9IHhc3U6rvETMg5n2XOBWNAna/c+ikXLoD3XX8Q9ejFPFEXmv9
QFA2DLBfqFCuVsQl1/cJxkvZMOJXfWN8XBFn1YSrZT3vwZKMsTKiEmqdPeRn
4ZgDh/L9EvZ/K6Hi7Nhj5TN5IGswIQDNykihGybxuLcQKgMOHOT5qIxKs8V/
u3MXgVqh3Mbyd2V0e1114ZtLEejuBXfnC6jg3qR4vOV6EVg+Z7j8O0wFp/qk
42tEi8FfTr3vlY4q6rR1+rWXPYCxYyb7AqdUcaTDjWt87wFYGjooRnir4sW7
k4+6bUpB1vn6LUK2Kn69J+XPvVsKM+QeYsumKmpkt1kUOzwCh3WP1tfVanhg
cLf0ApZD5+/Lq8JdaujBPFBJVVQOxxiThKLG1fDmrvtIONUT4BSvDtc7pI7N
GSmehzufQK/tntYbX3UsDp2M3HauBIMXd2rapDQw6abY7L3hKqh5+2hCDDTw
a/5aiQh7NQgPNLHGnNbAQNH9OSGzavi9MPGn4U0N1P3eMxTTVA0N/Ipybyc1
MIgnSGqvuAbkr7cXt+cdxan7FI3Mt54Bt8lWRheHJhZcDJn/2NQA653m2+IK
mqhjhy56B1/Ae7NCx+vGmsjh/MnP1O4FxFiZih67oonO8OSB+s8XsG6b87Rk
TBMfion8iNVsgvce0B35WAtXFC037355BTHRcfsaoIOMNbdW7g20givN6Lk0
ex2s0VLgqaF+Azqxyu1LATpY2yDcLKzxBtYTPt8qLtFBA33eTNrsN+CaJneE
jUEXC+t0uzY82kC38G/1pQ+6+Ga/wL6Y+S38eMXjfd+bgMS8eWbGkk7YtlHO
togmoI37gZ6Y0U7YnSF2bmb/542o/7Hh6gIalquS5l0EzNHKiJuN6wJul9HJ
H1KAlcx3DlMEdIPm70JHoxlAYgHbnNCpHgChO5IbTxHtgkzOHpXvA/2LIoSu
JsQjDQKinyz7wLC2wja/A3HGrCav1K8PiCbtMcSviFZM3QLdtX1g7bc1mcui
h5UdToMKhH4413KmwOiSHkqoOpLDHAfg5lnBw5my+mh8LTJ4qOEDEDzedV08
po+PppQKk6Y+wKZX6DVdQ310DNUov8wyCF6kgbEJZ31cyBLt3/IYBLObsQ/k
0/TxvSS3aw7nR2ApX1Z9s6WPAo7n3eIihiBrs9ny+18G2JjiYlERPgzW//rs
t/QboJy8Wmna02E4SMFbnT5mgAkFE4rVE8Nw9WAgp+a2AYrepFS5bzwCzvxS
I9FyhpgcylRtxTEKovopXofTDTEpM1jo2/Mv8CT57A2Ds0a4QZld4JI5Dg5R
1HbDPkZIVptuzagdB/rgh7IBoUaoL873ae7vcXB3WunPTzNCx5pMhkX6CTgi
Fym802aEVSalFfZhExDfmf+qStoY57/1/prwmgQP6rEtgXVjJDsv0v6wnwa+
K06+2zFENIw1qRXOnIOx4MkH9alE3Oj5ZfusYQ4KSV5fg3KJSFdnx+oxPAfi
vkEn12qJmHfVcJZHcB7kz97SXJgkopZfRE9/6TwQjF7SjKIp0qqXcWe8WgA3
Nv68ll1T5NnbeRFO8R0ePh55HxtkjsBf05W+vArCbtFF+lHmOJXURl9FswZZ
h2WCfyebI/Wh44VjR9YgMS6EP+ShOSpZu077mayBryebj+ewOWYq8HK6F62B
sogJvSFaoC91zl2y/To0ZtXoUzJZ4khozAnmDz+gNy7h+bViK/wypj2uSrEF
iYOjTBK91pjKrJAlVbEHfW8HwlgNTmJb9hWl9EwqnGYaV346dAqzOagJv9Tp
MC5EsUjbxhaNviyaPKJhwq2jGbZXFk7j8TRmLdWp/37NxyGibpg9bghMR3/f
4cDKTKftxfUzuH2dUcj8MA8KVm0vWiU44vXmLLHF+iMosDiYk0/jjNYn1v7V
OSGIC2HdKUUFLtj2vqZm6qgIVoRYuWXwuuKuffHxNTsxVMBP9r2DrpitPZvs
6yOBHHWX1ieK3LBUWE9Bpk0K9ZrEFnxcz6H0Xr1MC50stlYRKTX53JFOkhCx
eVIeH9pcafwy444GJXb5HZOKOHiju//XfQ9k2c0jp5Uro7ebVNKKnyf6iRZm
naBXRRvFH+5SWufRcGWmx+m8Gkbe+npvcOM8GnvZssnVqiPn3aFA59cXkMB7
0tlT9CiuKq+WOUZ4odejabeSiGMo2HSZMlfzIpYJNC0++6SJtasMO3VU3rjK
6EpBY6uNKc+brY1bvNFrVU9ws0kHB2QiTKuSfPBjgYeqtNFxdFJwKUw188W8
0xMd754TUFO4gruW9hI2jQkqsnEgXmumU3radwm/0r0R0BtBpF2OfiBC/hPz
7fz4XTL1cLPzYPMlRz+0oFiuCfXQx9yu/Z1wdn/0VZc59UvRAN22GIyv+/uj
ecNGdueSAX7e4Tvn99EfF9peBV1tMsSfxscrsjUCkCzjMKsUboSNDNz0M+kB
+MH//EStjjGqlmyoCWwH4GfPqUIqRhO0ip0ip54mYa3N0vRGjwmamJEtjtqT
8NKY/pxdnwkiixbD6BkS5rtRbjT+Y4Iqd8k3pZxJuPC5SDxq2AQ5S7XCmt1J
+OfkxDzznAmOvE25uORPwizGlX1paiJ60eoaEpNIyMknecxTi4huXbOUy7dI
KCPUcLxLl4gOyWktt8kk7BFlt1BAIlpwfdP+mkZCmlKG6z+Niagkka4SkkXC
9T9vGsb+QcRNwznBkgckHL1zXuexHxFX6G+Pmj4koQ612kvmQCLO9Ry/t/KI
hLHHrhqSQoj4+Y/bXDpPSPhsxtNHJ5yILz0ITAM1JPQ9qcDem0jEOun5rsvP
/uunzXpVyUSsXLodJ1BPwruWr9Iy04hYGDRPdfEFCW17kxXdsoiYrZnxmqWJ
hDaRk3TtOURM3yVEPHtJwk9aV+ZkC4iY+Hpex6GZhNtWln0p94l4Iybj134L
CaPYHFo2HhDxf2ta0ic=
       "]]},
     Annotation[#, "Charting`Private`Tag$157963#5"]& ]}, {}, {}},
  AspectRatio->NCache[GoldenRatio^(-1), 0.6180339887498948],
  Axes->{True, True},
  AxesLabel->{None, None},
  AxesOrigin->{0, 0},
  BaseStyle->{FontFamily -> "Arial"},
  DisplayFunction->Identity,
  Frame->{{False, False}, {False, False}},
  FrameLabel->{{None, None}, {None, None}},
  FrameTicks->{{Automatic, 
     Charting`ScaledFrameTicks[{Identity, Identity}]}, {Automatic, 
     Charting`ScaledFrameTicks[{Identity, Identity}]}},
  GridLines->{None, None},
  GridLinesStyle->Directive[
    GrayLevel[0.5, 0.4]],
  ImagePadding->All,
  ImageSize->{1139., Automatic},
  Method->{
   "DefaultBoundaryStyle" -> Automatic, "DefaultMeshStyle" -> 
    AbsolutePointSize[6], "ScalingFunctions" -> None, 
    "CoordinatesToolOptions" -> {"DisplayFunction" -> ({
        (Identity[#]& )[
         Part[#, 1]], 
        (Identity[#]& )[
         Part[#, 2]]}& ), "CopiedValueFunction" -> ({
        (Identity[#]& )[
         Part[#, 1]], 
        (Identity[#]& )[
         Part[#, 2]]}& )}},
  PlotRange->{{0, 300}, {-45.95367314312315, 49.29653159997816}},
  PlotRangeClipping->True,
  PlotRangePadding->{{
     Scaled[0.02], 
     Scaled[0.02]}, {
     Scaled[0.05], 
     Scaled[0.05]}},
  Ticks->{Automatic, Automatic}]], "Output",
 CellChangeTimes->{
  3.725790454653599*^9, 3.725790514460441*^9, 3.725790551700067*^9, 
   3.725790631266589*^9, 3.7403738145650263`*^9, 3.741166057760421*^9, 
   3.7411663256639023`*^9, 3.741166397999399*^9, 3.741318749767981*^9, {
   3.741320125263187*^9, 3.7413201485063477`*^9}, {3.741320987899673*^9, 
   3.74132099480273*^9}, 3.741336042699746*^9},
 ExpressionUUID -> "bd5628bf-a9bd-448a-a0ca-2f1f9b60ea52"]
}, Open  ]]
}, Closed]],

Cell[CellGroupData[{

Cell["Short-range Breit exchange energy per particle", "Subsubsection",
 CellChangeTimes->{{3.741166418018155*^9, 3.7411664232849703`*^9}, {
  3.7413205340984497`*^9, 3.7413205348182173`*^9}, {3.74133602876886*^9, 
  3.741336030013644*^9}},
 ExpressionUUID -> "06b94b3d-8b93-4c7d-959f-b1d15e5c7b43"],

Cell[BoxData[
 RowBox[{
  RowBox[{"ExRBsrPad\[EAcute]2", "=", 
   RowBox[{"ExRBsrPad\[EAcute]", "[", "2", "]"}]}], ";"}]], "Input",
 CellChangeTimes->{{3.722676673170491*^9, 3.7226766840788517`*^9}, {
   3.7226769607964897`*^9, 3.722676964008954*^9}, {3.722677058507019*^9, 
   3.72267715175624*^9}, 3.722750488409705*^9, 3.722750909349684*^9, 
   3.722751650069563*^9, {3.722751697031013*^9, 3.722751701925248*^9}, 
   3.722751733156549*^9, {3.722751776660254*^9, 3.722751780232744*^9}, {
   3.722752400242813*^9, 3.722752400432448*^9}, {3.722752467679291*^9, 
   3.72275252014501*^9}, {3.722752952275763*^9, 3.722752969101005*^9}, {
   3.72275303435499*^9, 3.7227530345334883`*^9}, {3.722754156545463*^9, 
   3.722754156795789*^9}, {3.722754188112558*^9, 3.722754208304021*^9}, 
   3.72275432057234*^9, {3.722754402080971*^9, 3.722754454383902*^9}, 
   3.7227544955051527`*^9, {3.722755499949471*^9, 3.722755529084709*^9}, {
   3.722755602590743*^9, 3.72275561222154*^9}, {3.722755806077857*^9, 
   3.722755808828918*^9}, {3.7227562912298307`*^9, 3.7227563187455587`*^9}, {
   3.722756509642661*^9, 3.722756533689232*^9}, {3.722756667772307*^9, 
   3.722756667930399*^9}, 3.722763826327332*^9, {3.7227640337205467`*^9, 
   3.722764094101956*^9}, {3.722764391670136*^9, 3.7227644061291647`*^9}, {
   3.722765493776552*^9, 3.722765494139145*^9}, 3.7227690116290216`*^9, {
   3.724470727309154*^9, 3.724470739564727*^9}, {3.724470771805664*^9, 
   3.724470785724593*^9}, {3.726898654440785*^9, 3.726898654805393*^9}, {
   3.740374409484497*^9, 3.7403744097069387`*^9}, 3.7403846191115026`*^9, {
   3.741164665136079*^9, 3.741164665361087*^9}, {3.741165865704812*^9, 
   3.74116586682211*^9}, {3.741166428171543*^9, 3.741166438232815*^9}, {
   3.741166673009337*^9, 3.741166673879197*^9}, {3.741320180328374*^9, 
   3.7413202006602716`*^9}, {3.741321040883649*^9, 3.741321042821103*^9}},
 ExpressionUUID -> "c6526e78-0a5f-4e7c-8651-dcd29ab5724e"],

Cell[BoxData[
 RowBox[{
  RowBox[{"ExRBsrPad\[EAcute]4", "=", 
   RowBox[{"ExRBsrPad\[EAcute]", "[", "4", "]"}]}], ";"}]], "Input",
 CellChangeTimes->{{3.74116594537556*^9, 3.7411659505081453`*^9}, {
  3.7411664420165*^9, 3.741166448399979*^9}, {3.741166669555909*^9, 
  3.7411666717409487`*^9}, {3.7413201851879263`*^9, 3.7413202036193867`*^9}, {
  3.741321047269231*^9, 3.741321049270521*^9}},
 ExpressionUUID -> "a4623d24-a591-4d29-b3b1-b2f3992c3e1b"],

Cell[BoxData[
 RowBox[{
  RowBox[{"ExRBsrPad\[EAcute]6", "=", 
   RowBox[{"ExRBsrPad\[EAcute]", "[", "6", "]"}]}], ";"}]], "Input",
 CellChangeTimes->{{3.741165952141227*^9, 3.741165955289587*^9}, {
  3.7411664557837667`*^9, 3.741166458935994*^9}, {3.7411666649928627`*^9, 
  3.741166668197682*^9}, {3.74132018654982*^9, 3.741320205987595*^9}, {
  3.741320411380327*^9, 3.741320433555772*^9}, {3.741321050932055*^9, 
  3.741321065013235*^9}, {3.741321101059639*^9, 3.741321101716072*^9}},
 ExpressionUUID -> "a141c3e4-4728-478e-be6f-236b474eb28b"],

Cell[CellGroupData[{

Cell[BoxData[
 RowBox[{"Plot", "[", 
  RowBox[{
   RowBox[{"{", 
    RowBox[{
     RowBox[{
      RowBox[{"ExRBsr", "[", 
       RowBox[{"\[Mu]", ",", "c"}], "]"}], "/.", 
      RowBox[{"{", 
       RowBox[{
        RowBox[{"c", "\[Rule]", 
         RowBox[{"137.036", "/", "kF"}]}], ",", 
        RowBox[{"\[Mu]", "\[Rule]", "0.6"}]}], "}"}]}], ",", 
     RowBox[{"ExRBsrOrder20", "/.", 
      RowBox[{"{", 
       RowBox[{
        RowBox[{"c", "\[Rule]", 
         RowBox[{"137.036", "/", "kF"}]}], ",", 
        RowBox[{"\[Mu]", "\[Rule]", "0.6"}]}], "}"}]}], ",", 
     RowBox[{"ExRBsrPad\[EAcute]2", "/.", 
      RowBox[{"{", 
       RowBox[{
        RowBox[{"c", "\[Rule]", 
         RowBox[{"137.036", "/", "kF"}]}], ",", 
        RowBox[{"\[Mu]", "\[Rule]", "0.6"}]}], "}"}]}], ",", 
     RowBox[{"ExRBsrPad\[EAcute]4", "/.", 
      RowBox[{"{", 
       RowBox[{
        RowBox[{"c", "\[Rule]", 
         RowBox[{"137.036", "/", "kF"}]}], ",", 
        RowBox[{"\[Mu]", "\[Rule]", "0.6"}]}], "}"}]}], ",", 
     RowBox[{"ExRBsrPad\[EAcute]6", "/.", 
      RowBox[{"{", 
       RowBox[{
        RowBox[{"c", "\[Rule]", 
         RowBox[{"137.036", "/", "kF"}]}], ",", 
        RowBox[{"\[Mu]", "\[Rule]", "0.6"}]}], "}"}]}]}], "}"}], ",", 
   RowBox[{"{", 
    RowBox[{"kF", ",", "0", ",", "300"}], "}"}], ",", 
   RowBox[{"PlotStyle", "\[Rule]", 
    RowBox[{"{", 
     RowBox[{"Blue", ",", "Red", ",", "Green", ",", "Purple", ",", "White"}], 
     "}"}]}]}], "]"}]], "Input",
 CellChangeTimes->{{3.725790426404578*^9, 3.725790453840857*^9}, {
  3.725790502785564*^9, 3.725790550992629*^9}, {3.726898837998486*^9, 
  3.726898847052638*^9}, {3.741165900638431*^9, 3.7411659400545387`*^9}, {
  3.741166056629149*^9, 3.741166057200569*^9}, {3.741166464014175*^9, 
  3.7411666068642197`*^9}, {3.741166645830902*^9, 3.741166658462842*^9}, {
  3.74132019589301*^9, 3.7413202316535683`*^9}, {3.741320284775901*^9, 
  3.741320289842805*^9}, {3.7413210566159077`*^9, 3.741321074166067*^9}, {
  3.741321109589614*^9, 3.741321122471397*^9}},
 ExpressionUUID -> "a01f6b7c-131d-44f0-8794-c7f96654fc25"],

Cell[BoxData[
 GraphicsBox[{{{}, {}, 
    TagBox[
     {RGBColor[0, 0, 1], AbsoluteThickness[1.6], Opacity[1.], 
      LineBox[CompressedData["
1:eJwVVnc414v/NYuS7JE9PvYeJfR+vbJFLmkR2TPC50ZDmR9ZGSEh8ZF1ZWZE
uD7oZhXhmyRCLt0ISUIlfv3+OM95znPOc57z55FwDTjhwUBHR7f8G//Pdae3
vi1VjhF3PgWesF8O1YvvOj9qk9wI20zpz7pieInUt1GhosndsO6R0KgTY0ws
y5UzJzwcAu/phWBCzpXImM3oZ0oehX7cpbVECSZ0qWF3woPeAVdPsVQbYwyx
olyvcuPhezARICT2yaURT/eWpenmzkLk0D9hk69yicz5++sbSf9B//DuGw2U
YsKnO82+IXwBjm4P3XAvrCL0i2PbyEFL4GzreTKasYGIO0pwZqmvQFoxN41r
s4UIqtF5GvLwCxy84u40LNtJ2ItpBp+S+gqNhTLRBG83YZSsLKuVuwan3xmc
CXj1glD5JTvGxbsOHxR89jxtHiL4/SQTvyRtgHJBZr8NZYSgGxc+MrjrO+TU
dWitDYwRC+b8n6vCf4AAn65l84NJ4n9NnAVJmz8hQHphbYxxhmiVZbP1C/oF
+lzjJzcZ5oiSzF3MFgvb8OL77W+0Ex+JnqiI8Qx1OrTqLPHU2fhE6Dff0GJa
psOSR/v4fNY+E4++XEv68yE9+ppAqZLsKiEjf+XDjCcDRt9dOhBHWSNynIPh
hBQjrng89zjGs0HszyJndUwxYm968teQN98JysuAL2q5TCjwS1iI839bxPdd
/seoZ5mxnnuanZ2RDi4SvoX7eXdhQ5pSev8TejhT6X5qOWk3Pl5jb6eLZoYX
sy5VjsdYsCZ04czlu7sBhZ129+9iRX3XiEHlflZQSLR7Uh6+B1nPsNY7Udkh
r/M0l5D+XpzdPDu8nM8B3D9sLyRs7sUZK3u0ZuCCLW8rEZ+gfZhcp1i3RccL
QVSLkDfK7FhzvZZmlscHH0bNXpousKOk0rL1YWsB8C4swHR1DuTgNm9iXRMC
SRBf6kvhQEfNBycXPojAxNu8bIZlDvww0EYftCIGNly5q0EPOXHfevlEk7Qk
sFUdyC9j4UI7C1GJdUsp6DLPtnjvyYXTP2UXb0ZKg25kZpG1FDeijatTIYcs
rAnz2sRFcuPHqgax6gtyUN2U/os2xY1mgXWZ7K/kQXol9bRqLg9Kqt3N7+lX
gsnE/YxeP3jwjZG3WKGTCmTLJlfnneVFj5pY9aEdVWB3SmRh5+XDyDq/Ee7H
6rDRH9O8mMSPcwOa2xM3tMEd9uhwrvEjf9UQfM8+CMM1yQ3a9gKY77P0s5p2
CKrS79aEyQjiPdacIylyuiDMLKxSeEsQt+zaZ1n89CA+hFrevSqIsxK+5rQn
+uBuV1bCQTuAr8Kr7SmXAIb7lKW1SUIYZ3iRfjUQAfVrC+wShXDd/5kqp/JR
EBJryX1wRhjHzh8PXW4wgOHZF2laKyJYXqTlaM9mAnjahsPutCj2uMsUNa+Y
QFX3SNKNVlG8up+1Q3HcFOIfTsZ1xYlhbcSdXbc7zUFc5wpUpIojA4vmXM67
4zAaqBvW9lQcc2JvcDesWUFy2Vbr4Lo4qraMBiCrNWwdiNT95iCBfAK6bYS6
DYz+itcm5CVRujOMKlJuC8kHLS9ZO0jiPHt9SPyJk2AUwF7nmiKJn75MCuf9
Ogm102lqsd8kMVwMmufPn4bkp/cUBzuk8FnEGJ3EH3ZgvOXoO7MmhXXVwgoL
PPawpSVetiYrjZou55rKJ+3Bt6RIRjBZGv/Rt66AMAcwjq+UcLUnIQ8vhdS+
7ARbHQHOl5JImM/oOF7j6wy1P9Tzb7aT0DYt1pM07Qzifo+Fy2VkkMXb5FrS
kAtsWdH411Zl0C0+68y/A25QxzO072aiHN5jMEhaOeQNrUFCs9otcjg7UHSk
9Jk3/DPg0Ty3IIfhRlmJ4ad84HXcD0/jY/Jo+PHISFGoL2xuSbUzsSogd2Bz
p9qMHxBzIeTom4ooMWYgNr0vCEwNOsw0Hyvi9TT1zXrPILDO3yv275wivuWd
5GtuDwIXO+pzA2MlbP2p/dXhChko/b3SDEzK+F9mUaXe+p/Q1yA8GhGpgl7N
Ye37VS7DMJdXpdojFVRvauQazrkM4wGPoqenVZDV2a7sX5YrsChvooaoinNd
6zZbH6/A/ryA+J1tVVS2dzx4+Mk1UDB8LwJtasi/vf33rXthUBW0i5X/tRoS
HRGlcqLhoElVXFteUsMohwvWGg/CQf9XcF+eiDo+L+I7aHEmAo437rm8fV0d
BxpniAt+kRCoqDX4t54GXnoTNenXHA2Th0x3RGw18JRz3jfuXRQ4bmSvEuar
gaVhj1WunqCAgmPELSJbA8P/SIiOXKLAXPILM9q6Bto0zXM8ULoJ9qvuHe2P
NHHw9ffM2Zdx0LN9eUW8VxOVw3FkRDYeDu1NFIuc1sS+3KDd6RHxwCP96MbR
/Vp4pPPbo0taCTBw6tfhTj8tpOct2VgsTgTDJ3dqn8pqY2rFH3sDapKh9tlf
76VAG91KqC4xvCkgPtzCQTmtjTTD+xrBoSmwvfD+olGMNkbdf3F8VToVmoRV
FJ/NaGOpV/Lirc1UUIroKuy6fxA5fhQ1P69PAz7TjYxebh1U3s+yZknJhNUe
i01pZR0cGT56rrMvE/qPUc9FmOigTuGYcDfnXaBYmUseuqqDFfP0jyMK7sLq
qXvVRZM6qMfB4NbZnQX97tAXXnYYj8krfvuseg8oUbE72qCHShaUQa3DVHBm
mnC9fVYPy2zIt6Y9qKB3U61rMUgPLd7TRsbTqLAaP3arsEgP/T2kmTqXfudv
Kx7g3KOPvdqpZNvSAtCnvtRafKWP3Gf9jtDkC+Hr3/y+D3wJdDEyXTjrXwKb
NmrZllEExiok+TVTS2BrzqxnPZtAUnRbvterEmBivyZj0UvgyFvjoWL9UuA7
PzHzVRbwfsNLj8ccf4HONvWc8RxggOAPaevuMgCxOzJr1Yh3PJV38gIqwcBH
guhtQbQ62LfeX1EJRnWVp/K6EWuuOqtaLVSCmWkXxWwK0W7Umd3QswqsAzZm
ctmPYp/XjjyjazW40uzyjf2PYusmbTSivgZinEQF7ioY4HS/RjjbeC0Q7s97
fQ4Z4PNcqsEMfR2se18J1TcywKVXxZ0LcnXgTR6efO9ogMYPLBwyLtfBsZib
xUq3DbCy+naFJX89sJcva3RuGCBdtZi2l3MDZK23HV/6xxBtWzNufBJsAuuf
F3ZoQ4Y4tVuk1dS0CVjpBB+lTRpi/BG3mrFLTXCN9U8enU1DjDEU48kfbAJH
YdnxKEUj1BqrPVyb8AQkDVK8BdKMMM+02WQfawtUJDlFGzoZo7famRwl1Taw
j2Q88/bCbx1AZxLs2gYswaUKQVeMsfznftO1O23g5vB5KO+2MUqI7Ltz51cb
HFAMF//x1Bj/kBC86PWSBnE9eX/XyJngyXhWyYq2dnBnnNwQWTXBNa1HPCGR
nSB01cFvk2KGLziKYk0cumAyeKb4caoZzlfcz+261gVUsvfUpVwzvPv3f1LO
2V0g7XfpxJc6M9xUu0+det0FSk63dBZmzJCR+exXDttuIIxbmSbQHEObqUtH
rXvAhVP4Pm3LHP130JTxfB+Ulo3337xkgZsyhvdFegZA3CWqwCDSAn9VeDkZ
rQxAloB88HaSBU74/ReVIPASEmJDhENKLdCH6zVDsM9L8PPgvODx1gJzaESL
y65BUJMwZTFCS4xTaTItrhiE5qxaA3q24+hIo3fmZB6Ggdj4xtBCK6x/WNTz
de4VJIxMsJEGrHFKbf+1yq9vYfDZ8HUOwxPokJVeXTQ9DbNs02rVo7aY26gS
Z8k+B7EhKgW6NqcwQX3R9ab3PGwczDh1deE0sjjlhMfkLsPe16Nm+tfP4mWX
ki55wVWouuuw+WnVDsvMZbyvfVwD0ZrNT1bx57BbddE0S3ETRD6N3MtjcsRM
Nwerg94/YeF6X0pB/nksNeF91yq8A5UhVi4Zgs74qU+8QPQKPSrjm7MDI86Y
OKiTqXWKEbkb/FffF7hgW6jqv8wBzHi0RWrhgrMrvjYZKJW7vBs7aszodYTc
sC+sqq6NwoqlNleb3825oaDFMii/3Isj0X1D3x+4o63IeVosHTv6usgmfg7w
wMbVsY64Qxxoo/LVTfawJ/p3PtGvDuDE8FtTOSNrngjyuR81s7iQJ3P0T8d2
LzR491ZB9PfPWlFbeXguzBunBPuyZ3h4UbTlMn2ujg+2TdSPhZrxYd3Knh8N
DL5oK83eYpzDjymNbdYmNF9cji9NmHgjgMPyYeY1iRdw5OpYf6n2AXRQPk9N
PeaHomqpC+phQqgjXslXx+yP2SO2D1o6hTG0bbdq9aA/amo8nNIhiSLzclSx
RPJFdDpiNi1DFsP1HtY2/3MB6NDP/jX0ojjm9u78uMEViNuLWcKREhLosrHH
JCIwEJ0NWAT0eiVw7IeQa8DrQHzSvDjaHy6J30yOVGZrB6FiOlvFqIIUNu/h
Y5lLC8LML9OB9P+TQo2iNU2RzSBU2Zv+aTleGq1u/pucepqMxntS4pm1SWh6
LNny4Fky3hd5ZcigQ0JkP7xnwo6MI+dKmHZ0SaiemRwj60hGj+b32Zv4+7eU
HL7e5kbGWmbkWrQk4fizFJ/FQDIGnqE79MqdhN7M+kZmiWQ8T+HQKssgoUvv
B/rlW2TUa2RrKrlLQvuk27T0ZDK+1+AxKMohoSXvf7pTt8mYqaHtnU8loSop
TT0ki4yKS9ZbdypIuG70UbSomIznNCOR8g8JP7OkT5iXktE/xV4qqpuEH18c
yfn8Fxn/oNKxRfSRcOxkOq9eBRldggqXQwdJ2OpOsA3XklFc+M3mnxMkbJCb
771c/9t3KmclT5GwajE9VuQxGVupSuKBMySkXppn8HlCRuUp+fN+H0mYrZPR
zt5Cxg7Mi/H9RMK0LSKsvpWMXj6Par2XSZjQPq9n3/a7P8VpzvMLCaMpGd93
aL/3zReJeKyR8P8AWkjCXw==
       "]]},
     Annotation[#, "Charting`Private`Tag$158336#1"]& ], 
    TagBox[
     {RGBColor[1, 0, 0], AbsoluteThickness[1.6], Opacity[1.], 
      LineBox[CompressedData["
1:eJwVl3c81d8fx+/Hysoq2ZJkz5B9zzsjKyIhUu69br7IzKzsUUZUMrNHpJJR
CYmbhIRKRkVEKWRvMn7399d5PB/nfR7v9+s9zuOcQySv0xdpcDicN4bD/X99
arO1MlP+FQ93rHFyY9e04lovDFgmvUDbrkVxb2K48be/RV4TTmpDj/RrrqnG
GOBnJR/Rxz/8hLrU/F5qSZLwKb9SuuiSBlDiL431yWh/vGZ+aGqYz3dUHHL8
Xz1tDH5e7pl8yMNRdGyww5lZMhn/hqUsWTP7F6pvLZH61puNT5vMWV1L/IOm
dzWPV0ffx7u2Jds/D5tCaV+lfzoWPcFr37/ReNlnBukyb8uE0z7Hxx7Hc2Yo
zaPxSc4EtvWXeJ9K9TcBDxfQ+PBE8QeJZrz9QWV/68NLiDZwP4sWdxteP0lO
QiV7Ge0f4KC51NuJl9+W+MrFvYou/9EnUOo/4XncRRMWEteQHO75HfPoPjxu
UFDnI8MGCiyps5rv/oqfMuaZexK2iei7LlU9LxzGf67lLEhc/4eeBT9DA7Rj
+AYJVit3n220SWMhu0Izji9JY6A3ndpBKqy3zBpOT+DbI8MHU5RwUPvH46jK
2l+8dn2ICt0sDsStDYzIy3P4qoWrib4PMXB7lDEtJbGIF5cK+j3mTAOTnNr0
MdHL+HsEf3T6MC2M5gTNnNi/hmfPuJzxeoQWysxrOHy/bOCjP3gtKGbTgRFH
4lvWz1v4DQYPk/yz9LCkE1zCQotDnni3InZuBnje93aiow5DtuVk69nEPZDu
9ClqO5Iedf4iPjlvwghdO/HvfdP3IBB03NPFwATyv/7NSnUxIekEu7pHYcxQ
HpDKey6fDeU223AJaLOARBfX6ek8DrRv0+pS/DoLEDRq481ouNCWi7mQq89e
6CjaH7+B40Y++aYBX+TYoFXj3FmD3APo94DRB8MpNljtUn+gasGLXIoK4K4S
B8R7KkTRLwsgUSQy03GLA6Y0z/WO/xZCQ99yM2lmOYBbdfio+/xBZMmVvejz
kBOukM4eqhETRaxP+PPKGLlgK19EY+nkYdRqnGk66swFg32FfVERYkgzIq3Y
4vA+WH3G9juPQwItC3JbxkbsAxGPPZcfXZJEFbV3t5tG9sHXnvvVzL1SSGz+
to1C9n54Z5Zq1NIli4YT2Gn/29wPNK2vEnId5VGmRFJF7llu8PFldOzcVUBs
jgmMbNwH4LoHjTRnjRJa64qpn07kgTrbZMrXEFVERszqnMs8cHsZP7CSeQz1
VCY9V7XnheaKJefHTWroyd30ylBxPpjrszVNkNREgvSC8kU3+aCO5fZrOnct
FBeQ/6htkQ/W6xuW6uu0EdmurISjiR8oWcezwvwQ6umQE1M9IgBpJ9mvz3kD
Au3qArsEAbhnMpXOJnccCRx8mV1oKwgcTfOlf5/rop5fnckq80Jg/sKW0Zb1
BAIbSw47G2E4714q+2L+BHrS1pcY0iAMgxGbRyQHDVHcw+HY1tiD4OmRfCix
2RiJqAehx7dFIMEhg5D23QwNeGuGNr4RAVOba+TKZXOUVLbV8HFVBMQd8mjw
TBZoiz9Cc8XhEITiacS0lSzRwHacKl5KFFqiBu7zP7JCScdO+lk4iIKr2m3S
9dNnkL4X21PSLVGoV3kye2/7DKr+kax4Y0UU5E10bH5fsEFJb7JkPr4+DMHe
MtJCp+yQwdZ5t7Hlw9DWoav6e7892lIRKVuWEIOG+Nri0mF75FZSLM6XJAYr
FB07rVAHZBBXfohkfwQ+O86avpx1RFuvvQh+iUfgk/WCwxM3AqreVMq7TjkC
lrzi/aI/CEjEvUbwkbg4yKuutcR/IqIt8yae5UVxGJgzP/Oj2wk93f9p7/UE
STit1zs0reaCGnwEfqm+lAQbJv/AorcuqKX7Yv34lCT80rWsuGbtivpjN50N
TKTgkXLr+/xrbmh96zCFjkkahLVb7WXH3BF+POBy1HUZsI42i/6+1wcZ6r42
Uq6RAVxZ/KlqZx9kkcdy8Oe4DHh/tCa8oPggol3+e10DWUh1tBexD7qMorve
idHQycHFof489VVf1PFccCA8Qh68H9gqs8oHoh6u/8oVq+ThrlWDX/e9QDTo
VRX144c87Lw/sznCGISmpU4oAihA1TYKX58IQuy5XnG7OwpQx14vqFp3FUnr
jQqhRkVQ3iPEHJsVip74MDDx9CtCp4/tyGHhMKScL7M8O6MInycpvnKFYUh7
278jV0gJbLcnqo1sw5HZC+bAnWAlmBoovO3iHoG8ZVQ+vtI6CjOrgb2u9VFo
WM1wV8jqKASYdo5wMEQjM317+VC3o2Amv8sacDoaSZ8Pv4nPPArav8uNQ2ei
0XhSp1HT6lFgGT5zP1f2OrJfJL+mVCnDzXGh5h8fYlH7TuC8yDtlOMBTvvhJ
Ig6psSQcjPihDGVFDDy3wuPQfrGqkOPsKvDp69X73irxqNt6W6PZXQU2K6Kr
Ju4nIL261Oo3Eqrw9dhjU7fKJFT99sHoYaQKK9WqyeHct5BIz0uOaBtVmOg3
svK+dgvtTI166seogkEDffec2G1UKygv83ZMFYr+NJnGr99GsuGtRa05x0DC
O7K3/VkyOmC4lvJunzo0W/X6G0enocV203UxOXXgrePuaexIQ10m+efCT6jD
S7e82Dec6Sja3FhU7Yo6pNK6sYQUpKNF66yK4mF1qO0pjW9sy0BdZNQRVqYB
OFOJV38VslB05I1dVaQFqscunzyqkY8IdEOkO2e1wFwpDBu+mI+0riu2Tvto
wX/nf+h9Tc5Hi3FfbxYVa0HdXhNy0wzV/o4MPyezNmTPqNVYlBYg7fwPKtO9
2tC9sWrQIFWEll7xuBW64WHwP0E/a48StG6pmHkyEg+H8u7P1uSXoK1xo/bV
TDz4Z3Lwk3tLEB3bVXHTd3hoVpvVKtQuRQcuDI0tSSBQkq+qrOZ4gNR38s8Z
jCOQexgtf7KtDKGDqeLLFQCTBfvD7nmVI13XQ/h3LwHYsjs83j0uR/pPy61z
2wBC8D45xlPlyMiwNdpoBODfoSA3vPMTZOG1NpbNdhy89jYQd4gViNRkl2fg
cRyEiVfMQ59VohhHYd50aV1I2/PgAdNgNcKT379zVdMFgfQXziPYU7TqEnRN
W18Xmt3sR/9IPkUul3uGR8/rgqOcgvedwKfIJOb6fdk7unDsYtFDY55niO3R
7NHmNV0ojPrKQCY8RxmrjWYzLXrwrFJu+Q9fLbL4d2m36ZMe2LtMy+ob1iIm
HF9V8rAe0JY6C/T71aKrTL771df1wORblG/Wx1p0XlBiMFJGH/aJUSKexNch
Ud1bLrzJ+hB3sdmRieklepzoGKXnaABOpjFnJBUakX0Ere23Swawz85u05vU
iBj9S6V9ggwgq//uylxqI3JymPuUe8cAOrP+qN3ZbkT8MmEim28MIMOtZIP0
oQnFtue+qpQ8Qb1vMz6WNVIQmXZ4TWjxBPylC0n1jWhGAlcc3NejjUDvb3m1
nkMrGvYfu19z2wi+Kp15++ZqK8q/7DLil20Et3nMTc5ntiIxd7/TC0+N4O2M
e/NQfyuSdbypPjVmBHRboqxsVm0Ib9BANwTGQE/hWMFbtCMip2BO05YxWOEP
KuAudKDSssGu636mMDjBYsPf3o1EiJEFuhGm8I+Whef4fDfK4JXy30k0haxW
D40bvB9Q/I0AwYBSU6Bwar/wcf2A3C9yXrr4zRT8+2L2ERg+IsVDhoz6cBL4
ymlyih5/RPUZ1boYqxmo2DE/ZafvQd034l5cKzIH8wFBycXxXhTfN8R6pNsC
hmxllR4vfUMf3/YEc+idBosb3keLf/xAv1h/KFYMWIHVKYYCE7ZxdCNAvkDT
0hrWnGftrrpMorVjKdZXpmzg4FZxDmTPIpb+ASPt4LMwWJyilsC7iJ6kO6z/
XbQD9fojl+R+LyPhyvW/5nHnwIVZ/Mq46DoS+tuXlUt3HnKxYgH8yX9oKrjj
VkHeBTjn+d+2NmUHPW5NfTx3/wJUH09bje7aQZ4cxHc6jy/As2zb/PZvO2ih
aI3mW+0FuCuUE6u7soPWO8QCuHougPfRRfFtqV3EwBfmEEXnCHoXnD94Je8i
0efKUhddHQHRrC9RKwC/dnYMnno5wn/t4u3nVHFQYtRBwgIcgWaFfytZCwdS
Q4TsnEhH6GhkPbhkiANF2iT2/ixHYHqgFhpIwAHecmLlRLcjEL4oNgfdxlHf
kebEFD4CuGnAxo2/OPicI2scI0iAI5037e/N42CjhVkp4CABCFc3DO+v4MBg
Xxvu7BECBNlNGhTv4uB7BcoXUCLAOZFgWb19GOydVBwpNCJAcKPqgd/qGChz
sLfdNSVAyKKOqI8OBnZqM0+izQkQH5Qbtngcg/sxZaHOZwjg/JCcNGCCgY6o
qLA0gQATma9CxB0w8Di373xVIAHqaze/VgVjcDdyQb/wKgFulnnsTwrHoK7s
g+zdEAKss0YOn4/GgH49YcsvigCRkQvnBhIwyEmhy1a/RQD2K/VesvcwePNy
LEoqmQDlXYF5eTkYTI5RLvGnEqCuX6uZrgADVaUQra17BFhsc6UvLsWgq2vl
W1MJAV69zLFTfIbB0vLn5soyAvx8+WJb9gUGfILVDwseE6BCqrODrx6Di26e
V6OqCVDD7zjd3ITBNsMfPsNGAvDtSw482YHBYfm3mPprAiSeNrv7phMDY+ui
SckWAlTufz8o+QGD1CLHOuYO6vn2xV8NnzGQgy9nu/uobJ2hRzuEAS4NX7rz
hQAqc2tdLMMY9P4tXpEfIoBcBqF1awSDB8dZ9B1HCCDrfqerbxSD4HSf5Ftj
BFCMWYpM+4mBxczAj6ZxAmx5pUbjx6nx6OEV5icIMHlH3KvrNwYds8ydFnME
cDUccsudxCBX34c/YpEA3+7bPRmZwsDn3oBL1QoBLFU8EcM0BvrzOi9G16n6
Ikqecs5gwHuimJ5riwDb/PvysFkMprOYz+juEoDrpl5KH5WbFrwLL9MQQc3g
uFjiHAbJhgPzhfREmAuKH5aYx8A5Rwd9ZqTu/2a1vE9lzaWiRFpWItxNFmGk
X6D2lzHzkDI7ER77RiadoPKPXG9pMhcROvac8nCl8rPl/qAUbiIQvm/JeFA5
1kSnrYWXCEpMthaWVHbIL+JeESDC3oTAC9xUVlxlIh85SITS/Ndfaqn+aE96
V1uLEqGXYQhpUbm/oB93/QgRrko+4sqmxvtwTftUjSQRDmmZdn+j6gk1K8r5
LUMEaWPm2VWq/tNFTNMHFIjAJ0X6O0fNj/iGl6bhUSIcIC3qvP2LwYZ5f2yg
KtV++8q5AGo+O4u1B0rVibCk++kFDTXf+ZuFR75oEYHT+WeL6x8M/CyY/BgR
ES7wPVh8SK2XYYlXs7ouEWy5hCreUuvJv9XH4WpABNZA5FxHrfespbZjphER
itToI2Oo/dBcWlj+zpQITFY2blLfMUjbZtzaMCfCAwaGmOJv1Hkr68uwtyZC
2Yz2sFAfBhy7Wn/izxIhzablO38PBr/OFKq+PEcEy4TsO9PdGNzEefUIkIhw
9ihTOEs7BgSbPpGTF4kQkDvkattCnffHWl7BLkSIGvZy9qdg8M2WkfW7JxEY
rw4MidVi8KTc037vZSL092guPXuKQQRt3wMdfyIUnna33l+BgWRFgUHuNSK8
yooRwN/HYIuOMaU7lAhfRi0Z9+Rj8MHec2wngqp3qPh0NnWeAxi0whxjiTBx
yGtF8hYGJg4FXbcSiNCaztcsHIeBUPUeQUoSET4P5vV+j8Sg5XxvrUgqEWrk
V1Kf+WOw77nH4mgBEXK5vILKz2Igm3iSf6iYCIIr7CHnLan9fVFGt7+UCLcy
HmNfjKn+uCfvdJQTYeqSfrGUJgZf/MlKT+uI4On7OUSaF4MFMz278gZqfoNo
X/OxY8AsLhpR2kQE8fqzV7roMdDqH/mY9ZYI+hDFHbaIg9xj57yjPxGB7OWE
W27HwQs2zYzQXiIw6BXSzL/CwcffvJSgAWo/i3p0l1XjAEvvZ/f4ToRdlXYN
qywckNcsK6wnidBsHkdLdsWBdK3RrDhGAp88rg+Wc7tI77bEgUN0JLh8XHBa
9OMucnBhwAvsIYFIR80Di8pdlMjbksi+lwSWEzv/1XnuovkgJLfOSwIu03Cb
yJ87iMlS2HpRgATnzyStbDbuIFGp7eBpYRKUDx+yaMzcQVZf6zt/iJFg1JKz
ScBsB9VoHHN/p0gCDUvxtJmH2+gDJ3fKG2USeLY+tw4K30YTk0svXx0jAX+G
iYCm9Tbiu1fFUq1NglucQiZnt7ZQ8Kbso3tGJJCtvOj6DLbQ8ZeHpy4RSFDc
eirxSt4m4jkVzm/rRIJa8Wd9hi6baGZsyETXmQQkngYVKcVNlMmc9ojXnapP
9YcF36sNtGDH6PE2kKq/n4Ni934dtc2QcyqvkuCB48G6SzfXUU7E666sEBIo
nh5mDzq5jozLrspfjiJB9Avbtsvv1lDB+vSc8C0SXO9/0ZVcs4oCbxqLMCdT
9To4OPN7rSIzkRKLlRQS+B0P0IoQX0Ubho5V7++R4GW7j+HwnRVkmf7pclAJ
CRzW+PW97JcRdqxm5dMrElS6CsPdigU08I5L/BWFBIG1ITvGZxZQ+Xkvmwdv
SPDpZ0Z6wdo8souRfBH6jgRLHuyioprzqKr3XpBMHwmSrTXjv52bQUTfsH/R
0ySQYNS9a5r5G6ntGZLxniPB7YmBzZTqcbQ3S93h3CIJUu65nohv/4Xqmhca
lNZJMPswU+PU1Bji5CKHDtM6wehGdrAq4zB6XWmEqQs4wTwjbauJYAfS95XL
IAk7wenEPzGKqm9RuyqXQuIhJwgiKKbzalHQx/pBhzEJJ/CyXPDtUH6Ahls8
a2+qOAFf6NHxO8GNTZtfUrxGzZyAbC37c258uCk06woDq6UTMNCFp8bhRpuw
Cxdyjp1xAkvp9Atzd8eaGH9KvE+wd4Lyk8Qj0Z3jTTwz9eLH/qPGE2tBv3F9
ukkFG/0eH+5E/R8TaGMzV5pq37z1ex7lBFmTunZVd1ebtK4/ZPlxnepvYSjY
/c5aky6Ln4ZqohO4aSc8aE3faLLk3pM6kukE32uc39t+2m7ylJI7qfLUCfIg
P9Ulgpay+Jfz54UaJ5BhaBP8K0RH8X+yeiWuzgmSlS/ishvoKMHKlNLhJqq9
tdRSMY6BEq9jRRvX6QSaFrGfBYsZKaWWV+q/j1P1XxwbUXNko3in9Uv3TDhB
wcjqrZ397BT1QeWs1r9OoOHEWsXdxU7pIM9eq1hwAvOTfCTJQg7KdKCTTsS2
E/gJN3qOSHBRjuaaUcS4yaB7vZnBx5ub8m/soSIfLxmaxKsGY0e4KS0SjAV7
BcjQVvU6gM7iAMW6qjliVYQM6+6BtmqqPJSgFjW9dlkyBOpfeoTj5KM0Th1q
vaRPhitEhcQ5TiHKDYWwYwRDMiT3Sp0+kSlEsfAbKjljQobw+ZpcQ1Fhyuh2
2g0dCzK0Srupntc4SKHjZDVmdyCDjrLOTYVGEYqJ2ur7al8ybDYbJYvIHabs
C7bSLg0gg+EA8rMMO0wZolQ+zrpChts3Ht+O6DlM8TC5lBgdRgYcjm996poY
xaCRXLpzgwwKKaW+3wOPUP4H3Id64Q==
       "]]},
     Annotation[#, "Charting`Private`Tag$158336#2"]& ], 
    TagBox[
     {RGBColor[0, 1, 0], AbsoluteThickness[1.6], Opacity[1.], 
      LineBox[CompressedData["
1:eJwVlvc714sbh2VlJbLKiPjYe5XQ+3nsmUiEyKxjFT4yiqzsvRIlKaKUkT06
iMwyG6KOdaiMJFmJfM/3h/t6Xfd1vf6A+4iT1+kLlBQUFEv/8f+tstxe+1Y6
SkimWVBITwepxXWeHzFLroNWt4K49igOInUsIuhwchdkadQGKUfpEEtiT2ji
S4ZgQuJKk5qYE5E5k9lHnTwC6tXHN+ci/QjV/JCboT7/QDSDxu9GqihiWbpa
5nrJFFDv673IIJZOtDM+TlfNnQE510Lxsbe5RNbc3fWNpC9Q8/uYRmXkQ8Kt
K92mJnQeAjaF/rUvKCPUH8Y0k32+gfHommQYVQ0Rq0GwZssvQ9hnqgTmzSbC
p0Kl3b/kB3zY/lg4INpG2PAr+lkI/YRHX3YY1Di6CO1kaVGl3FXg+zG/x+Pt
a0JmR3T0AMc6rMqJOLQ2DhFcnoIJP5I2YKIlMs0k8h1B8ZH3xCDtL/g542W+
3D9KzBtwfS8L3YKdtp2KmgfjxJt61vtJm78hQcwFRqimieeiTOaePjvwbPuT
5BrlLFGURUtjNP8H/lH8Zvz89FeiOyLsY6Y8Bd7qSJJX2lgg1BuvK1EvUWDE
RTY9l9XvxLMf15J8S/bg3vzeBXHRFUJEPPDz9EVKTJsWp46KXCVuO/jBaSEq
pH6zf1GXfYPYn03OfjFBhVTkSWbfD7+IyAGvH3K51KhCJdvO9Gab+EV7yTDf
igYLPm0WMlJRwGXCvWA/By2ONIx97m3YA2dLXSyWkvbiX7N9YTsRNPB6xrHM
zpAOPx7u7/K9tReQ135vHy09LlU6zIv30YNEgnXDk1AGdLesZT2Xzwx5bZYH
eNQZ0c567uTiPRZg2zL3iN9kxBmZ6qiTlAdg29WEz81nH6pIf474RcEBPvlG
/h+kmZFEO3xKJ48TPo/oD+jNMyOVzuE8ZdOD4FpwHzPkWVD9rbwfzSoPCILA
t94UFtR79bt99jMffBrLy6FcYsEWhk5+z2V+MDuQu+JTwop/7gaz15IEgamM
+95jugNoy6Ir8dNYCDoNcoymLh5AQcqYlzfCSaAanlVoKsSGupKJA/dYRGGV
l8MsNpwNBRNOWT3xEIPy+oydlgk2VNe2vMnwVhxIy6mWsrnsuHasW/BlnxSM
J+yn+muLHfedW3PIs5eBHNHk8jwrDjQ/UyfzelcWmO0T6Jg5ONGWxpmRtVYe
NvqiGheTuLBRISh19LoyuACDCusqF7bai99fyzkKwxXJNco2B5HlCSHxtOUY
lGXcqggROYQidfq78WKqwEvDK1OQeAiTO4o9qT3VIM4//0nXyiFcV+W72dig
Di7Wj4tYWrjR4repSOgVgOFeaZKyMA/uBB/V+e6NgOqV960TeLD2Nbcps7QG
8PA35T44y4vpdlqmCzWaMDzzOl1pmQ/TLdtjLJl0AS3NWKwtD2PIidx7tcu6
UNb1Lun68//8uG+C6Ec9iCsZj+2M5ccTk02uiW0GIKASCE9TBbDwTt65m/+c
hBFv1ZDmdgGkpWrWL181geTH288H1wWwbzXG9QS9KWxzh6uu2R7BZ60tl9Xk
zWBkJ06ZEBfErzLtpYeemEPyUeMrpraCqIRDllGnz4C2F3OVU4ogKrSs9OXs
nIHKyXS5mDVBbJ3W2zt73hKS2+9IDr4QwobhUA+eU9ags23nPr0qhGWBJMsZ
dhvYVhJ4vCpKwhBrsYKH4zbgXlQociiZhNJdzkzHQ2xBJ670iJONMNa5DxnV
L9nD9gsvhytJwvghh9T+1N0BKrfk70W3CuOLatKRI5MOIOBZy/tERAQTi6ff
xg45wrZJC9fqighSbViN/tPvDFXsQ/uiE8QQ5pQ+fz3mCs99eGaUm8Sw//qy
wb0OV3jZf6Fxdl4MOfWd9AMs3OB97NZFHUNxdDZhmb8T5A6b20Kt1PQSuBI6
6SAy7QnErD/5RrQkFnTL843u8wE9zRf6irWSOAlYWXrRB0zvMfL/OyuJdXVF
8ZWtPuBonf9KU0cKL5v8HD4TSIbIvh4SJbU0OnWw6Cis+0JvDe9IWLgMVnQ9
UqCSCYDhA3+Vyj2TwTF+N5aO2wHw0evZjclJGczkqJF5TxcIi+K6coiyqLGQ
O/btayDsz/OK2/0ji+x6pHSxhmsgoTXFB81y6Ckb9s7/TgiU+dDSc72XQ1ml
jh3Ww6GgmC+5uvRNDvNS/Ca4H4SC+o5fbx6fPMqdZCslzobByTqGgD/B8igc
C99sPcPBW1Jp8G81BZxSkzGwabwB48f0dvnMFTDmrX43BW0knNS2kQlxV0C2
SJYLF05HgoRdWCKRo4C/POZ9Pb9Fwmzya/2WdQVs0V1Qj5eKBpsVlxetzxSR
kfsu0TkQC91/ApYFehSR3dsivVY0Do4xJvCHTypi6VTLG3JYHLCTnl3X2K+E
1sKhcaeV4qHfYud4m+d/PtSc2fkwAbQabla2iyrjHpeQPqIiGSo7Hk0JgTLy
K1a0m3OkgMBwE0ukpTIm3e2X1AxKgT/zU5e1o5Tx0nnGMyOkVKjnlZHsmFbG
r+9j+y5vpoJUWGdB592jeEUo2KqoOh049TYye9hU8LO9jAN7ZBasdBttkqRV
UMVw5mhsbxb0GeafC9NVwVdnvc4nsN6CSBMDwWNXVbD3qWCRxv1bsGJxp7xw
XAU5GeyUg7uyoc8FekMfH8c6uEXOkb0DkRExu8qghtya1qqrKvngQP3JKc1K
DU33W9jnXcgHtWi5zkUfNTRfFqTPTs+HlbjRxIJCNRzx1B+/9u2/f5okNyuD
Or6x2ZSiKb4P6vkDSotv1fGrVeOEg3gB/Pyby/2BO4F+6nMtQ55FsGkml2Mc
QaCFY8lVufwi2J7V717PIbB7a2pk7E0RUDNfEzHqIbBj3OE4m3oxcJ7/NP1T
FLA41DuVi+URqPzJP6czCxhDW6aU1fkYgP+myGo54sTjjfkHl0tB0+0I0dOE
qNuVLN73pBS0q0ot8roQd722burPlYK+Xmek/gTiy6NqDxQvlIGp18Z0LrMG
vk8oFZ1wKAenFut7Opc0sMtxV+NDVQVE2R8+eEtCEw9uQZ/0WCUQLq963I5p
4i+Xa567FFWw7hoYpK6tidEj1XVUYlXgSh4en7LTxN/vxGoK/avAMCr6oVSa
JkpdKtg25KwG5idLCm0bmthOvk1B2NdA9nrzyW8vtfBpmlmf88F6MP3tsdsy
pIX1tzScG3TqgZ7i0LP0cS30CyvO0vath2v0vuwqm1ooUlUus91fD3a8oh8j
JLXx4Zps0kpsAwhqprgeTNfGTO1Apv17m+Bpkv0NLXsdLNscOHxHqhlswqnO
jnnoYKjOnepR+2ag8yuW8AnUQavK1hCTjGZwtv0+lJemg4NXL22NbTUDt2So
wFa7DhoGOWSEv26B2O68vyvEdNEwOSiL4e9WcKEa3+Bb0cWFkqPxrqFtwHPV
1nMzUh/j4knx3NadMO43/bA2VR/LRccLUwM6IZ/sOnElVx8bVZa5BLI6geR5
5fSPKn38d+AaX8KbTpCyT1SZn9bHq8ECGumnuoDQeU79CQ2Qt6G8xM24GxxZ
ee+2bBug3ceeREfrXih+/LEv+ooRqs6oa0a86AcBx4j7muFG6LogLn9zrh+y
D4r7/UkyQkeOx6ZdrAMQH+PP619shM/CXynFOQ2A5wVWjwtjRsh9u52xjXIQ
5I7o0WmjMS6ZWkiWPhqExuxKzT1MJ5EnO6nAnGIY+mPi6oIKTHBFfVvLeOIt
xL/7xCTcb4pDT82aer6MwWDHcDCL1mkMWvlh3Ph+EmaYJuXKR8xxzCFgbnln
BmL8Ze6rmlmghPDs6cRTc7BxNNPi6rwlNowePXnbfwkY34/oqwdbIbvxUFLe
zg8ou2W7ubBijc+9T3xJaluFwxWbCyZx59DCberTxY0N4Ft4dyeP2g5TWDiq
rwv9hvng3pT7986jqGLQrnzbHyj1N3HMPOSAPX+vCqyf2IPS+MGq/50DTtAN
8ywyUSFbzaWVqfuOyJKrOPCbnQY1moTmPRyc0NeWy4ePYS++qNDfo8LjjLf6
1+irKemx2Oxq4z+zzhh7pzwiT5ER393oHfr1wAX7fCUWYwz3obujaMJ3rwvo
K/h9MiRnP5rJ/HQWPX4R9ZUMhOd+smBo4sTtd6sXUeipuR4yHkD2rBFfu9a/
MJI+05mTYMNlueWScyGuuCbkMNRmz46HmwL25Kq44dn5Ele3EA6sWmbYqqF0
RwGjzDmuek5MqWs21W1xxyWXsa7FcS4cFg8xqEjwwFcYUpEhcAhtpc/npxp6
oplAjVyGCTeqCJRyVtFcQg3sPvIrgAeDmvfKlg9ewiehSrSDTbxIsxTx8Ejy
ZXRlKKBgWODD9W765kvnvPA00xWIVOLH3J7dresHvFE+TbjQRl0AHTcYdMO8
vXHt9vWcwTcCOLrF4+T13hsjpDwLMfAIrumeKM1R9kEa2pc35lgFsZGBk242
3Qflg9rOFjz6r2MKVxX5Nn1wxm7QVsVYCE2i/01OtSQjHVUA3eSMEOoZJhsf
tSKjonhHYdwXIUTm4wyfrMl43KMYFeeFUD4rOUrUjozPZvkCor8LIXvR8eBm
ZzK+CYwfl9oSwo8dKW6L3mTkmiPdvLqfhK406tr6CWQ8FtqSckCVhI49n/cs
JZLR+3XRoefqJLRJSmvJSCbj1PbQgwtAQmOOL6oTaWTktpuvrNcmoaxwurx/
NhkPNU/0nD9FwnXtr4cLH5KxMrpzsMSFhN/pMj4ZFJNxfuz1yTN/kfDr6xO3
vz8i4wfqHz07biQcPZPBofaUjCxRcS2mXiR87kIwDVeSUUi28d76VRLWiM31
BFSTkULgMkd+MAnLFjNi+GrJKGIvHW8QSsL8K3OUbg1kPH/3pXduJAlzVDJb
mZvISDBkT+vEkDB9mwipfk7G3/mXzL/HkTC+dU7NppmMNTxa7dmJJLwRmflr
t4WMo8qcCpopJPwfH/XD1g==
       "]]},
     Annotation[#, "Charting`Private`Tag$158336#3"]& ], 
    TagBox[
     {RGBColor[0.5, 0, 0.5], AbsoluteThickness[1.6], Opacity[1.], 
      LineBox[CompressedData["
1:eJwV1vc/1osfxnGzuEmIUsi8M7OV1ef9NiMjIyrZJKuDm1AkMjIiJFnJlmRE
ZIVyzCJETimrFLIpcsT3fH+4Hq9frj/gKeDgaXqRhoqKauG//b9VFls/50s/
EJKJ5lRHJwNVo9tthk3in8OSa150awQnkfDxZuDh+A7I0KoJVIzQJhZES+hj
HvdD63HfBlVRByL5a3IPXfwwhH5V3pgJv0KoZAffu+H9Ge5fV/+3njaCWDr6
TOr64wkQG+l2JokmEa1MxUkqmV+hoL1Q7ONgJpEy8+DXetx3GN1RUa8MLyBc
O5Isq2/MQsgH8S+2eWWEWsGtJor3PMiT/kiE0FYTUeoEW6rsErybYYtl2Wgg
vCuUWv0eL8OH0en8tyKvCEs++SvmQqvw04+DSZWzg9CKPyqikLkGNMOsNO6D
bwipPyIf2Dl/gdN3LbuW+n7igIdg7HLcOvBQVScahQ8RVCM8J/p2/Qbnwjqz
pd4PxKzegcWyG5uw8cb9aXXuKPGuli0nbuNfKAp6BsO0k0SjCLOZh/cfmKYx
lvxJM0UUpuyi15/dBiHmO4aNptNE582QkWRZKiz6fllOYf0HoVZ/XYFugQpZ
zbV1ndYWiafL1+J8HlOjdUnqnJjICnFELODbpDMNfmZTo48IXyPS7a6AqRAt
Dj8ImNfhWCf2plJSX47RYopRDavPP7+J8LeeyzKZdKjEGtfG/G6L+L3r8qns
c/Q4fSKokImWCv4i3PL2cu7Cx0Nt09111HC21Ml8IW433nLsD/tzkx7efLUv
sz7FgC+2Y1773N8NyGO7u2cXI3J//XdBrIcRxGPP15XcIGGK3z2uC9kskPXK
gp1bjQm5e9hN5x6ywr5NM/eYDSY8o1wbY0jDDlsuRryu3nuwPo8j5jcVJ3hn
6/v9c5QFq5UvnNPO2g/fhnXfnpxlwS89So8UjbnAJS8H78qyIuUv6TD6NW4Q
BP757jus+FrlwuDUN1749DErjWaBFVcURuU8lvjAhD1zxfsxG9o7nBOoERYE
5rJDD4sZ2HE8m1951UAI2vXS9Cec2bFuKHcoLFQYVEJT8o2F9mHPM5ZvD1lF
YI2H0yQqdB/OeeymlLiLQnnt3T/NY/vwwUBBJWlQDISXEiykMznQ3/Ce7t89
kjAau5f20iYHZrW9iM2ylYI0kfjyrHOcuENhsH2zIw0strEMLJz78dhlGnG2
GllY74mon4s7gDxnk1o+XFcEJyApsa0dwJFVYvhn2jEYqIivVrTkwrmyVecn
zceh7O79iuAjB7F58Kx+rKgK8NDzSOXdPoimpISXdB6qEO2XXdKxchAN6hpX
6+vUwOl8cSFr8yG8kqaeccMXYKD7qLAimRsJ/b2Ri14IqFaZcz6WG0l6s/dZ
jqoDN19DZu5ZHlxuXCr6Ua0BA1/fJCks8aJX1VmGs8w6gBYmrOctDuPspSLJ
50s6UNYxFHe98TA2BG2SRUdOQvTj0aj2KD7Md04SiHulB/xKAfAkgR9njVPt
Uj4bwrCXSnBTKz/u1Qt0qlgzgvjirca+X/yYfuYhDcFoDFuHQlV+WglguwKN
sJqsCQz/iVYkxARxzGe44FCJGcQfM/A1thLEq+QEh0jTM6DlyVLlcEcQ4/jL
FtL/nIHK8SSZWz8FsUbmhMU3GwuIb82Q6HsphFd1JcR5T58H7S1rt8k1IeTP
0lD8xmEJWwr8xWsiwjh3rja/aNQS3ArzjxyMF8ZjYSfOqwZbgXZ0qYCDJRk5
aBb0GxZsYeulp51vHBkXBZatytzsoHJT9mFkCxnnR8nvBcftgN+jhqfkyBHk
W/z1d0y/PWwZNR9YWzmCWVFGZ8Z7HaGKo39PZKwotrq/+zR33AUavbm/KjaI
4hE+X/+8Nhf4u/di/dSsKD7SMi4PNHeF91GbztqnxDCNoe11dqAbbGwJtdAx
iqNwzt+WkpMeQEz5UcIiJTCSZBD+eY83nNR4qStfI4Ea7NGnK529wfghE9+X
KQlsP3TG7nmLN9ifz36toS2J9y6e47cMoEB4T5cwDd1RnFEdfKj0ywe6q3mG
Q0KlcInXTJ5Zyh8G2C+VyjyVQoGrz3170/1hxPNp2Pi4FD7KPL05xhAAc2I6
MojSmMihErIxHQB7szyjd7alMcmtkkex7hqIa07wQpMMRvmxkqIygqHMexfj
gfcyeJXr1JjQ4Rsgny2xtjAvg0GNlT5Hc2+A2p8r3Vm8sphBNVGpezYEDJ+T
/LeDZHHnRWqCi0coeEko9L1QlUN5ZpdB1/owGD1+cofXTA7/CWoYY90VDoZa
llLBbnKo7zXP7GcaDuLWIbeJNDn8KpyuFzwfDlPxb3Sbf8khla9aQZZkJFiu
OL1seSqPL/b+fjn+Ngo6t/2X+LvkscoycqVfJBqOM8XyhY7LI8vs5/13QqKB
Q/jpdfW9CsgzaljgpRADveZ/lF95KGD7muHT6YJY0Ky7V9kqoojjJCt9t4p4
qGx7NCEEimhbMZEYwnkH+AcaWMMtFNH63ZKpV+Ad2J6d+EsrQhHv+w31LAon
QC2PlETbpCJu/4zQj9lIAMmQ9rz2B8dwvkZ6sPNZEuw/uZ7ctU8JF51kr+iF
p8BKp/6G8FElVHFy72/qToGeU9kXQnSU8JzD/K1WtvsQbqQnePyqEoZkF5Gu
59yHFfOM8vxRJbyX0hLd1JEKPU7QfaNYGcsGJxt+SGdA+M1bO4qgijqlavpy
ytlgR/fJIfGcKh4wO0E1ejEbVCNl2ue8VbG2NlHjQ1I2rER/uJ2Xr4q7ro07
NM//90+UOMRGUsOTUUnPjItyQC37rcLcoBpqujdpNorlweqLA265bgRepJbw
Mr9cCBsmMmkGNwlcHk2arckuhK0p3c5faQT+Dh3hdBosBDqWa0f0uwgUtPE+
nqtWBPttPk2uigB6vbhfUsn6CJS2sy9oTwHOsKyLGHQUA/DdO7JWjuhx2cc3
3bMUNFwFiK4GRAGafxy6npSCVlWpeVYHYv5eiSS92VLQPdkerjuG6E8fbkM4
l4Gx5/pkJos62oWcPrNtXw4Ozecfal9WR8YFkk7wswqIsD3MdV9cA0dE4zIY
RyqBcHrd5XpcAxcvKZ8fo66CXy4BgWpaGtim6/fuu2gVuFAGRiesNVB0x88+
0b8KTkVEFkgmauBQNX+63oFnwFKyIPdqXQPJWaIrjnbVkPqryXD+b030E5IY
/H6wFoz/dd9p7tdExzJmZq2TtcBIdfBp0qgmxrjm/x7yrYVrjD4cShuauMEz
dzqjrxaseURGbkpooY2ikmVZTB0Iatxx4UrSwmlqMWlGxgZ4EmcbpmmrjQ+W
qZlFpZvAMpT27Ed3bXzUxV7h5dAEDFeKxL0DtLHjZEjx4r0mcLRa7M9K1Eb/
Ze7phD9NcEjiBv9mqzbSlc/lOLxthqjOrBcVojoY/7Q+o7ipBZxoR9d5V3Tw
sXO4nk/oK+C+auWxEa6LLxUWuDWt2mH0ymRBTYIuThgXSbRea4dsisuYb6Yu
zggUlVqltYOwh6/pcpUuMuk95vv0vh0kbW8rzU7qorJxhNUesw4gtBvpPqEe
JpTtiBLGnWDPxvOgeUsPlQ1TeXesu6GoeKQn0lcfjSUYArg6e4Hf/maORqg+
iu/IycBSL6RyiV3ZjtPHpSeZehFcbyHmlh+PX5E+zlgwVHu6vgWPi2zuFz/q
IxOTwI7Nrj6QETjJoIUGKOIjZpP7pA/qUys1qJkN8Yto3R4W+gHovRX9PDDP
CINdpK0WpwYhZugTM7nXGG/1u5kWrH6EvraBIFZNUxT1qOrLHB+Hr8zjMuXD
ZhhQyXhWjWUKbvlJ5aiYmGMyxS/wkssMrB9LNr86a4H9a7rbepkLwPR+WFct
6Bw2XDOYW+VagbL7Vhs/Vs4jd7hwFf/0Ghyu2PhhFH0Bt82ILzQSG8D7Yygj
i84ad4cEJRtd+hdmg7rv5Dy0wRqDFybm3DtQ6mdkn3zQDqXD0ufY/anxKP5z
rnfIDvsk6XLrzWhxX/XllYkce7w+T6Ww5EGP6g1Cs+52Dtjyvlfbwnc3vqzQ
pVbidsQfmSWs9KGMWGRytf7zlCO2DARwnOhmwqGw7v7fuU7IN0jSPra5B93s
RWIXPS9ih5p4+VV5VjSRWnUUUXbGJTYX3yQ3Nrxxeyx9aM0ZL73W+LmUyI4c
KcM+1i2XMEuSdcJ1eB8uySw9vhDsgpeKbeZzmTjxcIM/daaSK4qH0yhGntiP
VUukzWoaN6woDnBT/s9Rd543Ges0u+FWuQZDXhcXDogF61XEumO5yPa1NqFD
aHXUJjvhlAfu7+AkZbpyoxJ/6f4q+suoLfv9nXoJDwY27ZYu77uM/IfEcsxJ
h5F+4WaBQPxf6C7N1N9nxoe/OhmbLl/wxOqDHmBozY+ZXTub19m9sFCIYJRj
EUD7dZJOiJcXHnyEdL1VAvhhk9vB870XWg37vFi8JIg/dU6Upil6o7vA/N47
rEJYT9rPMJXkjUTd6kflGiGUy1+T593wxms69O8M3YTRKPJLfIIFBf9Sddyd
zk7Gk6fiDY6do+DyliNNDCcZkUWZ9Ok8BWtzvamvcZFRNiU+QsSagrdT8pgs
D//nlkLloCZHCqpar5w+JE7GkbY7rnNeFIz++So5Q52MLvRqWrqxFHwu2L6a
7UVG+65v1Au3Keh2+qVLog8ZLeMSm+/GU5DsbzAR6kdGA87vKmOJFDSJpf3s
EERGaXKSrF8qBY9Nx2wLR5Hxl9b04fwCCmZ+ffat+OF/TmK4+0mviIJt334k
peeScfrNifTFRxRMXfDTiC0g44czdzlVn1DQ7tS1Eo8SMjY6EcwDlRRMlHib
L/2cjNWiM13+zyj4Wxfc+evJWDZ39xZvDQX1mL8psL0gY7bvDI1rHQWl1jr7
V16RMU0puYWlgYKkwT/5X9rImLRFBD9rpGBpn2XgYCcZY1pmVC2bKGit/+lM
22syhoUn/95ppmBXUbBsTS8Z/wcO3b7j
       "]]},
     Annotation[#, "Charting`Private`Tag$158336#4"]& ], 
    TagBox[
     {GrayLevel[1], AbsoluteThickness[1.6], Opacity[1.], 
      LineBox[CompressedData["
1:eJwVlXc01o8fxe0yEiIVynqyZ2Q9fd7vrKxERUgZSWZ4zG8ye5IRSSpKiMys
iDJChCgzIyk0VLYQkvHr98c999xzXv/dc+4Vsvc4fp6OhoZm5p/+72Xma7+n
CwcJqZtmNDJfAjWims8OmMY9gznnzKjGqzxE/IfwwL1xLXBfuyJQ+aoOMSP+
mDE6vxsaVXyqNcTticRvie0McQMQ+k1tZZzqS6inB98O8foEd4MO/62iv0rM
yTyVDcr/DJJDbY4s4glEI2tegnrKN8htzpb40JtC3Bl/sLQc+wNGN9UPl1Kz
COeWBKvykAkIHZT8apNZRJCzrtVSvKZBiWVdKpS+nIg8THAmKcxB7zhnDPtK
NeFVotrol/8LBod/PuoUayCs9h3wNRNZgCU/blYNnhZCO05GTCllEWgGOOhc
e98Ssutig1w8S3D+h7ZtfVU3wesmHPMrdhkEaMpvGlP7CJoh/kNdTH/AMbvy
xFzHIDGhzztbFLIKf966PinPGCbePed8GLvyF3IvP4UB+i9EjRjbCTevdZik
M5H+TTdGZN9hYjSc2ABRthtHa47/JF6Hhw4lKtBg7g93RaXlSYJcFaTEMEOD
O8x09BwWZ4knvy7FeufTos3jpCkJsXliv0TA9y+OdDjMSWa8Sl0k7tn6wnER
ehx6EDCty71MbE+iJL0cocd7xhUc3u//ENROj1/yKQxIcMQ2sb1bI/4wuRuk
WzDi+KHL2az0NHCRcMnczsOEBX1NP9sqaeFUoYPZTOwWjDnXfWU9nBHefrMr
OmOwFV9tRL/xvrsFkN9mSzsTM+779ndGop0ZJGMsKx+HsGCm3+1dp9PZIbXB
nIuPzIoi7VzHp9I4YMfqCdfoFVY8rfY8+igdF6w5GQs4e23D+kzu6D80POCV
buj3XoYdX6udttBJ3QnfB/Q6j0yw46921Vxlk13glPkQbylwIPWi3BXGRT4Q
BsHpthscOKl+unfsuwB8/JCaTDfDgTzKw4puc/vAlCtl3iufE93sLYQqRIWB
rWhPWt5WLpxLF1RbMBKBZv1kw8+OXDjYl9F3JUwU1MPuPDIR2YHjT9m/p3GI
wSI/j2lk2A7kc99CeewqDsXPb63XjezAkZ6sUpZeCRCdizeXS+HG/qO39V61
S8NwzHb6C6vcuNT0IibVRhaSxeKKUy14MMJ7q83bTTlgt4nZys6zE8Pd6SQ5
KxRguf1q1VQsLzadSqgfDFIGB2BR5VzkxcRFYuB38kHoKYkrV7bahe+LFxwL
6lSg6NbdkuD9u5Gp/5RhjLg68DPyy2Ze343vWONfMrhpQJRf+uOW+d24XFWz
UFVJBgfLvGyOuj04fv/w/RAfgJ42GVFlEh+mGm2PmPVEQHLpQ8sYPswzmLjL
LnMY+PZVp2Sc4kehurmcyXJN6Pn2NkFpTgAvPDu19RSbLqC5KYel+V4MccuR
fjanC0UtfbFBNXtxIWyVJD50BKLyhyObI/ehpXuCUGyDPgiqBkBBvCDGWifZ
3vl0FAY81YNrGwXR0DzQoWTRGOLy1mq6lgQRrNPoCGYTWNsTpv7bWgivEnSi
ZAVTGFiPUiYkhLHvykDWnscnIO6gkY+JtTAmqMTbRxw/Cdoe7GX2N4SxRKlo
5t76SSgdTZC/9lsYKQaHzL+fNYe4xvtSXS9FMMxTSlLgmCXorJ1x+bIogqNt
msrfua1gTUkwb1FMFLfHPH+UM2wFLtmP9u+OE8WLLw9ZagRbg05UoZC9FQkJ
2xnD6hkbWHvpYesTS8Lt5r+si1xsoXRVIS2inoSxu/b3C4/agqBbBf/j/fvR
Wnn5VXS3HawZ1/Euzu/HhVnjk6Md56CMu3tbRIw4Omv1fpxScYIaL75vytXi
OMfs65/Z5ASvOs5XjU2Io5CWaXGgmTP0R6466hhI4NCB5jfpgS6wsiZSz8As
iUhutpL+4gbEmB/lSoQUxlKPUj9t84Ijmi/1DlRIoXJe9LFSRy8wSWPd93VM
Cke6zGyf1XuBnWX6G00daZyzsRK0CqAAtb1VlI5BBt997E9TXfKGtnL+gdAw
WazKPXWATdYferguFMo/kUWukzU+Hff8YcjjyZXRUVmsfHtydWRrAExJ6Moj
ymHdBoSu/AyA7akeUZsbckjPUcWvXHkJJLU+C0CtPDpsEWCJvB8MRV5MzLz9
8jjldWpEZG8IHEiXWpyZlkffyXpvmYwQIK/7tqUKKGDN+s9SvVOhcPQZi//G
ZQV88z4j3sktDDyllLpeaChi87J/r3PVFRhWObIpcEIRWY3ejnAwUeGotpVs
sIsiHpLbZPM7TgXJM6HXiWRFJH8v1A+epsJY3Fu9uiVFVBo+mZUqHQFW8w4v
658cwIYxgYbRzkh4veE/J9j6L/MWzneLRYEKa8y+sNED2JXJxHsjNAq4RZ8E
Hd6uhHQfLmV5KkVDh9m6WoObEr4qoT75mRUDWpW3SxvFlNFHpcDQpSQOSpty
P4uAMhqUKyeE8twAwZ5qDqq5Mr4Y0DvhGXgDNiY+X9S+qoyhNYwds6Lx8Jxf
VqrpizJO/qgzjF6JB+nQ5szmBwfRwCO89/XTBNh5ZDmxdYcqGp/o9dWn3oH5
14YrojKqqFnJ01PbdgfaDdJPh+qqIpdzWmQj512gGusLq/ynikF0LqxBD+/C
vNn94kfDqnisJye6tiUJ2h2gLSRPDbn1xF5Myt0Havi1TWXQQA1FipGiWjrY
Mny0v2mhgVFSIbTD59NBI0K+ecpLA6fNR7UGE9JhPmrweuYjDbyy1cChbvof
f1NqDycLGZ98VakwyXkI5PROpaleMp6dWtKpkciEhRe8LhkuBB7V4/cxc8+G
FVP5ZKNwAq8HZc1UpGfD2pje66VkAp/7c+xx6M0GBvZL+w1bCdzDOaORQc6B
nWc/flkQA3xB+6SklCMXVDfST+uMAZa7UWWNWvIA9t3ev1iMuJ/EHXLPoxA0
nYWI1mrEY/xt7q0FhaBdVmiW2oKoUOn5QH+iEPSONFP1RhA7E/xdCMciMPFY
/pLCfhgtHartNuyKwb7OMk3H/TAGTgcYBz8tgas2e3fdldTEfpWcXOahUiAc
3rQ6q2hidnWF4whtGSw5BQSStTUxL9Ly8w/xMnCi9Ax/PqOJ3aqynjf9y8Dg
akSW9E1NzNHNyNfnfQrsj2cUG5Y1MYP2PZODbTkkLdUenX6lhfE0Uos/dj8H
k7+um3XdWqiXMS6tfeQ5MNPsfpIwrIXejef4+n2ewyVmb27VFS1cbA71vt/1
HM7wiw2FS2ljWXJNWFF0JQhr3nDalaCNjq0vbJiZq6Eg1uaKlo0O/s0LOiku
VwtWYfSnPrjq4Lb/TFc97Wthq2+OpFeADqrUxvyevV0L56xnu1Nv6uAUw4jK
zfVa2CMVIrjaqIM3W1L+2HfWQeTr1Bcl4rp4GxO68mrrwYF+eFlgXhcDxr1v
e4c1AN9/1m4rVD0knqWUalk3w7Dvl6yKeD3crNNsarzUDOkUpxGfFD1M9CQb
nEluBlE3n+O/yvSwY8iq4WN/M0jbXFed+KKHZwU52NhPtAChU8PwEfUx4dPa
ImHyGuw4+R/UreljGMc2OZqzbZCTN9Qe4WOI07aS5nted4CgXfhDzTBDtNCS
4T081wFJuyR8N2INcX3pltq1XZ0Qfc2P3y/HEE0mXZ55OXeC23lO1/MfDFGa
krPDlqkL5IWObNVGI5wj4YPMgi6oSirVpGU7ip+3FJRtZ+yBjmtRzwIzjVFV
fpvU/FgvRPd9ZCN1mKAP2ehYwcIH6GrqucyhdRyluk0fPBodhW9so/LFAydQ
ke+Q11H2MbjmJ/tQ3dQMr6eZFUU6jcPywUSz/ybMMSa2sScqZQZY+wf0yJct
MKZ4UEJm9zwU3bVemZy3xM+hZSwhPxdhb8nKpHHUaZRgyZZJlVoBgcm++6kM
Z9CkS3+D7PQXJi633XiYdha/W4sGNvJvQqGfsV3iblsEcSEeoQBalMH3Fh19
tlhAKuVVNqPHHeXu858f2uEnZu8Jeg9GPFwtMuFqa498p9xnBP234MsSPVpV
vnOYybsSUkRlxhzT/6o+jZ1D/pxbNds7Wf/9dFv3nwwHTD67MWdBw44udmIx
sx7nMVHRodhBhQNNZRfOiak5Is/JhfxLHpwYcn3kXt+iI4pIuaVN3uVC7jsD
3mfqL6Acc/FC1fAOnJOfyz8d7IQv302o23Lz4N5qf9oUVWe8Ef5vEI/sxLI5
ltVyOhfsy/0jfjGZF288qzXRrXNB4YaKwM6BXdgjEaxfEuOKdhUWPwyV9qC1
zNn0eAM3nEhPJkdf5kNVwcKdZYzuyHRev7+2nh8Da7fIFXe5485K0Yoe4b3I
OBOeJRR3EUO0Og1NPfbh0mvmWvfTHqh6nka53U0QU1o3V4O4PDHD9VXMtX1C
aLfMohvq6YmW0lF7F5uFcHCVz96j3xN7jx3UlAwSxt+6hwqTlb2Qe2BOvE9M
BKtYdm4dS/BCPzrB3OROEVR8tHhAYMULk/xGW7dHiKJxxNe4eHMKxsUtjBfK
k/CIQZzRQQsKVqYP++YeICGyq7F8tKTgIY7MLZkHSahwJ+6q2BkK/muGnEQm
IXe22uXacxRkmBSbCtcj4VDTDecpTwqKOZ89Y2lLQidGsrZeDAXpu565ssST
0K71O+3MdQrKCTXmM94ioVXszbpbcRTM/y0yS3OHhEY8P9RHblJw8UL/teX7
JJQjJSj4JVGwzjt25VsOCZe0f+59lEXBfW1v3tXXkXB2662P+jkUPN5j6ljT
QMKfbw/dm82loLv6zPqzJhIOnrzFo1FAwZQ3FuTiNySscSDYekopWKN1/feD
ARKWi4+3+j+lYPDmyZLkDyQsmrp1TaCCgvHSPJ63P5Ew3WeczrmSgnQPXDeu
fyVhsmpiPXs1BUVj/ryN/E7ChDUi+GkNBWcuXEynjpMwun5cw6qWgoGZLQGh
UyS8Qk38s1lHwYMCNOaXZ0n4P99Jy5s=
       "]]},
     Annotation[#, "Charting`Private`Tag$158336#5"]& ]}, {}, {}},
  AspectRatio->NCache[GoldenRatio^(-1), 0.6180339887498948],
  Axes->{True, True},
  AxesLabel->{None, None},
  AxesOrigin->{0, 0},
  BaseStyle->{FontFamily -> "Arial"},
  DisplayFunction->Identity,
  Frame->{{False, False}, {False, False}},
  FrameLabel->{{None, None}, {None, None}},
  FrameTicks->{{Automatic, 
     Charting`ScaledFrameTicks[{Identity, Identity}]}, {Automatic, 
     Charting`ScaledFrameTicks[{Identity, Identity}]}},
  GridLines->{None, None},
  GridLinesStyle->Directive[
    GrayLevel[0.5, 0.4]],
  ImagePadding->All,
  ImageSize->{587., Automatic},
  Method->{
   "DefaultBoundaryStyle" -> Automatic, "DefaultMeshStyle" -> 
    AbsolutePointSize[6], "ScalingFunctions" -> None, 
    "CoordinatesToolOptions" -> {"DisplayFunction" -> ({
        (Identity[#]& )[
         Part[#, 1]], 
        (Identity[#]& )[
         Part[#, 2]]}& ), "CopiedValueFunction" -> ({
        (Identity[#]& )[
         Part[#, 1]], 
        (Identity[#]& )[
         Part[#, 2]]}& )}},
  PlotRange->{{0, 300}, {-10.734111417967226`, 10.977333952313268`}},
  PlotRangeClipping->True,
  PlotRangePadding->{{
     Scaled[0.02], 
     Scaled[0.02]}, {
     Scaled[0.05], 
     Scaled[0.05]}},
  Ticks->{Automatic, Automatic}]], "Output",
 CellChangeTimes->{
  3.725790454653599*^9, 3.725790514460441*^9, 3.725790551700067*^9, 
   3.725790631266589*^9, 3.7403738145650263`*^9, 3.741166057760421*^9, 
   3.7411663256639023`*^9, 3.741166397999399*^9, 3.741166542593484*^9, 
   3.7411665895018*^9, 3.741166622965687*^9, 3.741166683533572*^9, 
   3.741320237523958*^9, 3.741320293440097*^9, {3.741321097461681*^9, 
   3.741321134912211*^9}, 3.741336059540638*^9},
 ExpressionUUID -> 
 "28c849dd-dc63-4cf6-b631-ee4b180affa0",ImageCache->GraphicsData[\
"CompressedBitmap", "\<\
eJztfQd8W9XZt8ieEEYpUCirbMpqS0tfGijQBgh0sNMPUlJWAoQZJ4QQyA6Z
ZCce8Y73lveQpzwkL1mSJe9tx3a894j/3znnnnslJbavlPb93vb3vc5PN7bu
fdY5z77PlV5ctW71e2tXrVvzzqpbln2x6rPVa9758pY/fvoFeWvmZQrFjOUK
xWXv3KKgv0OhEA/Xo6ysTDET77//Pv2N/QX2Gz08zP5W/O9F/z9cJFzzP8DJ
vfzE2e3b0fHBB5YTs+wE7F+6FGPXXec44NCDD2L47rsdBxy55RYMPPqo44C4
7LJLY5UCDj7yiP2A9/ATFfn5ILaOznfeEU7MthOwOiWFAbZ//rkN4EL23wKY
iqKwZcNBpOvLOIJS5EefxI5NG7Fx42bs8UqGzsT5nIZObVgYo3N227ZJ6Cy8
iI5JG4JtG/YgosAEs1EN3283YF+CDmaGTYZYg4cHI9Z8+LANMQZpRlHsbmwg
8s7E5+y4bnsANKUCnhmT8mNGYfRWrN+ThBKz8Hd+yLdYvy8Venv4aT50iPHT
4Olph/ClyPXahK+d1TAKyFCSsgvrtkShyMSJzZas+C7RrLZsYSRqw8P/CRJK
FJntkKf9s88YserUVBti89l/i1FmNiA3JR6x4a7Y6GS1iMqtcNqdAB1bRBO0
QZuxfr+di9j5j38wohVFRZMTNemQ4ncCezd/hg+/sGiSOT8U25x2IijPCFNJ
Gtw3OdmvSd0vv4yJmTMtJy4wD7M+Fce3HLIxD220M3ZsXIcv123CHs9EuqSy
5tH3hz9g/MorL6Ija7+Dv/oVRm691XHAkdtuw+AvfuE44PhVVzF2HQYEWcfu
V16xH/BufqJSoxGc27vvCifm2AlYk5jIANvWr3cMsC4oSPBWu3Y5Btjo7MwA
m44fdwyw5fvvGWC9v79jgG0bNzLAmri4iwEt0V68vOPDD9nlldnZjtHpfv11
BlhWWuoYYO+yZRi/4grLCXsBB379a4zcfLPjgMN33cWCvsOAY9dei/4nnnAc
cGLOHPT89a/2A4puu6K4WFDtt98WTsy1E7BapRLi9qefOgZYd2Egthew4fRp
QbWPHHEMsGXvXiH6+fg4BiipdnS0Y4A0v2RKrlY7BkjdEwUsF5XcGnDmRUG3
7+mnMb5kiQWPvXSGHnqIZZcOA44Se6DADgOeX7wYfc88Yz/gnfxEucHAlqT7
1VeFE/PsBKxSqxlgx5o1jgHWKpWC1960yTFAkl4Jad/Bg44BtuzbZ6uh9gK2
ffWVoKHx8Y4BdlBNohqam+sYoJSQmEyOAfY/+STGrrnGcsJewKH778fwvfdO
DmixCfFyWvf0P/6443QmZs9Gz0sv2Q94Bz9B1lBQNDE9mG8nYE1srKBoGzc6
Btjg5SUo2v79jgESzbQtBOwFbPv6a0HRYmIcA+x47z1B0XJyHAPsoYo2a5bl
hL2A/b/7HQukjgHOwNB997E/F9hJZ+xHP7IN1nJ0fsZPkAxGyEVffllhF0UR
UPRo5z76yDHAutBQBti6ZcvFgBYTEi9vPHlSiLQnTjhGh8R0BlgXEuIY4LmP
P2aAVRkZjgF2v/YaMGOGJWDaC0h3ju6gdMJewOF77mEuyWHA8auvZgHbbsDb
+QkpAr7xhnBioZ2ApDwW9OWTTxwDrPfzY4Atu3c7Bth84ICtf+GAQvZNklIz
qZF99mPzhnVwWr8Ju0/HoqB06vJUxNvm5CS4n4QEG7yXs/+oozahKPp7OH3n
jdQiE8ylGkTs24DtQVqYqIrL4O96800h7youtsE/WzTZi7o2C627Nux8SVos
4nMMtK5n7xnSf8CG70KRP11HQ2SApkY2RQpn4Gp+Xq/aB6fNwdDag4xFzHvu
uQiZgH4uDGpX7N3vhaQCI0y6dPhtW4dvfXNRymW1au/cKiovidz9v//9FCjn
oDTXC5u+3IIdmzdg3frN2O2qhMZonnJjb7PW7csuQ/eKFcKJRdZ4CTMlSdj9
9UGk6injMsiqk5OFmuSzzyZBRsBLc+G58SOsXrMGa9jrU2xTFk7fiRGR1/v4
CDaxZ48N8iltQgRs2b9fsAlvb8cA29etE5Q+MdExQEmbS0ocA+x76inWXpFO
2At4kVO0F5DqPC3Q7QYUFbKisNC24bzYTkBSzAmxcPNmxwAbXV0ZIImOjgG2
iq3RyMiLAWdeZGokjRQyJq3WMTp9ZB3PL1pkOWEvIL05MUyyH4cBWVFn3YqT
A7yFn5A6av/4h3DicjsBSWZhm8nYCyhlvu7ujgFKveaUFMcApQRWTE3sBWQt
Vevi3F5AVvpYZ6RygDfzE+U6HfPCxHEIJ66wE1Aypm++cQxQTDEbXVwcA7yo
4rUGtBiTeDntGtJytdxodIzO4C9/yZod0gl7AWmaZ7MJcoA/FW1CqxVsYtUq
4cQSOwHrAgKEjppoE/YCio2xel9fxwA7Vq+2beLaC0idhY2LsheQ3mIYeuAB
+wFvslZtofEvnLjSTsDa8HDbLpC9gFK7UfQ09gKKpXKV2DW0F5C2VmzCtr2A
ozfcgIHf/GZyQIsx3cgvZzGXuInOlSuFy6+SoSMCSrczdu50DFAqKIOCHAPs
+tvfWF1YISb09gIOPvywrfOVA/wJP1FmMuH8woXoffZZ4cTVdgIST2abtdoL
KCaWkg+1F1DMMCRFsxeQ6orNXIEc4A3i4pSW4vyCBdT+hRPX2AlIciZhcZyc
HAM8u3WrbdZtLyBtcFKHId3mtQa02IR4+cgdd2D4zjsteKah8zI7LpqqCsYU
sw1/YmBL7B2FmOr9Fxiaqy5G4xg3zKyIN10mbm2ZAVmnnLBm9RryFymrFIvx
6dYoFJoc4k7xrBy+UofYVDzPxS0zahBxchc2b9yA9eu/xrYTocg1mB1dvZlT
b6vQMqa51tRNCMPU4yQvMvAr7Z5AKZ1mMmX5pHvsOFsTtNDdtUvYY1rEm6FL
2IevdoZCK67F4kvicAqUM/65NRSU5xoGXhCxHU47g5FrJJtcmo/oH9bjG88c
6B3ndoY9mz515ycjcsqZnck3feoxn9xpxn8m33TH2RqiVU5SkrCWV7O1izry
NTZ874UErZGjuTQW5XBewgoqLHtuRK7/SZxO0UnwupSdWLclGuooh3mdZs9f
Z8f5vBkXgESPqcekJt/gqeaewpE8Da7lnBcrXLwzKc9Lx4+usbhCsx5ZYSex
fR3RcP8M6M2XxM9zDN3sSdAJhm3vEr3A45q5VIvoIxuw0TkdmY6zM82Gvcwd
1eQNTzXU0wyhObaBEUjxnBrX8ilcvKN8NS1bJq2aqUQFr21O2OafjWzHeVp+
ERoNShxfJkm1yMpo/Lfj8zUf4JMt3sgyGC9lpezYy8k7zaZpZ/uWi+7HwbnA
3GlwPjctzjKH+WzYuNHKpZHgmHQcB93VMPBV0qfux4YtYciIcpjXZbJow6HJ
dnhZrbk1apKRlKWnN1tgNuQilKjUTmUBChxfWVkdsL0rICQjc6cds5T238ER
zdJpcD7HPd1UOB3hsTYsTNInIzHCjesPQZlfCrO5CImnNmDDkVSUXAKPz3Ie
p8Kpd3AdRR51yfuI0vgjm+TRZkM2Qoij+C40H8ZL4FF2uxdNc99m0mFXsV6y
czZ2qvdf4E77IjSOccMmZZ6TIrAB6tAj2LbRCU7r1mPzAV+k6kyOsiaLzjEW
JSdOsjOl8w58te5LfPm5E747Esi22EHupimVWIXMDv9mz6lcy09U0hEL6xaX
0OxQXMfPJ0TEMuCAUx6Khew4E34nPOB30p2+FAvYkbx30gOBrr70RXIiepyN
MM9ARPqFSa/owEhyZVpCGjlmqTIlhs5xWuJIbsPp0za8XC5IxToR5PAEPVg4
TIlJZqcoH3PpcT5nk7PN/prN3wty9UKIqw99ETbpkbDp7guld5D0othnITFY
SY6ZyhRkRavYKy8hawYKVXkzYM4zElKVBeWoN9Sh0dSAc3Xn0FF/jtEc7htW
XAHyQ44j/SPsvbMVLagqqiAJkA6aRDXSI5OQEBiFCK8AxhNdTv+TnghyO4OY
YCW0ORrpXrz13l3xT7y35H8Udq71e+xVrtcLPbKnn+bj/f+Jcv2/359pxmgc
Q/tjmy0x6A3UNpk9UWsNdvdHoIsPV013YkCezHQiPP0R5x+O1PB4qGPTqEUw
PFWFFWgua0J3SzdVexKFqQkswujAKLqautBY2gATKXk1CWp2fcyZUAS7ehNv
4s7oULUvyi/6z9WEizW80c1NGiv6z5Xr30rDhSTlcqTGqRDuHQx/Z28Wj6ij
Dz3ty7SKaibVMqO6BHUlNehs6MTY0BjFM4cp5QL0n+tnPrlMY0JufCbigyIQ
6uELv1OnCUovRAdHkmRR//wkHKyYYrPp4wi0VUwHP1+ZEs72vTccE15AsZC9
R4IpApyFyBHi5oNYYrI0qujSC1BdVEmE7sD4yDiJIlTi+Tg/dh5djZ3MTPMS
sxBPJAxy94YvkTjY2x8ajUbx1JQ059iIyzz3okX09sir/z2SvsuO85lDCvEI
YFsc5OLFpKROpzRHj5byZgz3DpMoLUg4MTGBnpYeFmfzSIyND4wQHAxZoXDf
UBhKDApnTqvp2DHhBt2OHdZ3QyblZS07zkNmcgaCSXwOIKlOBOEpPSIR+sxi
pkejg6MCG/MwPjqOtupW6LOKkRwWixCilb6n3BEZHAaDyXCEU+h9/nk2gV1J
1l2OAyeucqqwZASd8CUvL8T4hCIvLpPtdV97H1+FuUzRm8yNKErTIiE4Cv6u
Hjhz2hNZ6izFPo67oqgI5+fPpwNu1ve7JqX9Daedk5KNYGeS4JEsJcY3BLmE
do2umloSgRBo0x3oIHqnVxcjMTQaAW6e8DntjrS0NMVOjvvszp3CKLf4VMs0
tLdz3UuLS4U/kTnUzRcZkcnMagldQeQ5TK2NOSVICouBnyuJVl4+KC4p/o5j
pA/d0bvF5QaDLMU9nGKqUoXA414II/udGZGMCq2ZUpzJKRLDQoOxHuq4NIR6
+cLH+TSSk5M2cow1MTFCUi1ONtw4NcUfOMXkoCQEHCOexysY+Yk5JJQ2U5sV
KM5myaUusxAx/qGEmhuilUrFOo5OnAmW5uamIXeMkyvSFCH0lD9CTvogNTQe
ZXmlGOwaFMnRgF2cUYAov2B4ubgiNjFG8YmoPVqtoD1Ll1rfXZ+UnAs7zkas
jxJBx72REhSD8jwThnqGFJJoRGPyU/MQcSYAHq7OSMpIUqzhuNrWrxdu+bq5
ydJy56KZSk2I9VQi5DgRLTgOlfnlNCefwffu/Ph5NJobkBaThDPup+Hj7wV9
uf4dBj2LDWjSOemR229nt7gvJMpo+nBSpfpSxLpFIYwYZXZkKlrIpk2cn5jB
JaNRpkRdhIiAILi5n0BCboLi76Id8CE5abzyp1NLFsBXMT9Zi9AjZ5DgFQGT
Wk83TCGJNSaIpYpOgKeHMwKi/VBaVrpCFKukBGPXX4/RG2+ks+NyFEOs1jLB
RYnI437IjUoXBJyQBGyraUNGggqeXqfgGeaC4vJihRgRxGnOFvGZjZunJhfJ
BcxT5iL8hzNIC4hHna6GCqWYYaWS2aRq9PZ1gXPgMeSV5yj+wqWjT6TQ2Tw2
1Gc2y5GL4eSK04sReTAAyV5KVOaVUS8ukett60Vumhpefs5wDjkCbYWGJx+W
RzMbvLysB9ImpZXAaRkLjYj9IRyJbhEoyzbStFii1d3cTQridLifOQGXqKMo
qChQiLeb6+mwEzFuEi+sZxEnpZXCaRm0BsQcCEOKhxI1+RUsDxBpnSOOJC0p
Ba6+x+CScJRt2VOikhQXs1mQ8csvR1Vmphy5dE6uKLMEMfvDkeYTj3pdLbUw
iVxTeRNiYiJx1HcPAjReVCUVS8VlXLHCdur+tqlpqTmL2qRixOwLR3agCu1V
bSIZGvUMWj38Qj3wQ+B2JJhjFL/laIiFMTK9zz0nkLl9ajJ5nEzmGQ3iDkVA
n1hArUxSitZeZKal4ZT/QZyK/h5F5YWKX3EQOvMzMW8ehu+4AxUFBXKU8tlx
IYwGYmFHUqFyjUNtfhWzY/pDY2mtsRZhUf445P0NYvK8FA9zUvSBPRrR6Kua
PnJdJj51MSmpYnHt0o2I258ATWg2upu6rb1UVnoGTp3ZRTR9HfJL0hT3i5Si
otgoPDUu9okSZeLzQJNSMnChEj1J7uOsQnVepSQQ9buVJZXwjzyNA54fITJh
B8ylBsVdnFTj6dOMDH2x5zHKxEfVJiVl4mCaLBOUR3KhjdCi92yv6A5pFZqk
ischny9x2mMFDLEB1DPcylWWusCONWvY4Asd8CFyCrpx14Wuvpy9sRgmkxlx
PtQbZhObqmHi0B9a3mpztHAO3o6DR59B7sEPURsdzbqgN3JqdJSeToxTLaQP
WUtzSHdPLV81p5uTYkbECR10iaUY6RsRdOP8BKoN1fCNccbew08j5vMH0fTl
WvY8ZkV+vuJa7r0bCF06mknp0mVt27RJimn3TE26ji+trsCMSOdSZIQYib70
zOC1E/UgUSnh2Ov5Fnz+Pg8tD95Eh8DoJ5qg6eRJppFkfYWhx3msWKj39WXP
CNOnyykzE3Pnouutt4QHvMhl903NTCM7XiWtf7yHAfUlLcw+6A+xTqRlpmJv
4Foc+Zz4rdsUAolZszB6000YeOwx9Lz4Ip2bx7m1a1lcIltCp5y7Vq5ks/h0
nIlcTn0W+8gSOuLU/sUXlmnPn0/N3ll2XISMGDOiTpbClFUraTxt/uWqc7E7
Zis2+fwWGavuw8hPbqBeYi4jNZs9DkCDFp2dphNc1WIK99DUJNu5kWnSy0hc
NqEooZJpIf2hiakuT4e9CQfwnv5juFWfgDlLpWDPipBjVVYW2xCKgdH55dR0
OjmdIg1RgxMm5ISXY6BzUDLmssIy/JBwGCtL3sPh5sMoruCjh7+eGmcPx1lq
KIfSxYQMvzJitX2SVleQ2u1o0jGsKFmF3S27kVeZJ8tnv4jTaIbSzYT0M+Xo
buyBgBSoLqnGsaTjeE33f/Bt67dIr0pXyPXIh6xwxribkeZdga56C85afS1O
JZ3CX4tfg1ObE5KrkwWcD0yNc5SbFdXkGA8TVJ4V6KiV3HCdoQ4nkk7gBcNf
8GX7l0is5qowjXFMsOMCxHmboXJn6CQWq3RVOJR8CM+UPYdP2z9FfE28nM9h
5y/jootspntVkuXslbbITLzCvpR9WFr1FD459wliavgTstPEBXZ+1gX7lHWm
Cn2t/ZI+0axlu2o7ftPwX1h7bi3iauJk0wJ2fq5VKI1yNiMnsBoDHYKijg2P
oSC7AOvT1+ORtkfYSiTUJFyckVomHRdwdIaSMmLSJuSH1xFTFuyLeuD09HS8
r34f93f/HJ+3f27ZqGnKLnZ+MUdcQFLNqBNmGJIaMT4q+Ir+9n7EqmLxav6r
uL//fmxo24DMqkwB8HoZxEs44pxUsmUny1Gd2wruHlnzK0AVgKXlT+DRgUex
9exWi1VdK4NYfBovVVmOBNdKtJR2SgVHnbEOh9MO487mO7G0fyn2tOyhiatd
Y7LXcoYTAsuJaVWjp6lPUoPiXB2+yvwK1/Zeiz/2/ZG5Fl25zr4p+Ou4OzYy
HSuDJqxOiprDPcNQpafizbw3sXh0MV7seRHOjc4wlhuttkduKHgRCkk9GUVW
2ZjcRBgWlrmroQuBSUFYaliKJeNLsKJrBfzq/WAuM1vplPzYf7aqHLHOFagv
arcsdEkDDqQcwE9bfoobxm7A+x3vI6o2isHJPbJ/K1/opJAKpHrRhe6X4kRB
VjHWZqzF/MH5uGP4DnzR/gVU1SoBUO6jgm63XujTFdCShR4dHBN0+dwAYpLi
sbxoOS6buAyPDD7CnHl+RT6DneYOuFXWtwj5uWWIPlWOiqyzkjq3mFvhmnga
dzXehXkT8/B87/M42XiSbuKEDNp7+FqkRpcjkShze1U3V7oJlGSVMhexcHAh
rhy/Em92vYmAugDFuAzO+zirZnMZYjzLkBtcK+nbIHFBcXEqLNe9AAX5d/Po
zfj43MfUX4zIoH2AnyjU0BWoIHl0G1eHuWjQNeO40pWpA0X78NDD2Ny6mRn1
oAzehzm7yREVSPG0qMPY8DiprPT4TPUl5gzPwayJWXi672kcbTpKeyN9k/rJ
X1ygAsVxTZI762nuRVhIPJbqn2BMXjF+BVZ0r6Br2iPD46McbW5mBWJcq9Bk
6JRimjmjGvvCj2FJ9xKG9qejP8Wn5z5FUnVSpwzaxzjaOP9KqAPrMNQ9LO1S
SmgeVqjfgmJCgcvIv18N/grbzm6jCtsug/a/+IlikrgoiVJVZLfynZqHhsKz
cPMPwt0N9zBuqb6+0PsCXBpdaB18Vgb1Us6xKqYKKd41JE8aECoOYmY5EQY4
xWzB7LHZDPW1Y9fivY73aMxslkH7JPt1HkpLCcce1ShJbJHcWJu5A4HeSXim
dNkMipfAPzD0AFMvTaVG0SCDWnjWfzEyVZWIda1GW2WPpF6FUeXYGXwM1/Vf
xzieMzEHz/Y+Ky6GolYG9x84bpOJBE+vKmgiGhhe+nOusguRp9V4S/sOw3vB
ivBaamrcz/IlycmiKleNFlOX4BmINpdEV+Oolx8e6XhEXBJqcVw9FBUyqJdz
tmP8qpAT1iD5yC6SqcU6F+CL9K8Zq6J+0KDk0eABU5lJYZbB/SLHXaAlbLtV
o1EvWAqtP/TRNTjtosTy1uXSktDg8eG5D6m1KEoF3Jf6OQV/4aTjg2uQG95o
I1Y8qVa3knh139B9jKxoUTQEFFUUKYTq45/+KANxIL1AW4mY0zVoNnVbNk1Z
A98TqXiv8X38aOxHjI0F5xfgpZ6X4FvvS8Ny8YVcTPuBBlNy8SpfiLjAGmii
miSV7KzpRsIxA44kejBPSj2qtcdKrUpVFAosTPmRB5ZPJXiVy6rJq0KsRy3O
lvdIshZHVCPoSDY2NG7AbSO3MSozyL/fDvwW+1v209xJa73ZdnwcwmSCruAs
0EgXG1CLgthmydtTtxH7gx6eycF4vft1LD6/mLFB/6eZUFhdWJ6tvjn68Qlv
cuq56mrEe9aio75P8oVa/3KEHs7FrvpdTM+ovlHqdw7fiY1tG6nnyrambueH
LKxkv15B/CSJwb61KEk5y+of+tNU1ArlPh0iVfH4oOMDyYIvdGqZtgt/SZ/H
sIqLnqWqQbJPPQkDg1I6qyb1mfK4Bi71LljWu0zSsuvHrhctPV3GibzDxTQa
STjwqiVa2CqJWZXegMjvi6DKzmArSVdUtOhHBx8V1UuhkqHxPhchObaaiNBA
ijMh9va19CHlmB6J7vkIqgu6SHdoFhZWG5Ysg341F0Gnq0SEWy2q8zuEhIFE
NX1UFcK/z4c2Px/ft3xvoyDUQdGGAPXjCTI0PuI0YoLrkBVicXjtZR2I21+M
jJBCGmpYyLlm/BrJn/+p50+ix1HEytBYy2nk5VaS4sVi5aOk+MzzJrXtAS30
Rj1ONJ3AE/1PYCb5JyaW69rXsXoxWobGp+zXJUyrI33qUJRg0eqarAZE7MxH
vkpHcTE/Rf0VpSFmhLRgIpodKUPmCy5KekotknwbSUkwZNnxozokuGhgMptY
qKMpkXXUpopL+ynhMjTWcVF0Oqq5DagptAp/4RUI36mBXqun9o9NbZsk7RWd
46HmQzS5DZEhs4GLEh9Zj5yoFsnDtxrbEb27AFlhrJWPwLpAvNr9KoszlAwt
A9/ufBvRNdGKIBkaG9mvC4l/r0YcWa6O+n6LjbsZEHMoDyajiYZP7Di7Aw8N
PaSwzkZ2texiodXfio4lUd9ktefRAU0ozTonZdQVZIMiyUIVZ5YwlpS1Sqzs
XMkSdtEMqVkSF35GRohvOZnU5Hqkh7ZguG9UygkSDxYh1ZvFIbrm2N+8H78e
+LVkivcM3yOaorcMmS2cTFERiYVnmtFSKYSCcbIvBX7EH+7Ng7HYyICI/2MW
KeYA1CL/0vMXnKk/4ylDZhv79UqWb8aGNaFY1S4ZSkNeE6J2aKFNLGBAtINw
vOm4jVHSUEybONmV2YrTMrR2clqZ6XVICWrBQNeIZC2qw0VIdM6B2cTSQaRV
pbG2G03mxJBDi2DPBk/mZFxkaO3mtHS6KijJ8jUYrVKJIDPCt6tZJ44CkSQU
bo1uWNZnCS3U2Ti1OzG5TsnQEqYp5gnVcXgztAltUqnRqG2GcnsucsI1M/hl
6ko182PWPodGU54PH5ehtp9LlpVZhwT/FvS1C1FmoG0AaYeJez6UxYyIAtG+
jFeDF5b3WtJjSpY2XtVVasVRGVoHOcs05ESeaUF1sVXyGUJWcUsWSnJLRMlI
bc4CqJifUclob4suLpHskAy1Q1brGB3ehLzYNin3ason67gthxQXGvGJBtp4
olpOtZ3l/aM3MF9O48NBGVJHOSm6iPF+Z9HbJjju/rP9SD1UgPgjWSRDN4uC
aSu12NS6ifWPKCmq/U/1PYVTjadomNgnQ+241TJGXLCMukATwreyZRQFC6gP
wF97/ioJdt3Ydfjo3Ecsmd4jQ+qk9RpGNCE3tl1aw0YNsect2ciJ5GtIBKvQ
4pvWbyTBaNCg5k3NvLS8dJcMNReOJpMsY5xfK1lGnvE0k/i3Px+Jx7LobIW1
YLQ2EQVjYbDjQ9aO2yFDys1aFQmpOkOvxR96G4gqpkOv0YuC0SYcreeto+Hv
+n+HY03HqB/bOmkEcbdZvBbi+M5Zsoa0OoRvyoQmWjtLFKcuAC/3vIz5E/MZ
Dep+V3esRkp1iuI7GXG8OKnU1HokBrVjsIdHkeouJOzMRdKxDMvKCeLQwHH3
8N2SOI/3P44jTUeoON/IUPPhaAoLqxHl346WKqHHQnt4uc5FCN+cQr2hKBhN
Ul/uJoKdFwS7Zuwalv/TdOVrGVJnOKnS0nJEhbaiJEtoMtB1LIupQNj6VGhj
+RoKgm1p3cIio7VgtCVHBNsgQy2Ao0lKakJqZAdGh3jWom9F9DeZULlm0pAi
ChZcF2wjmPWOOcmQChKdXF4togM70NEsuIyB9gFkHNQgapsKxiKjtWDftX53
0Y5xwb6QoRbC0ej1FYgMOYeKwl6L5w0wInRdMgpTCmdPsWPUstZ0rGGW9ZkM
qXCOIyb6LNRxnZK7qM9uQDjZrQzvLP6QhkUP7xq+S5KK3hXh/mKtDKlIyV/U
Iy64A30dQgbQXUdyp21qxO1R0WEzUSqaa14oFU2bqSP8SIaUkpMqKiI+N6gD
DWUDlirDuRBhGxKhU+tmX7Bd1nr4ZP+TONl0knr41TLUYjga1raLaENRRrfQ
yyev8tgKhH6ejJzQnDlWevhK9ytSEk09PO2Zk6xH8b4MqXhOKjm5CaqoTowM
WlQ+5us0JB9V0dBlLdiWs1tw7/C9ltDVL4Wud2SoJVppvTK4E50tw5LWp+/N
ReQ38dRziIKF1IXYVAe0Qqc3OTOqMhSrZEglW6l8REgHKootN3GKvEsQ8kk8
tHHaOVMYmBiTaelGko2Vk3p4oYSfL6Rq0W3ITe6RPHy1qgZhnyQizT2NnDcr
RJmoFlqHY5qSinnGmzIypXNmVapGJIR3Y7BXqKc7KjoQuzEVsTsSaBYvysTy
DFLD/WzkZ5JMz/Q9A9dGVyrTChlqmdJmVSMiuButdYKLGuoaQtbBXIR8GoOi
tKK5XDBSHuDF3helzPAnoz9hd3ppZvi6DCm11WaFhnTCqO23VKX+BgStjoY6
UD2XX5ZbmYv1betxy8gtUmZIOzk05yVJ6isy1HKsti0qqg1ZiX0YHxO2rT6r
HmEfxiP5cDLVe4W4lmLu+1zvc7ZZfZsTcipzXpIhqeFoMjKIq4roxUCPsHOd
VZ2I25CCyI3RVPHFtaRJPb2zeOPojVK9Qit+n3ofPr45Nal8TqqgoBqRYT1o
rhmWtk19IAeBH0QgPz5fXEuxXPlD3x8wc0Iow24fuZ0pDlGgF2WoFfK1NBrL
ERnZCUP+gM3OBayKRLpHOjMBUTraJrGuxqgpUJMgpsEfwp6ano6zHRt7FplJ
/Tb7FvJeNOJ3x1OfL0pHfBLzTdRHiUUmNXGaJBRUFDwrQ01vtW2xkf1k28Yt
2+aUjLAvIqHL1s3jgtEykzreH4/9WOqev9b9Gm3HKf4oQ8potW0RYb1ost62
/dnwXxUGjVIzz0owGk1oek2jCyX386GfY+fZnXSm6GkZaiarbQsP74I+f8hq
2/TwezMMqS6pbNtE6VKrU1l+LfZtaZfjb11/o7fVFb+XoVfO2Y6ObkV60qC0
bXUk1Q95R4nYbbHUc4nS0d4ATW0eH3hcku6hoYfY3RBduW6pDLVKyU82QBkx
iH6rbYv9MhEhH4ejOLN4PheMNjze7XgXV49fzShdfv5yvNX1FmtCPS5DqtrK
SYYE96GlXsi8hzqJk9yjxpk3g0mVmTNfdHDlehxsPsiGSsQ2Dr3Tv7dlLxXs
sUnDTC3fLL2+HCEh3TAUDUuhTOejg8+rwVCdUNHUVCHKRNuqf+/8u9SSov/T
v+mdvWlGzRi9eiv/GEHSj4yUYUtYS65G0JvhUG5W0vxUIQpGmGetYtpYs+52
H2g+QIWeZhKNkWziaJKSGhEdNYTBfiFrbC9th/KjWAR9EEJjzQIuHZ3koKon
9r2vGr8K73a+i8SaRMUjMqRaOKmcnBoSawbQ1swHMFr7kbY1Hb6vByA7OHsB
v4x2D6lRUeMSBXts4DEcaWa10oMy1Fr5WtJCMySkB2aDoB909jrfOR9ef/ZD
8pFkWp0pROmIu2BuQ0x7xIKJ1hXTTFUyeu38BG1bhoV1QJ0+ophBk0c6qR5d
jjMvBSFqYxQMBQZRwsKKQpbTWSerNAvnyeq9MhQ7JY/cgriYYYwMCVvXUtSC
8H9EIfCdQFpbLOTCsdqClLnW7Qgxp5ObsuvmpNJI9RwaMoTONsGue5t6kfRV
Mrxf8oU6QL2QX0bbEbTPcmH+wxtIcqN3vXzrNJoqBAb2obp8TCpz847kwWOZ
N5IOJbE0QZSOBGib1vxNozex9hht/E0z187o9VuZeWBgFzTZgqrQ5p8xyAjP
Z30RsT6Cbp1CFJGkHiwFoakIpTd7YjZrbHo3eNOUZZpHLBjJQStLDyXldUL8
CMZGLRE16I0QBLwdgILkAokkzYTcG9xt+pu3jtyKr9q+oncN+PMx/6pvZhzh
VBMSGok+D6Ov57yU8kZ/GAOvP3nRLV/E1z+rKguftX/GuneUsbkTc/Hnnj/D
v96fD5b/a7/LcYwvYGZmDYKCBtFYJ2jkwLlBZOzMgOuTpy/QESHjomWFdU5C
O2a8lX/9dGxe4lc8nuds0vI1IKAHep3AJpsxcSuE21J3RH4VyVRLXEqazNA+
oRjuadlMq0yazPx4Oh7t+GbIyXgE55G2eoKDzyFNNYbz58EKX+q5fJ8/A/+3
/VGUWqQQx+RLy0tZD462QqyzIDpoQtzaNZfCptW3S1pmCayGfOdBqWwmr1EM
D01Ini5sZTg8XvBAdlD2Yr6AqVWprGsi3tmk7vyN7jcQURuh4J8X+9/yVZRW
o4jzSQpE8uKQYXS0C3bTXd+DxHWJcHncRYo74moayg0sObG+x/Tw4MPY17KP
xvcrLuD5X/lNllYjyfORm1tFtLQfleUCz8M9I1DvU8P5Ny5QblLCUGhQiItM
B7TpzSoxd6MZwcqulWzAerGtK/pnvwWTHeZzHktKygmPXdBqxm0S59O/c2cR
jyQrEo/s3l3Lfpvb6IvOL6I3JRVy35nCDgs5UdoPCg1tR3LSOMYFuqhR1cDv
RX+mfDkhOXw2ZxZbmCf7nmQESf5iF53LOZ3Y2CZSFYygr5dPuNEs7H0lTv32
FJKPJrNEczHHRKeXaUgQ1tgOIks4kbS0WhLmBtHSzIe5WweQ+m0qjj14HMpv
hOzyOnsQXsURarVV8PPrRamBP0kyMAbtCS1OPeKMwHdJEpJaqJCb3WaHa6wC
sZ9fJ6n+zjMvRHPg0pBSuD/uDs8/edK8XiH3gcFWk9sLWJgNDm4lzmMMoyP8
tmhOIwJfCsTJ35yE6iRL4uU+mJsdrudMRkc3EgMfQW/PBA+MnYheHY3D9xwW
kvRio0Luw+WtJrWFffH1HURtjYCwj+7Ld6k4fOdhBK8OpoWTQm7qmx1ukval
El5evSgsmLAJOsfvP479N+1HmluafWZwM7cng4HksWc6CKfnhQhB9oXe9U08
WmiDaKat+76NW0Zw8Fmo1QIvAQG9dpEWv57J27uVBSi7tf3f7BOs/veif9Nv
pLe8wTtuisv+L5I9yRg=\
\>"]]
}, Open  ]],

Cell[CellGroupData[{

Cell[BoxData[
 RowBox[{"Plot", "[", 
  RowBox[{
   RowBox[{"{", 
    RowBox[{
     RowBox[{
      RowBox[{"ExRBsr", "[", 
       RowBox[{"\[Mu]", ",", "c"}], "]"}], "/.", 
      RowBox[{"{", 
       RowBox[{
        RowBox[{"c", "\[Rule]", 
         RowBox[{"1", "/", "2"}]}], ",", 
        RowBox[{"kF", "\[Rule]", "274"}]}], "}"}]}], ",", 
     RowBox[{"ExRBsrPad\[EAcute]2", "/.", 
      RowBox[{"{", 
       RowBox[{
        RowBox[{"c", "\[Rule]", 
         RowBox[{"1", "/", "2"}]}], ",", 
        RowBox[{"kF", "\[Rule]", "274"}]}], "}"}]}], ",", 
     RowBox[{"ExRBsrPad\[EAcute]4", "/.", 
      RowBox[{"{", 
       RowBox[{
        RowBox[{"c", "\[Rule]", 
         RowBox[{"1", "/", "2"}]}], ",", 
        RowBox[{"kF", "\[Rule]", "274"}]}], "}"}]}], ",", 
     RowBox[{"ExRBsrPad\[EAcute]6", "/.", 
      RowBox[{"{", 
       RowBox[{
        RowBox[{"c", "\[Rule]", 
         RowBox[{"1", "/", "2"}]}], ",", 
        RowBox[{"kF", "\[Rule]", "274"}]}], "}"}]}]}], "}"}], ",", 
   RowBox[{"{", 
    RowBox[{"\[Mu]", ",", "0.1", ",", "3"}], "}"}], ",", 
   RowBox[{"PlotStyle", "\[Rule]", 
    RowBox[{"{", 
     RowBox[{"Blue", ",", "Green", ",", "Purple", ",", "White"}], "}"}]}], 
   ",", 
   RowBox[{"PlotRange", "\[Rule]", 
    RowBox[{"{", 
     RowBox[{
      RowBox[{"{", 
       RowBox[{"0.1", ",", "3"}], "}"}], ",", 
      RowBox[{"{", 
       RowBox[{"0", ",", "45"}], "}"}]}], "}"}]}]}], "]"}]], "Input",
 CellChangeTimes->{{3.741166702088785*^9, 3.7411667403449783`*^9}, {
  3.74116711726934*^9, 3.7411671242508717`*^9}, {3.74116715876818*^9, 
  3.7411672068705463`*^9}, {3.741167873686638*^9, 3.741167910298462*^9}, {
  3.7413202993838654`*^9, 3.741320377250519*^9}, {3.7413210764552917`*^9, 
  3.741321082488275*^9}, {3.741321134981818*^9, 3.741321167766224*^9}, {
  3.741321212463162*^9, 3.74132121387894*^9}, {3.741336071025097*^9, 
  3.741336076542717*^9}},
 ExpressionUUID -> "ea32bece-a1d2-4c47-a49f-2d58811da32c"],

Cell[BoxData[
 GraphicsBox[{{{}, {}, 
    TagBox[
     {RGBColor[0, 0, 1], AbsoluteThickness[1.6], Opacity[1.], 
      LineBox[CompressedData["
1:eJwVxXk01AkcAPDB6Ccm5Yq0onM086SNjRr5frVKyaRVj0Y5cmRrqQymolLU
Gsmuo0triZ6XK10s46iJDhkWW2IKzQ9jxjluasju/vF5n5V+J90CVSkUCuc/
/19aWXfrTpoAuGa+jg1PEF9Kk7N63glgv6Tf60AeYpM2p2CDdjmYXzYLk2Qi
yn1lz6pjyiH5aGoEkYhopE7t7f+lAkxuHLBOCkKMZG+zZtlXwZuWkZwbJoim
Cg95SKgQlri4ZGobA3ZF113WXvoSxnn18fWjdvjat0JqPSsCT61jJaJKW3QQ
8HUsipphnft71tiBHzDrTWFL+Z4W8OmxTS44uQkflXywqLARg1CbK/4YbYkM
O6uJckk7WEUTF+nIxOpX6VW3R9rBs7GMy7Jk4iHXBXE8Sgeka25OPbSCidf8
xMs2mXWAhZMXCmcZqOBHQ55PB+x7WnPBuJyBxS2iq7c6O+CMtH8tzYaBcDJg
ZXh7J3Af2vQ+2rIeGc3O95cGSyCZJuAG+dJRle8cIwmTADcmd9nvbnQU2zt7
5UdJYLvfwiqhIx35hbv17BMkYLZGu9NhPR2lcbuiA/MlcLODWl8+tg7v2u/0
KJZLoK/dLvxS3Do0KHQg3AJJ8Jc3s6zK1iIlzjYo0bsL3g9H9Qqs1yAtHjpj
LXvAwapTZCVYiYrI3ZlP6b3w8eCniRODK1BDEGzo/00Gxa7pKmney7HrrMuq
JlEfGKw/760XZITXGZanecIBMDFMb+TlGeA5OjM2PXUIarbwAifP6iFLnyFW
JirAn2lybnWoDna8GPO99nwEdGskAfywxVhm2vHI8/4oPNhO6zMooGH0ZG3O
q+wxqNwmPXpAQxOPhDrwTiWOQ0WoVrSrhMANgRUDpQkTwO5WClqb1fHwnVSG
95VJeOsSFJijScWciBlHxxNTEOJqPrM0WRXFtd7UN8enIabr4MKu1SpoXv1T
Zrz7DAiD9xndlM5D22y2WsG2L+CpGVDX+3YOwh9O0o7ZfoWoEt/+XIESmBot
o0dXKUHzL6/drcov0NBWEqViNgvp4zhftmMGmvon/v5qNAeBdRtZNc+nYDhb
OGel8g1a1vx6sTJsEqb/SWxeOPcNZH2aGhzGBCzPk100lc+D3jl/etKScXCV
NM7uDqLgtF2ktkRnDIjcwgS3Hgo2mOygWeiNQkO1q4byoAomp9jptdqMQHxa
WGtoqwq2brQw1yobBrcar+t8tipy9BUT86whEC2aLtn7QhWXGWqdciYHYKu+
DqPbXg0HGu5L+bH9UBoymmBYrIYBd3OfpO3vA0asGxpbUVE4speZYCYHtsCP
U/+QivlZbkb5hAzOb9/iu2KNOh4/FV7M1e2Fe3FJAvtsdVRPOc5xXyaFVtMi
yrzhAqQMM/UBeqCiLbLwRMICFIfrZSgiuuEGuza/UINAGKelhuR2wTmD9ptX
zxP40ozw/zhOgupn3+Dr0QSubzzjIRohgZ8rdci4ROCMTY1u1RAJqSzF4OMr
BO56/aE9W0ZC/hHVH8WJBPIai0pPfyKh9YG5gp5BYKKzxd6dNSRs2hnh9OoZ
gS/UPawjUkkoW/z1u0YhgZ7iw5cvJJGwTXxhrK2aQJNF+qn8RBJ2BfP/HHxN
4P5Htwcy4kjwSfljXK+RwBrO4pj3USRc63yR6feZQO6RgkX+ASTo5u6MCCYJ
3MuxY545QsLtUJEzr5vA29IUtd+8SbhHbZmMlxEoZad1VxwkoZwh3/NYQeA9
hYunGZsEnAheWTFK4Nuf9zixnEl4VTU69XKcwNoNq4fcnUho2qfMapsmMPPQ
cb8kBxLcjS+e7vpCoPtnn++L7Elo76ayB5UE6si3ltWzSPB7EL9qao5Aj+pn
UwO2JMh42jPz8wTK3xUNam0m4V+wNqlF
       "]]},
     Annotation[#, "Charting`Private`Tag$218233#1"]& ], 
    TagBox[
     {RGBColor[0, 1, 0], AbsoluteThickness[1.6], Opacity[1.], 
      LineBox[CompressedData["
1:eJwV0/k/1HkcwPFxfil0KSRLxWpGk0doIzXvty65Sz0Uua/WUlJMFqV1hNCl
JJSMLUdKbB6O6WCKLBvJyojh4wqhSe5rbPvD6/H6C57r3f1tvcRpNJr9j/5/
yfPa26l3yuA02WdctAfwTd/1zN6mMohcMe0jpQf4XsH+0RaFcggITbnjpgE4
4Nr/khdRDg95bUKDBRYqS0l+/uLLBYG8hJZpCQtDrHYZGLNeQFhftKwSk4Xq
wqMDJwMqQFXpbrW1+i7sDq+NUljzBjZjW7G3mjFWu3L7DObroFQy0Cdt63Y0
KYtdwXzSCDRmsOgXKQPMfJvfXG7RDOwsNc8I2634tPgjk7u9FY6xvfJUM5nI
2Kk/Xk7aQafx74O92XTkVaW/SPnWDp+OaqJ8Ch2P20jHsGkCcKpWCzaJpWOC
e6uKnoYA2rXCs+t+paMwNhxyXQTAdWs292bQ8Vlz3eXbHQLYkSDgPynYhODv
uT6wvQOW877lOPO0kdFonr3Gj0Dio+SZKumfUTzWPIKcJZCS0HStdkYLW1nm
TnmhBBbvc0/zh7UwNt9sFSuegGd+2+iyJi3sizkQ7pVHYHysynIkQwvvs/Yf
fTZAQFFRTMrRWAtX55tQtl5dkL6UU9cRrIm0GMMTic7d0Bb/WEiX34hycdAR
qdsLPZ23RMqlGigMMcv4S/szfJXOaGLqqqFMmZ+Sh6gf1HJUkms/qmD375Yb
3tcNwmx+5MiJpUp4k6F7jl0xBNvH5xx12YoYpq0TmZ40Ak7uqiTTeyUaKzJa
5xKFsJC0rcEhdDkKKr+7Jrz6BkxP/SORZfJYqi546pA9CjZWB9yWqCzF8Ima
B1Wc77C+K2x2Lk0G3QJM2KcTx+CCio5l4Q1p3OLFHSqJH4eHdiH7/DMl0TE1
ieEcPQHuppXHfcfE8UHQ9N69pyZhJ9clvuiKGLbWOEu+/W0KEpLHPe5so+Em
3qGMOLtp8HAuSkxgiIA/z5F4tGsGDl83OhO8eR4CCybkfAxnQbrh60m60Szo
yDSPem+YAzMpLZnypGl4xy8OFdOYBzmHBuPLE5Pw/st4/azyAuzYWzL2KWoC
vnIqFvTFRDCoaV04bD4OUx8SG2UXRHB8ZjokeNUYqOb2X1QfWISlFhN8Cdnv
YEMa5s1O0JD3J7NbR3kUqJz8eNteGmbFR1211v4G73g2MnPHxDCi4EFfRcFX
iLtztiWgRQy9HAI2Ty0bAdvXTjdjrcRx3ZXBq5dyhqBOfqrYulIcTYU1wamu
X2CH4gpGD0sCfXWXG9SuHoSSk6PxSs8k0Enz7KL1ZD8wIm1xrb4kbrQN6hQ0
fQarMnf7fwokkatsNMas7YPzu41cf9KUwqHkJI5hdy9kxVwrY3GksPa83ZKk
yR5oUX9CW1SSxtme0MN7N/UAlx+SfypeGg1zj4X969MNt6xq8vJlKDwvSj7g
m90FYavbky+fp3BBgZ58e56AeKer381wCnnF5fVFMwRic/pM7v1BYVfuldf1
kwSSjIXDhdEUagcldcqMEshzE9/TmkhhUePujug+Ai2PNwm171Hokmr1nFNP
QG9/kGnVSwrd60stvDMJlC6bXddQQWHY88eJKfcI7Gq98J3Po/DylSNRdWkE
DvjF3h2uplD/ECdBP5mAy420sVUNFFYoicnK/XCW0FGZ4d5JIcvufmBHIIGV
OfuD/LooHLakE9UzP5wG1JmzeyjUqyqft/cnkCXZPBHXT+GjS3RTvg+BcsaA
RaGQQt+f2MoCZwI47reeO0qhRoBIXMORQNWL0ck3YxQ+EZWle9gTeH9wLpM/
ReH+q5fahg8TsFt78Vz3DIUjsisu6h0i0N4jaTU8RyHNJfxDsDUB98dxGyYX
KOTcGPzwyoJAP1thenGRwo25PhcpMwL/ARjqs8c=
       "]]},
     Annotation[#, "Charting`Private`Tag$218233#2"]& ], 
    TagBox[
     {RGBColor[0.5, 0, 0.5], AbsoluteThickness[1.6], Opacity[1.], 
      LineBox[CompressedData["
1:eJwV0/k71AkcwPExhu8oqzQI9eQIo/F0rCO25PNBjxxJqy3VrhqsToWECKNk
kVSWHBEr63FEpaiQsxyxriRsRvN1NI4Y1zAax7Y/vJ/XX/DWcPV0dKdSKJRj
3/vfl68bE+8nl0DUsHFlSiLi26HYjMGOEtDg5LbsvI3YJnfs0Ta5Upjf4RX/
8QbiMJtfUXO9FFpOnTHVuoSoLEX7Mnq+DDIrxlrn9yMG2u8x3G1WDtXGm+ND
JBHVBE7DF7yrwC3JX3aZb4b9nMYbckpv4dAKb6bvrSnWscuGDBebYFVm7FF+
ggmal0TKb33cDvKaq4IiDY0woz6/s9SuE3Y0h1b7/KKPT4s/bi0z7gF1NVrx
HcftyDI1mC3l9QJHdOV1nYoe1tSmlidN9gLV90G+kK6HvzpIR/hRuJDi3/ls
h4iFt1x7VPTVuVDa92Cw8SMLBZEcyD3JhYQsS8adeBYWdTbdTOzjQiGhbXNw
HQvB83eNy719cE59t2eY0hZktdtmK3nwwMjSfacyMpEaaXud58MDqU6+9mF9
JvaY2TrnXeVBjsSzlRQtJkbm2zDMonkQSHdw2ifDxKEIa457Hg94H05+YnTo
4F9mVk5FwzyYLuK6hJzRQcV8c8LRnQTxnGjT+fvaSIkwOR1zoh+OWo7NGKto
oWwU9IVtH4TxawfSjmdooCDQJv058wuox3Pczd9sQnqJx3q3ZT4MjuZSLu3a
gP0B+zXbmkZAX+HTXrl9yhjP2u7vVzUGbrqr7XbGKGIQUy8sNW4cDI/HJRaw
GbhbgdUjjhHAkkyaXvJxeeRWT7NvVU6C8+ZzyTJ2a/CVGvfp8ewpGN3HZlv/
IYscYUNW7cNpEPpUD1D4Mujibe7nFTMDUoUx7LZqAre5l429jJ4FB2kam/5C
Cn+7H8c6ES6EUHsvO50pSczyFe3de3EONOzvnr8WQMWehhO0+nPzEF2qmagl
J4G6NT+nRx0RQepcW8fW8hXoXnwo+WjPAiw5X8gy/HsJLj8Ryp41+QaHwLU4
NUEMevTOqVOaYlBkTG6U/rQAzd3FVyXUFyHAQJWmzBRB2+hsyzflJWgUTy8y
Mudg4mHVkoHEMrxvng8pOiqE+fcx7TJLyxDn23Jwdu0sbMjlh6oNr0CKxcEX
saJpcOC1LtqcpuB08k0FbfEUEDn50Y6DFHRa9W5b8dIkNNc40MVHJXC50PSQ
7+ZJiEr26fLukkBf0wmny7ET4PjGOT7Snoq3n1nM26wfh6Yf5osPVFOxxShY
YFcxBrsU5FkDZpJIHzFKsnQdhZcXpqLXF0niO5VPX98bjAArzBFVDWgoNKyX
tKYOg32J67F/ntDQY6yupmH0CwRb/MTepCWFZ70NDN7NDUFmxN0Ss4dS2JVs
lzG8PAhdao8pK+ul0YTpReNqD0JZd2D+xWhptKJX19x1HoB79g15+XQCJUVr
dsjF9kOQYm/CzWACc66PyLpwSaB+ZnvEcwjMXMl9d/hfEiJzhszTrhHIkfEa
tOoiIW634GthOIH8Tk0jo3YS8lyolj0xBCpadbxSqyWhq0BXwEwjsHE0PIYo
IEHfyndfbQWBazdGiM8Gk/BqzbeNrVUEchkXs4ICSdjTEzLdXUNgm3JAZaw/
CdYekQ++1hHIjM7hPPUm4eSfKTOMVgKziiQ+T3z/5lZfdbrrZwJbThQK0w+Q
sC7HyteDJDD7VMFCpR0JSd5Ntn4DBHquq2d8sCYhk9YpjOITmLhl9fiiBQml
rGG7QgGBGYLZe0HGJOCsh0bZFIEJ0RO0WEMSasun5t7OEPjc75rWkx9JaDso
zuieJzA+m5M8rkfCEdVQ//4FAq84ZamqbyGhd4Bm/1VMoKrSufBdOiS4FkRp
zi0RqKOytsZtMwl8PznRygqB3opPdUPVSfgPKLysLQ==
       "]]},
     Annotation[#, "Charting`Private`Tag$218233#3"]& ], 
    TagBox[
     {GrayLevel[1], AbsoluteThickness[1.6], Opacity[1.], 
      LineBox[CompressedData["
1:eJwVV3k8VI33Zu7VJJUWRMlaKVtSpEXnaPEmu7eyREnJkj0khaKyl5BEX0ub
nbTYSm9ZUkr2IktGmLkz9iVK8ru/v+ZzPvfcM+c5z/OcMyNr525mz+Dj49Pj
5+P7/8/iV7V3ku6WQpOfIXmhALGq/1Z6X3MpWNfrWgo8RmxYapmjurQMcpV3
OyfcQ+TYsl9XBJfB81uJpe/CEcUFyAHu2ZdgMlH//cRpRH9D7W279pTD4fM7
2r1WI0qPmHNcPd9AbZnpqLQIYG9Q7dWlYlVg4DihmjC0G9/Zvuzf9ucjVKsU
xnWXaKFOadhylfxG6BVWjV5hqoHpNbmtZfqtcGpNR+VlF3V88uKLysvt7TAY
Yz/8wH8zKu7eOlnW0wnpGUpCFbuUsKL6XnniaCfI1X/d2K6ohMeMF4T68nWB
vMpJzz8SShhl1y6hLtMFjXHf7R1mFHEkLAiyTnTBGKW/7PMLRXze+jHiTncX
PJBMYLapKyK4n5b17uyGK4fAJkdjEyo2HsoQc+mBlAr+K8XWCsgIOxTcc64H
Plb1p7OMFLB9zyGb7Is9oOa7tFxURwHDcvVW7onsgftScjXJ6xWwP/RgkH12
D2yb93SVGtmAaXt0zZ9zeuBGjqzsTMgGFM3VYZrZs6CTj7zw+fl65AvVcog+
3gvl25xvJ25Zh4vDoTtkcx9Yu5inBRbJ4oi/XuozhQGQN2BeqGJL4cJSl1Wn
/rJB9G4354rVGuy9YCDX8JECYwdbKZ9T4hivuPm87xse7LZb76/7WBQvKSiF
3IsbgtpXy2+tOb8Sd4kots9Gj4DSQJjuXbfl2PV23Dbqv1FQVpNj/HITxhLp
ridWGWNwL00qcOzxYgyaev+o+v44fPxQ+C6eXIQnPXV8PaInQOXvhA+rk4mq
9i95xZGToKZpI1z8WQCtk+IUj1+bgi/G1qvfM0l85DOzf7/bT3h98zDD8wYD
298fJ2ucp8FybOdrV1l+3Fhhmhp+dAYu+s8dWsaah7Y/94kc7V9gnDXwtaR6
DrwLphY7af2GDIV6bsmLWVBa2Dp2Rm4WMg1sv8vM/IK6thcX+WX+QJ+FUNDa
vTPQwJ38/Ft8DpBVJrG2/CcM338zt5X/L0i79UvWekzBdFN0o+DcX8i18kpe
u3ES1mSxL0tz5iExZP988eIJMO6p/6PnwIebcyJ3fVs6DszM3EizPj6MFVqb
Hb5sDOoqjBfOWvCjoASVLq0+CuF3z331/MqPwtVrhRbmDoNZpU18mCEDzaZq
pKO2DcHHJdMvjN4ykOGRczuvlgd9PjXMA5UM/BN1S9PWcRD+dt2x3FXNwGf7
Cu9A+DCI6zrmbKlh4NaZ3Z7Xlw2Cer7WnMIHBoa8Gm5hV/PAQEzQWOojA4Xk
3C2L8nlgH9ieJlLHwP1B1X4OeTwIHMgaX1TPwE0LuLMuD3mQaOS/n7+RgUZq
k+2Xh3nwtOhQwnQTAy157/0f8njwSWoNZ6iFgaNmOikbTvNg4DpvR98XBra+
aWUqx/Bgfvhl5Lc2Bn6K61VUfcsDcfOoroZvDPTyWuSrGccD9f+sN9d0MjDJ
ZJ3nGoILBgoqV8q7GZgq7HUs348HZ27ONT3rYeCyI+Gx/Od5wFhOjorzEUjU
nz07J8UDyQstOsIMAoVLviUO0bEm62GcAElgxS1IZ0nwwETPp39WgECz8+xN
eUt44FR4YPs4k0C9bPsnR/q4ECwhFs4RJPCkWUOE6xwX7l0Z+NYtRKAJuYs8
4MGFIqpIuXUJ/TyN7SS5mAcNpqGBH4UJFG//PaK6ggfcUvOGt8sJXGJg9mwR
kwek3Ea5kpUEHo/lS31E15eKmDmXL0pgYqGvRXInF7aPv69+uIrAjvidtSe+
csHE6u6qZAkCi1yKTlu2ccG5wsnp1hq6fxj1qvrEhauKO1+GriUwvueD2pUm
LqTELloSKE3gr0v/o5Kv8KDk97fj3rIE+s1ITZc95EKTXc4TZ3kCQ0VT4mJ3
cGGw9iLj5HoCd/Vsd7Qv5YLAVoPD5goEUo9tAnQP0f0lSz423ERge99hycsF
XNAihqb3KRH4n7dleAgdm50t19upQuCfjLJoiXQuuDRHJ6ttJtBD67SGdhAX
ru86PrRhC4GvGxOmqVQupD1QhbVbCQzkb16v686DMqH5mJUaBEomlzlaO3Oh
+Vx9r+B2AhXezy5eOkT315G6jW8HgcMDE9URq3iwYL/H9Z87CTQYFFqvE88F
mVxsG9xN4Ln+wF3DPlzYKbJc8cceAudcXZViaX7SbifOFiOBB7/HB0uc4cKC
VTJ1UXsJFPhZccFjHd1vYkbKyf0EDim/jJI+Rc9HYrOHpi6BSzs1s/ysaLzJ
RTpCBwkcH1Jf4HqUnq/knpU9egRKmel1vKXzyZTqvuf6BE7V5k8uoOflLG1Y
FG5I4PbsgwXBTlxoSGsJPW5MoFGFVkGMERc05awtt5oS6LPvmcvcbi4w1p/9
03mYQJbj+QVey7jg+Hi8rvAo3d9MX88SNS58VvBPvW5BoHRhR/kTOt6Wxe95
zIpA29WH9lMKXLirGL5XzZpATt23O/KVFPzNWSYicJzATpkf36IluXBaJbG/
/QSBfBVfujtXcKE2X7o4/yStn6xYE0EtLqipZYSFnCKwT0nLL2kxFxIKVa0s
7AkMqAyUCqb99ke9SEnFgUCRs7++jfdQYPdce47ficCjlND6gOVceK9R/fmL
M4H7vM4I3KunQLXYIC3HhcAwvYuHllZTEK/V4nnZjcAJNavv+9op+F16bN8R
DwK3bHaLTBylwHbXDxFFLwJrirrs5QcoePfKeeDvOfr7m1ovWnIpUN4zXtzs
Q+v7mQbqHOZC7H8XwjPPE2inzv876wsFM8h/LOACXU+galvOCwqOV4Qpm10k
sHRsWZrnZwqq9i37uyGAQItgGThqToFi9Z362UB6vgypT99bKIjRlU5vuEzg
z5tsne9NFPyseez1KJjAS+ayRz6kUmCtp7rf/yrtzyPPnTTDKaiofSFqfJ32
o+o5y4uhFGw00GbLhxH4ZY+EyNZrFNyoqyqZCaf5SS9YruRKwaSRQURdJK33
F+2bArMosGpoPnY/msCYsyt+TF+i4I3pMZXzNwk8QL5jXk+kYENz71/9WwTm
K2tVKt2iIOqwc4NMHIHc3RGm1G0KxlvH0qfiaX2JrfL3v0uBhfmFc7UJBBZv
LTc7dI6C1218B1ITCRx4vK/3UQgF66zCxLyT6P00qh+c40hBRIcw5+A9AhdY
Xdt8+QIFo9Z3Stem0PqYUHfT9KfgaLdU5HgqgWO/sucTtlHw6sRj65p0Ajcv
1WhY7USBHEtF9d4DAh2ts0J0TSkIs3sx7/GIQLe75vXaYWwY/rG78UAGgQ+c
OzzUT1Nw2L7q/uosAr1rInaF0/MvG9D3HskmcJOB5O4pCwpkHJsPVOUSmKYb
uS1LgILrlNWqu/kE2ngWjZZkUzDo3MtxfUIgZO30mTtCgdmgU9nep/T+DL34
+o84BcWuY5GrnhN4LDDTj9nMgcXjFQkri2i/sEztp2RovfrGpwuXEJih1RU1
KE3R+9A+V6iMQEO+Wwuk91OwNGh7MfMVgeHrhgkoo+A0IVhBvCZwpRO79dIQ
B8pCv32a/4/Ap/U2W44ZDsGyxblfZ98SGH3D0fe1GAVnYgJ6pysJvBPl5r1l
mgOvRIyHJqoJ/C1VG620goIVd2VmRmoIFLJWVj/sToHj2nHG4AcCVz/0yHUS
oqA8vXIJ5yOB/0yXFjJIOn/DbfG+OtqPmzP4r1EccMw+I99TT2D/ziNU+28O
vFbVUu1sJDCo8OFkby8HRJ4J7mhrJvBx214vt24OOG/v2NfSSmABV6l8HZsD
b17mGjV8pfla+uq3WQsHxDDQ8lM77YcTIRL/sjhwtsr49PsOAq3bIfvTeVqP
B2Xdq7roeQzJpZ2k8YvVjV948532f8gz48ivHHAxrbr6ikX7MclCxugVBypa
b98s+UHfk1k02lLEAXErh6Tn/fS9GE0PW9LIAbdurUdP2PQ9PZIIEXkcqLJb
9CSXovkVdzAS+MABCXZHWSaPxjPZ3feFjt3O5lU/HKL94fZqXjOXzh8JbEgb
of358dnCrgwOrPY26bg3RvNNCnry6NhjRnYgcYK+V2dP5byN48C7SxOj8VP0
PbDLu8PdSIEkf/VszDSt57rSu6IRHPC6lrAg+heB13PcK2ssBqFG0HF5+CyB
+nJKs1M3OCB5Y4fktTkCzywo2PsslM5fIaRwZZ5ApcEBF60QDrxP6NwSwE8i
mrcJ37XmgNSa/N0XCBKdD1TeplQ44J0a9I+PAInuDO/t109woFbe1MyT/p1a
l51yxOQSB2Qy5WxcBUm0uxm76ZwTB3yVJx2chEj8VvlcZ9aMA5+eVHvZLyFx
4WarS6LHOSCncSfgpDCJyd3y7+L1OeBX6hhms5zEDZ/XHVWi69dp74yzXEni
zLzG6T1A51cIpRwRJdG0zs+n35PO1+3KNF1FYuR5lXopGw58rs1/ZihB4m+P
NVyTvRxYZ3z5td4aEu/I7pDy1OGAf7PphwNrSTxUottSuIsDDebyLTrSJAp+
gumx9RzY0DnZrS1L4lTcs9qNWzlwyfYdtUOexKYP5IMmZQ409d2Z1FhP4k/b
73vNl3Ngo5PT/BYFEr+6y1OHO9gQOLRzkeomEn0bJa7GEhxo9lwsqqhEovzC
jFCxjXT+zy7pDSokLnt163a9OAcC/QsU5TaTWH1UO1V6GQda/l7WkNpCov3x
4MhrSzmgGGKGq7fS+KaNHS7TMaOqaOESDRJdbLZd/izAgQ5yTeO8Jon3blH6
s/wciLr+42T/ThKPLAonlafYcLrmH8W23SRmlBeEd46yQXth7njtHhLPFWxT
utjJBjG9ZS/LkcTzRXFs7k96v4V7hzzZS+JYsfh6gXY2vKtt03+wn0TucNKY
Rj0bUoW0RRJ0Sdy/prlpgMUGP4P0zrCDJA5fjZth0fhNogUeXTxEopVmMzO/
jQ2bPju5uhmQaOKXXev7mQ0M4c8aJ41INGjMS5DPZ8M3Y/W//5qQmOh5cNmS
x2x4FpPwTteMxGM8Pv7612yIavx9Y8dhEsddqQhtNo1nxQlz5aMkDjker/V7
QOP5t1Ja2oJESeESd/0YGk+8Ame5Ff2/6Ujn08Q0Gk9L5BPSmsQz1WmJ+pfY
UCM66jdtQ6KYSEHGh/tsSDt6WId7gsTpkbD+PDrf706JYNdJEjscLq5XiqPx
tEk21Z8isWBx93xYMo1H4kpShT2JB516vs4m0Xis+u1eOJD4UWn18mJXGk+S
nlKmE82PNvdMfQQbnnbkTSSdpetPdCa/u8iGSMkVr6JdSbwaF+iWnkvjsfG9
etmdxKgbNknl9PPdKd8MznmSmPddSNWwig0i3/eInjlHIrPI9amDCxuGpB90
WfiQeKBy5c/eUzQ/tszH+udJPJoJqjePsSEl/azbngs0H82vmQ5mbPDtrdfc
cpHmI231twZ5NhjLb5uXDyAxtWVcavQ0GzaeTqwRCyJxoL70Zyz9Pt+jPzcF
r5BoMTWXmnCUDW39thZ/gklsdd/6NFiXDYUbqmVGrpI4IrIw6oEfGyIcNlGs
67SeXwqlgTYb7DKjC1vCaP9eztJ7T+fvpMYu1ETQ9X7Hp2rtYcNKxaN7y6JI
TDG+K5gHbPr+lS3Ku0FixODN93pqbKjKkWpOjaH1WKmhpreRDfcGg5NjY0mU
JUJ2dKxkg48K+9S1eBIbnTv5O/5lg5GbvrJfAq3vN9GSKMKGDQUFk86JJBae
3M8I2sWGvyMry22S6P0jG7T+Ph8bvqr5XTO5R2LDgfwfTcJseOLZabgvhcSK
VQ/HFen3w56imGYarQ+jNrsIMTbYTjzs3nifxCvmG6TqCTbs2CaYseYhiXre
loGKfQOwwsfVfeljEu/zHOdZswPAfdG4nT+TxDlt7oOH0wNQ+VODbzKLRMeF
yWpvswbg3vak9wM5dD9DMZXywwPg7fc3pj2P5qdYYm392AAYltpZfiogUTP0
wLF1cwMQsHeHrdQ6AZxcErTWdqIfHoTGlO65L4CSb9afE/jTB1+l8/nmVy1A
zXZz9ybVPnjZ5p/rFrkAu50tBhtP/IDbhu+zcxcysXPnWvPUmF64JNqZEBHA
xIf9013ZHSxgfLd1iQ9iYsMCveUK7SwIy+zXSbnCRBfVWcEVX1mw1Mt5VWYI
EyVNe10Wt7AgbtfIYOE1JtqZCMDDJhaIC3hXvAxl4u/eV6Wr6liQ8nnmTnU4
E6OScMK6lgXrEgNc6yOZCDsPGhrVsCD7JGNfezQT//dv8K+MKhZ8zds4opDC
xKdbgmvU81igruvzT/VrJrZmqqiuDmBBifBvyfo3TBzwGr5beIEF2u2B420V
TNx6/Xmf+HkWVNwn3vdWMZG1PXZRgA8LDrqE/W/wHRNNW1q2r/RiwYnY5ImV
9Uws/Zel/Z89C6K636bafWeimWyMO8eIBSsydX1cWEzU0VSaEDFgQaLnx0O+
P5joESEao6DHggdk61Q4m4lljRWX/tvLgjJFjn7hCBNvDVQ9StvOApx0kX05
xsSpgOi9cltZUF0+9rNqgonzhLKE0xYWNJjMprdNM7HEa5OtgDILjq6+fL73
FxMDtPtKjmxiQecP0nBwlonDTVLsLxtYYJcXLvdzjom8l0tuicqzgO27dGZ+
nonusYNrOmVY8H+du5f1
       "]]},
     Annotation[#, "Charting`Private`Tag$218233#4"]& ]}, {}, {}},
  AspectRatio->NCache[GoldenRatio^(-1), 0.6180339887498948],
  Axes->{True, True},
  AxesLabel->{None, None},
  AxesOrigin->{0.1, 0},
  BaseStyle->{FontFamily -> "Arial"},
  DisplayFunction->Identity,
  Frame->{{False, False}, {False, False}},
  FrameLabel->{{None, None}, {None, None}},
  FrameTicks->{{Automatic, 
     Charting`ScaledFrameTicks[{Identity, Identity}]}, {Automatic, 
     Charting`ScaledFrameTicks[{Identity, Identity}]}},
  GridLines->{None, None},
  GridLinesStyle->Directive[
    GrayLevel[0.5, 0.4]],
  ImagePadding->All,
  ImageSize->{1417., Automatic},
  Method->{
   "DefaultBoundaryStyle" -> Automatic, "DefaultMeshStyle" -> 
    AbsolutePointSize[6], "ScalingFunctions" -> None, 
    "CoordinatesToolOptions" -> {"DisplayFunction" -> ({
        (Identity[#]& )[
         Part[#, 1]], 
        (Identity[#]& )[
         Part[#, 2]]}& ), "CopiedValueFunction" -> ({
        (Identity[#]& )[
         Part[#, 1]], 
        (Identity[#]& )[
         Part[#, 2]]}& )}},
  PlotRange->{{0.1, 3}, {0, 45}},
  PlotRangeClipping->True,
  PlotRangePadding->{{0, 0}, {0, 0}},
  Ticks->{Automatic, Automatic}]], "Output",
 CellChangeTimes->{
  3.741166779981697*^9, {3.7411671399470673`*^9, 3.7411671686750097`*^9}, {
   3.741167199651115*^9, 3.74116721940021*^9}, {3.741167884725768*^9, 
   3.741167931427692*^9}, {3.741320315663919*^9, 3.741320386793285*^9}, 
   3.741321103265731*^9, 3.74132114342878*^9, 3.741321175008293*^9, 
   3.7413212220986137`*^9, {3.741336063858914*^9, 3.741336079033958*^9}},
 ExpressionUUID -> "56021c73-243c-4585-8dee-218a89d53f7f"]
}, Open  ]]
}, Closed]]
}, Closed]]
}, Closed]],

Cell[CellGroupData[{

Cell["\<\
Relativistic short-range Coulomb-Breit exchange energy per particle\
\>", "Section",
 CellChangeTimes->{{3.741164071993136*^9, 3.741164088480412*^9}, {
  3.741336108106634*^9, 3.741336109917707*^9}},
 ExpressionUUID -> "7bec3435-db0f-4025-ad34-b96cb848dd5b"],

Cell[CellGroupData[{

Cell["General expressions of the energy", "Subsection",
 CellChangeTimes->{{3.74116431193472*^9, 3.741164315937715*^9}, {
  3.7413361340022087`*^9, 3.74133613543769*^9}},
 ExpressionUUID -> "9b1cab8b-888a-4cbf-a5f6-7f152f363bd4"],

Cell["\<\
The expression of the relativistic full-range exchange energy per particle \
for the Coulomb-Breit interaction potential is\
\>", "Text",
 CellChangeTimes->{{3.741312221879962*^9, 3.741312269736453*^9}, {
  3.741315812750471*^9, 3.741315813596662*^9}, {3.741316844732884*^9, 
  3.741316847053866*^9}, {3.74133613887786*^9, 3.74133614082997*^9}, {
  3.741408004038986*^9, 3.741408004297286*^9}},
 ExpressionUUID -> "3da15f4b-46b6-4fb2-b4c0-80f6fc969e71"],

Cell[BoxData[
 RowBox[{
  RowBox[{"ExRCB", "=", 
   RowBox[{
    RowBox[{"-", " ", 
     RowBox[{"(", 
      RowBox[{
       RowBox[{"(", 
        RowBox[{"3", " ", "kF"}], ")"}], "/", 
       RowBox[{"(", 
        RowBox[{"4", " ", "\[Pi]"}], ")"}]}], ")"}]}], 
    RowBox[{"(", 
     RowBox[{
      RowBox[{"11", "/", "6"}], "+", 
      RowBox[{
       RowBox[{"(", 
        RowBox[{"7", "/", "3"}], " ", ")"}], 
       SuperscriptBox["c", "2"]}], "-", 
      RowBox[{
       RowBox[{"(", 
        RowBox[{"1", "/", "3"}], ")"}], " ", 
       RowBox[{"(", 
        RowBox[{"1", "+", 
         RowBox[{"8", " ", 
          SuperscriptBox["c", "2"]}], "+", 
         RowBox[{"7", " ", 
          SuperscriptBox["c", "4"]}]}], ")"}], 
       RowBox[{"Log", "[", 
        RowBox[{"1", "+", 
         RowBox[{"1", "/", 
          SuperscriptBox["c", "2"]}]}], "]"}]}], "+", 
      RowBox[{
       RowBox[{"(", 
        RowBox[{"2", "/", "3"}], " ", ")"}], " ", 
       RowBox[{"Sqrt", "[", 
        RowBox[{"1", "+", 
         SuperscriptBox["c", "2"]}], "]"}], 
       RowBox[{"ArcSinh", "[", 
        RowBox[{"1", " ", "/", "c"}], "]"}]}], "-", 
      RowBox[{
       RowBox[{"(", 
        RowBox[{"5", "/", "2"}], ")"}], 
       SuperscriptBox[
        RowBox[{"(", 
         RowBox[{
          RowBox[{"Sqrt", "[", 
           RowBox[{"1", "+", 
            SuperscriptBox["c", "2"]}], "]"}], "-", 
          RowBox[{
           SuperscriptBox["c", "2"], 
           RowBox[{"ArcSinh", "[", 
            RowBox[{"1", " ", "/", "c"}], "]"}]}]}], ")"}], "2"]}]}], 
     ")"}]}]}], ";"}]], "Input",
 CellChangeTimes->{
  3.73744099515831*^9, {3.741316838751589*^9, 3.741316838829373*^9}, {
   3.741317773170949*^9, 3.7413177874888287`*^9}, {3.741409009534317*^9, 
   3.741409013919306*^9}, {3.741409127153754*^9, 3.7414091368779907`*^9}},
 ExpressionUUID -> "729a3301-0905-441b-9960-6fa58fb12181"],

Cell["\<\
The relativistic short-range exchange energy per particle for the \
Coulomb-Breit interaction potential can be calculated through numerical \
integration using\
\>", "Text",
 CellChangeTimes->{{3.741312281128374*^9, 3.741312335545431*^9}, {
  3.741312671624989*^9, 3.7413126773038692`*^9}, {3.741315815612306*^9, 
  3.7413158161560907`*^9}, {3.7413168494057426`*^9, 3.7413168504923353`*^9}, {
  3.7414080064359217`*^9, 3.7414080079144*^9}}],

Cell[BoxData[
 RowBox[{
  RowBox[{"ExRCBsr", "[", 
   RowBox[{"\[Mu]_", ",", "c_"}], "]"}], ":=", " ", 
  RowBox[{
   RowBox[{"NIntegrate", "[", 
    RowBox[{
     RowBox[{
      FractionBox["1", 
       RowBox[{"16", " ", 
        SqrtBox[
         RowBox[{
          RowBox[{"(", 
           RowBox[{
            SuperscriptBox["c", "2"], "+", 
            SuperscriptBox["k1", "2"]}], ")"}], " ", 
          RowBox[{"(", 
           RowBox[{
            SuperscriptBox["c", "2"], "+", 
            SuperscriptBox["k2", "2"]}], ")"}]}]], " ", "\[Pi]"}]], "3", " ", 
      
      SuperscriptBox["\[ExponentialE]", 
       RowBox[{"-", 
        FractionBox[
         SuperscriptBox[
          RowBox[{"(", 
           RowBox[{"k1", "+", "k2"}], ")"}], "2"], 
         RowBox[{"4", " ", 
          SuperscriptBox["\[Mu]", "2"]}]]}]], " ", "k1", " ", "k2", " ", "kF",
       " ", 
      RowBox[{"(", 
       RowBox[{
        RowBox[{"4", " ", 
         SuperscriptBox["\[ExponentialE]", 
          FractionBox[
           SuperscriptBox[
            RowBox[{"(", 
             RowBox[{"k1", "+", "k2"}], ")"}], "2"], 
           RowBox[{"4", " ", 
            SuperscriptBox["\[Mu]", "2"]}]]], " ", "k1", " ", "k2"}], "-", 
        RowBox[{"4", " ", 
         RowBox[{"(", 
          RowBox[{
           RowBox[{"-", "1"}], "+", 
           SuperscriptBox["\[ExponentialE]", 
            FractionBox[
             RowBox[{"k1", " ", "k2"}], 
             SuperscriptBox["\[Mu]", "2"]]]}], ")"}], " ", 
         SuperscriptBox["\[Mu]", "2"]}], "+", 
        RowBox[{
         SuperscriptBox["\[ExponentialE]", 
          FractionBox[
           SuperscriptBox[
            RowBox[{"(", 
             RowBox[{"k1", "+", "k2"}], ")"}], "2"], 
           RowBox[{"4", " ", 
            SuperscriptBox["\[Mu]", "2"]}]]], " ", 
         RowBox[{"(", 
          RowBox[{
           RowBox[{
            RowBox[{"-", "6"}], " ", 
            SuperscriptBox["c", "2"]}], "-", 
           SuperscriptBox["k1", "2"], "-", 
           SuperscriptBox["k2", "2"], "+", 
           RowBox[{"2", " ", 
            SqrtBox[
             RowBox[{
              RowBox[{"(", 
               RowBox[{
                SuperscriptBox["c", "2"], "+", 
                SuperscriptBox["k1", "2"]}], ")"}], " ", 
              RowBox[{"(", 
               RowBox[{
                SuperscriptBox["c", "2"], "+", 
                SuperscriptBox["k2", "2"]}], ")"}]}]]}]}], ")"}], " ", 
         RowBox[{"(", 
          RowBox[{
           RowBox[{"ExpIntegralEi", "[", 
            RowBox[{"-", 
             FractionBox[
              SuperscriptBox[
               RowBox[{"(", 
                RowBox[{"k1", "-", "k2"}], ")"}], "2"], 
              RowBox[{"4", " ", 
               SuperscriptBox["\[Mu]", "2"]}]]}], "]"}], "-", 
           RowBox[{"ExpIntegralEi", "[", 
            RowBox[{"-", 
             FractionBox[
              SuperscriptBox[
               RowBox[{"(", 
                RowBox[{"k1", "+", "k2"}], ")"}], "2"], 
              RowBox[{"4", " ", 
               SuperscriptBox["\[Mu]", "2"]}]]}], "]"}], "-", 
           RowBox[{"Log", "[", 
            SuperscriptBox[
             RowBox[{"(", 
              RowBox[{"k1", "-", "k2"}], ")"}], "2"], "]"}], "+", 
           RowBox[{"2", " ", 
            RowBox[{"Log", "[", 
             RowBox[{"k1", "+", "k2"}], "]"}]}]}], ")"}]}]}], ")"}]}], ",", 
     RowBox[{"{", 
      RowBox[{"k1", ",", "0", ",", "1"}], "}"}], ",", 
     RowBox[{"{", 
      RowBox[{"k2", ",", "0", ",", "1"}], "}"}], ",", 
     RowBox[{"Method", "\[Rule]", 
      RowBox[{"{", 
       RowBox[{"\"\<GlobalAdaptive\>\"", ",", 
        RowBox[{"\"\<MaxErrorIncreases\>\"", "\[Rule]", "2000"}]}], "}"}]}], 
     ",", 
     RowBox[{"WorkingPrecision", "\[Rule]", "8"}]}], "]"}], "//", 
   "Quiet"}]}]], "Input",
 CellChangeTimes->{{3.701145681788294*^9, 3.7011457077245607`*^9}, {
   3.7011457387970448`*^9, 3.701145742715835*^9}, {3.701145838955688*^9, 
   3.701145864971176*^9}, {3.701145973723259*^9, 3.701145997658729*^9}, 
   3.701146056572063*^9, {3.701146107515278*^9, 3.701146121611495*^9}, {
   3.701146196843637*^9, 3.701146247866346*^9}, {3.701146312635221*^9, 
   3.701146375081807*^9}, {3.7011464264741697`*^9, 3.701146477657305*^9}, {
   3.701146583432921*^9, 3.7011465958422613`*^9}, {3.701146635256982*^9, 
   3.701146673336335*^9}, {3.7011471055597353`*^9, 3.70114712658249*^9}, {
   3.701147399749424*^9, 3.701147402949328*^9}, {3.701147490165003*^9, 
   3.701147559316208*^9}, {3.701147589652295*^9, 3.70114760658006*^9}, {
   3.701147762259828*^9, 3.701147764355604*^9}, {3.701148064721983*^9, 
   3.701148067649757*^9}, {3.701148188946526*^9, 3.7011482124492397`*^9}, {
   3.7011483018407917`*^9, 3.701148396496244*^9}, {3.7011484538239727`*^9, 
   3.7011484901597433`*^9}, 3.7011485487194843`*^9, 3.701148617247799*^9, {
   3.701148653359206*^9, 3.70114865593461*^9}, {3.701148686398691*^9, 
   3.701148686638567*^9}, {3.7011492174203663`*^9, 3.701149217484399*^9}, 
   3.703923968822303*^9, 3.70392400506175*^9, {3.7039240660390387`*^9, 
   3.703924077057626*^9}, 3.703924120324793*^9, 3.7039244524507217`*^9, {
   3.703924650531103*^9, 3.7039246519228373`*^9}, {3.706590014367525*^9, 
   3.706590016210148*^9}, {3.714289166465165*^9, 3.714289168351822*^9}, {
   3.7177498205374203`*^9, 3.717749842137086*^9}, {3.717751156491482*^9, 
   3.717751186824505*^9}, {3.717751246744615*^9, 3.717751480920171*^9}, {
   3.717751518361574*^9, 3.7177515280449133`*^9}, {3.717751613705089*^9, 
   3.7177516876773376`*^9}, 3.7177517201526127`*^9, {3.717751803459509*^9, 
   3.7177518054711514`*^9}, {3.717752264568583*^9, 3.7177522695631037`*^9}, 
   3.717753253914151*^9, 3.717821459452956*^9, {3.7181908060799026`*^9, 
   3.718190806213161*^9}, 3.718190982122443*^9, {3.718191793953211*^9, 
   3.718191819001253*^9}, 3.718193884654935*^9, {3.718194736362905*^9, 
   3.718194737316622*^9}, 3.718779040850235*^9, {3.719032398425578*^9, 
   3.719032400770814*^9}, {3.719746947478065*^9, 3.71974694774881*^9}, {
   3.719807513934525*^9, 3.719807517786133*^9}, {3.7413168422728863`*^9, 
   3.741316842640888*^9}, {3.741317774978959*^9, 3.741317775367153*^9}},
 ExpressionUUID -> "6c0e9369-a9c4-4272-b057-ee96b9fe29ce"]
}, Closed]],

Cell[CellGroupData[{

Cell["Calculation of the large-c expansion and Pad\[EAcute] approximant", \
"Subsection",
 CellChangeTimes->{{3.722158370784416*^9, 3.722158376544992*^9}, 
   3.740375873100111*^9, {3.7413361620740137`*^9, 3.741336164173935*^9}},
 ExpressionUUID -> "981c67d4-b435-40bc-8042-96514f7ddd59"],

Cell[CellGroupData[{

Cell["Tables of the expansion coefficients", "Subsubsection",
 CellChangeTimes->{{3.741164766995187*^9, 3.741164769226877*^9}, {
  3.741164800614396*^9, 3.741164808695251*^9}, {3.7411649271723413`*^9, 
  3.741164931300631*^9}}],

Cell["\<\
We need first to consider and stock in matrix forms the coefficients which \
take part in the First Part of the exchange energy \
\>", "Text",
 CellChangeTimes->{{3.722158424609398*^9, 3.722158432240468*^9}, {
  3.741312800410178*^9, 3.741312967528989*^9}, {3.7413130008901443`*^9, 
  3.741313016467299*^9}, {3.741315945243114*^9, 3.741315948620363*^9}}],

Cell[BoxData[
 RowBox[{
  RowBox[{"Coef1CBsr", "[", 
   RowBox[{"M_", ",", "n_"}], "]"}], ":=", 
  RowBox[{"FullSimplify", "[", 
   RowBox[{"Coefficient", "[", 
    RowBox[{
     RowBox[{"(", 
      RowBox[{
       RowBox[{"Coefficient", "[", 
        RowBox[{
         RowBox[{"Series", "[", 
          RowBox[{
           FractionBox[
            SuperscriptBox["x", "2"], 
            RowBox[{" ", 
             RowBox[{
              SqrtBox[
               RowBox[{
                RowBox[{"(", 
                 RowBox[{"1", "+", 
                  RowBox[{
                   SuperscriptBox["x", "2"], " ", 
                   SuperscriptBox["k1", "2"]}]}], ")"}], " "}]], 
              SqrtBox[
               RowBox[{
                RowBox[{"(", 
                 RowBox[{"1", "+", 
                  RowBox[{
                   SuperscriptBox["x", "2"], " ", 
                   SuperscriptBox["k2", "2"]}]}], ")"}], " "}]], " "}]}]], 
           ",", 
           RowBox[{"{", 
            RowBox[{"x", ",", "0", ",", "M"}], "}"}]}], "]"}], ",", "x", ",", 
         "M"}], "]"}], "/.", 
       RowBox[{"{", 
        RowBox[{"k2", "\[Rule]", "1"}], "}"}]}], ")"}], ",", "k1", ",", "n"}],
     "]"}], "]"}]}]], "Input",
 CellChangeTimes->{{3.741067468632078*^9, 3.741067469775463*^9}, {
   3.741164676901334*^9, 3.741164680855814*^9}, {3.7411651769392443`*^9, 
   3.7411651785144653`*^9}, 3.741165729269765*^9, {3.741312742954957*^9, 
   3.7413127678181543`*^9}, 3.741316983089967*^9, 3.741318312825425*^9},
 ExpressionUUID -> "2333198c-7e35-4ceb-961c-11d51f7b8bb2"],

Cell[BoxData[
 RowBox[{
  RowBox[{"Coef1CBsr", "=", 
   RowBox[{"Table", "[", 
    RowBox[{
     RowBox[{"Coef1CBsr", "[", 
      RowBox[{
       RowBox[{"2", "i"}], ",", 
       RowBox[{"2", "j"}]}], "]"}], ",", 
     RowBox[{"{", 
      RowBox[{"i", ",", "0", ",", "10"}], "}"}], ",", 
     RowBox[{"{", 
      RowBox[{"j", ",", "0", ",", "10"}], "}"}]}], "]"}]}], ";"}]], "Input",
 CellChangeTimes->{{3.7220573274031277`*^9, 3.722057411958555*^9}, {
   3.722057553909235*^9, 3.722057558258687*^9}, 3.722058361827209*^9, {
   3.722059020563114*^9, 3.722059036001809*^9}, {3.722064043326339*^9, 
   3.7220640436134567`*^9}, {3.722068938617219*^9, 3.7220689488567133`*^9}, 
   3.7220690691792727`*^9, {3.722069129642337*^9, 3.722069129865574*^9}, {
   3.72207100528871*^9, 3.7220711073354273`*^9}, {3.72207151536589*^9, 
   3.722071516470203*^9}, {3.722071548694812*^9, 3.7220715507900457`*^9}, {
   3.722158613895567*^9, 3.7221586159691896`*^9}, {3.72215876562182*^9, 
   3.722158767779505*^9}, {3.740299010870399*^9, 3.740299012550469*^9}, {
   3.740299522922635*^9, 3.740299529194179*^9}, {3.740299573786133*^9, 
   3.7402995759288683`*^9}, {3.7402999926019487`*^9, 3.7402999947622147`*^9}, 
   3.740363775166651*^9, {3.74036395318329*^9, 3.740363953270483*^9}, {
   3.7410679449531727`*^9, 3.741067948530664*^9}, {3.7411646834503117`*^9, 
   3.74116468587321*^9}, {3.741165179680643*^9, 3.741165181922716*^9}, {
   3.74116573241179*^9, 3.741165736966127*^9}, {3.741312754730145*^9, 
   3.741312771899719*^9}, {3.741316988446138*^9, 3.741316989985941*^9}},
 ExpressionUUID -> "f8941efc-1f34-4606-b0c4-0130e6047c2f"],

Cell["\<\
and then consider and stock in matrix forms the coefficients which take part \
in the Second Part of the exchange energy \
\>", "Text",
 CellChangeTimes->{{3.7221584371697073`*^9, 3.7221584415565367`*^9}, {
  3.741313026071665*^9, 3.7413130337851467`*^9}, {3.7413159401083517`*^9, 
  3.741315942972286*^9}}],

Cell[BoxData[
 RowBox[{
  RowBox[{"Coef2CBsr", "[", 
   RowBox[{"M_", ",", "n_"}], "]"}], ":=", 
  RowBox[{"FullSimplify", "[", 
   RowBox[{"Coefficient", "[", 
    RowBox[{
     RowBox[{"(", 
      RowBox[{
       RowBox[{"Coefficient", "[", 
        RowBox[{
         RowBox[{"Series", "[", 
          RowBox[{
           RowBox[{
            FractionBox[
             RowBox[{"6", " ", "+", 
              RowBox[{
               SuperscriptBox["x", "2"], 
               RowBox[{"(", 
                RowBox[{
                 SuperscriptBox["k1", "2"], "+", 
                 SuperscriptBox["k2", "2"]}], ")"}]}]}], 
             RowBox[{" ", 
              SqrtBox[
               RowBox[{
                RowBox[{"(", 
                 RowBox[{"1", "+", " ", 
                  RowBox[{
                   SuperscriptBox["x", "2"], 
                   SuperscriptBox["k1", "2"]}]}], ")"}], " ", 
                RowBox[{"(", 
                 RowBox[{"1", "+", 
                  RowBox[{
                   SuperscriptBox["x", "2"], 
                   SuperscriptBox["k2", "2"]}]}], ")"}]}]], " "}]], "-", 
            "2"}], ",", 
           RowBox[{"{", 
            RowBox[{"x", ",", "0", ",", "M"}], "}"}]}], "]"}], ",", "x", ",", 
         "M"}], "]"}], "/.", 
       RowBox[{"{", 
        RowBox[{"k2", "\[Rule]", "1"}], "}"}]}], ")"}], ",", "k1", ",", "n"}],
     "]"}], "]"}]}]], "Input",
 CellChangeTimes->{{3.741067884946085*^9, 3.741067885275538*^9}, {
  3.741164679322756*^9, 3.7411646796226387`*^9}, {3.741165183607019*^9, 
  3.741165185606667*^9}, {3.74116570682456*^9, 3.7411657305145693`*^9}, {
  3.74131277413778*^9, 3.741312777544195*^9}, {3.74131698130158*^9, 
  3.741316984830863*^9}, {3.7413183165940523`*^9, 3.741318356066781*^9}},
 ExpressionUUID -> "127b6b20-41a8-4f6c-892d-db9ca8e56001"],

Cell[BoxData[
 RowBox[{
  RowBox[{"Coef2CBsr", "=", 
   RowBox[{"Table", "[", 
    RowBox[{
     RowBox[{"Coef2CBsr", "[", 
      RowBox[{
       RowBox[{"2", "i"}], ",", 
       RowBox[{"2", "j"}]}], "]"}], ",", 
     RowBox[{"{", 
      RowBox[{"i", ",", "0", ",", "10"}], "}"}], ",", 
     RowBox[{"{", 
      RowBox[{"j", ",", "0", ",", "10"}], "}"}]}], "]"}]}], ";"}]], "Input",
 CellChangeTimes->{{3.7220573274031277`*^9, 3.722057411958555*^9}, {
   3.722057553909235*^9, 3.722057558258687*^9}, 3.722058361827209*^9, {
   3.722059020563114*^9, 3.722059036001809*^9}, {3.722064043326339*^9, 
   3.7220640436134567`*^9}, {3.722068938617219*^9, 3.7220689488567133`*^9}, 
   3.7220690691792727`*^9, {3.722069129642337*^9, 3.722069129865574*^9}, {
   3.72207100528871*^9, 3.7220711073354273`*^9}, {3.72207151536589*^9, 
   3.722071516470203*^9}, {3.722071548694812*^9, 3.7220715507900457`*^9}, {
   3.722071640791222*^9, 3.7220716428698053`*^9}, {3.722158642706012*^9, 
   3.722158647632127*^9}, {3.7221587753440323`*^9, 3.722158777071834*^9}, {
   3.740299016390862*^9, 3.740299018742794*^9}, {3.740299562999009*^9, 
   3.740299566134993*^9}, {3.740299998439867*^9, 3.740300000263646*^9}, {
   3.7403637773136587`*^9, 3.7403637775028477`*^9}, {3.74036395662405*^9, 
   3.740363957136101*^9}, {3.741067949563488*^9, 3.741067953791477*^9}, {
   3.741164687935804*^9, 3.741164690479032*^9}, {3.741165187387107*^9, 
   3.741165189310234*^9}, {3.741165739048711*^9, 3.741165741896358*^9}, {
   3.741312779166647*^9, 3.7413127880905457`*^9}, {3.741315865935526*^9, 
   3.741315866604557*^9}, {3.741316986157724*^9, 3.741316992367715*^9}},
 ExpressionUUID -> "d113e35f-3b38-47bb-92a0-ed7c56e8adcb"]
}, Closed]],

Cell[CellGroupData[{

Cell["Large-c expansion", "Subsubsection",
 CellChangeTimes->{{3.741164836522542*^9, 3.741164866842805*^9}, {
  3.741316898925234*^9, 3.741316899565893*^9}, {3.741336192175099*^9, 
  3.7413361927979717`*^9}},
 ExpressionUUID -> "2d7f4872-cb17-4d53-8cb9-db2cb4fd1fd0"],

Cell["We have the large-c expansion expression", "Text",
 CellChangeTimes->{{3.724470606233453*^9, 3.724470623578065*^9}, {
  3.7411648516469088`*^9, 3.741164855153366*^9}, {3.741335882966888*^9, 
  3.741335886829115*^9}},
 ExpressionUUID -> "863298f1-c3df-4aeb-9adc-8b1a1d0739f3"],

Cell[BoxData[
 RowBox[{
  RowBox[{"ExRCBsrExpansion", "[", "N_", " ", "]"}], ":=", 
  RowBox[{"Simplify", "[", 
   RowBox[{"Sum", "[", 
    RowBox[{
     RowBox[{
      FractionBox["1", 
       SuperscriptBox["c", 
        RowBox[{"2", "n"}]]], 
      RowBox[{"Simplify", "[", 
       RowBox[{"(", 
        RowBox[{
         RowBox[{
          FractionBox[
           RowBox[{"3", "kF"}], 
           RowBox[{"4", "\[Pi]"}]], 
          RowBox[{"Simplify", "[", 
           RowBox[{"(", 
            RowBox[{
             RowBox[{"If", "[", 
              RowBox[{
               RowBox[{
                RowBox[{"Mod", "[", 
                 RowBox[{"n", ",", "2"}], "]"}], "==", "0"}], ",", 
               RowBox[{"Sum", "[", 
                RowBox[{
                 RowBox[{"2", " ", 
                  RowBox[{"Part", "[", 
                   RowBox[{"Coef1CBsr", ",", 
                    RowBox[{"n", "+", "1"}], ",", 
                    RowBox[{"\[Nu]", "+", "1"}]}], "]"}], 
                  RowBox[{"Simplify", "[", 
                   RowBox[{"(", 
                    RowBox[{
                    RowBox[{"Part1First", "[", 
                    RowBox[{
                    RowBox[{"n", "-", "1", "-", "\[NoBreak]", "\[Nu]"}], ",", 
                    "\[Nu]"}], "]"}], "+", 
                    RowBox[{
                    SuperscriptBox["\[Mu]", "2"], 
                    RowBox[{"Part1SecondminusThird", "[", 
                    RowBox[{
                    RowBox[{"n", "-", "1", "-", "\[NoBreak]", "\[Nu]"}], ",", 
                    "\[NoBreak]", "\[Nu]"}], "]"}]}]}], ")"}], "]"}]}], ",", 
                 RowBox[{"{", 
                  RowBox[{"\[Nu]", ",", "0", ",", 
                   RowBox[{
                    RowBox[{"(", 
                    RowBox[{"n", "-", "2"}], ")"}], "/", "2"}]}], "}"}]}], 
                "]"}], ",", "0"}], "]"}], "+", 
             RowBox[{"If", "[", 
              RowBox[{
               RowBox[{
                RowBox[{"Mod", "[", 
                 RowBox[{"n", ",", "2"}], "]"}], "\[Equal]", "1"}], ",", " ", 
               
               RowBox[{
                RowBox[{
                 RowBox[{"Part", "[", 
                  RowBox[{"Coef1CBsr", ",", 
                   RowBox[{"n", "+", "1"}], ",", 
                   RowBox[{
                    RowBox[{
                    RowBox[{"(", 
                    RowBox[{"n", "-", "1"}], ")"}], "/", "2"}], "+", "1"}]}], 
                  "]"}], 
                 RowBox[{"Simplify", "[", 
                  RowBox[{"(", 
                   RowBox[{
                    RowBox[{"Part1First", "[", 
                    RowBox[{
                    RowBox[{"n", "-", "1", "-", "\[NoBreak]", 
                    RowBox[{
                    RowBox[{"(", 
                    RowBox[{"n", "-", "1"}], ")"}], "/", "2"}]}], ",", 
                    RowBox[{
                    RowBox[{"(", 
                    RowBox[{"n", "-", "1"}], ")"}], "/", "2"}]}], "]"}], "+", 
                    
                    RowBox[{
                    SuperscriptBox["\[Mu]", "2"], 
                    RowBox[{"Part1SecondminusThird", "[", 
                    RowBox[{
                    RowBox[{"n", "-", "1", "-", "\[NoBreak]", 
                    RowBox[{
                    RowBox[{"(", 
                    RowBox[{"n", "-", "1"}], ")"}], "/", "2"}]}], ",", 
                    "\[NoBreak]", 
                    RowBox[{
                    RowBox[{"(", 
                    RowBox[{"n", "-", "1"}], ")"}], "/", "2"}]}], "]"}]}]}], 
                   ")"}], "]"}]}], "+", 
                RowBox[{"Sum", "[", 
                 RowBox[{
                  RowBox[{"2", 
                   RowBox[{"Part", "[", 
                    RowBox[{"Coef1CBsr", ",", 
                    RowBox[{"n", "+", "1"}], ",", 
                    RowBox[{"\[Nu]", "+", "1"}]}], "]"}], 
                   RowBox[{"Simplify", "[", 
                    RowBox[{"(", 
                    RowBox[{
                    RowBox[{"Part1First", "[", 
                    RowBox[{
                    RowBox[{"n", "-", "1", "-", "\[NoBreak]", "\[Nu]"}], ",", 
                    "\[Nu]"}], "]"}], "+", 
                    RowBox[{
                    SuperscriptBox["\[Mu]", "2"], 
                    RowBox[{"Part1SecondminusThird", "[", 
                    RowBox[{
                    RowBox[{"n", "-", "1", "-", "\[NoBreak]", "\[Nu]"}], ",", 
                    "\[NoBreak]", "\[Nu]"}], "]"}]}]}], ")"}], "]"}]}], ",", 
                  RowBox[{"{", 
                   RowBox[{"\[Nu]", ",", "0", ",", 
                    RowBox[{
                    RowBox[{"(", 
                    RowBox[{"n", "-", "3"}], ")"}], "/", "2"}]}], "}"}]}], 
                 "]"}]}], ",", "0"}], "]"}]}], ")"}], "]"}]}], "+", 
         RowBox[{
          FractionBox[
           RowBox[{"3", "kF"}], 
           RowBox[{"16", " ", "\[Pi]"}]], 
          RowBox[{"Simplify", "[", 
           RowBox[{"(", 
            RowBox[{
             RowBox[{"If", "[", 
              RowBox[{
               RowBox[{
                RowBox[{"Mod", "[", 
                 RowBox[{"n", ",", "2"}], "]"}], "\[Equal]", "1"}], ",", 
               RowBox[{"Sum", "[", 
                RowBox[{
                 RowBox[{"2", " ", 
                  RowBox[{"Part", "[", 
                   RowBox[{"Coef2CBsr", ",", 
                    RowBox[{"n", "+", "1"}], ",", 
                    RowBox[{"\[Nu]", "+", "1"}]}], "]"}], 
                  RowBox[{"Simplify", "[", 
                   RowBox[{"(", 
                    RowBox[{
                    RowBox[{"Part2ThirdminusFourth", "[", 
                    RowBox[{
                    RowBox[{"n", "-", "\[NoBreak]", "\[Nu]"}], ",", "\[Nu]"}],
                     "]"}], "-", 
                    RowBox[{"Part2SecondminusFirst", "[", 
                    RowBox[{
                    RowBox[{"n", "-", "\[NoBreak]", "\[Nu]"}], ",", "\[Nu]"}],
                     "]"}]}], ")"}], "]"}]}], ",", 
                 RowBox[{"{", 
                  RowBox[{"\[Nu]", ",", "0", ",", 
                   RowBox[{
                    RowBox[{"(", 
                    RowBox[{"n", "-", "1"}], ")"}], "/", "2"}]}], "}"}]}], 
                "]"}], ",", "0"}], "]"}], "+", 
             RowBox[{"If", "[", 
              RowBox[{
               RowBox[{
                RowBox[{"Mod", "[", 
                 RowBox[{"n", ",", "2"}], "]"}], "\[Equal]", "0"}], ",", " ", 
               
               RowBox[{
                RowBox[{
                 RowBox[{"Part", "[", 
                  RowBox[{"Coef2CBsr", ",", 
                   RowBox[{"n", "+", "1"}], ",", 
                   RowBox[{
                    RowBox[{"n", "/", "2"}], "+", "1"}]}], "]"}], 
                 RowBox[{"Simplify", "[", 
                  RowBox[{"(", 
                   RowBox[{
                    RowBox[{"Part2ThirdminusFourth", "[", 
                    RowBox[{
                    RowBox[{"n", "-", "\[NoBreak]", 
                    RowBox[{"n", "/", "2"}]}], ",", 
                    RowBox[{"n", "/", "2"}]}], "]"}], "-", 
                    RowBox[{"Part2SecondminusFirst", "[", 
                    RowBox[{
                    RowBox[{"n", "-", "\[NoBreak]", 
                    RowBox[{"n", "/", "2"}]}], ",", 
                    RowBox[{"n", "/", "2"}]}], "]"}]}], ")"}], "]"}]}], "+", 
                RowBox[{"Sum", "[", 
                 RowBox[{
                  RowBox[{"2", 
                   RowBox[{"Part", "[", 
                    RowBox[{"Coef2CBsr", ",", 
                    RowBox[{"n", "+", "1"}], ",", 
                    RowBox[{"\[Nu]", "+", "1"}]}], "]"}], 
                   RowBox[{"Simplify", "[", 
                    RowBox[{"(", 
                    RowBox[{
                    RowBox[{"Part2ThirdminusFourth", "[", 
                    RowBox[{
                    RowBox[{"n", "-", "\[NoBreak]", "\[Nu]"}], ",", "\[Nu]"}],
                     "]"}], "-", 
                    RowBox[{"Part2SecondminusFirst", "[", 
                    RowBox[{
                    RowBox[{"n", "-", "\[NoBreak]", "\[Nu]"}], ",", "\[Nu]"}],
                     "]"}]}], ")"}], "]"}]}], ",", 
                  RowBox[{"{", 
                   RowBox[{"\[Nu]", ",", "0", ",", 
                    RowBox[{
                    RowBox[{"(", 
                    RowBox[{"n", "-", "2"}], ")"}], "/", "2"}]}], "}"}]}], 
                 "]"}]}], ",", "0"}], "]"}]}], ")"}], "]"}]}]}], ")"}], 
       "]"}]}], ",", " ", 
     RowBox[{"{", 
      RowBox[{"n", ",", "0", ",", 
       RowBox[{"N", "/", "2"}]}], "}"}]}], "]"}], "]"}]}]], "Input",
 CellChangeTimes->{{3.722754572486408*^9, 3.7227546129606533`*^9}, {
   3.741165015141117*^9, 3.741165045250079*^9}, {3.741165197810758*^9, 
   3.741165254957601*^9}, 3.7413142880801487`*^9, {3.7413170449909363`*^9, 
   3.741317050005517*^9}, {3.7413170942104263`*^9, 3.741317105971739*^9}, {
   3.7413195318276863`*^9, 3.7413195330595627`*^9}},
 ExpressionUUID -> "05d67a11-2aa3-4020-80e7-0a47e86aefb0"],

Cell["\<\
We first calculate the large-c expansion to a satisfying order, let\
\[CloseCurlyQuote]s say 20.\
\>", "Text",
 CellChangeTimes->{{3.722658255655129*^9, 3.722658274741214*^9}, {
  3.741317036142239*^9, 3.7413170380458813`*^9}}],

Cell[BoxData[
 RowBox[{
  RowBox[{"ExRCBsrOrder20", "=", 
   RowBox[{
    StyleBox["ExRCBsrExpansion",
     FontWeight->"Plain"], "[", "20", "]"}]}], ";"}]], "Input",
 CellChangeTimes->{{3.722657885346245*^9, 3.722657905194455*^9}, {
   3.72265917006719*^9, 3.722659250932714*^9}, {3.722763920069398*^9, 
   3.722763928880912*^9}, {3.740299051015119*^9, 3.740299051080347*^9}, {
   3.740363795247789*^9, 3.740363796239716*^9}, {3.7411652585174932`*^9, 
   3.7411652633781548`*^9}, {3.741165795859723*^9, 3.7411657984422483`*^9}, {
   3.741313222841453*^9, 3.741313257225306*^9}, {3.741315481468864*^9, 
   3.741315506042829*^9}, 3.7413170548330317`*^9, {3.7413171211818953`*^9, 
   3.741317124333581*^9}, {3.741319538770235*^9, 3.7413195398281527`*^9}},
 ExpressionUUID -> "069bfa4c-e29a-4264-a8cf-80a3cbdb5355"],

Cell[BoxData[
 RowBox[{
  RowBox[{"ExRCBOrder20", "=", 
   RowBox[{"Limit", "[", 
    RowBox[{"ExRCBsrOrder20", ",", 
     RowBox[{"\[Mu]", "\[Rule]", "0"}]}], "]"}]}], ";"}]], "Input",
 CellChangeTimes->{
  3.7227558995802526`*^9, {3.7411657967815123`*^9, 3.7411657994598923`*^9}, 
   3.741313225929617*^9, {3.741313263481997*^9, 3.741313264425818*^9}, {
   3.741315509596798*^9, 3.741315510780417*^9}, {3.741316041485497*^9, 
   3.741316043549305*^9}, {3.741317122959085*^9, 3.7413171269906683`*^9}},
 ExpressionUUID -> "50fc455a-582e-4497-95b1-a9e9763bb1ea"]
}, Closed]],

Cell[CellGroupData[{

Cell["Pad\[EAcute] approximants", "Subsubsection",
 CellChangeTimes->{{3.7411649136217203`*^9, 3.741164917030664*^9}, {
  3.741164959746048*^9, 3.741164964829475*^9}, {3.741336245901672*^9, 
  3.741336246397785*^9}},
 ExpressionUUID -> "8337f428-a3aa-4a57-95c4-e1acad9b96a8"],

Cell["\<\
We prepare the coefficient of the large-c expansion for the short-range \
exchange energy and for the \[Mu] \[RightArrow] 0 limit\
\>", "Text",
 CellChangeTimes->{{3.7227553188603687`*^9, 3.722755371373106*^9}, {
   3.72275562759557*^9, 3.7227556515776443`*^9}, {3.724470657833439*^9, 
   3.72447066020118*^9}, {3.741315414203617*^9, 3.741315470363694*^9}, 
   3.741408113867116*^9}],

Cell[BoxData[
 RowBox[{
  RowBox[{"CoefficientCBsr", "[", 
   RowBox[{"M_", ",", "n_"}], "]"}], ":=", 
  RowBox[{"Simplify", "[", 
   RowBox[{"Coefficient", "[", 
    RowBox[{
     RowBox[{"ExRCBsrOrder20", "/.", 
      RowBox[{"{", 
       RowBox[{"c", "\[Rule]", 
        RowBox[{"1", "/", "x"}]}], "}"}]}], ",", "x", ",", "n"}], "]"}], 
   "]"}]}]], "Input",
 CellChangeTimes->{{3.7226678420237913`*^9, 3.722667861528064*^9}, {
   3.72266815372162*^9, 3.7226681849194813`*^9}, {3.7226721981498747`*^9, 
   3.722672207155808*^9}, 3.7227550567672377`*^9, {3.722755656577574*^9, 
   3.7227556642370653`*^9}, {3.741165279910945*^9, 3.741165280303294*^9}, {
   3.741165801108734*^9, 3.741165802557379*^9}, {3.741314586153861*^9, 
   3.741314586281663*^9}, {3.7413148850075493`*^9, 3.741314885241417*^9}, {
   3.741315516652811*^9, 3.7413155175013733`*^9}, {3.741317163840336*^9, 
   3.741317166336734*^9}},
 ExpressionUUID -> "1406cbfc-301a-43ac-960c-f892ff571a64"],

Cell[BoxData[
 RowBox[{
  RowBox[{"CoefficientCB", "[", 
   RowBox[{"M_", ",", "n_"}], "]"}], ":=", 
  RowBox[{"Simplify", "[", 
   RowBox[{"Coefficient", "[", 
    RowBox[{
     RowBox[{"ExRCBOrder20", "/.", 
      RowBox[{"{", 
       RowBox[{"c", "\[Rule]", 
        RowBox[{"1", "/", "x"}]}], "}"}]}], ",", "x", ",", "n"}], "]"}], 
   "]"}]}]], "Input",
 CellChangeTimes->{{3.7227556735963917`*^9, 3.7227556754363728`*^9}, {
   3.741165291318172*^9, 3.7411653095641212`*^9}, {3.7411658075165567`*^9, 
   3.741165809802228*^9}, {3.741314633492703*^9, 3.741314634757943*^9}, 
   3.741314919610902*^9, {3.741315520381742*^9, 3.741315521149824*^9}, {
   3.7413171687525177`*^9, 3.741317170207755*^9}},
 ExpressionUUID -> "2589e2ec-9b7e-419a-90a8-0433937ec42c"],

Cell[BoxData[
 RowBox[{
  RowBox[{"CoefCBsr", "[", "M_", "]"}], ":=", 
  RowBox[{"Table", "[", 
   RowBox[{
    RowBox[{
     SubscriptBox["T", "i"], "->", 
     RowBox[{"CoefficientCBsr", "[", 
      RowBox[{"M", ",", "i"}], "]"}]}], ",", 
    RowBox[{"{", 
     RowBox[{"i", ",", "0", ",", "M"}], "}"}]}], "]"}]}]], "Input",
 CellChangeTimes->{{3.722749765088842*^9, 3.722749844950129*^9}, {
   3.72275111355685*^9, 3.7227511736510963`*^9}, {3.7227512675099688`*^9, 
   3.722751272325121*^9}, 3.722752713870413*^9, {3.7227542354300613`*^9, 
   3.722754236382597*^9}, {3.722755666317625*^9, 3.7227556680165157`*^9}, {
   3.7411652856659613`*^9, 3.741165288839732*^9}, {3.741165803964905*^9, 
   3.741165805816494*^9}, {3.741314890229391*^9, 3.741314893738743*^9}, {
   3.7413149288437023`*^9, 3.741314934843973*^9}, {3.741317171137334*^9, 
   3.741317173008121*^9}},
 ExpressionUUID -> "8b73be0b-7e9a-449f-a15b-668a721cf499"],

Cell[BoxData[
 RowBox[{
  RowBox[{"CoefCB", "[", "M_", "]"}], ":=", 
  RowBox[{"Table", "[", 
   RowBox[{
    RowBox[{
     SubscriptBox["T", "i"], "->", 
     RowBox[{"CoefficientCB", "[", 
      RowBox[{"M", ",", "i"}], "]"}]}], ",", 
    RowBox[{"{", 
     RowBox[{"i", ",", "0", ",", "M"}], "}"}]}], "]"}]}]], "Input",
 CellChangeTimes->{{3.722755679643105*^9, 3.722755680670816*^9}, {
   3.7411652967818327`*^9, 3.7411652992974167`*^9}, 3.7411658123477707`*^9, 
   3.7411662521890163`*^9, {3.741314937994246*^9, 3.741314954859644*^9}, {
   3.741317171872368*^9, 3.741317174943747*^9}},
 ExpressionUUID -> "2206b0ab-be15-4179-8235-4327de1fe24e"],

Cell["\<\
We now express the specific coefficients for our Pad\[EAcute] approximant \
using the order-20 large-c expansion\
\>", "Text",
 CellChangeTimes->{{3.722763848195755*^9, 3.722763880899667*^9}, {
  3.741315729450776*^9, 3.7413157473068323`*^9}, {3.741336257341878*^9, 
  3.741336266557869*^9}},ExpressionUUID->"54576dfe-7cdd-4295-9d77-\
1e5ca59e1357"],

Cell[BoxData[
 RowBox[{
  RowBox[{"CoefBPad\[EAcute]CB", "=", 
   RowBox[{
    RowBox[{"CoefBPad\[EAcute]", "[", "10", "]"}], "/.", 
    RowBox[{"CoefCB", "[", "20", "]"}]}]}], ";"}]], "Input",
 CellChangeTimes->{{3.722753594171132*^9, 3.722753620589405*^9}, 
   3.722753773971465*^9, 3.722753896092773*^9, {3.722754258580085*^9, 
   3.7227542587988586`*^9}, {3.722754465761252*^9, 3.722754485745597*^9}, {
   3.72275541074507*^9, 3.722755440462531*^9}, {3.722755709305892*^9, 
   3.7227557107485*^9}, {3.7227560316951523`*^9, 3.722756055026368*^9}, {
   3.722756395457559*^9, 3.722756409823081*^9}, {3.741165336843622*^9, 
   3.741165357183463*^9}, {3.741165825467124*^9, 3.7411658299082203`*^9}, {
   3.7413149650996237`*^9, 3.7413149699957933`*^9}, {3.741315265420334*^9, 
   3.741315266187937*^9}, {3.741315550782506*^9, 3.7413155823186483`*^9}, {
   3.741315643371585*^9, 3.741315647437683*^9}, {3.7413171802708197`*^9, 
   3.741317189296322*^9}},
 ExpressionUUID -> "cf32c0d3-09c7-4575-bf34-c5efe816ae85"],

Cell[BoxData[
 RowBox[{
  RowBox[{"CoefBPad\[EAcute]CBsr", "=", 
   RowBox[{
    RowBox[{"CoefBPad\[EAcute]", "[", "10", "]"}], "/.", 
    RowBox[{"CoefCBsr", "[", "20", "]"}]}]}], ";"}]], "Input",
 CellChangeTimes->{{3.7227563927641907`*^9, 3.722756424828418*^9}, {
  3.722756470028845*^9, 3.722756471262659*^9}, {3.741165338166099*^9, 
  3.74116535636982*^9}, {3.741165826280868*^9, 3.741165830758252*^9}, {
  3.741314982347934*^9, 3.7413149848775673`*^9}, {3.741315268045794*^9, 
  3.74131526958106*^9}, {3.741315564238062*^9, 3.741315585069827*^9}, {
  3.741315648332552*^9, 3.741315649151641*^9}, {3.741317181311077*^9, 
  3.74131719129498*^9}},
 ExpressionUUID -> "97dbb62f-da46-4012-9537-599545f24376"],

Cell[BoxData[
 RowBox[{
  RowBox[{"CoefAPad\[EAcute]CB", "=", 
   RowBox[{
    RowBox[{"CoefAPad\[EAcute]", "[", "10", "]"}], "/.", 
    RowBox[{"CoefCB", "[", "20", "]"}]}]}], ";"}]], "Input",
 CellChangeTimes->{{3.722754029546383*^9, 3.722754044308186*^9}, {
   3.722754301982415*^9, 3.722754302035227*^9}, {3.7227544718864326`*^9, 
   3.722754488205662*^9}, {3.722755452684111*^9, 3.722755452924046*^9}, 
   3.7227557289252*^9, {3.722756027149149*^9, 3.722756058413001*^9}, 
   3.722756119853417*^9, 3.722756296716875*^9, {3.722756447367597*^9, 
   3.722756450307869*^9}, {3.741165339561618*^9, 3.741165355379118*^9}, {
   3.741165827109076*^9, 3.741165832083321*^9}, {3.741314987228261*^9, 
   3.7413149885234613`*^9}, {3.741315271836527*^9, 3.741315272429305*^9}, {
   3.7413155708925943`*^9, 3.741315586204362*^9}, {3.741315650300768*^9, 
   3.741315651546886*^9}, {3.741317182383655*^9, 3.741317192575685*^9}},
 ExpressionUUID -> "ee416689-2436-40d2-9581-eb4cef77d76a"],

Cell[BoxData[
 RowBox[{
  RowBox[{"CoefAPad\[EAcute]CBsr", "=", 
   RowBox[{
    RowBox[{"CoefAPad\[EAcute]", "[", "10", "]"}], "/.", 
    RowBox[{"CoefCBsr", "[", "20", "]"}]}]}], ";"}]], "Input",
 CellChangeTimes->{{3.722756457980381*^9, 3.722756467531996*^9}, {
  3.741165343013163*^9, 3.741165354109902*^9}, {3.741165828153932*^9, 
  3.741165833829134*^9}, {3.741314992123789*^9, 3.741314992987317*^9}, {
  3.741315274700562*^9, 3.741315280252084*^9}, {3.74131558898942*^9, 
  3.741315591501307*^9}, {3.741315652989523*^9, 3.7413156541452312`*^9}, {
  3.7413171836345167`*^9, 3.741317193758781*^9}},
 ExpressionUUID -> "572d5ae0-cc56-499c-a412-a3727f02dc7c"],

Cell["\<\
We can now define our Pad\[EAcute] approximants for the full-range and the \
short-range Coulomb-Breit exchange energies per particle\
\>", "Text",
 CellChangeTimes->{{3.7227640074737988`*^9, 3.722764017491691*^9}, {
  3.741336272956201*^9, 3.741336298059808*^9}},
 ExpressionUUID -> "a8589cfc-f394-44e2-9ff0-36d20fb38cd8"],

Cell[BoxData[
 RowBox[{
  RowBox[{"ExRCBPad\[EAcute]", " ", "[", "M_", "]"}], ":=", 
  RowBox[{
   RowBox[{"(", 
    RowBox[{"Sum", "[", 
     RowBox[{
      FractionBox[
       RowBox[{"Part", "[", 
        RowBox[{"CoefAPad\[EAcute]CB", ",", "M", ",", 
         RowBox[{"k", "+", "1"}]}], "]"}], 
       SuperscriptBox["c", "k"]], ",", 
      RowBox[{"{", 
       RowBox[{"k", ",", "0", ",", "M"}], "}"}]}], "]"}], ")"}], "/", 
   RowBox[{"(", 
    RowBox[{"1", "+", 
     RowBox[{"Sum", "[", 
      RowBox[{
       FractionBox[
        RowBox[{"Part", "[", 
         RowBox[{"CoefBPad\[EAcute]CB", ",", "M", ",", "k"}], "]"}], 
        SuperscriptBox["c", "k"]], ",", 
       RowBox[{"{", 
        RowBox[{"k", ",", "1", ",", "M"}], "}"}]}], "]"}]}], 
    ")"}]}]}]], "Input",
 CellChangeTimes->{{3.7227562198866377`*^9, 3.722756223232061*^9}, {
  3.722756344477265*^9, 3.722756374429248*^9}, {3.724472328737096*^9, 
  3.7244723404597588`*^9}, {3.7244725391989813`*^9, 3.724472541421919*^9}, {
  3.7244732518101883`*^9, 3.724473255736369*^9}, {3.7411651613833103`*^9, 
  3.741165167052189*^9}, {3.7411653461762133`*^9, 3.7411653497927322`*^9}, {
  3.741165839085773*^9, 3.741165845925786*^9}, {3.7413156004345922`*^9, 
  3.7413156087854156`*^9}, {3.741316207389226*^9, 3.7413162096777487`*^9}, {
  3.7413172006726522`*^9, 3.741317206304834*^9}, {3.741319553107644*^9, 
  3.741319555457955*^9}},
 ExpressionUUID -> "acb5750c-3d70-4332-828d-a97bb35318ee"],

Cell[BoxData[
 RowBox[{
  RowBox[{"ExRCBsrPad\[EAcute]", "[", "M_", "]"}], ":=", 
  RowBox[{
   RowBox[{"(", 
    RowBox[{"Sum", "[", 
     RowBox[{
      FractionBox[
       RowBox[{"Part", "[", 
        RowBox[{"CoefAPad\[EAcute]CBsr", ",", "M", ",", 
         RowBox[{"k", "+", "1"}]}], "]"}], 
       SuperscriptBox["c", "k"]], ",", 
      RowBox[{"{", 
       RowBox[{"k", ",", "0", ",", "M"}], "}"}]}], "]"}], ")"}], "/", 
   RowBox[{"(", 
    RowBox[{"1", "+", 
     RowBox[{"Sum", "[", 
      RowBox[{
       FractionBox[
        RowBox[{"Part", "[", 
         RowBox[{"CoefBPad\[EAcute]CBsr", ",", "M", ",", "k"}], "]"}], 
        SuperscriptBox["c", "k"]], ",", 
       RowBox[{"{", 
        RowBox[{"k", ",", "1", ",", "M"}], "}"}]}], "]"}]}], 
    ")"}]}]}]], "Input",
 CellChangeTimes->{{3.722754133946948*^9, 3.722754168197061*^9}, 
   3.722755764286047*^9, {3.722755795648616*^9, 3.7227557972443647`*^9}, {
   3.722756165936594*^9, 3.7227562108616667`*^9}, {3.722756481371945*^9, 
   3.722756490285556*^9}, {3.724472343389707*^9, 3.724472353121357*^9}, {
   3.724473258746921*^9, 3.724473263323648*^9}, {3.741165168482983*^9, 
   3.741165168762787*^9}, {3.7411653511334343`*^9, 3.741165353067666*^9}, {
   3.7411658422331877`*^9, 3.741165847801704*^9}, {3.741315603778873*^9, 
   3.741315606040073*^9}, {3.741316210380775*^9, 3.741316213918049*^9}, {
   3.741317204271682*^9, 3.741317209296047*^9}, {3.741319552498263*^9, 
   3.741319557377345*^9}},
 ExpressionUUID -> "6c765e43-939b-42be-acda-e29fb0dfc8fb"]
}, Closed]]
}, Closed]],

Cell[CellGroupData[{

Cell["Tests", "Subsection",
 CellChangeTimes->{{3.7411646556876497`*^9, 3.741164658735076*^9}}],

Cell[CellGroupData[{

Cell["Full-range Coulomb-Breit exchange energy per particle", "Subsubsection",
 CellChangeTimes->{{3.741166404504117*^9, 3.74116641070641*^9}, {
   3.741167541886691*^9, 3.7411675425073566`*^9}, {3.741168333819334*^9, 
   3.741168335505926*^9}, 3.741317345474846*^9, 3.741317827137011*^9, 
   3.741321459049239*^9, {3.7413363084281607`*^9, 3.741336319549921*^9}},
 ExpressionUUID -> "8c46be18-9638-41c1-a77d-6cc07feaedde"],

Cell[CellGroupData[{

Cell[BoxData[
 RowBox[{"ExRCBPad\[EAcute]2", "=", 
  RowBox[{"Simplify", "[", 
   RowBox[{"ExRCBPad\[EAcute]", "[", "2", "]"}], "]"}]}]], "Input",
 CellChangeTimes->{{3.741321460133788*^9, 3.741321473045063*^9}},
 ExpressionUUID -> "45f34441-4b0c-428c-805c-89a2f689dfe8"],

Cell[BoxData[
 FractionBox[
  RowBox[{
   RowBox[{"3", " ", "kF"}], "-", 
   RowBox[{"360", " ", 
    SuperscriptBox["c", "2"], " ", "kF"}]}], 
  RowBox[{
   RowBox[{"316", " ", "\[Pi]"}], "+", 
   RowBox[{"480", " ", 
    SuperscriptBox["c", "2"], " ", "\[Pi]"}]}]]], "Output",
 CellChangeTimes->{{3.7413215107533283`*^9, 3.741321510835943*^9}, 
   3.741336331704485*^9, 3.741407719481429*^9, 3.741409698563037*^9, 
   3.7414098736304893`*^9},
 ExpressionUUID -> "0eed0191-1251-4a6f-b65e-3e920ee31c3b"]
}, Open  ]],

Cell[CellGroupData[{

Cell[BoxData[
 RowBox[{"ExRCBPad\[EAcute]4", "=", 
  RowBox[{"Simplify", "[", 
   RowBox[{"ExRCBPad\[EAcute]", "[", "4", "]"}], "]"}]}]], "Input",
 CellChangeTimes->{{3.741317837207673*^9, 3.741317840816615*^9}, {
  3.741321467124851*^9, 3.741321475062307*^9}},
 ExpressionUUID -> "c397f0cc-d072-42f2-8f4f-f807b992da61"],

Cell[BoxData[
 RowBox[{"-", 
  FractionBox[
   RowBox[{
    RowBox[{"(", 
     RowBox[{
      RowBox[{"-", "257731"}], "+", 
      RowBox[{"2979480", " ", 
       SuperscriptBox["c", "2"]}], "+", 
      RowBox[{"5434380", " ", 
       SuperscriptBox["c", "4"]}]}], ")"}], " ", "kF"}], 
   RowBox[{"240", " ", 
    RowBox[{"(", 
     RowBox[{"9771", "+", 
      RowBox[{"36680", " ", 
       SuperscriptBox["c", "2"]}], "+", 
      RowBox[{"30191", " ", 
       SuperscriptBox["c", "4"]}]}], ")"}], " ", "\[Pi]"}]]}]], "Output",
 CellChangeTimes->{3.74131784160071*^9, 3.741318068355565*^9, 
  3.741318498789768*^9, 3.7413185440542917`*^9, 3.741321510919129*^9, 
  3.741336331766756*^9, 3.741407719663846*^9, 3.74140970087391*^9, 
  3.741409873787133*^9},
 ExpressionUUID -> "5edd830e-c074-437d-af00-9f8273d88419"]
}, Open  ]],

Cell[CellGroupData[{

Cell[BoxData[
 RowBox[{"ExRCBPad\[EAcute]6", "=", 
  RowBox[{"Simplify", "[", 
   RowBox[{"ExRCBPad\[EAcute]", "[", "6", "]"}], "]"}]}]], "Input",
 CellChangeTimes->{{3.741317225501252*^9, 3.741317226637229*^9}, {
  3.741321480823491*^9, 3.741321482644245*^9}},
 ExpressionUUID -> "0ceed1ab-5d69-40ee-be37-c6132b29719d"],

Cell[BoxData[
 RowBox[{"-", 
  FractionBox[
   RowBox[{
    RowBox[{"(", 
     RowBox[{
      RowBox[{"-", "16903484947"}], "+", 
      RowBox[{"130008734584", " ", 
       SuperscriptBox["c", "2"]}], "+", 
      RowBox[{"738591716940", " ", 
       SuperscriptBox["c", "4"]}], "+", 
      RowBox[{"685393188480", " ", 
       SuperscriptBox["c", "6"]}]}], ")"}], " ", "kF"}], 
   RowBox[{"80", " ", 
    RowBox[{"(", 
     RowBox[{"1557582577", "+", 
      RowBox[{"10436849208", " ", 
       SuperscriptBox["c", "2"]}], "+", 
      RowBox[{"19925341821", " ", 
       SuperscriptBox["c", "4"]}], "+", 
      RowBox[{"11423219808", " ", 
       SuperscriptBox["c", "6"]}]}], ")"}], " ", "\[Pi]"}]]}]], "Output",
 CellChangeTimes->{3.741317267926578*^9, 3.741318068565544*^9, 
  3.741318498900236*^9, 3.741321510991588*^9, 3.741336331799388*^9, 
  3.741409761852223*^9, 3.7414098739356537`*^9, 3.741410742083489*^9},
 ExpressionUUID -> "92bab5ee-b979-40be-b364-ed203813c872"]
}, Open  ]],

Cell[BoxData[
 RowBox[{
  RowBox[{"ExRCBPad\[EAcute]8", "=", 
   RowBox[{"Simplify", "[", 
    RowBox[{"ExRCBPad\[EAcute]", "[", "8", "]"}], "]"}]}], ";"}]], "Input",
 CellChangeTimes->{{3.741410708715969*^9, 3.741410710315734*^9}, {
  3.7414107438447104`*^9, 3.74141074409336*^9}}],

Cell[CellGroupData[{

Cell[BoxData[
 RowBox[{"Plot", "[", 
  RowBox[{
   RowBox[{"{", 
    RowBox[{
     RowBox[{"ExRCB", "/.", 
      RowBox[{"{", 
       RowBox[{"c", "\[Rule]", 
        RowBox[{"137.036", "/", "kF"}]}], "}"}]}], ",", 
     RowBox[{"ExRCBsrOrder20", "/.", 
      RowBox[{"{", 
       RowBox[{"c", "\[Rule]", 
        RowBox[{"137.036", "/", "kF"}]}], "}"}]}], ",", 
     RowBox[{"ExRCBPad\[EAcute]2", "/.", 
      RowBox[{"{", 
       RowBox[{"c", "\[Rule]", 
        RowBox[{"137.036", "/", "kF"}]}], "}"}]}], ",", 
     RowBox[{"ExRCBPad\[EAcute]4", "/.", 
      RowBox[{"{", 
       RowBox[{"c", "\[Rule]", 
        RowBox[{"137.036", "/", "kF"}]}], "}"}]}], ",", 
     RowBox[{"ExRCBPad\[EAcute]6", "/.", 
      RowBox[{"{", 
       RowBox[{"c", "\[Rule]", 
        RowBox[{"137.036", "/", "kF"}]}], "}"}]}]}], "}"}], ",", 
   RowBox[{"{", 
    RowBox[{"kF", ",", "0", ",", "300"}], "}"}], ",", 
   RowBox[{"PlotStyle", "\[Rule]", 
    RowBox[{"{", 
     RowBox[{"Blue", ",", "Red", ",", "Green", ",", "Purple", ",", "White"}], 
     "}"}]}]}], "]"}]], "Input",
 CellChangeTimes->{{3.725790426404578*^9, 3.725790453840857*^9}, {
   3.725790502785564*^9, 3.725790550992629*^9}, {3.726898837998486*^9, 
   3.726898847052638*^9}, {3.741165900638431*^9, 3.7411659400545387`*^9}, {
   3.741166056629149*^9, 3.741166057200569*^9}, {3.741167570406251*^9, 
   3.741167578360379*^9}, {3.7411676879490023`*^9, 3.741167733059924*^9}, {
   3.7411683511705103`*^9, 3.7411683875175333`*^9}, {3.741317765906069*^9, 
   3.741317768479063*^9}, 3.7413178131487017`*^9, {3.741317848321776*^9, 
   3.7413178490895643`*^9}, {3.741321493221766*^9, 3.741321498596739*^9}, {
   3.7414077516612453`*^9, 3.741407751761806*^9}},
 ExpressionUUID -> "54336d13-6168-476a-96f7-1665bcd2c24e"],

Cell[BoxData[
 GraphicsBox[{{{}, {}, 
    TagBox[
     {RGBColor[0, 0, 1], AbsoluteThickness[1.6], Opacity[1.], 
      LineBox[CompressedData["
1:eJwt13k4Vd/XAHDKlEjJVKGUjJnuMWa4K5lTkVLme8+5hBQuGRKKJBlKpBIl
U0XmKCV3RymKr1SoVDSQyJC5gd/ufd7zz3k+z7nP3mftu/da68iR/rs8F3Fx
cW3i5uL6d9cQ/tVhn3KHzvX/V0KTe9c/M0sMRkSOZnDOvo2JkE15Qn9a+yh6
LrKQM6JUzHu66AVdZ0xV48GHck76l/RWnpQuuuqo5oBuVA1nc07U+ejA9/TD
8o0VNTJ1nDG12+qRRX30JC6l3qwPiJMxmD09kzxAL409dUc8qonj8+Scc3X0
d/qDXTeL2rY3c4wK4uvZgT/o00sVuU/IPOcElus3hhSN00svJd5if2jnSPqt
TxxPnqFvPFOacS+yk8P1Ttq4nW+OHpR2fffJr12c79aSo6XRv+g5q5bZ7Nz+
hlOnKOTgF/iXbv3X+HeXdA+nYvxIclARNzj0vVrb+76Xs7eEtWckmR+0Qif8
qKP9nOdfmKVuNgIQarKhQUlzgAPSHvytfEtg3T4xl6HPAxyVRKfa4mhBOC+Q
sLB/2yDnj/cOGZ9AYZCtbmg2Wj3MsRfN+hlYtAJ8SnOGct6NcWZa4+4NJ0vC
YvfZv6Kh0xwWXVB/xaQkZIqpudO7pzkd5SnVOs5S8MTcN93bYIZTmnahPEph
FQTp12yv+D3DYTndLFzOWQ1tP/kiVx+b43R8eX5Oe0wGJk6NrodTfzhdfxN0
TJTXg/Vqn4YHNtyoSuyF8MlEJegppMK97fhRgKp2+wNDGmRfS77nqrMCSVjO
pDev1IfsNdasLfESaOKBpG+urwnkfEpYK7tWGsV5yEpdUDGFiesVewXOrUO3
kj1it3qYg+jjRQKiKhvQmnBXv9kTVmB55/SWztSN6PrNd60ng7fB+bGLtvtL
FFFbfMKdiLwd4BSzzzKiTRmdft0jtLHNDsS/sANP5Kui9scdR5dv3QUMW8uk
rbZq6ItQr2ZZlwO8/auu6zKijuJD1K9ttt8D97PetrYqaKIZ3fQ94d8d4b25
Uvzedk20tLPLyujoPnjbul/MiNRCpRdcZ4d+OkFjavuhlG4ttFxA9YT5nBOk
vd816ftWC7HD5kSuLjhByC5JM4seLaTjlKG4S8gZYoPNt8591EJ1q9sd7250
huzIXU12A1qoJXtr9Yl9zkCz3728aUoL9eepsGXqncHq2fYtz1bQkGz57NCO
BBcwcRVHthY0JLjxrorRGRcYyz/+o8GShqYvhfoon3cBx5U1q/Staagtdrp/
8TUX4Jcy9F9rS0NReyf77t51gcXrRcU+2dPQh/nRrvXfXGAD3y9/PTcaurJ9
oHHawhWWc0+2bAiiIZmh15ev8LiB/JXF88JZNMR6UHBdcKkb9DfoMTyyaejW
mcNVISvcgDkol1d2hYY2a4s/2yHrBtJ06ee212jIMXL3r3k9N5CQfFIRXkhD
Z0Ve7vM44AbCWdy8V8ppiEe7XXxdhxskOgqeF31EQ9v4cuSSut2A2zkxCR7T
0Lluf7XZD24wljPud7CJhuQiRczbh9ygterwYONTGjJp2hF8jNcdwuzTuqlW
Ggrd19rRq+8OkyPjT/07aej70ZYz1666wylm1cPaAfy+TedvjRa4g/a8bjj6
RkOHljObjW+5Q/TPYtWmQRoaz5tZ9PauO5je9IxpG6Kh2Rb5ENEOd/h24Pff
jlEa4lsV7RrL4wH07R2s4hkaWl9NKHv6eICTd23RZT4CfZmfN6/y9wA0lbQ5
hp9AhVYtJHeIB6zM1m7dL0Ag5R5GVnaMB1Qt/PmtIUggzcUpIp2XPWC+yuXk
bWECmdh/m7Jo84C4b1fjUsQIVBKyg5m+igEZ0PwtXo5AL7M3WcdJM8BRzWVy
y3oCzT0S1ApZy4A/PkEqv7HNVz7h2reRAZ/5eSQPyBPofRk9Z40WA3KlTGdA
kUDCg5ofc60YUHdiOffjTQQ66LLSrSKUAScsynI09AiUFjNulnuEAWV2roz/
sGtv/rcpLZIB40Izdof0CcQ7m/gnOJYBV2QaHt80IFB2Ok+W/hkGEFXmiyWN
CNTaOvWWU8iAJp3bv1qAQGrQva/tNQN4dxhDpjWBuDJMrs93M0DE5eBjVRsC
vRrKn1LvYYClfY17HfbRC4HnznxiQMX0+ba32wjUMiL43G6UAcZyOUVCOwjk
lW1MfynABM9fAUlmuwi0eSIvebEQE3iEjgU+wRa2FuwhRJjA+VFxyNqBQLcn
O8PSxZmw8DO60mY3gRbbBlTuWc+EJbntXqaOBMr5lbux25AJ2dpn7/E5EyjY
bkmwAJ0J3nyz9Ahsy0L/Bn1TJhgnxPeNYI/YG3lcsmICfZXskZcuBDK++fqi
8x4mlLqqCpxzI9DbvQJC7w8x4Xtdw39fGARaWX3wZ981Jmwmjz/75EWgTcm2
q3vymXDgrXy4zn4CmXmqmnZeZ8KGEKn98dgh4oOpLSVM0DOs51H2JlD3YZZW
VS0TpBoLbCkfAl3RdQk48YIJlqv7DG8fINCdZZsvRr1igkROHt9v7PZ+KRTW
xQRR52GxLX4E4r7QKXLwPROOqLz/04LNmrEv2zPIhB69VwuvDxJI5a7ViAI3
CSk3H80/9SfQ1rOKEnI8JPR29aziCSCQqzefyRp+Er6fLY4wwU6WepQsIkxC
WL+eWAX2WBhdbVaKBCr30pXkQAItsZfd83MNCeYdE5MN2OuV/x4dliXhaVBm
2gy2w5t7z3vlSVh36kKRO5tANQa6fs2aJCzMd5vJBxHovxXi6Y0ECWMjsp8d
sL8NTtx/oEuCQIH5sxjsVZkVSyuNSJAQWwj/gH3016biTCsSylj5jsnBBNpy
f8P3AwwSvkTU6DcfJpDkzmOr91IkxBXVdA1j//jUY2PqRcKTveUtIiEEuiSY
USzlR0LJDdsSB+xxJ4GDj0NJOCq90/cl9pMfrOzyIyREsraUjmNnH3/YejmS
hJaIAkuRUAJZ3zyizo4lYdeTqAgr7Guzw6OyZ0gI18kYrsQOTbJeJ3iOhDcn
9fqeYW9fV2g3lU6CjPvDTV+w5yw9Kp5lkrA7yrpZNAzH/+5+X002CUihYLUy
doG/lGhuDglzK/MbTbDtL7xghxWSEENYyHhjK6qq51E3Sdh21qItAvtv/emX
O26R4BCf35WCfbN/q/bGShJu7SQmK7G5dWumXjwg4a1ChdMEdlezqMIDRIIi
o6qDOxznGzd/xxuNJAhnnywQwXaKU7oT1UxC/h4nJ2VsjVVxAz7PSQh1rt6s
g81b0ie55z8S+A9fDgHsileZYaqvSdhcWT+/Gzvee+aGRDcJKxT3bXPHdvvj
8Ib7HQkejtoTXtjE2fIlP96TULf3+PQh7CXywpu7e3E8Rgf3hGB/vOPj2/gZ
75dlCssjsau3NWWW9pOg3f5GIRY78eP6Z5cGSSiOqrl0CpsZFP37xDAJnGXf
vZOx9fh7VANGSTh2KDc9FVv4sr6ry088XpywzHnsz+rnkyymSLhIc1p0Ebu2
YbxOa5YEBbsqs0zsM447fkj/JuFumfWXy9ie34tkBOZJMJS26cvCNozi3zHB
RUG10yfDbOwVoqyoD4sp6JSHyX/PBwpQaTMfBfpEquA/PzCQ+Xh7CQXHicXR
/8ZPaw0XyRGiQLO10f7f/D7MTnqiCAWBOVyx/96PPkULCBGl4KDFgOg5bPGE
MzlMcQoI+wLuFOwh6eF2WykKtm3z3pmA/bDcilt/DR7/rtuff+tjFqR2kZSl
QK2Y79i/9XuqI6qRLEfBZ6uPFv/W13Z2+vEdeQq8UuXs/61/+713rp8UKfgR
zn/VE3t3JJoQUqVg8keLpit2F73gtJ46BV1tBXy7sD88OnQ3SZuCG8oJ0YbY
ZLzDzjt6FGQRvBs0sL9a6/f3baYguiV66Xrs4TZuMb0tFMjt3HuLFzsgtb+I
aUZBSoSi5zTejxMOz7YkWVKgUNlD9WP/6k7379uO47HpIR5hR10O5xOyp4Dv
0iXe/9vP7u7ZurspWPZMTvYqtsBnxWeJzhQMbgmTD8VOKhAia9xwvOtqRUns
5d7js70MCsoli6xssSV/3FPQ3U8BQ+R4kix2ZtnVBwxfCvbvfZPJhy3LPrE7
8SCe37xp/Ac+rwoz22N6g3C8GqZH7mFrc/e9P32Mgsvlf37bYN9tfBxcHUvB
9ID2HjVsw5NFS3tPUuA/9HR2Gbbp0mADnWQKtOUG1rbjfGIvzn/+4yUKmo6p
TVpjv+oaUhXMpsDw8uFCBex9me0N2jkUfF30IX8RNmNt5lhCIV5fjfGTd3E+
O6SsZqtdhef/aNW/Bvvn0IrP7jUUiJ65v/AT58PDpdPhCbUUmDKW72/GPkqg
6x84FBjFwbpg7NPGDosTnlPwx+qN6UOcT6/bh997/5WCjKi68M04PwdkdKp0
fKNgtHrpEkFs/XfE5aYhCuKmTbne4HzewhqJKBunwOy4jOJh7OFQyvj4Xwo2
HPBzKcT1gXZlO5IXZ8Etv7y44UME+v2pSHOVFAse14XeqMR+pChwTXgNC/Yu
LOiEYe+paDg+vY4FFeofUrmxwx7pbX26iQWbpG/ZC+N6Vf9drumAGQv2HbCW
WoLrXbxGtC7DEv9+RO73Y18C2QX3FO62YUHei8BtMdh9fzPije1YEOapqDOH
6yfPCiFrEVcWNJVUa/Xi+mqjN/2sMogFkVXXps7h+vw6tuXFXC4Lcm/zv0li
4vMxU3ZDrZAF2s/7MjSxG3zPRzNvsmD5toXSl7i+l9oz1JrLWDBy4cOIJPap
tdOnLtaxoD90fdVFd9yf3JcDvU4WJJbpRUbgfiHnZ1hp8BJP4BZ5e/YJ7kck
vNzjbgh5wrs1HxccsZPebHXtEfGEVxJ9/33F/Us4WiZoJuEJtS/K0rixd6Xk
e67c4AnjsVvKtexx/lVpl6408gSFDMcDwdsJ5MtUTBz19wSdk41748xxv3D2
tK9YkCd0vs2vWYz9gvPD2iDEE3KLU2KOm+H/U/a2QOxRT8g+YkJGbCUQ/zs4
KZHgCSoOHhbeWwiUv9v5uHGuJwzI8DxXMMbn3TI5NPGVJ0gbHJDR18b7V32C
UjTwAsmX8no16/B++NgmLWHkBaNXs/2ksU1Ti17z0L3Ah//Yppi1+LxMMi0/
mXnBqS0StrayOP577SrZdl5wviJj2bs1BOoxLx0X9faCZnXjh58kCOTt5hM9
n+EFHhu5P1wWIlB00sfM15NecDLm+se6aRoSy+gKckP7QaM//VXyQxoa0xwr
conyhoUEczWbBPy9dD+UO0vfBwrJbokA/P1TNSb4q3qRLxz+JhWQwkNDZ+7U
21lwfIFV+y35cJ0W6lCOsi5PPADlhOtGWx8t5KrmnnPWxg/q9ruXOEtqIf11
JRJVvAcBpR6yc27URBH1/Bpl7QdB687VvGMsTcQ7ElMgl3IIfJvKU1sENNH0
0yX1B138oaNy1iDeTANlNS/8ihQNgDndq+tCD6sj5oygxbGAAJBQyiwtLVND
b36tIf07A6D8q0p/6atNaMrCuOSSTiC8P7XcieLZhO4JSgh8PRcIq18a7JnS
VkW0/ElCZjYQvlo5nii2U0E7Tn5OOevIBvVlAbTRMGVkaZNiq7uPDcXj7V4K
h5URLDMQ7HFiQ5vEFz+3QGWklZESp+jGhs8Vx0dafJSRWKHB0XqKDfN8Ri15
zsro3eMzPsMBbBgXuDpra6SMvHmNzKwS2aCf0tsZuaCEmM393CNJbKgpKPQv
+62EnJNTOWkpbKjPEn3fO6OEbMUHNn9MxXbS1906poQ0Np7TCrnIhqYYky+8
fUpo2uybbH4BG4T362yNbVBCowJpPdbX2ZCXKK5VWa+Evj03zhy9wYZDRwSm
eu8poTe708QNb7GhtuXYgnGVEqpjmQh1VLKha0JDbjpPCVUrDTaH3maDInNN
w4YcJVQ6nBYvU8OG5sHnBvZZSigneHCRTy0bNPa+KylOV0KX9NPRsvtsWFbC
Kuo+q4TO/TGJul3Hhj8LQlG8yUroNBo0dK5nw0LQdyVaghKKPZE+t8Bhww35
lcXucUrof8zU2KM=
       "]]},
     Annotation[#, "Charting`Private`Tag$13633#1"]& ], {}, 
    TagBox[
     {RGBColor[0, 1, 0], AbsoluteThickness[1.6], Opacity[1.], 
      LineBox[CompressedData["
1:eJwV13c8Ve8fAHBKw0wSKpFvRvZ1D1LIJ1KojEJk3XHuJbtr5ZctCdkjI4WM
+BIRGZUnSaEtI6OiKaJkfbV+j7/u6/2655x7nuf5rCvD8DnCWsHFxSXCzcW1
/Fln+2vua9WrPXYzHeNXYhrvxHU491sl3TQIcHI+GxuW1ZoyGHVaKumBwaBO
j7xNWGlrxvuMxzxJ/QZe6uqWO8MaWrPG8+cXEj8ZTLac79wY1tEq7vlPwvfE
BYMHyvm5zaF9rceqSJupxDUgl/yfJzPkY+vC45jmyURxeKnH90ckaL61TvS5
4NmEHfBrRizczXIN8lXWfHZblwqCLmafHLXWI7EDCxmdG3SgwnhFlmGsGPpx
W9y9yH0P1FJLBGWlJVGMi5TEBSVDEPs4byCStg1VJrpEG7kYwxBzU7i60na0
JdjRc/GMCbRNRttKp8mhsvKhx2f9D4IH/em3v1UK6Els3M3TV8zhSO7u09VP
FVF877CA3BNLkNIaVqssVUbP7r8IETY6AnMWx3xHLFTRe4G3lOr+oyC5/t2o
+awaig1UK9xtZQNvm2JXOShT0IJ2hk3wF1uo3RfYatRPQfx9/SZ6IXagqX/J
3sJTA1274Lg4MWMP4oNB5X4fNZBUzeKEeZwDiPx+cDTAnoq2TvTmXeJxgvE7
sVVH6qmIvF1SxsfvBC63Mg/dbaCiyuSAusD1TrDN9sZ7tUYq2q25sdtcygme
yhzhXtNCRbah1kt/djpBcI/dbAWiopR1PXYuHk6QvW5yZVs3FfFoPtu47YUT
SLoJjKiNUtGXkK7kwsvO8Ptj4HZRXgJVdmRWTpc4QxArZVCfj0DewvRO/Upn
OGOTXsrmJ9D3KwsrBhudoY0vKKxekECLXbKBIi+c4adJgZaJCIFWbwp3jOZx
gTeLj7gMtxDon3pCkXXCBQ4PL/HEqRCoKtCcnrGJBrNbFNP8DxGoJ1/FNEaS
BlIxqpk2hwn0XzufRqA0DWRzTYa0zAlkvOEBl50cDTxf/6sxa0GgkWqDgi0a
NMi+EiPodpRAguOUN0UmNJgnfW+oHCeQl8MGp+tBNJCsKbBRdiVQetT3fUX/
o4FYg7jKHHZT+VOV9FAalHp/PHTHjUCrFhN++UfTYP3ESW9zdwLlZ/Bc1Emm
we7ClJ1sLwI9fjw32FpKA+srdqL+fgRShQG7J700uPDbOp4vnEBcWXvK/gzQ
YIOtFvUx9suJ4jm1YRqU8HMLJkcQKOTCybTkMRqIWoU6CkcRqGuK75HlNA1C
G5bceWMIxM7XN+hZSwel2KCY3ngCFSwVyQ3o0oGyTaiiP5NA/pa8/msN6GD2
6qxuZBaBDpT6tOkY0iGiaHqt0gUCTVnpueSY0GHJr9ouOJtA+uW92cdt6HBf
t7FHKI9Ag8fWCox408Eg/HDgxgICbaj3mhktpEPntLlzejmBVBIPbR4upoOE
zFPrLRUE2sdSNuwro8NI/earRdiBG8dTu6rosOizyKr+l0ADAaRGXRMdylfw
G9+tItAlbQffM8/p0LbLtq3jOoGUGk2m5LkZcJKYNT7eRCCjFAUxGR4GrOMf
MHqC7ei2es+WNQzgyOWU7G0mUKJEe+I6QQYsfUnLlG8h0LdTBqqLEgwoFItU
Hb9FoIZd2p6dFAb8HePztkIE2tuy/YsHjQEHX7yvr+4gkLhFxOZjTAbcavap
F3pAoK9jw2aGbAa09SfLeWHn8GX9K+HJgEe9TnY7HuL4tV/rdT+IAYK9zwWz
OwlUuDg5LZXMgHvD3B8cHxGIW7th7vltBtyPaisPfU6g/k4R+duIAWoB4tLd
2FVOPrZX7zGgew+NX+IFgexjdtwM62TA4/Qs0xrs6y9zTyn3MiDvhihjsIdA
dL/wn2cmGeDHpai+sY9Ad2tMuHW2MEGlSzFLfhDvt59qNkOKCZ8drDzcsB9q
iagnyjBhciiqtBz7WfOQ45gCE5IXf1soDRHodbt343lNJtysVgyUHSbQ0kCG
z+hhfD351PjXCIHC8oJXC1gxgSb/OFvzNV6Ps3O+tjUTXIJv2nhir32n0J1w
nAlPT5kIDWKLf22W13ZlgrO0eOS1NwTS5B4diY9gwj1N4Su6owRqvHffvz6a
CbEJl6+7Y+uereB/e5YJPsbTqjnYhvz+u7QSmXCqq813Fttq45rMNzlMOLZ9
SK54DOdD/4QyXz6+fvW68ifYdrnP2jQLmFCX/ilvEZsmnfstrpQJpTVBz83e
4XqjqHpIs44Jl2+XRX3GnplY/865gQm2cplxQu8JFHBtPjiuiQkTdWtWaGKH
EKjsdSsT8hgeJqHY8fpHV8Y9YsLgqToN3g/4S6vg5pEPTJgZPlCx+iOBfLP6
lF58ZsIb6uCcDLbOEJHXMcGEnJrkh3rYXeTU6erv+HyctvOcxJ4MYupH/mYC
X7jcqx7s+luoKoCLBNcTvMwJ7DBuKSn3lSQcvJMYsOITgdYlDPw5wksCl7uW
ljo29dJhJLuRhNKzarLR2D/HKiibJEjg7TVazMJuV1hbKLiFhJS3frYV2DbX
2yLnt5EQcOrt9afYp9p3Gj1UIaFNfN0X0c84/nkz626pk7BVSEpUDpvPfGb7
dSoJ22RaOzWx8/oreXJ1SNjsyRk4gn3ni0yHxz4SJkobzsVhx6qHa9MOkPC/
jz6iWdiW/sOl1mYkOFWqqxZhj/7OitW3JOG4VMjqJuwKw9kFjaMkuNmyHtzD
5sRaucnbklCgIiT2BJtnvYDpOkcS8kyOOY1iP7Y50bTShYR/Wo7afsHOyu1Q
XKSTYC/3cGQG2/nN9txJkoTB8LEfS9gKspF8o64kHL35LHvFOM5/t9f/63Un
IaESPeLFbqzSnej0IsFB822yMLbZzvnuWj8S/Dew2iWxN4Qc1SsLJKFjQE77
H+xhVFOZF0xCi8DjnQrYxauEtqaEkBBpcq5TGdvLzCPxTDg+r00xE+rY2skP
f5+KIoHO9T2fwP7TI+ftFUOCqN9/b7WxH0hEv6afI+HeYPeNXdgpTm/NbRNI
6M3I3KSHbVek32qWRMLtmeh1e7BlPuWqG6SS8GNXe5YB9hflxctEBgm/rkRX
A3atr43wjgsksJyn7fdin66vjZDMxffHa2Yte9/Suu/C+SRc3hNBLlvAwIu+
qoCEsui/7cv390Z3Pf+vCJ/fsTc3l59/aKH6qmopCekluRLLv9/mnhlOLyeh
WOTvoi62zuv/2WZW4vNoMLZffv9rVjTVzmocnxfKdi2vT/a+Mc/vWhyf/zrl
UrHzdJSHKA0kfHpVcFoNW6RSuJZsIkF4oXxEEfuc9Py57FskDD+4jmSX9ytt
yOVRK45Xru+y0tj+q+9qc90j4dS+Ar5Ny+sPLhXU7CBhSn7xpAg2/WvCe9dO
EiyVNBz4sQdoJ1vyHpEQg6I7VmKbv7RNe/qUhHdmO278xPGxu0UGdvaREOFt
Ir4cTzVqa8Q9XpEQG6SZ+HY5foomv14aJmG39dGzfdiicTfzVr8j4fl13pV3
seN/XeTs/kjCw63rY+uxuXyjTL3HcfwSysnl2F9tDy/0TpNwMSRQJQWb7KI+
4f2B80lMvC0Ke1BfokR/Hj9fvnzYH7tD9t2Rkl8ksFF44THsgplT1/x5WWDa
t8pXHFuM7RxzVYAFPml7idXY518ZOQ6vY8H0XsXQWZzPwUiIb58YC36EDpQs
5/eRpGLWhu0sGBhusIzAfsgdr3dAngVjm49aeGAbBPhsOK3IguAiqz4bbBXH
3XfH1FkwFWoRpoi9SumZZK0eC1KsQK8b16OQ/PofHwxYMKQ7Gl2LPSOc17XJ
CL/f5SybHOzXC6xTkaYsmKkSy2ZhN97/2WNpy4JuC4vLi7heutMVEqZ9WPDe
KfbDWuxLKfHuon4scB/ZHjaO6+vz1q+muwJZkP/X8monto7UjbXRISxwi5Kr
PYe9ZgjOisWx4FCEWiE3drH18Uj9IhZIDxhLvMH1fiD6No1RwgL1B/tHG7H5
67ZB7FUWCDfP7EnD5qz/9OfZNRZcVxRuMsLe+8QvhGxhQaHp7apC3F9eH0gM
SnjJAoGVyfdM3+L4DPpmW9PPgnk9hSlJbOPSo9q9g3j/IwNqpnE/q+TZPCc1
yoKantlf6din75Zyar+yoOdza3M/7n8Susjr1Wo2xIvQfhzE/dNK7QdTYRcb
5CdPFH9+hfvBmyeSYnpseN99fmUdtmFqRS+PARsIeTHBUGzNWfqBsX1sYAbP
SAtjizU/U8q3ZEMX7YsJdQDXI+Nr30Xc2GD5MeghG/d/N6cT4X+y2JB0sTEi
Fc8Lo0LGOl9z2EDtTvW3wj6Otn0fusgGaVUv8fXYB7cPMJqK2CDG2+KejOcP
tfH9+/2vsWHD1uKD554RaNZfVvDLfTb8TRES83hCoPDzb3J7Z9kQAoIdc3i+
KfU0al65yIamMrFLJdiPDpW90vjJBvsVmyVtsCUEfSSSuF3hZUUrXx2ej2oT
/2TuF3KFkS0ON93x/PQ+aWvqTQVXsG039O9sx/U31SE257grzFhqVRm34nzL
6vdzQq6gEjnlaVhHoIjFOk+be64Qvj+x710tgSaOp7AOd7iCn/Xc0hnsNmnT
Y/qPXOGuVIn/8rzoW968e+uAK6h3b1HfX0Og7lv53CPTrlD1aeWIDp4vo94x
kx2l3aBV0vPvRCnuD5RvFQ5hbnCufMEiJYdAUi1B3Bd1TgCxcl6qGA8Ddd/4
lupXuAMzXdU33Z5AyTfvWO5vdQcLS/vXL7UI9EIxzLQmwQME9frO7RTA86iq
c0GKmSc4k4Mza95Rkc62KrG6VV4gwPTzfYD/X52+s0a9+pkXWP3McFWMo6JV
U1ElMknekPr61mZzByqaf8h7x8vBB/xZMqk2O6joYuffpVARX4jnF/1Hf04D
0Rf49kf4+oKs+nelnnYN9GppC8OnzxfGDKc0a5M10Nx+/aocrZPwp9z2T6mT
BmrmE1v7Ie0k5MzvQ4dVNBC1eJbYungSuOeEO1LmKcj87LukFFsOrPGbX3Ws
nYIOmCUd0rbjAONKWmPgPQoCoV18w/YcEFcK8MhqoyCNrKQYBScO0JhKL3oR
BYmW7gq5w+TAx/vbiq1vU9DQ/eQTk74ccPSOpx1poCC3VXr7TBI4IJE35Wl+
lYLonR+5p85zYKxAWdu7jIKOJ6a2pidxQGw4hSuplIIObfy0+00qBwj16ezH
xRSkLpemEZjNgV3STQOHCiloft9nqeISDty5TuYezKWg6bXpw6ZlHEgMMA/2
yKGgz4/0c6evckC+rts+IZuCXlmnb9St5IDzZK50dxYF3SL3CLyo5UA4Mmo1
S6eg+h3jnUE3ONDcG/GvexoFXZtMj93awIG/ZTE58akUVOA/vuJEEwfe07hO
dyVTUI5OBhJq4YC6arT3lyQKSvu1J+zGLQ4MR35i8mHHo3Hd43c40P+QcFBK
pKDoMxn//W3lQIibt7XZeQr6P5CNSxw=
       "]]},
     Annotation[#, "Charting`Private`Tag$13633#3"]& ], 
    TagBox[
     {RGBColor[0.5, 0, 0.5], AbsoluteThickness[1.6], Opacity[1.], 
      LineBox[CompressedData["
1:eJwV13k4VG0bAHBeRJYUkVZbaIjMHNkKd5ElSwplG2bOGSKEIUuWFlt2IUUU
KW0oUbTg+UpEKSpLZUslsqYsafue/prrd80159zPnHs78qT/Ho//eHh4JHl5
eP59Vu79NTNe9sbQcbpxpDiupi6x0a1rd1q1USjTLT4hOqc+4+3xiHVpTUZv
dV8pO0SX1Gd/zG7lT+sy8t+0yVYn+k59zkjB7FzqZ6OR+ynNUtGN9St8FZK/
ps4ZVaoW5N2L6qzfV8ZxmEgVhFaLH75U5FD9XGvcvbHUFZA3Pf9bInS2vnJ5
u1h88gaYCqDCvWwFUYCaVlvtFgZovE2957p5GZI2m8tultSFY2NWnG0J0uhb
7YoDFw4YwtSBu7LrZNegOPd1MqdVt4NQ9y5HoUw5VJrqHmPsvgPmff1FJFQV
0epwV9/5WHMInnq+q/OkErp89V1rfLAlsAXnwveXqaDnCYnVEcU2EFEq1xbx
nIaSOnpElZ7bAmHf2Bh3UQ21PX4ZudR4DxAdR06YWqmjj6IDmje67GBn7Y8m
9oQGSgjRKNLf7QCvN63Veq2siea0sx3Cv+yFDZeZg1SbJhLp7DLfGukIPCdW
7ttD0lH5adf50WknyKofNK/spqOlQmqxO344QcSbpWsy3tIRN+yH+Pm/TvCo
ffE9nx462uyUo7JH1BkYIob7ZAfo6MGqtr01Ss5gsm1gTdhnOmopML4d6+gM
nZHdi6Zm6GioWJW7ts4Z4oPshheWMdC6m/OjNokukHC+szrRlIGElWpUt6a7
QHR8gB2POQPN5oZ60065gLVF6MQhCwZ6HjM7xFfkAsfFMhXdrBgoet/39zU1
LhB/zy9dYQ8D9f2Z7FIYdgGVGJ/cCCYDnbP+/GjW1BWuMOU6/YMYaO1ox9lz
/EzQNU4S981nIE7tpcvCIkx4XRm0pq6AgUrTD1WGLGOC06JlIuLnGUhfS+qp
zTommDb6p5UVMdDeKPuFPzpMUP+5oNVbwkAZ4q8c3X2Y4PvUdotgBQPxa7VJ
yb1kwng4/9+EBgayXFQon9LNBJsItUd3HjNQZre/+nwfE1LSnQM/NjKQfJT4
jrZRJqgc7k3Z2sxAho02wUcF3KAp5UVTfysDhTq2vhzQdYNnEsYnpjsZ6Etk
S3rReTcwiUwWsRzG8TaeKp285AZBcX8r9oww0MGl7GaDUjcYOlNs7/SFgb4W
z/33tsYNqhMj06kxBppvWR8i8dINGpeEDvpMMdCilUdcY/jdofzF481W8wyk
cJugeXi7g76JvL21IIE+/vmzo9LfHU4ZKP/WEiJQiXkLyRviDpruntdWLyYQ
rYeVX3DcHXxk8iSGhAmkyZcm3nnWHQov9Mr5LyGQ4e7hGdPn+HqGln57pAhU
FmLDzl7JAqeO84nuCgR6VbDRIm4NC7wKaptWKRLoR4MwPUSWBdXcenoH9g7J
Jh5HJRZQM5BkpkSg3htGhavpLNgmM7dHYQOBxEY0+y+Ys8B9lWjgTXUC+blI
MitCWVD+KstGU5dAWce/mlw4zIKmupqD7dh3r77YmBXFgutt1v8L1COQwHzy
r+AYHM+53D839AlUkM2fr5vOguRf/v0KBgRqbZ15W1/CAvLTy/2D2wikDt2O
zztY8EDyA0/LTgLx5Bhe/tPNgtYq9S1MSwK9Hr04o9HDguiO2ORJ7MjTgZnp
gyzI7GT7L7MmUMuE8DPbSRYIP5G23LmLQJ4FBkavhNgg9N4tJcOOQPrfilP5
RNnwbTLaVMoen89CuIcQZ0NwxfNVudhV3zvDsqXYcCdGQPKcA4H4rAJuOSiw
4f6wkEXBPgIVLlxQ6t7ChhUmqwUCXQgUbLs4WMgIXw8Uj33GNivxf6i7nQ2h
l8JXM10JNLF7q3uuORtcimVKdzAJZHC144yzAxt26O8yEXUn0Nt9QqK9B9mw
cqNIkj9JIMnbftPvi9jgkf9dK8OLQBtTrVb1XGSDqPLSnx+xTTzUtndeZsMD
+SQ+PW8ChUiNnGwpY0OvpF9PH3b3IQ698i4bmiyqK+V9CHRO2yUgtp0Nyz3S
lWP9CFS9RP9M9Gs2mD6zV2vFbhuSQWFdbLD42HBI6iCBeE93ivv14vNHhfYU
Y3Pmdt9wGGGDX9yn2Wp/AqnWmE8o85LwRftZam0ggYwzVKTl+Uno8O8S+Int
6rXIcLUgCc701406XAKlyjSkiouRQDcIWn8DeyrMSH1ehgTdu7/sTgUR6I6e
tm+zJglVb15VGB0i0ItlUtmPCBIUyf3tgdjDI9/u12rj+0WpGxRjr8yrELm1
lYSvvXILfCH4+S9svJ5nTkLIsI14Lfa2+4pffFgkvGkSei0WRqAVu46u2kfh
+FwbRLWwxwd7dm73JGHQtuWsE3aucM51GV8SNu0Mrb2A/dVJyO9xKAllb4qW
q4cTqGmcU3DzMAmhI7/4bbALjv2v9WwUCWIXlKwPYltcPazBjSFhyKDoUyl2
0fzY5Lp0ElqlT2xVOEyg0BQLOeFMHF/a6SkDbGu5EtuZbBIy/WZ/O2L/MHOv
eJpHgnQLqZSKvft0OzeshIThAJ3ScWwVNY1i6ioJ+Q18mvwRBPpdl/TKppQE
pWvnl6zCvjpkrKV0i4TPjwV6jbF5te/MtNeSkC3Z9Cgdu6tZQrkWkWA8a6lY
hF3G9N975REJQvPr+iuwneI2VEc3k7BI8aBvO/amlXGfvZ+R0FBoYTiALVD2
foXDCxJKhuh+E9gVr/PC1DpI6FX9PCgUSaAEr7kr0t0kHDOXVJXCZv6ye8P7
joQBX+EXcthExs3F470kfJT+1a6GvXi9mH73AAkVdSsIbez+au8Djz6QUN2R
Mm2EfduyMa98iITcxqSlFtjsoCM/Y8dIuFrX5+WErSPYoxYwiZ9XeFYxC1vs
rK6ryzQJesFpBvuxP2icSjGdIcFn/o+2H/bdh18f0OdJCDNbnsHFTt9rM77m
Jwlm+b/NQ7E9vlxbK/QH54fqF3YE9pZoQZtvPBToyy1+F429TIIT3cdHwcUL
iVXHsD9fQuXNiyjY3Z43EYNdq7e2v2oxBakNPolx2Fmt4eKFohRUparFxWN7
szuNksUpkNVZPPjPRjOMgBAJCvQaiMJ/lkpML2RLUbhe3tb/+/3omrE2KxkK
hoLUtsVi/++mOa/uago2Ht67/ji2SZD6GXIdBTWCP5WPYD/ZLLEpVZ4CM91p
/3/xW83PPq5eT4Hqu9C/Idht9965DqpQMHC7qSMQ2z4KfRNVo2B57NpvPthd
RpeSdDRw/HNV+zywnf9LkifpFBA1zXxu2H0NB2tStCgQ5Zyec8AmE+x2VetQ
oJHuRFhjf7LQHXqvT0HdI8tqY2wv0bVRooYUTBy7GqOHPfacd7nONgrGjMrP
aGAHnBy6xjahYMr71KwC9je7p9tSzChQJvMKpLEXurP931tTUCw52vQT51v0
2fBForsp+OtWZjn+L7/d3Aq07Sm4nH94ZR+20AeVp8nOFLwuVsiuxU65JEre
YVIQXh60rRR7qdfX+QEWBUXqD/TysFeM31PW3k/BjbOyosHYeTfO17IO4Psf
vjnkjr2OG2uf7EeBbul6MUts5Tnr4wNBFISGXzCUxdbifd+bdJSC6Ai2fj2u
z5pHj4Nvx1BQyBtx+BL2lvhrIgPxFMRetxZKxt4uEqy3OZWCk6lCS+z/1beU
4Kn+XAqeaes96cX94nXXqJpwAQVPXxyNrMN2zGt7qFVIQeBD+6PnsFmyeVOJ
JRTMJySFumIfpKlbaVVSsEk4UbUN96vp0WUf3O5QEKSZzr6Ofah8NjzxLs5P
4+mROGz8l17uq6dArvzOpC52koEdX+IzCtLvJ3XkhOIvd4ff6/1Ewdu41q0M
3D8DcjpVXw7jfJj53iWArfuOONs4SsHNTqW+btx/WzgTETe+UrDlPXNjFPZY
KGVw7DcF96f1O+qCCcQ4Z43WS3Fwv9t4TBn395+D1zRXynBgintxcAr3/wYV
oSKx1RyQfLn41j1sh4qHx2blOGDca3/WCjusQcf4yUYO6Dh+zffG86Tui3yj
jwkH0nJ3x57A8ydh0xFtlhkHTh9f/dYC2za4p8R+JwfEjpcXCmO//52TYGDL
geajn44m4fnFv0zUQtyVAw0NqZkxeN7t1Jl9eiuIA+MkU8EFz8eOmJb2Hxc4
kJQyqFHkietn7sYV9RIOhGqe2bwT++GBU0fYVzmg6XMzb9qDQOW7WerNNzgw
E/zl6DbsE7KzJ8484EDfQPmjLgrvF/flQaeTAzmORXZDLLwvTIeVBy/2gEbT
McVUZwJJe7rFXRH1gLqXBykF7JQ3xq494h5AU7QUqnYiUDhaImwi7QFna8eO
9zkSaE/aRQ9JRQ/Q6X65TRnvHwKqbWtubfWARx0/pHLxPnOArZI86e8BUTMF
WWJWeN5nJB1YHuQBwhsjtDLxftReP26hF+IBKn5tptLYuuuqhGIiPYDLV4bW
4P1K8B3ESyd6AF9hxRJFcwJdtHc+ZnDBA2Tp74ykTHD9m6WGJr/2gA2jPXYn
t+D81fhGqeh5Qh/bT+Ab3g9b+p+vkd7qCaXzk8os7O0nr3XwG3nC2zOru56p
4Hr5zjYbNPEEf0uhjxeV8fnvtakW2HqCR59f1a71BOrZUf5VwssTTh77a5sh
i/sH0/vInxxPqGhcHluH99kjKf15Hd89YYRvv0gXD4GW53QFMdF+kJNwH+d5
zkBTmlPXXKK9oLA8wXb7Gfy+cz+UN1/XG/ZFWeZruTFQ5ZTwwu3/DoBXQvJQ
/UoGSq+uszWtPwAbsi7u39JBRy9p0RY3k31geRrNkoqnI1d1t8KMnb6APlCz
Q7p0pCtXJl0p4Ad/PrR1l49ooog6wU032vxgdFe/dXSGJhKYOH5JPu0gMAa0
p2P1NdHsk8V1fi7+UMor+9f39iaU3/x3IUoiAOiprSdOf9dA7Dlh06MBASCj
tsyVz0ADvVlYTfp3BoBJNuOhP1cdzZgalOVuDoSsV491/W9tRPeEpYU+ZQaC
8nD2tYFvaohx8Tuxdj4QzGgr9g8pqCGb+A9pGXu58DhkiYCsmyoy25lmpe3I
hbCF7V9KnVURLNET7nHiwokXSyr196kiek5anAqTCzp8LZMOtqpoeYleZB3F
hX2pLjLJ21XRu8fp3mMBXHh/h9CfUlZFXgJbTcyTuXDXU4RdMklD7OYh3okU
Ljg/afmkOUZDzqkn67PSuHBW+pft/WEaspL6rN9/kgudzmLvXrynoU1KmfSQ
M1z4UrYXzb2ioVmT4XUXL3Ghob9pcHsNDU0KZfVYXOaC3anf3U+raGj4mUHe
5BUuWOTzV9tX0NAb+yypLaVcCNfvVfW8RkMPOIaiL29xQWCR1PeEfBq6vWGk
ObSKCyOv6GpLc2mofCwrYe0dLnC2P9t55hQNFQaP/Od9lwt7jrwwvpJGQ7m6
2WjJfS6kzZJrNZNpKPOXYXTVAy5IsJr7qxPw+z8a2eJcxwWFhRXJRrE0FBOb
/eNvPRdUFyjZpqM09H/hhBcx
       "]]},
     Annotation[#, "Charting`Private`Tag$13633#4"]& ], 
    TagBox[
     {GrayLevel[1], AbsoluteThickness[1.6], Opacity[1.], 
      LineBox[CompressedData["
1:eJwV13k4VF0YAPCkIpHsiogIkZhrL7yyF0rWrDP3zthKNPYWla3sRCpFWpCy
FFlScdp8KJKyFYmKLFHJ1sJ3+mue3zP3ueecOe82MmTAXtbSJUuWiHEsWfLv
s8Lxz/TXkh4D5x8NI9dia+riGzy6bFOqDUPdPeJORWbVp72NOiKV8p/hW53X
mxwiC+ozP2W2LEvpMgzYunWPdmRVfdZIzsxs8rDhyP2kJpHIhnqxA7KJ35Nn
Dcs352TXHuusdyphOkwkc0Gr5fwB6uhQ/WxLbO14shhc/DH3VzBspr5C+BVf
XKIilAZQET57uFCgskbbw200sLqZXOumKYBEzWczm4R0IFjMkml0ShRNPRTz
u+pnALof46WlpCVRrKeU+LnNO2BHxR0n7jMbUHGyZ7SxpylconFyC27eiCQi
3A7MxVjAeHWyUWe6PCosetcSF7wLTp8otPIuUUCtp+Krj1yzAUOlbPMjrUoo
oaOXV751D7CznNgx15VR27P2o2uM98LuIzMpxlZb0CfeD2plXXYQJrnGwHVC
FZ0KVb2iZ+sA3J35XS2b1NCsVqZDxKgj2OprXXZqU0OrOrssth91hleFiju3
k+qo9Jzb3NiPfWBk1t2T0q2O1nArx5jO7wMB41T6/rfqiB0+z395cR/UhSXe
MetVR5r7shT28rrAFjqtYr5fHT1Y1+ZYI+8CB1sct9kOq6PmHOPKGGcXGH0h
l9YwrY6Grm1mr69zgbH3Hj3PBWhI6vbcmE28Kxiwuc9am9EQj3zN5u2prjBi
H/30iTkNzVwI81U66wqNrc0/dCxpqDV6Zojziivc8Iy22mBFQ5FOPwdqalzB
bvvc/KAtDb1fmOyS/eIKEZwL3jruNJRrPfxkxswN/vbNj8oF0dD6sY6Lucvc
4UGiznH+SzTEfJhfyLPKHTr8lT7Tc2ioODWkIlTAHb55divfyaUhPQ2R5zZS
7mBXHuxmc4WGHI/Z/1rQdoeWigbbIwU0lMb/2tlzvzvc9R55dvk2DS3TaBPZ
0O4OaWvP5Qo/paFdK/JkkrrdIcv2Z/aOZzR0pjtgy9x7dxB9AycCGmhI5hi/
aduYOyxWl61oaKQhgwab4BPLPeCSqRSPVwsNhTm3tH/Q8YCPYRLy7E4aGj3a
nHrlsgdE5CYfeTCM99twtngy3wO2i2roPvlCQwfXMJr0iz3g2Yuu740jNPT9
2uzStzUe8GqlkMOrMRqaa5YLFWz3gPW/9Uc7JmloxdrjbtHLPMF4+Hxc6SwN
yVYSSixfT3j25qjR5RUE+rSwYFoR4An17aI9sVwEKrBoJjlCPWErIyNoPzeB
lHrpl3KiPCHBRr2c4CGQGmcKf+dFT7gfMe5Ww0cgA9sv02atntA49fjyGWEC
lYTaMDLX0kFTaF1WkgyBXueoWMZK0kGg9dlNM1kCzT/lUQ+VpkPB4orRRWxT
of+WOMvTYY2N2EiAHIH6ygzzJNTpwJJePWmqQCC+EbX+qxZ04JsyNW9WIZC/
q5D7nTA6xJaqpmlqEygj6rvJ1cN0kPmP07UD+17RS5WMY3SQC+p2DNYh0PK5
xD/B0XTwp6wHy3QJlJO57JJOKh0eWyxar99OoJaW6bf1BXR47m+Z/woItAW6
nVs76DAWpHbviiWBlmQZFC5000FtWNya2EmgN2PXp1V76aA9RJt+gn303KEz
qYN0EONZjBrcRaDmCZ4Xeybp4JjMf0nYhkBeOfqGr7kZ8EUL/bHaSyC9qWvJ
nLwMcC6W+fESm8+Sp5fgZ4B3FVq0tSPQ3Z+d4ZkiDFgYuse0sycQp1VguYMs
A7J1brjtciRQ3q+r8t3bGFBV2799jQuBgvesDOY2ZIATh9ObGGzzgoDHOjsY
4L5E6PQc9oTtds8LFgyoI1xM+1wJpF/Ucd7FgQEhccpSl9wJ9NaJm7fvIAOK
wmZPTNIJJFTp/2PgCt5v2mDzhBeBVJKt1vVeZ4DLB55kI28CmbCUd3QWMqD2
S15qBnaoyEh6cwkDbrZ+ctT0IVB3CFO94h4DogIPTQX4EihXyzUw5hUDSmNr
0h/tJ1D1ar3zkW8YwLVnhM19gEBtQ+IovIsB03zonA02x7lOfv8+BqSWq5R0
YzNnbcscRhhwLjqX95M/gTbXWExs4iBBK+V2c1cAgYzTFERllpHAfmu8IBhI
IDefFQYSXCTMVpaFW2Mniz9N5ucjoWmqdwfC/hZuuGVOnIQ5eWlaziECrbSV
cvghQcL3O9xX27Fllf4eHZciQXyA4cLFJpBdT+2LD3IkBBqo5h/ErtLVOtCk
RoLM1vs3NIII9FJAJPMJQcJ53VIGE/vLyNT9h1p4vYACZgb22uw7q8q3kzB4
K9ByEvvoL5Vb2Rb4eeGpjNxgAhnd3zi6n06C7fI253chBBLbfWKdE4W//2Qs
vIj9dbB35w4vEjSvdG6UDSXQBZ6sW+IHSKhuEAEv7O/7uP2fhZHAMy3HHsL+
7ysz5/ZhEgIka18vC8PxfvJRy8VjJHwqHE6QxbYsOqzKjiZhl3bjL1fsK3Pj
k1KpJNiPPfncgB2WZLmB5wwJUYJG8/3Y1hsK9kxnkiCZ3krNYc+be955nk3C
NeFOA4VwfP539weqckgIaSop08fODxAXvJqH70PTNtwO2/bcK3Z4AV5vV5XA
MWwFZdVrVBEJvIc6BtOw/9YlvLYpJqHc9AjvdeyiIWMN+XISPG+J+DVic2hV
Tb96SMKVp7l2KyMI1NUkuOkhIuH1GO+EGHaJe4DjjSd4/yGhg/LY+2IVqyOb
SEhKmO4xxN66NnbY9wUJG6e8+3ZhLy8ZEHN4SeL+lrrNCfvOm+xw5Q4SCk2q
uQ9gn/KZvSHaTUInIRwegu3+x66H4x0J7Un9OyKxibTbK7/2kbD6jLlvHPZK
OT697g8kqB0/PJaM3V/t6/fkIwnc8QVNmdiVuxqyS4dISO6b57yIndgv+/zC
CAlvr13NzsNmBB3/HTNOgsKf1uR8bG2uXuXASRJeLhb3FWHzXdRxc/1Bgv4j
v4QS7I+qZ5PMpkn4uUsr8zb2vcffH6jP4fdf1/9djp3qaPNV8jcJRY2l9Xex
WaM313Mv4HworR6oxN4WyWUztYQCFfM4RhW2gCAz8j0nBYsRFob/PJyPSptW
UKCqpHLk3/MPddf3311JgddWT5F/78toieDP46XAlc6/+t96voxOw0R+Cm6f
9mOVYRtO0wJDBSlY8M+VKMYWiU/NY4hQ8F9rt9oN7DHJ8TYrcQpiSfP8a9iP
bltw6EhQkNQjFpGLbRK05TwpRUFd1XqF89iNmoJbk2Uo4IhKFE/HtpqbeVYt
R8GB4IvW8dhtte/cBhUo0Ht4quEEtv0xNMWrTEHxyYTosH/xYpifoK1KgWxf
X4w/9vunB2uSNCioyvRw+Hf/5Cm73dXa2NOLcv/i47OlztCAHgUBsz26Btjj
rRzC2kYUXAuX1pDFDkwfuskwoeBF8cJaIewpu+dGSeb4vKN/TTmxf3VnBgxY
U/DxuPGhARy/kRcjVvDaUhCp9zfw5b949vDI0bKnYLjhYfUDbO6PCs8TXSjY
VqIrcRY7KZ+XrHKnoGatj84J7DU+3+c+0CmQPhad44ct9rV2k5Y3BS59XvAv
37LLLj+k+1EwmH0lUh5bih1jn+hPQUVb6XI+7E2z1lEfgihgVspP9uD81eAY
6Es4QUFveoPmfuyaJ8+CK6MpOH66E1ljb4u7uepDHAX3eKKytmLvWBWsq5lM
gWBoqux3XF9sRbjO9l+g4O/v+0/2Y7/pGlPmyaHg7q0PRRbYztltjzXy8O/h
4d0rh02Xzv4WX0DBIZNjCv/q20GlLVYaFRR8Gp53NcT+MSbw0aOKgs9v3W+J
YoeUzkTE36PAv2DY4iuuj0cJVPi+noLEYeuA89gJ+nac8S8o6MhNCBjC9bTQ
NqK27zMF6QKtBxm4PgdmdW5u/0JBcuhJDXVsnXfExYYxCnYcdCWXYDczJ46U
fcfx8F579hKu9+NhlP7JvxTM+kXxvMT9gZZrjeREmJDPQAuiuL/8Hryptlac
CV6mv137DhLoqQL3FT4JJiyTUJG7hu1w5/HJmQ1M+LZbdkYFO/yptnGjChMm
ZozydXG/qhuVadhvwoRJ221O2rj/ndp6XItuzoT+ZZXhP/0ItCe4t8B+JxOo
ojGuO9gDf7NO6e9hgrQnBCpiLxPgteR3Y8LXxn3+a3A/3ak987w8iAk/5h8b
PsP9uSO6+dX8VSb4M+lhTxg4P2bLbmwpYILENu5ob+zHfmePM4qYUMdhM8KD
XWpL39JUxoSC8pSG3bjfn5aeOX3+AT6v9UDTKw88n9yXAe1OJnTujd9YjeeF
vB/hpcErWRDO6ZrL7UAgUS+P2Bu8LPjLv877PJ5PknqM3Xr5WVB7Wy9dATsC
reYxEWUBezaExwTPM3tTrrOENrLAd6wgK8QW19/NbZLl21ng/c3N5L41gfwY
ComTASwQiBljtZvieSEtwU84iAVcf/uUbLFf1X+11A1lwWEzE9eXJvg+pe5y
Rx9lgZetGlezMYG43kGcaDwLin72n64xItB1e5eT+ldZUG1r6nFYH+e7eXJY
4hsWzEuuvn5GA8ev6hSloOsFCnIyfBvwfNrc3yoput0L5FVdHsRtwPGefrNj
maEXFOr6z4xL43z5yTAfNPGCZeuqV9VI4fPXtm3O2eMFqke+1VlIEqjXtPS7
oI8XVAql+9iLEcjH3ff4QpYXPN159LkIno+PJ/Vnd/z0gl9JEs8t8PwtnNUV
5I68QWcse5XFYxr6pvbtpmukD6jxhjTrJuD/S/fDOC7p+MJyiS+LudY0VPGN
51flUj94pNcwyb+ChlKr6/aY1ftBLHuhfm+dOmpXirS8nbgf2hmhCbn71ZHb
Fo+8tJ0H4GCU44TKOnWks6FEtGK5Pxz41df8oEENHanj2lrW5g/LdbpCsnzU
0PKJqHyZlIOwUrhyJJdPDc00rqzzdw2AgaKgwaV7tqJLTYu/jgkGwudJr0Oz
UaqIMctjdiIwEEgxjm/m9VtQzy8JMqAzEAwTTge0DKmgaTP9kguah+Cc6CnD
dWtVUC2PKPfnM4fg64bBH0FWyoh2/Sexfu4QZAwvsIL3b0Y2cR9T0hzZEC66
dJTvnBIy35lipeXMhrrdj7LtM5QQrNbl6d3HhuiIINmLqUpIPSslVsGdDVKJ
QtUKp5WQcIHu0TqKDWWS07MGEUro3bNU3/FANjhXV3xluSohn+XbTSwS2fCU
8X1vlrQSYjQNcUwkseFwjLVAt4QScklOr89IYUNH9dWiteJKyEpkWK8/nQ2r
6rJ8Lq1RQlvlz6iHnmeDkJuObB6HEpox+SJ1PR+v97jvfN5HRTTJndFrWcgG
+YImjg/9iujLC/3syRtsSHaRM5PuVUQ99hki24rZYB8axch5o4geMA1428vZ
4LSP9fncM0VUqTjSFHaXDXofdql0PlJEpeMZp9ZXsYG3x3m3cJ0iygseWep7
jw0sG6PNaVWK6IJOJlp9nw2JVjsHW8oV0Zk/BpF3H7BhtP5N6KoyRZSARra5
1LFB0H522OKWIoqOyZxfrGeDRHGjZlyhIvofWUNFqg==
       "]]},
     Annotation[#, "Charting`Private`Tag$13633#5"]& ]}, {}, {}},
  AspectRatio->NCache[GoldenRatio^(-1), 0.6180339887498948],
  Axes->{True, True},
  AxesLabel->{None, None},
  AxesOrigin->{0, 0},
  BaseStyle->{FontFamily -> "Arial"},
  DisplayFunction->Identity,
  Frame->{{False, False}, {False, False}},
  FrameLabel->{{None, None}, {None, None}},
  FrameTicks->{{Automatic, Automatic}, {Automatic, Automatic}},
  GridLines->{None, None},
  GridLinesStyle->Directive[
    GrayLevel[0.5, 0.4]],
  ImagePadding->All,
  ImageSize->{920., Automatic},
  Method->{
   "DefaultBoundaryStyle" -> Automatic, "DefaultMeshStyle" -> 
    AbsolutePointSize[6], "ScalingFunctions" -> None, 
    "CoordinatesToolOptions" -> {"DisplayFunction" -> ({
        (Part[{{Identity, Identity}, {Identity, Identity}}, 1, 2][#]& )[
         Part[#, 1]], 
        (Part[{{Identity, Identity}, {Identity, Identity}}, 2, 2][#]& )[
         Part[#, 2]]}& ), "CopiedValueFunction" -> ({
        (Part[{{Identity, Identity}, {Identity, Identity}}, 1, 2][#]& )[
         Part[#, 1]], 
        (Part[{{Identity, Identity}, {Identity, Identity}}, 2, 2][#]& )[
         Part[#, 2]]}& )}},
  PlotRange->{{0, 300}, {-19.911157024219154`, 0.}},
  PlotRangeClipping->True,
  PlotRangePadding->{{
     Scaled[0.02], 
     Scaled[0.02]}, {
     Scaled[0.05], 
     Scaled[0.05]}},
  Ticks->{Automatic, Automatic}]], "Output",
 CellChangeTimes->{
  3.725790454653599*^9, 3.725790514460441*^9, 3.725790551700067*^9, 
   3.725790631266589*^9, 3.7403738145650263`*^9, 3.741166057760421*^9, 
   3.7411663256639023`*^9, 3.741166397999399*^9, {3.741167681216887*^9, 
   3.74116773414235*^9}, {3.741168364703821*^9, 3.741168388275528*^9}, 
   3.741168493622514*^9, {3.741317845408305*^9, 3.7413178500129128`*^9}, 
   3.741318068963941*^9, 3.74131849956246*^9, 3.741318547293433*^9, 
   3.741321511158698*^9, 3.741336331894384*^9, 3.741407724194812*^9, 
   3.7414077751594687`*^9},
 ExpressionUUID -> "93f1d5fc-e967-455e-9b12-4cf754484e9b"]
}, Open  ]]
}, Closed]],

Cell[CellGroupData[{

Cell["Short-range Coulomb-Breit exchange energy per particle", "Subsubsection",
 CellChangeTimes->{{3.7411679892957087`*^9, 3.741167998517291*^9}, {
  3.741336322890379*^9, 3.741336323837853*^9}},
 ExpressionUUID -> "e9e85745-2c33-4e4f-b9e9-22820e71bac6"],

Cell[BoxData[
 RowBox[{
  RowBox[{"ExRCBsrPad\[EAcute]2", "=", 
   RowBox[{"ExRCBsrPad\[EAcute]", "[", "2", "]"}]}], ";"}]], "Input",
 CellChangeTimes->{{3.722676673170491*^9, 3.7226766840788517`*^9}, {
   3.7226769607964897`*^9, 3.722676964008954*^9}, {3.722677058507019*^9, 
   3.72267715175624*^9}, 3.722750488409705*^9, 3.722750909349684*^9, 
   3.722751650069563*^9, {3.722751697031013*^9, 3.722751701925248*^9}, 
   3.722751733156549*^9, {3.722751776660254*^9, 3.722751780232744*^9}, {
   3.722752400242813*^9, 3.722752400432448*^9}, {3.722752467679291*^9, 
   3.72275252014501*^9}, {3.722752952275763*^9, 3.722752969101005*^9}, {
   3.72275303435499*^9, 3.7227530345334883`*^9}, {3.722754156545463*^9, 
   3.722754156795789*^9}, {3.722754188112558*^9, 3.722754208304021*^9}, 
   3.72275432057234*^9, {3.722754402080971*^9, 3.722754454383902*^9}, 
   3.7227544955051527`*^9, {3.722755499949471*^9, 3.722755529084709*^9}, {
   3.722755602590743*^9, 3.72275561222154*^9}, {3.722755806077857*^9, 
   3.722755808828918*^9}, {3.7227562912298307`*^9, 3.7227563187455587`*^9}, {
   3.722756509642661*^9, 3.722756533689232*^9}, {3.722756667772307*^9, 
   3.722756667930399*^9}, 3.722763826327332*^9, {3.7227640337205467`*^9, 
   3.722764094101956*^9}, {3.722764391670136*^9, 3.7227644061291647`*^9}, {
   3.722765493776552*^9, 3.722765494139145*^9}, 3.7227690116290216`*^9, {
   3.724470727309154*^9, 3.724470739564727*^9}, {3.724470771805664*^9, 
   3.724470785724593*^9}, {3.726898654440785*^9, 3.726898654805393*^9}, {
   3.740374409484497*^9, 3.7403744097069387`*^9}, 3.7403846191115026`*^9, {
   3.741164665136079*^9, 3.741164665361087*^9}, {3.741165865704812*^9, 
   3.74116586682211*^9}, {3.741166428171543*^9, 3.741166438232815*^9}, {
   3.741166673009337*^9, 3.741166673879197*^9}, {3.741167748737232*^9, 
   3.7411677511349583`*^9}, {3.741168021316937*^9, 3.741168022632657*^9}, {
   3.7411681425034733`*^9, 3.741168145529846*^9}, {3.741321534823586*^9, 
   3.741321542997918*^9}},
 ExpressionUUID -> "7e506951-1380-494a-8baa-cf1ec31e4571"],

Cell[BoxData[
 RowBox[{
  RowBox[{"ExRCBsrPad\[EAcute]4", "=", 
   RowBox[{"ExRCBsrPad\[EAcute]", "[", "4", "]"}]}], ";"}]], "Input",
 CellChangeTimes->{{3.74116594537556*^9, 3.7411659505081453`*^9}, {
  3.7411664420165*^9, 3.741166448399979*^9}, {3.741166669555909*^9, 
  3.7411666717409487`*^9}, {3.741167753072113*^9, 3.741167754480927*^9}, {
  3.741168023539118*^9, 3.741168024730907*^9}, {3.741321535958165*^9, 
  3.741321550389876*^9}},
 ExpressionUUID -> "4af9915c-b420-414e-acf0-58e094618525"],

Cell[BoxData[
 RowBox[{
  RowBox[{"ExRCBsrPad\[EAcute]6", "=", 
   RowBox[{"ExRCBsrPad\[EAcute]", "[", "6", "]"}]}], ";"}]], "Input",
 CellChangeTimes->{{3.741165952141227*^9, 3.741165955289587*^9}, {
  3.7411664557837667`*^9, 3.741166458935994*^9}, {3.7411666649928627`*^9, 
  3.741166668197682*^9}, {3.741167756085778*^9, 3.741167757366679*^9}, {
  3.741168025756399*^9, 3.741168026922258*^9}, {3.741321536699048*^9, 
  3.7413215485815907`*^9}},
 ExpressionUUID -> "cbc8c773-ec6f-4b64-bd98-b3bede9069d2"],

Cell[CellGroupData[{

Cell[BoxData[
 RowBox[{"Plot", "[", 
  RowBox[{
   RowBox[{"{", 
    RowBox[{
     RowBox[{
      RowBox[{"ExRCBsr", "[", 
       RowBox[{"\[Mu]", ",", "c"}], "]"}], "/.", 
      RowBox[{"{", 
       RowBox[{
        RowBox[{"c", "\[Rule]", 
         RowBox[{"1", "/", "2"}]}], ",", 
        RowBox[{"kF", "\[Rule]", "274"}]}], "}"}]}], ",", 
     RowBox[{"ExRCBsrPad\[EAcute]2", "/.", 
      RowBox[{"{", 
       RowBox[{
        RowBox[{"c", "\[Rule]", 
         RowBox[{"1", "/", "2"}]}], ",", 
        RowBox[{"kF", "\[Rule]", "274"}]}], "}"}]}], ",", 
     RowBox[{"ExRCBsrPad\[EAcute]4", "/.", 
      RowBox[{"{", 
       RowBox[{
        RowBox[{"c", "\[Rule]", 
         RowBox[{"1", "/", "2"}]}], ",", 
        RowBox[{"kF", "\[Rule]", "274"}]}], "}"}]}], ",", 
     RowBox[{"ExRCBsrPad\[EAcute]6", "/.", 
      RowBox[{"{", 
       RowBox[{
        RowBox[{"c", "\[Rule]", 
         RowBox[{"1", "/", "2"}]}], ",", 
        RowBox[{"kF", "\[Rule]", "274"}]}], "}"}]}]}], "}"}], ",", 
   RowBox[{"{", 
    RowBox[{"\[Mu]", ",", "0.1", ",", "2"}], "}"}], ",", 
   RowBox[{"PlotStyle", "\[Rule]", 
    RowBox[{"{", 
     RowBox[{"Blue", ",", "Green", ",", "Purple", ",", "White"}], "}"}]}], 
   ",", 
   RowBox[{"PlotRange", "\[Rule]", 
    RowBox[{"{", 
     RowBox[{
      RowBox[{"{", 
       RowBox[{"0.1", ",", "2"}], "}"}], ",", 
      RowBox[{"{", 
       RowBox[{
        RowBox[{"-", "20"}], ",", "0"}], "}"}]}], "}"}]}]}], "]"}]], "Input",
 CellChangeTimes->{{3.7411679661811457`*^9, 3.741167967531138*^9}, {
   3.7411680291468143`*^9, 3.741168031456386*^9}, 3.741168197592033*^9, {
   3.741321553738572*^9, 3.74132156271201*^9}, {3.741321610024235*^9, 
   3.741321632728929*^9}, {3.741336365744958*^9, 3.7413363721111097`*^9}},
 ExpressionUUID -> "1011efde-e4fb-40b1-93ed-9359668086ec"],

Cell[BoxData[
 GraphicsBox[{{{}, {}, 
    TagBox[
     {RGBColor[0, 0, 1], AbsoluteThickness[1.6], Opacity[1.], 
      LineBox[CompressedData["
1:eJwthwk01IvbgMeSLTupyFqpbKHcFPVKsicqJdeaFtRtodVSylaTUhKRkCWS
EBJDvb8i1559n4xhGsY2Yxfxv98533POc57zKJ+6dOQMN4lE6v7P/+ulko1G
8XEl4NqiKz4brUIE1Sp/q8ESMOS+paRzX4V4QlU0WWSUQA/l2KiFvwqRz7XB
3EmXApn3RfY+dFchZi2kbRVqKTB6z+eDtZYKEdDN65ayVApnPabbaqqUCfIi
406W6xcI+eymWMilTDQrtLpSo74C66R3tA2/InFZqKWkGCvhVJYifN6ynsBJ
tlVVdC385Ftle/2iNPG4OOFWaUYtLF/YstHdWZpwuW2ekUOpBSGm4f4T1tLE
smAy93NaLWw69O7oGTVpYp/y4RJ3jToYe/cpTIApRZQdfq+6WF4H8hqhe5+f
kiKKs724tKbq4cw7an+1uyThsONKT/XWRiDXSXzKCRInnkX6C0jsaIRsZZkj
ClfEiYaRUD2HvY3gtZhoFO8uTpikxUf+smsEW8vBVZ+MxQntNRUHePwbIddU
PDd4lTjBPyeTbVjfCIVXmlJqZMWIIkpZQO6VJuDj0RGwsRYhpIwFFJ5TmqHZ
/bkPe1qQMO+9V6BR0QwW85B+gipIBFz/Y15R3wxjA7VzTd8FicGsSd8pWjNM
Bgm1rcQIEkVS1Go7/haI+ubtCHsECQfGh2uix1rgg/PlRpMQASLh/t/14WMt
4GR70VFFlZ9Q/ZET4KfUBmuOy831J/IS7+nOmX1qbdB89q/NW8i8xM5Z4VYT
vTbgzhml3LnGSxyQP68uZtkGT5we/fK25iXczm/pTvVtA0UlYWLLIg/xkj95
V31lGwQW+YZsd+IhxI2eTir+0w6+j33C12pwEy+OGimE3mgHM+WUbbnruQnF
cxMWrLvtsGHDYKADPzeh9fjQ68KYdpBZkuOj0bkIq15BWwuiHXYJbVn3NZ6L
CLt5772PVAckdb53RREuYjHP1/N7SQeEZ6YMHSKRiPjzrat/l3eA390Kvpe0
FdRX1cvVaugA+56+9SXECl5/OTsTS++AENPAq3Z3V5AdeivYe3UnlC/+2cvm
WcFBxzuJYs6d4KT91q5RdBkbeB+2niR1QXBZN1/wniW8gCM3Hgt1QW1Fdpem
whKu9rOWK5fugqj8ZzemuZbQfELklMa2LhisLitsrV7E8q4nE8t2XXCmLzn2
p+MiFufECKWldkFAgPxennu/8bVDitG4aTe8EBOxGR2YR307X2tf224wixMc
eFI3j40WJg7zJ7tB5iFF0erjPJIMfl3i/qcbZL20zEjh8+gmr5Yk86wb9N9t
tzuvPo9K9A9/9vV1g/FFj/s7b85h8vmvlMgbPZBzK89srfIs6p+OqpS+2wPW
lrqaNsKz2Ojk0RxH7gG/SvnQF3MzSLJZxUp91QP8+rvNzzXMoJu2xfri8h6Y
PL4o2BEwg0ozjTdoYr3QdOSzuDd1GpNu03bqZPYCRFQ9tcieQjKb0R6c3wtZ
oR22Ri+m8NqpkZvtZb0gs5gRYhUyhVams2X+Tb0w8OT770SnKZwTET5Y+bsX
ji1UzuwSncLDr3bZ/32ICm4v6ctK1yZxpfTxtdBJKhxoT1hvbcdBlmb02s4l
Krwg6TPeAQfbkuJK1Ph/wm0eoQp5LQ6+C07780PuJ+RkivnuWs3BE1aUUNmD
P8G/UyLZqJKNud2M57mxP4F44ZwfD2x0XTAs6jLsgyR/quVw4DiavM0nAkz7
ILkpetu82zhuPbm1VtG2D8RW6dermIwju1iKdsajD6gpLxdqhMbx3k2W4OSD
PthmJi1wOm4M0+ZinYU6+iDLTuVQSukozvjduvdKnwYfm10uJkqNoMGt1m0N
zTQQvEpasBMewuJNQ97hHTTYcezOL65ZJv7VuPjOqJcGFkmvair7mKi7ZaNW
AYMGeyveq0YWMFGt7Yrui3kayBZ95FrnxMR1OmIGpxT6wc52g+xC3i+cGbKw
nvXqB6XUNFlfLwb6RDs/yr3YDwH3Prgn2DOQDVcaPH37QTl1u1HnfgaOxryw
7Qnoh8UM/oBwWQYOmjCPEZH9ILrgu/y1bhCbk0OcyR/7QW94lBq7cxBzHfCi
Ahcd+Nb61RyWGMB2ozG/fXx08EteOa6+TMflrXLhLqvp8JfAWzPZETpaL1xP
SlxDBy1ZXV7d73RkxWk1KqjRgdyuWWTqR8dNPa90FI/SIdfH9/UUsx/jnQOm
FdPpsGfgfUNrIw2/HswiGWXRQYYEAnNIwyHNTmG3XDpobwozVsul4a7lHZuT
S+hwrqbzSvkjGrYmjtgrNdDhwAORui9WNBSjOX5SmqND/N5HztHP+zDk1G4/
ZYsBOGAlWuT3loqZXkmU4UMD0PFY8Z+SR1Ssu7xq8cORAaAeq5CV9KGi9J0m
f2OnASgLFJ8WN6Bi2kuvQI9LA8AS3dy7v6EXK1rjgtKfD8DWH3++OC704Cqz
32Hb6P/9gHM2unejmo3bv5xfA+DfPPNFxKIbbewr+SkjAyB591mVj3Y3xnhE
3becGYBiL8Fzd1e6UDVIjXxeYBD0vehuOYldaFri+Oi91iCoq1aI7+zvxDD1
0mc6/oNAbHOROHm9A49dMkhyCxoEd8+VcyEuHahcUJoVGToIcj1mCf+admDZ
nrKvY5GDIJQ/rP98bQdOWnyeeJs2CMeZ6mGWlHZ09UQrlYZBOEuWZPLztqN+
ejmPlDIDUt549qhmtiLf8AExY1UGBC4Grig8a8UWjQrZK+oMuGZuK6xxuxUv
Flbo/NBjgOiGrfdDjrViWvl314eWDBjprErX4G5Fcfq/pTxXGfBxKSzX1L0F
hxXqfKcrGYDL3hfEtZrR+K/NBqvrGHBdSfNhi1wzJhy6za3SxABaRcuxTMFm
tAnQfnq4hwGct9uTwxhNmN8VnZM1wYCqGiFF6cQmDIh2HnZb9wveTz0x8JBs
QlGhCZd6r1/Ad3Pk00n+Rtw5I2H5RpgJxrY2Scb76pCsnnrwjAQTgrvubAjd
WIc09537N8kwYfXr62f6BOowouG4fooiEzQz3pB6WmpxIOOlaqIuEzq/vWKN
eNdilONmnhgHJthLylq6v6pBNuqXhaYxYUyP5ymvVDW+I7tqnTEcAkmV5jfl
hpWY9Udohrx/CKK9uBtCN//3l4tK80yH4LtlsYSLaCVmHhexWLIdgjop0+e2
tO/4RqXU49mZISj7vFHJIPQ7vqbIxH19PAQultc0pFoqMJZVz6PQPwTbAjJl
DG6XY7ClYVd76DA8UoVUCdGvGNSr2JpGHgYqGz05SwQGXOT54RM5DGOR5mq0
EQKvRtVUiMYNw3BZixermsDT3Q55ptnDEH443CEvjEAT72vhRc3DEFRfKjrL
TeAqco5ejCILJE0NWtcJf8HwaqUo+xIW0C7cPmp/joIaLxQcyF9YsPhtI93f
goLNZzcoYDkLxpt6Xb6oU1CBd13W1gYW3HZRKYxhl2DhPrFvi3QWnJh++OOp
fwnSCv5wXguPQKmSuF58TDHuSey2G3cdAeZ24Q5DWhGO+kRLhPONgtmTkkyv
sgKUX3P+WerqUcixO5Sjk16ANp/2ryHER4GdR6oQfVyAHxbH1y3IjoK82eMf
/G4FeD3EQun89lEoEDXYM8VbgKSYZa3DDqPQuENAP/FIPkqVeFqvzRqFloj2
fFzKwz0rhuEZh8ZAo/EBN1n8PXoSVnsvHBkDmoZKw8JYNsbcdZzSPjEG85xd
EWG12TjJc9OV4jYGxpUDfrNh2fhWoGBXve8YuKamndZceYfrJLcNTcaNQRyL
Wt0/nYVzm9ZY7Ps1Bia29g/LpjOx0HJMqO32ONRKVHbv25+OEeYyEaSQcVDJ
p5A6VNLRwxRENB6Mw4+zt8hk3nSUNH4qFvxsHOq3R3gcqErDy7v1pHUyx6FA
Tc5rwTYN1bcGyj9qGge0Zy25nUvFlFUi2gc3TUA2T+ymaxmvMZLQsP9YPQGX
rXZ/dexLwNPUR0IPGibgbLJ2Hld+Aur/HkenlgmIHQ4nN4QkIG3HBzVe6gQM
fFEM6lJLQO0MPdJR9gRUMNmjeTdf4pBpkv3N1WxQCpzfYCkXjw80M0kyumw4
ECmhY+MfizW/S47b3WHD3xKRTruTo/D35HGx3LtsGDWL5d8SEIVqI1P/Coew
QeOGibauQxSSezR3V91nw9F9qXHJ4lFoUfZaDqLYcJL0Sa3n3lOsCnxA00hn
w9rewsD8C0+wknTSW6CWDevtI75EZkXgN775QJThgMW4ikwQKwRN5VUSbNdz
wHZH5+HSrBCs3WFN6ZfjQMOPJbnt50Ow1S15lkeZA9sL+dJxNBiZFPNL5uoc
SBq8KnNn8h4KX4pzawIOyAcUsq0F7uLxjj0HBjw5kFy7vv3DJz9kZQQK8Jdy
wGdtHzXTwxvH6suNLnzmwJWy3uj16V7InhK81YQcoAQalm9leuIsxAy/rOCA
a5VquNI/55C7M6dGu4ED1TfkyzyDTqOsAC3CsZ8Dy8yJc63hzmjhaSyRwz8J
mqzaPRHte3FvnLpv3ppJIP0//wPAdBj6
       "]]},
     Annotation[#, "Charting`Private`Tag$352519#1"]& ], 
    TagBox[
     {RGBColor[0, 1, 0], AbsoluteThickness[1.6], Opacity[1.], 
      LineBox[CompressedData["
1:eJwVjXk81PkfgOUsd02OLleJJNIhV95Wligi2Rw5fjZbUtGihChnSpSUkJTI
sRubmayzz6ccS65JrgY7YxjlGMcMgxn6br8/ntfzev561H0DT/oJCwkJPfrB
/x1Ytd0iK7MKzlubmJsvaeGbreofPqIqmDI8eKtgXAvfH1K1ErCqAM8Li24Y
0MLla7YePbOvGm61lXfx67Qwz3ajo0prNfwxs7FPKk4LR9JEffJWaiBENvb2
nvVa+I6AFV3i/Q4y3I54ROvvxF0q3d5Dae+h5GTtc2rkDhwk+bmqEjWB9MPx
nxRV1DHizB5rTm8Fm5Keyajardh1/5WBFm0qNOtTCpUVlfHD1Ii16/dTIWPo
p+ooEWXcMRl/0PUwFV5serEwN6uErfKzUsecqKA/5NNLtCrhvQoNR0QiqLBY
8+1jZYwSllhU/NOsnQrCU1Z12RxFXFFdG1l25ROMZ/qRxAcVMMlyrcqj6i6Y
9JbxOt1NwkcHY8i6DV0QcnJSf6KRhCOvrh5taO8CbnXy/xL/JuHREk4wl9EF
r8RdPjGySLiCNNTiJPEZps5SveR8SdiV9SZU9tRnqDRuED3N2YCf3vZoT2R/
ho5Wx8DLmzfgnZ2lkeFqPSCxLBaVnyiPXzM9i+g6PWBTPrNYGC6PD/Cku60O
9sBEsOHOikvy+Mi2gN1ydj0QIMSP4zjLY58ALdrL4B5QodBTJtTkcbbE80Pt
TT1wpXBv/8vrclje4gFH9VIv5IdsevN0SQYL/go+31jVBzPnWqyFDaRwVkC3
FL++D9aOlpHdt0pho50Hy/Q6+kDlinJ0g4QUvprNW8hg9sHXwoffW/+VxLPx
12MvSPXDo953ZsX3JPGoe/QzOc9+4Nz//eWD6XW4Q/Rut5vQF9ArqNL9ULsW
v3DNs5i2pkGSRrHHTKI4NnIKPh7sSANckWF8JkwcU22tXJfcaBCYue9Oz3lx
LGQ6Fih8iQal6fc92bbi2GebTq7iQxokqHU1/CUtjtWYb1bN6TSQdqv2jUoX
w88D3lenXhsA3oZM/fk/RXFuFOOAQdEg6Gn8Ne5MCOM7s6ze2PJBiKs7LBo7
J4xDfSfDemsHweglU+PdiDA+Zs2rjfg0CLMPzCxdm4Xxooz0z038QcjZZjWy
OU0Yn8g55OJhPwQ3SGGPqVrCmKhJCY3nDEGaJy+0wmMN9l42q/hiRgeN52qh
aU0Esioux5HWdCjPldjR+YZA2m7araqOdLA9VX5vaw6BZitJDL9f6fDrK2PX
8WACxYRNrOMk0SHXocLMVoNA+YsZnpJ9dMiTzhAoxHxHC+HXY3KMGLAQb28e
a7+KTK937+roYoDjrenLHfICVLnj24XEPgaQFbWCNYUEyJAq+MNikAH1tP6A
pBk+2qe1XY/MYsB7h3jZsA4+0um5su/JEgNM7omMTSfzkbKBnKmvyjC4vG30
NZbmo4Vvtsd5/sMQocu9vUhaRmWu6LLKGiYUpgTpjv68iHot2OHm4kw4XnLV
bcVwEX3X3pLoJcUEp68WPWrai+j48tXcZwpMuBQReDdFchFNZOpRVXSY0Hyw
iCLo5KEdAzkGqs5M2GlbvJfkyUNZnpHzqgVMiGt2ezYRvYDifI3D1W1HwNBZ
LJDP4qIi/9zqcfsRID9Oyc+jcVFbkJjgzckROHP4FzfnTi7aGP0pwvLMCDSm
uW3vqOSi/Gz/G78GjkBndukl7WQuaujOvFnwaASSBmjp/ge4SMyGn7CLOQIi
7mDNvsNBCbtrHhpEjMLuHTMKiQ5z6FSgaa7PzVHwooHsCas5pE6uKUmNH4Wj
cjIbVU3mUK1J7Xt26iiE/BKg06c5hzi2dTPF+aPgdopHfrU6i7zPo2MaHaNA
sFfptaWzyKigXoSkzgJxVZpZuuIsGldpC55vYsHr5MrL8zw2sjTUNJVqY8E4
91D2pTE2emofJazxiQW9C/vVuD1s5BC598GJARZMWLRJbH/LRuVf0ktLZlgA
HitbFULYKDLdc9xHeQz2j7etGs1PIVnJGa92/zGYM2kqNFydRAcW1tu9kv4K
3vFb9jL1J9Afd7z1/My+gcWiHPmZyVcUa2f2pTd+HIKdq+02xo+ixBa1NJeq
CZiak3nR7c1EU7+nr08Un4KJ0f2kdWcZyIQwSyy0Z8OWp9dG/UKGEMWOLdkT
NQ3hWWKnvRtpKBXrurxtmQFRUXxXx7wffeRX/eIUPQvUFb1lIf1e9EF86QZS
nIM9ikonjp3rRhOFN9ZK1MyBvec5WSVyFyrSltjscooDHml5NRS7TyjDvD8l
ks8BlW2ZwYfpnYjfWB+VncOF0MOt8+dutSOuLnkBH5wHppBx3Z8JrWjrrolO
RJuHiPTftH2etKBBUU2DxpAFcFrnoGm59A+SPxku80GKBzYFWxLS45tQyAEl
+ydlPHj9saBvk3Ijusz7mxR6dBGsd5grPhmuR5n2zw/vnl4E0PvttHfpB+Qe
lzz99fYS1NtfV5Eoeo9SdR9ufqq2DLKB2NKlBqMF/+HiXY3L4JObOmz5DKG5
hP24zosPNmzDrGWJd2ibcbvxbjEBJDVfTE26UovqztzSu18kgLfHBJGOa2oQ
19u4RGCxAvOgfrXgQxVyXzJKshhbgQr6cEz2rUp0Oshs5u7NVTDVc/BovvA3
anZzp3YofQdPBTsz64AKdKEfbZys+Q5bLu57Ynf+Lcoz3MWQcSFg0tyLYZNA
QRYzUUVVpwko9t0ici2GgoYKu4P83AnAuy8aF0ZRkPKmm2vqvAlo6K//V/Ia
BaUIejUuXiAgLOixEP0cBYXjOL+P0QTQx0psqm0p6KQdYyKhhICM2OJtJrIU
NCtsSN73mgDNuJhvdyQp6F7N3Yh/ywgI5GhWD4pTULPuIWnDtwRMXzwbFEuQ
kblcyh4WIuBG2Ny2oVky0uk2DTrSQ0BRhrfW+89k1Jz8wGimj4BIrXQDDSoZ
+f38VSibRsARb7JZXBsZPa9Ie8ChEzCwcN75WCMZKWaOl7+YIKB1jHedVUFG
FCeIsGcT8P2fvTcdyGTkJPnoyPIMATmlnNjKMjJKjrDodlwg4HhAdGxq0Y//
gcdPVxZ/9JurUSv5P/5Tk2eL+AS8zBsOvfCCjH4r+GnPqVUCwluM/L/kkJGI
V8YCQRCQpqjpaptFRv8BCtn5DA==
       "]]},
     Annotation[#, "Charting`Private`Tag$352519#2"]& ], 
    TagBox[
     {RGBColor[0.5, 0, 0.5], AbsoluteThickness[1.6], Opacity[1.], 
      LineBox[CompressedData["
1:eJwtTgk01Iv/nSxZK7K1IVRk6aG8J9QHybMVoqIFqR6lQsqWtBF5lVeJEMbS
I2Ws2fX5WvKSJbvMkLGMZWxjxqQG+fU/53/Pueeee+4991wld+8j5/lIJBLr
F/9PvctUjBPiy8DgYcsgR16FuN2oVPMJy0BGv5zRL6FC/NOvaLbIKIP3x+Sm
mvhViIJVWyxO6ZZDZOCCaPmEMvHNUtpOobEcQoI297W+UyZCqAJuaUsV4EhT
leYcViaiFhm3sl3fQ4B7xe+bw5WIdoVO1/6n1aB78Dc7/1VbCR/RjrJSrIcy
ZYfoCrFNBLJZ1h9jGkFLS6oheJ8M8bj0ZVBFZiMkk197b9KUIVxCLTIp5Y1A
Fljv+GGTDPFThMz3nN4IH8YVPht9lyb2K9mWndFsApGALueCQmmi0jZnx2Jt
E/xIJwkWa0oTpW8vrNrFaYZGyUd6EqpShNNuX1qDWiuU+DMFQowkiWfRN4Ql
d7eCHH/7QoKmJNEyGa7ntK8VTB9VONVvkSTMMhKiR+1bgXnC44jpsgShLVN3
gP9GK9iZqGW0vJcghBZk3xo1t4JViDB5j5kEUVxeGZLr2wa3eG3dO/LWElKm
wgrPy9vBzuLhqZGDYoRF391Czbp2GF1zeLBaS4wI8V+2qGtuh7QHwSUFMmLE
SDbbj0Nvh8GlfO0WhihRLNXfYC/UASpyKSaT90UJJ0b+9bWOHWAqFKH8rkmE
eBl5sjliugM0t9nMG/8lTOz4TAkJ3toF5Ei8x2kRJHKGTmcNqHfB0Zhm8fwy
QWLPN/FOM70u0PvNSf9uhiBxQN5LY51VF0z/Z2DsGixIuHmpUtP9usB0p00M
n6ogkShE/qO5vgtGvTuODN0TICSMn7AVL3fDA4c/Df+15ideOBgrhAd0A3VR
8WGVPj+h6DFrybzTDasPmjWMbucndj0+lFoU2w150s1tV0j8hHWfiJ0l0Q3f
3tYnORTzEfcD7+ZcleqBA9K1v5/bzkcs5vl5fijrgQSK+HNTiVVEglenGK+2
B/KTsy0aV0iE/g693F0tPVCTwpd2dpZE+Cd+48YN9QCxO0SqtoVEsMKD7l0U
+wIfK189MXxMIkZO3Eped/oL6MzLCgtLkIgWgb87nUm9IGqja+2z7yemOqUZ
z5hT4UxwyI3kRh7q2/vZ+NlRYbmsSTa0kIetlmZO352pkFT6s8AvkYckw1Fv
vstUaFiJySB78dBNXj1F9hkVXuy+fWlFnIdbh/KX9w9QQTtqiEI4/ECyV3V5
dAANVsLE+LtYC6h/7mm99B0aXP7zPN2etoCtp862x0fRIDpgPHzowwKSDgsy
05NoQPVaGdmfuIBu2pYbS2tpMHKpXnbIfAG3clsD6Ov6IJa8El6b+g1TQul7
dLL64CBT5U3oeS5GsRjd9wr6YKeh+sYSOy5ed58M7K7sA/9sz1MCRly0Nv9W
eaOtD1KWVNf3r+fiwhrxg/W8PlhY1hQLr55H26Q/jp481A/9PL/xJOV5XKl4
fD2c3Q/lhe/XXOKwkakVI/dlqR/GH43bbBxkY1dKfJm60FcgjZXwvrSw8c29
jOXPm79ClMcZ5+hsNh63Lg/fdPArPO7uU+12Z2MulfE8N+4r6HUbuFd2z6Hr
D6PiXqMBuCynucW3kYVmrwuIEPMBGLLRMzxVyUI1Z7VGRbsB2DXFiTiaw0JW
qRT9/NkBmHLZe/1qNAvvBjJF2A8GwPk9XcPRkYUZC3GnRXsGoN7thvrx6lnk
BgfdTdKnw8EaUk/q6hk0DOrc2dJOh9ztcS3xNCaWbhu/GNFDh1ca09sM6pj4
e+viG+M+Oui4VLFn3zJRV1VlVyGDDqxLn9MTQ5mo3uWr++I7HXJ6C9XmlJm4
QWedobvCIHg0XHa95z2B3HFLm28XBoH6mqxSJTeOV2NOP8q9Mgi+oZeCR/nG
kQW+LZ5+v/p00SHlmTGcin1hRwsZhCZrl8TOujEcMRtzJKIH4UD8PtzoN4bt
5LDTUe8GIfG4v8XmjlHMdcIrCquGgOIW9/gumYHdxtPB+1cPwfH0kotODxn4
U21zhIvYEIQHndQxDWSgzQ//lGSZIbCw7NGwt2MgM35Xq4L6EMg//Rx/YhUD
t9GSdBQdhoC8VPpexGMEE06HzCu+GoIKBu26nfEwhrnvDVayHIYt75qtg3YM
YtaFlPKJQ8OQJVvYWC03iE0+gov5R4bhgNbYWzmRQZS+1XbD9NQwtBdHuk5O
0jEj8cLNs97DoDqVpaBTQMe6zvjbr54Pg4N577y6CR0F/+Td3zk0DEK1NBGB
tq94X6Pimc6NEbA+N2PsWURDR2/DFLfbIxBxQ+MdN4GGSoUV2dHhI+BtY96b
eIeGlQaV1dPRI1Bi4/BJx5aGbMuq2dcZI6B/5tL9O5NUdPVEa+WWEVBWGrqW
oEZF/Ve1/FJKDPDMWy8hXPQFJxSa/ObrGTBoFG3VKdqNpr9vNxRrYgD39wxd
nYUufHkolE+5jQGpaWLXycNdeDhE+4ktjQFqAa/fv6vswoLeGEr2LAMezWi7
l3l3YUjM6Qm3DaOgatWzXqa3E9eKzro0XxiFQ+Md+9NLO3APV9LqX/ExoFbz
aKGZbRilkX7wvOQYVCXc0v3+og3pZ/aYbJMdg209hzg3o9rwYcsx/TTFMSiK
zw+nXG7D4czEHcm6YzCTbpaTtqcNn57Yzh/rNAY8bt7O5rpWZKF+ZXjGGOTG
DdtX0j7jmyjXXeeNxsEvq0zxRHUTZi+LcqNMxuG2Tk99f+Yv71NckWc+DrN+
1xIDHzdh1rE1lkt247C49aIv52QT/qtccfbZ+XFwOPL2yOJCI6aWy8ZXPx4H
Zk6JtfGeRoxjNvMrDI6DwgJ5bnVVA96zMurtDp8AFRGHkrVi/+HtPsXOjKgJ
MN5snCf5vR5DrvB/vho9AYPKGX7bGPV47emnurXxE7CkGbk1COvxHNUpz/zt
BPRdSQjrv1aPZhevRxS3T8AauSTd+0MfUDCKoheryITzm4zaFj7WYUTD1qdH
y5hw14tF/htrUPOFglPUeybIr2HWtFBqsP2vLQpYywQKLyZva3INKghsyFZr
YcIO3853rJAaLNq/rmZxiAnNMfv7wLAG6YXLc6nik/CnlrTH4/JqNEim2s+4
TsJEM6n3US2BU1djJCNWT4Gm79VPid+rUF7G61m62BScLfOY1ftahYdLTGQI
iSngE2NHjtZWYf7izIYfm6Zg1kHhv6joKvQPs9zq9dsUGMQIaPWrViEp9ucu
W6cpqOqT6og7VYlSZZ42ctm/8lQ3c2pXORqsGEVkHpqGyDPaqbf5S9GTsN53
6cg0/JnpvCl6tgRj75zgaB+fhj/k1bfk0EqQzR/oWu42DcVbFMPlikrwtXDh
H81+05DS5xSacb4EN6zfOc6On4Y8VvHHZ43FuLBNxnL/6DQc+e7L75P2Dous
pkW7Qmdg2sPzS3hQIT60kH1ICpuBkE9ankUehXjWHNZoPpgBxUCpurmjhbje
9Mm6e89mYLuuS/YL3UL02asnrZM1A49X3a16PlWAGmo35R+1zUDVM1OyydkC
TBNco31w2ywsSZ5rETqZj9GE5tF3DbPwpO3c2JlhCp7rfyT6oGUWNL6NPT38
kYL6vBk81TEL1e62I7Y5FKTvzlcX6J+FWg9+nX8CKKidqUdyYM2CuphqiuAa
Co6bpxwNFGOB01kXs3eGOfhAK4skq8sC4wVnh+LMN/iJV3bM/hYLIr6H1g4V
ZyGPfWxd7h0WvNAVS5kiZ6H6JOc/8TAWHPrUk7X67yyMomnt/RjJAurgCxkv
1yy0rEzdDE9ZUJB7eIojnIUfbz6ga75iwasHJ5N4LplYT3K+KNzIgmIJytP7
sv9izervN1F2DqqK2NVr8tPRXF75pd3GOViXIfBGPykdG3fblA9u/pUH5u31
e5COnW7kb/xKc5AsHCsj556OY+UW3hYac9D3Jth1g3Q6invHu7XBHIis96Zx
g9PwWI/BgWHPOYiwD3hf55CKzMybwkIVc7Dh4tFWbZdknG6uNb5UNQdbKA9y
P0AysjgiQW04Byraca99lJLxG8ROJNb9+mNWhMKMJOT7Qvmk3TIHAT6HXsHl
JNwkTH94YnAOQmoPXS278xItPU0lKUJsCE/1dPUqT8AsNaFNRx3ZsHJS4c5Z
jzgkXaaWTB9jw9SBY++HrePQKT/n6H1nNmg737sYpB2HQgaOT0pc2DAbv2lh
5Ecs/mWdKrzpAhsGsmfzyh/F4rYrhgtfb7LBlpreZV/2HMmF3p2emWwwuel5
sUwxBuP2f3kcwmNDf125Dnv7EyyaihMVWWaD46KlR9m6J9iecPz+8xU2LC2r
3Xny4x9cu9B9kyLAgaUjr3WvNf+DYbldl+hrOfAuInItn/8/6LO1w8pMhQP/
Hdvg5BkTjRZ8LavFbThgbGg/obP8EHkfakMTkziQaGW35+bOSIy9lyK9lMKB
uvb6W7pCkahrciP7VBoHLEZNGCsjEXixUrdbPpMDt3a4rhsmR2BvQaoWOY8D
3honoj9ujMDSlFt9GbUcGOndL7hK4j76BxkaUCY4cLDi55eCNWHI0SzkEnrz
EBrg4hBvdRtHhLfMOerPQ/r7NsFLGrexcyRsatxgHgSXicvHxG9j8ctjwxLG
8zC31J018vIWBorzWt2s5mG7TVNHRGYo/pw0fktynQdHN9Oh0A8hKPymxd04
ch4w5rWfvkoQbtnJ/IzUeVDQDWf/7XIV/5b2Zqj2z4OnXZi/z66ryFvh8KIH
5sHLce/DgJ+++KV7ebvbyDyYl1RvnEz2xZgwyRDSzDzsXUd4eg76oDhdX81k
FRcOPixyseu9gkuxEbdrVLmwb6/FKo0/LmCfwHadD9e44GkVEKvkfBolT8Ru
UwrgwoCcmsuBilNoniu04WYQFzCk1qdd/hTmOjN/7gnlgplzfcy+kRN4l5Lb
lBHBBfKRhr06/k6408nAMyzh1/6BhgFrigP6v7FNOUBwQUfT5/pnqhnaXn6T
lzPNBdL/43+nKe8+
       "]]},
     Annotation[#, "Charting`Private`Tag$352519#3"]& ], 
    TagBox[
     {GrayLevel[1], AbsoluteThickness[1.6], Opacity[1.], 
      LineBox[CompressedData["
1:eJwtiQk01Iv7hydklzUVIZTKliUpS68UWUpaSN1IUVer0ELRVUKmcEmirCUk
S9lixu39uiSyNHYGGcNkLMPMCKXod//n/D/nPOc5z/mon/Y9dEaARCLR/+P/
7FupafU0uRKej18t/ZylQYQ2qv/7CSsh1f6RLvOJBvH3gNqen6xKuMdKz/xB
1iCKl621O2FEgR1zZ6NN/TSIOXsFZ9VGCvjfzCyfttQggulCns9/UeHJQn3S
4R51gvyT9VfeyfeQann5x4KMOtGm2nFyIL4aaqyN+JHr1Ygr4u2VFVgHvvt/
+8taryGQz3WsT2gEqetzu3ZEKBAxFSlB1JxG0BiuEFS7pkB43LbLKaQ0gt7f
VnxpbwViSSxD4DGjEW7nizjJWysQO9UPVJ7SbYIAx3WN6UvyRNWBAq2fNU0g
Xr1nZUuQPFGRf26Z/kwzaJ6O07gSKEe4Gfv1NWyigT89bdE4UYZ4FHtLVNaY
BlJB1GVPI2SIlolwEzdLGkx/HjoheUOG2JP1NPbrQRpwpGeWK7rJEAYra3cL
3qLBYu/GzColGUJkXjHfopkGWxI9sl7ukSbKKVXBRX6tMG8cmEW6JkXIW4uq
Pqa0QX103u8/lcUJu/67Jbq1bZBGebHwXlCcCL6+aFfb3AbNe0eVN0+KESN5
/IAZRhtIese/2vaPGFEuP9BwUKQdmo7I9pt4ihFurLfXVhxph/09Oweor0SJ
lPt/NEdy2qGK5mqV7iBCaH0uDL65rhM2beSGhVQLEQVM99xB7U6IK7jWWZwv
RGydk+zYY9IJW+w4j38+ESJ2q1zQkXbohDBjab2Pl4UIzwsb6S8COuG7qbeJ
jYoQ8Uwkw7S5rhN6h+hltBBBQsYqjq92qQtq8ndnftgnQCQdtlINv9EFG9ea
HnAyEyDU/py2H7/TBUeunytnbxQg9GP2Z5YmdkHD3Z9BhwQFCMd+MWd7ogsK
lqLcvlOWERGBdwv85bth9u6rmDt6y4ifbwJ8PlR2w65GYdBRIxFPL3RILNR0
w8sIZzEVaRKxXcukSL+lGwT3W8RbLP3G68/mZp8wu+HB+UlO6vvfyA0PCjsv
0QM5zm+Pfbb6jSPH/0qTdu8BOT3xLd0OS9gi9KDjGKkXwjTWfm+++gsz3Z5b
TdnSYYN53U1Z5R+4/WDAvgBnOvBCW5zSBX8gzX6P2/djdGjMUem0nvyOJPOv
vgKX6GCRfaTo0z/f0VNFO13xER18L02n9J36juuYbxd3DtJhqlY9jl8wjxkX
qimxN/rgYItodKDLHG73jq9TuNMHhmWXFpOt5pB2wqstmdwHG2xPj7fozCHJ
afn4i9Q++PJJcc5fYA49DezXVNT0gZZL/ELmm1lcN0u7wZDuh4t5byWiZWYx
/TZjq2FuP9jXXVFd/2UGyVxWV1hxP4xOP5oT+jSD105PBHZV9UP7WbbTQtkM
OtrOVd1q7QehGV8DjZgZnJeStKlb6AeOg8oDb5jBA6mmLn/sH4DyT6v9n7/k
429qzLVw/gAUlthVBofycFwvYVXPrwHQZtsI11/mYWd6cqW2yBfY6XjAb4M7
D1+HZS1+Vv4CPC25Y4pmPDzqSAlXsvkCVK87gS3fuFhEZz0uevIFOlpiLt+/
xMWTPyzKey0GQdgnc9mR7inc86qYCLYdhPGDStJAmcJNxzY1qjkPQoaS2YxN
6hRyK+QZZ7wGIbsovTPbawrvBo6L8aMG4dInV81iHgez5p+4i3cPQvnnIt0e
OQ7O3gy6m7qdAVES90re+EygeVDH5pY2BlzdoF/s5M7GivXs85HdDHgbK/xs
0JaN22g/X1v1M2DCMy0q3ICNRhs19UtYDPC72LxRRoiN2p1+RknfGTBXSDVT
zR/F1YbS5qdVh8C/MYQsSRrFWbb9vrlzQ5B/Z5H1upyF/gnu0UWXh0DgXeiv
d89ZyAW/Fp+AIaAvpVR0xbBwMjHJuS94CGQrSXTHP1k4smf0CBE7BGd1gCa3
hoVtGffcyWVD0KRWbSwUOoJFbnhZdRkTvDc/81k8PoxdVpybO4WZQOEkaVH3
DuPSJuVIDwkm1Aedd3u4dRj3/bienraSCcdKxet8VgzjeLI+TVWbCVHm0gki
NUxc35dqqHb4v39sfVLjFiY+dQ/+pvaSCfER9ZZfFYew2iaPZJXHhK6jtg8n
lw8hW69H0rOICblk7XHBWQaaLhlvyKhkQuIPk4dn2hnYkTbhsq6FCZa0yUD+
3wyUZhx/t26eCZ1y3ws1pRl47/SOm+r2w+AhVS9E1/+CuefSKWP7h8GREzA2
KvcFm64s//n20DDYLBT0S88PoMJfrbesTwyDQVZhZAEOYNazcyFevsOg5Gmh
q3JoAGs7kkNfPh6GGrERxrtb/bh870LEZuYw/FJfums4REdtJ8+PvK/DYOeu
mn6wno5OLnUilIlhmGzhf7xfRMdEr/j7DrPDEKBJ+2p+m45aodrkC6IjoLCC
wy5eS0fbyuPRBfojEN1wlkJz78UIHeojw1sjINaROW3C7cYjvubpnqEjsOXi
tmNGPd2oXkLNiw0fgZSI5xW2RDdWmVVVc2JH4Hxtzrfyv7uRb//P9KusEfAu
c80sNurGkz7oqNEyAj0psVuX3erC7S9rBOXVWdD9smvp8NpOFB7bLW2txQKf
khyNdSKd2K5bq+Snw4JfRTtsl/E78HJpreFnExaYCD82EKjvwKyaDycfOLCA
FXDC9NfVDpRhfqQKXmXB+w+G29+3teOYalPAtzoW1B0NXcVOaUPrbRvMJZpY
wJvaU3CX3IYp+28LaLSyYGG9j8CWwDZ0CjaIO9DHApdzrplVh9uwuDehMG+a
BTn7pkpfSbRhcIL7mOfqr2D61L+YersVV4hPezSf+wr0fEaArR8Nt87KOmRL
joLerQEvumgzknVe2JyRHYVNRwUl6JwmZJzaumu94ihEDQ0k8dqa8GGL6/bn
aqMQdJWk5pPahMM5z7TSjEaBqTZkd8W4CeOPbxBMdBuF0fmFsl6vRuTi9qrw
rFFwyCyeu9nZgK/JJ/XPWLAhvlXfmjxfh3mL4rPkXWxQ8ghNk2D811fKqW9s
2SA3m7TtRX0d5rpK2f9yZsPNMDGKwtM6zNagej06wwbbhNcflizrMJOimFwd
w4bdq+3C+qI+4JPxZkHVITZoZhqYaxrWYpiDRW9X+BhIGOk9i62sxtB+tY4s
8hjoOK9M3pFbjcGXBT/7x47Bg6Tr2fzEarwa/6l2RfIYCOX/+BV3tRq96W5v
bPPHoJiWqh5mUI17zl+LLG8bgzrNMzc1XxO4nFxokqg2DvlWDT4kV8TIhnXx
LpXjEIXbLHuzqKibpOpGfj8O8lHp9k8iqNh2dq0q1oxDiWrgbT8fKqoKrc7b
1DIOVtsvFQbpUrF0p/S/P5njwI30ceouoyCjZJGXKTkB8O30XH5zJZql0Q9O
nZyAePlXL6RkK3DSP0E2UngS1Lao6VgMlaLKyguPXkhMwt2B3Qm5DaXo9G7X
SkJmEoxNU7y1i0vx7c+p1T+UJmFqr5HPpbBSvH7Pft2FLZMQM0ku52iVIilx
Sf+A2yQU+8d4N/qVoHylz75VeZOQN9eh7KtYjGa/LSJz9nOgO/bN/lb9IvQh
HC0vHuLAXsWElFyJIky8c3zG4CgHYkNHtVLZhcgXDDxJ8eSAOe1AVf/zQnwl
WmLaHMCBJ6OrDpWsLsTVcpvZ/OT/OnGjcZlYAc6vX2m/8ysHbiu5RRwlvcZS
B4545+0paPm2eZu8eQ4+tFN8SLo3BQpDGfGKa3PQyxakdKOmYIvq24tGi9ko
Zx0nHfZoCrbWXy4nMBuv7DBRMMydgthKj8/qttmosylEJbp1CrT8OqKnj77E
58ulDGzWT4P81aYtv2JeYCyh61LWMA0ii4NEj00Geg9Ei0e1TENZg6hToX4G
bl+YwhPt0+D5VOB64qoMZBi/1RYamAYf7RfHdrano0GOCekwdxq8o1c90lNJ
R7ZtukugBBeMl3OpQhWpGKWXS1I04oID22zwo+gz/LRQ6XrwLy4E7FpYYy2T
iAt8V+miO1xYbrJvrfPEY9SemPkoeY8LlNrbq0PqHiO5T29H/X0u3JdrLFsf
8hjtqzKVIZ4Lyh2BwoyJBKwPiWLovuSCV6O0Ja3lEdaRjp0XbeSCNNnMte5V
HP4r/D0EFXkgy/be8cXjAdqqaKQ4r+FB/B+abFuVB9hovI8ypMyDq0sbDRX6
ydjhmTEnqM6DBvFw1w3HyThKsfO10+FBYW2Fx6hbFEr6Jnu2Ag8WDzbekDoV
ia7dZruHfXhwYJfl1KfkMBzPCREVofKgKSlbKMMmCDnNNVYX/+FBd2HEnQvD
gcidEQtqRR7QDp8z9rwTiHOQOPaslgeWr2oeZL6/gQI9hZ8MWniQapf2Ps7i
OiqJMh4eH+LBYLjHcoG9AWjvYy1bKMIH54b3wWs3X8DcTSJKLkf4wA1xNw2x
skPSJfo7jisfTs2bxZEe2KDb2wKXiGN86B2jJt7otEYRsyNx7zz4sK3VUHma
Z4ZnHTNFlc7xYcJDLp5do4h1e9vWcS/wgfT/+x9kUycG
       "]]},
     Annotation[#, "Charting`Private`Tag$352519#4"]& ]}, {}, {}},
  AspectRatio->NCache[GoldenRatio^(-1), 0.6180339887498948],
  Axes->{True, True},
  AxesLabel->{None, None},
  AxesOrigin->{0.1, 0},
  BaseStyle->{FontFamily -> "Arial"},
  DisplayFunction->Identity,
  Frame->{{False, False}, {False, False}},
  FrameLabel->{{None, None}, {None, None}},
  FrameTicks->{{Automatic, 
     Charting`ScaledFrameTicks[{Identity, Identity}]}, {Automatic, 
     Charting`ScaledFrameTicks[{Identity, Identity}]}},
  GridLines->{None, None},
  GridLinesStyle->Directive[
    GrayLevel[0.5, 0.4]],
  ImagePadding->All,
  ImageSize->{567., Automatic},
  Method->{
   "DefaultBoundaryStyle" -> Automatic, "DefaultMeshStyle" -> 
    AbsolutePointSize[6], "ScalingFunctions" -> None, 
    "CoordinatesToolOptions" -> {"DisplayFunction" -> ({
        (Identity[#]& )[
         Part[#, 1]], 
        (Identity[#]& )[
         Part[#, 2]]}& ), "CopiedValueFunction" -> ({
        (Identity[#]& )[
         Part[#, 1]], 
        (Identity[#]& )[
         Part[#, 2]]}& )}},
  PlotRange->{{0.1, 2}, {-20, 0}},
  PlotRangeClipping->True,
  PlotRangePadding->{{0, 0}, {0, 0}},
  Ticks->{Automatic, Automatic}]], "Output",
 CellChangeTimes->{
  3.741168138733508*^9, 3.7411681776484528`*^9, 3.7411682353993053`*^9, 
   3.7413215955254917`*^9, 3.741321662280582*^9, {3.741336360943344*^9, 
   3.741336389827526*^9}},
 ExpressionUUID -> "4c1b08e3-10c6-4afc-a050-0e3dbf53dbd6"]
}, Open  ]]
}, Closed]]
}, Closed]],

Cell[CellGroupData[{

Cell["Comparison Coulomb+Breit vs Coulomb-Breit", "Subsection",
 CellChangeTimes->{{3.741168509392405*^9, 3.7411685159577637`*^9}, {
  3.7413217101002398`*^9, 3.741321720757092*^9}},
 ExpressionUUID -> "c97b8246-25a5-4f00-b619-eca6a4fef585"],

Cell["\<\
We compare here the energies obtained through the sum of the separated Pad\
\[EAcute] approximants for the Coulomb and the Breit interactions and through \
the single Pad\[EAcute] approximant for the Coulomb-Breit interaction.\
\>", "Text",
 CellChangeTimes->{{3.7227640074737988`*^9, 3.722764017491691*^9}, {
  3.741336272956201*^9, 3.741336298059808*^9}, {3.741336419710352*^9, 
  3.7413365717745543`*^9}, {3.7414051975283623`*^9, 3.741405261999998*^9}},
 ExpressionUUID -> "3c7b13c3-f1b8-4484-99e1-517652503e54"],

Cell[CellGroupData[{

Cell["Full-range Coulomb-Breit exchange energy per particle", "Subsubsection",
 CellChangeTimes->{{3.741168851764793*^9, 3.741168854275404*^9}, {
  3.741336584027039*^9, 3.741336595594573*^9}},
 ExpressionUUID -> "9b323a65-e1a5-4811-ba2b-d47dab926fe7"],

Cell["\<\
If we first compare the analytical the full-range exchange energies as \
functions of kF, we have\
\>", "Text",
 CellChangeTimes->{{3.741408500229847*^9, 3.741408530990829*^9}, {
  3.741411373291616*^9, 3.741411379526082*^9}, {3.741411416586712*^9, 
  3.741411423784045*^9}}],

Cell[CellGroupData[{

Cell[BoxData[
 RowBox[{"Plot", "[", 
  RowBox[{
   RowBox[{"{", 
    RowBox[{
     RowBox[{"ExRCB", "/.", 
      RowBox[{"{", 
       RowBox[{"c", "\[Rule]", 
        RowBox[{"137.036", "/", "kF"}]}], "}"}]}], ",", 
     RowBox[{
      RowBox[{"(", 
       RowBox[{"ExRC", "+", "ExRB"}], ")"}], "/.", 
      RowBox[{"{", 
       RowBox[{"c", "\[Rule]", 
        RowBox[{"137.036", "/", "kF"}]}], "}"}]}]}], "}"}], ",", 
   RowBox[{"{", 
    RowBox[{"kF", ",", "0", ",", "300"}], "}"}], ",", 
   RowBox[{"PlotStyle", "\[Rule]", 
    RowBox[{"{", 
     RowBox[{"Red", ",", "Blue"}], "}"}]}]}], "]"}]], "Input",
 CellChangeTimes->{{3.725790426404578*^9, 3.725790453840857*^9}, {
  3.725790502785564*^9, 3.725790550992629*^9}, {3.726898837998486*^9, 
  3.726898847052638*^9}, {3.741165900638431*^9, 3.7411659400545387`*^9}, {
  3.741166056629149*^9, 3.741166057200569*^9}, {3.741167570406251*^9, 
  3.741167578360379*^9}, {3.7411676879490023`*^9, 3.741167733059924*^9}, {
  3.7411683511705103`*^9, 3.7411683875175333`*^9}, {3.741168536351231*^9, 
  3.741168630571225*^9}, {3.7413217259749537`*^9, 3.7413217809332047`*^9}, {
  3.741322251418695*^9, 3.74132227686432*^9}, {3.741322320459354*^9, 
  3.741322331351248*^9}, {3.741322406684924*^9, 3.741322586107451*^9}, {
  3.741408584165186*^9, 3.741408614204226*^9}, {3.741408660450047*^9, 
  3.741408675782901*^9}, {3.7414104263922243`*^9, 3.741410430020135*^9}},
 ExpressionUUID -> "ade67d13-a5d2-4d84-87cd-58eabf4cca23"],

Cell[BoxData[
 GraphicsBox[{{{}, {}, 
    TagBox[
     {RGBColor[1, 0, 0], AbsoluteThickness[1.6], Opacity[1.], 
      LineBox[CompressedData["
1:eJwt13k4Vd/XAHDKlEjJVKGUjJnuMWa4K5lTkVLme8+5hBQuGRKKJBlKpBIl
U0XmKCV3RymKr1SoVDSQyJC5gd/ufd7zz3k+z7nP3mftu/da68iR/rs8F3Fx
cW3i5uL6d9cQ/tVhn3KHzvX/V0KTe9c/M0sMRkSOZnDOvo2JkE15Qn9a+yh6
LrKQM6JUzHu66AVdZ0xV48GHck76l/RWnpQuuuqo5oBuVA1nc07U+ejA9/TD
8o0VNTJ1nDG12+qRRX30JC6l3qwPiJMxmD09kzxAL409dUc8qonj8+Scc3X0
d/qDXTeL2rY3c4wK4uvZgT/o00sVuU/IPOcElus3hhSN00svJd5if2jnSPqt
TxxPnqFvPFOacS+yk8P1Ttq4nW+OHpR2fffJr12c79aSo6XRv+g5q5bZ7Nz+
hlOnKOTgF/iXbv3X+HeXdA+nYvxIclARNzj0vVrb+76Xs7eEtWckmR+0Qif8
qKP9nOdfmKVuNgIQarKhQUlzgAPSHvytfEtg3T4xl6HPAxyVRKfa4mhBOC+Q
sLB/2yDnj/cOGZ9AYZCtbmg2Wj3MsRfN+hlYtAJ8SnOGct6NcWZa4+4NJ0vC
YvfZv6Kh0xwWXVB/xaQkZIqpudO7pzkd5SnVOs5S8MTcN93bYIZTmnahPEph
FQTp12yv+D3DYTndLFzOWQ1tP/kiVx+b43R8eX5Oe0wGJk6NrodTfzhdfxN0
TJTXg/Vqn4YHNtyoSuyF8MlEJegppMK97fhRgKp2+wNDGmRfS77nqrMCSVjO
pDev1IfsNdasLfESaOKBpG+urwnkfEpYK7tWGsV5yEpdUDGFiesVewXOrUO3
kj1it3qYg+jjRQKiKhvQmnBXv9kTVmB55/SWztSN6PrNd60ng7fB+bGLtvtL
FFFbfMKdiLwd4BSzzzKiTRmdft0jtLHNDsS/sANP5Kui9scdR5dv3QUMW8uk
rbZq6ItQr2ZZlwO8/auu6zKijuJD1K9ttt8D97PetrYqaKIZ3fQ94d8d4b25
Uvzedk20tLPLyujoPnjbul/MiNRCpRdcZ4d+OkFjavuhlG4ttFxA9YT5nBOk
vd816ftWC7HD5kSuLjhByC5JM4seLaTjlKG4S8gZYoPNt8591EJ1q9sd7250
huzIXU12A1qoJXtr9Yl9zkCz3728aUoL9eepsGXqncHq2fYtz1bQkGz57NCO
BBcwcRVHthY0JLjxrorRGRcYyz/+o8GShqYvhfoon3cBx5U1q/Staagtdrp/
8TUX4Jcy9F9rS0NReyf77t51gcXrRcU+2dPQh/nRrvXfXGAD3y9/PTcaurJ9
oHHawhWWc0+2bAiiIZmh15ev8LiB/JXF88JZNMR6UHBdcKkb9DfoMTyyaejW
mcNVISvcgDkol1d2hYY2a4s/2yHrBtJ06ee212jIMXL3r3k9N5CQfFIRXkhD
Z0Ve7vM44AbCWdy8V8ppiEe7XXxdhxskOgqeF31EQ9v4cuSSut2A2zkxCR7T
0Lluf7XZD24wljPud7CJhuQiRczbh9ygterwYONTGjJp2hF8jNcdwuzTuqlW
Ggrd19rRq+8OkyPjT/07aej70ZYz1666wylm1cPaAfy+TedvjRa4g/a8bjj6
RkOHljObjW+5Q/TPYtWmQRoaz5tZ9PauO5je9IxpG6Kh2Rb5ENEOd/h24Pff
jlEa4lsV7RrL4wH07R2s4hkaWl9NKHv6eICTd23RZT4CfZmfN6/y9wA0lbQ5
hp9AhVYtJHeIB6zM1m7dL0Ag5R5GVnaMB1Qt/PmtIUggzcUpIp2XPWC+yuXk
bWECmdh/m7Jo84C4b1fjUsQIVBKyg5m+igEZ0PwtXo5AL7M3WcdJM8BRzWVy
y3oCzT0S1ApZy4A/PkEqv7HNVz7h2reRAZ/5eSQPyBPofRk9Z40WA3KlTGdA
kUDCg5ofc60YUHdiOffjTQQ66LLSrSKUAScsynI09AiUFjNulnuEAWV2roz/
sGtv/rcpLZIB40Izdof0CcQ7m/gnOJYBV2QaHt80IFB2Ok+W/hkGEFXmiyWN
CNTaOvWWU8iAJp3bv1qAQGrQva/tNQN4dxhDpjWBuDJMrs93M0DE5eBjVRsC
vRrKn1LvYYClfY17HfbRC4HnznxiQMX0+ba32wjUMiL43G6UAcZyOUVCOwjk
lW1MfynABM9fAUlmuwi0eSIvebEQE3iEjgU+wRa2FuwhRJjA+VFxyNqBQLcn
O8PSxZmw8DO60mY3gRbbBlTuWc+EJbntXqaOBMr5lbux25AJ2dpn7/E5EyjY
bkmwAJ0J3nyz9Ahsy0L/Bn1TJhgnxPeNYI/YG3lcsmICfZXskZcuBDK++fqi
8x4mlLqqCpxzI9DbvQJC7w8x4Xtdw39fGARaWX3wZ981Jmwmjz/75EWgTcm2
q3vymXDgrXy4zn4CmXmqmnZeZ8KGEKn98dgh4oOpLSVM0DOs51H2JlD3YZZW
VS0TpBoLbCkfAl3RdQk48YIJlqv7DG8fINCdZZsvRr1igkROHt9v7PZ+KRTW
xQRR52GxLX4E4r7QKXLwPROOqLz/04LNmrEv2zPIhB69VwuvDxJI5a7ViAI3
CSk3H80/9SfQ1rOKEnI8JPR29aziCSCQqzefyRp+Er6fLY4wwU6WepQsIkxC
WL+eWAX2WBhdbVaKBCr30pXkQAItsZfd83MNCeYdE5MN2OuV/x4dliXhaVBm
2gy2w5t7z3vlSVh36kKRO5tANQa6fs2aJCzMd5vJBxHovxXi6Y0ECWMjsp8d
sL8NTtx/oEuCQIH5sxjsVZkVSyuNSJAQWwj/gH3016biTCsSylj5jsnBBNpy
f8P3AwwSvkTU6DcfJpDkzmOr91IkxBXVdA1j//jUY2PqRcKTveUtIiEEuiSY
USzlR0LJDdsSB+xxJ4GDj0NJOCq90/cl9pMfrOzyIyREsraUjmNnH3/YejmS
hJaIAkuRUAJZ3zyizo4lYdeTqAgr7Guzw6OyZ0gI18kYrsQOTbJeJ3iOhDcn
9fqeYW9fV2g3lU6CjPvDTV+w5yw9Kp5lkrA7yrpZNAzH/+5+X002CUihYLUy
doG/lGhuDglzK/MbTbDtL7xghxWSEENYyHhjK6qq51E3Sdh21qItAvtv/emX
O26R4BCf35WCfbN/q/bGShJu7SQmK7G5dWumXjwg4a1ChdMEdlezqMIDRIIi
o6qDOxznGzd/xxuNJAhnnywQwXaKU7oT1UxC/h4nJ2VsjVVxAz7PSQh1rt6s
g81b0ie55z8S+A9fDgHsileZYaqvSdhcWT+/Gzvee+aGRDcJKxT3bXPHdvvj
8Ib7HQkejtoTXtjE2fIlP96TULf3+PQh7CXywpu7e3E8Rgf3hGB/vOPj2/gZ
75dlCssjsau3NWWW9pOg3f5GIRY78eP6Z5cGSSiOqrl0CpsZFP37xDAJnGXf
vZOx9fh7VANGSTh2KDc9FVv4sr6ry088XpywzHnsz+rnkyymSLhIc1p0Ebu2
YbxOa5YEBbsqs0zsM447fkj/JuFumfWXy9ie34tkBOZJMJS26cvCNozi3zHB
RUG10yfDbOwVoqyoD4sp6JSHyX/PBwpQaTMfBfpEquA/PzCQ+Xh7CQXHicXR
/8ZPaw0XyRGiQLO10f7f/D7MTnqiCAWBOVyx/96PPkULCBGl4KDFgOg5bPGE
MzlMcQoI+wLuFOwh6eF2WykKtm3z3pmA/bDcilt/DR7/rtuff+tjFqR2kZSl
QK2Y79i/9XuqI6qRLEfBZ6uPFv/W13Z2+vEdeQq8UuXs/61/+713rp8UKfgR
zn/VE3t3JJoQUqVg8keLpit2F73gtJ46BV1tBXy7sD88OnQ3SZuCG8oJ0YbY
ZLzDzjt6FGQRvBs0sL9a6/f3baYguiV66Xrs4TZuMb0tFMjt3HuLFzsgtb+I
aUZBSoSi5zTejxMOz7YkWVKgUNlD9WP/6k7379uO47HpIR5hR10O5xOyp4Dv
0iXe/9vP7u7ZurspWPZMTvYqtsBnxWeJzhQMbgmTD8VOKhAia9xwvOtqRUns
5d7js70MCsoli6xssSV/3FPQ3U8BQ+R4kix2ZtnVBwxfCvbvfZPJhy3LPrE7
8SCe37xp/Ac+rwoz22N6g3C8GqZH7mFrc/e9P32Mgsvlf37bYN9tfBxcHUvB
9ID2HjVsw5NFS3tPUuA/9HR2Gbbp0mADnWQKtOUG1rbjfGIvzn/+4yUKmo6p
TVpjv+oaUhXMpsDw8uFCBex9me0N2jkUfF30IX8RNmNt5lhCIV5fjfGTd3E+
O6SsZqtdhef/aNW/Bvvn0IrP7jUUiJ65v/AT58PDpdPhCbUUmDKW72/GPkqg
6x84FBjFwbpg7NPGDosTnlPwx+qN6UOcT6/bh997/5WCjKi68M04PwdkdKp0
fKNgtHrpEkFs/XfE5aYhCuKmTbne4HzewhqJKBunwOy4jOJh7OFQyvj4Xwo2
HPBzKcT1gXZlO5IXZ8Etv7y44UME+v2pSHOVFAse14XeqMR+pChwTXgNC/Yu
LOiEYe+paDg+vY4FFeofUrmxwx7pbX26iQWbpG/ZC+N6Vf9drumAGQv2HbCW
WoLrXbxGtC7DEv9+RO73Y18C2QX3FO62YUHei8BtMdh9fzPije1YEOapqDOH
6yfPCiFrEVcWNJVUa/Xi+mqjN/2sMogFkVXXps7h+vw6tuXFXC4Lcm/zv0li
4vMxU3ZDrZAF2s/7MjSxG3zPRzNvsmD5toXSl7i+l9oz1JrLWDBy4cOIJPap
tdOnLtaxoD90fdVFd9yf3JcDvU4WJJbpRUbgfiHnZ1hp8BJP4BZ5e/YJ7kck
vNzjbgh5wrs1HxccsZPebHXtEfGEVxJ9/33F/Us4WiZoJuEJtS/K0rixd6Xk
e67c4AnjsVvKtexx/lVpl6408gSFDMcDwdsJ5MtUTBz19wSdk41748xxv3D2
tK9YkCd0vs2vWYz9gvPD2iDEE3KLU2KOm+H/U/a2QOxRT8g+YkJGbCUQ/zs4
KZHgCSoOHhbeWwiUv9v5uHGuJwzI8DxXMMbn3TI5NPGVJ0gbHJDR18b7V32C
UjTwAsmX8no16/B++NgmLWHkBaNXs/2ksU1Ti17z0L3Ah//Yppi1+LxMMi0/
mXnBqS0StrayOP577SrZdl5wviJj2bs1BOoxLx0X9faCZnXjh58kCOTt5hM9
n+EFHhu5P1wWIlB00sfM15NecDLm+se6aRoSy+gKckP7QaM//VXyQxoa0xwr
conyhoUEczWbBPy9dD+UO0vfBwrJbokA/P1TNSb4q3qRLxz+JhWQwkNDZ+7U
21lwfIFV+y35cJ0W6lCOsi5PPADlhOtGWx8t5KrmnnPWxg/q9ruXOEtqIf11
JRJVvAcBpR6yc27URBH1/Bpl7QdB687VvGMsTcQ7ElMgl3IIfJvKU1sENNH0
0yX1B138oaNy1iDeTANlNS/8ihQNgDndq+tCD6sj5oygxbGAAJBQyiwtLVND
b36tIf07A6D8q0p/6atNaMrCuOSSTiC8P7XcieLZhO4JSgh8PRcIq18a7JnS
VkW0/ElCZjYQvlo5nii2U0E7Tn5OOevIBvVlAbTRMGVkaZNiq7uPDcXj7V4K
h5URLDMQ7HFiQ5vEFz+3QGWklZESp+jGhs8Vx0dafJSRWKHB0XqKDfN8Ri15
zsro3eMzPsMBbBgXuDpra6SMvHmNzKwS2aCf0tsZuaCEmM393CNJbKgpKPQv
+62EnJNTOWkpbKjPEn3fO6OEbMUHNn9MxXbS1906poQ0Np7TCrnIhqYYky+8
fUpo2uybbH4BG4T362yNbVBCowJpPdbX2ZCXKK5VWa+Evj03zhy9wYZDRwSm
eu8poTe708QNb7GhtuXYgnGVEqpjmQh1VLKha0JDbjpPCVUrDTaH3maDInNN
w4YcJVQ6nBYvU8OG5sHnBvZZSigneHCRTy0bNPa+KylOV0KX9NPRsvtsWFbC
Kuo+q4TO/TGJul3Hhj8LQlG8yUroNBo0dK5nw0LQdyVaghKKPZE+t8Bhww35
lcXucUrof8zU2KM=
       "]]},
     Annotation[#, "Charting`Private`Tag$22316#1"]& ], 
    TagBox[
     {RGBColor[0, 0, 1], AbsoluteThickness[1.6], Opacity[1.], 
      LineBox[CompressedData["
1:eJwd13k8VO0XAHDKlpSSrULxikHEXFtFcxRCFJXKPnPvjMg+iWSNkCzZUolS
oSi7VJJ50mrr1YakUF4lUrIW8Xv6/TWf72c+97n3nPs855yrSPrt5izg4+Nb
z8/H9/d38/iqDruU24x7ORklVpPGKOGJ6/89071HaXZRFi+1KzpUIeUpI/qA
ImcquJA3QrsheKr4BUPVadz4S285L7M/s1UgpYMx6T+yuDmshrcpL+JMZMB7
xpKVwneE5et4PzSrtcKL+xjtZe1a9z8gXtZg7uRU8meGZZG3j3TEE57n03TH
W5FfGd8cv+3stWnkGRXE13MDvjE4QfV+8fItvIByw4dBxaOMorPP6wM+tPFk
vJUSR5OnGKf9ZCxrw9t5fO/kjNuEfjEk7Na3xv3XwftqKfO9NPI3o6Nr7vou
m7e8OlWxPd4Bfxhfdz373CHXzasYPZZ8uJgf1IJIw973vbz9JWz7kWRhaBqf
dafCBngt/axSFysRSB8Lf0HT/swDOTfhVqFFgKavOw59+sxTT3S4eyNSFBb1
DAp67BjkzXrslPcMWAJo1fanRquGeXYSOT8DipfDsKP/UN67H7yp1tja4WQZ
uNDZPysRPMljM0QNl4/LwFxYuCujc5L3sjzllp6jLLw6u/qMx8YpXmnG2fII
lZXwwKrDpmJmisd2KCpcxlsFDx1Y4auifvFe9rek6/6QhyO6M0pwcpbX8SdB
b4uaElyhuTXct+JHVZIvlsQl0uCEFzPEw1YY+Wvott3fTIdOw+RaZ73lSHr7
VGbjCkN4M2LBNomXRmP3ZQ5dObQFproS1iiskUOxbgqyZ9W3gk1+xX6R9LXo
ZrJbzDY3M+DULRCRUP8HrQ5x9p4+YQGud0+ZtKetQ9eK3rXGBe6AE6PnrA+W
qKLn8Qm3Q6/uhN/HD2wPfa6GTr3pFlv33BayP3EDTuRroLbHL8OWbdsNzTu2
J22z1kT9Yr3aZR17oOqPlr7TiBaKD9K6vMnOHmpzulpbVbTRlH6mfcjXffDM
jBa/v00bLW7vsDAKOwB9rQcljUgdVHrWeXropwNUp7X5pnTqoGUiGifMfjnA
mfe7xw916SDu0V/il+YdIGq3jKl5tw7Sc8hS3S3mCGGBZtt+9eigulVt++6s
c4Ts8N1PbD/roKbcbbdOHHAEVbu9y55M6KCBq+pc+XpHsGy2MWleTkcK5dND
OxOcAJylkLU5HYmuu6NudNoJJvKPf2vYTkeT54M91c44wYEVNSsNLenoeczk
wMLLTjAjs9lvjTUdRewf77tzxwnmFCUkP9rR0Ye57x1KX5xgrdBvPwMXOrpo
8/nhpLkzzPKNN/1zmI7kh95cuCjgAmsvLpxbkkNH7PsF10QXu0BfgwHTLZeO
bp4+UhW03AVcBxWvll2ko026Us07FVxAgiHXYn2ZjvaF7/09Z+ACsjJPK0IK
6ShV/NUBNy8XEM3hF7xYTkcCum1Sa1+6QNY+0TMSj+hoh1CeYlInvt4xMQke
01F6p5/m9AcXGMgb9fZ5QkeK4eJmbUMu0FJ1ZPDhMzra8mRnYJSgK4TZZXRS
rXQUfKD1Za+hKwyPjD7za6ejr2FNpy9fcoUkVtWDu5/x8z45c/N7gSvQ5/RD
0Bc68l3GajS+6QqxP29oPBmko9GrUwu67rgCo4gT/XyIjqablIMkXrrCR6+Z
Py+/05HQykjnGAE3MLR5yb4xRUdKtwg1jqcb2HrcLb4gRKD+uTmzKj83eDaR
tClamECFFk0kf5AbLM7VbT0oQiC1bmZObrQb5M/PzmwQJZD2whTx9gtuwFft
FFe9hEBb7L5MmD93g6Avl2JTJAlUErSTlbmSCeeg8Uu8IoFe5a63jJVjwi5N
p3ETJQL9eiSqE7SGCYKHDqvPYJuteMp3YB0TeoUFZLyUCfS+jJG3WocJF2W3
ToEqgZYMavdcsWBC3Yll/I/XE8jHaYVLRTATIszL8jYYECgjetT0yjEmJNk6
M//Fvlv07/qMcCbMiU3Z+hoSSHA6cTYwhgkZ8g2PizYSKDdTIMfwNBPoVWYL
ZYwI1No60cUrZMIjverfTUAgTeg88PwNExbsNIZsSwLxZW25NtfJhBVOPo81
rAj0eih/QqubCTvsalzrsMPOBqSf/siE0skzz7t2EKhpRLTF9jsTDBXzisV2
Esg915jxSoQFvr/9k0x3E2jT2NXkhWIsEBSLCniKvcRStJsQZ0H1twpfyz0E
qh5vP5opxYKFY5GVVnsJtNDav9JeiQXCV9rct+4jUN7vK+s6N7MgTze1VsiR
QIG2iwJFGCzwFppmhGJvL/RrMNzKAv2E+L4R7BE7I7fzFiwgVioce+VEIOOi
N+cc7Vlw3VlDJN2FQF37RcTe+7Lgd13Dv/1MAq245fOz7zILgDze/NGdQOuT
rVd157PAp0s5RO8ggUw5Glvbr7FAI0j2YDx2kNRgWlMJCzZtrhdQ8yBQ5xG2
TtVdFkg+LLCmPAl0Ud/J/8QLFliv6ttc7UWg20s3nYt4zQLpvKtCM9htA7Lo
aAcLljkOS5p4E4j/bLu4z3ucL/X3s03Y7Cm7MvtBFnw0eD3/xodA6ncsRlT4
SYgrejT3zI9A21JVpRUFSOjq6F4p4E8gZw+hLauFSWhOvRG6BTtZ9lGy+BIS
jg0YSFZg/zjK0JyWJcH1yvmLyQEEWmSnYP9zNQmWL8fGG7CV1P6EDSuQwDuc
nTGFvedtbUuvMgm0k2eLXbkEqtmo792oTYLAfKep8mEC/btcKvMhQcLYiMKn
PdhfBsfu3dcnQazArDkae2V2xeJKIxIUJOdDPmCH/V5/I9uChEp2/r7kQAKZ
3PvnqxeThP7QGsPGIwSS2RW1aj9FQlJxTccw9reP3VZb3Ulo2F/eJB5EoPOi
WTdkvUm4ft26ZA/2qIOIz+NgEsLkdh16hf30Gzu3/BgJgWyT0lHs3OMPWi+E
4+tDC7aLBxPIsuiYFjeGhN1PI0ItsC9PD39XOE1CqF7WcCV2cJLlWtF0El7E
GfQ1Y9usLbSdyCRB1vXB+n7sX9vdKpqzSbCIsGyUOIrjf3evryaXhDqVglVq
2AV+shJX8kgYX5H/cAu23dkX3KOFJHgT5vIe2KoaWlepIhJ2pZo/D8X+U3/q
1c6bJDjG53ekYBcNbNNdV0lCyS5ivBKbX79m4sV9El6rVDiMYXc0SqjcRySs
Z1a95A/B9cbFb9/1hyTM58QViGM7xNJuRzSSkGfv4KCGvWFl7GfPFpwPx1ub
9LAFS/pk7P8lYTrwQhBgV7zOPqrxBq9XWT+3FzveY+q6dCcJa1UP7HDFdpnd
85b/HQkH9umOuWMTqeWLvr0noWL/8Ulf7EXKSzZ19uJ4jHzsg7B7bnseeviJ
BLmlKsvCsW/teJJdOkACve2tSgx2Yo9S8/lBEu5G1Jw/ic06HDlzYpiEZ0u/
eiRjGwh3a/h/JyHC90pmGvaSC4bOTj9JkIpdIn8G+5PWmSTzCRwf3WHBOey7
DaN1OtMkqNlWmWZjn96385vcDF6/zLL/Ajbna7G8yBwJIGfVl4O9OUJ45xgf
BaUOHzfnYi+XYEd8WEhBgzKM//3/cwEqbRSiQI9IE/3r+xvle6oXUZBMLIz8
u35Ga4h4nhgF9NaHdn/v78lqZySKU+Cfxxfz9/kYE3T/IAkKuOafJdKxpRJO
57GkKFCyK+BPwR6SG26zlqXAZofHrgTsB+UW/IarKTh5x2X2b35MD2ueIxUo
ULghFPU3f8/0JDYkK1IwYNFj/je/1tOTj28rU8BJU7T7m/+22nfOH1Up+Bgi
fImDvTccjYlpUDD9rUnbGbuDUXDKQIuClucFQruxPzzyvZOkS8FFtYTIzdhk
/J5dtw0oyCIE/9mA/Z+l4UDfJgqimiIXK2EPP+eXNDChQHrX/puC2P5pA8Us
U/y8oaqcSbwfx/Y0myRtp0CxspsawP7dmenXZ0PBKatu4hF2xIUQITE7CoTO
nxf8/352dc3V30vB0mZFhUvYIp9UmxMdKeg3OaocjJ1UIEbWuGCvvStBYi/z
GJ3uZVJQK1NsYY0t861WRf8gBUzx40kK2Nlll+4zD1Hgsf9tthC2AvfE3kQf
CkLNnox+w+dVZcomuvcwBfkbth6rxdbl73t/KoqC3PLZGSvsOw8fB96KoeDH
Z117TezNccWLe+Mo8Bp6Nr0Ue+viwI16yRSoKH5e04briZ2U8Jme83i/RGmO
W2K/7hjSEM2lwOTCkUIV7APZbQ26efh9LPiQvwCbuSb7R0IhBYUbRuPu4Hrm
q6ZprVtFwbUei4HV2D+Hln9yraFA7PS9+Z+4Hh4pnQxJuEuBGXPZwUbsMAJd
+8CjwCgW1gZinzLeszChhYKfFm+3PsD19JpdSO37/yhIj6gL2YTrs39Wu/rL
LxRM3lq8SBTb8B1x4ckQBTGTW/ne4nrexB4JLRulYOtxedUj2MPBlPHxPzg+
L2+nQtwf6BdtkLIUG654X40d9iXQzMdi7ZWybGioC75eif1IVeTyktVssJ2f
1zuKbV/RcHxyLRsqtT6k8WMffWSw7dl6NhjJ3bRbgvtV/VfFJ16mbLD0spRd
hPtd/IZIfeZ2NhSPKM48PkQg28Duwr1WbCh4EbAjGrvvT1a8sS0bAjiqer9w
/xRYLmYp7syGppJbOr24v1oZTDZXHmZDdNXliXTcn9/ENL34dQWvVy38NomF
z8dU2XXNQjZotvRlaWM3HDoTySpig9CO+dJXuL+X2jE1G8vYMHL2w4gM9sk1
kyfP1bHhbbBS1TlXPJ/cUwSDdjaklhmEh+J5Ie/n0dLARRyYWNqV+hTPI9Lu
rrHXxTjwaXXP/D7spLfbnLvFOdAn3ffvf3h+CUFLRU2lOcB7UZbBj707JZ+z
4h8OfIkxKdexw/VXvU2u0ogDSln7vAJtCHSIpZr43Y8DhnEP98ea4Xkh9dQh
ycMceNOVX7MQ+wXvm+XGIA5cvpESfdwUv0+FapGYMA5cPLaFDN1GIOF3ECed
wAGFPW7mHiYEyt/reNz4Cgd+yAu0qBjj8749OTjxNQeUN3rJG+ri/as1Rqlu
dIeVr5QNatbi/dDzXE7ayB2GLuV6y2FvTSt+I8BwBx/hqPXRa/B5GWdt/2jq
DqdMpK2tFXD8tW3qubbucKUia+m71QTqNisdlfBwh8daxg8+ShPIw8Uzci7L
HVzX8X+4IEagyKSe7Dfj7hARfa2nbpKOJLM6Drugg6A1kPk6+QEd/dD+UewU
4QECp8w0rRLw99K9YP4cQ08oJzul/fH3T9UP0d+3FhzC87Wsf4oAHZ2+XW9r
zjsEXne/JB+p00Ev1SIsyxO94BrhvM7aUwc5a7rmpVp5Q81B1xJHGR1kuLZE
ukrQB2rTfG0dH2qj0HrhDWVtPmB4+9LVKLY2EhyJLlBM8QX3J+VpTSLaaPLZ
onofJz+4Xjm9Md50A8ppnP8dLuEPfAaX1gYf0UKsKVHzKH9/EKBll5aWaaK3
v1eTfu3+kPmf+kDp6/Vowty45LxeAHSfXOZACaxHtaLSIv+lB8CyVxvtJ3Q1
ED1/nJCfDoBHFvtO3LBVRzvjPqWk7uOC9VJ/+vejami7VYq1/gEu5I+2uasc
UUOwdKNotwMXWqT7vV0C1JBOVkqsqgsXnlUcH2nyVEOShRvD6iku6AobNV11
VEPvHp/2HPbnwqzIpWlrIzXkIWhkapHIBaOU3vbweRpiNQ7wjyRxoa6g0K9s
hoYck9N4GSlc6MyReN87RUPWUp839aRx4ZGDof62HzS0YV26TtA5LrRFb+kX
7KOhSdMvCvkFXBA4qLctpoGGvotkdFte40J1opROZT0NfWkxzv5+nQvsYyIT
vbU09HZvhtTmm1xIaoqaN66ioTr2FrGXlVzoHdugOHmVhm7RBhuDq3H8rNUN
/+TRUOlwRrx8Db7fYMtGuxwaygscXOB5lwuG+9+V3MikofOGmWjpPS5IlrCL
O1NpKH12S0R1HY53XixCMJmGTqHBzY71XFwsv9LoCTQUcyLz1zwP5095xQ3X
WBr6H0mp4hw=
       "]]},
     Annotation[#, "Charting`Private`Tag$22316#2"]& ]}, {}, {}},
  AspectRatio->NCache[GoldenRatio^(-1), 0.6180339887498948],
  Axes->{True, True},
  AxesLabel->{None, None},
  AxesOrigin->{0, 0},
  BaseStyle->{FontFamily -> "Arial"},
  DisplayFunction->Identity,
  Frame->{{False, False}, {False, False}},
  FrameLabel->{{None, None}, {None, None}},
  FrameTicks->{{Automatic, Automatic}, {Automatic, Automatic}},
  GridLines->{None, None},
  GridLinesStyle->Directive[
    GrayLevel[0.5, 0.4]],
  ImagePadding->All,
  ImageSize->{450., Automatic},
  Method->{
   "DefaultBoundaryStyle" -> Automatic, "DefaultMeshStyle" -> 
    AbsolutePointSize[6], "ScalingFunctions" -> None, 
    "CoordinatesToolOptions" -> {"DisplayFunction" -> ({
        (Part[{{Identity, Identity}, {Identity, Identity}}, 1, 2][#]& )[
         Part[#, 1]], 
        (Part[{{Identity, Identity}, {Identity, Identity}}, 2, 2][#]& )[
         Part[#, 2]]}& ), "CopiedValueFunction" -> ({
        (Part[{{Identity, Identity}, {Identity, Identity}}, 1, 2][#]& )[
         Part[#, 1]], 
        (Part[{{Identity, Identity}, {Identity, Identity}}, 2, 2][#]& )[
         Part[#, 2]]}& )}},
  PlotRange->{{0, 300}, {-29.96207699636282, 0.}},
  PlotRangeClipping->True,
  PlotRangePadding->{{
     Scaled[0.02], 
     Scaled[0.02]}, {
     Scaled[0.05], 
     Scaled[0.05]}},
  Ticks->{Automatic, Automatic}]], "Output",
 CellChangeTimes->{
  3.725790454653599*^9, 3.725790514460441*^9, 3.725790551700067*^9, 
   3.725790631266589*^9, 3.7403738145650263`*^9, 3.741166057760421*^9, 
   3.7411663256639023`*^9, 3.741166397999399*^9, {3.741167681216887*^9, 
   3.74116773414235*^9}, {3.741168364703821*^9, 3.741168388275528*^9}, 
   3.741168493622514*^9, {3.741168554100766*^9, 3.741168631110404*^9}, 
   3.741321812929913*^9, {3.741322277676489*^9, 3.741322287590631*^9}, {
   3.7413223209987288`*^9, 3.741322331941712*^9}, 3.741322442471143*^9, {
   3.741322494162796*^9, 3.741322536978307*^9}, 3.7413225868968267`*^9, 
   3.741336603499173*^9, {3.741336654850569*^9, 3.7413366844734993`*^9}, {
   3.741408661391165*^9, 3.741408676235229*^9}, 3.741410430933453*^9},
 ExpressionUUID -> "3c20f12b-2592-4eb1-99bb-bc5ca2be3aec"]
}, Open  ]],

Cell["Where the errors between the two are negligible.", "Text",
 CellChangeTimes->{{3.741408500229847*^9, 3.741408530990829*^9}, {
  3.741408683549642*^9, 3.741408692001103*^9}, {3.741408910060608*^9, 
  3.741408914724769*^9}}],

Cell[CellGroupData[{

Cell[BoxData[
 RowBox[{"Plot", "[", 
  RowBox[{
   RowBox[{"{", 
    RowBox[{
     RowBox[{"(", 
      RowBox[{"1", "-", 
       RowBox[{
        RowBox[{"(", 
         RowBox[{"ExRC", "+", "ExRB"}], ")"}], "/", "ExRCB"}]}], ")"}], "/.", 
     
     RowBox[{"{", 
      RowBox[{"c", "\[Rule]", 
       RowBox[{"137.036", "/", "kF"}]}], "}"}]}], "}"}], ",", 
   RowBox[{"{", 
    RowBox[{"kF", ",", "0", ",", "300"}], "}"}], ",", 
   RowBox[{"PlotStyle", "\[Rule]", 
    RowBox[{"{", "Blue", "}"}]}], ",", 
   RowBox[{"PlotRange", "\[Rule]", 
    RowBox[{"{", 
     RowBox[{
      RowBox[{"{", 
       RowBox[{"0", ",", "300"}], "}"}], ",", 
      RowBox[{"{", 
       RowBox[{
        RowBox[{"-", "0.00000001"}], ",", "0.00000001"}], "}"}]}], "}"}]}]}], 
  "]"}]], "Input",
 CellChangeTimes->{{3.741168670979035*^9, 3.7411688252008953`*^9}, {
  3.741321842616331*^9, 3.741321854663926*^9}, {3.741321907976462*^9, 
  3.741322007351549*^9}, {3.741408697036919*^9, 3.741408779178293*^9}, {
  3.7414088109665337`*^9, 3.741408882302599*^9}},
 ExpressionUUID -> "bf8397c8-5348-4031-901d-01845368c763"],

Cell[BoxData[
 GraphicsBox[{{{}, {}, 
    TagBox[
     {RGBColor[0, 0, 1], AbsoluteThickness[1.6], Opacity[1.], 
      LineBox[CompressedData["
1:eJxM13k81c33APAbEpItW5KdbJUlS5qRnYQoCVmjQsmStJeKqCQJiUiSJEkq
VJ+PJEklJCHJvofs5EE/3+5n7vz+el7v58ycOefM3Osmudtv2x4mGo2Wt5RG
+99/LWcX6/5y5NXTiVRpjzpmXGTDd2s0IItXbyFEGxli1eXMEbn9gI3vn82J
bli2+eaWtr3/HHL3GHtRSJfQtPC7f1Z5PyChq3M2Pt1aevn/nGp1SKZoXFTA
JuLsP/trsmsWPS68Pve65Z/dvidJFPnY8mVNQf7/ufX3EfkimeFou3W3/jmk
lpdbt/kyN/O+mX92i5qSLLq5Oupxir3Av3rSXJmLbN9yOtXl/7ME0Sesy+V6
mY1LQPDf+ayyqkXlM+zPjQ/9s54u/5qic/ER7qe+/LPb9U/iukBtCdfzdUL/
zrvhu6po6nPYy4Er/9zqHC6v67mJQ5t3nB4PkucsqsmNeq7hKPzvfI9LYkV6
UsvVHYvpPpa0vCjn+o3c03Ir/lmRZ5IUXSy69m4k3S3Mk+TF4NSH70f/Wc+L
WahoskdGYcBe5F98OPMx9HR4kMHzmu4DTgvnfVwjoyG78t/5X3VZdfVA3h2H
y3T/6vgDcx5pip8e+We39yv5dVeKv7qVtlP0X/zk6AiMiN4k8p78Z9qi49y6
k4tKb/ySXvUvnl3JVOR5yEyA59I/02ojmXRrOiti1g/TvX5NI6lnZ8PjYCf2
z6mv75A5779dOUXQbTf9FYpucFyaJiX+z2Ln+8mLWc0RZRF0P3o1CCdXerD+
GvrnkGqVRUV5ZWNvwhUl/sWrjSpJ77/PaYnOdIcMD5MS2kc3ZUfTzbntF1nv
r3O66C3dCd3fyKgHs0T1JN3FxVXQuL3ov3YFyX82m24jZ0XO6kw40a1dVwqf
bjc8tiSaiovWkj6RiwtXvKWbSWeElHj3flJpkm4ZvhJYP3dRQ1dB6p/797bD
KE2LIGsnuuX3lEEjP66nu6/S/Yz2Bv53v3okqIRutrJuMq81RiV8gm7WqD7S
e8UOv5vy0v8Mpn+QEtuEch7uopuml0bWX/o+QEbRfetGDxn1Nkmp+g3dhV++
ksazzj7t43SbRTWRs+slHoyvlvlnab/f8Klvew/rLroTDn0lfTLS5VZE0S1i
/g1Ktuzdo/SGbo8nPbBBSCEdjtN9a9s7GGX9q33raln6+1v6kjS++EhytyPd
8kpf4OwbP7egK3TncXTAvBnV2xeK6c5cV0x6q4//TBiju+59E5Q4kC/6UE6O
3l99PKxPP7qLdKB798UvMOqnTmJVJN0SEW+hseBcQ9trukOY0uGs1Wuh8VG6
zQQ+kk/Dz9qxyq2mvz/RYuhTbBgn7ED3wOQbKPlnca1iJN3FkUmwQbWcD76m
u+JhPXnV55LN1lG6EwrKoMldi2h3WXl6fQFP4ewPrqpD9nSnSi+cx/9l2YXL
dNsWvYFEwMpOjVd09/IWw9LKPS+7+unW2x9LflbKjY4TUaDnq/xA1kXM7DU2
p3wnh2zuMoITx+gWvvmG7DG4uvzeA7qrld6Qw7e/99l+p7tC+y2cnpUuZmFX
pM/jdgG5yPFg/DNtunM5KyFHQeEBTy8UTyL5+JkN+RPoBgZv4coAyxWl7+l2
Si2HMpU3fh+aorv1wBuorNT+Tnq1Er3+ZZWkRoTyra92dCdoFEDdruDA8xfo
tr/znjQ1eGOmnk93iHIZaX17qXhHF92tBfdI+9kdEzECyvT386KAdHdI/WRg
THfqshjok99/ZzSIbmvb12Tgco2jael00+LPkif8z1htq6W7eioPhn7+IMPE
soZ+3qt75BVF/v+eqNMdvTIHxoe7fHH3oOIR52BKZ+Z93ut0077lk/f1x069
KaH87DjMTYG2AaN0txq9gYX/hStKSq3950zHd/CNfQ3tiw3dIQ2J8ONz0fqQ
s3TrqT6FNXz7Hqk8oVtF5i784ffkfGsr3a3rM8jOiv8connW0fu1zScHFExU
9PToduPPgBMXolmH/egufpgA5zsam27fplvv1DWSVV/26dYqKt5WSHKn+F38
O083bdwdRs41Pd4ppEKPJ98jeZSZktato1t4TSGMdVx9YYkpFed/RK64aBHQ
4kI3bcVTMqUgwKkgmHJxOCnVHW96NYruELtkmMFPqO3LoDwdTSoatq3aVES3
3vlImBPAyi5UR/nsdVI9VWl8aJDKd+saWVhp3VK2WJV+PyXpEMwd/piyiu7U
goewWCnpebAG3SHXIkkjx+JUK0vKs/fJ8oiuy3J76Ka1p5GWBRxH5k9STpWB
NV3rdtfFUt4eBe34d1jmZFP7DR6TjQbHtS+U0t0qkUq6BNyWdmmi1mdbwPbb
pVya49T6jFtwX2Xfn2WcanQPXCQHZrm6uqTpTn3yCPorra8mN1JxxwTYrGX6
d9V2uvVWJEBLI8e1p33olhDPJQlrX+fms3TTVJyhonNIpO5Nar3GBXjT+/qr
lFxqfUoiZAvO6J9/T7e1choMPvdihWsLdX5ADOyKqjB7PUmtL4mHtkktR8S5
1On16B+GJfdHM87I0q0XFgdVny2uawFU3COaTC0WXqxnSzdteRTJ9Vlpfep+
uovtb8JT33U9aOepOPNxcqDLJsYtkbLLedJx1PNN8RNq/dVrZPn8kWGJD3S7
qSdBraWXxc+2UuedjyMzhFKs2qao9RujSX6ZJ6f0udfT/TQOnlMpzb4jR3dI
XCg5Aup/LNKl4jyh0G1zP8fuHXTTtgXDyh1zG0oOUM40IMFuHm+pUMrTR+DD
g9IJ55Lobk2JhiInNN+351FxniswInzzpMFHyjG+cOq6k+zdNsrCu8m9qX62
zH8o2znA2uxz5z14NOj2t4aGL+Ly3q6mbBZO5r3LbJPeRPn4PlKi5hVPqB3l
ASN4tblyU6cvZSM/ON/fdtAojO7iHaHwwNR4cvotKp5znPzBzPaZ5RkVX3oe
mvOsnPX8RMXdzsJC0bVK79op+x0l5RT0HWVnqPUiV2Cchu3FMF5N+jy/HoEs
BvsKu+QpF50jA62O9xjr0a3HEUe2Ol4RzNhJxfUuk1v3pRqz+tFNG4wgiw49
Ddp7gbLqEagcUna3LJla3xhNJkZ+r5F7Tlk6DLLfHFgUXkGtVz5KHr33V6Wn
g7KXDux+wudm+h/lEAVyR5Hs1ft8WnTXnYelH7WLlijSHXL8FFSr3zK4T5+K
r/aHdzpcRMvtKWfugDzDAVvk/SlPHyBPz4YejwinfP4YHGRLeNCbQllPBjoJ
PGwwy6e8NRh+lCxa8uAzZTF3csPaL5rsXZSdTpCZOp17vGcp2+4nBU2nYj8s
16a78gwcLd8yLbOG8r0g+Nk8dVeICeXtHjCzYrzohytlmzNkqNVmKa1jdIco
BEK36uSwmBjKAyHkxm2jvYMPqfW3Fs6rNbHY/A6ddxyO7kh6nN5Mt55AKKys
/81Hm6biS86QDxyMgnfxbqC7eh8Z+iPhe74iZb0T0M15EPAZ0R3iGkZubNFP
9XWmu3j6HBR0j2f+EEytH/OEo+39e2WiUT5n8rPnpo9nHlC2DoSZ3dfX/Cih
fHw/GerVG63ZRHnNKejaD8avTVD5Uy5DnQPXdg5y6dDjjQdJwaGul2bylPl2
wBE/HbF0fcrCRmTFSNTZv450h2SeJzMPdXQ6BlHO9YehE1pm+Veo9SEAuh6J
fMh7n/KyYFLnTyuXbzHlWztJwRMageXfKUfthaOzF79Jj1GmbYefTzdrn+Hc
SHe/B5lJU7/VKEu5OQCGngv/q7GJsttq6MbStPuaPd0hZufJjRdUygYCqHhB
EBRkC1Mwu0zZP4gcvfg98m46ZTM1WLl07fA8SblVjXxw5dx2x3oq37JgGMpd
n/98mIpHe5Ju15REeDkAPX7xGATLQ04dkKabNnyMFIqrbX0PKJdrwFFBBSNp
O8ofDpGVCafun/ajHO9FZonUcDRGUE7eB8NuyR3USKM84Eq6iZ34Ev2Kcqsv
CVKr1g/UUg71JIWlZBJMhyhXWMKxu0f/S1sCqfcQACtlP7vMS9Ad4nsMZt2X
LHHQoeKi2+EFhWDZ59spZ+pC94cfI3h8KYvsIcEa8YH9FyjP+5DCjw9tfX+b
yvfiLDmuUp4n9YKK94SQVXmigqdrUD5zMmt9wLHvvyiXepAX8t81rV+sS3ev
JemuLaIXLUZ3yOETELw8ePeXFhVXDiSFwVtWUxvKoiZwjBTySfOhfNAGTtuo
3LQ4R9nGB852mZVP3qT8bDdJO+4+lfqEcv4BkoXruNyWD5T7D0K2tJgdE62U
abNgmebD0NvTlIODIN/Ht08382yiO1UKCro0tY+tpjukOwCKjI7zpmyi4mWH
SbELy/TNdlJuMoVSInL+owcp226Hq3N0b9+6QDnInlQ22FlpkkK5dTepUuc3
N/yccuZWcr1PhHLSZxS3JLXnU3cZd1Hnp/pDEPPi0u9ZKj6/G0os72uy4NCj
218XSjkfHpcUpKyiS8reX8Q5JUlZgh/Kj1yRrlhDOVWVVNwosvHOBsoX9pHK
YRnbgo0pD1vDtVVqPltsKNt5kCorXp+VcKbcfgCqeWy5OeFF+ZYhXP+oPvdj
EGULH6g55VF+O4TyjD3U1h9uCYqknKkKdS6fnNqcQFlPgATf2LjF0ymf94Sb
xOPkxh+jOA808JbU/fCK8qXt0Ojpox0p75E9ocncBt9DXymPuUMz07JQsxbK
sXbQ/Nq2W6t+UeYxJy1+ND8dnUTz2kBaye7/9J5Jn5rXPtLab6r9FhflIA9y
24vzMwEilKe9oS0zD5+pHGU3OWhneUtBVI2y7Q7S4Ya8/gik3MoLndqe2Zdt
pizjRboo6fsn7UD7tUi3w5/D/d0pZzrA3a8dbhv7Uk5dS3qyd+eLHKN8euH3
0/bAyt+hlP1VSa/k+a7SaMpeeuT+nktzN29RLrcmD6oKCfhlUhbzhv4n7iob
PaPMqQ8D360zWlFMWduIDOImdg19omxtQgY7mB16W085RIc8erf2UkIH5fXW
5PFBtzTf36heQ/Kk1uALg/8oRxvC02ePfRFaYkDNV58M+bS4b4CPcvVO8pxA
DK1EjDLXThjmKiZ8Q5GyigXU9fz0wVuLMm0zOel19AQwopxuAh/7yq7htqEc
Yk56BdY0tzlTLt4IJY6ciX7mQzlyJ/n9hLJB+BHKPLpkTMj3MYdQAzRPaB52
4Z7yNcprd0GmS+o7/yajfDLkq6hWtposyiXWMOj6lZfpBag/U1I5QefAkVLK
Xo5k562eVeZfUP28MPlObJVoM+Wg3dAuQ//s737KJ/Uh18MhtZIp1L8uLHuc
1BnLYkjNdx155plZ/D5eysV8UPvFhKmOGGUnQzhMpv3hVKJcrU0+KNn6sEWL
MrCDu9/POuUZUdZbQYpUPOAKs0FeR36ttive6UK5QRNGfmMOVNyPznOBRo25
0nNHKC+8n7lm529VoZQLdWB+B0d42jXKrZA82FugfTiFcvQmcvWgZ7/pQ8pu
0mTrCO8tkUJUrxaZMFlkOVhKmTYHrP/b//f1F8o8+iQ7bcWTmGbKwpqwhKVs
955f6DwN8jj7IX7taWR1qM4lUcax2IjyRnKA7/ORn7yU9fRgutBxhVwxyrRG
4Cy6+sc5JcrVMlBQsjZyhzblYiuyUvasrrwxZQlFGK64dnjGhnK0Gam37sed
zy6U0y3gtHrE9tT9lN3WkU+0NRYfOkrZfwPpA9vzjcMo5wIoZXDVSzgGrd9I
NpoAkV8pqF4r8vqWvk/kQ8p7d0IL6/hT0YWoHkiy7DBc5/GOcgiNJB2GWzVq
0P6tZLBLcgxbC8pvRq71MDf68QvVr0727JuaeDSN5sEMUw+k3w9ZbIzqI+0D
bBy281GuVoe8wfMccuKUGwzgx+MPiWklyoXW8NwZ+4OftCmHiJAbQxdLpBhT
LhaD4xF5X/y3IUvA7Cuu5w1dKc84QcezzDsb91OmqZNsh+8rBhylnLrw3ry2
zC8JoywhT3o4/f6Sco2ysgnksb5+TyOFspsGWWSodawiC9WvAQ9o/bDwKKDM
sxqKKJ2RmHmL1m8iy8Wkx6OrKVtrk8F879+v/km5XBPKsO5PKuqjPGACv/zh
8tsxieqRIE8P5hkMMJnQzbYNKrfZCZ7npjwMycbamb4VopQlJMmI8hQyV57y
UWNSkzC4ZqpB2X817Hzc7dmsT5lWS8TcvaR92Ar5F9h0Yy0n5y7KkeZw4FJN
S9o+ymYmZOLp4KcbgigXS5JmgSLh1SGUq+Xh5J4ix31XkAGZ7rB77fxNynoa
cJslK1NcBmUvQ0jTz/qm9JSymzb5aL3Vg5LXlFsFoaP86EmHCtSfPmQTjbce
bkD9GZL53Doy4V0orkZ6MjdPrRpF/bCTfFNnPz2bp2ytQRb3y97estSUbnsD
8mDzh8B2IcryanBlja/JMRkUNyLL3/GK8KhSJkxh8IvngxmQcqs0KfPI4Q00
p5wqB2tS52Jr7SgvvJeQ2Dte+z0oh8iTayOMAZM/5YXvz6YTfdw3T1IW1oAX
/a50rLvIyEdqeqgWlMVRHlaDnXbfLjmnMfLBGPNjLuM5lKvVSD3dVWqXX1HO
XQOHVN8sliqnXKxA3pLd872wlvJRAM1XsD/a2kY5GsIpzkch3YOUrdfAdJqN
7akZyhKa5Lbx8dX8S8yo+bKStN6E/7KWU1ZRhjk/QJW+BGUeeehU1ZrWoIys
TrK/DQ3224D2K5D5+fLmrCYoLgc9sypWJW+jbC0B+VL8R9RdKS/83im+xv/u
434UVycPhhUmuB+lHCIHVx5zOjAdSnnh71fz4fZ7+dGUJcRgaqBXS9AtymxG
cLffkLB6JqpnCsgcCNo28hTlWw67vWYuP36Nzgcwc0/IO99PlPUUSZ/drH+V
6vE8lF0jtfvbkSXg0C6+wMwh5AYi1z7h4d4ZyrlqMHCHWJcM62bKKqTGtnSx
Dl7K/lpw2krR/s4qyrRu4uWW3GuuCsiC5EkzzU+rNJBVoa4xwdKkR1lFg6QZ
GOgmWqB4MyjRLT9ib0/ZTYYM3Wj1RNATxQcIU+3a/lo/ygvfhxwajjLXT6B4
LVGh2upsE468hIxau/cG93V0nha0Vhqo/pyC4sKQTz6QIzILeQ1ZKzNtaJ7P
6AfES54+xVZCWU+YtBdjKSj7TLl4LSmy8tJw6HfKIbpkkxCPomEXiquSKfzx
HotGKHtthO68osmvZ1F+XlKGK63uFJs5lV+E7OaQ5wH8lBfea+aSnM0z4pRT
10EflvXnC5XQ+o2k8qKXRLAW5ZBxMDS3aXK9IWW3VTB35t26MSsU5yYDp7Z4
P3FE+ZTJ9eNf0vz2Im+Ak8M7m9YEovW8ZOHgT4GBU5SL5cgT/R5bsy4iryF1
e/oivOIo++uQtE6/Erk7lGnlREnrxH+d2cgaMPTnCY27hah+YdKkcZGfeyny
CpKtPjxTvBqZBX78uqz95w/KXjrwSvX1lbd6UH1roPXnFTscx1D+5STfx9tR
wn9RHJC1ZbLldRxbKIvD+LcPF8UJUqatJ+2LVTdul0KuBiJkQRDvWuRx0PQC
5lRtoMyjAVPy3/ZcMaZspgLdnm6WtLChrKcEpXKrHDmc0f5G0Jm9I7bcC1kc
3n/w4/OFIMoSMqSE+7k7BmcpL/x7K0FY4fD8FRSXJ3mrq8xeJlIuZoKXwoNF
g+9TzpWHTJtWDas+Q+ulyROTb98OFlNulYbjj3xuPPiM9kuTB/bw7t/TiOoZ
Ap2ihbqSPYz1pHOtC9/PMdQPG6y7vLg7gWZB7V8ErQyzX9guo0ybIspmtl3h
EaGcKws35f1xq5BDcSFY6J26PkKdcogUVJE0ZTPSo7zw9y6zYfDHXwu0npeU
jI59/MqBsr8aTDTdeP7IXsrVypDvb5ud+iFUDx+8nB+h+PsMyi9JshxcN58V
SblVAJ6Urfuy9yayFDnRdPKeVAZaLwgPxkofa85D+RTI7i0fLRJfo3pWk67M
ARJ2Fej8tbDhpdA473e0nwVaBxa9/9yF8kuQHxT2JF0cRfv/AoO2pX7Gf1F+
JfJlQp7BIk5Laj8fVLN2ECSFKReLwIdLaP1HZSnrsUKZ1xnkejVLRj23gi2v
DesijxECa8c9s7cg/wFRXYnaXvbI5QRrsj6nzB6UfzV5xra3pSUAWRhOL736
NOk0Ws9D+r/VCN95GZlG6zve5Lg8AdVDg7vVzq+tSkfxxWRjnwLT5Scozktu
v1P9zaQIxTnICvsjD5g+oX55oBGP2KmienS+EEm8L7U+3onWS5AaZ/bLaI5Q
Xvj+z9Hkmx6ZQ3F2Um6o8NMjDivKDeD2Pdfb3kKUF/79KuzMekhWhjKPFIzm
f2TSpoLWFxPsFdtFkiFlCWl47vzMoL055ZAl5IzOnTf8Oyn7S8JDo6Zx1R6U
U9fAgQdDXpH+KF8/8HSPA2an0P4J8FMY8LBcQuv5oV11e8freMoL76My/GLB
ibuo3mVwlxnfiMtjtJ9G9rIlKRq8QvnHicMfpD1l31PW4yOZLmUns31F8Xbi
qrlG/a9mFOeAokuLeKr6UZwTPvhkYp43STlaCmpGVp2PY9pKxWnkWwt78igX
5RBF0npZ2+QuEeT/wM/P3iqb5NB6ZtInatRbSg25CUxZnbi7WBetp8FQbpaf
vZsp+8tDvupIwYodlIvFydvRAtaP3SnrcUJlm5SLMb4oXzXxknf128PHkJdC
05rHs/ZhyIvI2hhtTXCNsoQodN/+xk88GeXnh0PLzR8wPUBeCU/U1rR3PUP7
pwm2uF2iH4qRR4i4HZ07siuQF0MpQd+rVxuQ2cjHdRPlgZ2Mfglw4zST3TDl
hd+/H3YuARtmKedKQCXOch0uFmu6rWVh4IHI+r/slBe+LworrINGuBkm55UF
eDsEKNNWkcZXvj+qXYm8jIwcTDYvk0TrR0CN5e6egtWUi9mhcI5c6IM1lPX4
SVeuXxJJ6sgCZMbBx2TkBpRvkhioPOR4ehPKtxSqrdOe8jNG5iOPXZ297r4F
5ecli38Xq2y3Qfv7CVbrsM9GO5GZSMvczT6azsg0MpaHa4m8B3Ir0ehfc3eF
N8ovREp+iddb6ocsTnqp7vo5G4Q8DnKuiR8fOo72jxITIx2CrSGM+iDYlvn0
ywUU7wDn8g5Yv41EngMf+FQHn8UgFwOeQxMXMxLQfjZo9/WFXEIK6o8F3lI/
/fZiOmU3SbLjuoHbiSwUXwYVx1nnDuSi/dPA3/bTTZd8lP83yH92VdOaQPPm
Jef4bb/ql6D1zNDosLC/ejlaLw0vfWvilK1kzBdueXTr5fRXFJ8gOMOcvCq+
I7OQn51EBVNb0HoBGLW+6e2hLhRnhVs5bwWY/sLz4OncJb5yBHkQ1Lxa+Xlo
EnmAuH79x/GSWdTvcmi7P0k+nsmGincTgoa76rzZkMXIepGVoZCLspsgTBht
VOXlp6zHAx0+JrZ0rkBxUSiS5nilUNwG9U/+OCayMVIW5WsEt2wae12VkCeB
s0JivLoqcjkhtsjRaIkW8jTR0rBitBEgt4HU3O+3cwyQhwn3iJuW58yQmaGU
m8N/O6xQPTywQ2vFAwVbFB8E6dzf7eYckHOJPT0JLF9cKbeugHKv7fPS91BO
FYI98cJuR/ej9bMg82DDMosAygu/x7xNEl6JH0FxbqgoZu89dhJ5jhiYEBJ6
fw6Zk3z0ub40MQLtZ4UH790IPBiF4stIlVM7JQxikfngiK1QpUAimicTzFOu
P9F3G8VriUMsNxTIe8jVxPomu/roh2j9EjjxVDDM8wmK85L5l+vUtAuQK8AR
j/jWpSRaz0Fqb7SLailB8V7wh08QPC1nmHjZ/63vQiVaz0aeKIm74ViLvIgE
iTuM1zaieQrAuQCBsUWtKD4GijZ/S/3Whfs5Ixln9eAXshDU+2M7e3IEnTcK
Fn3hz7KeQvNaRZZk1u6UmWOcD43sbZ9+YttGmR2+X1LLdYif8sLfj4iW64SJ
CDIraV6w3UdEAq1fDJdeXS48JIvixaBi79d3b5Swr+hePxSnSnnh+8JKcLuk
txaKTxPcQ3xVACJPgOp3NSd5DCm78cOBmbSp3ZtRfI5gUzkU+HwrOp+LlNlj
OLjEDpkN6icu93J0QusbCJeqjvbs3ci1xHGWZ85/vdD6cRC/IbTBxg+ZE+Yd
tN2efhitHyUq78pUTp6grLcE/moYN9t8DsXHCTaud2+TIlC9PFDGME53KArF
pwi9o3te6MWh/ZzQ6ZHG+utJeP/R9sWPu+4gzxBxQnUK2pmoHmaYZ5GRfinn
/9VzNlj85zPkbqI/3yRx3SvkMYJ1QFDg3Bvk30BKsudq7Xvc7ya7Ao7VlcjT
wOlyeNixWuRJcLR4J62iEb+H2InVJ8TaUL5+kKs4PeHfg7wIVriW+78dROv/
gL7YhF8C4yg+DFg/eu31mkHxpaTUX+22l7Tt1DyYoO56dqdlSyiHDANH7+91
rssoL/xeCE55YJO3HK1fDmO+HqtgEUHrF5M5bOamOyXQ+mrwCYqUPJBD8WnQ
G9gPZpWRWSBL5ssCK3W0vp2Q+HlJ7c4GFF/4/PHtejS2CZ9vb6okb2KC3A0O
n/wvLcECeYCIefJp1a9tyH9BTndSAnRA+fjIjysPLI92RfE+0G0Notr3oDgH
yXSBk13jAIqPAfFXTefDA1G/SyEYzp7/fpSRn7CXPXVM+QzyIAhytBw/HYby
MZPRV1f5fbmM4iNEdulgn3QM8ijx4Q/pGZyA491ro1rKU5BbCSZPF8eV91A+
dlLs5tpvvg9RvAboVM5vLX6C/IewY676yFeIPAwOad823lPEyAeiff2KC0qR
y0F22qaNHJ8Y8wXl9dz5Tl/QeXOgk7NV5XE98hi4ZHLHJe4nnrdqyO7IEx0o
zgMbXki/dO9DZoWnxzp7TH8zTMqsyRBYO8G4P+LT3n2G/P/h8wNT5QNmaLaU
h4BwY19KKysyE1m0/GFFGSfyALHH8sBMNh9yB+AMXyN/XRi5k8grHtpxTAx5
DjjMPD7vKoPz09YHPDFWROYiM3zVWpRUkAeB5f0xTj5NZA5yvPWZzvRGZBqZ
KBLs1axPeeE969tqxZeaojgr2Xtl+m2WJXITEfX+xUj0drSeCWosOiF+xIHR
D2jSAZbOrihOI88FzR033IPi7YR8TlGmwn7kBqKq50wddwDyDAiW1GeZDEb7
F5Giu5jUmk4iz4OS2LeuJefQ+h7gXRl6JTMCxScBD5vJq6goPL98/SV9QbGM
ekmnE+WCuxJRvAswP79opJ+K4sxk1pB54OoMvN9anjN1WTbyMDHp/vnz2BNc
b3JS1H/fC5BrCaNvWxWKSZRvDvRz8e7MeIvPizarCY38gOLcUOvc9bzAKuS/
oPmVbav9N3zfoRMCXJt+IBcCxXX1G2XbkLuJL14J3kt7cH1H0xxujAygfLNA
rEnkXf0o475ppQJNo+Q08hTYvzVZIn0eeTHJd9HF6hLLDmr/YrKwRPykP8cO
Rn6X2dYHdjwo/gcs1kyrB4IoPkNk+3kslhZFTgXbHsios0uh9azkdHuX2+/V
KN5E3Ba9H/VtDXIvYWLnRbxSR64mBq4q9N/ZgDxEXP/QLxSxCTmX0GHONj5o
jPIzk63A95DtFlxvePDaOzo2yDRaxDLards70fpF8FL6l3gWF2QajNx495q3
J1rfSkTVBEVW+iAPgGhvk3D1AORJIoYmfC7hCHInEXuj7+TcKeQGIm7tqyO7
Q5EHQfy7yMD3l5CniAQnF1/la7ifxLF1Xtdu4PNvXVrkMZmM96dIfnXelY7c
CFIL0+2Ls5D7ibStwdtln+D+73abWl0qwE4/tWLzbxL5N8jg/2VoW4r8l8h8
SOi++IjzZRlEbRD7wugPZH93XX++Hs1rDOT4q67r/YniY0TuEmZFy07kcuJJ
Sq1MXj+eV55GhrjQCJ7Ps4ojIien8HvI99gs0DaHXAgKZ0R4TFjsGPW/vDbA
8ZADmQYJ+aLFPLzIo0TR66u0w0LIncRrO/f/vq9C7iWKB9UmdWWQh4iSUJaR
u4rII0TpyrpfbKrI7URZ3v1uXy3khb8vm4+11UCc72OreZOWEXIhqDgiWn/L
HLkLfOYa+rLIBnmcqLz3umLvTuRpohpce//JGZkJ1nzdXaLiiTwAan3Wk3E+
uL+6RayFM/6UQyZAQ0J9nusRFO8HjesePCo9xZgP7UfZ8UyFULR+HDQ5W9yN
uoTiDaB5fFXKWDTDROvl3wn2N/D6dqk318lk5L+g80VMlFQ6Wp+78PvD82J4
Fj6vt0cjdCAXu+/0kjM2BTh/v8D3Y/kk8hgYyM4KWlmK3AaGDE/6hXzE/Qw3
Wvp0VeN5jgaI7zGvR/VMgnG2EdfHP/F9TN4uceTvRB4EU5qxO471o/VjIMjY
3b14GHkUDG9f67tkinEecWD3f0et5pC7iV7/8tA45p3U+mHQdmX3LWkeygt/
fxuzZp8+EUUeAHYvPryelkIeI2rex3/apIDcSVjVedRfWIdcTnzqVOn4rIFt
NjY3xA+Qa0Dpok8zuwyQZ4EeTwLrXTPkaoIQ28PXb4XqmwPaa9TEVHfg855t
/KtwdBder2JeofHaHbmXeGR/U5/VC7mJUNy319LyIHIzyDis7hAbhNxKSIXS
9vw4jvtNifnsL3UWuQ6I3Ek86R2OPEnceLwvIvcKcingL1ofO3UduRtEVyxK
1U3E9XH+qHwYlopcTET0JRVUZCBPESzTXm+XP8L5zrJqVjk+Ra4l5vmZf9x5
gfcfl67u7n2N3E5MqiaPritD7gGBej7zwRWM/sCQlRZHUQ1yI9jvzCK4+Dty
Kujd/0XSogX363k8Zc31LjT/EdAasX9D4y9cj9MNbWPJUXy/DfcW23hNM+YN
djyrcXo8T7mYGdaU3PaaZLGn4hXA6suBILgUuZX42LIhJJSX8sJ7NBlijfwk
hOLdRMns1xt8Yig+D3SX3rnrIIPiI8TLFQcfpyoiDxNa8htf9aig9XPgmSbb
+7VaKE6jqRh/qzkMkXNB9va0ZsIQuQfI7/brZzZHriXS/cGkuTVyI5A8w84U
Y4c8RaRcqVv23Qm5EIjcurtCwgO5DsRn+cvu80YuB3wvoGqOHyM/iHrPAScO
M+ohltbVm4GTyE0EX1/cEqFzyL1AeHZ72Ug4Ix8hzs0XVnEFr5eTqja8fx3n
V9aIYjp3E7kfqJtZvHG6jevT2cURonUPuZPQO1iuy/cQuZ0wOXthbiAXeYyw
jDUi3uej+Y4C2/tMJ9IIFG8Gji+LN5wqwfW5fT49vbMc97evFRSoVTLqIQ6O
zRxeVss4HwSxvljf+53RL3F8xZGxkhac/6yyRl5yF3IpiNg05n/0F+M9gaht
T9ZtH0HuArF7/IbWTCFXg6Sjax6xzWGnXf61v4PJgXIjyEx5oFjE5sDYn/Nk
X18CF3Ir8bxUNvMQP/IEQdR37LUSQa4mSvrvyCpIII8Q5XOuncxyyP1EFY/Y
3WYl5IUbkG5yf6GK3EA0aSZKxGohlxPtm+1bDkLkWtDnJJiy2RC5Awz71TrJ
bEYeICbPxaz8a4XXz8ZZN363Ra4AzA+4bj5zRM4FHETFzqtujPMAT9UlQZ+9
yFNAsN3sm9EBnG/VBGuseCByKZBhe7dt5ggjH6G48jzvt1PYqmv1qx+fR04F
2vp/oy5dxHFdW9Jyz1Vs430nOPXikJuBxfENn0SSkIvBtitTFydS8XwcUp+b
VWcg9wG3p4eWPMxm3BfYW6ZaFpaH8/l+/x3qVojnFzTwyHBjEb7/43/3MwmW
IncTIXyKb4Y/4HmFy/ae+VSFPEREaWfoZnxDngGxWzznQn7g/YkuUsSuNny/
dwJaj2v2IA+CzNCUDbyDjPkSOTecpn+NMu5z4d9/SqHGfxj9E4FH/3Df/ovc
TtT2vk+aXuzImI+GQ/zqbZzIjSD+g+fTh3zIQ8T0BvVNi1c4MvY7Zi365CLO
iANCpNquUBbnE7uc0s6rjPeH/Hfg4H415C7Qvn/jTKk2Ps+wif2C2CbkMSLd
ooH3qDHjPMBKZiR/2YI8AbzWHFZQ2obcBD4mGz4PtUfuBMpcfPrNLsjVIOp0
a4XWHuRWMDyUY39tP3IFsHE91dkfQHnh91Re1RZ/o6OM/QS/nshs8mnkPhCc
2xs+FYqcChokCpbbXEZuIHSuhd3Ouobz31pkq8SSgNwP5gOkCpxTcH2u7cMG
BenI5UTxtteVPA+RO4DU2yuOPk/w/lB1p+63BcgLL+auYuCqIuRcwoz/z1xw
KWMeRFbo+4vVH/F5nBNxAopfkEuB7x7PO+fr8fwqv6mt+fkT16NisuiFZiee
X0x+lVF0P57PuFxKdd8w4z4IuxsHnAynkBf+/bJkY++tOTTfYSBylD1oknkX
Y/+J3vq/Wzl2MfLrfggSYhZCbgdMWbzr8qWRO0HZpRwTbxXkbnBx/xYXUYjc
B/p/rOg/bMjIDywseg9XbUauADlE/iIFa3w+z5qwK+fskHOJwOTtK5qckMtB
7TKpexoeDBOap4dVrnrj/TeGioheP+QaMO1yxcwgmFEv4Vi1qzbpJPIwIDYp
uk2cw/2J5U7/srqIXExwyBYqgqs4/+TNI94KcTjezqWVKZiE66k8P9nNfAfP
4+X0c9mRDDzPDN/Dns3ZyKNETPv6u5/ykBuI0zvH2woL8bx8Kp5KZBThedjp
H3K9XornZ5CvlhLyEXkArFUabfKtxvMXSX2yclcdcg9gFQhwNGvC/Y5eVLmp
0Y7n0zz/u16qF+f/eOixIM8Q7j+/9+COuTHKC78f0pzXxvb/wfujagZr6v/i
eRw3fcT7brET5VqwlzhgnbfUiRHfpqp89TYv8sLfk4xfnyOFkHuA4sqHnMdX
ITcRgtE+W/ZJI7cCpsWKl2wVGPnA0LG+cv11yL2gcShzyToN5IV/P3t4mYhu
RK4m8hpWh7HrI/eDFMuet5MmlBc+H5dKMpg6LVC8gQjW2qv/ZRvDYHe2bEiR
PXIxsJLsKnrogs/TiU+fS/BE7gJySz3BBR+cjy9E+sQhf8Z8iPnx9hduwTh/
v3fatOVJ5FRQ1+yutfEcchso2S4ZLB+BvPB5Km99JhCFPEokwtQxplg8nwt5
rmrDN3G9gavFA37exvW43Gp+/PEezmfOmzJU8BDPS/OC85p7T5AbgdR/ogdi
CvB5XP5NWWdIfJ8znUl9B94il4Juh13yjh8Y8wE1lSL7TKvwfIoMG++t/4Zc
CLIKb3ZK/kDuJOLXOEhzt+F5nEsT3j3bjes5KNSQ2jeAXAccI2+01I3i/SaL
doqVTuP+1IIFnZ/MI9Noq359S0phcUb9Ak/y3n2Opci1IPvq4afBvMjlYMzd
+HW7EMOEznqBT1ZiyG0L/x7sqnspg1xMlDc8a5dTQm4G3A9Dh2JUcX67U7Yz
81p4ffJWGdb9usgLHUiO89YbIbcTyuNvVxluwfFDZdcVHtsg54KXCR4aK+1x
Pqb96vrhLrj+zZDZcswTuQZEc3+1d93PWA/q29I8PwXg/GLPAv21jjLOB3sv
GJy8exq5deHf73wR3GHIDWBcsf36ict4nmDuye2ea4x+ifNVZx9uT8Dnf7xj
U/A6BXmE4A2SfKt0D7kO2JuMVN54yDgPpAq/aWTOQ04FPf3R3X6FeJ5rSbfR
H0X4/OCrKvOm7yiHTADSncbx7BPyOGBZXy0gUYPnu4U1VTKyAXmAiGnwWzPd
jM9vzNq0wbMLny95itu4+heev9fWFmswilwBciUfO2VOIzeCqbHTXvx/cVy3
zCooZLEL5XIiLEEsZGApdoXP0GV7PuRasBwW3SgVdmHkc+SOuqsijjxM3Glz
fnxLFrmJ6H265hWbMnI3oXJhrixIDbkPHLH/XNOqjfMVKSY3W2xCriZY5w70
FxojFxOWVWBSxgI5l4i9w8l0bRtyA/hxqGnZnD1yG5AyyV7h7YrcA7yFT8p+
28PoD+T2b1HVP4D7nSJWwkeByENA9+ovsxXHkCvABfdXtmFnkGm0z+qX3UbC
GPUCftZdB5wjcb9ODYpHP8Tgfu5mzZzXuMmYJ9F/8uPVO7dxPLssLvv3PUZ/
4CCP+weYzeiPUHFU7r6ch/sfuTvF1FiIXAryBkvE5V8jtxNBWlEg+B1yJ6F5
1sGh9BNjnmD6o0wwXw2+35f8wzFuDfg+Trq8epzTjPvVzbxQMduJ7/fviE2f
+S98n8UbV7HeHEFuBefCeqV6ppALgVHV000a88i9BOuKM07nWVwZ55fvNj/2
hQO5mLiULRAvzottMdma5yuEXE4s08uuerUKmUarvHhkgF0GeZSI/mrAbq/I
yE9sW8Ull6GCXAr49303GNdEziXqctNdDSByE5Ew43cy2hC5EDgabbzZvBm5
FayMYs1XtkauAU31X2qO2+HzUiSTf5c7IfcAt/1enEIeyNVA6rm6wh5vxnmg
c37e+KkfPj/D7OPuRcE47hUTd2brSeROoNDkdiv5HHI/6JdVfvErAu/P9pv6
tuEq7vfgi5LR8Djkhc8jcxR3XRKe76iFg7JMGj7vWbzM5sBMHA9u/b2nOAdb
S/HVOa7nyHVg+tCF206vcP6XpA2R9QavP7lk1ffp93h+uja9EyaVuH5a0lO+
uFp8nyWdp9d1NOJ+QteaW6i24XzGRwW8z/TgellLWsM+DzLioHxpdtrKceQh
cGnHkdfeM/g+M7ZKDu2iuVHOJcLHL8yeY0YuJ7xuDnBksbox8m3W3bbiCzty
J1DsKFg9zYlcSyyNWKUpzsNYTwwonzcyWY7cRFR86d3mK4j3Pwq2co9dgdd/
TVbeHCaK3Aj+lHKoBovj/eIDvcL7pJBLgfHy9zR7Wez9Ovd6zeSxr7mfr96g
hOsriHAvVFyL3E38fLwpdaUqcgVgrl8Vwbke968w/5/fnCZyD9gq27hzaAMy
jXbYonBTC0CuAUmH4ldXb8L9vEkM4n5jgOfX82bb1BNjvH9Zn0pLmhm2Og/3
++tbcD0OWoM5oVbI7eCMy6f4wzb4vHthD07vtcXz+ZQdvnfnTtzvyNc9VmaO
uB6h/ww1Nzjj/FBKSkzRjTEP4LGZxrrSA9d70b95cOle5Drw+AbxbdYLORV8
K0okB/fj8//rOnqv+SDjfCC5bOeVqgDG+wKm6zUOFwchVxO+u5Y7PzmC118/
N2KUdpxyyBx48aBK+fopxnshWqof8YeG4HoXT1+eDTqP56Mk7tO55wKu38bE
rMLuIp7HEV+5Z6aROJ4cy3JL+ypyIXj7qv28Qgyup6+9eL9IHH4P3By3ty9N
wPs1VE9tnE3E8V32u6QHk7HPntmwtDkVeZi4nyE0VnkX9//580Tj6wx8/hxr
zwrTIvx+1+g12Fd+Y+QDtHjd+/MNeH/tr/SJtU34vEz9pUauLfh+Tt4IiLna
juu1Hqxvfd2F80kb6q4b7sX3O5mQfkpiALmB+DjEUWH9m3EeSDEKEDk7ij8P
AYn1Xk8mcH6jYVjQNo3fl7BJ+mK+WVzfQBKHrcFf/H3zesQ/LZDJnfIvEGNa
P5y2GLkD7E2Gm76yITcROmN3rzBzujP2L9vM0aTOjdwOWlP8FT35kGvAs/G6
o7ECyOVEhDl8XyqM3AycUu8KTKzE61Um2T1lxZHbALOFf94OKeRiUHenjnZB
FnkAZE2BrfnyuL7TlneTu5Vwfdvusg8IrkOuJeT++OmYqiH3gj9WdRFHNJA7
QUU6qL+vjVxNpM6kyTZsxPUHWbMHsW3CNs3wK9E2QK4DIrPfeLyNGfUSQzbA
9aYZnmfJ/bRHH7YgD4L4ObbZP1a4Xp/tfuaK25AXvh8efEtw3MGoH/D83dhz
yR65EHTapmm82oXcAAqz2EJ/uTDqA5E0v5qVu3E/bnbfJCz24PPUszf6nfTC
ZmVKI7P34/WNO9k4fx5E7idyHh10XBaI+z3L/C0THsbrbR02TvkeRU4F8o/v
GKecwPOYZWGLrTyN3E1UOR5snz+LPATScmtV1oXh9cGsG8+4RiA3AnOnO5+v
XsbzW5W3RLQ4Cvc/vOSgz/A15Fai1Lm2UCIO15PwVGeJTQLu9wD7nR1nkxgG
eq5L0p+kMPIRy5/7jrbdwe9H+YqFSFM6rs9oj5JB3X283hly+FRn4fcVLNB3
7eMj/F6iBt+/KM3F599/l9FW9JTx+SGKk8PYX+Tj99xw2FP16QvkUjBiaejw
iMCfFw45qbP3X+N+peZpD+6U4Pwb61qqk95h2+YUTceV43kcuJAsEf2JcR4I
czlpdqkS50vR3OUf+gXfbwGXTsLpWuSF/9MtXHy0Hr/H3qKpnsBG/D4W3ajj
9v2JP18ifs+19rXi/Gqmsa7uHXg+W8QPhe/qxvP1nLJ5vKMPz/9UlUr91gFc
b/x97r+bf+P8OWeG5IxGcb3vd3620p3A82tdlx2sPY3nO73kcoraf/jzxtvq
XaY8j/crFpoNyS3aTbkRGEavFpRkQa4BTl6suiuXUA75A4L0uvYIcKB4O7gi
XHqFexlyLpExnPacnQe5FhSVn/3JvBy5GtSnui2eF0DuJYaPblozLYzj7DZi
O0ZXMkxIKcydHBBDbgY6i5rSuyWRy8H27y8rWmWQm4gDT26ON65mGIRePCr6
TRG5DyS77zSqWoPz5W/QPPBBBZ9XxSsQ+1adkZ/o7Rt7RWriOK2kpqNgA+5/
ReKTpXkAn68WGK2evQn3b27utyvDANfrIWV1PtUY5zs5o/ww0QyfF1uz9Gvs
FjzPR1n9M1FWyDRa2bkPUhdtkLuJZsdM8/O2eP2UWnjgqZ3IQ4Bn6d7EI47I
HUC+w6gkwBmv138l3b/fDTkVCG0NEdnpgdxADLY3mRvsRa4Bb4M3nFjjzdgP
bnLEPxQ+gPv1Sxn9weyH+zVW28r5OwC5EKwsewgagxjriREHNt93R3B/7wc9
k3OPIzeD5LNvPiedQm4ChwTE5i+EIFeAzQ+Orw08j+sXh/UuzheQi8FEtfpV
s4sME588o1+rR2LfmR74LXYVz+NI5GYJjhjkRmApkWE9EYv7k37GdLb1Bj7v
j6nrk0+JyJ2g6sertvxkXN89P2G+tFTkanCC+bDBlbs4n82NL4FHMyiHjIDV
SmvvejxgzI+YK7r01Sobz+vrth5mncfIbeBBt+F62Txc/5njqZ48z/G8dnDN
xf5XgPtVSnN41/0SmUZbpJk/8YVErgP1H/jkyGJGvcQjZz+7zLfI3eD8yKcL
18twPw5h8gWnP+B+160I6/GuQC4Fix+1Ce2oQu4FP/R0zfRqGPMintQmHlX6
htwDwr2mMgUbGOsJ59nt3xf9wPWpR+eyD/7E/bPLLNNpaMXzainw9nnbget5
vqUsMacbuRBcbpH6dLOP0Q/hfujMf6EDjHkRWkualPx/M+YFliVpO+0aRW4H
HWvjIk0m8PoXJSOE6jQ+/6qd1aDof8i5xJ7+rFVs88i1xMbTS6zGaB6Mfnj5
PE83MyMPg557xTkfWJFLAblhVcszduRO4vrnY9ypnMjFhLd73abL3MipYNOE
mn8wH3I1IXDxaqq7APIv8Et0oNpCGDmXeJNrtkh7JXIDYXRoTcJuMeR+UK7B
t+6KJD7PYnryXYEMciGofvnDqX01chuo33TvktZa5HbQXHqwMHI9cjPYHb59
a4EW4zzQtVm7u00H1+PFueoUpy5yDRioXMSvpY/z+V/rznI3wvMb2/5JP9KU
0S8IFsxtyDfH85hpiPVrs0Re+P2cdIyV0wZ54f27uCRr2mKHShiud9/JqAew
daz+dNkRuQJE3uPcne+M1/N4jUy3ujHqI2IV664u9URuBUKDL+U09+H1iY9v
k24+uF+xwFDby764n7T13r+e++P5yE1Znms9hM/PeqG2YukR7DUnhXI1jiMP
glzdWRO3U8jlYP2itp+XQvD9Fb59F/T8PHIt2Hgha2nrBby+yOxqGsclPC+D
pUEbNK4g94Cyz/bVrtG4H/NouO/SdUY+onKb1PyzeEY+wkZgSVzLTZy/tv6X
Ekcyfm/2idUl61MZ9YEmp+cOrndxvW7iicMXMxjzJDrbToc/e4Dve1+6h1hL
Nq6nf6/Zc/ZcnP+gwhqL9U/x52f0F2+HSz7efzhn8tjFF/i8af8fPM8IXO9J
9eL7za/xe6JNpuuyv8X9nS+8+E29DPfPeuLgAZcPuJ5LcDvzxQr8/rlo2olP
q3C+ayWiqs01+D3why0qZ6vD7yfBtNtF/Tt+D6Icnyacm/D5qRWPIyNa8PuR
uRor/bQduQPctzn28mcXfi/+8XWKNb14Pto/1JPKfuHP8yKJa0tfDeHP30fP
oROPR/D9xDzYMnB3HPe3ayjTKWEKf9/IqLN+jpzB6weOeMCzc7je50Txo8M0
T8b5pxeJifkwezL2m5iciHJhRW4nuC83zG9jR64ADVUafqac2Kn811s2cnsy
8ns7DG9V4UOuA2oplsUyAsht4L/2LJUVwsiloHQ1251lK/H6yAN7eJnEkFuJ
HU9Kzk5KIC98XifFR/ulGQbdOqd2t8gh/wKPzzTWfFXA8aOlWoblysj9hD57
3FNiHfIAwWE1Kv1EjdEvqInZGntPA/efVJ/NkqiN3ER4inIcjtrIMFB239d1
ThfPY+Je6Y4j+sjNoKhfsmy/EXIvCF93RtPNFPdrHdSUYWuO+xN+sUFosyXj
fkDbXHw4tMbOMhifUt2O5xMYbuMlZ4e88PetIqdBxAG5GLDwcm7mdsL383mH
9wtmV3x+fGKZwrQ73u/SIp044Infw2qZsxxt+xj5iGGv5uPffJAXXuyjjb8+
+DLWg7OjCbuK/PH8zbUmP+UdwvmWn9wO7gcjdxNNxbnZScdwf+mLuVZFn8T1
+ZrvvxJ6hnF/QPNq+dzRczjf/FfZg75heP974fPN7hH4/GjnViu7y7h++zT4
2jwKW7Incd2ma5RDhkG/0vRt9Vgcz/PfwSN/gzE/cOJ5XohoIr5/oxnuEZ5k
5EbAucnXfXEqvp9v5z9++ZOG34/F1OPMNRl4f4lP3Bn3B/jzod183C4uG7/H
HBu3NR8eI6cCmXfGLHN5+D6TtJV+qOTjevmyefI8X+D3HiE+GZFAIHeB+Zgf
rhWvUb+TIIj1jSbtLc7Xfyxj2foy/B7dBy937vuA30eDW8CrpAoct6q1i6mq
wvMpNQXezF/x+9N5JamnVYfvK3ftEqH933F8ddrAYEoTciFIEagprWlhzA/w
XyxIYu3A7+HS7K1AnW4cp/mf23ywj1EfGLSznPr2G9vzo1ol+xiedyMUvgcn
cT/WT+ZOBPxB7gBlMh3b7s3iekBCucL3v3i+T5fm0JYx72H0r3jmer0eK/LC
34PRozlB7MidQHCvS1gmJ3IDEfnd0KmJmxEnmCwV1HmW4/ixYi4OI0HkamJY
fbz1yArkYmLv/e8FD0UZcdAk8jqqRRy5idgWlb5nuTRyMyhfdAmYyiEPE5sO
+y0/oYCd32vbn6OM+1F20nnTvg65EKRViScIqiN3AWHDxX7mmsipICq/3/j0
BuR2YrFitWgeQK4APu6rL//2w/WnRF/y4T+E9395Pbh5QzDjfMDy21rB5Rgy
jaYt9ozt/Elc3wFLod77Z5BridSTx99XnMPn1z78mTEShu9jyQ+9C4IXkTuA
Dkf6no2RyAPg4IYlxm5XGftBmpePTFgMnn/djc/MWXHYHO9VOioT8Plw8nrJ
WBLu11926o7wbeRuIt3W8SxMw/ejX3nopOcrfP/NpleOXK7Fcb4jw3a59fg9
GGds1/zWiNwHjn7LF5j5ie8/m0VkQqwN99eqfqrWsBO5DvB7tD716mHkB2Yx
htev9ON5n3iTEZg3iPwb5Ayzb6sfxvNsF/dVnR3D8xTcWs0jOcXoD5ifVh82
nsH3e/pRfJXPHPaTpj85V2l7KQ8TnUudo54x72XkF95Y7PudFbkCWPhIW86z
IxeCMzcvKEsvQ+4GeeV9S814kBuI7imLXweWI1cTIqtzP14TRM4FlnbLs/JX
IDcRIWHBF3+IIpeDZ8++e9EkGOuJ3g5gJiuN61m5PHW1uRxyI7AyYF7ip8DY
T5wL2Nt9XRm5lshP/fCucB3jPNBfpXzvpxpyMRD7ezWUSRPns1k75rF6Az7/
Y0ulqCDA5xtcy/rGsgmf98rgQtSYPu53/bi7absR3p99D9K+mDLOI2R3rnjx
2hzXl8I2EZBjiZwKBF9WKyZbM+ZLXN2f3XF5O3IrwbYq4tZxO+QaEFLpscPb
AZ//58wmLnsnfB+Bqivfm7gi9xP97ZNnNHYj02gesTXaMntwvibjnBE+L0Y+
sGPqYtai/diVmXs8hn3xfhNHfdEWf8Z54PXSVd8+H0L+DbTJ6StEMJ537sFa
k4fHkLuAgkTu35snkX+BtC+XCyPOINeBlef3BRw5x3ifIHa9oeLeMPz+OLvF
Omwj8LzCbswkGV7G9c2b1dmqReF5B888WSZ5DZ//++GVMu5Y3L+Xs/eZ+Xh8
H21cxtqDN3HcsVhi5MctPO+agNkHH2/j+rZIN+x+kYbPK619ujLzHu4PXLha
G5+J632utf9K2EPKC7931vaZmATl4PPvJ0r93f0EW8JivsDmGSM/SJj77q9X
gM/nffxcYd1LHL/kdq19FYnrZeLzTeIsxp+3E2/NbP8rwfWMB8ks63+HPAh8
5WhlDeX489Fd/+P0+0/4PbtcLNDKr8Tr63WuD6d/wZ8P64GDD67X4vXlyea7
z9Xj8/W3yq0MaERuAy9pTLWuP/H3hVrez0irVnyfDz1eGMMO5GYgIxA3r9SN
39etMv8CkT6cX+CohT/7AHIHiFKQV5gewt8/rD+Y27tH8Ps+E9mS+G0c5884
YPiSeRp5DFRY3P+u+h9eP6q89I/rPP68CS/zE45atI9yKdAdrNEiWJCriT2f
NXf2L0FuApGPEoOFl+J43pX5OBMu5IWMvrufB/EilxPzlmW1afx4vcxaxfFq
IeRaYgtX1PK/Ish1IHBoRG2NGPIASKjcsW2XJHIuUZTzIuCiDHID0Rm16lrB
amwOv7O5XYr4PNWtXVXL1yL/BvbrNv/WV8X9nuZ+xOW/Hteb/ptnbYoWru9j
VZBlhQ4jDoYfNxyYgcj9QCgaRMrr4/no+qc+tDNCLgSe1iyfQk1xP5dUvPrz
zJErQC5PBXubJWM/UTe8ToHbBtczV33dDNriemSeTO3bvxP3a35tV/hNR9yv
f8DrjPfOyMVEvI102YQb7pdQDe+S9sTxDt5fLNv2MfYDjlErmRAf5GGgUpNn
mOPLOA/Y5Ql6NPnj+zgZc/wcRxByJ0gLbL6jfQT3+2GbwZu9x/H7GFbLaI09
hdwIBJdz0N6G4HmBMV/xkfPIzWD31y+64uF4HhFPNVwsL2E/vn7z1IkreD51
h+ZuPYjG8539v6bLNB7Lr4njCFkKISklWUooEaUckogQKUmUSkSyhZJElC1R
ElKo275LkdAha9YkJCHJvmXfkur5v+hc87z8fs65Zn7zm5lzc+wc/vwQ4gnL
VbQzPSLcjzV5t/7a+QT6azcTuM4sGjiseWJPMA3y4RyDk0VxhLtwd2jetdFE
6AfLlfUR61JBz/bjnq81M+B7A/nelqtZ1PfIbbXmXHw24f/+fpxNW92US+lD
VZ845ekL4PuxV04G0oUwL7zhn51OFxOmIc+FbJvjZdDfEeNgi8PvwH/DQhtT
9WqYl9KNh04o1UH/H/fSH9rWCP1xSCnYu6GV8H+/t+yPdq5uh+817JykVnZC
v1826IkxfYd5ENwpJfi7B/TdCWNZM9sP+mbmezl/DIFfZ41LWPpG4T2oxdH0
X8dh33ZtvL7YPAXfx3oZTtfNUt+jlb2yo+UL0I9rBzn78C/wrzd55GvOH5gP
PfaqlnR6K+I3LrCN/xDPSDgPbW7wrIpaTrgYh8ieLgllI9yHfofuKQhcSXgI
Wc2vzvbmgnjNJ6fSbvAQ7sIquD7emY9wM0oTTIu2WUu4HPF5+YWbryfci271
nL9/aiN1H4+pq/gbCBPuQCeT13vpiBH+LwLbT1c1cdC/w/aTI5Ik3IKiPry4
JLedcANaLnvPXEqGMA05hlqfFpUj3Io75w4art9N5cNaJ0X0ePcSzkKv3vzV
WKEE+oUEO1QYVQh/R4GeeXuWVAm3ofnuUNkZdajPTP2y5Kgm+FufdFi0V5s6
x3vYJDZ06ILeeBtmvmZ9qJfrQzdHnQF87ybzdnn5CcKDqP9hJB02JvwDHZ1z
+Zl9GvwrNDKYSjsL/RF/s2Mk7jzED92wsjfyAvSTznOo4+FFqOdSd8WnuzaQ
v0Uttv62PfihmuRR6eZI6cGZrCbFTleofGitze78S9fge+96npfn3YAndkyk
mnhA/9fqaaWreVH+Y1Xb+Ixt3oQnkfXdP5l8flD/wxSjrL93oJ+48uWLwUDC
o6i3b0X2x/sQfyWjZU5BCOFOtEu45FVcGOEqfEZF4HVgBNUP7G96Je9KJOj9
8mTrG40Y4Bs8IcUj6fB9gsxoSfNz+L5e72BZ4UuoZ86WVp74Cvq/MXCx4n4e
+KmZalB57Q3od6jKrDpXBPke97PUaJVQ+VAp4/naneWwb8PChXXrK2F+efav
qWeqgX6gM5c/jNVB/83daxs+fwA9QZFijcWN4Gdu/s2mlE9QT+fnL80hrYS7
0fK5nS1u7bB/O3jvfTbvhHkzkh1sPfwd5tHriGrbrl7CdSjVLqp94wD40xg4
18Ey/I89p9Cv1COdk6Pgj2h16re2cdCvM8D4vWwK+ArTme70WajnqUh+T9gC
+PduP0+fxy+4P37Gtt/yD+Tn96gcOEJ/8R8PIJWoTUN7GAl3oIsFbsPCywk3
o5DWTyPsbIR70Zs56R8zKwgX417egLGvnITp6Fbs7B1/x024EcnrK08+X019
j03tI6Yi+AnTkG/Q1LSXAOR/nqYzay1IeAK1VifOHdtEuArTD9ItIFHCQ0iC
2eSn2BbCrfio6KtFDgnI56bKuTQvRbgFxZ+9+LtLmsqH6zzK/lTLEm5As1Eb
6LLloV7BNy70UQqEu/HMcuOL5YpQb40B+jiqDPpoMYJ7VqtCPS5jdDFK6nCu
q9jDckGTcBcW9a9wuKcN+hebk1pzdeH7hk0BKt/0CdehRDub5OXH/7HnNHJ/
o8u1w4icZyEDFplrRibgv8Rxni5PU8hPFzurkXIO4rWMfX7+0ZzqJ0pXLFiz
aAn9ve0fdVP4EvTL+JPHgJYdzM8O4XN6TpcpfxCz/YHXkc6UHtzxRmxjuQvE
e8nC4jd6Heq7c3x4jNcD/DwbW2eo5AV6d41nFll4E85DK9CDzff8CP9A3f5O
93IDqP7hvE/H5zqDIN59YQXT5Q8g/wX7de+kQ0EfwkvbjB5BP7hZv4V5PgF/
Bo+X/E6OhvhFsXEWH2mER1DYuM/7n3FwboOs5IWToD7VO1rRWqmEhzF/ixST
UwbkHxPmtI3Mgvvl9pPNZdlU/SgSN6HRXOiPI2tuPG8B+KNpGLFCqZDwIBaM
u+5sUQzxZ8ZPdQSVwbzUoH1que+gXzF3NqV3VoO+ay3LeJe/J9yPdUX63aQb
IJ6oQ1XPiSbC5WgRp2p7tsB70cAalJ38BfqVZGgv8LGD8Az2iNO//fMb7JvB
xM6RTT1Qn4QS3zGtfugfXcBCgeMQVR9qaWkTjhyF8wyRwoCycfDL2+HZ1MgU
9NO40MuYdw783cFmXop+Qj3MJw5KWCzB9x1x4iFBfwm3oewJtsVXDNbU/fq3
ForJTISb8fC94htPWAj3YiZTgaJAdsJ0dELbrv714CDch9BSg8rlVYSr8Ila
yVvneSlGjk98y46vITyB7138zqi5jnArSlVAB/duINyFK5Y/8pMSgu+7Wiar
BEUg/lKCDtuqzYTLEf+VJO1lWwl34J1qDEGzkoSLsS7P6fqB7fC9dfdrzjYZ
ON/UbC725ywwint7YeI83DdyXJfcfQH8cdp/Zaj5IuE6dI+rQaLSBu6nfpOw
ybcnPIgrMn0y0hwJ56Eu966x6CsQb0lHcUfwNfCXf3345VtuEG/nyMRLZw+4
r1ugPXPBi6oXWd9JlD/pTfUL+RrRu2j7QT0xW07lKQUQbkF4LvendBDEa61Y
pSgcTDGaCbW5wfsQvuc0ryxkDic8hiR2Cv9diCDcgA8yuKuMREI/zT5+9vr6
FNidJlv2IYZwP46wD2IsjSfcjXOUB9VzkqDfDSsP+CWmwvcjHdFVERlUfsyc
vsB6N4swDQm7HdN2z4Z4SlqZgfa51Hwjo7Ws9efy4dx58DynAQb/7r8uOnLw
LZUPG72KWXApJTyKhbO9aSkVhKfQSJalZnsVnOdkak2sqAM/3dO3RSh/IDyA
DqZyqTg0wr5xJk8PxHwC/1oTWu43tRL+gWLi8nczdQBbx0R92/Xt/+b72U0/
q26qHrQUZSb9pA/2seKJ+ufaQfDnXoT4zd8j4N+JcPYt0uMwD0KhY/Vnp0DP
0IOPV0NmoZ6X93MEyxeo+rFb0KN3s7/AT7W71+22/IX+rrxzmu8kw6V/3IVb
fFWKApgIZ6Fn3iIXMAvhCWx1i5ljjJ0wHZ2M59CrjZzUfbzoXndan5twLy5z
e850ezXhOhToGpKRww/3j7tcOd4vQPg7Erxi9HvNRsLNaMBRMeGQMOFulOUg
eNhNjPAgcrWjn00Xp+5jVZveqE5Jwq2Y3bpSjUsa8jVbpo7ulyVMQ9EWQaFO
8oSH0YXzDihBAb6XPnest0WR8BxeMN0VyLKPcBUqObVWbq8q4RYUYLzUfkkd
/Dtm9O12tCbhfrzesFTygzbhedR3LKGJTo/yH2Xq+7vJHiVcjK/pXRIxPw71
7j+sWxtmRLgDs2nLOFWaQD+aNXkFfppS+lH0wflSCTOId0GtzfqUBbC0aiH3
PSvQt7CPVvD2EuEpXKJ022zS7h//9/9CgOIFNhFHqh/42J5DLw2ugL71u6WM
fa9B/j45ToY8NyofypSdShnyINyGXHZ80he4RbgBq2zP+6njQ7gcsUpFxnj4
E+5EjVs9DmXdBb+6Ur7UpN2DfoxtlddJegD+LKUEv48NhXlkkxjVffoI7vOn
ajQ8fgLzv1kiTj8sGvovl/qnMZhGeBQdkDA2CIyDfh9NffXJLxHm66zEqhO3
U+DcLtWm1SMdzm9IVJ28/hz6FZAq0n7lJeE8FCFx89TlV5RelJja9tUmD/Tm
SOw6Y/UG7pemPug6XwR+NEj8OHemBPrbmarZY1wO/fghEW9uWAnnS6l/+/Rr
IB6bpInl4ffUPmD+tNxBzQboz2ZJbmu1Jtg3uTTbkX0tUJ+qZLWN4hfQeyRN
dGxXB/TTVNLTXvYbxLNJa5/Y1g37fl1yt+PWPup77J8WMi06CH49khxzFhqB
9ygx7dCcwBi8DzmSCS5rJuF+aRrdT+4Zah5Qg+Sp6xzz1PeoM+31L9ZF0D8q
yePO9Bv8WUyz+0NHZ0PVyyJVc3OJgXAe4ksXo19gIpyFRKW8bk2zEC5Hsukd
y8bZCffi/VIKPsMchNvQkfSHzP2rCLciU6lxv++8hP/LnK7F+nUN4Q50XSox
oHUdlQ/7p9OvaN5AuB+HS50O+iBEeBLHp+dx1IoQ7kYvpXiD322GeMXp9qtK
txKuQvVStSGFUnDekb6ZN1+acAMakboVliMLvJj+lS9LHvSwbNsTkaZAuBjz
ZYSuTVKk4mPRbRNPYpUJT2PZDO31T/dT+pHKtqTox2rgt24Gw8YwDUoPPrXN
lBasRbgFiV/cLeF+mPAgmo7nyrl4hNKHi7qGlAyPUfXjgPVllaqGoM/QKEpf
+iThMbwp9Eq7wCkqPxr9oGvBcgb057GLj8+cg/54a9C7fjcH1rvdxlBvCd+v
e5sdWGAN89K/GMiXZEvpxS92XaA9dCDciG447pPwdIJ6NTP5c2yuEh5CPMOT
SiddCY9ilS+GFuw+EM+u6k1gYTCc72UM40t9CP1nUrGjhYcDN7hpSNx+DPej
Xgvl2EfB/FpN/1Q69Qz83CndVKkZC/n+WKfryyfA/NQk+rRvSqbmHYV3m1pw
pMF+nBNUGF/MgPqkjFe5DmRBvxfChhmaswl3ofKPZYHFudDf+yuj+TLyQZ/x
oau0xxj82+yjJ+H7Fs6nisVzHEtBT+ESvfKZCsI05K/QXqldRe0fNnDO0Veo
hX3dmBXULloP+zU8csFi1UeIn7tFZfx3E+yD1/m1rsMtMF86z6YYPn8Bf/jb
awPLOgh/Rz18CXxZ3wgPoMyjHrSobvDn+r0TEnf6YP7Ua3bkXBmEcy5mNmWz
EcIzuGN/T6XuGOxvsjvWV5wkPIyd8sPat8xAvcqzdha88zC/bDKa43SL4FeL
zSbXH0v/+L//32OSFxna/oIfNr1Nge8YbCl9CkIZfNlMhJvRiwCO5d9YbKn4
ErP282wrCJejuDMfB3ZxEu7F62tkW824CTcgOue8x9wbgV071wYoCxPuxlOa
btetxah8+FJ2h3W4OHUf925QNimVhPin/Z9pj20n3IFapujQOlnCrfjIaTOp
g/JUPai6smy9owKwqqzYyqeKUA+O8v1drQx65JcP/pjdD/czLx/q3KROeAzT
Dq5466pNeBiHCHx49lGf8CBm990R/NuAcB3ynnjgudWIMA39Np52OG4C9V2t
MDjnZQp+jkvn6mecI9yJrJ6sUf1iTngEfWd0lWWyAv3G9m3CMpeo/KjpiyLP
aTvKD6SjFr3szmWopyLzz3SOM9SjvPZsb5cL6H19u6R5hRvhRrRjTLhCwYOq
F6UYeb8y9yLcgoTL+hKCvUFP5DaNcOwH9fFGJPsOBhAeRUEMbC689yjGzLaX
LFUeUP6jm5/rTtiEAi/s364Z8YhwMbqcfl+h/AnUM8w3KT4RTbgPnfc6unZ9
DOEe1DGSzaoZD/09brh60SkJvq8vvjr8LJVwP9aQbG2rzSCchYvD9tTOZ0F9
e+gi34jkEP6BXlovpem9hnolP52OcisgnIfi970NTCqE+dyQKuTeVAx6wnlv
2f4tg/o4b/aclqwk/Av7D6npnqghPIQYDBKVb7+HeG5Fy6WfNwDvTfu+EN9E
+DtaePSm9EkLtS841zssMPgL4QHkfNne0LeDqhfJmh4SuvEN9E9oiQxf7oZ5
yNz9O9uyD9hG9LP76UHor8SqFxrHRmCfB38HrDo0Bv1MHDZvV56E98bis3KC
3AzMg2g5v73EPPjbnTWlILQI+06LrmPg+w3+mQYk1rHT2f3j//4/c/EMp19G
uBm3nTc+O89EuA1FHJGT+MFiR8UzVOKY6WYnnIV5JQYLWzkI01AjX6lf/SrC
ozh4WZR+OS+w3sQVgYI1hBsRx1e9vufrIF5d9dbnCRsI//f3S+4y10ghSh/S
jPuq+kCEcCdiDn69wm8z4RZUfuNBy42thKfRrYuXaI5ShKuwiqG6tZX0P/ac
RH9UN8qZypLzOoSlf/4+Jk+4C19f31R5SAH8UWDNeLBPkfAUnpv1NZFXJtyD
crrPiknuJ9yLHT/sHRdSo+pBMpg3n08D6p1IHru1QovKhzLDqnQYDhMuRja3
YvkW9Ai3Ign7G10/jhIew4Mmhqk9xwnT0SVq7nD+YgR+mcuzKX8wAT+FhXuX
V5hS/cRdHEUfC87B909/PYrMMgc9pwYvWyRagp8Cn7Slo6wJT6C2ErGfD2zB
n4jMv6V+DpR+bBj5JdDdCfTz+mcbOl0l3IAbnYOELrpS/UHB5yyHTW9Q97Gu
7v4cg5vg5wpFAQ+tW4SHUM2WWQ0VH7jvz/th1S5/mLeD9CntknfhnGnsVsKm
e1R+5MDa98nwAeTvENVgDgyF/miqpOwqeQTzmmPCbjn3BOoVcrF9JPmU0ocC
Qz5Uno2B+VzIkFkIiydcjsyrH4rXJoH/Db2zRnRp4BeiM7ojnwn9ShYoyLd+
Afp5dq8ffpYDejyOeqz79Brma9i2S4vtDfTP8I6q274i6G9pfHyacwno217M
3JFSDv140m614lsl+Mc8X4N4a8GPy9zbbA/Vw/cd2+5He3yE90Tz0OT77GbC
eSjH/Nifwc/gj5Dnq+2C7eBfYOSaM8c6Yd4Xcl3v+3+Hes0b298W9kL+Dz+U
JqYGqP1De1lpQuIjoCdRlEH/9Bgwt4q5V8gkxPcwefeicgbeq+Gr4t1L83Bu
GBLALfsL9JZmjKpa/qHqQ9uqdZ2i6O0p/RG9WXEfGQnPI0Y6nmZmFsJV2EHg
CiNit6e+79j1We4yB+ExpHl0j0XiKuo+yrGNDGvnJZyFhe78ruDiJzyO7saf
mVMXoOLhubclm90ECXcis3aRE1mbCNPR1c/5+PWJEu7Ge7kHX68Th/iJ27QG
9SQJ/8Lch9L5fbbDfQ9zjkMFMoS78NBNB9dxOcI0ZBDZmCKqQHgEFefKtZ1U
JDyIpRrD2e4rE25EET8W9pbvJ5yHGFlNLv1UIzyFHUQLI7drUv6ijn0b685r
Q30aJl5LEbpQ38urPVL1+oQbsGCI+ullx0FPQEZSkIIR4SE0V8VaZGvyjz1n
0Uba0NxDU/BT06VauuAc4V58WTfFqssc9D4RuxPDbAV+lC1ZtUldgv6NNmny
HLMDfavTxHVcL1N+I+VbLD7PnGE+LE8OFla4QL7gHVVzI9cJf0f5y5OluT1g
Xro7/awUvEAPe65ljKk39T2SC9Jo8/YDP06bb+FJCyA8in0Vl+t8DCJch55z
D3jPB0P9rUPvCjeEwnzTlyTOHXhEeBJLRPhKWz+Bfhyzv2AVHE24Bd04eDAm
lwbzk7Bhc1tHHOEOXD/DxLMsCeZvvrZPe2sq4TYkFFfhrZcBfh26nlB4JQv8
cdT3mYvMhniR4hbSpbmEf+Lyv2pWg/mQf6xFNIajEPxek8nYJldMeBqr+PRy
m5TBfFqfKtf2egf+PtwZ751UDf5hNu/C93WEi3Hf9/Nz0x9g3jnyD0iva4J6
dgeLWKm0gN6zlstiLnwh3IfuKPd8Ceyg9KKXq8u4s78RHsbto7HaX7phPxnL
b3n/7YP42yLNCsWGqPjI0FF1TnsU/Lp5SFjacZzwAEoWYrCKmIL5/Tj/nVY0
C/oX60u+9C5Q9SKRxBhu9iXYRx13L22Zv2R/JtHe1B2lkvQOJB76EEbrLGIg
PIjMvbh+6TMSbkQLNp5r+pgI9+JAo4md15YTzsKb1M4eYWcl3I9ypRtsnrIR
LsZaAip3ZFb8Y88J1MmclVC+kpz3IKepjaUnOAk3YJbO+53DXOT+Aoqq/rvo
zk3Oq/CxOUnGOR7CzZhNxGil3WpyfwqV6Hnz9fOR8+/o2o2sjab8hIexdEqH
eMtawkOo/xOLrK4AFQ9FM8grvlsP+g2kz6kpC0J+9lNBh3M3Ev7v99k/33D7
JsLdyPVV35lEYcLlaEf3qouConA+wKHsGC5GeAw/VbR249hC+YkMrcK9fcVB
78qw0qA/W6n+4PKSsfCrkpRf6MbYOtqYFOjdKaCRcmE71Q88rOH0slOayodi
nJ+9MZQh3IaMYmrL62Whfs76+fcH5aj5wO8WRT4XyRPuwO5bjnTt2g165Qxu
DGUqEG5FI57JU5v3QvzYjOZfTxVhfk620TGtUaLqQ1zLt3HcVwa/KneeXLNc
hYqHPc76CN3cD/7LB73YOq9KeA6P5n+VtVcDvXH9rGhAHfIb8+xSP6MBelep
mOl+1qTqQVU2907oaZH5mUaejwvOVmqT8060+13/xX2HYV/GpridXuvCvCdu
3HdD+gj097TOJZ8kfdgfXtdH9zYeA321CWWPHhlQfqBbjeM0TkPo156/Aql+
J2C/JiQ1s/8awX4mGTljF2OYf1MfWsW4CeFpvPplXb3ladBT17nw+Zsp1H+b
Xez7ibOwf3sV9Ic/nAO9k+bu0xrnCeeh5AcpS2/NCbegM0WfmBQuUPEx3wg9
Z5Yl6Hm/Zju/+EXCfchbzXgTzZrwJFK87CvBbwP7ORX9cmewLex/ak0nYrGH
83PzbAc9HYDtFN0Y+B2pePjGzZGi506EJ3BAmYmbxhWoN2J53e5vV6HeRG00
c/Ua5Mu5n57FcR32q7RpvW2iG/jdsCZoq7I74Z+o0+R33ycP2L/RZ7axtp7Q
38Wer6ZMt2BeWMR1BaJvQ7/5bIo+y/kQnsWiWdtD63xBr+zM0yPm/vA+7VPg
XLl0B+ZB58bN6od3YT+Mi8d9JINgXq0Yz6qW3YP+XdVs+GMcDPV6B6q8mXoA
8xHSkOUS8BD6T+PdJCccBvkyjR5M5IfDfRxFn6EfAftT03X54tBjeD9aRbvF
vCLhfey3OtrNHw37OpNe+jTrKewzw6SsiSYN5olLPm5NVwzM0wZXnmaXOMIj
SKLwdjBnAvXeIQX6GZ2kRMJ16KC6Oeu+ZMhncKe5oiUF+mX2Xu2WXRq8rw6r
XikzZ4A/HsfFfkVnwvsc+DjstXwW+PHkK5Pz+xfgV/KmqzsssiFfrkX/6FIO
3C9PMUwJzYV+Nv54ZyGVB/veJbNbuDyf8gONXUnqNHkDfv/KXxM5jWF+WP74
nbhbBPvFp7rAI1IM76eor1VDQQn0R7amNfBoGeRT4Th0aLgc5kf3aD7TrXdw
/1T41tK1VeCvddtjjxfV8P5fE2RTPFRLeAr5ml2f76qD/QxNHM6+Vg/xY4eN
HbgaCA+grO21UskfYd+KHBWH9jURHkV1uWkJn5sJ09CXRQEz+xbC44jNU5N9
9DP0Zy/TlRyrL1CfdUDM6b42mL8nnPXMZh2wnzWhi887v0J/fq3dctLkG7xv
Us+OMbR2QT2nRD3TDLopfTgwJd3gYw+cF27/8vtwH/gzls2UVNMP8yS4R/aI
xiDMt26R6c+yIZi/mwfuxqqMUPODsqpeaxeOgt6uw70ze8YgHlcT19Pcceq9
Q/uNlDR2TsK+OH69OPF8CvYx1iz8sdQM1Nc4UKqaMgv9W2Y7PiI2D3rkpgTC
YhfgfTV30VTeuAjvWeiS80DkL3hvKrxigvl/w7zOMdfvCfsD+7E5cLF7Fd1l
yh/f8GPy7MsI9+IBWrofIzOca6Yxtf1mgfPkV6ZS8+yEu3Dr3rufnFYSHsOs
xa89Jjj+sec82qveu8WWi5x/R9Y1XB+HVhHux0/0lK5f4IHz2uaLIj28kH/p
ZHjdGT7IJ/Wt9ErHGsLN+JT5uODJtYQHUdCQQNWnddR9VGSnefnoeqJnDo1N
O6/7sAHyCbrGlGlvJNyK9f68t6kSIjyFPG8vrlYXJpyHsli2vC0RIfwDdQUd
s1IWI1yMVvF4rnqzmXALUo1IL9gtDvodN3w5n7OVcAOKjWVaKSMJ9TRtkc3N
kIJzOdm7LEnS1Dkyf/36hYgMpReFol5jmizUW17CxbhBjvB/v2gHlTIeywMz
pia3ceyGfvGu5GXxViDcg0Qcbsr/3EN4Gsk2DZvZKRLOQnZnIvgP7Ad2L112
ME8V/AkUs3fapkbpx5H+bbRYdcLDOHVEvX6NBuFJnK/74legJuF5XPVi/VYG
LdD7mdff0EUbuN9l+vaoDvg522b64pwu+MGoXNPZogf94YmRX6GjD98LM8bs
KTkK/ZaxXGG5y4BwG1KpcQlNOw79OLKtp0ToBOFGdCZYdzzMiPAotpvOX89u
TLgOeRiKaXmaQL+C8oNdZk+Bnqj1S/HWpjAfaTctG7+dgXkv6G78a3AO9qNa
XXlbjRk1j7g1OcV4nzlhGhpgX+2fYwH1zNl5vtpqCf4yNY50P7Wi+ol55U9w
8VrDfZGIUqU7lwj3Idlf2y79sYF+7Dd9HOFkR+lDR0oY3w3agz9nRB2mT18m
vIDt/NqFmhxhntyHD+pqOsO8BR5+6VZ4haoPRWZtSJF1AT9See60JF2DfS64
OrNsw3XQV/3ljEyIG+Eq1IpqTZe7U4wHn+0KvOFBvVdoniE2f/ImzCPzhZUD
F7zg/urqa7wdtwiPI1Gp3v363lD/zvt69u98YN5UpwqiFP1Av/7xzTVZ/tR8
o7N5D+bFAmBe7AV+i0behfseHlZHuYKgf0Hfm2763AN/o9T2ZSzeJzyB05JS
2+wfwPcFbHwsfSEwr0I+FYOuoVCv71/nao5w0DvqKpoa9wjek6MzTQEKj6Ef
eXa3L71/QrgbCw7J6phFER5A3ue7peajqXM09PXBysBn0A9do/1jQjEwDzmN
E/WvYsHvdYdpz7XiYd48K/WCvyXAe9G//6+DcxKc6+BMfdYU8O/lLlPZp6kQ
n//FSp6d6cAekoXTlRmEO1Fvgk3zqeewj1pC619NZgFnPakN830J9fKtdrsq
kAN6b9yXOJH1ivBP3M3atlv9NfRLw/sOf1sezCe36+CXZRj877TViNz2FuZf
bXDOrbQYfh9SzRJPnSiF/nJ9Pa40Wgb9uXqCSdCrAvR0fMz5s7oS/FfVMf+W
WgXvWfI7nuJ9NZQezLG/jNZcC/vk/MbR6+J7iNcmL2z2px7eI5Wsj6oPG2Ce
EiS8RMQb4f1hS9jBWNgE7LCxq1f/E/X+45bH9yv6W6AfiHdfolsr+BV7b8yX
qw30srA+tUxoJ7/HU8ju9mHNvV9BT/PvJfEPnfC+7r2WzmreBfNBmzIZXvgO
+Zlt2WuDeuD9tBkoSBPug/eu8Zx14Ot++L1S6FhrqzMIep8aVh/+PgS/H8s+
Xtt+dQT6a6Utzsn+g+ovrq/4PP5sjNKH5FT8GuQmCP/FTwp2vaiehPh08v0P
TKep/uMLz8Mcp2fgPa/bqn7Mf47wEJKNn9m5YYH4M4MKzpylf/QT9B0QqKvn
+gXzVteyOypgCfbJICTuIuMf8KvjMOduj7/w+2vB6sa4QOdIxRsr7/94mYFw
F77qefTZyDLCA+iPYpGNBRPhRuQ3v3XvN2bCxYgrO2z5SRaIF2FH/6mRlXAe
EpKwjdVhJzyJk/ta7d+tIPwT74hRU1LhINyJ8k9lsRVwEu7HqvzrW3euIvwb
1zT5JWRwE55AR+9PO27hJTyH2rTOqMSsJtyBzJhrVwqsAX0jJbvaQ/kJZyFn
99hkjnXASwocV/0FCDdj7xnXAwwbqHO8MquP64Yg5A+/pN85uxHuC24pTLPf
ROXDid3irkPChL8j6aehB8+LEm5AeSfpeL+Kgb8qq22+G24B/VUNnzMbxAn3
Iv3AAze0JAgPojaN54fKJYHNlgmsUd4G9QwX+fa+3g7+Ol2feiGzA/q9JG96
M02G8hd5T1briO0EvSsy5Nc9k6P8xWFWMQP8u6C/gqIrX4Xshv4kfrt2a8Ue
ON8e2avnuxfmJdfwyAY6BPOlzI2HXZWgP5Xvt+RNK1P+4CN3HvrYqkA9rWp/
jw7sJ9yNz9JdEjp3AHjwTcuPNjXwy8FF9Y3BQTj/KZvpX68B8W+NrTXUPET1
E7Ol+oiUahGmoRCLyQlFHcJTWGDT6aJXhwm3ofiOqrvSeoSHsVSE3MmUI4TH
cM4x2maRozD/SpwrZqKOEe5B72pcSviOU/ODdH177gUbQj4NrXs6u4xgXlQ4
9rB1nAR/FRp7Kr1MwB+Z8Hs+W05T+ZCE8Z4D700JLyFhwV46p7P/2JOuUKD7
XhG/GeUX5k3cc6PoPGH6wpXWvXvMLQj/wczb78+zWpLv59HfyT2vnltBvoVX
vY7HrUHvpOv9Hb8uUf3Hw0p7x2i2hEdQN31f2kF72Jf2ivsXRx2o+cfNd/Zu
CXGEftUd7uvd7fyPi+mUKlYFx369QvTMoaJPe8/edoF8rx/3bdjqCpx1Ori9
/jrhOpSySfGx8w3CVSi2r89wnQf0MzIlmLf4JuUfDrVVbLTwAr8DZfrvs9+G
/vnMBh9+4Q3z55GvyH7Cl3A5uureX7XkB++b/f4HvrF3CI8jKyakpnkX9J6r
7qcfC6T0YeOgB28f3oN5OqaP3PcEE25BOqsH9n57APfVvzxY8H4I+ZSjUa5E
GMVo17kBp4ZweH+kxUJkrkaA/+JDaFzgCbx/QhkD6SWREH/t5RBry2joD7e8
kvjKZzCf7D8H+l7SYL4YC0PijGJhnn57Kp37Ewfv0ZzaoGB8AtQzzvKw41AS
6B+sU3oyngznXcGDJ8JS4f34YvBwtWI6vGeN/MpNXRnwfU3HYLDvc8JDqIz2
UFfqBWE6OmyuvKLxJbznr8SHql1yCC/gzNGHfhtyod6kLGX1stcwfzTnIYaL
+TDPjxVCiznewP2QJWWPHAz5AoqHFI2LCM/i296hP/++JTyP/wdwyDAN
       "]], 
      LineBox[{{3.3939504394632203`, -1.*^-8}, {
       3.4043485100485915`, -9.359141017739603*^-9}, {
       3.4963577637675, -5.9435136812169276`*^-9}, {
       3.5883670174864086`, -5.9050160317042355`*^-9}, {3.6803762712053167`, 
       5.266004743376129*^-9}, {3.7537187022218914`, -1.*^-8}}], 
      LineBox[{{4.016730575917462, -1.*^-8}, {
       4.048413286080951, -4.734239000825369*^-9}, {4.140422539799859, 
       5.045933226810462*^-9}, {
       4.232431793518767, -1.1524121656947273`*^-9}, {
       4.307680624594284, -1.*^-8}}], 
      LineBox[{{3.103234041670681, -1.*^-8}, {3.1283207488918663`, 
       1.0464336064330837`*^-9}, {
       3.220330002610775, -2.183144998113562*^-9}, {
       3.276314799602281, -1.*^-8}}], 
      LineBox[{{3.789705745380885, -1.*^-8}, {3.864394778643134, 
       6.754980130807553*^-9}, {3.921957542013565, -1.*^-8}}], 
      LineBox[{{2.9539673299856957`, 1.*^-8}, {2.987259211641674, -1.*^-8}}], 
      LineBox[{{1.5077097137836162`, 1.*^-8}, {
       1.5113447795647572`, -1.*^-8}}], 
      LineBox[{{1.8663569372735958`, 1.*^-8}, {
       1.8830984480382928`, -1.*^-8}}], 
      LineBox[{{2.6209041797285964`, -1.*^-8}, {2.627412324482937, 1.*^-8}}], 
      LineBox[{{0.2461448889451349, 1.*^-8}, {
       0.24614607961512902`, -1.*^-8}}], 
      LineBox[{{2.4407246361207497`, -1.*^-8}, {2.4838572519765343`, 
       1.*^-8}}], 
      LineBox[{{2.0393275788331553`, -1.*^-8}, {2.046726965368327, 1.*^-8}}], 
      LineBox[{{1.3550038245320668`, 1.*^-8}, {
       1.3559814177586502`, -1.*^-8}}], 
      LineBox[{{0.5304027987297177, 1.*^-8}, {0.5304176170703712, -1.*^-8}}], 
      LineBox[{{0.3377152899936586, -1.*^-8}, {0.33771774725682197`, 
       1.*^-8}}], 
      LineBox[{{1.8157625431201623`, -1.*^-8}, {1.82529409215811, 1.*^-8}}], 
      LineBox[{{1.0207327390379488`, -1.*^-8}, {1.0226946708048907`, 
       1.*^-8}}], 
      LineBox[{{2.4843640715322977`, 1.*^-8}, {
       2.4960579123294386`, -1.*^-8}}], 
      LineBox[{{2.1769439233212187`, 1.*^-8}, {2.183409812036653, -1.*^-8}}], 
      LineBox[{{1.4442101037960573`, -1.*^-8}, {1.4468020153379755`, 
       1.*^-8}}]},
     Annotation[#, "Charting`Private`Tag$18536#1"]& ]}, {}, {}},
  AspectRatio->NCache[GoldenRatio^(-1), 0.6180339887498948],
  Axes->{True, True},
  AxesLabel->{None, None},
  AxesOrigin->{0, 0},
  BaseStyle->{FontFamily -> "Arial"},
  DisplayFunction->Identity,
  Frame->{{False, False}, {False, False}},
  FrameLabel->{{None, None}, {None, None}},
  FrameTicks->{{Automatic, Automatic}, {Automatic, Automatic}},
  GridLines->{None, None},
  GridLinesStyle->Directive[
    GrayLevel[0.5, 0.4]],
  ImagePadding->All,
  ImageSize->{753., Automatic},
  Method->{
   "DefaultBoundaryStyle" -> Automatic, "DefaultMeshStyle" -> 
    AbsolutePointSize[6], "ScalingFunctions" -> None, 
    "CoordinatesToolOptions" -> {"DisplayFunction" -> ({
        (Part[{{Identity, Identity}, {Identity, Identity}}, 1, 2][#]& )[
         Part[#, 1]], 
        (Part[{{Identity, Identity}, {Identity, Identity}}, 2, 2][#]& )[
         Part[#, 2]]}& ), "CopiedValueFunction" -> ({
        (Part[{{Identity, Identity}, {Identity, Identity}}, 1, 2][#]& )[
         Part[#, 1]], 
        (Part[{{Identity, Identity}, {Identity, Identity}}, 2, 2][#]& )[
         Part[#, 2]]}& )}},
  PlotRange->{{0, 300}, {-1.*^-8, 1.*^-8}},
  PlotRangeClipping->True,
  PlotRangePadding->{{0, 0}, {0, 0}},
  Ticks->{Automatic, Automatic}]], "Output",
 CellChangeTimes->{{3.7411687137864122`*^9, 3.741168826023624*^9}, {
   3.741321894836523*^9, 3.741321911483397*^9}, {3.7413219631318083`*^9, 
   3.741322008030081*^9}, 3.741336607876193*^9, {3.74140871019598*^9, 
   3.7414087801796207`*^9}, {3.74140883400991*^9, 3.741408888993909*^9}, 
   3.741410200012617*^9},
 ExpressionUUID -> "356a3658-4a5a-4a1f-b497-996744b850ad"]
}, Open  ]],

Cell["\<\
Then we can compare the Pad\[EAcute] approximants of the full-range exchange \
energies for different orders as functions of kF\
\>", "Text",
 CellChangeTimes->{{3.741408500229847*^9, 3.741408530990829*^9}, {
  3.741410512083131*^9, 3.741410526979538*^9}, {3.741411306569736*^9, 
  3.741411340076364*^9}, {3.7414114012460947`*^9, 3.741411403760552*^9}}],

Cell[CellGroupData[{

Cell[BoxData[
 RowBox[{"Plot", "[", 
  RowBox[{
   RowBox[{"{", 
    RowBox[{
     RowBox[{
      RowBox[{"(", 
       RowBox[{"ExRCPad\[EAcute]2", "+", "ExRBPad\[EAcute]2"}], ")"}], "/.", 
      RowBox[{"{", 
       RowBox[{"c", "\[Rule]", 
        RowBox[{"137.036", "/", "kF"}]}], "}"}]}], ",", 
     RowBox[{
      RowBox[{"(", "ExRCBPad\[EAcute]2", ")"}], "/.", 
      RowBox[{"{", 
       RowBox[{"c", "\[Rule]", 
        RowBox[{"137.036", "/", "kF"}]}], "}"}]}], ",", 
     RowBox[{
      RowBox[{"(", 
       RowBox[{"ExRCPad\[EAcute]4", "+", "ExRBPad\[EAcute]4"}], ")"}], "/.", 
      RowBox[{"{", 
       RowBox[{"c", "\[Rule]", 
        RowBox[{"137.036", "/", "kF"}]}], "}"}]}], ",", 
     RowBox[{
      RowBox[{"(", "ExRCBPad\[EAcute]4", ")"}], "/.", 
      RowBox[{"{", 
       RowBox[{"c", "\[Rule]", 
        RowBox[{"137.036", "/", "kF"}]}], "}"}]}], ",", 
     RowBox[{
      RowBox[{"(", 
       RowBox[{"ExRCPad\[EAcute]6", "+", "ExRBPad\[EAcute]6"}], ")"}], "/.", 
      RowBox[{"{", 
       RowBox[{"c", "\[Rule]", 
        RowBox[{"137.036", "/", "kF"}]}], "}"}]}], ",", 
     RowBox[{
      RowBox[{"(", "ExRCBPad\[EAcute]6", ")"}], "/.", 
      RowBox[{"{", 
       RowBox[{"c", "\[Rule]", 
        RowBox[{"137.036", "/", "kF"}]}], "}"}]}]}], "}"}], ",", 
   RowBox[{"{", 
    RowBox[{"kF", ",", "0", ",", "300"}], "}"}], ",", 
   RowBox[{"PlotStyle", "\[Rule]", 
    RowBox[{"{", 
     RowBox[{
     "Red", ",", "Blue", ",", "Brown", ",", "Green", ",", "Pink", ",", 
      "Purple"}], "}"}]}]}], "]"}]], "Input",
 CellChangeTimes->{{3.741408474718514*^9, 3.7414084756842623`*^9}, {
  3.741410208407321*^9, 3.74141022884708*^9}, {3.741410300557962*^9, 
  3.741410394975423*^9}, {3.741410441039117*^9, 3.741410463781569*^9}}],

Cell[BoxData[
 GraphicsBox[{{{}, {}, 
    TagBox[
     {RGBColor[1, 0, 0], AbsoluteThickness[1.6], Opacity[1.], 
      LineBox[CompressedData["
1:eJwd13k4VN8bAHCKkpBUkiwpkWxjrlDI+yV7SQtJllnuDIlorEWUQsi+FNIi
DYqEyBankiwlkSWkUMqSUraU+p1+f83zec5zzz33nPe87ztyDM/9rEU8PDxi
vDw8/35LbH9Pfyl4s/PQ9/qRm2HlNZH1Tl37Yh8Y+Dk6hUcEp9bG94QGysQ+
M+jVaVewCebWJn9IfsEX22Xgoa5urR1cVps6kjkzG/PJYKLqYuOa4Prate4b
oydjZg0alDPTK0931h4qIG0mYpaCbNxPd2bQcO3si7DK8Zi1QOoK/hHzn6kt
Wf1KODx6CzSfFA9xtV6KvJQ1Wx/qUmEu1+STw7aVSNx0NrlxlQ5YTn5OMYwQ
Rz8ernXLctsJebcUheVlpVCYs4zEpa2GYJG82UAscQPKj3E+Z+RsDEqR+UHq
Wzeh9Scd3OfOm8HttvPWsombUU5e74twH0uof3Tgw98CRdQSEfkg8KYVFLE3
MApfKqGojj6hzS3W4HxZalE+Vxm1Pm0LEjXaDx9+fd78dq8q+iD0nlLYdQAY
7eEuVlNqKMJP7caOfTYQ6+Cba69MQbNayTYnR21Bw6WRatRFQcs7u8z0guyg
oWhbrJW7Brp7yWFu7PthqJ4rT+QMayCZe3NjVpFHoO2ebqf3YSqSHuvIuMrn
CGa/X1dYl1IR+fBWjuByR0iyv2dbW0ZF+XG+JX4rHcEoLX1cpZyKdmiuabaS
cYTQgCY+/ioqsj19cP6PtiMksN9P5CIqil/Rbud8zBG8P+iP1zZTEZ9m65oN
bY7ATs68pjJARaNBTXE3rjnBwZuiKSuXESi/PiX/6y0nEJeNN9cVJNBxUXqj
fr4TTOnOipHLCTR5c3ZRT7kTsLsyPxYLE2iuSd5PrM0JWvm1E43FCLRkXYjD
OT5nOFM8ZmqwnkAbSwkl1lFnUDtdLxuuQqACPyt68joavDbMsTqxm0DtmSrm
YVLY/i1W+/cQ6GedoIafLA0+5AkmUq0IZLzqGY/dZhq4S94Z/LaXQG8LDa6v
16CB0OxoMXmAQMIjlHdZZjSoT7E2VLInkMeRVY5F/jQw+6lWouhCoKTQyV1Z
p2iwyywxfBK7Iu+lStJpGuyNt8yudCUQ/1z0b59zNOhb4NZauBEoM5nvik4c
DdZ1WgcxPAj04sV0Ty2XBhs7ew28vAmkCt12LR00SJ4WCV0SQiCe1J05f7pp
4FrsoNCI/Xose1qtjwbzFUkLUWcIFHTpRGLcIA3+ur03FgolUNOE4HPrrzT4
WPXRmD+MQOxMfYN2ATr4sUWMXkUR6Pp81uZuXTrI09yU21MI5GO9zEfAgA5u
F4QrglIJZMr1fKxjSIfKm1dDN18i0MQ+Pec0MzrModwmn8sE0s/ruGxvQ4ep
UhUtwQwC9RwSEHp7nA48LvsrRK8TaFWpx/eBG3S4ONdDi80jkErMbsm+bDoM
SkQcEL9NoF0sZcPOHDoIPPydlYntt2YkoamADhtnthy+fYdA3b6kRkkFHbp5
H2+pLiDQVa0jXudf4fd9rg1/VESgreVmEwq8DJB/Y9d0sIJARvGK4nJ8DOCY
qtQ1YDu4Ltm5fikDssV65fQqCRQjURezQpgBHhG3l8lVEehbgIHqnAQDSCPV
hKFqApVt13JvpDAg+tX5e5aIQP9VbRo9RsPz50Xfz6sn0Nq9ZyQPMRlwHPUX
Cjwj0JfBPgtDNgO8NZ+ud8FOE0y9I+HOAIadpMnGBhy/hwU8nvozwD0kfDSh
kUA35sa/ysQx4MJWq2u2zwnEq1U2/eohA3Yk9Uj7vyJQV6OYwkPEgPqg6tg6
7AJHT9vcJwyYp8f7rWwj0OGwLQ+CGxkgfKTrTh520ev0AOUOBgz40Irb2wlE
9w75dX6cAafoGkdEOgn06J4Zr856JryOMQ6Q7cH77a16mSHDhPl8OzM6dsM2
MfUYOSZcjPAOzsJurex1GFRkAokqpTf1Eqi/7nj5RU0mfDMn1aX7CDTfnew5
sIcJjPmMjqm3BArOOLlEaB8TxlYyNqn24+9xcsrUOsiEL+FivSS2wJBic7Q9
E0ZVlSLbsNd+qVTQcmHCYOHnYe47AmnyDryNOsOEsuuH+4kBApU/eepTeo4J
B/ljPzGwdcNvL38fzgSZy2ecErANl/ts3xaD51NPSh3H3rdmacq7NCYs0lih
dWUQ34euMWXBTCZQTnaW1GPbpbc+1rzOBAMtuPENmyab/i2Sy4Q+sfFmwyGc
b5RUd2uWMCFeZrvLe+zvYyuHnMqYYA+5rks+EMj37szJyAomnD6Q3quMHUSg
nP5aJpS7zYj7YkfpH1gc+ZwJ61+uHuX5iAf3nax8+5EJWmhs2x9sr9TOrW2f
8fo79YLWDRNIp5fIqB9jgopiobkmdhM5EVg4yQTW/bJTrtjj/kz9swt4PSGR
O5qxS6tRgS8PCZfrpGoHsYN5ZWTcFpMQEmH1/Cf2iujuP/uXkWBqbnlW4ROB
qFf3IPk1JHie6rI/hf1r8DZlnQQJbjUXlWKx6xQFbgivJ+FHm33oDWybosdn
ZzaQIPlgoa0eO6BO26hBhQRG99np5Z9x/C9LKalWJ+Gns5ykFLag1fdNRVQS
atbua1LGzujK50vXIWFoeH2LOXbNqFz9sV0kmKwJcD2DHaEeokUzJaE/tHji
Ira1Tx/3oAUJwVGTvGnYAwupEfrWJBBVWq2F2LcNp2Y1DuDnvdKiK7E5Eftc
FWxJONRV8boOm2+lkPkKBxIuWY+LdmO/sDlasdiZhIw4e74B7NT0eqU5Ogm6
PTvDR7Cd3m1KHydJ2Kj0LHUSW1H+rOCACwlLjspp/cT+5tp/qsONhNJTgSTP
CI6/At2xRg8ShInFG5diW2jPNBd7k5BduN9yFfaqoAN6OX4kzA34PpDA7kP3
8jNOkqBy6XSJNHY2v4h0fBAJp1wvGWzE9rA4FnM+hASpoW9HFLC14hoWAkJJ
cLnwQGAr9p/2zcc9wkgoeyFhoor9TOJcP/0CCd5Shqsp2PGO761so0kQbaN5
U7HtsvRrLWJJEIIspia23Kd0dYMEEibuEB+3YY8qz10jknE87DWc08Iu9rIR
3XKJhNxDv65oYweWFp+RSiehYji6/Z93za+YFM0kQVxM7v/jQgYedP7rJHgN
fZr593zHuaZXP7NI8LUT/vBv/t2zhbmqXBJEtBJ2/nv/Y7eUEHoeCd2TVRL/
1qfTf8o2JZ8E2s16jjr23X001cZCErj7RnerYMs/NeZbKCZB4YdzzhbsDB3l
XkoZCQ0etFB5bLF80WKygoThVPl+WewLsjMXLleTYEN8rJT8t1+Jvc7Pa0mw
mu2RWIPts+SRFs8TEsLCd86J/Pv+k1xhzXoSVvmYHRbApn+J/uDSSMJ5Qw09
Xuxu2omqjOc4HpkaN/6dv9Vr28SXL/F92n72wr/42FElB9qd+Hw0J/vfYd9T
W7r22BsSrjWeter8Fz9Z41+u9pGw8N3wv+fYqyMfZCwZwuenrF1Uhh31+wpn
xzAJ+xV61O5g83iFmh8fIeF6dAzlGvYX2z2zHV/x/pbxPQrDJpuoLct+kOA/
qG0dgN2jL3FLf4aEPSb2pBt2vfzQ/lu/cbw1W0jtwb7+PeCuzzIW3G4eaRXC
Fmc7heUKsaBOgRvzC9/fi2+MHPpWsEBPW+jVCPZJJCK4S5wF1wKLxuuw98dm
s1ZtYoGcAP20L3YDb5SeqQILts8d86VhG/h6rgpUYkHFVOe0BbaKw45Hg+os
2Lg4J14Gm39rq1SxHgv2knKaCOefoMzSHx8NWPBNUtY3B/u7aEbTOiMWhIuo
Qyx2/ywr4Kw5C3wiHX3tscuf/mq3tmWBpHY3/QvOj250xeivnix4bKLEWcD5
9Gp8lNtqbxYoxsvw9WO/qv1ivt2PBQ9ssxRrsHVk7gucC2IBo1ha/jT20l4I
F49kgTjXfm4a5+/sg/Zn9bNYcF3Ce3s7zvfd5x7SGLdYoBR1+1c+9vKSDRCR
ywLDvqj94diclZ/+tN7F67khWKuN/V+LdxBZxYLSJsblFFxf+k1j/KNfs8Bf
S95f/z2OT/9vtve6WJDS2pouim3MPaDV0cOCEwc1bIdwPcvnk5yWGcD7/aQl
OQI78BGXU/yFBS/jqrWacf2T0EUeb5awgfWfnrYBrp/71H4wFbezwfHpcb/e
N7gevGuREtdjw+iK/pZb2IYJtzv4DNjQ+7folSe25hTddHAXG9h/pbsWYYtX
tm7NtGaDqpnsR/lunI+M706KubKhrsNF7TCu/66OR0P+pLLB7iUKOIf7hQER
Y50vaWygr8xnGWHbow2TvVfYcLfsEu9ibMtN3YyKLDb8zOMxPYv7D7URExOf
u2yoIQSFTrUSaMpHXnj0KRvSO52uOrQQKOTiu/SOKTyfenffMO5vuO5GlYvn
2GCtJ1uQiv18d84bjV9s4Mo5bTLBlhD2lIjldYHIOJ9F2bg/Ko75k2Ii4gJr
93fHHcH904dY6YQHii7QPTEmXFmH82/CkYg0exegsm4921aL71tql7cjcgHU
UxaqUUKgM3Ml7jZPXEA4IuNDWzGBxuzjWXvqXeDxfVNeH+zHsuaH9J+7QP3R
U8dKcb/olVe5Q7rbBT5fHViy7R6Bmqszed9+dQHrFzZ+iri/DB1ixjnIusLH
hnOSPVxcHyjfbh8JdoVdz5yOnk4jkEyVP+8VnaNgtMNSOQ43AyXfBOdLF7mB
1M2/m4MOEyjuQY21Sa0bGEsMW1ZtI1CbUrD5vehjIFulyFgvhPtRVafr8Rbu
ML5QajkySEU6GwrES/g9wPPTJuDi/1eBNUvVC1s9YNklLo0/kor4J0JvycUe
B4XhxsOKR6hopmFZjccRT1ArC3ymvIWKrjT+nT8t5gV+E6UWotMaiD4raHLG
ywvsA5luN+s00Jv59QzPTi/ont+qFxKngaZN9AvStp2ApitT016OGqhSUFzg
Y+IJoIbT7qxW0UDU7ClCeu4ESOy9anNwhoKswodi42054KTMdF1bR0GmFrG7
tew48JxbIaT9hIJAZLtg32EO9N23KbJ9TEEaqbFhio4cKC8O/JWCKGg1d3tQ
DZMDdactklc/pKDep3FHx704MFUE/SvLKMiVX2+XWTQHNjao8QvnUhC9cZh3
4iIe3yKCVHIoyD4moTYplgMyfGuCdnMpaPeaTzveJXBA0uX+bHQ2BalvTtTw
u8wBvprZBcEbFDSz67NM9i0OBPt5716WTkFfBZL6zHM4EMA3JaWURkGfn+un
f83lgLvN0q9mlynozcGkNbr5HPidwHP5QioFVZM7hdqKOXB/eGphaRIFlW4Z
afS/z4E/4k96FRMp6O54UoR0GQfS99pVmSZQ0HWfkUVHKzggVT4ZEhFHQWk6
yUikigPUlkWsnFgKSvy9M/h+NQdmyqcsn8VQUBQa0bWv4QB38IXmp4sUdO58
8s+/tRzoKUqWXYr9P/aiU3g=
       "]]},
     Annotation[#, "Charting`Private`Tag$22655#1"]& ], 
    TagBox[
     {RGBColor[0, 0, 1], AbsoluteThickness[1.6], Opacity[1.], 
      LineBox[CompressedData["
1:eJwV13c8Ve8fAHBKw0wSKpFvRvZ1D1LIJ1KojEJk3XHuJbtr5ZctCdkjI4WM
+BIRGZUnSaEtI6OiKaJkfbV+j7/u6/2655x7nuf5rCvD8DnCWsHFxSXCzcW1
/Fln+2vua9WrPXYzHeNXYhrvxHU491sl3TQIcHI+GxuW1ZoyGHVaKumBwaBO
j7xNWGlrxvuMxzxJ/QZe6uqWO8MaWrPG8+cXEj8ZTLac79wY1tEq7vlPwvfE
BYMHyvm5zaF9rceqSJupxDUgl/yfJzPkY+vC45jmyURxeKnH90ckaL61TvS5
4NmEHfBrRizczXIN8lXWfHZblwqCLmafHLXWI7EDCxmdG3SgwnhFlmGsGPpx
W9y9yH0P1FJLBGWlJVGMi5TEBSVDEPs4byCStg1VJrpEG7kYwxBzU7i60na0
JdjRc/GMCbRNRttKp8mhsvKhx2f9D4IH/em3v1UK6Els3M3TV8zhSO7u09VP
FVF877CA3BNLkNIaVqssVUbP7r8IETY6AnMWx3xHLFTRe4G3lOr+oyC5/t2o
+awaig1UK9xtZQNvm2JXOShT0IJ2hk3wF1uo3RfYatRPQfx9/SZ6IXagqX/J
3sJTA1274Lg4MWMP4oNB5X4fNZBUzeKEeZwDiPx+cDTAnoq2TvTmXeJxgvE7
sVVH6qmIvF1SxsfvBC63Mg/dbaCiyuSAusD1TrDN9sZ7tUYq2q25sdtcygme
yhzhXtNCRbah1kt/djpBcI/dbAWiopR1PXYuHk6QvW5yZVs3FfFoPtu47YUT
SLoJjKiNUtGXkK7kwsvO8Ptj4HZRXgJVdmRWTpc4QxArZVCfj0DewvRO/Upn
OGOTXsrmJ9D3KwsrBhudoY0vKKxekECLXbKBIi+c4adJgZaJCIFWbwp3jOZx
gTeLj7gMtxDon3pCkXXCBQ4PL/HEqRCoKtCcnrGJBrNbFNP8DxGoJ1/FNEaS
BlIxqpk2hwn0XzufRqA0DWRzTYa0zAlkvOEBl50cDTxf/6sxa0GgkWqDgi0a
NMi+EiPodpRAguOUN0UmNJgnfW+oHCeQl8MGp+tBNJCsKbBRdiVQetT3fUX/
o4FYg7jKHHZT+VOV9FAalHp/PHTHjUCrFhN++UfTYP3ESW9zdwLlZ/Bc1Emm
we7ClJ1sLwI9fjw32FpKA+srdqL+fgRShQG7J700uPDbOp4vnEBcWXvK/gzQ
YIOtFvUx9suJ4jm1YRqU8HMLJkcQKOTCybTkMRqIWoU6CkcRqGuK75HlNA1C
G5bceWMIxM7XN+hZSwel2KCY3ngCFSwVyQ3o0oGyTaiiP5NA/pa8/msN6GD2
6qxuZBaBDpT6tOkY0iGiaHqt0gUCTVnpueSY0GHJr9ouOJtA+uW92cdt6HBf
t7FHKI9Ag8fWCox408Eg/HDgxgICbaj3mhktpEPntLlzejmBVBIPbR4upoOE
zFPrLRUE2sdSNuwro8NI/earRdiBG8dTu6rosOizyKr+l0ADAaRGXRMdylfw
G9+tItAlbQffM8/p0LbLtq3jOoGUGk2m5LkZcJKYNT7eRCCjFAUxGR4GrOMf
MHqC7ei2es+WNQzgyOWU7G0mUKJEe+I6QQYsfUnLlG8h0LdTBqqLEgwoFItU
Hb9FoIZd2p6dFAb8HePztkIE2tuy/YsHjQEHX7yvr+4gkLhFxOZjTAbcavap
F3pAoK9jw2aGbAa09SfLeWHn8GX9K+HJgEe9TnY7HuL4tV/rdT+IAYK9zwWz
OwlUuDg5LZXMgHvD3B8cHxGIW7th7vltBtyPaisPfU6g/k4R+duIAWoB4tLd
2FVOPrZX7zGgew+NX+IFgexjdtwM62TA4/Qs0xrs6y9zTyn3MiDvhihjsIdA
dL/wn2cmGeDHpai+sY9Ad2tMuHW2MEGlSzFLfhDvt59qNkOKCZ8drDzcsB9q
iagnyjBhciiqtBz7WfOQ45gCE5IXf1soDRHodbt343lNJtysVgyUHSbQ0kCG
z+hhfD351PjXCIHC8oJXC1gxgSb/OFvzNV6Ps3O+tjUTXIJv2nhir32n0J1w
nAlPT5kIDWKLf22W13ZlgrO0eOS1NwTS5B4diY9gwj1N4Su6owRqvHffvz6a
CbEJl6+7Y+uereB/e5YJPsbTqjnYhvz+u7QSmXCqq813Fttq45rMNzlMOLZ9
SK54DOdD/4QyXz6+fvW68ifYdrnP2jQLmFCX/ilvEZsmnfstrpQJpTVBz83e
4XqjqHpIs44Jl2+XRX3GnplY/865gQm2cplxQu8JFHBtPjiuiQkTdWtWaGKH
EKjsdSsT8hgeJqHY8fpHV8Y9YsLgqToN3g/4S6vg5pEPTJgZPlCx+iOBfLP6
lF58ZsIb6uCcDLbOEJHXMcGEnJrkh3rYXeTU6erv+HyctvOcxJ4MYupH/mYC
X7jcqx7s+luoKoCLBNcTvMwJ7DBuKSn3lSQcvJMYsOITgdYlDPw5wksCl7uW
ljo29dJhJLuRhNKzarLR2D/HKiibJEjg7TVazMJuV1hbKLiFhJS3frYV2DbX
2yLnt5EQcOrt9afYp9p3Gj1UIaFNfN0X0c84/nkz626pk7BVSEpUDpvPfGb7
dSoJ22RaOzWx8/oreXJ1SNjsyRk4gn3ni0yHxz4SJkobzsVhx6qHa9MOkPC/
jz6iWdiW/sOl1mYkOFWqqxZhj/7OitW3JOG4VMjqJuwKw9kFjaMkuNmyHtzD
5sRaucnbklCgIiT2BJtnvYDpOkcS8kyOOY1iP7Y50bTShYR/Wo7afsHOyu1Q
XKSTYC/3cGQG2/nN9txJkoTB8LEfS9gKspF8o64kHL35LHvFOM5/t9f/63Un
IaESPeLFbqzSnej0IsFB822yMLbZzvnuWj8S/Dew2iWxN4Qc1SsLJKFjQE77
H+xhVFOZF0xCi8DjnQrYxauEtqaEkBBpcq5TGdvLzCPxTDg+r00xE+rY2skP
f5+KIoHO9T2fwP7TI+ftFUOCqN9/b7WxH0hEv6afI+HeYPeNXdgpTm/NbRNI
6M3I3KSHbVek32qWRMLtmeh1e7BlPuWqG6SS8GNXe5YB9hflxctEBgm/rkRX
A3atr43wjgsksJyn7fdin66vjZDMxffHa2Yte9/Suu/C+SRc3hNBLlvAwIu+
qoCEsui/7cv390Z3Pf+vCJ/fsTc3l59/aKH6qmopCekluRLLv9/mnhlOLyeh
WOTvoi62zuv/2WZW4vNoMLZffv9rVjTVzmocnxfKdi2vT/a+Mc/vWhyf/zrl
UrHzdJSHKA0kfHpVcFoNW6RSuJZsIkF4oXxEEfuc9Py57FskDD+4jmSX9ytt
yOVRK45Xru+y0tj+q+9qc90j4dS+Ar5Ny+sPLhXU7CBhSn7xpAg2/WvCe9dO
EiyVNBz4sQdoJ1vyHpEQg6I7VmKbv7RNe/qUhHdmO278xPGxu0UGdvaREOFt
Ir4cTzVqa8Q9XpEQG6SZ+HY5foomv14aJmG39dGzfdiicTfzVr8j4fl13pV3
seN/XeTs/kjCw63rY+uxuXyjTL3HcfwSysnl2F9tDy/0TpNwMSRQJQWb7KI+
4f2B80lMvC0Ke1BfokR/Hj9fvnzYH7tD9t2Rkl8ksFF44THsgplT1/x5WWDa
t8pXHFuM7RxzVYAFPml7idXY518ZOQ6vY8H0XsXQWZzPwUiIb58YC36EDpQs
5/eRpGLWhu0sGBhusIzAfsgdr3dAngVjm49aeGAbBPhsOK3IguAiqz4bbBXH
3XfH1FkwFWoRpoi9SumZZK0eC1KsQK8b16OQ/PofHwxYMKQ7Gl2LPSOc17XJ
CL/f5SybHOzXC6xTkaYsmKkSy2ZhN97/2WNpy4JuC4vLi7heutMVEqZ9WPDe
KfbDWuxLKfHuon4scB/ZHjaO6+vz1q+muwJZkP/X8monto7UjbXRISxwi5Kr
PYe9ZgjOisWx4FCEWiE3drH18Uj9IhZIDxhLvMH1fiD6No1RwgL1B/tHG7H5
67ZB7FUWCDfP7EnD5qz/9OfZNRZcVxRuMsLe+8QvhGxhQaHp7apC3F9eH0gM
SnjJAoGVyfdM3+L4DPpmW9PPgnk9hSlJbOPSo9q9g3j/IwNqpnE/q+TZPCc1
yoKantlf6din75Zyar+yoOdza3M/7n8Susjr1Wo2xIvQfhzE/dNK7QdTYRcb
5CdPFH9+hfvBmyeSYnpseN99fmUdtmFqRS+PARsIeTHBUGzNWfqBsX1sYAbP
SAtjizU/U8q3ZEMX7YsJdQDXI+Nr30Xc2GD5MeghG/d/N6cT4X+y2JB0sTEi
Fc8Lo0LGOl9z2EDtTvW3wj6Otn0fusgGaVUv8fXYB7cPMJqK2CDG2+KejOcP
tfH9+/2vsWHD1uKD554RaNZfVvDLfTb8TRES83hCoPDzb3J7Z9kQAoIdc3i+
KfU0al65yIamMrFLJdiPDpW90vjJBvsVmyVtsCUEfSSSuF3hZUUrXx2ej2oT
/2TuF3KFkS0ON93x/PQ+aWvqTQVXsG039O9sx/U31SE257grzFhqVRm34nzL
6vdzQq6gEjnlaVhHoIjFOk+be64Qvj+x710tgSaOp7AOd7iCn/Xc0hnsNmnT
Y/qPXOGuVIn/8rzoW968e+uAK6h3b1HfX0Og7lv53CPTrlD1aeWIDp4vo94x
kx2l3aBV0vPvRCnuD5RvFQ5hbnCufMEiJYdAUi1B3Bd1TgCxcl6qGA8Ddd/4
lupXuAMzXdU33Z5AyTfvWO5vdQcLS/vXL7UI9EIxzLQmwQME9frO7RTA86iq
c0GKmSc4k4Mza95Rkc62KrG6VV4gwPTzfYD/X52+s0a9+pkXWP3McFWMo6JV
U1ElMknekPr61mZzByqaf8h7x8vBB/xZMqk2O6joYuffpVARX4jnF/1Hf04D
0Rf49kf4+oKs+nelnnYN9GppC8OnzxfGDKc0a5M10Nx+/aocrZPwp9z2T6mT
BmrmE1v7Ie0k5MzvQ4dVNBC1eJbYungSuOeEO1LmKcj87LukFFsOrPGbX3Ws
nYIOmCUd0rbjAONKWmPgPQoCoV18w/YcEFcK8MhqoyCNrKQYBScO0JhKL3oR
BYmW7gq5w+TAx/vbiq1vU9DQ/eQTk74ccPSOpx1poCC3VXr7TBI4IJE35Wl+
lYLonR+5p85zYKxAWdu7jIKOJ6a2pidxQGw4hSuplIIObfy0+00qBwj16ezH
xRSkLpemEZjNgV3STQOHCiloft9nqeISDty5TuYezKWg6bXpw6ZlHEgMMA/2
yKGgz4/0c6evckC+rts+IZuCXlmnb9St5IDzZK50dxYF3SL3CLyo5UA4Mmo1
S6eg+h3jnUE3ONDcG/GvexoFXZtMj93awIG/ZTE58akUVOA/vuJEEwfe07hO
dyVTUI5OBhJq4YC6arT3lyQKSvu1J+zGLQ4MR35i8mHHo3Hd43c40P+QcFBK
pKDoMxn//W3lQIibt7XZeQr6P5CNSxw=
       "]]},
     Annotation[#, "Charting`Private`Tag$22655#2"]& ], 
    TagBox[
     {RGBColor[0.6, 0.4, 0.2], AbsoluteThickness[1.6], Opacity[1.], 
      LineBox[CompressedData["
1:eJwV13k8VF8UAHAqZYsoWixFoRnZ5smW5UTWJETZhpn3ZoSyNGQppBTZJQml
UqJNkiwl3DZFKS2WRKuE7GXNT7/bX/P5fmbenfPOu/ec8xTIQEfuPD4+vqX8
fHz/Pst2zo4PFr833jVW33fpWFVtQr1nm0Nqpcl+pmdcfHRWXXrHkYPyqU9N
OvTeKjtHF9Zldmc2LUhtM/HX0LDXja6oy+rLm5hM+WHSX53cIBVdX7d8r2LS
aMqkSTk9L/deVGvdrmKO81DKImiynt5LRfbUTTYduzeQshxyx6b+kwybqCtb
9npxXNJ6GAqiInzsF6EgVe3mmk0MoHek3PPYKIGkLSczG5bqgdSALWdzvDT6
VbPc76KfMZRz766WXy2LjnnJrzhNN4Wr9dtdBDPWoBspXrFmXuYwLBooIklf
i2QiPPZOHbWCWHbT9tYTSqjo6oemuJCtcEN6LGJ3sQp6GZ9QefCSHZxtkWg+
+JKGEls6RZVe2kNvUH79sQJV1PzkTeQSM0fIzVQ7bmGrhrpFP2uWtO2AoRzz
p+whdRQfqp5v4OAMLakBxDtlTTSpk+kc0b8TwtzEvlDNmkiktc3KMNIFLs4g
J0dSC9087TH1c8wV7uosNC9r10JLBFWPmk+7QqDFhhXpHVqIFz4tfv6vK5xT
lqvY06mFNrpmqTiKukGvwOYdqz9rofurmndWKblBQ9eDFeE/tFBjnln5URc3
aC0ImTcyroV6LtF5crVucMTG9duMBAPJ35r6aZfgDo5PokoTLBhIWKmKbpjm
Dgc9RLfxWTHQRE6YL+2UO4zULurdb81AL2Mneubnu0NEuoicpy0DRe/6/aWq
yh3cUquOKzoy0Me54TbFXncwfeCccZDJQOe2/Xg0YeEBGmKGLwODGUjuZ8uZ
cwuYYLfwlcDeswzEqblcJCzChPGlRZK1eQx0I21/WagEE2z6Gfzi5xnIQFvq
uZ08E25zA44W5zPQziinmTldJoh8LKV3FTJQuvhbF689TFDcHqy5qJSBFmg3
S615wwTL7r6x+McMtHXhBYXkdiakKs1WVDxhoIz2QLWpj0yY8pDmdtczkEKU
uHnzTyaAbmCMYQMDGdfbhcQIeIL/c5HqT00MFObS9OaznifUPXp5YKyVgfoj
G9Pyz3tC6Ny5WZteHG/9qRvDlz2hsG/momMfAwUsYTcY3fCEpro4c9d+Bhq9
NDmvo8oTqtrUY6gBBppqXBcq+cYTgtXr3+wZYaCFKw95xC7wgu44KyXbKQZS
LCdoXF8vOEAf27xtEYG65+bMywK9YNm3jn5tQQIVWjWS/KFe0Hth7rSMEIFo
nayzeUe8YB5t+u93YQJpzk8Vbz3jBbZFzxYHihHI2KF33OKlF5j6Wro6ShGo
ONSOnbmSBS5+F4O9FAn0Nm+D9TFZFvAl5peuWkug6cfCWqGrWTDv1FGZFmzz
pU/5XJRYMCL7LNhSiUBdJSYXZLRYIFLCZ6i4nkCL+zQ/XbRigbnIMtdbagTy
d1/KLA1jQUJxlLamHoFOHhndcvEAC2RjDjm9xr579dWGk1EsMHUaLdynTyCB
qaTZkFgWOOlMfCsxIFBe5oKzemks6Jo2fKxoRKCmpvGOukIWPIqP2Pp1M4HU
oN3lZQsL1l1d/bXBhkB8WcZFc+04/gljWeZWAr37WTCu3smCggy/vcPYkaf3
ZaR9ZUHen+HtEtsI1Dgk/MJ+mAVPwn/RbbYTyDvPyOStIBuORrzyS99BIINf
l1Lmi7JBQ/nBOiknfH/Wwp2EOBtYO75OZWPf+d0aninFBm3v6pE8ZwLNtw26
7azIBtNBPuW8XQS6MHNRqX0TGxxHUj4HuRMoxF4oRNCEDaUuHI8f2JaFgQ/1
TNng9fv4hIcHgYYcDL1yrNjw++GjOHMmgYyutmS7ObPhVoyGvKgXgTp2CYp2
BbAho3wrGUgSaGm5/9iXfDY0Rb0QSvch0IYU21WdBWxI9Sp71Y29hatq2lrE
hqLDU216vgQKleo70VjMBknVfbc+Yrfv52iV3WUDPbQ7TmEPgc7puAcdfc0G
q00CU7H+BKoUM8iOfseG7a8zZl9gN/esQOFtbEjpbrSQCiAQ/+lWcf8ufP17
0eJL2JxJhxLnPjY8Uj5dXxlIIHqV1ZAyPwk9cTfca/YRyCxdRVphAQnphZFv
Z7A9fBYayywiYetK40xdHoFSVjxOEV9MQmgPd/Qm9ki4idrUChJI5tzqU8EE
qtDX2dugSYKHft9Bk/0EeiUhlfmIIIG92fjMPuzevl/VNTokbLn8ZOEl7JW5
pSK3DUk4NWTwaH4ofv4zG67nWpEQucGv7T725uq1/XtYJCR0yOQuDifQ8u0x
q3ZRJKiWZ70hsAe/dtqYepNQUunOdsXOEc66vmIvCe9U4o5cxB51FfR/EkZC
gNDV9g0RBHo6yMm7dYCEv/kPnm3Dzjv8oOlMFAn614uWBGBbXz2gzoslIcYk
78oN7PypgWH5NJwPcv+cwgEChSVbrxHOIKH8HNw2wt62ptB+PJOETULudS7Y
05Zepc9zSfjZbNSTjO1w+jUvvJAEq7OzewaxVVTVL1FXSajuPTI8/yCB/qtN
fGt3gwSBlPamldhXe8y0lW6T8D6s9IwZNr9OxfjrGhIqCp0Pp2G3NUgq1yAS
ft/M+HwBu5gZuPPKI5z/M3JnS7Fdj62vjG4gYX//h/WvsTVWHvvh+4KEPfkB
M5+wBYq/LHd+RYLs98W0IezSd7nhqi0k7ORpnhOMJFC8z+QV6XYShjokvy/D
Zs7ueM//gQQfMZSwBptIvyU02EVCRtLuZFVsoXWLDdo/4/w26g1uxP5U6ev3
6BsJdobUDRPs8q31uTd7SLi/VbrRCpsdfOjP0QESQp6/VXDF1l3UqRo0TMLn
IUMPFvbiM3oe7mMkCEoPjHtjf1M/lWwxjtdPWDK8F/vuw9H7WlMkXE98b8nD
TttpNyj7h4RUp1C+MGxu/zU5wTkS+ldJrzyIvSl6kd0vPgqQcO+JaGwJSU70
x/kUKNrI7DmM/eMyutmwkALcZApisWv05T7dEaJgqRppcgz7ZFOE+AVRCoRn
3hrEYfuyW02SxClw8KVO/7PJOCMoVJICvWgT53+WSki7wJaiYE77dMi/63/K
DjTbrqCg40jO+L/1H9yy4teToUBs5/72f/+/JVgtm5SnYHfpo45/8T3bKKmR
okCBoDdn7b/4bacmnlSuo0Da7OTtUOzmex88vqpQ8Gtx8vF92E5R6JeoKgUr
jiRe3oPdZnI5UVedgg0OjUJcbLd5iQqkFgVjivHlTOyPjwOqkrUpsDo1e8UZ
m4zfsb1SF+fD0LvbFvu7tV7PFwMKDuT/3W2G7SMqFyVqTIGb+QJtfeyBl/zL
dDdT8CqvxEodO+hEzzX2Fgr6pY0KFbF/7Xi+OdmSgmuSvbbS2DPtmYFftlEg
3xsb+gfvt+gzEQtFHShI3vFzeuDf/vb0zNNxooDOZT7twhb8pvI8yY0CWw27
zTXYyZdFyQomBUXrzYauYy/xGZ36zKLgubVGTw728sF7yjq7KVgm9b4yGDu3
5HwNy4+CyJuiGV7Y8ryjTkn+FGjara2ywVae3HbkczAFqmLfe+Wxtfm/dCXG
UMDZvv5bLT6fVY+ehJTHUvBG4aviZexNcddEPsdRcLjB6VYitqlIiP7GFAok
qu3Kd/w731KLTn3KoeDZy2n/Llwv3rX9VBXOo2Bg0yeFWmyX3OaH2hfw8y6z
VzqHzVqdO5JQiPfDCSTjgR1AU7PVLsO/j9VoeoXr1dhPiW+eFRRUzDbPv469
/+ZERMJdCgwlXiUdw8YpLfpYh/dr8rN0PexEox3zE17g/PfO258Vhr90iLjX
9Z2CVYPz3mvh+hmU1Up/04vXu/Q0WABb7wNxpv4nBRaxpyLacf1t5AwdLBml
4MmthU8jsQfCKKPD/+Hv8xwDakMIxDi3Da2T4kD2+mXLlXF9//P1mubKFRyQ
rV0XPoLr/2MVwfzFMhzojlW0vIftXPrw8MQaDjyOzNOwxQ5/rGv2bAMHbB2y
NHxxP6ntV6jfs4UDCuvylx7H/Sde45AOy5IDXUJ/fayx7UM6C51sOPDkrpKG
MPaX/7Lijew5sFQ7ViwR968FEqLW4h4cuNsaIv+v/9noTjy/HcyB1+XPrrnh
/tgS2/h6+iIHIvJkbl3wxudnsuSKWiEHXLIdKqyxH/qdOsS+yoHJ532rxrgE
uunAUmso4cDwDUW+zdjHV08cz77PgZMun6GNwvNFtQLotnJgZUjZi+8sPC+M
hd8MEeLCM+2wzGQ3Akl7ex67IsrF9THgrQJ28nszj05xLjy1rg2rcCVQBBIT
3iLNheATFqNdLgRyTC3gLl3LhR6v8WIlPH8I0JtlbxtyYYPwmahsPM/4sVWS
hgO5cO30yKioLe736Yl+y4K54Gqpl3ECz0ev6wat9UO5IHFu8pIUtp78HcHY
SC6EaRfJyuL5atEHiJNO4IKOwjYfRSsCFTi5HTa6yIWWkMLMZVvw+bdMCUt6
xwV/h+pz6Zvw/lX/Ranoe0Otlf6mMTwfNn56KStt6A0zm1d4eGGbnrjWssDE
Gzp6zou8UMHn5Tfb8usWbzBOMFteoIzv/14zPc/eG/IyJL/brSNQp/nNUUkf
bwjZzY1MW43rB9P30FyWN0jxygtq8Dx7KPlTbstvbzBwcpVq5SPQsqy2YCba
Da1Rd9BfPL+PaI5cc4/2Ab93H/sgG7/vVIfxn9XzBVlO9zjDk4HKRoRnyuf5
QXbA2FjNSgZKq6y1t6jzgyPqxuv0W7TQG1q09a2kPVA/k3yFFaeFPNQ8L6Tb
7IWFjklj3/S0kN6aYukyAX9o9ar2v96niQ7WLtIoafaHO3FffQ+kayKBoSOX
FVID4CHrv8wYA0008Uyo1t89EDQPF6hS5RrobMPfmSjJIEAei9OSf6sj9qSw
RUxQEIgOnjSZNFRH72dkyMDWINBbN8+V5KmhcQuj4pyN+6C75+Nx1u0N6J6w
tOD3jH1gH5RzvfmXKmIU/CbkpvbBAjY58E5RFdnFfUtN38kDqNBbKepJR5Y2
qbY6LjzYq9I1meNGRyCmL9zpygPbluX3VHbRkVZW6jEVJg8Eo4r7TO3paFmh
fmQtxYPZ2Z7JMFM6+vAkzXcgiAfZPh+6O5XpyEfAcItVEg+ujMvlZwzTELuh
h38omQfHf9NXyw3QkFvKibqTqTxof3UltqiXhmylfhh8OsEDj7ntfPe/0JCG
UoZWaDZez6+q8dtbGprY0itfcBnHw7+xUr2KhoYFT3ZaF/FgCVVUWHmHhnpf
GOUOX+FBuGB/FJTS0Hunk1KbbmDf0+l2uEZD9znGom9u80BbzCYj+CwNla/v
awi7w4M7cmce/smmoZsDJ+PlKniw/oHPh9hTNHQhpG+e710cv+mr+pOpNJSj
l4nEqnnwuCEjRyaJhjJmjaPv3OeBrO5650vx+P0f9W1yq+XBgoaCafpRGoo9
mjn9tw6vVy4XfzuGhv4HR1oaHg==
       "]]},
     Annotation[#, "Charting`Private`Tag$22655#3"]& ], 
    TagBox[
     {RGBColor[0, 1, 0], AbsoluteThickness[1.6], Opacity[1.], 
      LineBox[CompressedData["
1:eJwV13k4VG0bAHBeRJYUkVZbaIjMHNkKd5ElSwplG2bOGSKEIUuWFlt2IUUU
KW0oUbTg+UpEKSpLZUslsqYsafue/prrd80159zPnHs78qT/Ho//eHh4JHl5
eP59Vu79NTNe9sbQcbpxpDiupi6x0a1rd1q1USjTLT4hOqc+4+3xiHVpTUZv
dV8pO0SX1Gd/zG7lT+sy8t+0yVYn+k59zkjB7FzqZ6OR+ynNUtGN9St8FZK/
ps4ZVaoW5N2L6qzfV8ZxmEgVhFaLH75U5FD9XGvcvbHUFZA3Pf9bInS2vnJ5
u1h88gaYCqDCvWwFUYCaVlvtFgZovE2957p5GZI2m8tultSFY2NWnG0J0uhb
7YoDFw4YwtSBu7LrZNegOPd1MqdVt4NQ9y5HoUw5VJrqHmPsvgPmff1FJFQV
0epwV9/5WHMInnq+q/OkErp89V1rfLAlsAXnwveXqaDnCYnVEcU2EFEq1xbx
nIaSOnpElZ7bAmHf2Bh3UQ21PX4ZudR4DxAdR06YWqmjj6IDmje67GBn7Y8m
9oQGSgjRKNLf7QCvN63Veq2siea0sx3Cv+yFDZeZg1SbJhLp7DLfGukIPCdW
7ttD0lH5adf50WknyKofNK/spqOlQmqxO344QcSbpWsy3tIRN+yH+Pm/TvCo
ffE9nx462uyUo7JH1BkYIob7ZAfo6MGqtr01Ss5gsm1gTdhnOmopML4d6+gM
nZHdi6Zm6GioWJW7ts4Z4oPshheWMdC6m/OjNokukHC+szrRlIGElWpUt6a7
QHR8gB2POQPN5oZ60065gLVF6MQhCwZ6HjM7xFfkAsfFMhXdrBgoet/39zU1
LhB/zy9dYQ8D9f2Z7FIYdgGVGJ/cCCYDnbP+/GjW1BWuMOU6/YMYaO1ox9lz
/EzQNU4S981nIE7tpcvCIkx4XRm0pq6AgUrTD1WGLGOC06JlIuLnGUhfS+qp
zTommDb6p5UVMdDeKPuFPzpMUP+5oNVbwkAZ4q8c3X2Y4PvUdotgBQPxa7VJ
yb1kwng4/9+EBgayXFQon9LNBJsItUd3HjNQZre/+nwfE1LSnQM/NjKQfJT4
jrZRJqgc7k3Z2sxAho02wUcF3KAp5UVTfysDhTq2vhzQdYNnEsYnpjsZ6Etk
S3rReTcwiUwWsRzG8TaeKp285AZBcX8r9oww0MGl7GaDUjcYOlNs7/SFgb4W
z/33tsYNqhMj06kxBppvWR8i8dINGpeEDvpMMdCilUdcY/jdofzF481W8wyk
cJugeXi7g76JvL21IIE+/vmzo9LfHU4ZKP/WEiJQiXkLyRviDpruntdWLyYQ
rYeVX3DcHXxk8iSGhAmkyZcm3nnWHQov9Mr5LyGQ4e7hGdPn+HqGln57pAhU
FmLDzl7JAqeO84nuCgR6VbDRIm4NC7wKaptWKRLoR4MwPUSWBdXcenoH9g7J
Jh5HJRZQM5BkpkSg3htGhavpLNgmM7dHYQOBxEY0+y+Ys8B9lWjgTXUC+blI
MitCWVD+KstGU5dAWce/mlw4zIKmupqD7dh3r77YmBXFgutt1v8L1COQwHzy
r+AYHM+53D839AlUkM2fr5vOguRf/v0KBgRqbZ15W1/CAvLTy/2D2wikDt2O
zztY8EDyA0/LTgLx5Bhe/tPNgtYq9S1MSwK9Hr04o9HDguiO2ORJ7MjTgZnp
gyzI7GT7L7MmUMuE8DPbSRYIP5G23LmLQJ4FBkavhNgg9N4tJcOOQPrfilP5
RNnwbTLaVMoen89CuIcQZ0NwxfNVudhV3zvDsqXYcCdGQPKcA4H4rAJuOSiw
4f6wkEXBPgIVLlxQ6t7ChhUmqwUCXQgUbLs4WMgIXw8Uj33GNivxf6i7nQ2h
l8JXM10JNLF7q3uuORtcimVKdzAJZHC144yzAxt26O8yEXUn0Nt9QqK9B9mw
cqNIkj9JIMnbftPvi9jgkf9dK8OLQBtTrVb1XGSDqPLSnx+xTTzUtndeZsMD
+SQ+PW8ChUiNnGwpY0OvpF9PH3b3IQ698i4bmiyqK+V9CHRO2yUgtp0Nyz3S
lWP9CFS9RP9M9Gs2mD6zV2vFbhuSQWFdbLD42HBI6iCBeE93ivv14vNHhfYU
Y3Pmdt9wGGGDX9yn2Wp/AqnWmE8o85LwRftZam0ggYwzVKTl+Uno8O8S+Int
6rXIcLUgCc701406XAKlyjSkiouRQDcIWn8DeyrMSH1ehgTdu7/sTgUR6I6e
tm+zJglVb15VGB0i0ItlUtmPCBIUyf3tgdjDI9/u12rj+0WpGxRjr8yrELm1
lYSvvXILfCH4+S9svJ5nTkLIsI14Lfa2+4pffFgkvGkSei0WRqAVu46u2kfh
+FwbRLWwxwd7dm73JGHQtuWsE3aucM51GV8SNu0Mrb2A/dVJyO9xKAllb4qW
q4cTqGmcU3DzMAmhI7/4bbALjv2v9WwUCWIXlKwPYltcPazBjSFhyKDoUyl2
0fzY5Lp0ElqlT2xVOEyg0BQLOeFMHF/a6SkDbGu5EtuZbBIy/WZ/O2L/MHOv
eJpHgnQLqZSKvft0OzeshIThAJ3ScWwVNY1i6ioJ+Q18mvwRBPpdl/TKppQE
pWvnl6zCvjpkrKV0i4TPjwV6jbF5te/MtNeSkC3Z9Cgdu6tZQrkWkWA8a6lY
hF3G9N975REJQvPr+iuwneI2VEc3k7BI8aBvO/amlXGfvZ+R0FBoYTiALVD2
foXDCxJKhuh+E9gVr/PC1DpI6FX9PCgUSaAEr7kr0t0kHDOXVJXCZv6ye8P7
joQBX+EXcthExs3F470kfJT+1a6GvXi9mH73AAkVdSsIbez+au8Djz6QUN2R
Mm2EfduyMa98iITcxqSlFtjsoCM/Y8dIuFrX5+WErSPYoxYwiZ9XeFYxC1vs
rK6ryzQJesFpBvuxP2icSjGdIcFn/o+2H/bdh18f0OdJCDNbnsHFTt9rM77m
Jwlm+b/NQ7E9vlxbK/QH54fqF3YE9pZoQZtvPBToyy1+F429TIIT3cdHwcUL
iVXHsD9fQuXNiyjY3Z43EYNdq7e2v2oxBakNPolx2Fmt4eKFohRUparFxWN7
szuNksUpkNVZPPjPRjOMgBAJCvQaiMJ/lkpML2RLUbhe3tb/+/3omrE2KxkK
hoLUtsVi/++mOa/uago2Ht67/ji2SZD6GXIdBTWCP5WPYD/ZLLEpVZ4CM91p
/3/xW83PPq5eT4Hqu9C/Idht9965DqpQMHC7qSMQ2z4KfRNVo2B57NpvPthd
RpeSdDRw/HNV+zywnf9LkifpFBA1zXxu2H0NB2tStCgQ5Zyec8AmE+x2VetQ
oJHuRFhjf7LQHXqvT0HdI8tqY2wv0bVRooYUTBy7GqOHPfacd7nONgrGjMrP
aGAHnBy6xjahYMr71KwC9je7p9tSzChQJvMKpLEXurP931tTUCw52vQT51v0
2fBForsp+OtWZjn+L7/d3Aq07Sm4nH94ZR+20AeVp8nOFLwuVsiuxU65JEre
YVIQXh60rRR7qdfX+QEWBUXqD/TysFeM31PW3k/BjbOyosHYeTfO17IO4Psf
vjnkjr2OG2uf7EeBbul6MUts5Tnr4wNBFISGXzCUxdbifd+bdJSC6Ai2fj2u
z5pHj4Nvx1BQyBtx+BL2lvhrIgPxFMRetxZKxt4uEqy3OZWCk6lCS+z/1beU
4Kn+XAqeaes96cX94nXXqJpwAQVPXxyNrMN2zGt7qFVIQeBD+6PnsFmyeVOJ
JRTMJySFumIfpKlbaVVSsEk4UbUN96vp0WUf3O5QEKSZzr6Ofah8NjzxLs5P
4+mROGz8l17uq6dArvzOpC52koEdX+IzCtLvJ3XkhOIvd4ff6/1Ewdu41q0M
3D8DcjpVXw7jfJj53iWArfuOONs4SsHNTqW+btx/WzgTETe+UrDlPXNjFPZY
KGVw7DcF96f1O+qCCcQ4Z43WS3Fwv9t4TBn395+D1zRXynBgintxcAr3/wYV
oSKx1RyQfLn41j1sh4qHx2blOGDca3/WCjusQcf4yUYO6Dh+zffG86Tui3yj
jwkH0nJ3x57A8ydh0xFtlhkHTh9f/dYC2za4p8R+JwfEjpcXCmO//52TYGDL
geajn44m4fnFv0zUQtyVAw0NqZkxeN7t1Jl9eiuIA+MkU8EFz8eOmJb2Hxc4
kJQyqFHkietn7sYV9RIOhGqe2bwT++GBU0fYVzmg6XMzb9qDQOW7WerNNzgw
E/zl6DbsE7KzJ8484EDfQPmjLgrvF/flQaeTAzmORXZDLLwvTIeVBy/2gEbT
McVUZwJJe7rFXRH1gLqXBykF7JQ3xq494h5AU7QUqnYiUDhaImwi7QFna8eO
9zkSaE/aRQ9JRQ/Q6X65TRnvHwKqbWtubfWARx0/pHLxPnOArZI86e8BUTMF
WWJWeN5nJB1YHuQBwhsjtDLxftReP26hF+IBKn5tptLYuuuqhGIiPYDLV4bW
4P1K8B3ESyd6AF9hxRJFcwJdtHc+ZnDBA2Tp74ykTHD9m6WGJr/2gA2jPXYn
t+D81fhGqeh5Qh/bT+Ab3g9b+p+vkd7qCaXzk8os7O0nr3XwG3nC2zOru56p
4Hr5zjYbNPEEf0uhjxeV8fnvtakW2HqCR59f1a71BOrZUf5VwssTTh77a5sh
i/sH0/vInxxPqGhcHluH99kjKf15Hd89YYRvv0gXD4GW53QFMdF+kJNwH+d5
zkBTmlPXXKK9oLA8wXb7Gfy+cz+UN1/XG/ZFWeZruTFQ5ZTwwu3/DoBXQvJQ
/UoGSq+uszWtPwAbsi7u39JBRy9p0RY3k31geRrNkoqnI1d1t8KMnb6APlCz
Q7p0pCtXJl0p4Ad/PrR1l49ooog6wU032vxgdFe/dXSGJhKYOH5JPu0gMAa0
p2P1NdHsk8V1fi7+UMor+9f39iaU3/x3IUoiAOiprSdOf9dA7Dlh06MBASCj
tsyVz0ADvVlYTfp3BoBJNuOhP1cdzZgalOVuDoSsV491/W9tRPeEpYU+ZQaC
8nD2tYFvaohx8Tuxdj4QzGgr9g8pqCGb+A9pGXu58DhkiYCsmyoy25lmpe3I
hbCF7V9KnVURLNET7nHiwokXSyr196kiek5anAqTCzp8LZMOtqpoeYleZB3F
hX2pLjLJ21XRu8fp3mMBXHh/h9CfUlZFXgJbTcyTuXDXU4RdMklD7OYh3okU
Ljg/afmkOUZDzqkn67PSuHBW+pft/WEaspL6rN9/kgudzmLvXrynoU1KmfSQ
M1z4UrYXzb2ioVmT4XUXL3Ghob9pcHsNDU0KZfVYXOaC3anf3U+raGj4mUHe
5BUuWOTzV9tX0NAb+yypLaVcCNfvVfW8RkMPOIaiL29xQWCR1PeEfBq6vWGk
ObSKCyOv6GpLc2mofCwrYe0dLnC2P9t55hQNFQaP/Od9lwt7jrwwvpJGQ7m6
2WjJfS6kzZJrNZNpKPOXYXTVAy5IsJr7qxPw+z8a2eJcxwWFhRXJRrE0FBOb
/eNvPRdUFyjZpqM09H/hhBcx
       "]]},
     Annotation[#, "Charting`Private`Tag$22655#4"]& ], 
    TagBox[
     {RGBColor[1, 0.5, 0.5], AbsoluteThickness[1.6], Opacity[1.], 
      LineBox[CompressedData["
1:eJwV13k4VF0YAHAiW0S29IkQMbQwV6Vsb2UPISQMM/cOWbINWZKlsnzZQ4oi
lRQRomjjlCJaLGWplKUSCVGWfKXv9Nc8v+feueeeOe82imSAnccSLi6uldxc
XH8/qx1/zYyXvzbYN900eim+rv5Ek1uPbVqtYTjDLSExOqch482xSPm0ZsPX
Oi/XOUQXN2R/zH7Om9Zj6L9pk83W6FsNOaP5s3Opnw2/3E1pkYpualh5UCl5
KnXOsEY9P+9OVHfDvnK2w0QqP7SZ/zxIHRlumHsef+dr6krIm57/LR4221At
2SGSkKwG1wKoCC8bfhSood1+X5cO1qWpd1w3r0DSpnPZLRI6ELrSnL0jURp9
v7/S56KPAWz/cGKN/JrVKN5dXua0+k6A6qp9ApkKqCzV/fgud2NIo/MIiKuv
RbIRrgfn48wgtTZ1R/dJFXSl5O3zhJDd0Bh9xfJAuSp6kXiiNvKSNRgr5plG
vqChpK4+YZUXNtB8eB8nrkgDtT/uPCK2yw6S1WbTdlluQB+FBzQrevbCGXVR
A5eJjSgxdOOF7bYO8KC0qOf5Ok00tyXbIeKLIyiSxPl97ZpoWXePmd4RJ2i2
VrLQI7XQ9dOu82PT+2Gw+unrtF4tJCagEWf8cz/cTTnG9H2jhTjhP0XP/9kP
K/Ojq0z6tNDm/TmqdsLO0K2rUv2zXwvd+6fdsU7FGRgrzHVtP2uh1vxdN+Oc
nMGiTSqjaUYLDV9S58jVOwOPmNXrpyvoSL5yfsz6hAvUnJrMtjKhIyGVOnW9
dBc4rOvzqNGUjmZzw7xpp1xgMqxqWsecjl4cnx3mueACESnelgqWdBS978dg
XZ0LbPZ593PIlo7eL072KI24QOWqwQM6DDoqsPrcOGviCkOOvV+Ug+lIbqzr
bAEvAx52L4sRPUdH7PuXrwgtYwDX7l8fmfl0VJZ+qDp0BQOcXpRqVBXQ0XZt
qafW8gzwAxNX6wt05Bhlv7C4lQESoTm2kcV0lCH60sndlwF87JuPz1fSEa92
u5RCJwOuPXIukHxER7v5ChVTehlA+tfm7XxMR5m9ARvm3zPgEIsnNqCJjhSj
RI3bxxgguTaIr+kJHRk0WYfELnUDfbd3gp7P6SjM6XnngI4b+N/oUuZ009GX
I63pF867wQhNP/LeZ/y+TafKJi+7Qd3EkE7jCB35i7Fa9MvcYOFb/NSTUTqa
ujS35E2dGwQ+aLDvGKOj+VblUPFON6C3fB7tmqQjvlUxrsd53WG6QC/h+hwd
Kd0kaB7e7vB9p8SO83wE+ri4aFwd4A7S7mW98fwEKjZrJblDsYXUgn0FCETr
Y57LP+YOlRqPqgghAmnypIl2n3WHM9ciXetECGRgOzJj8sIdRqIszmdKEqg8
1JqVvYoJB+YyTqUoEuhl/nrz+NVMWCzVLTVRItDPR0JaoWuYcPVl5OgfbGOJ
Zi4nFSYoLEsaCVAm0LsKw0JZLSbw5R2ZMFYlkMioZv9FMyYUZ18zaV1PID8X
CUZVGBO09Y+mb95KoKxjU0YXDzPBXtLBuQv7dknb+qwoJnw5ouYYokOgpfPJ
v0KOM8F1IG+wYhuB8rN5z+mkM2E8y9RKTo9Az5/PvGkoZkLrdEJRBxBoA/Q6
vehiwps2x7oL5gTiyjG4stjLhMJz+paEBYFejRXNbOxjQui0w49G7COngzLT
h5jw7K78saHdBGqdEHpmM8mEAS+1s5LWBPLM1zd8KcCCuvet/1naEWj790up
PMIsqI1Vn2rDFjEX6iNEWeBT07xou5dANT+6w7OlWOC96T61155APJaBNxyU
WCAwfclltyOBChcuqvTqsiC38amumDOBQmwEQwQMWSDPt+NlHLZpccBDnZ0s
eP97IWEee8JWzz3XjAVKqwyM3rkQSL+k64yzAwtGJPnlzjEI9GafgPA7fxYM
3X4QM8kkkMRNv+nBCyz4tyixZcKTQOtTLf/pK2LBhrLy5B0HCGTkobGz+woL
srx3pGVhh0qNnmwtZ0F7RazDZi8C9R5ia1XfZoHiGM90gDeBCra4BMZ1sCAq
a2vGA18C1S7ffib6FQt+DXgECRwkUPuwDArvYcE5+e051tjcp7tF/d6xAOou
XOvFZs/ZVjiMsiDcXHDZRz8CqdeZTazjJiGfxtfSE0CgXRmq0oq8JOihnF/i
gQRy9eIzkOUn4fDQn1Ar7FSZR6miIiQUXlTdgbC/hRtumJch4U6Zm2Z+EIEE
beUdpmVJMPIwLuzEVqL9PvJVngTt+2ed+DkE2vv6zrMBZRIuM8lL/ti3tm05
2KJJgl3Fh2LtYAK1rZDKbiRISGp+6c7GHhn9fvf+FhLy+FvILOxVeVXLbuiR
kL071XQS+8jC+mt5ZiTYZPNkFoQQaMfdtV98mfj6sWbHt4cItHJP7D/7KBIU
DHXE/2CPD/VZ7PQkYfFVs6JSKIFyhXKuyRwkYbCQy8ATe2q/gN/jMBLUxpYE
DmM3j7PzKw+TYNaW3cEbhuP96IPnZ6PwehIN/yphm5cc3sg5TgLFnzvvgn1h
/uukfDoJHLvED03YYSnmCkKZJLRKcs/1Y1spFNvMZJOwRz2ZNY/909S96mke
CU9eJOuphuP9v707eCsfn4cIs1wf+3KAjPjFQrz+nz+H9mLbnu7ghBeTcEjC
TTQKW1Vj4yWqBD+/KmIgA/t3fdJL6zISri7IChVhlwzv0la5QUK0bsWBJ9jc
W27NdNwnoaCLZisYQaCeFvF19xH+vm322ErsckaA49VGEh5oLPSrYO+PV6uN
biFB91VQjyH2plXxn72f4fOIGXizG3tp+eBKhzYSPHbybtuHXfUqL1yji4TO
KGW+g9iJXnNXpXtJsM6POnQIm/Fr72vutyRMKxpDNDaRUSk4/o4EZesSzwRs
QWWR7b0DJKQwekdSsftrvX0aP5DwI46rORv75u6mvOvDJFhN7+E+i53cr/Q0
d5SEymc/Thdis4Jj/ov7iuNJWy75MvZW/j6NwEkSEnbOvSnBFjmr4+oyTcIN
warEcuwPG0+lmMyQsO9U+MlK7NsPp+5pzZMg9CVy/gZ2uqP1+Or/SPBbOnqv
BtvjS6mcwCIJsu/H39/E1o3mt/7ORUE7Ved2C3uFODv6PQ8FEBOq99efL6Pr
LXwUrBZ3DP97//1tcv01ghRIzcWJ/31e1vMI0UJhCl5xay37u543q9swWZSC
hcVEsgLbcIYeGCpOgUJNrUwZttSJ9EKWFAWof3zDVeyx1V/bLWUosNjmdPES
9oNKM24dWQqkg5RDC7CNgjecIeUpEC9XUT6D/WSz+KZURQrWdqRJncS2nJ99
XKtMAVM6z+IEdvudt65DqhT8uHa0MRbbPgp9F9agQK02Jjbsb7wYXk7aupEC
s70vjvphv3/kX5eiTcFohLHd3/MnE/fuqd1KgZ7gkOLf+PhkrjM8uJ0CZaJ2
iwH21xfcklt34N9jelpTCTvw5HApy4iCNt3n0hLY3/c+3ZFiSoHVieadPNgL
vdkBg1YUTNB4/Adx/EafjeATtsUeqPVr+xvPbm75W+wpIKngmnvYAh9UnyY7
U1Ci9GnlKeyUy8LkLQYFi0HLN8dii3lNzQ8wKeioUs7zwV45fmfdlgMUHKr9
rfc33/Iqzt9n+lAwrk9EqmDLc+Lsk/3w/rfoLhHBXjdndWwgmIKp5Ctjr3H+
anMPvkuKpUDuPzrdF7uu8XHIzeMU1MTr37fC1k0oXTaQQIHGqQ+Zm7B3LgvZ
tjmVgkq+YfkpXF9spfhP9edSIGb6q8EX+1XPmIZQPgU69rLFZthOee0PtQsp
4HI716uMzVyT9+1EMQUpb4vX/q1v/rQNltrVFMw7CzsZYk+PrfjgdosC42Cf
K9LYh67PRpy4ja+7ThiN4/p4hEBX3jdQ8O2Rme8Z7CT9vTwnnlFgEOznO4zr
6RXbiDvvPuH3D47xYeH6HJjTrd45QoHwzHpNLWydt8TZpjEK0pdwu3Fht7In
IiumKNie1DF9Dtf7r2GU/tHfFPya5eFrw/2BXmCFlKXYMOkttiCN+8t/Q6Wa
q2TYELpotO+dP4EeqQpcEJFlw3RUwJpL2A5VD4/OKrChc8ppaj12+KOtu56s
Z8Orh26F23C/qv+i2ORrxIZcubV2W3H/S9wUs4VpygYNsZzgHz4EsgnpK7a3
YIPo+OMlVdiDv3MS9W3YcP23sK8aNu8KYXNRVzaseyzkJYb7qcXW2ac3gvH9
lrrbH+P+3HW8tePnRTYcvsQKamTh/JiruLqhmA3pCtxRB7Af+pyKYZWwwTDO
4IMQ9nVb5oaWCjZ8svNHe3C//3fN7L9n7rGBqi1o7HDD88ldRdjazYZbsVxy
tXheKJwOvx4i6AHupganBRwIJO3pFn9V2ANK6r+7n8HzScrrXa59oh7wqkEo
SRU7Ai0XMpL2AOWrdB4jPM/YpRV5SKz1AC+WXvohW1x/1dtX39DzAM/pC3p3
rQjkw1JNngzwAEWfREanMZ4XMpJ8JIM9wE4lQNEWu6Nh3HxbqAcIFLfatRnh
85SvETh+xAMcFgsXW3YRiP8tJEif8ACpWuXYuh0EKrJ3Pqp/0QMk1mo6HNbH
+W6aGpb8ygO0KL28TG0cvxu/U6rbPCFtsIpbAc+nrf0vVkvrecJy2feVCQo4
3k+WdvEaekKVxccvX9fgfPnBMh0y8gRlW0muOnm8/zvt6vk2njAesqrabDWB
+oyvT4l7eQLHc4+r/UoCeTG8YxZzPEHez7VeCs/HMSn9eV0/PKFP+597Znj+
lszpCWagAxA+8nTO9CEdfdP8VuoS7QXtfrSqbUn4/9LdMO5zOt7AVNQYKLCi
o+pvQgs3l/hANP1WsygfHaXX1tuYNPhAa3Zzml29FuqkRZtXJvuC5kypVYGv
FnLd4FaYYXEQkq0EL6//RwvpKJRLVy/1g6bh08H3mjRRZD3/pop2P6CfYojk
eGmipRPHLium+cOwqHJAgYgmmn0iWO/nEgAylgcfcNtsQuda/ixEiQcC72dr
hdljGxFrTsgkNjAQYvcE+5k0bECvF2TJgO5AKHyicOPp8Ho0Y6Jfnrs5CDK0
FE1kVq1Hd4SkBT5lBoEkq/N2kKUGohf9IOTmg+AH024oyFcdWSd8SMtw5EDG
Lj/ZZadpyNQizXKLEwdSbDtbbbNoCJZvE+rbzwHJUZrtmXQa0spJi1dlcEDs
gsQH5X9pSLJ425F6igNxpcfl9SJo6O3jdO+vgRxY/W63IOVCQ15L9YzMkjnA
pbvHKWsNDbFahrknUjhQZG4k1SVLQ86pJxuy0jjA5qaXScvQkKXU5+39JzlQ
+NrBK1eMhjapZGqFnuFAJditzuemoVmjEfmiyxwoa8lNzP+ghiYFsvrMr3Dg
kbzMZF+/Ghp5pp83eRWv946XvrpPDb22z5LSLeMAb1e8Rd4rNXSPbSDceYMD
HzNLnmQ/VkM31UZbwmqwLdcsf/lADV3/mpUod4sDv8TublpRr4YKQ0aXeN/m
gNqnBv7UW2ooVycbLb/LgZFQx/rWG2oo85dBdM09DnyV8rcVqFBDSWhU17me
A0/85B4YX1NDx+Oyf/5pwPtRjBQ5fkUN/Q+1ICV7
       "]]},
     Annotation[#, "Charting`Private`Tag$22655#5"]& ], 
    TagBox[
     {RGBColor[0.5, 0, 0.5], AbsoluteThickness[1.6], Opacity[1.], 
      LineBox[CompressedData["
1:eJwV13k4VF0YAPCkIpHsiogIkZhrL7yyF0rWrDP3zthKNPYWla3sRCpFWpCy
FFlScdp8KJKyFYmKLFHJ1sJ3+mue3zP3ueecOe82MmTAXtbSJUuWiHEsWfLv
s8Lxz/TXkh4D5x8NI9dia+riGzy6bFOqDUPdPeJORWbVp72NOiKV8p/hW53X
mxwiC+ozP2W2LEvpMgzYunWPdmRVfdZIzsxs8rDhyP2kJpHIhnqxA7KJ35Nn
Dcs352TXHuusdyphOkwkc0Gr5fwB6uhQ/WxLbO14shhc/DH3VzBspr5C+BVf
XKIilAZQET57uFCgskbbw200sLqZXOumKYBEzWczm4R0IFjMkml0ShRNPRTz
u+pnALof46WlpCVRrKeU+LnNO2BHxR0n7jMbUHGyZ7SxpylconFyC27eiCQi
3A7MxVjAeHWyUWe6PCosetcSF7wLTp8otPIuUUCtp+Krj1yzAUOlbPMjrUoo
oaOXV751D7CznNgx15VR27P2o2uM98LuIzMpxlZb0CfeD2plXXYQJrnGwHVC
FZ0KVb2iZ+sA3J35XS2b1NCsVqZDxKgj2OprXXZqU0OrOrssth91hleFiju3
k+qo9Jzb3NiPfWBk1t2T0q2O1nArx5jO7wMB41T6/rfqiB0+z395cR/UhSXe
MetVR5r7shT28rrAFjqtYr5fHT1Y1+ZYI+8CB1sct9kOq6PmHOPKGGcXGH0h
l9YwrY6Grm1mr69zgbH3Hj3PBWhI6vbcmE28Kxiwuc9am9EQj3zN5u2prjBi
H/30iTkNzVwI81U66wqNrc0/dCxpqDV6Zojziivc8Iy22mBFQ5FOPwdqalzB
bvvc/KAtDb1fmOyS/eIKEZwL3jruNJRrPfxkxswN/vbNj8oF0dD6sY6Lucvc
4UGiznH+SzTEfJhfyLPKHTr8lT7Tc2ioODWkIlTAHb55divfyaUhPQ2R5zZS
7mBXHuxmc4WGHI/Z/1rQdoeWigbbIwU0lMb/2tlzvzvc9R55dvk2DS3TaBPZ
0O4OaWvP5Qo/paFdK/JkkrrdIcv2Z/aOZzR0pjtgy9x7dxB9AycCGmhI5hi/
aduYOyxWl61oaKQhgwab4BPLPeCSqRSPVwsNhTm3tH/Q8YCPYRLy7E4aGj3a
nHrlsgdE5CYfeTCM99twtngy3wO2i2roPvlCQwfXMJr0iz3g2Yuu740jNPT9
2uzStzUe8GqlkMOrMRqaa5YLFWz3gPW/9Uc7JmloxdrjbtHLPMF4+Hxc6SwN
yVYSSixfT3j25qjR5RUE+rSwYFoR4An17aI9sVwEKrBoJjlCPWErIyNoPzeB
lHrpl3KiPCHBRr2c4CGQGmcKf+dFT7gfMe5Ww0cgA9sv02atntA49fjyGWEC
lYTaMDLX0kFTaF1WkgyBXueoWMZK0kGg9dlNM1kCzT/lUQ+VpkPB4orRRWxT
of+WOMvTYY2N2EiAHIH6ygzzJNTpwJJePWmqQCC+EbX+qxZ04JsyNW9WIZC/
q5D7nTA6xJaqpmlqEygj6rvJ1cN0kPmP07UD+17RS5WMY3SQC+p2DNYh0PK5
xD/B0XTwp6wHy3QJlJO57JJOKh0eWyxar99OoJaW6bf1BXR47m+Z/woItAW6
nVs76DAWpHbviiWBlmQZFC5000FtWNya2EmgN2PXp1V76aA9RJt+gn303KEz
qYN0EONZjBrcRaDmCZ4Xeybp4JjMf0nYhkBeOfqGr7kZ8EUL/bHaSyC9qWvJ
nLwMcC6W+fESm8+Sp5fgZ4B3FVq0tSPQ3Z+d4ZkiDFgYuse0sycQp1VguYMs
A7J1brjtciRQ3q+r8t3bGFBV2799jQuBgvesDOY2ZIATh9ObGGzzgoDHOjsY
4L5E6PQc9oTtds8LFgyoI1xM+1wJpF/Ucd7FgQEhccpSl9wJ9NaJm7fvIAOK
wmZPTNIJJFTp/2PgCt5v2mDzhBeBVJKt1vVeZ4DLB55kI28CmbCUd3QWMqD2
S15qBnaoyEh6cwkDbrZ+ctT0IVB3CFO94h4DogIPTQX4EihXyzUw5hUDSmNr
0h/tJ1D1ar3zkW8YwLVnhM19gEBtQ+IovIsB03zonA02x7lOfv8+BqSWq5R0
YzNnbcscRhhwLjqX95M/gTbXWExs4iBBK+V2c1cAgYzTFERllpHAfmu8IBhI
IDefFQYSXCTMVpaFW2Mniz9N5ucjoWmqdwfC/hZuuGVOnIQ5eWlaziECrbSV
cvghQcL3O9xX27Fllf4eHZciQXyA4cLFJpBdT+2LD3IkBBqo5h/ErtLVOtCk
RoLM1vs3NIII9FJAJPMJQcJ53VIGE/vLyNT9h1p4vYACZgb22uw7q8q3kzB4
K9ByEvvoL5Vb2Rb4eeGpjNxgAhnd3zi6n06C7fI253chBBLbfWKdE4W//2Qs
vIj9dbB35w4vEjSvdG6UDSXQBZ6sW+IHSKhuEAEv7O/7uP2fhZHAMy3HHsL+
7ysz5/ZhEgIka18vC8PxfvJRy8VjJHwqHE6QxbYsOqzKjiZhl3bjL1fsK3Pj
k1KpJNiPPfncgB2WZLmB5wwJUYJG8/3Y1hsK9kxnkiCZ3krNYc+be955nk3C
NeFOA4VwfP539weqckgIaSop08fODxAXvJqH70PTNtwO2/bcK3Z4AV5vV5XA
MWwFZdVrVBEJvIc6BtOw/9YlvLYpJqHc9AjvdeyiIWMN+XISPG+J+DVic2hV
Tb96SMKVp7l2KyMI1NUkuOkhIuH1GO+EGHaJe4DjjSd4/yGhg/LY+2IVqyOb
SEhKmO4xxN66NnbY9wUJG6e8+3ZhLy8ZEHN4SeL+lrrNCfvOm+xw5Q4SCk2q
uQ9gn/KZvSHaTUInIRwegu3+x66H4x0J7Un9OyKxibTbK7/2kbD6jLlvHPZK
OT697g8kqB0/PJaM3V/t6/fkIwnc8QVNmdiVuxqyS4dISO6b57yIndgv+/zC
CAlvr13NzsNmBB3/HTNOgsKf1uR8bG2uXuXASRJeLhb3FWHzXdRxc/1Bgv4j
v4QS7I+qZ5PMpkn4uUsr8zb2vcffH6jP4fdf1/9djp3qaPNV8jcJRY2l9Xex
WaM313Mv4HworR6oxN4WyWUztYQCFfM4RhW2gCAz8j0nBYsRFob/PJyPSptW
UKCqpHLk3/MPddf3311JgddWT5F/78toieDP46XAlc6/+t96voxOw0R+Cm6f
9mOVYRtO0wJDBSlY8M+VKMYWiU/NY4hQ8F9rt9oN7DHJ8TYrcQpiSfP8a9iP
bltw6EhQkNQjFpGLbRK05TwpRUFd1XqF89iNmoJbk2Uo4IhKFE/HtpqbeVYt
R8GB4IvW8dhtte/cBhUo0Ht4quEEtv0xNMWrTEHxyYTosH/xYpifoK1KgWxf
X4w/9vunB2uSNCioyvRw+Hf/5Cm73dXa2NOLcv/i47OlztCAHgUBsz26Btjj
rRzC2kYUXAuX1pDFDkwfuskwoeBF8cJaIewpu+dGSeb4vKN/TTmxf3VnBgxY
U/DxuPGhARy/kRcjVvDaUhCp9zfw5b949vDI0bKnYLjhYfUDbO6PCs8TXSjY
VqIrcRY7KZ+XrHKnoGatj84J7DU+3+c+0CmQPhad44ct9rV2k5Y3BS59XvAv
37LLLj+k+1EwmH0lUh5bih1jn+hPQUVb6XI+7E2z1lEfgihgVspP9uD81eAY
6Es4QUFveoPmfuyaJ8+CK6MpOH66E1ljb4u7uepDHAX3eKKytmLvWBWsq5lM
gWBoqux3XF9sRbjO9l+g4O/v+0/2Y7/pGlPmyaHg7q0PRRbYztltjzXy8O/h
4d0rh02Xzv4WX0DBIZNjCv/q20GlLVYaFRR8Gp53NcT+MSbw0aOKgs9v3W+J
YoeUzkTE36PAv2DY4iuuj0cJVPi+noLEYeuA89gJ+nac8S8o6MhNCBjC9bTQ
NqK27zMF6QKtBxm4PgdmdW5u/0JBcuhJDXVsnXfExYYxCnYcdCWXYDczJ46U
fcfx8F579hKu9+NhlP7JvxTM+kXxvMT9gZZrjeREmJDPQAuiuL/8Hryptlac
CV6mv137DhLoqQL3FT4JJiyTUJG7hu1w5/HJmQ1M+LZbdkYFO/yptnGjChMm
ZozydXG/qhuVadhvwoRJ221O2rj/ndp6XItuzoT+ZZXhP/0ItCe4t8B+JxOo
ojGuO9gDf7NO6e9hgrQnBCpiLxPgteR3Y8LXxn3+a3A/3ak987w8iAk/5h8b
PsP9uSO6+dX8VSb4M+lhTxg4P2bLbmwpYILENu5ob+zHfmePM4qYUMdhM8KD
XWpL39JUxoSC8pSG3bjfn5aeOX3+AT6v9UDTKw88n9yXAe1OJnTujd9YjeeF
vB/hpcErWRDO6ZrL7UAgUS+P2Bu8LPjLv877PJ5PknqM3Xr5WVB7Wy9dATsC
reYxEWUBezaExwTPM3tTrrOENrLAd6wgK8QW19/NbZLl21ng/c3N5L41gfwY
ComTASwQiBljtZvieSEtwU84iAVcf/uUbLFf1X+11A1lwWEzE9eXJvg+pe5y
Rx9lgZetGlezMYG43kGcaDwLin72n64xItB1e5eT+ldZUG1r6nFYH+e7eXJY
4hsWzEuuvn5GA8ev6hSloOsFCnIyfBvwfNrc3yoput0L5FVdHsRtwPGefrNj
maEXFOr6z4xL43z5yTAfNPGCZeuqV9VI4fPXtm3O2eMFqke+1VlIEqjXtPS7
oI8XVAql+9iLEcjH3ff4QpYXPN159LkIno+PJ/Vnd/z0gl9JEs8t8PwtnNUV
5I68QWcse5XFYxr6pvbtpmukD6jxhjTrJuD/S/fDOC7p+MJyiS+LudY0VPGN
51flUj94pNcwyb+ChlKr6/aY1ftBLHuhfm+dOmpXirS8nbgf2hmhCbn71ZHb
Fo+8tJ0H4GCU44TKOnWks6FEtGK5Pxz41df8oEENHanj2lrW5g/LdbpCsnzU
0PKJqHyZlIOwUrhyJJdPDc00rqzzdw2AgaKgwaV7tqJLTYu/jgkGwudJr0Oz
UaqIMctjdiIwEEgxjm/m9VtQzy8JMqAzEAwTTge0DKmgaTP9kguah+Cc6CnD
dWtVUC2PKPfnM4fg64bBH0FWyoh2/Sexfu4QZAwvsIL3b0Y2cR9T0hzZEC66
dJTvnBIy35lipeXMhrrdj7LtM5QQrNbl6d3HhuiIINmLqUpIPSslVsGdDVKJ
QtUKp5WQcIHu0TqKDWWS07MGEUro3bNU3/FANjhXV3xluSohn+XbTSwS2fCU
8X1vlrQSYjQNcUwkseFwjLVAt4QScklOr89IYUNH9dWiteJKyEpkWK8/nQ2r
6rJ8Lq1RQlvlz6iHnmeDkJuObB6HEpox+SJ1PR+v97jvfN5HRTTJndFrWcgG
+YImjg/9iujLC/3syRtsSHaRM5PuVUQ99hki24rZYB8axch5o4geMA1428vZ
4LSP9fncM0VUqTjSFHaXDXofdql0PlJEpeMZp9ZXsYG3x3m3cJ0iygseWep7
jw0sG6PNaVWK6IJOJlp9nw2JVjsHW8oV0Zk/BpF3H7BhtP5N6KoyRZSARra5
1LFB0H522OKWIoqOyZxfrGeDRHGjZlyhIvofWUNFqg==
       "]]},
     Annotation[#, "Charting`Private`Tag$22655#6"]& ]}, {}, {}},
  AspectRatio->NCache[GoldenRatio^(-1), 0.6180339887498948],
  Axes->{True, True},
  AxesLabel->{None, None},
  AxesOrigin->{0, 0},
  BaseStyle->{FontFamily -> "Arial"},
  DisplayFunction->Identity,
  Frame->{{False, False}, {False, False}},
  FrameLabel->{{None, None}, {None, None}},
  FrameTicks->{{Automatic, Automatic}, {Automatic, Automatic}},
  GridLines->{None, None},
  GridLinesStyle->Directive[
    GrayLevel[0.5, 0.4]],
  ImagePadding->All,
  ImageSize->{432., Automatic},
  Method->{
   "DefaultBoundaryStyle" -> Automatic, "DefaultMeshStyle" -> 
    AbsolutePointSize[6], "ScalingFunctions" -> None, 
    "CoordinatesToolOptions" -> {"DisplayFunction" -> ({
        (Part[{{Identity, Identity}, {Identity, Identity}}, 1, 2][#]& )[
         Part[#, 1]], 
        (Part[{{Identity, Identity}, {Identity, Identity}}, 2, 2][#]& )[
         Part[#, 2]]}& ), "CopiedValueFunction" -> ({
        (Part[{{Identity, Identity}, {Identity, Identity}}, 1, 2][#]& )[
         Part[#, 1]], 
        (Part[{{Identity, Identity}, {Identity, Identity}}, 2, 2][#]& )[
         Part[#, 2]]}& )}},
  PlotRange->{{0, 300}, {-19.911157024219154`, 0.}},
  PlotRangeClipping->True,
  PlotRangePadding->{{
     Scaled[0.02], 
     Scaled[0.02]}, {
     Scaled[0.05], 
     Scaled[0.05]}},
  Ticks->{Automatic, Automatic}]], "Output",
 CellChangeTimes->{{3.741410202833365*^9, 3.741410229523147*^9}, 
   3.741410324175556*^9, {3.741410385503212*^9, 3.741410397437392*^9}, 
   3.741410464346018*^9}]
}, Open  ]],

Cell["\<\
Where the errors between the two same order of the Pad\[EAcute] approximants \
increase with the value of kF, but are very low for the order 6 and above.\
\>", "Text",
 CellChangeTimes->{{3.741408500229847*^9, 3.741408530990829*^9}, {
  3.741410537064831*^9, 3.741410568017324*^9}, {3.7414106024652567`*^9, 
  3.7414106461993647`*^9}}],

Cell[CellGroupData[{

Cell[BoxData[
 RowBox[{"Plot", "[", 
  RowBox[{
   RowBox[{"{", 
    RowBox[{
     RowBox[{
      RowBox[{"(", 
       RowBox[{"1", "-", 
        RowBox[{
         RowBox[{"(", 
          RowBox[{"ExRCPad\[EAcute]2", "+", "ExRBPad\[EAcute]2"}], ")"}], "/",
          "ExRCBPad\[EAcute]2"}]}], ")"}], "/.", 
      RowBox[{"{", 
       RowBox[{"c", "\[Rule]", 
        RowBox[{"137.036", "/", "kF"}]}], "}"}]}], ",", 
     RowBox[{
      RowBox[{"(", 
       RowBox[{"1", "-", 
        RowBox[{
         RowBox[{"(", 
          RowBox[{"ExRCPad\[EAcute]4", "+", "ExRBPad\[EAcute]4"}], ")"}], "/",
          "ExRCBPad\[EAcute]4"}]}], ")"}], "/.", 
      RowBox[{"{", 
       RowBox[{"c", "\[Rule]", 
        RowBox[{"137.036", "/", "kF"}]}], "}"}]}], ",", 
     RowBox[{
      RowBox[{"(", 
       RowBox[{"1", "-", 
        RowBox[{
         RowBox[{"(", 
          RowBox[{"ExRCPad\[EAcute]6", "+", "ExRBPad\[EAcute]6"}], ")"}], "/",
          "ExRCBPad\[EAcute]6"}]}], ")"}], "/.", 
      RowBox[{"{", 
       RowBox[{"c", "\[Rule]", 
        RowBox[{"137.036", "/", "kF"}]}], "}"}]}]}], "}"}], ",", 
   RowBox[{"{", 
    RowBox[{"kF", ",", "0", ",", "300"}], "}"}], ",", 
   RowBox[{"PlotStyle", "\[Rule]", 
    RowBox[{"{", 
     RowBox[{"Green", ",", "Purple", ",", "Blue"}], "}"}]}]}], "]"}]], "Input",\

 CellChangeTimes->{{3.741168670979035*^9, 3.7411688252008953`*^9}, {
  3.741321842616331*^9, 3.741321854663926*^9}, {3.741321907976462*^9, 
  3.741322007351549*^9}, {3.741410258516222*^9, 3.741410259753636*^9}, {
  3.741410720317428*^9, 3.7414107322885313`*^9}, {3.741411449834115*^9, 
  3.741411451785789*^9}},
 ExpressionUUID -> "bf8397c8-5348-4031-901d-01845368c763"],

Cell[BoxData[
 GraphicsBox[{{{}, {}, 
    TagBox[
     {RGBColor[0, 1, 0], AbsoluteThickness[1.6], Opacity[1.], 
      LineBox[CompressedData["
1:eJw90nk8VN0fB/BJHiRZE8ky1oQkIXnmfI1diR+VXVlSlpRIolJDCmXNki2G
FqlQSZSWoZKEUKh4pKLQZgtJ+nXPvTX/zOv9+nzO95x775H3CtywjYtGox2d
Q6MR/+UOM98+l7wEGvWLq9vSaZdYaUjqyu3kV1EHZBMfGf7J0/rSmrgTO/86
Y/D0xGTCh799iQCFEyMJk39zWpc0auH5/tdDayW+lh6e/tu/vVRgY0DQz7/5
+Qyef6yGZv+6PorVlbaSxqT6DMatCB3uL39cxbg6sj9hz8U5f62yLOz92+1c
f/vZHnsNNyjOpcxmCGUGZ9a8/uNGRvTTwBGtXG7KDxi7wP+MkDjP39yxxNv+
SwIv5RZGY59n6eZ1fJSfM5jS7rxNPPMov2BUbHTzYNz/416G2gnnm5cO81N+
w8irdRBdwphP+R1DbHrjjuNTfzzIiF1p9+D7dQHKXxgzvjYyfkELKA8zgthW
oS+WC1IeZbzvtHxqMUSZ9Y3hKmSuWnleiMqnGL5nCpipK4UpzzAUDOmfG5Io
s34xul/lZXF9+WMulBEqY26wXoQyN7ITzR0NukiZw4sESqXyi/lEqXn8qG5t
ltWb7ZRZgojVLzEl+ZByrzAyiMw4a6soRpotisalxe1iIyn3LkRlVak/772m
zJJA/ptEL06ihaQ9pJDScLLDilzKLBnUc0Jors80ZSYdZS1NLMtzEictrIA2
3Rdw67hBmaaEBN1P8AmKL6L6Kqh+el6F2R7KyaooKiPWM6KVMk0dMbR5BStW
SFDnW44mm47e+pRA2UMLeRvy64uMU6Zro7YriRW6LpLUeh3EVBBb5cL5Yz1U
mnrqyiGVxaQt9ZH0P9KaZ+Ipsw1QXCj70qPRPzlC3s7F54XvSZGONUJtDcuV
dJWXkNYwQUzGtQLnE5Q/maLSEj25QyOU683RErnq3EJHadItlig22VDq0R3K
NCs0MefBqY+KMqRtrVFbX+NJnWHK+naI6WAn7OwgS/rsBlT6qD0h4jZltU1I
eo3L/EIFOdLN9ijuYk9sXSzlaEc0sWQrz8cvlJ2c0bW6sZoYNTppG1dE1w8z
vJxMOdcdde42OHT3PuUfHiixeOZ2ywRlAy80IxVp8M1NnvQ3b1S+0SScN5ny
7u3IP/6fqsX3KdN8UefPOF1YpkB6xw6UqLc+xNaNsulOZBooWO6VRPnfQHSt
96RWzDfSrNtByG+xfWCWqiKZvwtG9A0SpZdcSbMkQ1Di/Rz1lhoqvx6KzGY2
+78dp3LpMDSjQy8eX6pE5hnhyP/8WZXFiaRZdQeR/Ovt29RrKB88hF5ILDuL
xkkzlVnILK5E3stFGZsjEoVmagI9QhIoLzmCrk2vzD/GIc3Sikb0gBvSl1RU
yP2ijqHOs2Gud5xJc+7FoMT/DLKfxpNmzY9DMzb3JMZHqX7rCVQeE+nAo7KU
zK0SkD/HJF3SmTSnIxG9WFkviu6RZgqnoPKFrQuOnVDF7m1IQ7eDlvTpVpOm
1aSjB83bbvUPkWZxMlBH7PR2s3XLsNndmain3xR9CyftMZ2FPhgniZ0rpqyQ
g6ZmFDnc89RIp55Gc1x2ZVzXJ93bnYf4K6sCvH1JMxez0ZIg68UPHpEeZhUg
6A8NPnJMnVyffxZZGNdYrrpBOewcss2fL/eun3SL03nk6cx+YmymgZ2sdQH5
3xgqGA0hbatajILFdMMKz5LWUr2IopseK3FxLydzo8soQW3hj6urSNNdS1BG
zJZWz62kORGlqMhoLKKmlnLgFdRQId3JitQk39eCctQm6lOidZV0WE056gq8
eqS3l7Tvgevo0zJzLSZzBXl+2g0klBcY92uWdNiGmyj+Z3eZo4QW+Tx6t5Cw
BlfOihWke+Wr0eK49UGvt5AOE7iD1EzeyBjeJb0wl4NKg3jmSXSQFlavQavY
6uNfPpOm3a1BjJ97G/JkVmJLD9ci60r+fbMHSXfHPERt/Su8OtJIL1xThxwW
2luXXibN97UObQnKV9zSTdrDrx7tVtdpufOvNnZf9hPUs9ril8xG0szdjcja
1EXzkD/pgXVNSG0zKx6ySF8Wfor6Exst702QNt/dijblvN4nJ7gKu2qkFdUW
jZ4/rEwaQtsQmyP5D3MT6e7YZ8hl1LuGc5X0q/Z2VD+7b5j+mHRtUAdaPf+E
XGQvaYZIJ1qodDXCSEiHtOsL1Gz/c01tAGlNmS7E8BL2U4gmze7sQpd2KWZG
5VD9jG4UG7N2wriBtBS9B5ncTL92f6kutvX1XnTt4YU3ioakpRTfIHpbtXC0
A2lIe4Nmh97sMj1Kui3iLaqS1lR/+Ja0YmAfUllm5KI8TfrnSB9K190Ud1RE
Dzt+Xz8Kttn/wYxJ+uvx90iDVXem7jRpoecDKDv+ZZtKBWnOzkE0L+vTnJhG
0kf4h9D7q6IeFj9I77T+iArebZGud1qNLT/9GS2ymEx7LKZPmLX+5wgarbea
UlpO+vSuUdS0ju3KMsemGbwdRdE2axVWh5P5gZYxNGqfU3a2h7R6wzfU3PlV
lDZF9vtsJlCxs2moq8ganOt2TCCPzZ8Zoqakmz9NoiZvw4bDxdi0cYNpdOF9
6vKuWtLZ7dMo2ncgWa+btOaeH8ggIMXxs6ABtlXlDLqw512fSwjpfO9fKDoq
5peu4b+Emb9KucCDu9srxQmbFrFoLvx7TKvuUxCZtx2eC6NxL+PPnCVzGSdu
8EhRlxLhZxDmDMrxAEOMFRGgiE3ryuABifTnvY8YpF8J8UJzZkTRoUBs1hI+
PmCwn+p8ek7m+0T5QVJBKdPiCzkvO5sfxs6E/SjkRXh/XuX5cLFIvtbZAJvz
nCkAkmV7/vcon7R0uiCM3ZHwL/QHPK+ySwSm7LSy1kdh944vF4WZfsv6iSxs
pl+kKHAL7lexekzmczXEYNGW7rdjSw0Js32SF4L+LNvVrB+bppElAYyTN49/
ncGmJ9EkgS422L2en4nnbfOTBOWiOQKT8tj0A4aLQfOptr+VHTb73k8pMJRL
Vxkvw2a51MmCsZ88PK4m1/eZy4FpeYl93iPsXqXHcmBpURdt+ZrsB/rRwTZw
8m2uoBH5PiPkweuec77ZTmytI88UwXve+xtS4dhXchSUYPvG4Oav0WT/RrAS
7Phw/GdWLrbHtLgyhAjddv3yBFuY308FjrrLSp5SM8b9NJNlAN5PHvutxr6i
dHkZTPiGHWCYYg+LL1ID3+C2njebsenqX9Rg3dFj5zRSsDmRZRogeOmLdu0k
Np8Y0oK6spy+NG4TwvrGEVpw+Lplho8INo15VwuG7xR+F1DHvlJmvBKetThw
HLeQ/Ux7bcicuGv9+QG2k9s5HbD9sePXvVbsqYAxHZhHW3z1ZA92/U5jXdg/
b89C/SnsZMt3urBZemlXlLop4d0FWqtBwTjJV/IktmTvjzXwypwh9TEP+wKX
iwGkWg0+uXMJW9XgpgFw25us2PoQ+8XI/n/hg8/kt5Ip7OT6+QguJ7gfMXE3
w/1CbSa4RM51fLUDW2fAjwl8e4vUgsKw6Y8KmLDV7WtrXgr21CYxI5BSP0yf
vo/t++ynEcTW5925ompOmBExYgJ6t41TLHSxvT9pm0Jf2XvvHiNsy3l7TcHw
lKaAgCt2n90PU5jYdtfFJwG73lTYHLzn9kzKjGK7fXSzBNHJyCfXZ7Gle4ot
gTOknG813wLfp/RJS1jSttM8XAnbwyF9LbSxf6Y9d8DebfNqHTBBRvtENbaA
7wlrWBLuFjAVbUl4JqfBDnr2vj13Ixl7YMMPO2AH+74OycXW3KuxAZQCQjaM
lGNfnk3aABru8fpDb7Hr9d02Apjd5u5mriUc9WGePdCMjSF7PXbLBSN7qIX6
fU5O2I294fZgof986Hkg9nTlR3uwVf/U0pSHnSbR7gCeItKn781gXze55wRK
goUdEXzrCBs3zDrBe35VYcZC7Ixn4Az+3DpHqtSxbwdxnCF40srvqgv28Mhj
F4j+74DumSrszPIJNygq7mo6FmJF+NK+Hg+ge0YVGEdiixXye0Km5LK9swnY
HaqrPeF4TKh0aBF2qXWKJwRsE9mx7RW2LPc6L9CSt+AzZa4n7FjYtBUuvPjc
9Ws9dnf7r60gn5xWVu2M3bJL2xtEf71xWLWH7D/L9IZv3QfPKZzHZuzz3wa3
Mq8ZzxGwJpxSJu8D2rbOi+5IYr9jufjAJV7aUJgytmpNqg/khlqnDAO2bAqv
LxzeNPD6dRB28+FxXzAVlo2424mtqdTnD80xcZUHztgQjqPJBYKrpejIljJs
HjmvQBjgy1EzrsYWvXIuELiOXz7N94wwS3CRxG7Qi396JJ3rf4TPWRfuhvxk
cdsyT8I0o8H7QVDVaBsyImRLuKFRNwRmNcRF3okTZrkIu4eAWcLLkudLcG6V
ERsCbdZeHyqXYkf6d4fAp+Y9LocMsY8xYvaCfGsGc34gXv/r8WAoHG/vFlBu
xvmZS33hYFWSe2vqGc4bn4nvB4Gjbr6NL7EVzSz2Q6JO9/09/bifxH1pP6Sm
du2vncEund17AHLtXg24q9sR/ThFqQgoaep8kB1LmBZcbMOCXedOBe9KxC5c
EsACrQhHunEaYc7/KuNYcE2j88BgPs7rdzxkwY0THdr6lYSZmU0QCXfXtrPb
+/H8gMw1UdDysO2gsMkGIucNsI2GT9OFk15rCXPknEKjgU9rT3DF/3CudSA3
GoyyxXxd3LDn+QxGw7Vdmzae3YvN7jp6FNIlOpbpX8C28318DFz8Xna4L9hI
7MeVdjAOQvOK7a6JEaZVPy6Og5PPwhu5pbA3o844eIKkaotVsI1fax8Hhqhr
yZghXv9U7PNxkKvuPhITTJhjELwzHvoEerXKOgkzlbPzk+C4ecGW9P9w38C3
NQlWsrziD7wjzDa5OScZDo31fbD4StjDRFYnGSRfDeb18mwi+uX22clgXTQm
IKpHmB2TFJACN4x4B0PSCNP6X6qmgtuB+kWu2YTp0eVmqTC3Is7UiI371qVe
qWCrKsBecJkws5b3dCoMCYo4nr9PuPfjerE0kO2Wetg5iuct1uNJh5hQzQID
O3viPKWreE5B7AJabr4jYbqwptopOH62NYN7C2GWzEabU5DYFhLf7E+YfVfm
1ClI16ze5xWN8/NVaplw5r2FzfFKnCfJu2TBPQfPHy9lHIjzLDj3Kgc4n7Un
QIkwG+lw50JtNPfIGTXCvdqjy3Oh7lrR+52rcX9sOjIXmgS/tM6xI0z3MdE4
DV11+y8siybM0WqKy4NJvTT78CHCw0Md19kQYubpyRkmTLP/t5ENwxs1d/JO
Ek62qnrHhoHd9dHpcx2J/aVnRAvg1cWZ8qvShG2FSoIL4LbsNtEhG8K7VWr1
CiGSR++pSznOv6u2nYH5HZ2WjINOv63luMO5CEQH03klogjbcvvvLQLJmY11
IzE4j4lMKQIVhRaTolQnfJ9+PC4C5q56EL1E2GNainEBQnhu6gy8JCz8YZFy
MXTrZdPTVjsTz6/jxn8JSk+5TX0cJdwrMaVUBsJ86tFm3wkP/xe5rgyCw74L
5f8ivPuaxu4y0HXOWLpBwIWY96S/ugxuS7U4VCkTHri/R+0KNJw2qYh2ItzS
kVN3Bd6fUQuWuUu4Svne/Gsge2Xqo02c62/z5co+uQ78ylVqjCTCvrdu9V6H
iax9fsvSCevz+Uxch+YjE+/nFhCeshqWr4BDjuNvqqoIxy6vC6+AntmvnQoD
eL34UY0bkGf94f6EudtvZ66JyKsEmY/tOXncm4n39aSm4hZ43zlXxD+fMI3r
UestuJy0tzxUhLAw/c3nW2CgI/7ERpaw7apNKtXgELFpenY1Yb4MvcxqSBZ6
5uS+gzBrw9jh28Ct0yJOb8PzD0W734Whgw1JBflbiP293LVqoCTUxjNtsQdx
v3hTzz2E5cwXTs3thHPtmOENIFaxc/RNgedvHzOdBy1gVK04tMPD67dnRXUD
n0HNFcs5+ku2Et/jbdhIBxTZhd/6r5/wWSXTlV3QfqSh9Xuh929H9SVmvAZ/
z6UnvgZu++2rBv/seAt2mmNbl67ZTtxnRjv0w+H419nt44RzSkqlB2BhRuee
zRyf345/+jD8IwxrDV90PeRLfO/a5q4vIFu9b06uvh+TxuK/83HVCJQP809X
cPn/tlTLT6Mx2CYRNWdqsz+TWTVm8wLG4f9Objtc
       "]]},
     Annotation[#, "Charting`Private`Tag$40136#1"]& ], 
    TagBox[
     {RGBColor[0.5, 0, 0.5], AbsoluteThickness[1.6], Opacity[1.], 
      LineBox[CompressedData["
1:eJxF13c01W8cB/ArkqRCUb+UlZEZZaX7PK5NGihbskPZq5StSERWknSVUJKi
ZBQ3lRWyIqOS7OysSvp1n+/33vzBeZ33+/N5nu/3Os4hYOtu6LCKQCDs+PuN
+rPIeHl+Ir8LEtAXmXip2qrT4MozFcyPiPHdYed4r9So0PKkgaRGpiud9FyZ
HJQc7PkRN4EwLfVEOvD+F3r/1bp7CcrpA3SnjN5cWIwdps0/d65JMH8aPEbf
R7wbWeHlOUF3lCrkSJWdptvzkdIrv/sz9PO2nBa8PBO7SN9H6NkOmpl/0PMx
3S1TD4N/0t1WwpEZu/SL3n8uynb0tOdv+v7sFObVemMr9H5tWEhPkiyBhKmE
SCwLlGOapJlAeDwTEOt9n4FuEbEzQ/2Oq0i0/WnWviqGOxnpjnjnPiOTzkT3
D2bXA2TT1XS7QZc7G7mY6fv6fU8uB7Uw03OTfHujydg1JNr7XGy8UDYeu4Xe
L9rcsv7i5V20PvG5J8+AfPkuev66yaFscOyfO6J+OmoeEKN7aXknhWmtOH2e
wdwt5YkS3c9Zn5WctneimUzk3MyovjlVnD7P43nov9c1//pCTdemvBf/5ZIS
/W92ikrQ36d8lGR6m7EEvQ8H/bzCL9JMea6t9lJnb/G/vv6tdXxfB2kmE02X
jeYTuCTp+23MyG/VNCXpuUvxWOasjyR93muT/JnbWf98ziP4sGH7v35EY53Q
KiYp+n1ixTf/eryXbmJKpFWLjZ0UvZ8xkJvDkfgvz1H9Hviy6p8fZYBjnrP/
XPIrUlxAUJru+qfbO0NCaaYQxdW/7FCpkMHdQPSQkGt+sX8P3Yc0zKWDXGju
IIofD4mB1//5unNiecYjmruJLH7ZYys1/zx4pUGncuGfq3Jms4OF9+LuJZIp
W1eTjtHcTwzsgnaEcJoHieaz9i8pj2keICquu8wX2vcv3yz0OFB1oxzuEeIM
sbOHAdI8Tmwy+r2v6jTNE8Q8t52pYTf+OSpSd0GtHnfIDHEx0VL4zhdaPkd0
JLsfY/xB83di+4OwcDt2ebw/R1QvTS58JYqbsEjkby1njzD+55WxL24aF2j9
H8QeRpZGpie0/BexZLu0xJt+Wr5CTJY/dukChwJmEgF4HQ4Y1iThJqwCR06S
NZndcYcwAsmQ6jvVN3FTmEBaTFeryFNafzVYe32cIbKB5jVg6DGntfYvmtcC
owrhuBxORXyeBbyuV6pYI46bwAr2dOpNnFTFHbIOZH612l5rSuuzAfZpT71d
HrhJ60HQckRAVCQt3wAmWFLvjWTQ5jcCS668DzrFuMnsoF6gYs29Rto8B9gn
3aKwdpA2zwFylQccnJdxW3MCbu3FpLpNSpj5N4HZWr0lISncfZtA4wGyRYgW
bvJmkNswV9FzAncIF4g4rCuoeJaWcwPr5psXEhJo+Raw33B2ZCKPlm8F3O1a
B3Xf4Kb8B2aNbhRkfcJN2gaaOqc4CUu0nAfcM9Pws+DYh993O4joSe0qFsdN
4AXWxyeInBq4+fnA/s+qZNfjuNn5AbdNCmOdH24KP2i0V6kPvkebFwS5Q4lS
PVW4+wRBhNNIvEIvbv2d4MQYce7qPO18IaB8+qrJxAZlfF4Y5Hp/HTD3we2x
C0TMK+oUx+K2FgMn/GPyOHJwT4sB5R99G1wpuGUkAPc5ea/aLto+STC7fOn9
zu+4myVBY9AnpWC2/fh9pEEuYW96tzBumd0gIizyj7wKzTLAmqnX9qop7mYZ
sP+iTPW4J24PWTB7qSvmThbu3D2gaZ309MoL3NZ7wb3YsKPmnbin94KIjZ3F
T6dxU+SA9VWJbRysRPzzlQfETSGBp3fi1lEAW5Lb+2qIuFkUQVNqYE6QO+5c
JUAkv5Mbb8etTwRbBYVStSdx7wLg+50zv26vAfg+CO7nCFSZKePeRQJbC7yP
1NzC7aEG5mRqCwVLcbOog3eF27mDWnE/UgcXi9/0yq2GmOc0wPcXW1xuu+Bu
1wZLBjLXD4bhjtcBy4M6tQvXcWvoAqYNASJ6dbgbDgBuq97+76Iq+H0Og22z
cxwZKriZjgDei+tVdUxw9x4Bog/hrfSLuEf0gdIK2UJzEPeCISAmlEZPLeP2
Ogr4N432HmQl4c9zDAjnMLAtCuCWMQLS7/a46BngzjUBMv9VhvIfx33MFOyx
07s+74R7lRlQWLSrvRWC28kcqPAli8wV4HY7DtScBWBdOW4lK6BRlG+UUYOb
7QTQ0a6O0PmM28oa6Lsv9qdvUMW83xYYlob/9NyGu9AWHGNk59QWwb3HDphd
26U6A3Ar2APbSrNbmq64TzsC+7VDxdvO4mY4CRyPejVNReC+fhKcGo7+fT0d
d5cT8Nn43GLyLe7QU8DPTMf7VSdu2dPgzJ326NSvuMdOg/OKE6Vqv3DbuYEL
J3i3XhNXw1ztAaD92zpnRcwh+z3BgtOZc0QN3IWewMmr9dOX47hzvMCBCxfv
Sl7FXewDVkXvNflzE9+n4QvKr/SxtN7H8xZfIJmqfNr/NZ7/9gMb8ib3VC3i
uf9ZUF1wYyCJSR3LeQNA8BOdlJMcuN8GgOkXt3+wSeCWPg/amo0pJla4RYNB
zHtGL/FTmEOmgoFG96Odv/3x3CoEFH9ljbx9FTNJLhSkLlQcmniN5z/CgP6v
U38qW3B7hoO1hP8eJ3zC/S0cBKz13qy0hJkyHAGObxftCZPQwM5jjATcAu0x
Rkq4r0aCJuFQuEsTt2AUIO3uyWy0wn34EhBUi3PamoC74TLo1iJu+5aBmeId
AxL1Rt++yMNM4osFTEbqu+3e4A67AoZPLs7nL2HmL40HD2JPhKuf0EQmr0sC
5qGMJt2nMIcEJgEW3xxxzzN4PpME7CynWjKuYrb+kgy2SQTz/3yFmdJ7DdTy
7pyLb8bMb5sK/DhrakQ/Yu4bTQUtPza4Gy3g+whpIKo248WjXVqYj6QDhedq
V7XlMVPG0sFAwZD9J1U8j7oJVK5Js7FZYOZvzAALDhXmJ2Mxk16QgT3jp8Ud
s5gfld8BnIuhb5+sYI7fmQUoY8K39NZpY88XmwV4Wl21zgph9nC8C1rJv5Pa
jTFPy+SAkKRMp1N2mMm5OUA6SpO4ygOfF8wFl9xjv+6+hJmy/R4gwR17Lpdj
tpbMA5OyL1cL1mImFOeBdGGHrpJ2zPpqD8AiW37I0AQ+b5MPHvYQ36ny62D3
rSwAPGctTy9FYG4OKgSffPvvFsdjXmotBGQvp88+6Zgf7SoCQqd9DGeKMH/o
LAKSJ2KUxvox92k9BZMWnF65k5hNs5+CR6apeY4/MW9dUwzkDbN4v3LoYnlj
MYCaz5l6SZiXTpUAgpoaTDuIObezBFTBWn9TUzzXKAXaSu1j7e6YnYTKgL7E
eHNjBmaZpXJgw7H9ZuUy5qiFSiC04XZHIMsB7H2qUMAQ6y524mbMTyIowIVJ
LrxEArMM50vgtajn/Ngcc8m+KhDx8Zz8nRLMcy9eA61uBneb15gbNr0BLJ2R
uXzNmJtd3oDY5kSe9GHMHturQcqrPIZkbj1sf1wNyLnX03jRBzPb03rAbxOW
qRaKmST2FqRuFfNdicUsd+stiI702+6Xg9k+vgGcduA45dCNOSSqCcgIaLNo
kA4ie7m0gNwPEz1/DmJuLWoBAvFJBeVmmJVWWgDnny/Ge70xE1NawXzv+buC
2ZjPt7WBstRCNQa2Q8i7LnaAPfpm3C+2Ymbu7wB5awhjZ4TxXKUTpPsdujoN
MTv97gTBx0Y+f/bE3HSpC2iw8wZWdGI2HuoFz2te6wcMYE4x/Qjkg08JKcxg
Nm34CEQmS97msx5GTi35BNY2HN12E2CWMewDTZGXnp27gznRsR9Y6HDOWBVg
PpnbD0ZYboirlWNe+63/79//BzdZ2jBXeH0FCjHvwpNXHUEWihkAt+K59Ats
MLePDAFJg4xLCa6YI5SGQRmH6Cvfs5hFLg2D9gQlBeJVzDpSI4Al2WJ7HQV3
6CgoadD3mdmoj+xjPg5WJLk4vnJhPlE2DjRju/LbefCcZwK0HrIdfiaKeaRv
Aow3eZsHqWC+cHYKCLSkkNa5Y97gNQOcZC0+Lvsgh4TlzYCHV/kCJgOwPGNw
BhANc4taLmJ+YzELjNtKRVIz8Hn97yD6fS+bcBM2P2E2D/Ty08uW2jCvvzkP
2C5YOjV0YR7smwdX5HpfeQ9irnRZAImJPQFVy5j1IxdBukH3yAkJA2TbwR/g
uFhayl5ZZEKl3E/Ay2CusUYR83jET0B+1HXroRrmKtFfIGtjl/FvM8zZ/ssg
v7HzdVoUtq9N9Q9wu3vNy+0Klu+/9QfIBJrwqyVhTvj9BxRKdp4bvYVMirUi
wOLLHXuUniFTxnYywArd9+T3g9i+kepVsPlN63l2dUPkLF9mOP7z9qKtLuZf
ZcyQRcbb6+kRZBIrwxqomrbJydwSmWIatwYWuh07muWL+csTFpi8pUNMKRcz
j/A6WHgwOyv6oSH2/H7rYFOoH9/HJ9g+hbp1kHmcmyvsJZbf9WCDZygmhIZu
LC+tWw/Nnbs6Tqw/SjW/+FF26Jdxz6BwEzKBKZwdJrSdbWDahtxnVMQO34Jt
VfdEkK1PcnFAIqdF/ncVZJL5Zw7IV94bHumF7Tt1eRMcYOuTKejE5m/obYHR
WplWyR+RKZJRW6BsiG3Mua/YPvU3W2DQ94Fh7Sns/LWqW+HW7tGMPuZjyJwq
/8FDOd/ZOBWQQ74b8cC5vifKS/sxn7zBA9O2+Tl9UsXs+YUHjsQuvbp/CPMR
9+0wzOd3gLoDct+BhB2wWHXNqE8SMkV+gQ9anqvltkhDnn4ryA8Zn17SUCVj
/eYD/FB/Fxt5/QOs33WDH45t4DDJfoXcPK8qAHl7t73pnMXy3gxBGOknnals
YIT23b0lDKPWE9JvmSBbm3YKw+islhQmK2RyxEYReKXVJ6bJBVnmSKgITJYu
97eNQKa8dBGFd4a0D0c/Q47/YiQGswL/0516gcyfniwGszd/Uz/2Gpn0+b0Y
vK92ZR9vCzKBwVQcPs5oFyocQw5pspWAlcY2v7p2GCPbJ0pBysSeBSiE/Iij
VwpWRTDN3BFH5jcWlobVhTlDrorI07ml0rBxw2QLgwHWTxjdDXuqA3LFIpAJ
+Xtl4aJCktHZMSxnn9kLfTRtbCjTyB6r+OTg9FFp1zWLyJRDh+TgiEdtRDKj
CerP3peD3feXix5vR16KcJGHz3kdOMcOI2/V+aUAQ5kV3pkXIdcanlSGK5sZ
ezJLkQnRmcowYGfz0Eglso5UrzL0Irms+DVg82WG+6F9QIZU4iB23ooGEWpN
Mse83WKK7lMFIVzX0alDPI98elhTFXKOJq/ZEoYc9e2kKty6fLR6JhK5QTRa
FYoINqvnJCI3675ThSS3WsiZhyxDtFSDPsylciNdyJY8oeqwVyGNP0nRjOpd
vUuasF/X9LMbQLb3F9SCo5bcGbrqyE7HDmrBhbAEnj+HkVnek7Ug+7tobhdH
5PEfB7Wh5slzbKRk5KhthTrw4TXLpW+zyOxshXqQnUUiQvMHsnXDiB70OvNj
460/yE+G+A5CebMUUUM2c/S+JOIOwufbmo1LhJGbCV6HYP1N9acRpshnNHSP
wKE74l47KpClX5ANoM7mH7/9XiO7yVYZwPsRNZea65FNu78aQFcH+8zwTuTZ
elFDOCeS0Tw6jRwkXWgIV93n2F2804LqDsWWo5D30dK3w5eQ9UWUjSGrcIk4
MQ45a+mEMVy47u8slozMTrhoDJvCF4YYM5GVClqNYZDJ3JeSEmRKkpsJ/LQy
1Sk4gtxb8MgUZhwafrWgZYl+/9+csIDRVdmrBg4iB+THWEA/RUfVFkNk1tZS
C3hYYLAizwq5o2WzJVyZ6y+19kNeLmy0hFbpnwrq7yKz7dWzgju+vb+RwXQc
vU+/cmto/+JuDus6ZCOxD9bwQZxvkR8H8jOmeWuoLMf19jAv8hb53TbQOPDY
zxVF5I2hd21g/MY20xOnkCe+XbeFTHLNXPytyGfU79hDPWayQMwH5DajN/Yw
4YO71NInZLaUYXsoELhRs/kb8ihZ0gHC6sM+IautqFYbLHGA/qaNrX1KyMEG
3Y5w7Hx9XOYt5AFmNWf4oDr5wdRd5FpfZ2foxm5TBx4gF3BfdYYzdxZXdZcg
a031OcOleiE/zlbkl4RwF8j8X7BlONMJqsubmk9Bwad7xRyckV+5JLnBgZUV
zSJ35GD/KjeYrVNvy+CHbPR82g2K9Vqn3wxDFpw65A5lGK9s7LiBfDx4tQeE
BiPzWk3IR37UeMB8v8M2Sf9Z/3XIvJ6dF2y7Kal7YTvVhL59573gj9essn58
KF+tnuwFNTfVEEyFUW6fU+MFPxaokHlkUV5WJuUN14/KfL6tgyzP98cbulps
Ov7YH1nr3DNfmBg2o3E7AM2//dXmC0vvvZNMDEQ2SZv2hauXLi/7hCMPyYr7
wZtJTOlKcciujRl+sLFxvrsyG+2zqI/1h1KkD6ZN75FBSPhZSEiBOSsfkD/k
ZZ+F7d+y5qV70Txxpe4sPH/NMyGuH+VtWzgCYP0ka4P+FMqLBTIDoOPffznb
WGyodsyrPQfJP28Lf9hPdcgWb4Ug6KO/1odFBeU2T6yCoHa2e5WSGsrt+SOD
4KQB8cR1HZTznf0QBMG996nmRsgzMoHBsNuEhe2jG9UU41MnQ+Cmp66zXzJR
LjhTFwolYw9u681CtjL5HAo1HCTUOnLQftbWuVDoxzV6tT6fatIAE38Y/OBr
L1tUivYJ2PqHwQwFC4+IFuTfzOLhULxEZ1KEwZY6/9byVgRULd85dsqaaspF
y8ZIuOVIyDYTO6pJF6uHI+FEf+8BNUeqCTe1V0XB66wpeVtPo75enGIUnDFj
cX3jjwwV7kTBzKXxKd44ND88GXQJMigUz7e8QPOR7jqX4ctHOgxKPHbUfu9H
kTio4S2Vastrhz5/zQNxsFaec3esALJio2scbC7rsewXpZrUrPw0Dn567VYS
I4fmr9UJxsOfH5LcvxxC/Rqh4ngox/DlY3QI1dYr4qNXYY7B2bKPg1TzZ90J
S4IeKR3irSNU97HsuJYElXr23qj+hvpHsvOSYL395LmCGXRe5kh7Ehz3twOh
v1FfVWpXMtyTcYgixGVPPe/Di5ZkWDEmUH1Kg2pSmqLsNfg+vL7lx22qKYuu
O9PgwcWCXKlsqvnvy8M0WOWSHGxzj2pyDKdZGnxoYC1VV2CP7sMWlwaj+Bai
Up+jfbx/fqVB5XIBkmIHOi9rqusGJM+eeeiz1oE6T9HNvgldbEQvT7lT3Vxa
9JIMM+KjXTZ7Uy2TmNFChi2VE7r7/KgmMSd/IUMl3ics4edRvymLIROu6SFd
5L5EtfUFfbVMmHXMPBTcRg74+CYTftKO9b/cTrWHzPz729BA+rud6D5H6r6X
ljx3YXDM57T3c44oNxu8BzendHofp5yk5uNHfhbAaZnp+xZBTn/N3lSjWwR5
y/0Z0pWc/zp+t8ifYlg0zfrz6SoX6vONjlwvh3HPKvS1KqleLqqGFNgqFqT7
6PKpv56u11J5BS2lrMjxB05T56OinaqhEn8+d9Fq178+49v+qQ6eq1izu6CZ
6hIHB/YmuHoy7K7AFbe/LnP+Lt8CF2rXVrhauP81K5fU+zaYXvfnZyCnB9UW
/I87oM0iq1aIB9XtLvB2F+z6yWPr3kH1Ale+8Ec4rwXyr8t7/vW90HvWfbCM
lZtlMIHqGy4jR/rhnqy5vTuWqOazLE4fgIcvfr0Sb+z113N8EQtDUPvAlYMK
plQzFp9nGIakDftYe82ofp94lm0YyqZcuSB6nGplqRDBYbg5e9/5CjuqCYwv
Dw/DnjdxzuMeVOtkcOYOQ6fVRA2dy1Rf+0CwGoE2dUMMkzFUs4ddcB6B5rFX
KxOvUL0zZ4PvCDzINaz8+Srqu0jHjMDdwgmyfqlUN6zOKhuBCxojvFl3qeZl
cd46CqdYEnt1c6jOl1MQGoUjDSBtKpfq5sU1MqOw61gi1/4HVMvplmqPwuf2
kK21kOoh7aP+o/DprtE6/ydUHzTXDB+FD8cTI3cUU72Hgxg3Csk+o6ucS6nO
9lbMGYXXlZIoG8qpfiJILBqFCcsw6Mlzqo8GalaOwmjK6H7zCqpNLhx9OwrD
I5J+/Kmk2oXo2DkK/wcDl1rK
       "]]},
     Annotation[#, "Charting`Private`Tag$40136#2"]& ], 
    TagBox[
     {RGBColor[0, 0, 1], AbsoluteThickness[1.6], Opacity[1.], 
      LineBox[CompressedData["
1:eJxF1nk0lVsYBvBjVpmTSgiJRKKE6tu7Y4okUaaQjF1DMqSjMoYoMmW4KnSU
UCFRURlOqCQVkjlTkTlUyDXczjec4w+t33re99l7f6vVSsrB84gzK4lESvj7
i/5nsfnC7/H8dkhCfwqRK69tW01iS/bhLovvCPWXiH1DGEn6lvSePbYVdymy
hxqUHOz9hZFPbnusFHi/DzeJVL3q3rU9ad8YfSnD6TOzMd8Zdn1zzepJ8AjD
yN3ICh/vcca+d6FGNeX+FMNrT0lHT8XMMuZJnWKggfMP4z4jB9b+KAieZ8x/
KhXMjJn7DzcNKZPjOXrKexE3FclO4eQ4OLLEuH9taEhnkgqJTOwjzwNV2ScI
F5Y9mroQc+Y+C5nok5U/N9h/kpVM9N2wO7vvyCY2hvlTfVJf9rAx+sI/ek4p
p7Ez+v5wehhQLTkII6eh2x3+NZyMeYt8J7OJGC6GZ99fej4Ws5bRXyzcyBsR
vYVMvL/l8vxJXQN5hucWNtHYV2xlGA5QfMIiFBj7dU/EWkMuKjHObxL6J1/5
EWEa0un5KKy3V4kxPya/X5lM3s64D3+G55XlJaavLnY9tFirzHifgCLrze3b
lRn7SVZyEVx6TK+/YujdY0uYVpZR4m1TQlFm9EkPpujFxTLns4XLdvyTzcy3
aveJ76tg7hd4c65Y28L0TqrCr4lxwqVI6QfjntccKox9ZPFsXYY40zSFm08o
u5jWsaJRjQ6pMPZrLw9Eyzoz80MlK/2WAgj//X4D2x1akpi5ubDZoYI8wrVI
h9YFjYga5ryt961Ntl0Ml/XfquFT+8U8758Pw394eXYw3j+2wDcwsIlpLwXV
hvK9hGll3ep6y+JHdzD6D+lYKQW5ESaRyow9jndfJFyDbD0echVeZ/Zdd018
kVHI7OOmZI8svWH0lVFCn60/0UO4FBmIrdevnGHmpjd7/Dby7WS4Kmc6O3gz
YRJJ5TFHSw/CzKm0dRxkU8K0Mr73CqpUd2Ye2A4dSWFMjw2YXLO7wTBiNe30
kvaI2V+75Dcp+ZY5r74qeuPFXsJ///6szTDqmyVcigjLPArU5FdlOFS5Ji9T
VpWxP4W0drJAVUa/3YGRlQ5mqoy+D2aLu6tOMee1nyUXVcvtYlhEbzbp7WoN
xvt+lq91u+0GGfmcifJ1w1DCNGRhQL925jrhvz8X7Gepjxh5GTvfBdmDb5nz
3Levmf3uJUxFeNUehN+aY/QjIrZd/T/l9jEsOv1LMGPfPsa8RASvpr4F4RpE
WlTWa/o0YRJJrgDeSotgWmOJaq07wPS+jcmyvx6SGdZylYJvXxCmIjrF+WYZ
bwgXlunrvQ7X72HOGyQcSRMfJVyDGHZ2F0/PMOYRo83u796wajLea+w525/G
R7gUOfIsbN5bVJOxb8omIKQnq8noNz+UJi+2Q5PRd+zfLZpTgLnvUHnslq4H
YSritGLwqeh5pk8e9fnwI5x5vkv60kBNPLPP/XvU4vU0Zp8vf5n1xDumKcf0
z1S3MufP3WmOSv3K7A9QH3+m9R8zv3RCYt2/W7UY50Gnd29d1QnXIzMu5/wR
HWbu4tPU3Xdci7Ev6Rcc/9iN6XZ/Ra1IP8KlyLWQ9p/HwglTEYNLEXcVEwj/
/T9B1E6L5XRm/4vYXu6m+4RrEN/EmOdZJcxcMXXPKb8awrXIt7Tv4gaNhJuQ
9Mykj2LdzH2+BxM7qmaZniy//YdHQZvxvk8N5jQLW8I05OpnNp+t7tqMeZ2O
wk2Lfsz86deVkbcTCNcicuNOI3oPCDchqTMVh8ZrmL6w4oywxhzhZuS4mFxn
qIIO7jaEvL0z870t09JacS7rrhHuRTr2I6KjGYRbkMSDw+/KHxDuQwyNUwLj
Swl3IOxm2tsdXzHny49N9u5qItyFUGzTr3H3EO5GlBwNdDpHmX3f/5n9nT9H
+CtCPZWVE8Khy7Clt8mxo0KE+5G6Cw/K5hSYDg22PP1Ogzm/N5xDMkOXmf+6
XNTodYTwAJIXcyJM+wThYYT7bM5W73PM3NHmR2NGAuERRFQhWHK+mmmK0Js3
cl8ITyKNf/g8zWaYVuwzFwnj3485ZBK5XJtRXrgFN2kaUSvTStDbRfgn8u3h
oFO3JtP7/lXi4bFmzt8IohTv9iX6fiMzzhVW/8QQnkGOHOJkTc4mPIvkqxrd
q6okPI9wi6UYT7Yx7cTWPSs+TXgBoY1svnVwlR5+HglsaPLYf16G6dpXgqIC
KrhpJEB59mQ8G+AmswCZ/GMvgQHuEBbQRF1MajYn9tnAFc+Yr9uvEOYAZCi+
I/oF0ccB0jY7t5c2E/tcYJYnP2RwnMi5QUEn8lFTUh/f5wE2H3tvtyniJvOC
FdXhFM/duGk84OnTLQac+4l5fuB0v148/QhuSQFASxB+VeeOu1cAbDhvc2ou
HLedIKD6uPT4phH7QkDmlO+RqWLivNVg0GU++mElsb8a5DqHvPJ4R5y/Grg5
cC4rtBIWBoonrmqM9OMOWQMKLVMfnJzHTRUBu45kSXwVPIDfby14frAw4YQ8
brt1AOqWsXeRcYesB1Ww1s/SEjdNFOhpNI80e+ImiYGVu6xkEv2JfXFQr9J7
3CQSN1UcGCuMNbzPwE3eCJpl5rQNnhLzksBSgr3k9XuiTwqIboiaDG/HHS8F
utYKbNUewD0pBTKEUxxZpoh9aWAvKJZeuUDMSwMZvtstgdwG+Ps2gcGVWwQQ
YdwNm0AuV8GB+Y1ELgPc2FXDShVw98oARZbnZRR1Yl4GTCzum1HVxh2/GRTO
v9r+0wh34WbgM3vQ9ZEVbqosUP3VeNvzJG6SHJiZtOja5kPkcqB0/MuasUDc
AluA/4jj4ftXcIdsAfD78GWXZOI+WwDpm2eVbCZheRD+xX/XnVJiXwHs72Dx
tK8h7qMAuFsjczc24LZTBHWfePu/dOKmKYKYhsQNad+J87aBlOoHLMkiB/Hv
oQwsaSp7j0rjdlEGouUlvoJKuHuVQcbT6u8xurhTVUDOvc73Eb7E/k4gaR+a
qXURN3UnSF0nf3YpBvc6VRAVSRGj5OAW2AVOOQu6O3fg3qIOvomVQqnvuEvV
wfFmW6EvP3FbagAj7bxnpryG+Pt2A2UpPW4dMu6GvSC3bbxz2RC3FwKk4pMe
vjiGWxkAoeU+851ncIdA8Lsr4K50Nu5cMjidtOl8dxFuYU0weLDO8EYlbl9N
0PZ87S/BdtxkLfA8tUiLhecQ5jltsMP4mEj5Otw2OuABF2nk3GbcbTogjXIo
YRLiLtUFwaZDPT3euHP1wNyquOKbQbjJ+sCrelekRTTuen3gsCNM6WMW7qED
QEdAIrCiFbeqISh7U2N84RvuBkOwK9hdRm0Kt+8hIDtR+i5/pRHmMiOwov6o
aDrAXWQMPkReKfG/g7v2KLDWF5qyfYhb0hQMcd/cqvUCd5QpYI3KS+f+hNvU
DKhd/RiWzHoYM58FqDa0LD/HhzvIAhjz9s1Yi+KetgBusdOu0jtwN1uCW/Fr
jB/a426zAoomGVeueeA2twbPBeWqz57HPWgNmq9pqCEJRJ8N4E62FntLw616
ApTWG/tO8RtjFnAAS4prBL+uwe3mAHRj2vObN+CudABNhxy+l8jh9nEEYx/O
WAXtwz3iBHZs15j11MWt7wzOxy0k2h/E/dAZcBpfeq9jgfv8SSDVmEJe5Ylb
1gW4qFh/WfDFnewCChI2Xpi4gJvdFSBHcosbI3CPuwLzT89kUzNwN7uDqM9d
PJs/EPNe4GB+2vO5T5hDDngBnks2LvXteB7nBWJVu6rPDOCW9gaJiZ0Xqhbw
eXMfYOp+c0sKqwnmuz5ARNu6xZUbM2nGB6ROd6gICuN56hmQZtIxdEKByH3B
cfkbKTtV8PzwWSDBYqXDpY7nD84CamH7rQIt3M4UkMXfbr54DPeoH8h/31pz
4zJusj84ffdfn9OxuIv9gXKghaRWEm7ZAFCk2Oo/fAs/b3UgeBrdskOjBM+X
g0DFgc/UzwOYyTcugmCpZKN7o7j7LwLyH9OFgCl8XiEUVOU2W8gs4nllKHjD
1cx3RvgI/r4w0PCqKUBAG/eNCDA2f3vW4QDmkP8iALfyGZ8nh/H8RCTQvLHa
xcoGt/xlUHTa9GjWWcy0xivgwx2ZDzP+uPdFgdG2X/oHQvG+h1FARjsZTsTi
+0nRIHlti7xGLj7vHQOKDLOzogpwj8WADxcpG788xkx2jwWcYyJrQl/ife5x
4BzNglTfgc9XxQMr1/aWE7xHUVN5EgEl455J0WrMdlaJ4Nqn8/Xsophp9xLB
OyBadU8Wc8jBJIAIWef/3IdZMj0ZbHzRFRbpg+8HpAJkMm+p/RxmUncqsNwc
eF4xGN/XvA7i48Q9G6Px81fdAKxOtlYb7uLzRTfBN55e5YeteJ/eLRC1P9M2
+Qt+3rNbQCXE4ar/V8xkESoI+vntu94P3NFUsK5jOKOX0xS7f1AmOJTzk0dI
DXPI1TvgV+/jPXN7MTc03gE3RCku3Zq412aBoZi56vuHMJNyskCo7+IFbWfM
yg13wVNNrmHfJLzvcC6w8a8Vsb6BufBOLmB7ckVHk4pZ8k8uMN7CQ+XNw9yb
fQ+M8AlaZFdjjud/ACS6RF+1TmOeXFMAatZ0TZfP4fsBBcD9cLpk1hJm468F
oLRqY4DXSjPsvCcPwZF7MjtXSGP2elwIIilKmXtMMIdEFoHLvKS0WxaYyXVF
ICqrMYXdFvNl3mIQ2+R79YMbZuV/i0Gy0gs/h3DM1MePwZ1BPaOoEsy5G0pA
VuD6Az/KMQ+dKgHZwqPapjWY5ypKwH2t2N0SjXjfyVLwKKNZpmgEs8bLZ6DS
3P6/dnFz7PwHZYA2vmMGymCm8ZaDqnD2qTtbMZ/zLgevi3IGPdQxCyAV4D3f
RCOLCebenkrQ+fpCrnw4Pl/0EnQdN7wTG4W5Yfwl6P4lnvEzHnOtfBXol36Z
WJ6Oee5OFRgO4go2KcHPp1aDWbUks/MjmJ0qXgFfXXt72iRmHfbXYPKokgfX
LOZfBq/BkFdteDKbBXZex2vQcX+h+JEY5gW2WlAm4Sw0YoS5N6gOaGzbIaFi
hlmmqQ483rssf84as53sO5BveV2T0wVzXuM7kHHtvZf0Rcz6O9+Di5xqH62K
MTcJNYAlYbbOzGeYEZ0GcGFTw+BQJWYNSgPwIbstUeoxl3Y2AKcLGdsSBzCb
5zeC/ROcV9+ttcTOc/8EVrW06iMBmCtsW4HQcDLX2lDM8xmtYN3C0ddTkZhp
Pa1AVrpBOycRs7RjGyCfroVCDzBTvNuBL+cz1aF2zBr5neDCer+fVT2YS2c7
wUXFXUXpA5intbpA7JFH249OYfbt7AK5Gfe2VnAfQz0o3A261G5IJqljvm3W
C/oPWPacBpifh/SCYRuRjAPamNXzesFM6LUNy0aYPdj7gMDHKBG3k/j+sz6g
+48/DzkZ8xqNr6DgX5u50WnMv6MGgQC3QrjuH8z8bweBz7k//LeWMdO4voNd
x1LkjvBYof4e8R2UiTaYl27GfObqEKhL134Sbok548kIUOQT0uy2xVy4OAJi
g3rr1Z0xe+wfBSYnAr+NeGMeaB8FbZIlq02iMa9ZMQ4G72z1Ea/AHH3lB9AX
/rNIqcE82PUD3A9/c6WhDnPYukng4eyUGdaKOqTaYxL8ks1oGJ7E8nGxKcB6
X3D7003WaB4WOw0kCudGja5gtqr5DVZuLt2KxGEemv0NZq77uconW2P3U5gB
H8JmBtkyMa9PngFBFr/6Sksx55yaBd1LP1qlh7D9QeU/oO7MQxGBCczn3P+A
p0OnzRZ/Yg7N/vP336PxptZlzHPi8wBmj76/utYGNVXoP5Bx6Hv1zH7MnqsX
QVRVNus3Q8wfzBYBRf2kZuMR1KSi1EVgJDVQ8cAWM7vkElj61f/MjoKZddcy
sE3rflh3F9u/UkaC4qOfb2awH0fNpcEGncrv5qxchbnPmQ3mxZ0tpgiiJosm
scE9qmveGUlgzptig+aBpvNL6qhJ9o/YYTz/J8sT7qhpadqcsLXvttM7b8yP
/TihxGMfL/Vz2L56HifMtxS6zH8J2w8Q4YJ1mSYllRmYRSa5ILtqwxrJJsy7
S1fAg5xUqatt2L7WzxXwWpvntrlurL9SaSWUCuTXbRjF8o05KyF8beQbwmGL
5oHpq6Cf5fumXg3UJPdMXjgSUBeXeQs1tZNDEOa9Ts77cRebf7tVEJ4WsH8L
8lD3LhwWhFN3Zlk7SjHvvCkI5+pkKEJNWN+0qhDkXB9sE8Z+Av1+/JTVUPrJ
TnlnV9R2wyoi8NvSkm6xJ2qSmZ0IzNavc2ChoKaujhOB8l12aemh2H7MuAhU
Zovlb7mJuvdiwVoITYZ+7/+A7beS18N8ipF90no7tL/hvhj8lK544JIYasnq
XjH4p2alCmUj5lVrxaHu6jcky82oQ7LCxeGXh/uoG1RQk5cdJSDvsHLPbX3U
Ar3rJaGH9erjj/ywfVteaZgYOqVz+wLqBkRJGj6791ExMRCbNzosDTnmohd8
w7D+VdekYXoSe5pGHGra7PpN8P373x2V2ahJjTtl4DZym+WHz9i+U4IsJKXA
nKU2rD+yTBY2j2b9VupCHT/1XRYG/Ot9La4fe+/1fXKwbmJlvfEPbF53Wg6e
TAf7PnHbo9/L3lkeUudvb27bi1rA8pIi9DVe4cu9DzPrc0Wol+1ZpaGF2mtp
QhFOmCAnruujbpg8tg2Ce59TrcywvHanEuyw4Ob5chrrz5jdDlc/8Zjuy0Tt
4tenAhVjDEW7slDHay6rQB1nBa2WHNSWu8R3QMqa4YS6fNTUtGM7YNtZJ5Xi
Z6hJp5p3wAw1a6/wRqxvT9NOuLVUf0KWxQF9788fu6B2vJyIFDvq1BOr1aCN
CyfcwIV6y4KaGoxZVxPDz4v63JsgNTh5bt+2uXXY/gMBdfh0t9qpt8rYfBvQ
gJovNo2426Gm6VfugWsPh4haOKKWtBjaA8f7uwy0TqJuuyG4F15fmfJg3SnU
hVVOe+HUMW6PV36o113nRWDm3NgPiTjsfomuALKoPf3dWI76m6wsGba+FZIt
p6GWUYdkmH/c0zy3GnWAszkZHru0pSToLWp98UgyfNR845zCZ+x+/w2Tof2Z
4P/Cx7D5uCea8GWhPovGBke6xcactKHOmW2pDhKoEbswbVi7S2h7jBTqkIVM
bdjwvNOmXw41e0GPNuyuOV16VRW1zR8bHTjfluTZdwjrszihC1VZ+r5EhWB9
tuF6sLT6le+TMNQk+Vw9uDfi/qreCNSqUvV6UGuV7+5dMdj+TWF9aLKGK7nn
OurLz3L04Wn5bYaqxajra1sOwByT88+/DKDeEnjMEHqltGxtGkJNjgwxhBqd
O2++HkUtXJFjCOucJvwfTqFWLp4xhGN+juDiIp6nHII7Mg7RZNY40V3q32ME
K0akXrvroE6zqTOGkduD1ez0UHO39hpDY9+ubFMD1AFus8awbzElEhijbu6S
MYHsgjwH+G1QZ02FmEAD9Zl3RWdQs/8AR+DnsLrGP7dRC7S8OwoNZx/mbstG
PfP6+1FY5ZYcbH8P9ek2NlNYYGK37e1D1NAWMYWXN85cTi1DHTJbYAr3vJAi
q7egpvjfMIPU6XMFviuc6Z6/FW0BRU7aXsrlQd3f/8ACXm3XtuniR21gUG8B
z9P4VuqIoLaJ5LWER2KznFdvQs1akWAJObY2iBUhqB12Zx6DbvZy0T88UU8f
/mINM+Kj3ITPoOYuYbGBjZXjB3ZTUJvqytpADYnH3GEBqA3bPG0gVyc5QuQK
6u4O9uMwy9TqIriNWtpTzRZ268X4RTejDjphYweF/CbNC1tRAzlvO6ibfVTt
cwfqp+wRdjCPXfS3RB9qUZZCO+j/MtunaBx1GguHPVy3l+bRznmS7h/KxfbQ
ROmno9xu1JKvJR1hXc8HMREEdf1HNUeolXD/M/s+1OYTho5Q9Ze9Xr8OaiW3
845Q5HnD1nRj1E9tPznCLt2CKSEX1Nb60U7Q5bhr8FIKao6oVSdhH5+uxvh1
1LmGMiehFU1yqjMN9XpZcBIe3NTm8Ow26gRxz5NQaXj/ft8C1G8km0/CX74y
vCOvUItG3P4HBl/tufH5F+pJaOIKs09pP2ebQz1/xNMV1hvmtKv8hxqEx7jC
dbye62JZ/qG7HNa5wqKYpeT9fKg5RXTd4LdY8YQSOdSzdmR3aJBgHXndCjWF
1cgDCqe0njlOoztkTHXAC4bMFZ8yq0ZN/jPjBUet4p0PvUbnG+u5vWHVxgMW
oB7N8zIVvaHXved7xNvQPJvtrDd8V5bO8uUHmks94vaBoV8d42w2utDzC3N7
z8BJ5cn71kF0hyz4NZ+F6w8b5OlcRL1jdPgs1PLIyt8Wjs5HeS6fhYn3LAuX
r6D5rQdbKVBN+uWTO8lo/nz6IgUGrL5GG81DnfZqpx/kmtnZ4t+JWvtN1jko
8cKPJU3Dle6l2Ap/+IvLyrVmL+rGTx3+sM4UaRyDqKe2z/pDvwlSJtBFTVZS
DoANUlHkHhO6Qxp07gTAsMtpwdLuqE0GYwLhkNnLxdx01Bb2Z4Nh8eTK+Ses
bn9NO7mv9iL8UOm8N5eDblKpTdtFOBJLC7jBTTe56dLQRSi5jbIcxEd3iMd/
3KEw1rWPXV8UzTnPGoRCt/4S/g4VtO+fnI+hUKrZafOSHZo/VvsaBuNKKoz3
V6I2PascAS2fZM75VaHnqVvoRkDp4nDqvVeox/WtIuDjAoNJnnq0r986PAK2
3W2J+9SG7vNptkdAyaSJD3bTqFUEIiJhoZfEIf/N7vR5H5axy7BJPuhAYTTd
JL7do9HQZpstNd7gFN1jUzIJUEMyX6SYw+Ov7SR4PyZB/wqu7Q8b6Cbljftd
hxwToXelYk/TczvNqAw4U7uiwsPak94vvXj2Nkx7uzwfKORF/x7eN9dlQ/vZ
lftDvOimhZMX78H2+Q0Oni2oZwKaCuDv/SD/+i7vv77MnrvwCD5fKcI9cI3u
OdZLbY/hjqxfO8Xn6O79l+N4KTSK+Bobb+7z11TBm8JlUM8g1lDNku7LL/fI
lkEy3+6VXcfotqz9ql4GVVJiL8kdp3towsS6DApn7w6ocKRbUvzW7TLY+SrO
dcyLbpcF0s5y6MKB6OhH002SYrOugPZvB1kmrtIdn9viUQGtYhIqE2Pp9hJ7
HFIBDdd839OTQPeWL1ezK+D2zddUKKl0c+9/Ol0BZ3SGJLLuov3LY1cr4Q/u
xK4DOeh+oj21Eg7Vgxs/cukudegtroTtpolr9ubR3ftqoaMSljlBnqYiumsT
24Rp8MmW4bd+j+lm5y+ToMGCscRI8ad0J73I2kKDVN9hVtdndOcVX0Jo8LpG
Eo3vBdrHFrSfBq8twKDHZXQvxPkb02AUbXivVQXdTlZBVjQYFp70Z7kStXOE
Ew3+Dx1sQ/E=
       "]]},
     Annotation[#, "Charting`Private`Tag$40136#3"]& ]}, {}, {}},
  AspectRatio->NCache[GoldenRatio^(-1), 0.6180339887498948],
  Axes->{True, True},
  AxesLabel->{None, None},
  AxesOrigin->{0, 0},
  BaseStyle->{FontFamily -> "Arial"},
  DisplayFunction->Identity,
  Frame->{{False, False}, {False, False}},
  FrameLabel->{{None, None}, {None, None}},
  FrameTicks->{{Automatic, Automatic}, {Automatic, Automatic}},
  GridLines->{None, None},
  GridLinesStyle->Directive[
    GrayLevel[0.5, 0.4]],
  ImagePadding->All,
  ImageSize->{432., Automatic},
  Method->{
   "DefaultBoundaryStyle" -> Automatic, "DefaultMeshStyle" -> 
    AbsolutePointSize[6], "ScalingFunctions" -> None, 
    "CoordinatesToolOptions" -> {"DisplayFunction" -> ({
        (Part[{{Identity, Identity}, {Identity, Identity}}, 1, 2][#]& )[
         Part[#, 1]], 
        (Part[{{Identity, Identity}, {Identity, Identity}}, 2, 2][#]& )[
         Part[#, 2]]}& ), "CopiedValueFunction" -> ({
        (Part[{{Identity, Identity}, {Identity, Identity}}, 1, 2][#]& )[
         Part[#, 1]], 
        (Part[{{Identity, Identity}, {Identity, Identity}}, 2, 2][#]& )[
         Part[#, 2]]}& )}},
  PlotRange->{{0, 300}, {-4.440892098500626*^-16, 0.000019307602028222287`}},
  PlotRangeClipping->True,
  PlotRangePadding->{{
     Scaled[0.02], 
     Scaled[0.02]}, {
     Scaled[0.05], 
     Scaled[0.05]}},
  Ticks->{Automatic, Automatic}]], "Output",
 CellChangeTimes->{{3.7411687137864122`*^9, 3.741168826023624*^9}, {
   3.741321894836523*^9, 3.741321911483397*^9}, {3.7413219631318083`*^9, 
   3.741322008030081*^9}, 3.741336607876193*^9, 3.7414102605241537`*^9, 
   3.74141083249891*^9, 3.741411452925015*^9},
 ExpressionUUID -> "356a3658-4a5a-4a1f-b497-996744b850ad"]
}, Open  ]],

Cell[TextData[{
 "It appears that the error between the full-range exchange energy obtained \
through the sum of the separate Coulomb and Breit calculations and the \
full-range exchange energy obtained through the Coulomb-Breit calculation is \
of the order of ",
 Cell[BoxData[
  FormBox[
   SuperscriptBox["10", 
    RowBox[{"-", "6"}]], TraditionalForm]]],
 " , and could go even lower with higher orders of the Pad\[EAcute] \
approximants. It thus seems to be a quite fast convergence between the two \
methods if one increases the approximants orders."
}], "Text",
 CellChangeTimes->{{3.741408144599476*^9, 3.7414083738714046`*^9}, {
  3.741411465903193*^9, 3.74141149133498*^9}}]
}, Closed]],

Cell[CellGroupData[{

Cell["Short-range Coulomb-Breit exchange energy per particle", "Subsubsection",
 CellChangeTimes->{{3.7411688643589897`*^9, 3.741168870392864*^9}, {
  3.741336613245928*^9, 3.741336616860119*^9}},
 ExpressionUUID -> "f3feca71-e0f9-47e4-91f2-fbfc3aba4350"],

Cell["\<\
If one changes the value of \[Mu], there is no great modification of the \
error as functions of kF (the observed divergences are related to the change \
of sign of the energy).\
\>", "Text",
 CellChangeTimes->{{3.741410918468523*^9, 3.741410972604892*^9}, {
  3.741411025984765*^9, 3.741411066305449*^9}, {3.741411593297097*^9, 
  3.74141160867727*^9}}],

Cell[CellGroupData[{

Cell[BoxData[
 RowBox[{"Plot", "[", 
  RowBox[{
   RowBox[{"{", 
    RowBox[{
     RowBox[{
      RowBox[{"(", 
       RowBox[{"1", "-", 
        RowBox[{
         RowBox[{"(", 
          RowBox[{"ExRCsrPad\[EAcute]2", "+", "ExRBsrPad\[EAcute]2"}], ")"}], 
         "/", "ExRCBsrPad\[EAcute]2"}]}], ")"}], "/.", 
      RowBox[{"{", 
       RowBox[{
        RowBox[{"c", "\[Rule]", 
         RowBox[{"137.036", "/", "kF"}]}], ",", 
        RowBox[{"\[Mu]", "\[Rule]", "0.5"}]}], "}"}]}], ",", 
     RowBox[{
      RowBox[{"(", 
       RowBox[{"1", "-", 
        RowBox[{
         RowBox[{"(", 
          RowBox[{"ExRCsrPad\[EAcute]4", "+", "ExRBsrPad\[EAcute]4"}], ")"}], 
         "/", "ExRCBsrPad\[EAcute]4"}]}], ")"}], "/.", 
      RowBox[{"{", 
       RowBox[{
        RowBox[{"c", "\[Rule]", 
         RowBox[{"137.036", "/", "kF"}]}], ",", 
        RowBox[{"\[Mu]", "\[Rule]", "0.5"}]}], "}"}]}], ",", 
     RowBox[{
      RowBox[{"(", 
       RowBox[{"1", "-", 
        RowBox[{
         RowBox[{"(", 
          RowBox[{"ExRCsrPad\[EAcute]6", "+", "ExRBsrPad\[EAcute]6"}], ")"}], 
         "/", "ExRCBsrPad\[EAcute]6"}]}], ")"}], "/.", 
      RowBox[{"{", 
       RowBox[{
        RowBox[{"c", "\[Rule]", 
         RowBox[{"137.036", "/", "kF"}]}], ",", 
        RowBox[{"\[Mu]", "\[Rule]", "0.5"}]}], "}"}]}]}], "}"}], ",", 
   RowBox[{"{", 
    RowBox[{"kF", ",", "0.0001", ",", "300"}], "}"}], ",", 
   RowBox[{"PlotStyle", "\[Rule]", 
    RowBox[{"{", 
     RowBox[{"Green", ",", "Purple", ",", "White"}], "}"}]}]}], 
  "]"}]], "Input",
 CellChangeTimes->{{3.7413221639125347`*^9, 3.741322204366685*^9}, {
  3.7414109808000526`*^9, 3.741410981942337*^9}, {3.741411014298759*^9, 
  3.741411022102293*^9}},
 ExpressionUUID -> "2eb4ac15-e08d-404a-8f37-6f3e14a4471f"],

Cell[BoxData[
 GraphicsBox[{{{}, {}, 
    TagBox[
     {RGBColor[0, 1, 0], AbsoluteThickness[1.6], Opacity[1.], 
      LineBox[CompressedData["
1:eJxF0Xk4Ve3XwPGThIxJigwZMqYoCTn3ckJEhkhmoSgpGYtKdfQ7SskQSkmS
UKRSPCVJJEVJ5ylFHnFUVBIynpBe+96b1z+uz/Vda+37QnFbkIMfD41GOzeL
RiN+O1kcq6r6V8aYRv3kJnoKt6fep1xU7uGl0uh75vmMDSzmll5LbJqZVzUa
16hL+DpjgY7Iw8eZ3TPzP46PsE1Df1LOort85xq1F/yambcsv9/5SHlwpq9N
3J+YkTE0vU/X2qZneEhyZKbL6Q19ck0YpVxKFxUoPm3A/3um0/4LWbOIOTbz
/V83dTjD3PEZf2L2nWwM+TMz/3bzLd3i7smZvi3lXm/tShpj+n2bd+w7f61g
1ozrXzv+XLiThzE9b2a42uS48uxp09cID/7wzeCdmZe6G2yslMA/05NkNqWe
sRKY8dwY7e80/rmUK+nHekUhuHratfQx597k9qOClJ/SezRv0iu4QpTZ9I9/
dndlhIjMzDvt3GgkvEKUcjO9ga2ZdKh72o10i7WCnd15YjOd8++Q7M2V8yhz
6BnHfZ9/Sfx/uxg1hsj2TruLvqDfVNbRWpxyJ/3fnOJncQXT7qEnuCqHVAvM
p9xPtxJNkRnfMe1BOl81z7NVNdMeoj+JCA0OUJYgzRyhH9H6tDg7mjKNSzfq
sK/50D7dx+ncs1VB4rCA6pP0EquViy0zKDNnoeC/WU+ZY5QZs5FWybygUhdJ
ynPQN3+mdP89ykx+lCvXX60muZC6J4i2vfHa6xVGmSGM5E+8lkr7d9piqMXI
uLpBexFlcXSu/1YgXwJlmgQS0+B+0xyatiSK9Vnna+cmRdp7EaKln2oPq6TM
lEYH3rx1O68qTd2TRQOCcu/LT1OmLUEBpjvsOwYoKyiiz4du189xXUy6SAl5
lHAtNB9TZixF73rWVduqyFDfU0W2KnEQFkeZoY6eezY+SPtFOVgTMc7J6ZU7
y5LmaKEHDTuKOI8oe2ujVfxFy+YslSM9byVSjjRRsu2f9mqUURR3KdRJnnqP
HlrwvVEqrZxysD7ic9spxoldQtrfCB1NLjrF20c5EqGozoljqZoKpCuN0bCc
+WRpEmUPE7SqrNvoZfV0N0V7nRIPfByhrLMeFQzo3u/TUCT91Bx1JTQPzfKk
7LEBKS07vGpBEmVZK+T1XDFYtZryxEbU/Dfgh5WGEul+O7QgQ0zD04OygD2y
NyjZEZRIWcsBvQj+05EyTDnPEfGJZC/JU1cmPbYFmeabe5a6U97qjMo7Eptb
qygHuCHu4dUL+4YoC3ogvcUfNs9SX0r6mSe65aD0WiWB8iNv1N37TNigivJj
H6Qat9vKaohy7TZ0ubqkZq+bCnXPD7V6uc6OjqcMO5DUxB9GSiXlIztR0mqL
8vuqqqR1A1A9+8fvOlfKV3ejuYFJ+q2nKasFomO5H+7SBilrB6OKdUf656uq
kRYJQeMflVaouJJmDoSg8IV78i0fU24NQztOTF5OjlMnrRuJTPRgn8lDyg4H
0JLPh60GuknTDh9EzfBnyN5Kg7oXhUp66C9mHaSMjqCk9KjLd/Ipnz2KLEfG
LcXnamJXrolGqjlGS6oMSDNGoxGPw6GhYH/Kj46hsptjmeznpJneLKTl93sw
8fgycp8nFglIGNYZ3yNNo51EnZWRmX2dVOc9hTJluRvs1muR+5qn0cEX+vJ/
w0kzNsYj58iIwVs5lPcloHmNI5dEeZeT+2FJqCd6TViFLumsRWdQnfb+DXu3
k2ZUnUHH4oYHXj2hvDQFDZoMWcRHryCtcw6x+3Xl0B3S3jxpqDAzbKCHQ5rT
koZ8xwYyrBna5HzWBfT+zq9fQn9Jc45cQi23z3/2XKRDvv9kJqo9btCgp02a
k34Z5ayOvNq5lfSmH1nIM2nUZn0FabbrVWS9M81A7j3pYFoOWgv6ysM/qX4j
By3s2c/NkVuJnTQvDzVYjGTzHiYdvDAflcufi29NJb2pMx8VDOtFlhRS/UEB
OnF1n41vK2nv0ELE+Ds0Wm20CrtfsggV28eoLt1MOji5aOr/LbmFFUD6m/gd
JGK55q7ZBdKRi++iluSIPTUjpIs2lyCbTv6LKqK62Ne7S1Cl/vm6GBXSG2L+
QddaS1XNHUmfr7mHwlXHOM/ukP4W/gB9jTwlplZHmq1ZhtxeLoYTHNLNX8rQ
umCjixZiq7G5fuVItCxqS+0e0pxLj1G0sAhLnUW6xKgSDW29dDf2Iumhgkr0
3+wKMcsXpNlJVei6zd+6OjU97D2HqpFMViJXw5h05UQ1ShhYonbKifQX5lO0
L43BsoohnXGmBpl0RMPLT6St3z9H/+jOD1w2Rlo2qBapH8++GCe+hrRQHRJb
Vs3dyCBdZP0CtYbzFtdfojq3Htk9T+3Q+od0zo1X6Im0yrz4etLsbQ0ov2J9
oM04aVrra7Rf4IRag4s+Nu+Rf5FYxtyM1xIG5PzfRhRqx57UXE7ahPUONfKk
+Rw3J+0r9B6d37VUDR0g3aXYhJT0je8WtJFeHPIBsbrnSPJxSVsJt6Cvl+oj
fMQNsaMKWlAhrxuSMiO9of8/pPcmvDYmn3Rkdhs6H2O0rOMJaQ/ndjRmwJNA
byXdzM9BFZcTNw+KrsXeVcNBGwIL2rzDSW9y+oTcBThDRsZG2GvedaKKh3nO
aS6kPWy7kEJQYNlACOm8ui705d3Y0fwc0i3PvqK9VyWFFgnSsU+0fkdsp9bA
UGXS7J3dSFfwKvsVnTRzuBtxg3XOsYJII6keFA0bFQcaSS+K6kVffomzbHpJ
J8r0IfPc5q7r/Ai77FEfEhTeUei1lrR8TD9K/cDUf3WZ9MFPv9C18Hs21wOA
MLP2yxBqKbKKcjiGTdNdP4yEf7YVTFwgu8i1YRTsxy9gX0daJmgErXVyefJb
zRh7vjgXNeiPrdnYiU3bkjWOZoUn+A1PkD1PegItdhF/YSfIwL0wdQJZp+Zy
fytiM38k/kFFwg1bbO1JP7z4Fx38Iz9v9DY24398PJAis0ut/iHZJ+15oNCw
GK48J/vhTB5o32cRuLEdu/L02tlg1hv04rLoOuwNR3lBpL2StSEQm3YD8YPq
H8EMuQPYjLx0fmDIbCkeYJFmc/kh1Pl7R0YGNvNpqQC8fy1u/OsleS/SQhCy
Krf9vqBpgt2YLQIrxWoL9uhjMz/KicITz+UexmZkj00Xhc9joxVfPMneeF4M
VPXiWdpnsBntjfOgMP++WM0oNsdrngQgrmxVGq8p3h9zl4AG82OhAeLYWaeu
S0DfZ+t3YsuwOWfMFsAq+U/pblvJeVasJJQmC6v2PyW7mokUWHaEND35F5up
nykFLdpNsWfbsGm+41IwXn/lx1oueV/+gTQAv/6dmGVmhBV8TWTg6SEfukwy
NjMtQR62vHj282cmdmX5H3noktK6XHkDm7Fs7xLgvzcya0cNdnCEhgJY9cc9
L+JiZ+kuVAS27z0Hc6/12G3zlEH5l4Tqx93YtDUOyrD/cMjvsEhsBbNUZZA7
p5V15Qy2TuzipRDwPPvnRDW290dtFeDVTIwtVjcn3L/oqBo43+txt9LDVjhd
rwYFJlbaHeuwvV8vVgd79znvRd2xi148UIfM04eUA+Kxg5/M0gSDvp0VCgOk
dR9qQdyhmjP3J7HZOxcuhzZ+ZT9bIQt873jocohRaBOKWoqdFLd8Bbyxd3Rt
csLW6bqlDXtKGEPxD7Fr6cEr4coBac1x1gbCBkZ8euDxwnP7gyRshhJDD6Rk
sjMiMrDVTx3Ug4RyTbGhYmwdTr8eRP01Gur5hM0s/7wGnGK2VrQxLAnHcj8Z
gPj77NEMa2z/LSqGUK/6VcfdBZuxzt8QTGuDrjYFYTfX9hmCjlB0LDuT7Hfn
GIHgmasOTyaw2Q9tENR0fI1jCljhe+EXEDBXadXAAuzSF50IRt+W6D9chi3l
yAT4svCZbIkbdu1wuTFUZHzryi3FZl/TXAeh15cfOhm+Ef997/GaQa5GvO36
aOxNLEMzaC7oUZyVgC38ZK8ZoJs3aiOvYfcntpiBwF2Nhf4t2Ndj76+Hyw9V
7pgzrAlzT52wgDf0GBaPDXZlQbUF8FZ8ca5wxb6+nrYBAiqvTuqFYdP6D26A
NTWK1ip55L7mfkuob5D7OlvYBvcO1kb4a3e47LEUdrBw3UZY9W9r/CEVbOHH
ItZw/u3F1YOAXV9+3hq2N0sf+xRCdp1/bGCsQ1Kuqgm71YF3E6gNi2w+ctWW
cFdpogM8Wet42uc2trdyqQN4MNNrzB5iCzRyHCBZSM1A6C22wVzdzTCpyJA7
z2OH779q2QyNtqFf7/hgZ8w12ALrHH88GhDbRJjTuswFRCMS3L5IYi+t8HSB
1gsrR9/JYGv9SnSB/e0ROg/UsNVth12gMID36lFjbKvealeQipaLFQ7C3iMX
4g59N+0cVBuwuSMiXpDZ1/v391vs/kxLL7BemXDz1QfsvCsxXlBQUi+wrxP7
aemkF/g+tHxcPYG9M+OgN7TUmmr5LLMnPPLjgA88/azPlxGL3bDi0nYIU2kq
DkrAvjivajso7dzvY5qKra7auR2OdpeUd1/GPvBzuS+s/bUyzPA+dtpAlS/c
nlzGed+J/WfOkB+kSyuUiZs6EI5nR/sDa7B+ta8l9gfDIn8IenXg9j07bN1v
bf5gFv02x90De60k2gW9344n5u7DPlk6sQvWlf70NbyOfcr35G745vRQzEdk
M2E/j5a98EbH/1SxBDZjVDwIHglKzuFbjB3DsQyC5Iq9YwWq2CmXy4KArqrU
OWSMLd5jFwxJw7FlsaHYTQ/pIaCf6uRX1ESYyX2lFwZO7JHkcx9x705zDINw
4bTKqM/YjrFhYVDEapKx7MNe8PFOGGjuc3nTwedI7H9z1QkHeSc3Y4k1hGkB
Fav3AZ/UVun9qbjzKXpEwFLHSXOPdNz/N340AkyTMsNNsnAvo+VEAFOg/bVo
Ie6/4noiYIzrdfxaNe76+Ucj4ecHn8HmAewl8rcOQONFv1dG9lsIe/7QioIV
wRK1Wc6EaQXtrlEQa1b1ZM5W3EOFTkQB+ilb+joA20DwUxTkQWP2dhZ2Tn76
YYjsMImMu49tcWHhUZBVU1D+T85pyowIM7lo2D/+So6xFNvWVz8a2K8PSeVq
Eqa1ZdtHQ0xkk0iQPvaZqOPR0FuXwOWxJ8z8nPMrGir3/HmlySJcWd/26hhs
v9sSebAbz9/NzWRBZi6LVdWP7280LmdBy/kVSQKjeJ/5+wML7I8eu3ZutjOx
v5QtGQPG1prv78pi9wkkxoBM1wHdH7bYLx+dOA5vpaV73YsJM9+1J8eCqEj1
7+wH2BblJbFgRQuc0/0Yz+8ofx8LVV2VspH1hBkL1GVOwu1i/42pnbi33849
CXE2pdfrF7kQNkmrOgWm0c7bURRhxj/7JePh7vshRalj2Mu9DeNBSSuZM3CC
MDNot2c8zGqq97yegvdzvubGw2MtExeJG9hKBwwSwKhZy+b7B+z2+b6JoKvN
o39W33XKnLn/dSeB8sdCwZ8DhBW+lKakQMML53Pmv7EPKhemwMFSHqWsv4Rp
8rlPU4Cd4mK4WdiNuFf7czgFjljx+j9QIczUO+eaCs333WtiXAgr/LBTOQun
kwWZ8hWEGU4vG87BsIX/sN1J9ylnXRIPTIfGNL7VKJGw97a8k+lQ8jUnVPMs
doBDXjqEnujo471CuDKsvz0d+p+5dT8oJcypXu94EbrX27QrfyPMWOi9LgPa
TFfVjZp7EO+dzF+eCc+NJzIu83riv9c19SvwSe36dSEhwgqPjhpdgUkxx5II
ccJFJ3faXoHVnBsv7eQJM574hV+BLKb72F99wt6pclVXILKqzNl7N+HK3mjP
bNAwPTBf8Q3hTYHO2VchznzkRPblrcT7ZIS25kGsTWZOfy5hxoUL4XnAcjSv
gkLCWSKGcXkQte3cWEspYZ3xgtI82HtkTaDEG8KVbPcF12DTvf0OLF4v4vtn
uQ3XYKHqqOyOXYTnMV3s84HNM9GcKu1NuP3E6UJoUd9V3/COcHNW0J074Ol0
0ufTFZ8pqz8bFL4H3i8kt+zx3jZlF9EvL8vg9GJVfwOZ7VP2/W4sUQkrQ7/L
tnUS5sbv31UNTvOkdcayfYn3PBD7/QyG/hn/0hfkN2WD5HdbX0KZ/rYHaoY7
plw+IKLCBhpNr+fdEOGlZeHlb+Dx67JKz8qdU87j5/32DiY7Cwfdj/gT37Mv
Rh/Ar1nJPMNg15RXVE10tcL6NxvX3uMJmHJ+7sQtDuTO7zht/pjwd+s7fJ/h
iJtGdFHc7inzn9X+3AlN3z6+TbLaM+XB3SFfv4GGxtWTnVV7GE4uu20/8P2A
/wOtDK6j
       "]]},
     Annotation[#, "Charting`Private`Tag$38625#1"]& ], 
    TagBox[
     {RGBColor[0.5, 0, 0.5], AbsoluteThickness[1.6], Opacity[1.], 
      LineBox[CompressedData["
1:eJxF0Xc41W8YBnBJkhktm2SUVBIR530cEqmMZGVlFiESUvnVIZUyk5WEjEIq
ISLVEYoSspOsipIiZCV+fcfBH1yf676f531f37X2HkZOzExMTPH/fmF/TXUC
y8reCakzkT8ZEdacXdFFpFMoVoekmhyvvprPVXSWPb4T0TpvabU/G6rD++ct
ojTWezB8gnRuKTdbfqjK0imGKUwfjm9fQ5uez3tpQ5ebjv+dn288cH9b/sDs
vO2vFf6s2spEZdznwGGf+DvZi+ZdU2f8Y/URZtJ0itYORc2L6xbP59s5R787
JrJQGfv48zzVJcKXUhn3iR2+784avmY+P3xpNjkqZP28NZXAR/PJgsU+/bdn
ZIDh3NKZyKdiqYIbSD+mtMHfsf17GM6lFAxSXi86Pe/SyAT/5IdZDKdQ3HaX
etu9X5jXHf+jy7tMlvGeUul0NbEyFYb/fTOjM2OezrLz+zrnSqrF42Xn50vu
TSfVv1rox1qqetMmFnxi2WldeZmN85ZzmhqNuMhwCmVUc0wnLGDz/P3rh7eJ
oIfzLs1JOjEy2L15vu84PZK4j7plfh81U8FrxoPhxxQRUy+dnOQFTy/OE7aq
W3DLw1+/OOa2zO9vfxD/yXqN/LyrLqrUKm2Rn+8XWrc95tKZzynpin5pX2wY
TqFEcfCHP/VdyGm9RX4x4Qv5sWIzB/fbC7aOnNDb9WzhvH1H4lREWhbOUwXl
db9/LOxbv6qV6+2SrfP56kHfyXSRBbOUr/7kr7TgkeuFb431ts7v7/Y0fSzn
NG9Krc54Kst/DDMxlYrGhnVELzj7t5JfQQ7DdEp8TbN9aAXDKZRLaT56jh0L
9j29SoUyttB33P9IYiWnAukKitF6E67BdQrzferc2ES5msJ8vz3qpFvlOMM1
FG/p6e6XD7eRrqJwl/ibVLkpkm6gZOrNVVfLKM07fERM5oopwx0Unzhq0J4L
DLdRvn6rz8tOXMitKHY97AULeV34Lx7XNwz3UDR7AuBN74J5NpZP7qVuJ/2Z
0uHNkl9zc8EvBKSWh9Uw3E/JerbLXe8Pw18pwrwtN+7xKZMepEQ6HH7NJcvw
D8riwvFJd42F3JftkkytOWnaMOWbxRrTzZ6MfJhide9OUPilhVzTqKpHv5CR
/6I8Sjdf/uAtI/9FWT/xFXi+MDxKSdQ95e4xw/AIhSdxWWLdChXSvylNzHF2
F7VJM01Q4l0kZdApRj5Jsa5/ODh6l+EpioSyel52J6P/h9J/s+akHe8O0nOU
HBYLxK9FmsqEuB+Lp5ywJk1bhDxd+5nrfBk5M2oQve8kG0mazoyUGryrLmQx
vBhNqzCHUzoY+5egZ8kRB0a5Vcl5ViR+wLRQfz1pOis6zyoikK3BMBvqK/50
ZokladoytNs9u9PWm2F2lC1+XKM0jDQTB+JqUk5fc4eRc6IG1UqX2veMfdwo
9pbRlgucauT5y5ElW/eYmjppW1707Mltszhz0jQ+JO7hXjJynDSdD31unj6X
lU5afCU6lraKYw07hZxfg+pNO9y91pFm4kfb2NPq31JIUwVQ7FOXbRtMSYsL
oklP+dggD8a8ILKQnJjsCibdLYRKW59aqqUycmEUAHvXjjSRpomiz794g/R+
MnIxpJ3R1pe5FJHniaNM82RdlrWkxdcids7DOYdUSdPWIrfncjxPDjByCVTn
NXp8tTvpXAmkIF3SdPwiacN1KPo9TfltMun6dWg8VCdhfTGjL4kOUrn/nm9g
9KWQ6J0bL1SXANmXRne8C/Uyj5JmkkXtuXv8jQJJ58oizh+d2TPXSUduRJ5O
S9n2V5OmbkKpt25s/9NNWnwzav64xSljkvTwZsQmWHHNYLk6uV8eqZqav5iS
IW0oj9yiBofT1Em3yaPkWpqYvhlp262IRSfLP/UiwwqoVnl6+94vpCMV0SLv
cKffM6TllZCgOe9rA3Yq+T4ltC86Y3JqLWl+ZZTLWWuiv5901Q5ULcvvvs6a
tLMq6t1tHzTpTNpWDa26MJ6XSmP0Kej0X9HlEw9Is1DRNSEXmZonpP2pKGdH
Ptx6RforFXX56Ljv7SLdpoG0fnq8TubWINy9E1lzlvR4C5J21EK+sixTutKk
B7VQ5uF4mTFEmlMbcXXRg3a7k/bcjaT/sieKnCLNr4uoQib5I0Gkq3SRl9m3
nsRE0pJ7UUsdr/qvN6Qn9dDQD0vTl62Mvj5i47ztfuMT6VADpLZbNXHXH9IJ
hiiFbj91XVaTsJER2spTle2mTLrWCL2w3mSlrkVa/wD6ND3x7LM1aRtjJK0U
FrTlKul0U1R0fkSJOYk01QztbjDrb8om3WKGXDwk9pyuIC15EOVkFfFUTjBy
S4QmhcviWHYSjrZCtdqBXkd5SRtZo6FP+5p5NpJusEEKor0JFjakOexQuZvO
vk2upE/aIeMnOX/nTpL+aod8zE/aZlwlXW+PHkdxSg9XkH7piHR7jre+eEda
1wm1b2kNjulknOeE/tTc+q46SfrzYQRLlR9e2KhFWMEF1Zkk2purkH7ngmzT
F63cuIu0+1EUoFHjW29D+okrqjhjRxGKIu13DJm8fvnjRxJpeQ/Uxy+XTL9L
etADLS0cX3S4kjCt2BPtGQ55lTtJ2tQL1TsWGmkf2kX0mXzRul8rpD+6kj7j
i3z/Oz51wo/0rC8SiZVLuXWVMI3ZDx19lfpjppzMlU6jpweYyq7Vk/mr02h5
t3W07Ecytz6Diib51czHSUf6IxbZiOD89dqEhc4hs8JByz1KhGkvz6FszT1b
ejQI01VpaL/lkhZuS8LUHzSUFHpm3dEwMj8SiFSGjjwTHyFdeAGFnKm8WjRL
ev1F1Ll0nZM+hw4xf/MiuiDeyeEvSTrsEmrYb3yw1ZQwPfgykup8KHfMgcy5
riC/ozxMSzwJM0VfQWLnX99WuEzmWSHIrYA6FvaE9HAYek5NeiVZRZgWHI74
3v5JeNJE7l8XgYq/FGp8+0FYfGskYl2zKUJLfDfRp11Ft04JyP4JIizuHI2s
Xls7FEcSpldGI36h1MSTiWRfMgaFl8ryjOUT7u6LQf5zamODvYSpZ+OQsiFt
092fZN4fh0ZSKg67TBO2PRCPXDT13n/h1SX2bbmOTC/YPOukEqb/SUC8LakT
iftIe91ANdL98pbmuuT3uIF2VnmktXoQFv+SiOQ5AoLrk8j+YBJiv5pm9GKG
cPf9W6iypz+ExrYH9/D0LURTkKuElYSZdqeiicYC5ScbCUd+SUWfV78ULrAg
TN2cjp4lfu3LeEz2Z26jUz/kxB0rCNMs7yBFOH5Qop6wZ+kddLdr6k1SP+Hu
wEwUL8HxMG71Xtzy4tnIK3PTmcvehA3T7qGMDWH6uwII20rdR23Zg2sXhRNe
nnUfoXt3q/zukHnhA8SWt2G1czvh7rFclPxE6qE2dR9uFat81EC5EMSsR1j8
fj5iefbZ7NlBwn6LCtBRetqs0gnC8XcL0PbKtfukbhPu5i5ENbUi/Ys59Yj/
18piNGfwX8lzftJnipHCu46wM1KEPT8Xo/jGG4qjQPhxcQlyaBMI7D1OONi3
FE33rBIpayXsL0pHmxx8hv0/E063oSPbz03lKr8I05PpqLLv2tFcdn1iXrIM
RX7nfZyMCC/f8QLJ/OY6cDaNsGJkBXqhahxq94CwbXsFsqIlVGo9IewvVYmi
OGRUOBoJWz2rRLNrqSLxzAa4vf+8RE36Xv0P7QhHZ1Qjj+jH4jHuhIPmqhF7
++xBv1OEIy1eI6pTSA1cJdy04g26eyb94Rs64Y5rNUjD+PvTER5D3MI1dYj7
ZLjF51WETYXrUcf1rRPNQoS1DtQj366T8sUyhL++qEc5R1nSzqkTpmS/Q/wB
IsGcHoRvX29EfWl0yVlvwjXtjSj/pUPZ0GkyF25C+pzZ0w0XSac2oaC47e7X
kwjXFjWjoXsGRtK1hN3Y2lDS0M+5qUbChcZtaN/W8Htv3xN+casNZRfUsPl8
IewN75HjE93n5TOE2QPbUXvVTjm7jftxd277iILZP71X3EpYM/wjUt4XeIlN
mXD4t48ouo7e+0CTMH9aJzJoQddnDxKeXt6NKj4psyYGEzbN7EEnpFrzPcIJ
Z3zsQRJHfO12RhM+t6IXnRsoKB1IJvyB1otUf209saOI8CH7T+jB7Mbuli9k
X+MLShAQL+HdaYT76qlvKGi0RtFRl7BQ9Tfk8fbUg0IDwgECA0groDHd0opw
TekA+vn1YkSGD+E2rkGk8fiH445Mwgc+/ERyUQldIfcJq+4YQqvddCw6Cwiv
jB9CA2K3DM6X4aY5yA2j6EvGqm/bCS8bHUZfTZ/w2HEdwPtwfQQ1yDtfyV9B
2LV+BD1lX7WEVRA3bRPbKIp6dmw6W5qw5alRRJGW+DKmTvQv2Y+hyN/BJcFe
hA32jyPlaFOn3FbCMVnTyLR+PCr2IzH/fmgaeXPG0f0/EX68/Q/KDWoV0h0i
+kde/kGyPuYNPazGeO74YwaJmlqor9hOeKvlHKJETbtNqRkT3/PuHLKsTUjo
0iDyM3/nULz2h9939XBT9+5nAj5lqxwtJ9z0wmkmYOW3EfCNJuxwiBkkjWe1
rRKI+fwwZtgZmeStmULYqZQZaGxdddw5xHkzgothevLQxTvlxPxEx2L48d5u
tG2E6Pd4L4GmG05v1fab4P37U2yw2XNFVYoZbiq72jII1ip7scQGN23afxmg
H8KP644S/RhmdrgNTakOQUS/fSUH+PVo+oUUEXmYKRc0PBr2Gn5K5LG3uEDu
SpK7SQWRa/3ggh6FaXuxd0QefpEb9gQ91MsfwE1nK+MBYRnxdR9ETDGnGG3k
Bd8/b0Wokrht1U15ob7uDH+GLG7qpQBeuODXyuWhjJtpy3te+FkdPsm8n+j3
h/IB3e3vW9kgss+6Ehzy2v1ODxD5Xp01kJQRFFQ2TOQj/62B9vjNkWwThFke
rYH95wLvxC42w/f7SfKD+j7ZljxhwjfYBECo79S27/q4xc/1CYLp+3XqCiaE
DSSFIKrm7Z5TloSv2wvBsvy19kudcXcndAvBxLnqyHUBuG3de4WhUUDgp2U+
burAX1Hg5iqfSi0mzsvcKQZ7mNyXDDwn5gcui0FZH13Yrwb38ByHODzId94b
/YXYt/umOIToPc6sWWOO/39na9bCzgAzB+SPm7bIURLyWsbW8gfiZuIOkwQJ
uajukUu46w8VSsKi1hrrzGu4U1qXScFzOU3zFXdxR4oWSIFam5zet/e4u11W
y8C2LczKMcoH8fcWrZSF1KDk3x4I97COjizwtVMK9uwkLHtaFn4FndzKZIB7
+UC3LDxoH9zoehg3zS5vI2y82CquEYPb9pLTJlj3MYf9xwju9YOX5KH2tVms
9hRuZ88seTj9mFkiZQ73pNwbeai/Zr7jAKcF5lxjnq1wdg+Lc7EUbhW7hK3Q
VmRZecEcd/yjJwoQGsVOE32G2zBqkxIo0x5x+FXgjvxoqgS97rZx714T+TGa
EuzQLbwf1Iq7yqJJCfrm7D4ODBPneZ7bDlT3YtWidZaY2zp7leG3jvNvg8u4
1+v3qEJTHKsiisAd7LRcDQr6071kY4j+C3U18LrUM8RyCze/QbIaDL+0GCh+
jNsz344CA7v0utZ9xZ07NYqgc6dC9YS2FWZvp0wqPL1Wv/TLPtzBsRVUSPx0
TLvBCHf3UDcVLM/fLc+xwd0hKKgBbS8kn9n54l55MFwDGjTW5L/JwK2VcFYT
XqnPJCazWOPzZ85pQa9MZiYHB+HmNC2Y5TEuOMmLO9qpSgsUu+++MRDFnSvD
twtSaJbTc8q4c1DmLvArKzGzdcXN39+pDRt2nuJb24C7nslPF7Q2SomGtRH7
o9N0wXbFuw1Tnbidnet0IfbTeo1333Gvr5bZA8xBbR4BS2wwywV+2APtFcpv
e1Rwu7Eb7IMQ7fFLqcm4U/ydDSBYLyl9OAN36fEbBhBkrF0GObi/ZtUagL99
7HT7Y9zc44KGcOzsdvcVDbgj288bgmGhr1EQyyHMQfut9sNq6Qnhwy64c+bW
HwC+Tck7Cjxwp/LoHABuRR1TZl/cY9pOB2CpZlxEUiBuObnUAzBprczcegN3
W4OIMXyIOdmvU4vbsUTYBOqZZ9qiBWzx/byqZuBcVE2/IIy7b9LCDJjc4jJ9
xXB3svqbgXyzgp+5FO6SuGdmcPWOyxrhrbiFI3aZg9G+VpO03bgLxi0OQnNM
XsPDk7jH76VbwrE9tJLU07hV8l5bAuucXuq1/3B39Axbwnbnb8d9zuOOL0dW
EKsqzrsjgtgf894KzLvCDOi3cYvHCNhA+3qXmtpm3C94bWwhMuup4FwbboMq
H1vQluVz2dKBW/pGmC3kbXyyJLIXt0/sU1u4splLff8Q7kP9onagpvjwYSOb
HeYdbP12kKg+FdumhtuUI9wBjOh6X9jUcYtdyHIANo3UbTs0cY+LVjqAt+be
+uu7cf/Nm3GAfbtuLrM0wS1yyN0RZvZo+H88hjuk19gJrE0v2/Xewp3mgo7A
5mCzyx3puHcxWR6B2WKphy13cP985HcEkkReML25h1v/XMER6Pw8nZxfjHtn
6CZnsDnh1hn0DrfrbSkXsIk0sJRZZI/5cMxmV9j8QuT8Whbc33YausLs6Pds
oaW4mVZ5uUKSWfA0DxfueLFCV+gULbs+yY/btVXdDQ7dU2irlsct8f2gO9i+
XmXiZos7xT3LA25x2F8wc8Cd+KnWA3r33X+keRj3hrNjHuBQp71awA135XJx
TzjcdLK18iRuiyg3T3DtfH9QLAJ3vtCy4+A7ctOm4SlmWnuOoRcUbRsIf0rH
rV/r5AWT3tufZ5bjZmE54wWnJmrFzlXj88w5GV7gPzPXvbEZzz2G/3hBAKu9
w4VBPB8+mHMCQgWlnVWEHLA8W0jEBwZkpmbtRXHv7dvuA7pKNTFha3F3vDb0
AVZDr/JeGdxxvUE+QLvwTDRM0QG/r/5PH/AZNm3u0cM9sPGlL9i8vKQZQsMd
eO2KH2z1+ibc+QV3CLerP2TLbw9r+Irv42q77A8SQ4F/X37Hffhppj+sdBPu
fPALt8CHPn8YdzJIDviL+/5hx/+g5OCjtVKrHDFX1zqeBS2NAGk3LczUghJE
A9PlAvLTqZiZaG6BgTCYMMi6+TaeH1aOC4TzUvSPdln4/NCqnEDIVT0SUv0A
75tytQQCu9OjvvhSPE/+KnsenhXvv6ncQvSt286DlMMVdp9lTv9MP5SreQHG
Hv35POSB2ybIPBj+GOhVrDyBmWnlVq9gYB5IStvhi3vzWEgwLBfVtD/vj5mm
+/x5MGy6GNy1+jLuH87rL8Nh01XtKBX3WsHZy9A6vrkupAn3Os8nIVCibF8s
s+Mw9h6B4YAI+BC4yWs1BTNtNC85AmbeTsouUcedGvY0AsAxIrFXC3fQlakI
KI8sPXfTEJ8/Y7QjEmq+rdZe4YzZNvlRQSR8vPGmYTYW759qL7gKTExKg81j
eL/hWsc1UF9ziYNlEjO9jTJ8Dc5ufi+r8AfPb44vjoYZq/9cwhcdwealEjdG
w2RxZZ82N2bb0IdnomH4hGlPkQxmJsHlYjHQ3X+y5boFZnHuKa9YeF5XQrem
4/2Bs0bXgT/+YrFJOd43F3O5Dp62Rnl6LzGnHHx37jpI/PqWhmrwvuzRe9fh
Ip/AJZE2zN1pnssSQN/kpN7HIbwf11GRAJ3t29qtxJyx+1qE6ibC7JecUcuz
mMUrDcOSoerp+JhWAGbbGsXMZLgaQx3fFISZ1itXngySu5om5y7j8zYWU8mw
N/3P37QYzMv1TbalQLz9HrbBHHzeKzY1BRS6+oX9P+AO4bt8C5zaJLQTVVz+
2bA572Qa7PMfvVehhnk4ee/lNFAUr1j1AzDT7o4kpMFiZ6cvaBdm6oTrszS4
NXEnqGs/5hRJTtZ0+Lh6U7mEK+b641zx6WBiokzNuom5u8D5VQbsatirWsh8
9J9znU1MM0FbJvZM5hLM4oJeRzNht393aQIbZrpU0tlM2Cvto36OG7OnpuSd
TNh/OklrtyDmSO6ByUywlvil374Vs7zMkeQs8PGKdZi1xWy4lDaZDRl8PaHa
zzEzqYp13oOKbXmKfi8w0+iBk/fgs/H5jqxK3Gtm+O6DRJyUHFcN5m7trbvv
Q4rQ0TeNbZiXC93Jvw+JkqPL7EYw1ws1hD+AqO1LLp2RcsWcY3U3F85abAjI
DcGc+6QjPg8ey3kz54Rj3l3Bk5kHv2afnb9zFbPtB/2iPHBMM76YFIf3L/5q
zgPdwXMhoWmY6SXVK/Jh5dmWGOcnmJk86q7mQ/at89ni3/HzXtDiCqD168fG
yD1u2PvjNtUUQuDr29b/6WFuO3+4sxDkcjz6XQwxB4vcHy4EmseiP5qmmKmH
XFYVwfpxSYnfdpiXj189VAR+i908D57CXL+zaLwI+EWnOSUy8f03i+WL4eCB
1dr5S9yx+7vxtT4B8UWHt3exYXb23D/0BL7efyTNwYk5U+f20lLwYzdZ6sCH
+bFJlEopxJddq+ITw0wT9b1RCm1bePd6qWDOjQl0egqmnJyGW10x797jxPEc
jCsXWTyoxxzqomNUBtsl36zLaMTcXRxiWwb856N/JLRg/vq241gZdFBlAi52
4PezzAgpA8fSfZnWXzFb/XhXWQYn8uPGOZiOYe/Zl0F5AVG3Nl1z3oJ5pVaq
Yjl4M01Y2ShgZim+oVUOpofo0sZKmPlb04zLQVDkQIm6Gu7L3d7lcCver2e1
DuYCC67CcsiNKN9SaYM5N0hLrQLq/jtYszYc8/ot9/ZXQm1m1ozpVby/QcLp
nxun5EKjMU+a3vX75w0JYeMJmI1lp5P/ubld/80dzFpXwoYqoWaT1TvvMsxB
GWlRL6H6o03LqzHMwzVW315BFdsD1r8TmLsjQuf+edvcdoU/mOtVmlZVQdXl
5LjERR5YnnRX85+Vus2Pc2N29j17swpehtl9EFyPOfpDo1k1lCPHbndLzPIP
dna/BkU/BYFoG8ySuTD1GtLzmIxK7DB32JjwvYEgmZvlrM74PGuL1hvQ5m25
neyNOejmhrtv4PVnHfd3YZjZjNT/q4GGkI3TinTMY132KrWg+XJKwbIcc2Kz
tEkt5DNVuQa8xGy4ktOrFqJ9HD++rcEcmayWU/vv+9ykH36PefKGokQdvFfg
uRQ/gllu8yH2ehh2m1p2ls/zn68862d/B4/sRVaMr8D8de6k4Ds4ba4hfGwV
Zll+Qdl3sETr8mYbfrzPH637DgSFBA6AKObpa/aX34FWtUri7AbMWrvPczZA
nJTf5nMamNO/PljbCFZCicoTmnjO8mhbI0jw0qkeWphFJ+p2NULOzNIDh3Qw
23TpHG0EemPcSXU9zIovdhY0wkBAEX3OHPOsbPi+JoDOcSOaJ+bdjyIjmoFP
1YaH3wvvX3e63Qx9MZVvHpzAHOxk8bQZwvWitbp88fvnpn9vhq7SrdvhP8xG
KuW6LUC74SYwcxnzSKg9ZyuUm/d2nUzDnHNO+l4bxBfoJvJk4Oeb0qrawG35
Q/M7tzHLH138uQ1WVp1715KFOSHlotB7cFQWKVfKxSwoGRL6HlhXm98eLcXc
8abLtx12N75182jBnKQZ6tEBWUtHVg22Yg60iQvvAHbK6ufO7zGb9r271wE1
6Ta89h34fba1DnbAft+hR8a9mAspm90/goUA79yOn5iZ1nue7AT3Q8ZXWViP
//Po8zqLbqi95qcasBRz6NBz926Qr0r89JcNc0pRHa0bRuS/KE1wYA66bHCn
G3yZfdu/8WIuj2/73Q20jLh1dSKYC0fNr/dA1Pf2R9eVMLtFRs/0Qo4MfOJW
xqy8496KT1DpcGt5kApmtqQh2U8w+eGI6zE1zEppowc/gU3NmPhODczeVSwl
n0D2Hnfo4D7MTn8LAj+D1rfjxXb6mKfHbiV+Bmup5r4WA8zfTtMLP0PkzRsa
ZUaYr8pHf/8M42HrJ2LMMbtI3Db7Ai+OadqrO2KmVk7u6IOO7IyIAifMXcU7
zfrgdx/b0w1HMO/tqvbug/WH6tasPIqZ5+aV3D4IN7B6+9UDs8TgL9l+sJD3
VYk6g/mV0CK5r/DrVxb3lyjMh1LEnQZAMNpw6FQ05tms7PAB0Nw+Uccdi9lu
Z+LjAWj6K8I3EX+camruqv+e9Tv8D7JXYsc=
       "]]},
     Annotation[#, "Charting`Private`Tag$38625#2"]& ], 
    TagBox[
     {GrayLevel[1], AbsoluteThickness[1.6], Opacity[1.], 
      LineBox[CompressedData["
1:eJxF13lcTVsUB/DQJGmipIGkSUIaDWftQlK9JtFAg0pFKSVJCDcqkZJKhSQN
JKRJwi1JkUol0aBREyWSpEmee84+ef+8z/fzW2vttfe9r3pLHD3NnGeysbHt
5mBjY/3bYsupZ8/eiGuxkf8kEqkXbHnboh9is7HZ7JKtc7r4cjo/ODFXcMXd
N9Nes2V2/q0L9diZzN+R7LukD7ZM2+Hbn1PGdzqm58mtn1j2Krx3Oufu8Dse
zOibzvuDR2o2eQ9M2+rz6Pq29O/T9frMh90FS39Me90F3wvx8cPT9UqO6muP
CY9M55Lqwx93hP/CzidEs720pMO5tHFOxAxmeHCGL9Cm+13OTF2PDFWYtvaf
4V/P16vQ9cycrUFyMttolxByKcLmgW7/8isjqae7AmgXEXP1NbJ1Lv/z8IAF
P0cZ7TKiKfKwe+kI7XzCqJvrqiyf6vT5RZpxr4JkaVcSaucURruJf77VnC+n
u512JiG2St/85j7aiUR4QONpztP/5s2oc812uUK7iOkjN97+Imu6n9nrd45f
/tW/fGeFGDrT/q+/SvKOe++vf+dv8Fp/dQu/2vR5ucUVr27J0a4lFIRtRrmQ
2nT/1T1f5Paa0y4h+B77m5e50y5iBvDODVQIpJ1PDNtdyw65SruM2Ju1ouNT
9j9/mFXIr1/+b76xhTG63UG7jlmc1uo+e+zffuoT+6+6CqjT/cw0oz+vXsnT
zifEEy+MLtOiXUOEDy2WP2ehPj1/5uZM8z4P2g3MQ7HagQZB/+o/fa7JTo+f
nk/YEA4dPLm0E4nq8O/8+ypo1zE3dgSgio/TJh6oCnksH6ddxFQITroaKqgx
/d7xDSrl/Qq0Swj+5c9H/9OmXUScOr5N/q4l7URipLrTnNeTdi3hKu0T6B5M
u51o9mHPqbxGm43N5GV0h9KD6XnM4oWyAmGV/87XcH+ABjr/+XbhZg+jCdqZ
hITg+6v3hDSn7xOx26V8riLtRGJW3sioxwbN6X5f7jPyVVa0W4nPOxdYrPSi
XcS0uXcrMPwM7Xyi+o9mztcE2rXERrOyDuM82u+JBylWAvdfT5/PVPj1CfF3
/zsvXv+Ih+ck7b/vFz87vnreGuwyprdJzZTiCtr5RN3MWIdgXdqthEaebUnH
LtqDRJyrjDwcoZ3JHJfoPxsXSZuNzbYm68uPO//yotN+JialtDsIaU2t7PRW
2h+JwD4OYc5R2nVE77XKww6Ca6dtsDWqialIu4i4y74TRHXWTs/ny5dKPGhL
u4Hw2tc7s9qXdiJRuyjDWTGCdiWhXutTFnSbNhtbXND65R3FtPOJ8TUzw4lm
2u8Jmy9lg7E///UXXr+w7QffOuwaptQ2izxjhX8+zSm5MH0D7Wai51HnMQ5r
2mxseh7prfY+tGuJdKkDG5hhtOuIuXWaKQtu0W4nvM5McR4sov2JWbuu1LWq
kXYHofY1tHLZD9rdRMwNs1VBvOun9x3dvjCyXZb2V8Kau314vRbt90Thk5uW
sVa02dikPD0eDx2gXcM8Ja0maRxKO5Poejd+8nbKtJm6Z599ZC+k3UTcJkI2
29fTHmTyDhqnPRn8t8/+ZOE5C3gI7O/MGotmD++ltGsJVZ7kmtcE7SJmTIGr
6jIL2r3EqJdyTKAn7XbmTplfo20htIcIZn2B9fok2mXMRaGBhTFP/tUHoP+W
DNX9c9d3wUCjr7SbCN3Uhp40LsBuZqZZXddnX4LNmCB4eF3u7loH0/Pdnyrx
P9lG+ztR7f3jgIgH7QFCRe5x3YFg2l1EdCND8/X1f/0j57dcUXhEu5LYoc33
+3Qt7UyC+aNuV1v/tJmLbl0tXseB8D5swNjpKBuzCNHzmR/nLgv5rkmbjU3n
2bc+w620m4lbPnlGaW60O4imTAN/s1O0Ownegdb0ycu0i5ho2cHGm1n0eUOE
lzMX99ZXdF5JJN24qjHRTrubeNeyyjl1lHY+wS1WEmUioIXdQKyzsCoek6c9
TLhHfhlM1qLdR1yvYiw2tqRdQtTyCBuP7qfdxWTfcts/KXjahMZpuGOYQLuV
cH36pnHkAe12ZvyEM/eN17SbmVWa4xr/ddMuI2b4hDv/nJzOCTErwXITHu3p
elVf6w4ZEdrDhGF06ujYEtqDTOfsb/zVK2iPME/UrJVPWUu7n4j9ehod2Uy7
hpnJW2VuvJV2PvFKUdRjqS3tIeZHPcfA0b20G4hJl7tXX/vQrmMKB41kJzFo
9xArk7XLD5+nXcTUe3auwzCO9iemQ1vd6JIUbMYUcfT3IoFf9+n8JzNK3FW+
8gntMuLu2hx04yVtDnhh+dvc9y3tTGbboS0e/7X9u89o1MVAqX56/m9CKPvD
1Z8jdN5KLK+RzSmfuYF+H0Lnq2f5dT7aY0xb3scdPmK0vzN9FdnH9OVoDxMX
9IwFFqvQ7iHSXOLkh4F2DfEs8CN6pU/7M9GUpGSRYI799/s6XOTrcdCB9ggx
t60oUM+Drp8Fcr954iWP0K4ltMXNc4YCaZcQO9ZeL38ZMb0v4W35uSM+fnof
Zugh1bEDafT8QSIl6rjAllza34mCrJfyEkV0/U/m+2pBre8VtBuY3wasLV7U
0/7I5Oa96XG1k/YEIa04GOj1jZ73i1ivty5+8wSdDxHbXQJzxLg2Ypcx9wdW
lX8Tot1AnEkS/ViyCFt7NiQWOY5dVqTzmQWr+cvS3TXpnAOKbVfYaOlgM34Q
Zncj5wptpevHiM7xX4VdtrQ/Ez76tl4P3ej6KYI9rnjJucN0XkRc6pF/axNI
+zshpx4WuOoidhE3PDw9pD4zYXp/Qq/WsrcunXYH0SBVEHfrIe2PhKuntMHR
Evq8YWK84MyE4Rs6/0qc4x24u7h1up4pbm1mN9RH308Q7t5+yF/6i87bCRiV
eBbLvgnP+0lU6Z7ydhPELpoBdpd6l8Ii7L8/H751Gr7jX07XDxIMlezgj5q0
JwmBgAVrHujQ9XXEjWr/z2e2/punsujjlZ122FIC8Nx9i+GKfXQ/X8H2J3d/
/zlM939nds0Wul8bSLuGecjqsH3qxemc4LzVLOiXQPf/IGJ+bnhucIfOuwl5
nVs+kvl0/p3Ij+SVGyyh8yFCv+NAffEbbG1eaFpVH3Kplc4nCbcTxLq9/fT+
s2Gi8kb/ulE6LyPOi3Ndm8uhM/3eEm7uxu2CtMuY9/Lf/MlepDN9PuLSzApa
Tud1zGrzeEerNXTOVWCfMmP+8s10PkgMDrmU/t5K+wszYEOlb40dXT9ECEWs
VkjeR+ftzKTWmMZDfrTHCdUVk+f0grC12aHkmAMhHkn3zwDz8hcDAwn/+ntE
la4X3aHNX+C756JpVD5d/5vgyhuZ4VJK531EHLtNzpra6fsSCtueOc1po/2T
eHRDTqS1/9/+BoOhLzNHaRcRH9B3v9Mcm6fr3cMsFC2ENk/vN/nhyQeFxXTO
CWGKS8ImlmMX8cCiI8Goag229hzIeNn/LXHzdH2BlsjWGwfN6HlzC2qc8sx0
d2FLzYel3+fJteyj64XA9/iBsYN+tDOZ5bOrK3mC/u0nGaOUeOMiPY+zwEv6
3ME1CXQ+SpRk9OpWp9OuJRas3yzm8pDeTwjcXiYNTD6n8xpmwTa2Z1E1tOcW
CLTbRiu20PWC4OT+ZM+zz3T+iflwVHS91QidcwBPkC/ft5m6lO0XgZ1gXUcQ
P7Y2H2RdW/1AQgL77/eNXfFCSI4CdhE7WOZ9sTZQp/MFBekbDVZ1bKCdyZyq
ujXTzxi7XQi2WnO857Om83ZmSq/j7dQ99PmiMHqwyJ/wofNa4j+2RaZvGbr0
e0HC+WNL3cJoC8B30cYRtiu0RQp0UjXKY29iSwlB3Oroaytz6H0XQH/Bd6/S
p3T9EIEMTHRsKun6eRD5/u6CHw10vTB0O/L0n+2m92ki1nzbUyg1RPs7EXqs
9OLDKXreGNHKtdTZeM4WbC5QiWas6V6AzTbBDJJqneMvQ3ucaLi7vk1oNe1M
Qmnt5ezbQHuUebJ0JEjbgJ43q6B26/Yd9RbY2nNBtjVLaf9uuv4L08+Nn43D
C9teECpH3N9e9afzBbD4dPlNlbN0Lg7e/ApHX12i548QL64GGdknYReJwUKF
TqlfGXR/CeGeqz0c9oTuF4an2gkvZcqm71sg9HriypM6Ol8CLjt27DfroD0P
HnXnbfg8QM9jY+P1ni/MGMduFwH7qQOfRLj08OehADnnqp/cm4f99+89zgUr
LuhI0Z4LO5PPOX5Qwi6aD/dWfVL3XovNGCfYmJtnz9alzQHb9ZKbr5vRZoNb
dWyZGrvo8wRh3N7u9Ot9tEXBeOCJhZMfXT9M3DiyUHEiEFtbGWzKbXc/iqD3
GWKKiifFH46n95kBb/f1vFNPoy0C4UxF/uEcvenPx2Cup172U+xBKeCwywnw
qqDnjRBFGb8er6zHTpQE/z/rh798pOcJgKYpY8Wdr7S5YCixxMV1nO7/xcz4
zp0oz6mP95UE141Gjd2C2H9/HstEXRRKkaQ9RbR3vvvPcZk+/fkUXFUTC5JS
pz1BWATZFbZq0+4hBN8n/Yo3xJaSgEq5XmVrKzqfByGHl7stdKLPnwGbyjyT
6z3pfFHBlGhu86Vj9Plz4LHrqPD2M7TnFhx6TJgIRWErS4HynICQmgQ6nwX9
1qXPwtPpeexw8+7sCcM8Op9R4PjbSG1OMb2fAkgaR3q8ek3nfNCQ8P7mmUa6
fylEfxNr39xN+zNhor1rIfv3f/vxXEw2K56cng8MFaVSNN8A1/8hfr3N1Xyy
HFt7JmTLjHkd0aTzIWL/IUjX3IQtpQLLXgR0/jSm63mgS+SFRO5ObPtlcH0P
j4W3C52vgp35xheUvbH/fv4is6PKvh7HbleGNzvqZ9w7S583QZxPF1+/7xJ9
nhDoTezyWXYDW0AeZhmm3Ou9S9ezQ2H8p57UfGwGLxwZUJJyKsFOXAhq6MAO
6Rp6v6UwGP4gsv0DdoQc3Gkbq0jopef1ES7KiMP2B7bXcpAOOIXE/9Dny0LL
mxeHG3n+w/eZCXHSc7JiRWizwbaDJn3m0tjtssBXErV0/kpsU1kon99gU7uW
rheBIGeJmIjN2GzzQTvPvtp4K50vhEnOVO65tnQ+xXxo+XlDxV7aHOCdtuLY
WR/aCpC6LMx4cwBtNmhI/7JkRjh2ohzwKBn+ZF7B/vv7Ce7dKfO7hR2hDEn3
3TwHi+jzlYE7e5nI3iZsPWVYr3r289JeOleE/bmfmG0/sJUV4Ia6XsRVNkN8
fzmoy7u123Iu9t+/X7jWcGnOE8NmU4N1j1x4quWwE+eD+7oXLedUsf9+f68/
kc3S1abrNaGWCAqcaYQtpQzshV2WhTuwaxRBU0tn+VEXbG3hArei5Cn1g3Qu
A9c2zKr9fhJbVBlqih1T753H9lKAWTrFfq6X6X5J0ChdYih7E1tZBVx1AxZ3
ZGNnKkD8y/ah+Kf0/mJQpaf9wqqSzpfBjPLrl+c3Yo+qgtp/f9xrurH//v3i
UmmnfX6Ivi8PXDYqnKf3h76fHFRWSfbO4jWibKoOf0yOP34qis0mBSpvmsOO
yWInSoCzGeGgqULnPAVxb6+q/UDYDAmo2D7Bdf8/Ou8kpt7t/OBmhd2+ApQt
H2fIOWMXzYHdDQtPfTxAWwNidhwxTziBLbUcypoaFHaGYjeowoT1mknhOHqf
BbCyJbb6TQo29wZwsPuVFJaFrbAeotssfPULsbXV4KV9nj5HBbaAGox3CEs+
q8f20oAVuw8N+ndh79UA+66652u+0/dTgkhntdjh39h+qlDaE+WWyWNMOU4d
Rvf8APcF2MpLQfGzmaCCDHaNHNi6ZXd1KmOvUYWIfsH864Cto/33/98OhFob
YP/9vo4M1NgtsMQuWwPLPJVV3u7GTlMBm8ELHBe8sM9vgAsHvjUYHKf710Lx
kPFdznPYgyowfDDjZHEMtpQ6yP+cu+1EMrbp3/p128873Mf2+/v7nHGlVOcJ
tp4m/Cptn5J/Sd9PHSLnyK+Z8xabWw1WbPU48LWVPn89lMXkpL/po/MNsLt5
rDN3BNt+C0wt0ZaMm2lCWcQULu8JtjjGhy2hA2r3Ki/YiWH7b4SqIaFXG+Sw
/daA65odM2VVsJXXAvuJ6+u5Efbe/yDhebdPvz523BZYO1spo8oc214b6oy9
e7McsE2VwDM6X+qSBzZjHvA0Te3wO4KtoAqpizdHWQdhZ+qCtnNoJbqIHbIJ
PqS/4ZC+Ru+3DnwHF2hx3MZ23wICGnZ+n3KxrTbAnWMpWRVF2Pl6oPusry+j
EjtaG9o5V8tENtDz9OCY4WHbQ13Y7YYgElkQYzWInaYJWfWzatZPYtdthpt8
qYH87Kb4fVTBZ7Xekhk82P56sGF7f8EQP/b5jcB3OHxnlzC2jz40X1796504
ttQGuM2si3q5BDuNAN+2w8qP5LFLNoPOTPHX6SuwFbeCoGyha7wqNvsmaN3i
wBm+FrvOGO66sSef1MIe3gJHw25pHdiMvXcTbMk0aHb8D9tUF+a/HfDbvhXb
Sxc+/owQ1rXE3q4DmaJq2Zq22GzGcHx9vfGy3djRG8HA7mi/mCu2kzGIBkiG
8HpiS5hAT3KRzJQPdqUh5LzY/ezbUewIS2B85rTrYNDzdcGYN328Nph+H1OQ
WGUUW3Ie+9MW+Lx1UDUvkn4fQ8jziaq5FUffzxQCYzU8LidgBxqD2ePG2aEp
2PZ6sLjF/6Z/OnauMXz5s3jT/kz6/kbwWPp52648eh9DOLPZxX8rEztEF7bv
nb1wUzH2GiOQDr37QK2M3ncrfLtnYiZXRb+PESR8+/pn7C02cxsYrg6/97oR
224bTHivsL7Rhp24HdJzK7kPddO5GViN7MvT66fva/H39/EcJ4nv2JNWkHck
XXBwBNvGCJye6D99PonNbQ3zfn9yj525lXKtFRSjELF93NgCZuDFkC9DfNh8
FrC4+MUhofnYuQZQNctlac9C7Pid4L+Z482jxdiEBSw/k3IiTBY7zhyayjYp
OSzHjtwGITydjWqrsQctQNPw1BluTWx2G+gJW6LeTPybF11d9PH+Rnq/nbBJ
0D7itB52hh0Mmf0BS2NshhUkRif0K27H3mgNJu/h8tQO7BpzmFrQolu7C1vN
Cu7u8B9OdcbmMQfrq+JJR/Zh++8EnpbHJkYHsBUsIX/Rzt9Sh7Erd8Ee+7H0
YX9sKTsQSYqzKjuFbWADJZ2anPEh2OKOcFC2PsczHPu4PUjv8XXYFI1duAtq
0oT5F1zBZlrByb5cZt91bCtbWKm03a0wFVtiNzR7/FgQeQd7rjOE3o8sdc7C
bt8N676vPrj2IbagM3xSeSM1twD7hyPE+nhVtRdjTziAbh6/f24Ztq8NDP/K
WBZShb3LAZLXGtdb12FHO4HZsYHAVU3Y3xyBreC8yqx2bOndcH9qefv7bvo9
XcBOuyIsvR97gRPwnnJbf+I7dqc9PHk++/PWX9jHHMGN43aM7G/sJU4gukVP
Z2ymGT5/N7wM6f1eyY29Yy/4lgdfT+TDlnQCGV45I5/52MEu8NaodHyLGPY8
Bzh1wSlNXMpsej/lN7MsvslimzpDm1DyrOfLsWOdIXz7xqyY1di3XIGI6bBz
08S+6Az99QxeBNgMN7iyUOqx4CZs5l4I/FGp5qSP3eYGnq+P3M8zofffAztv
ySnOtsCu2AM6AW9TrG2wQ/fBSmvG4gxHbMN9sFB9xRU2V+wYV2Dnb5q/zROb
0xW+fgq+kHoI28ANGopVeUaPYQfug+fx7YEGp7B79kKGb9if+BBs3v0QZ7ru
6LdwygwrLzil2Du84RLO2bzAnT3aM/oq9l43sGjV7uu5gT25DzbkDzitTcOe
4QVKkVfaQjOw+1xBxH3LztZc7MOuwKY7XKf8BHvVAehbfMPk9DNsLk+oGzMq
f/cSe9Adnr4d11Gowr6xH9Lv3Xp6tA473xuiz2xf97oJ7+9yEE44zHiwuAO7
whtc12es8u7F9aPesF3YOr1kAOc2PoC+cckuGMaOPAQKr3Kvu45jMw/CvGQH
MSbbNqo/+yBM+fNd4uPCjvaGTxZP+B3mYkf6QK3y3nM58ygzzvtAAY8wB6cY
dsYhSOt6dtJKCjvzEEQW7h9Pl8P9yAf848QP/VbCTveBPd5l30xUsRt8wMzw
kFvSWtwv5weEnHT3sBbO231Ajq161xZdnG/yBcGmY02XDXEueQwmcxTMv5hh
v/P7+/P4XTXagf3HD2r2nDK4uAv3t/nBkw2rSjudset84aZ4s5aGO65PPAoR
P0Meh3hj3zoKR6vV1T/4Ye84Cs63P95fcRK78CiYnr6gyAjC1vSHdbZEam0o
nu97AmQ0Py+WjcR5sT/wC8ZcORyHLX4Cxvs2CpcnUNbWYUBXybcLEqmUizgC
oCohnsfzDp6nfhwe+ekHPcvC9ZIMSDEb+TMvH+fzT0K4UvJRl0I8f8tJ8OM0
/ZlfgvNfDHBsn/ScU4Hn2waA4ePbfbZvsHkCQDPawjmzHns7AyxqRiJjWvA8
vZPgwxtb5N+Jz+9gQKSe5lfHz9hBpyAzsF5c/xs+r/UEVBUd1l/1E88TOgUD
kwsOC0/g+rcBwLs2P2WCbTvl26dA8ZBVbQcnZYboadDLGv3zkhd78WnYMxC3
IkOIMhvXaQhettY6WpRykfBpSHFuDDm6CM9TDoLiG0fy7GVwf2MgdLQs7NJV
xPXVgcAm9lhwhTKeVxwMiyx2as3TwP1uwUBEjruPrce5TxBYV1250rYB2y4Y
jvKsLyvdgi0cBHG6H37eMcJODoK8U8eWRm7D5yufgXeF4lv9duB8MBiGx5+c
sNuF8wVnQEjT5q6OM3bNGVA+ONmouA974RkwuR/PJXgA76d9Fvb3E+q/fPF9
7p+B8/Itji3+OJc5C+m7j0c8P4W98iy8ui5ZeDsEnz/zLHz6UNB/IRxb4Rxw
itot9I3GXnYOZLZP6dpcwQ47D5siEnw2JmLLnQPHSpSkcBOfX3MWGNxt1Xx3
cR57DhJ0Tv4ezsL7a52HAsbi5R8e4vqBMGhmPrV6VoDrt4TC+Oiu4FvP8b55
oSCqzpYb9gr3T4SB5oHEjoPVOOcKA4t72vw73+F5feHg87md0P6A6zeFQaRs
gJtcB56/6jxkOiyJ4+3F9dsuQNW1Z6VDX3C9xQUYaHT40TBE2V7qIvCKzFzy
dPSfFc2SjFOnKLeLRIBe+Eb/UHZzyiMR4FL+8fYBHspsOyMgkPN0vaUAZfvl
FyF541IOJIJdGgHFJ56ryEhQZthchPbHu+15pClLFVyEqZFZ4YPylIvML4Kk
asqT9ysoJ2pHAuGp85mpivu1o2DnnS6R5LV4n4uR4NcbqHNWC/crRUHsUllv
z834fK9oyNtVet38P5x/j4K6q86v12+lrM0eBSu95pUlWuLzTkZBiM6zYg47
fB4RDR9FPQvcnPB9d10CGJDIr3bD875EQ9yz8my1A/Q+l2Dokt+9y4fx+dox
YOgmlzZ1HN9XOAZuorqk3YH4vGcxwDbv1LWyc/i8tzGws3dV3IqLuP9ILOQ+
aYmMjMXnpcUCf0Ro2K9ruH4qFtyc1obYpOB5grFQsqb31LN0vM/XGFg099Jx
uSzsiTjw69joF/oQz78SBxLyUks/SFpQ91tyHXwnXktqy1AukrwONdXHRFMV
saUSQTFl2Tye1ZQFxBIhyK9+rqcmznuvQ7thEHcd4Lw+EdYtUZ21Voeyl/gN
iP7Z/vuaAeWIzTfg66vw0ZlbKWu3JIJeAvFjjyXlxNAbkOTdN1BpS9nU5AZM
6sZ9Wu2E+8WTwFJctzPGjbLUjRuQ/e1Hy4QXZeWwJOAtudFgfxjXf0oClziT
t6XHKTPckqHI/fdrxUB8vmMyiG24U3bhHOWaoCTwEd7xfDiCcmZIMlR95izc
EYtdmgzLCnPzC69RHlRMgcBIx5ylKfg8sxRodRHICEnHeVMKrFlfmDaQie+n
kgqR/O7JZg/x+6unwpfOhQkPC/D+Gamgm/8yTqKEcrtHKiSePxQVUI7fm+sm
jNsvDe+pwf2Mm7Bd/U3If/WU7bNuQsbsk6czW/C+qTeBu1XphHAXnl9yE3Zn
N/kd7cP5jluQkBoY+GwQ91fcgqa4lRHcv/B7LU4DkfMNV01+4883Pg22njx1
K2aWJeVdt+G8t1JOy2zKpom3ocz5faGMAGVlttvAvoNRvk8E5/q3QctQ8X22
BM6t00G854hqv7El/r7dA4vGpVoq5pQTBe5BZOVrgyPWlL3O3oOqp4ctihwo
s/13D2bnLHHk2kvZ3jkDdG5WeBjvp8wIyADG5UNHLvng8+0ygHl+cVDzUcqZ
ivfh18lXEUsD8PzP90Hl4MF4tzOUI+ruw34XybSsMMraopmQvuNlzmgUPu9z
JnQbHniqdYXypweZIKUtXhGciO/Tkgk2qqXvX9/E+cosiJPz/Dj/Hr6faxa8
Xbjwq3UOZW79LOCb+3ws6RHl0ZNZYMDmwdH3lLLV9ywI/iEiuPoFfr/IbHjW
UyThV4nvA9lwP2fvf9HdeN66HOi7KWT5oZ9ymU0OyF1hOkoP4f2yc8AxzGW/
6yjuv5ID1xgCRzOnsFfnQqhRflrlAivSChwP4IW2Y+68RZS1LzyAmWq8RTtl
KHstzwMkn1dxQ5FymV8eHBGzr/+kTDmu+wHkzuXpXKWJ+zfmwSBb7ldfoFxU
lwdKw7bjBZsoJz7Kgz29XJwcBpQZ9g9hU4DlbvCnrJz6CLLfDy8RPYX3a30E
0kqR7UNnKEsdewyRAauuvw7D9aaPYUZ9pW1aFOXB0cfgpeQmcfoyZdHhx9Ae
wPXB9jrlTKcnYFqfcnlNKj7/xBN4qrTRat4dyqajT2DlqTaRr5k4P8qEhHr/
d2V5+P57mcC3Qiw6mUnZvoUJx089NDtRjN8LCuBL/XbBHWWUa5oKwGbFULVq
FZ43WgDrG5SMPjfifV4UguqqmZqXNHeQDtxcDEmB1396AmWBZcUg1ETkGmyi
rORaDKdWNXnL6uP6g8XwPfDwajYTymodxWDfNH+waTtl0dfFULMqO+PBTsqG
i56DdpCJR4Q95aKjz+F+05fl+1wo69x6DsuD66U2XKIcrVcKVz74tIlfpSxR
Ugo8q4USRhIpRySVwtHg+zZvblKuE38Bnz8Yit+9i+etfgFWq/sag7MpE9Iv
oCz4TJxDPuWamy9gTbOMJVFI2Yn/JdxaXSy8oISyDNdLWNpyl2dgCO/P+wqq
yi1jdMcouxu8gqP5M6UT/+D3sn4Fsjfv3Rvj2En1h76Cmiirtdt4KbMLl4N/
wKzSu0KUB4+Xg7xnhinnQsqT+8qh1mZH867F2I3lcMKAfe8jWcr2Oypg2Zr7
P4SUKHPbVUCd7M6T7iqUAzsqYPmMzJjFWpQjdlXC+687pY9spvypohJONXNk
1P5HWUfgNawoz1yrZIbr9V5Dw0Pr0iAryoZHX8PpVM6tbXaU0z68hpVRWc1r
nCl7MaqgiWGzN3If5dy8KgjazzXcfwDff0k1KNtkn9zsRzlkczU069vOuX4C
u6AaVGRzpM1CKSeq1UCLkF3GnYuU7ZbUQAjb7HUccZR3nq0Bta85pXYJlK3S
a6Dtg93W/BTK77Nr4Nyr2S2CdyjflXwDGg9z9+7LonxT9g2cj+RhLCqkfOri
G9BkPJjjV0J55Ys38NHDPvZNOeX4wTewVj8vI7Ce8rh5LXRpOKxrbaHcalkL
ETK8LzS7KAvk18J6oYdbL/ZRHhmshZ4/Di19g5RTNN/CxQFeV51fuH7bWyA+
PBy+9pvyiai38KnMkfFrljX1PjlvISpvLu9WHsonJt4CSsmPTRegXKNTB30X
dy9lX0A5c1MdXDrJd99WkjIzsg60PR6te7iU8tClOujf6fRCQJEy22gdxOjx
m7kpU/6i9Q42ajxuea5BOT7oHQwsdXaVBMoWce8gTlDgp+8myl+H34HOn8eM
Gn3Ko+vfw7cvzryKppQ/wXu40iQQd9qC8s5j7+Hnlr0/Tc5SLk9ugLpYTjW4
QHlNUAPk9qZ4K16inPurAaI0N2UtuIr7RxrA+0zHN/YblGO2N4JZ/cmVQzcp
611uhNXyizza7lJOfNcIAoeZdyqz8fs1NcLgi519j/Ipr3NogmqRMYVbhbh/
XxNkuMTuiS6hzP2mCcLz1G8GlFMWmfUBPDjruvbXUJbm/wCGFt5Lbd5Tzij4
AEo3BRz1m3Fe9wHmjGQkanykrP3lA/RtNmpb+ony5LpmeHWpX1LwK2Wz8GZI
6z5rM/WD8nBdM4SoK1ztH6M837IF9gS9aGz4g9/bvQV03zmJvuCwoeYHtICc
7CzLnDmU25e2AsehG5cSBSnrCbdCV4lWXdgCyhkmrdC6SeXVL13KWyzboSCq
hqvbkPKiY+0Q37lft9aMsv2rdvBXnRv01IrykdftYH36zvO7dpSXCnTAurf6
M684UX4wvwPEln7SPuNGudOyA8a8g0/6eOHcsQMaimUKHXwpN1zrgNoNC3Iq
UinX8XdC1sUH3/PvUF4++REiOrYp38yibLG6E7xWD+2PekjZ5nQnmARE3GMU
UP4d2wkr36z84vGcsmV1J/Atea1o/Yry5clOGPDa56pXTVlGvgsqi2anqb+j
/E6hC+4KpPVIf8D7He+CUHtdWYEOyhEPusAts2v37x7K/aVdf/++Op3U94Wy
//xuWGa6pKN+iPJBw27gTny6uHSUsgqjGz59s7XLnsL73umGl1qT8dfZbUmv
eNgNH+XT0ubMoazF3gNT/NtzDwtS9tXpgYWjf552LqA8P6gH1NrvVJgsonyO
2QMmZZb1T2QoV5b3/N13Vqf8csrLF/RCIsN6/I8mZXFGL/g9e2xpv4/yL9PP
EHXbZXflAcqcSZ8h46KQ5xo/yrMGP8OrI4VHU05QllHsgy4Ht2CBIMoV//WB
6UyxB0UJlD9r98OyTUeEltRSJlwHQGe57KKwBspnLw+A/bw3y8ZaKW/8OgAx
nQob3vTj+rNfIauizhCGKP+u+gqVOQyr26OUPeZ8g96rSk7Cfyj7G32DmYEN
ngEcdtTnV/sNJN0Djw3MoZzy9Rus2a58ZocQaUacxCBsI5ojS0Upj6JB2C8T
krB6MeUQ50FoKtF83bGG6m8dHoRQ3ZEzSdcpX4j7ASFGCSmDqZSN7vyAwO26
z9Bdqn/lrx/g7xgz3pRP5Vxmw7D/hIbHvFoqXzf7J5jm+ZoFsu8ic73jIyAi
90vCxZXyrodjILTi+tpcT8qPR8eAT22LxUxfyodXjwPP+m/epv6UR/aOA9fG
2AsJpygPpI0Du77W3S8hpBllfePAZtpbtu4C5QMLJmDS4kJ3yCWqnt9hAkZt
NWfWX6X81WsCPlw63Luliqqf4fwbamZONkQvtGdZWzOLDe19+KooSIKycTMb
YnOPTfNdTLl+gg0pv1Pxs5IlXRS+eQa6eMt1gcRqKs+vnIHMDOvNk/UoZ9XP
RO8uZddmHSbNVoM40H4DxuOko1S+yp0Dcf4xSoo6TuUzwzlQQo74uUAGacZg
PgfS2Pv5wKHTVL3aOw4Us05KcO0Fqn7WSU5k1RZmUnSTyoU6uVCTgmtl1Tsq
f1LAgyJuF4j9aaAsPsaDdBWFXFc1U/PPE3PQZLrLw11tVH7Zaw7KXv6EI+Ij
ZZ9Lc9C5lXO1tn6j6sWP8qL1allZb7kdyPtH6fKheK2xmIb1pLUbeASRWZFR
N7cW6XYlTUHEvSFJde1GB+q/B3NB5LPxv5rLeqQZk/GCyHDztdnW5tS8teJC
aNJgg3/Lfqp/r+o8ZGtx1uHjDSo/EiGMVoZYnm1Ooby8SBhNPZLNen+Lmt/U
LYyq+n801KSTTgxjF0EJksVsFfeonE9eBLV2jV/PeUT1K1eLILuD7q2Bb6h9
1vKLIrsIE2v5GY7kfbgeiaGVxZKnl7CTZjwbFkNTP/rTxblIJyaJiKMEy5Bx
/rmkpYTdxVHromeXR0Upf1CQQLvuqTS8UiZdNOO2JLIvFzZ3tyededtLCt2Y
4xhkuZu0gF24FPpomPFgowtp0/ZkKbS7WldkoTtpr7wPUsil7nB96WHSbDc3
LUH7Wht3LL5AOkJ/uTTyHbpmV1tA1V/mlkEPVfvCC4qo+nB5GTTqo/E07Tm1
j7y+DDryq2rxyVek2wPOyCD/yT/ty99R95fnkkUBnI67g75Q/Tn8cui8mNze
NeK7WVZO/08B9cmPTTkuIp3I466A9NUrL4UtIV3TdU0BcZp6P/8oT7qdrVcB
MYIKF4WpkdYuj1qGDg1avOswIj34vFMR2b04szGUQfXnlaxAzLc7Gx+cps67
PboCiXes8GoPps4TkVqJGibeXlMPI216hLESbVstNdZ2mapX1l+F9OLz76vl
kPZT9VRGq70/S7R2k2YLXqqC0pU1wmo/kY47Ragg6W+nfr/oJ13WYqWC5rtL
tN7/Tjo/MFQFjTibXA/4TVqBe0QFPd7xYImssBP5ngsaVZHOhgA5dx3SmW8f
qCPmn9cx9ltI6zHq1JF6oRiXuQHpCNtf6ijDf89hfSPScS8FNZDc+txeMCVd
ZrRSA3Gr96bx25C2H8vWQK8VjJbnHKQs/UQTWQgsVB5PIp2m07IWfbnyhXPl
TdJ7c7jWodOyRS0Ot0nXaKqsQ5nr9oS+uk+d189Yh3icH/TEMUmveSexHhU+
2npN8z1pqaX7CCS7+xzPodnO5PueWqaFmAO2HWm8pBOXWGohM7/V+c38pLWX
ntZCJ8IanHVESKf1dGihhodyz+YtJT151UQbned9fjibIC1zad4GNPxgouub
J+kusbsb0YSJUcn8g9R5XC83opl9CclrfUnzynVuRAKLNjqe9idtv3b+JrQi
OKRN5CxpH3nGJuRiIdwESaQFrjjooPqRldWhdVR+YY0uao1gZGTWUxa20EU9
irVh75pI5xr76qJhu0OGiztIN3vn6iKBl09eZQ+Q9k9W34L0YvVKGjldWP60
RE0PPdZ0fCS/lnRIh4UB+nBqhbcIQVpH3s8ATb4eVeTQIl3kddUAIacL8R91
SA9/bzRAzyOYJ6+ZkmYedPgPVX4W0Z23l3Tddz9D1HK1onYqhrRPw1NjNNUT
EzpwmTT7tW5jJKXiqNMcTzrficcEOZaNPniURDpCcocJ6hmWveyTQdp/YNQE
fTVi7OorJa2SEmeK2NjUv7wbJm3A9Xkr0lpwZg77KOn4a2xm6MTKRkWVCdLB
+4TN0KTNcdfwGXvIenNdMzT6qLRHl490XWeKGRo8aNHxUJ50zIjbNtTee/j9
5Z1U/pzHHC3+8+rnS1vSM+/ImSM7EQnhEXvSfMMbzVGzTtE2sz2kTa8fMUcN
N7jf8PiQZl/ea45qrC9XHAsj3RRRboGeVj8usi0iXaiYboVE44IfmT8nrfvq
pRXysjfLNnpBuiuhywpJf/+cDJWk3f0W7UDBQgvPSDaQruqN2YGMzQ8btXwj
nRBwZidqbVJtslm8l3wPjbM2SDP5T+12adIlHek2KGJfRYWhLGld83IbtHHS
sYBYTnqv0lxbdFMyMlFCk3Tr5ShbtN9+0KXZmLRT5S07NNV994f1CdJbzA7Z
o7KCkWGdANKDe4Pt0cVL2iMrAklz7r9sj2Q2143+OUv6fUOhPfovZeJ38iXS
BiU8DijO0YD7y13S2eLJDkilrVfC/wPpwqU9jmgyb/Ui51bSz96NOaLS8GOL
jTtIfxrh242sEL+0VC9p7v1rdqOT1zTkS4ZIj84N340qrYNW8/K4suxhsc4J
OTdI68avIX3yxE1nZOj/417JetIcX546IzWpEuEBRNrgZ4MzmrXXuRs2k3Y7
x+uCbvy6Fdi2lbTuTl8X1CKy4rn0PtL6Jfp7kLm5pvbta6TH9vK4ImKMK+1N
ImmHLjlXJHOtgX88mXSj7GZX9KPrSJtBOukPZSdd0UUf5okveaQJnp+u6HXU
hoJVNaRncvS7oc21/63Lm+lG3mfgszvSlY85lsZB+vw9Lg+k59/OvMJNeraV
vAf6T+6Q1kk+0kd6nDzQ1qMJOnpipJmXPnogW+nvxk2rSV9h796PDnnH7J6y
Z5nRn8PwQr4v21MGd5O5Dl+kF/KTWN7z0YXMbXySvdCxF0/3vnQn89p9L7xQ
gNhnjwg/0k8q+Q6gsOL1ftIRZP3cRYkHUKpQx3ndp2ReHV7tjUpUs9X8iknv
t+ryRl3bTzffLiV9+e2YN5KOlVWaW0n2z9grdxAlirtVvG2g8tX+B1G8zI/Z
DkOkHzxR9kGRGhxnjsnuYzlX6tYhlG35fuU9BZYZ/BZFh9Abv1vvW5eTLrJq
OIQEnujLbVQh64/YcfuiMK3wUm4tMj+p5+GLQvQWsMdYkdZLX3sYndi5LCAz
lPQWiW4/lK/kM/NuOOnx4j9+6PtU4elbF0m/VV14BDklbw9OiCVt3GB4BOl/
ORl6Ppm0wNiDI2j+ifeX9j4hnd564ShKv3E6Xaqf9Ktl2/1R18Gq5RJfqfvk
evsjSd2F9xZ8Jx3dfcEfRfRl3Of7RdbvuVjhjw6pNuVOznRn5UqFm44j7VLl
pw1iLDPWHdc8geo/tbyNMCDzukwJBjpVftP2uBFp+2ElBlK669nrakrWMxOA
gRieMyY2WpBOUNvFQAojMtI/HVgumuWYyEB+s9y9dhxhWbvjhUIAEl00ziud
RubySrqnUPGf4hi+O6QbpixPIfeOUKmJe2T9+V63U6goRVKtLoc8/0rwhVNo
7/IN1sFPSYdXNJ1C+WtCbve9Jy1qcfA02rFNRDeHw4PV73MrLxBJzXDRaONm
uchZrCoQfcp4IDeHl2VG12BXIPLjMefaLUTWG/8UDEJxz6LKhBaTucWB/UGo
YZXgf95ryH7jTUrByIKX13T1PjIXvc08gxY9tta23U/muzXen0E9e+4onz1A
5osOD55Bvs8NBDsOk159TiYExRw9WxsR6EHuf/pCCHr3idN88Bp5/uBJ17No
e+mMnfdryHzZO/VQpCFTsTT1LTm/ym1rKBI9HT1w5T05b8rEIxQ1a8sHBDeT
/WdcU0ORE9MwzfYTaXNe0fPoYE7syBy2/az+x5YzwlDkjRVRe1exrJ26+Us4
8mH7ZWOnsp/8ebib9wKy2FUkt12dzOvfLb+AxCS3PdZaT/Y/8Ha/gG7E+XWI
bCHzJRFfL6DMC89XldqxnDh7y/EIVH18R+WScJbtu/+LuYiq0m5PWlwk5zfk
pP/12zGl89Fk/8juwr9ediVs5Ao5P1el56/fNRlX3CL78w5pRqLKFTZvfJ6x
zDhHtEWiVy12718Os9xuunhDNCrjvs/5+xfZv/al5V+r/tFQmSDrL/3Y/9dn
r8fGz/BkzVv76Npfq7dbHeBjmaEdNBmNXoQ5fBBTIPNg8aJL6Dk4tXtYs5x4
57JtLFLzU1kYbcey9o3ZR2JRSjab2WMH0vkno2JRoPy155x7WZbiV3kVi3QF
39+87uNJfl4HNOJQedcWjzdhLLefVBS9jGpDl4+rFbHMtrtw5Ara+GJMxfo5
Wd+9WOQqymEr2xfwgszzhNWvouhDTi2vK8n5+nd9rv79fK4VuTSS+94R/3kV
Narwn4kbIuez503Fo0H3sdknhLxY9efC1K6jB46S80bmscywSra8jo5abZDY
L8yy/Qfvo9cRh87ZlXaiLGvPLi+6jsTEF25Di1guYnssn4h0Xq2Jn1rGsmnm
2seJKFbWb+XJDSx7qe74cQPZiMdr/trIsvJAOVcSkhYs0vbUIedbCUgkobuT
XNt2bSHnl2zcnISK3sYe1jJiuZ0xfjkJ9QU8LPpjRebBG/WSEWodMWN4sZzY
ep+ZgoTW2fGLerNcYyBfn4J6LpVW3D9I1h9WGEpB4UbROm2+5L5+YgqpqI25
WgMdZ3nwoO2lVMS46r5w8iy5X9mnIzfRc6uPbYeTyXxehUsaisvVj+dPJe8n
JhqShtwFsqxu3SStInQ7Dc0vO/nm/W3yPL+xvjTkpCn5XD2TvN/hNwduI04R
q5s/mOR8f4nz6Ujv7Wt3z/ekbb4O3UW3uYaEv9SzzMajv/Ae4iFEnu5tJL0w
EN1DlSl2go7N5D73O8/fQ1t9vz3Y/pGc3xK6PAPtXCj4Z+1X8vOT6Tp0Hz0x
Uk/L+0a+z4/ZifeRxKkdW1W/sxyR5FF+H7X13UhWGib3fftBIPPvzwMVvcXj
5Pfh0SXXTOSxa/tFds4Dfz26xFM6C1VF+a0L4GK5/azTuiykXBbf+Zub5UzJ
DLMsNKTcrf5rDstpwXmns5DvTN+mz4IsNxyp6s1CjNTYpdWSLNek7snPRpH9
TQ8uq7Ps1bMtKBfdlUedfJosc1c7Jeei0t03BALXsKwgqVmci0Y/7Nm3fz3L
Ui/H/+Qiu8phqU0byPPLEk48QIr3+M5/MWRZgJdxNg/pfD7wyMGYZeXug3fy
kK3su573Jixrv2KvzkMR165ueGZG3ufSPuGHaCRM4dclK9I3F956iIr3b3TU
cmKZjbm0KR81p6deyHUmzwt8PeMR+tnDXbBsD8umGb+XPUIKu6oXzHdjmbFq
/NgjFG5i8/qTJzmv0kfmMdqp7Lsm8hg5L4vz7BPk497ozHWcvO/53w+foLA0
Isr/BGnuxb1PUJHUrK8uAeQ8+aO6TCQnGJG8/gz5vuM+cwrQ9++3+bojyfv9
3HW/EIlFm347Ek3e733350K0UeNXNV8My3GNHPJPUeRRnYtrLpPvuedj4lOk
Nqtt3vnrLPt5bjItQn7z5y9Uvcvy/Fuxjs9QYt7jsZf3yPc+HhL8DL2ycmiy
uU/et9HuzjMkdi3janA2yzLzFUaeoSey+oua8lmOR3yRxWhK48TSgFKW3av2
dT5Hco0y7CIvWT7/6bNACTI5VtGVXkZ+XkvfQwlKfCp6s66CnD88daUEbdTL
UVCoJed5WdmWIre+HbML3rKstjDnQimKOs/Wt/Ud+V5qJ4pLUVeN0Z1jDeT3
9ZXz8hcoaMenFdWtZC7dyPkSZUyE8zm1k+91I1zrJXp/Tf3baAfLX1LOHnmJ
5D6eypTuJuszFAdfojI3SVXffvLz89nzuQzx+putkRwl33NmjUAFKh55wBE7
xnI+I9SiAh0+sPCtwATLdd95r1Wgjy7tHuxTLCu9alpRifK37k/un+X915/c
ru56jfZXvvFy5mA5cb/i/ddo6RZ11MbJspfDA7YqFE5MNtTOZjll9GRaFdot
f47vMT/L0YIiHDVINGngg6ogy1+v8KnWoCqJrbfvCbFsqnnDsQatERLVuSHM
8ka5t89rEN/v1CMh4ix/XKEd+QaVHJ69ZaYky6PZvmVv0JEh9/n+i1gu36vJ
Vou6elXvey5heco5y7sWPa591mUhz/LR6zv2vEVeRrLZNQrk/p+4094i2bKQ
kwaKLIdYnOh7iyIKTMTQCnJex5WDdcg5rcVEVpXlqtdvLr9DYks3SF5XYzl/
seqnd6jmWkqfqAbL6w7dW/MerYvaF8S7lpwv+qv1PRI4Mfb4B2J5cmfJlgb0
YtQmxEOb5fiyhrQGdOxgkXnvBpatzCPmNKKevWcGm3RYNsvd0dSI4jv7Crbr
slwZX6LbhLbaGYdWbSHf9+fsvCbE3CYsV2zAsoBUUcIH5F3l92O9IXn/6/Gi
zUhev7nogRHLMac0YppRJEq2vm3K8hWP4WstaM+y1RcjLFgeWbKxuw3V5dUa
a1ix7Ncf81870tbx4W3ewbJxxcNb7Uhs18Mz8rYsn43Ic+9AZ75YbX5tR75f
/dJ3HWj4yPjMg/Ys72zQ3vgRVUXDicLd5OcfpqfUidZLt613cma560bs7U6U
dp8xNnsP2X+zWanr79/jz33M3Vi+/d/XLd3om6WzysQ+llufWbd3I5tuzsFE
D/L9BxoYPUiDzWDfFy+WAypvt/Si5LB+hUhvlqNkZl39hATEw3o0fVjukTvp
9BkdT1uZ0nKIvF/f2nV9yIrreOnOw97aFlb7jBs5+9H/E/ZNPg==
       "]], 
      LineBox[{{298.7356485110892, 0.00001288736025399307}, {
       298.73663458571764`, -7.732404831575487*^-6}}]},
     Annotation[#, "Charting`Private`Tag$38625#3"]& ]}, {}, {}},
  AspectRatio->NCache[GoldenRatio^(-1), 0.6180339887498948],
  Axes->{True, True},
  AxesLabel->{None, None},
  AxesOrigin->{0, 0},
  BaseStyle->{FontFamily -> "Arial"},
  DisplayFunction->Identity,
  Frame->{{False, False}, {False, False}},
  FrameLabel->{{None, None}, {None, None}},
  FrameTicks->{{Automatic, Automatic}, {Automatic, Automatic}},
  GridLines->{None, None},
  GridLinesStyle->Directive[
    GrayLevel[0.5, 0.4]],
  ImagePadding->All,
  ImageSize->{720., Automatic},
  Method->{
   "DefaultBoundaryStyle" -> Automatic, "DefaultMeshStyle" -> 
    AbsolutePointSize[6], "ScalingFunctions" -> None, 
    "CoordinatesToolOptions" -> {"DisplayFunction" -> ({
        (Part[{{Identity, Identity}, {Identity, Identity}}, 1, 2][#]& )[
         Part[#, 1]], 
        (Part[{{Identity, Identity}, {Identity, Identity}}, 2, 2][#]& )[
         Part[#, 2]]}& ), "CopiedValueFunction" -> ({
        (Part[{{Identity, Identity}, {Identity, Identity}}, 1, 2][#]& )[
         Part[#, 1]], 
        (Part[{{Identity, Identity}, {Identity, Identity}}, 2, 2][#]& )[
         Part[#, 2]]}& )}},
  PlotRange->{{0.0001, 300}, {-7.732404831575487*^-6, 0.00001288736025399307}},
  PlotRangeClipping->True,
  PlotRangePadding->{{
     Scaled[0.02], 
     Scaled[0.02]}, {
     Scaled[0.05], 
     Scaled[0.05]}},
  Ticks->{Automatic, Automatic}]], "Output",
 CellChangeTimes->{3.741322230960338*^9, 3.741336744583336*^9, 
  3.741411009889214*^9, 3.741411051636655*^9},
 ExpressionUUID -> "84f13310-5ea1-469b-9a52-9716d6ef5586"]
}, Open  ]],

Cell["\<\
If we now observe the errors for a given value of kF as functions of \[Mu] \
\>", "Text",
 CellChangeTimes->{{3.741411098065399*^9, 3.7414111299635067`*^9}, {
  3.741411292773777*^9, 3.741411295026606*^9}, {3.741411661741335*^9, 
  3.741411673545601*^9}}],

Cell[CellGroupData[{

Cell[BoxData[
 RowBox[{"Plot", "[", 
  RowBox[{
   RowBox[{"{", 
    RowBox[{
     RowBox[{
      RowBox[{"(", 
       RowBox[{"1", "-", 
        RowBox[{
         RowBox[{"(", 
          RowBox[{"ExRCsrPad\[EAcute]2", "+", "ExRBsrPad\[EAcute]2"}], ")"}], 
         "/", "ExRCBsrPad\[EAcute]2"}]}], ")"}], "/.", 
      RowBox[{"{", 
       RowBox[{
        RowBox[{"c", "\[Rule]", 
         RowBox[{"137.036", "/", "274"}]}], ",", 
        RowBox[{"kF", "\[Rule]", "274"}]}], "}"}]}], ",", 
     RowBox[{
      RowBox[{"(", 
       RowBox[{"1", "-", 
        RowBox[{
         RowBox[{"(", 
          RowBox[{"ExRCsrPad\[EAcute]4", "+", "ExRBsrPad\[EAcute]4"}], ")"}], 
         "/", "ExRCBsrPad\[EAcute]4"}]}], ")"}], "/.", 
      RowBox[{"{", 
       RowBox[{
        RowBox[{"c", "\[Rule]", 
         RowBox[{"137.036", "/", "274"}]}], ",", 
        RowBox[{"kF", "\[Rule]", "274"}]}], "}"}]}], ",", 
     RowBox[{
      RowBox[{"(", 
       RowBox[{"1", "-", 
        RowBox[{
         RowBox[{"(", 
          RowBox[{"ExRCsrPad\[EAcute]6", "+", "ExRBsrPad\[EAcute]6"}], ")"}], 
         "/", "ExRCBsrPad\[EAcute]6"}]}], ")"}], "/.", 
      RowBox[{"{", 
       RowBox[{
        RowBox[{"c", "\[Rule]", 
         RowBox[{"137.036", "/", "274"}]}], ",", 
        RowBox[{"kF", "\[Rule]", "274"}]}], "}"}]}]}], "}"}], ",", 
   RowBox[{"{", 
    RowBox[{"\[Mu]", ",", "0.001", ",", "1"}], "}"}], ",", 
   RowBox[{"PlotStyle", "\[Rule]", 
    RowBox[{"{", 
     RowBox[{"Green", ",", "Purple", ",", "White"}], "}"}]}], ",", 
   RowBox[{"PlotRange", "\[Rule]", 
    RowBox[{"{", 
     RowBox[{
      RowBox[{"{", 
       RowBox[{"0", ",", "1"}], "}"}], ",", 
      RowBox[{"{", 
       RowBox[{"0", ",", "0.00005"}], "}"}]}], "}"}]}]}], "]"}]], "Input",
 CellChangeTimes->{{3.741168877965126*^9, 3.7411689927770243`*^9}, {
  3.741169029017823*^9, 3.741169075797423*^9}, {3.741322031706285*^9, 
  3.741322116198372*^9}, {3.741411694600963*^9, 3.7414117025762243`*^9}, {
  3.7414122396427526`*^9, 3.7414122712187777`*^9}},
 ExpressionUUID -> "a84f8f60-fbdc-43fe-a81b-e885050237db"],

Cell[BoxData[
 GraphicsBox[{{{}, {}, 
    TagBox[
     {RGBColor[0, 1, 0], AbsoluteThickness[1.6], Opacity[1.], 
      LineBox[CompressedData["
1:eJwd2Hk8VVsbB/Dj2IabUJImJEUpDQpNrKWoKClDSPIWhaQUQsIlKnET5ZYx
SiEiMyGZhxAZIhzOOabMQ2biXc/9y+f7+T3r2evsvdba59hkaqNzlU6j0V5x
0Gjwd4OZSKaZ6VlMy3eM7erjwaUGfwxdLM4R6w2uzuXBtppdc4HWRsRT6SF+
PLh7/fmNZodNMY1WsydcngcrU1vNAo9ZY5o7S8rZixs7XL98Z17WieRs8/37
uPDrba3hR27eJXmIvs0yLlzVrVf66KMzsbDcBIvCkpfU1wjvdSX1dKozgMIW
cS+NX2zwIL6VrTHJiVdFuC0mSjwk9X4FzAo6jnXNEdIpAB9LyXhHx8h4Rnry
8iPiibX1HnRsuc72zOEob+K5ZMYhOs57fjWyTMqX+DXn7iQOrKAmvenWan/y
eazuWMXQMOsAf5H3+n9JPqgv4/sHBfYk14feBo9bKmv9QeqB+l2J5cS0IsOW
lX9Q4kgEV6PDC5JnSMSHLCCX6L3qm+pfkvxQvF/KPBIRNqz+5BtC8kn753Oz
6GvBAqOKTUybdi8vmUWuNq+HOw6GEsuvcAqYRV1f+wW5f4F5VVW3z6JkD1cd
HbVw4oa525dnkObIm6b+hQhiR5p99xRy/7Z5YlEmkvRn+A5kTqHzUg4u3ufA
JQdqfabQ8vr1T0I/REL/QobcFLLbdSWxwOg1seDF316TSKV7apQ/8w08D1sj
NIFadUQdom3ekdyN3j4zhnatn7l6Oghs+DL15xhyZ9Wfm8gHKxfVZ48h6Vu+
CkeFoonPpY65jqFbT+YmGGlg395AnjFElTfbrZ6LIf1zftG3jSL9p2lmuZKx
JB+8cJR/FL3X99c1OwV+KundPYK0uk/sSw4DRweudR1BwfTMcU38nrg0QS1l
GO1S/ve2l1ccsfvGyX1DyJ26fXlHAnilpQb3EKqv1NSuawSbya76OYicjCg5
ia3xxHKvON0HUaGj3WhOBdj0E64fQAYp2ja/BRKI2x+b+/Uj960CN0yDPxJX
5lVr/0IdwxcOKBeAtX+0yP1CKOM959o+MM1FRegXcnsjWW0umkScVC/U0IuU
5fLMRK3BLvEFF3pRttak/yO+ZOItf+U69yCrvWFT9hvB2grcl3rQOhFVY9N9
4M2CEcd6kBPDf6vyBXCTe/bKHrTfWjZvPA5sEeid0I3SHpsNXDyZQtxxjOd3
F7pyY5n2KRPwNoG5ti60Sjs544AtWKRnb1kXsl275LEqBLyszD6sC8nFhKyt
6AOLv9pxsgslFn8/Jv84Fe7Xr/nkTmQS6xS/KRzMOi0S2Yn4/9m4UjAZzDhj
49eJrHVvtPU1g43sWq93oh1sXruIbWnEVY7+Mp0odglHLisHq3UIJbHRuK23
RSwDPMhIi2QjpZ7aXcd/gysWgwLYqKbq8mcP8XR4vpVS9mw0FezZMmMPrmhV
U2IjFf6q1y98wEdkB3axkY+78DX5SPD2ZbWb2EjM4t20TSV4Va4uLxupyZcJ
927KILa7tL+ZhfxiBNu89oMnnUurWKh5vWGU5Gnwlg7/Aha6ztEnZ+IEvjzb
GM9Cz74tO9P4DfyzX8SThdqO6IrYdYH5vty5y0LS6aGMFXP/9e9efouFskNl
rTWlMonTCtgXWYhlqfW46B44aftmJRba3vbi7OUA8LWZQ/IsZH+mY81SNHjA
wluWhXgVb0UfqgN/6i0UYyGd91k3mnvBTww/irBQmCiHgsMf8OCOWkEW2sP5
rCh5WxbxcGkCnYWcHVp8ziDw9NS1BSYq7pPUGdIFxxqdn2Iig9pU5ra/wZ5B
tf1M5Bbe+CeiESwgte4HE5WvEC9RHgD/2GTxnYmEvMz/aaV9Ik7Y1FPFRO+s
ptevkQVLbnEoZqJhBmanHQHvfPcwn4kOaHu/1zEAV0iX5TJR1f51B/zug3X3
NqUzkUj85aUdQeDOI9EpTHRJPK60IgH8xfjtRyaKCxh/YlEEnjvx/QMT/aYO
n+P6CV5ZIRvHREpOnqJRw2C96IwYJno4UNmpQmXD/Yu++Y6Jak2E49vXgdFz
vSgmWl9nbOuyG6y/z/I1E0X+uTYUqwpWyS6JYCJpGUfLRgOwf9rJV0z0Qc+r
k8MavHV6KoyJ9rkHmOxyB5safA1louz4Vz+NAsHi8cUhTKTSFK/3KBbMVdEd
zESl9E81qbn/2Xsnseau0pPMWnD1l9AgJqo7X1+yvBv8P/U9xIYPmCoHZ8Gy
c/0vmag9aSjnKn8OcV5iJfHVtjnFZ5vAp3Ad8SAPb0qeAhg9XCS23bd654AG
+LjJWdJvxkQydo0J+PCbMmI3n92b1WzBnTuvkPlQGUqvbj0EezCkyPx9WBrr
wkPA2k+Wk8+3gt8gsCIR7Lt+Lfn8Lw9cEZwqBGebqoczkfiV2z6STeBI1XBy
v94+deM6MwAuDBWJZKLtOb7u95bAvRpp5H4n9QTNx6zKhfN8pwN5HopC0Q4N
W8G7pI3J88pVTh2jKYHnV5mT51keWN17/gr4q3Z3PBNp5beYPnQCL7tilMhE
DQO9jJR/wEqj40lMxDpKb+BLB1suPclgIsubgmcOVIA7Tvh/IuszWPTrFQb4
4L/pZD3OjSrmf+b6TDxbbVnERO6iaof714GbPKZKmYhbXTtDZBf4TWX0V7L+
I65/sNEH+2TcrGOioK9OW8OswN8kH5L9Ij714E25Gzgn50sLE+04HRm0KQZs
IhDcyURq8w1e9dNgcQ8W2X9fpdlLS3x58HnCeMj+PKsz4iwrAc6VOMPBQhff
/3X7gTpYYPnR5SzkYIAu7g8Gz06nbWah2NQYhdBDX4hH7XINWaj8pr6Q01nw
hTSfSyzUJ8M1omcOPhjtZknOm0jTWIFn4OfKTU4sFP+P2Ib7fWCx9+qhLNSU
ouEur5kP74sva3tZyHLF62FJA/Axo/1jLDRzY8Z4pSm4SdV5noXWysQcHHYE
CyVZr2Ajwwjqd0wUWLiQg5zPLb5frm6YB68YbQ1mI6s+kYa/uAtgf2koRrPR
3PGbR2dWgOn5qSlstIEutrFRGnwqZ00VGxk7OTf76YC/zXnQOhHjisIpehy4
WrfWphMxleP39BkWEr+NarPoQvYbOv59awYu3rLDqQvxzArN/+8meO56sHcX
2pXmXPLDE1zF1/i+C93bftKoOBEs/LV0qAuJrOnzjKCKiM0bH9zrRpqj0k3n
ksCtivMJPYhZbaS0Mgf8ZHJTYQ+yi/d7XVUCNtQ1/9GDQsynrqu2gt9HnFjq
Qb1tJTQ57mJibgsrnV50v+LK9uXGYMHgjYu9KPPNG9dCnhLi9QFZVn3Isi1L
qWQl2OppvXsfWi9SM1+2AawoyP2yD7k9nr9bvRucfDy5qA+p3dJzaDYAC7uI
i/ejWmVum+EYsH7h0aZ+1N987dJ69VLiz1sljQaRmKCcqq13GbHxjVPhI2S9
jCntwl/J96+21TIVvxHHD/WP+WVVxB9kIuqmERfKb/ZXrYH5SwzWzKPoKvnQ
jLlaYo5pT/YSsj7NouUtEbuL1TBGl9Deb0/MS6jv8P45sGdpCX2u6ZFrECBW
cdHo4Kfhhrqg8jFJyMUFVLbTMMfPhUnZU+CPWsdNadi4u/hsVChxfnMXrqFh
oUU9bn+lOtL/15MfoRw4j33Ni/Mocb54vc0bDmxV5kZ3PAF20ON8z4GL/GMX
L+oQq3TMrM3gwPabF6Z2WEJeeWqxhgP/UI/qLXsOueH5BDodBz8fK1/qh/6H
Yj3M6Pi4E/cJu1FwjofRNToeN95Q0jMJ7hPdaUPHJ6WPFVTT6km/jH++ONPx
XFbQp1ARYlrYUlAAHRu347j9R8Gq3zbk0bGEjJ+vTTDURxqfFeLE306vfFDx
iliFMaC2hhO72Aa6bX4LZu3eJ8qJm3JCbjclgpNqF6Q4sZ9WjAEuhn5nzqgd
5MR/7PI3C45AHr4zyoQTt+SN5ySqNZD+RWPBbzmxd+eddN6T4Ey+olhOrMg7
m2h6hlhF/0v3B04coL30WsQI8jXja9I5sXoXn7ebDfjT/d0lnDjzLyk9rZAG
OH9P7ejixIF6BoNDI2BBOQMxCmvHVD4bmIB63aG7EhQWmMMH+2bB9RIvN1PY
O2Lbwy7ORng/jObLUNilf3Zj6xpilQT1OgUKm7mH6ZZjYncR/0FNCkvUr5gr
UWuE+ymReYbCbVIPIos0oN5e0UWHwvqVN4bydMGSk5MGFD4pgh+lW0B/Z0aM
KYX3fmBlv3kK7jPhdqTwyOK5y5GB0P9r2d27FP6g/ZXnVTCM7yjvvUdh6ekU
veAouF5YUKo7hdcd9Rp+mgl2frHMh8K0ZmlJ1w7ol3UuM5TCn7eHljt3Qb91
ww3hFHZ2FbRx6gNbKA5FUHhCcibH7jf0N2nnf0vhXzcqzlnx/CB+9UnwA4Vr
OK0fG+wmzn8ovSaHwrbZ6uoF8uAgbp7PFBa5LcWz4xAxLbx8NI8i66fda1GN
2P3aQnIhhfuztN3fGYGR5UAFhf1sdmHBS+DQ8LhKCstJ8y06XQWLVphVU9jp
efE9zVvQ7+7y4loKc9/c7/j7Afhvf6UmCsdtEVa86AvzS8qvbKbw6dbRiVJ/
GC+yoNdC4UD1ONuQUKhvijzHIL+3N4vdPJIMPjgs2Elh1Ey/+rQN6tM3XB+i
MNuvY/MsC3Ipw7BhCj84lss27YVc91vZCIWrUu5cUhyH67Hs+McpbPTk1wUG
TxOpX5jRnaLwomrJ+hP8xCquhgbTFH499/pnkhDk+5edmyH30+KCgZcYsfup
23iOwneOftPZsQ/qeaNr/1B47Wzcyn8PQH3SaPQihXM/PqpdVIZ8Z4zjEoXp
Yke06tSJ89Ov8HJw4eh6MX4lLcg325YTa/jMVb7Thf73Z+7TubD/dKrGXRPw
QddeTi4sn+jP22kG/VfeD6C4cNOVG2Wa1yDfz6/IxYXF66SPSdhDfqvoJjcX
/vAhWKXsMTiSP4KXC5sEWHxo8IPrC5is/osLr3RQWMt+Dnka7RGxA/4+shAO
tj1hvIwLb9sScWFZFMxvy9gX4lbeG2VrYuF6KjPifFxYpY43Ym8K9MuWqSEe
z/ixTCUT8rjzEsu58LvQtw6nc6Gf/rg1saG7LduoAPInU2nEy66qaFmWgoWv
zRB/1hDIvlMJ12vU3M/PhW/tapPyrIX+pW9vE0uuigvwb4T8vV0MceO045/w
Fsi1cpuJvduOXYvvgH7NHlwCXPhQwarGrC6oHyndSTz0jqVS2gfzsfHTJo70
+fihfhjG32+9Raxj47qW9Rvyn0m+xFx6p7yGZ8DOK98QZx1YNzr/B2xJSyO2
Euu98BdnM5yv7gXEovT0MhFe8JHAr8Q1Pff3beEHW+Ea4vuVZyPkhIjdjbzA
8knifHgN5NvMK4l7AgcdNEXBLb2FxMF3s9nnN/03fnkGsaaJt5aFNHG+z4+3
xItH9bPtd4CLNZ4SJ23dIn1/D1jP8g6x2fLxgKcK4EkFA2KRsS9/wg4RqxSm
yROXNz65FodhPt9/8RM7Z19ozFSDerUGNrmfOyNkjpRowPXNnFOJn1mWrGXq
Qu5PVydWO/3ca8gQxqf38xFPy10enbsIuXNwJXmexvMLZastYby+ASIWZH7d
t/kG1B+xHiPrpbA4KGKPLXiDXiTxVj95x1MuMB7FjpH11mJL7zT0gPzF+kDi
fwxqtcwfwvzZ1/cSj0tYS3v4Q31gpilZv2+5Dj3z+xfy5swJst4N+nkWQ0Pg
+pei7hPnpkY1ZryFnFv9GQ8Xvhl0+0jxe+i/i0eYeJMrTvieCP26PweQ/fPw
eKvXYBb4qpgH2V9nfwrJS1aDW+Z3k/3Yt0kjK7QO+gmYe5H9et/qb6XVzdBv
fk8D2c9p8wNqvJ2QP5i5SuPC68RLzg3PwHzkPuuQ8yLFfP6nxSLkwqH3Fyis
+VHOhMX5k4yXnk2Yp7CbyivzBgHwm2PTs+R8M3V0zN5CTJPx0yPn1b34hPl9
24lVilovTVJYeKLz74TdkItVWE5Q+PiDs96Rh2B84rPr5LyLj5EJfniWOP/w
WWVyPtoPtmbruECOfgl3U5hfQQhXeUC+io9BztdoV/WiY4+gX8Ly12wKNwuk
Vx54BvV8uaJMCivL+bWJx4I5DneS85rbQWWxvx7GP5BJqqHwy6W3Rzx3tJD5
WSldzSDvR2+NI517WmB/1malkfN4xbCKqiJx/jibN5Wcj5L7VTiPENMG/F59
pLC1WgXy1IfxD65HxlL46OOhw54ekLMsOEIoPCSkqOjZBP2skrSdyfs+tEWh
sw3quZYOO5H3xZa/FVTZ4F9oswOFDRXK5TmH4HqDr37dpnChgdE+T3or6Rer
euYahYPC3PZ47myF9bH7KXm/q0qXbff0bIX/T6aMyVF4sM246aE3cb5KU9xu
Cr94Pu7p8wTG01Mu7yTvR5o4I+AljFcILN9G4Wet9k8j4yH31b+3kcJMf8mJ
z/XQb1DWcTn5PjLv+nlmcxupvxbRQr7fZNTKn71ZTExjb2M+5cRV9jlP/yfR
TuoD7x0tpOP3YU/4lK52kOt/P5wywoHvsB2TW7WZpH6weesaDmxhp2AVtkis
cizKcisNK5euLaiLYJHxhnmpTxdR17+8Uv9osUn91r1WqQso72r+lPAcsftJ
3pmhOeQyHW6+KqST5BoK+wxmER+3d2fgiS74PSsnlzKNXH+8XPTtA39Jvqo8
hSRjbB7peHcTj9260zmBgiZ0xcLke+D7QiLn/d9onNNE+0IjMY2p8EhzHIn5
2z8L9+wl/rHOXWgMybYn3T4n/Yv4IhVDG0U3ZNPz2krAycOLy4aR+3TJ2l7b
PmJ+sy6BQeTgtbDCQrif2HGPwrl+pOyHRayKwMxjNS9/of1BJx8r2QwQF0lP
cvSi1VfuhXgJDhLLqnu/7kbFH7KyznwGM+Z+K3chg8wNd/z/NwS/B7/t/qsT
iRYej4hcBM+cTh1moVQNtx/74oeJK1cpf2einc9b45U0R4gTN1xM6UAvjGmf
+M6AX5jS4zoQTVqqtEUbzNSIe92BGrJuMp0MwA7faAEdyKWdY3W66X+5eLVN
B/oqs81t512wmlv7zg5kmW9/VjwanJXNjG9HdY+DLw7F/lc/2RDVjpR086xy
48E+B6pD29GKHp4HRsngOpMi33aUyRf66UUuuMuk+no74jYokBSsB3u/Oyfb
jm5J9OxubwQXWt/e0o5a+pYpJzSDRYKfirajBBc9g1PtYKWy+uXtSO9Nr++j
PvAPV8chBsq7vjxYfxAs/CS6m4G2KchFS42Aj2s1Mxhoocw5v2jiv/lbH/nG
QOYBEdXPpsFX5JxLGajWqLjl8hw4iS89j4EObenr3fMHPO4ynsFAUUP8k0tL
4PwUuY8M9H8+SkJs
       "]]},
     Annotation[#, "Charting`Private`Tag$40900#1"]& ], 
    TagBox[
     {RGBColor[0.5, 0, 0.5], AbsoluteThickness[1.6], Opacity[1.], 
      LineBox[CompressedData["
1:eJwd13k4Vk0UAHAhoaKEkFSKhA+VkDSWKCRlSUKSneyVJMmWkLIkW7KkIqRI
SBJlLeq1XbKFV7YsJakkfee8//D8njN37rwzZ87M3WTtbmjHzMTE1At/8P86
G/4SG+sjqkxM9b6rN38itcf+mvo5HAVbl1iN9hEvvaH5OBczcGpTZk4f+Sx0
fIPNHmvwVBGl1kf2sm61idNyAXs1CNr0Eu/Tp879kfYB1wa9bu4mGRLdd9Td
LoB9iyzudpPGz8a1Vx/7gvdf6zrTTUSttNfy7rgE5v/xSqCbOOQkWMSvC8T3
1fx26iJr0vwX8zeGgiPKLCQ+kuxLL3gMq9Bb/EeZPxJi8Uv8x6mr4MSZ1N5O
4ijodXhPZhi4yLIrrpNU3LRLrxO7BnZRt+XoJLs0xTd58EWD46zsODpIwFPN
3Co79Ps3xl8o8lbUZteaYvTgZHMTRayWpOsUm8SA+4WF4ihyrULQayEhFsy+
zk6MIgNKK9+ECd0Cpw+mmrWTuOGC1tue6DyWL2rtRDvOZCi/Hs3FWrq1neRP
py1t944HS1RYzbURvwc7tDe1JoCTN15IbCOyxh2m8pKJ4PIlI4FtZHCJn9OB
QHRPafHpNqJzoibCVTYJbOjpptZG+HlNm55fSwYfiRGZaiVvqxZ6GwfR3t8t
u1rJJfeMqU+7b4PlOaZrW8nQ23FutlG0L1md0UoKAi8ZGmrewf6blxxvJXrT
dzvGF9LAMgMtVAsJeL95dnFbOrhY+3VdCzku5u0XdhQt9/V3aQtZ0Sp0/XYe
ulFDMqWFnJGxza8yy8D17fG1ayF6V4oVDoaiTfXtTVuIeA/7q7YCdOKzGwdb
SFf4ow8j7HfB9xZCdrQQtc9zX1eWoBWk+VlaiJCKzoWEQbQ4U+3PZjIbe3vJ
Jq5M8Eat7IlmkqWmxiNvhx7l/Uc1E66U8J1ma+5h/mpz5DeTbkNh7wfu97F9
Q7ttM5ER+mV3KBHdqLpg0UwCBlqPzlaik//pHW0m4h7XdmnwPMD53H10fzPx
uD4/21uEnopkkWwmr42poZBedHGO+uZmwidc2CbFlgUuNb0r3EzKcpyKLhxD
a4e85m4mrPWdZ/jm0ZoeXj9pxCSqyKZcNBvXf+7hNxp5aBJtZHMQXVv09wuN
6H8+sLMgBZ3jwDRAI0nMJTN6qg/BbbV6jTQy0RA7+N0BXZFgXUcjJMatJTma
Ea+Ke00jQxvEC0cH0JIBGs9pRGbvLc+QkByw8p/mLBoJYPU8JfUIXdr2OJNG
Wt/pGbS0o719stNoxMeMdfvGrbngmes9CTTy+vyZry8a0Ezyx8JphFf1cL/1
DNo0ZOIKjTiwSdE41uXhfCvEB9HIiluDj4+5oCMoKT8aOVZo4P6d6xH+vqiD
HjSSc+G/k8mKaHkqyJVGFtQ4DqtboUXu0Zxp5O6HSpmoArS2+z07GpmNTxFR
6EIPL2yzoZEDlj5cvcz5+Hv+VlrBfEzITkkao+WyJSxgPoqW9zX7odkbfhyn
kZiLI00+99HlCe3HaESBM+1R7RxaWqPBCOZjK5erddJjfF7noh6NfJoyV9pb
hbbf8FEX+it+yCIwhk4+e0CHRvzvijbZCz/B/N1zeD/Mb2jDDmM5tPyXMU0a
6XPySFTXRL/vjt1HI3u3V9gIu6BVBHnUYby8dg0cAWiNmBFVGkn5tVz25010
p2ADgfl4dXy++QX6bvdzFRrJy2SyevUBTeXU7qER86tZNXl0tNCNfmUaKdP/
EX11eQHO3xuym0acd6TMnd2A5n0aoEQjgvz7LKx3os/upSnSSP3vsarDB9Au
z6XBPr3RW/eaoxf5ExRoRKJK8bqkO7o4YQW4817fzNpgtPb2qF00EhZ2xXRp
Avpe2Xqwoot0xUwO2m1tqTyNDB9u3dxfgX77wQocv9M3vKkFnSzCB96/dtN0
2TC6qK11J43MzdcZZ8+jK7jSwQ/63MpucRWCPXy9wUdf820MFkXH1puDWR+U
X/FQQHsH64CLwm2+nNBFcx7WBNu6choctETLjGmD1xgUFCt5ob26j4Nfy5sK
i4eiWSOxfy+Bf4FrktELunfAogv3R5jy0ezbmsEtn/QOTVWh0+tXwPiD3nwv
7G5HK586Ct6elSzQMIamqT8E90eo+xf/RSuILoX5iXYbpWeufgrmeeEKVjOM
0okRQ7PWfQJ/3aXw2H83+kbvCZjvdMFeXpdDaGWJIfDhv8G+x0+hj9ich/XK
r27Wkg9Hx//3HNbXMtsnd9MdtNwtB1j/lZEbVnMXoN+KikJ+uBi59ox1oo0/
PIX8EVbk1eiYQFsNXYP8ahR6kVXNVIT1UNp1L41IDbKfSZNAr1qrB/nZVfO4
M1IFLSSuq0YjEQ9NiO8RNOdWA8jncY97HEd90HcvXoJ8z/6nms5Zj/ZV36dN
IzNeYQ7ZveiWd1mwf1SGaTL7v6MXPPkP0siHxlMvA0WeYX2cW6MP+ZAU3PXr
LFqo+LoxzNfKxoz4CLSh7n4TeH8Ar5N8Ojrk5zJTGlnvcP+n+zu0OMkxpxFN
+TrekU3FuL+XOUK9uJHF3ROiiE5/5wH1pFPINFP0EFr8VLADjZxeMrbd0gcd
2VB9mkZi33Mebn+PNssqO0sjA4764W8uloAL+7zCaESyJ/7IqRi02zjPNRo5
e/jT2n8PShj1s+I6jbAreDxQbkEX88ncpBE5ltg3BRKluL/t/VOhftxp/5vW
jn4S1lYM+3GVSM3eL2hpNfYyGuEJsY/sZnoO9s/VfEkj951/Cq2VRiuc7nwD
66UoqHQjCD165XQzjQi1WHj5yZbh+xz3TEH+/HWazN6HHmwrh/NFfNt5x/Zj
6FILrR80sjMgxlImAK1c4r5AI3oytbr9NPTQnfXLm4l/hOxmTa8XmA/1Y9ua
yYAGc9vyZ+VYT4IVXZuJoxv3YaUGtGh+nmczmUoSfmvbi5bTl/RuJvNfFSpf
Ln2Jv2/rnsvNhCftdJ67CTperSSmmWj+aQtp/Yk2/SZc2kyyn2btuq38Cs9n
i5ucLaTezYTH5wj6V7fbqhYytm3ptLE9eoLPmL+FSKZbZ3PFovO/KIq2kNzI
9euCxtCc+U7KLaSjUCdAXq8S6+X9sy5wv7j2ym7dHzSzvkhHC3Ee42/jYKvC
epfL09dC5ve7afxahX6SuupzC1nHvH5DuzhaRVXsewux8PHtvGGInip8xt1K
em13HWTOQbO2eem2kv69uXJjpq/B40kacL86u+7TrXs26PQlm963kmW/ef6c
dEOXSiyjWolMkW8NFYzeYvDlcyu5KKlrVp2Pfuu4mg3uc2vHgtNY34Dnd7cc
aCN6X8U7jj5BP7jL1NxGSu7evfR6WQ2ex/eSfrWT9dzb93mF1eH+3tFm2Qnz
901FRvUt7m+ZH9u7yRJK+3FlXSN4v8jN3l6ylFR2Ru/7AF6xj+m/fuJFV9A1
1Ud7NYjt6Cf9YY9ebDiO5nmprdhPylqTU/Pd0IWzoer9xM3pnG1jEnpl9NDR
fkLFSX5d9hX9u2CDfz9pO/c2WFWfBuYe8GnsJw8a5W8Xz6ON3QdODhCXQwNM
Ff/QLxvnbQbIjvfX7WtYm8HXTqx2HCAvPwxvb+NCN+ju8hggbS2J9d9E0ffq
TQMGyJKPCz+kD6ILbq9IHyAWn6uPZN5GswYI9g4QUXvP4px0dMeWD/0DZHR4
vXDhffTniMChAXJm1Huk8jF68nrPlwES8UXCv+8NWv/p6fkBUvItMldwAr3p
5AT/IOFZNGaLVmkBs9W5HRokFYNOISwaaKY5JoNB4lznz3z+APqjQpTxIHkT
nb14whAt15NmPkjObl6Yk3JEN62KcRoklHbmSN1N9BS9MGSQJN38Vv9vHC15
crpkkOz3YTtw5iu6LprpxSCZsVhXM/wDHfx2ZcUg0RXXqmpiasX12CxcPUjm
SxOf3+ZHf21aRhskFn2qOYoa6OfX1o0Mko3bblxzT0JfdNvFQyfvD62+0pCK
/nujlJdO/Lzi/DffQ1+pUlxLJx0vkj078tF29pLCdHJDP+uYajU6/We/GJ38
PVO5mXsazTURq0QnOYn71jvNomPudCjTienLWv43v9F9QQJ76aSIrYnjPGsb
+EfGDXU6cUn6ON0niFbx1dOlk66KmRf5muj4XdzmdBJGP/eMXRe9YTv/CTpR
YP+db30Y/cdV8CSdxBj8y+A3Q5e589rQifbQ8jB/d3RhYY8znZRwiBnrJ6N9
PhVfoJM442MTk9PoO57JcXRikPUu9sssOtuJK55OuOZVd4/9Rjetu5wA70+T
CB1iaQe/GTVJhvkZ/72hey1aTbM/jU5sAlKM6lXRlTNmOXSysXXVfI0m+s7W
lFw66RG7kv5GBz0t1pVHJybvXCcrjNDFg3qP6USXX/XqMwe00qqVRXSyI2+g
7G4U+vTgr3I6mV48eio9Dl2ewl5BJ3kGb5elJqFFVfle0Yn4z0LjpEx0qItY
FZ0IaoRMRZWgH9lsqqETpk5x0Uuf0HSW8EY6eSl5u953CM0b69hEJ76XuN19
xtAqslrv6WRW9NeLM9/R79x+fKCTUdeGo87LKPDxzh2tdPKBxSX8mCya5G76
SCdeZdraVfJoCZsBML+n2DIpZXRm3p0uOuRfX8iiJvqX/IoeOhkvNQi4b4Ye
IlV9kE/uMqrcVmgpPvtPdLJdfPmijx1atGFZP5343Ky+qOeBLlyvPkAnbG6K
579fQcs5RNIh37bwKpy4hp5lXjtEJ4e6v87WRqP5PVPBcdo5Xsm30ReSMj/T
iejm9W7qBejr8ldH6KT242/p3GK04/pfYKdo6gtvOZq9326UTp78jXIarUU3
dyuO0QnpZLaL6mG4/dk4nQze+LT59wDaIH3lFzq5olU+aD2CjttoDW4sPGel
MINu/LVkgk48nAw3pP9Eh28/BF6zUbaP4y9ayP4W2Oz6qHnvsg7wpWzhSTpZ
3FcjdGAl2jDOHJwxn/HxCQ86JSQBrFngnygkgI5wooFHHcyPhaxHHzJnm6KT
ayJK/FOiaCaJ3WCZdt72YxLoGmYn8DmN94ZSOxn9pb4CC/zOWX1LCf3Ebxhc
/vgqbXEvOsqac5pOTtrbRjnuQ/8jUmDm9er6Ldpobxkd8IPW9StV9NH962zB
OhHz7+4boVeK+oEn1DoiuI+jM5ViwNE/n+pcsER3WWeC5fOj2ek2aNGUQnCH
rWudnhOa71sF2HedbmixG1rYqB4s0iKutfEsemnze/DrMBbWiAvoPJ8WsJ1q
/+vv/mhOhVYw+1x54IkQtBlvMzgvL0mtLhy9nbcRbBnjkNd2A315uhq82nuX
wOBNxvilXoCrzVhCphPRN3/ng71Vm6cX7qD/s0wHS2xJM+fMRN81jgJ3s7vW
rc1G65deBN+YVN4p9ggdU2sHVmthT9tRiGbROwSeKaY41UrQZyN2gO/fvud9
qBzNJccHNg3wGjSrQstG/ID14bRT03esRV+80Ap+qcNVdu4d+uNcPthDpkcs
mIY+yRMGbv95/u+dLvTstp3gsB4tp9xPjPbbloKVq9a0lw6h/Z61QT6lRzzO
a51CC426gA3dLwkMfEebuuwCLzU+GDL1izG+x38gf53Xj5hzsHRiPdoaCBZm
flbHz44WN1EDfxgO2rllJfrtqb+wP+SfiCxXXYsOtPMAL2qYlJ2VQg8vKsP+
erJ1i3iQHLr28wjsP5sVMzFRu9C/82PB9e3XnXJU0Qn2A7BfYx1rBPqN0GfV
bGE/ax66GTJpii46/W+YTn5uP/V1/gS69XQi2OLPQh2fI5r7wxuoD1tvyJ8/
6IdWf8oE9aPLi5luGoje6xkB9SbyGE3fPhT9SZIHPLPRRTwwGs0ivW4Q9svT
zPbie2iFt2ugfh35yCMv2oS+rJjRTSdjm3RKb7egQ1j/Qn0Mcr6swteJNjMx
ARf9+aLJTke/GVsC9VRQpObo1C900oIKBfXG+vz5si0fwS/CNWl0cjH30Z+d
kuh4qYtQr3ln6ZcfyaLZWh9DPd9/5UhYujK6bhsP1PvcrG1JoUfQta7lDXRy
dqK7zNAPfdf+4Ws6WbmLR7UxEH3Q4iWcJw8uab/RuoqmGX+opJNOrmfvlGLR
Kksn4Tzau/1Gj0g2WucW9wuoz95qi+Ot6M4n3wvpJOHfPfVgqS7cP837M+B8
C9NRp8uh39luSof6uGpKbZ8C+pLVfCrUE1FFNRZ1dLdQVgrcDzQbSLAJelXe
FziPNcIn9wQHom8Xbb5BJ5M8CgrBHejzchZwvu8Tr5MMDu7G/fnn+EGoNz0W
HaFhaJ7wSR06ib85ExxxHe2zMUAbziMmkd6YBHR2WYYW5E/32aj0XPTbmQ5V
OumPFp192Yre92aVPJz/fy69/LW5B/wz6+U6OimmyR9xq0YrJx0eHSSNZ19E
ndzYB35emu42SB6mXF+uYvcJ6+Mm19kBcm7wfEG3QT/OP03DZ4A4nNnlnLKI
Duz4Ot1P9tYKVLWkDYBFym959pOhW+xikfqDuL9Md3Z8IhV2lXO88+iyayIf
+4jfzzv2a5Lp4CABoblespwtjB53YAj89YnCil5yiUpYvDaGFt6uT3qIaJb7
VcOwzzjet3cDuknirNH6FPlhsFdRTWUXmWGxNDBvR5udZlrXRdZHn429EzyC
6/ml7NxHIt33xPOo+Cg4kq93tJO4Sj+r6KlBmxakne4kAT9rBEa8xrDerc78
1kG8QxZWOfCOg0cXiyM7yN4bqvzOb9DOH3r+6yC2ZcutBGvRhoJp0h0kcrjj
YX09ulJmj1QHjNhj79b36OqOHIkO4jedbjvUiY5lMdvcQcqPMD+1nEJzJrUI
dBDlNTWHjQS/4PzZf2DtIIqJuuEq7ujQ+4afKGJvHvXwpSea7euRPorEi7Q1
kLNoE88lvRSpGRAYf+WN1pNV6KHI7L0TnOoX0DI++t0UKSzwuKYVjDZbfqyD
IjLv4q/rJ6DJHZYPFBFfHIyxeoWeOyldSRGTqq2FA1Xo+s19FRS5EuLSYl2N
jhsIf0mRogMFM/RaNGfUBvAQ5xyPXQP6rJNIOUV43yvvHH6HruxXe0GRfTGX
jRzeo2lfmcoo4mVcfWaUhhYS3fGcInfXcsQ5taKZJ2ZKKNLSdahovB39VrIC
vCQ1tu10J9ot62oxReROdcxOdKGT0zyfUcRqizCfWy+6LDu1iCIi22XjvUbQ
VrxmBRThs72YHMI9AQ7zM8ikiNLx2do9PGhlZYO7FDHTd/0+w4u+J34xgyKX
9g1vyFmLZp95mU6RdKWTeqeE0KlPbdMo8vq/Th+B9ehskVepFPksanD/wwbG
88c/3KGI5Mp9i3vF0Ks8ZVIoolbMaf1TGW08PRBHERf25G3O9mjaw4NhFIn6
y2OyyQmtnXLkKqzXzLWgztNo0VgqlCJtI6yPo9zQb4t/X6HIz55L3fs90YVZ
p8FCLXPLFs+gjwgZhVBEpc5d/pk32uP7bDBFTpaPWrlcYIxfdTCIIkEFp65v
9kP7j6QHUuT+g67nXf5oy1xJcP1to+GYQDR/VmUARcajG3l0QtBbNlRfpsjK
UC1VpqvoIKVdYLmLFadLwtGj+/9cooihh2KiWyRao0AffM7uSbVYFFpTZMCP
Iolm2771xKCVclaBq/NKSw+/RDtytXpQZEop50XnK7SI9qQ7RQRqbleceo2W
jnoM1jC4XjVejc7/IgB27fWvPlPH+L1fv7pB/04edQsNaOe6K66wXj9Ovb3S
iC6z1ARPBBo1cX1AL1Z5uVCEn0uLltCMnqp9eZoiTu7NI58+M9bL0tiBInF/
Xo87jqK7aAbgiqtFk9/G0RJ5XvYUGV3z4KvvJOP3b26wowhPesJ3lq/or7FP
bWE9pMPnImfQZqQI7FDq+5vvB9pKa8CGIrGaLgupP9FsDnwQL6ed+Ld1njG+
V/nWFBm2OMxcsMCYf0Ex8KoxtaXK/9BCf1jByud2sL9ZMonjswg7RRG7JVuW
67GiS62FwNHX+bja2dA3uCWsKFImuGy1JQe6xWD+JOzf+7/WjCxH5+1mBnPt
GOf34EJ3frxkCfulolvw9yq0Xt7fExSx1m0SDlqD1sg7A46kKjYs52c42QRc
Yv1ENE4A/dU6yYIig1MZYuvXoW2XLgOvuHhT4sF6tNtaZXOKKCy7IiW7EX1E
XQJsddNbplSU8b4abnDEBsft6mJoL3+b41B/co/Lv92KHmJ9DO5TPKhoJIlO
r2MDc1SrKPdIo9lebQIXzjLvZ1JE3y1oN6FIT8CsdvhutHLx4lGKsK0cPsij
gvZxLwfLJXXo3yZo59wSY4qYizUYbFFHJ66kwKEFZcaP9jHap5uDn+zNO6aw
nzGf298YUaSr4Y7ZK210ZCYHxFlNok5oH0S/r1sKlhkMsGo+hLb47WVIkeNu
XjZmR9BybS/BIfM29nRDxvMNq8D5oUedXI6ix6OHDSjSyXPA5ccxtC6vBJg5
Tcnd3wxtf4ETLC0l6bXsBDr69OwRihwrWXcu+iSjvX7rYdj/NtXPVlijBc57
gfO5XefCbBnr1RgH/viCT3GpA2N9kn/pw/gdK84HOqHLlueBZXkdSv+eRlvJ
Vx6C+lnJ/fuCGyPfmMQgfsWldPecBzrEmQPiTwRO+XqdQbO20vUowu774LLx
Vcb8l27TpchO8cOVtHDG/H4kYMuWn0yHItEuld46FAn3T1dvuIEuOuqlDesv
qROkFYOu7OaB+Cfq2+uqm+igkK8Q5wxOZiHx6P5aDbCC7D7NskT0gpDNAYqc
6v4SonAb7WvFBfHIq3E1hXcY+T+bAvHSnXvZZNPRoZmp+ylC//R5f+5dRv5w
lIG5Im9c3XofzWW3DtrvVlKsz8xizB8vJ8Rthz6xb8xBT1U6a0F9jw7TSclD
z5l/1oT9p7I9QuAxw2IPwZ9HP76NK2Dk/4oW8KpbQctXF6FjAybAe9Sl9K4X
M+Zjlc0+uA9MtkZyPEeL04IhHpPk13TlBXrQa1ID6oeWGBdzBeP3njgC7Ue+
Nen7VzLmw04YzJPqHTX/Gp1j0A/t9+puoHnXoONYhtUp4jhXt+p7HSP/Jach
fvOuh4H7W8bzGWoQr9AXjP3SiFYbF4H42HxVi8MH9OhGUzBvlvOaoWZ0fKUR
tFczWmNs1cbYr1MWahQ5/e9FXA/F2C/nZ8Hxubbtph/RKYnG4NfHVvK3dzP6
rzEAT7IUmxj0oSu4/MACTywTmvrRyYlbwfsslnXq0NFbpi+C3difCNR+Rstv
8lOlSFKR6XGNUcZ+2hAJrrZaklwxzpjf3AFCkekVOV3Kk2i/+USw0HPDdSXT
jHoqlATWsvtjvnMG/as3Geyx+l7K41l0m3wh+PZLvV6pn4z85nywlyK1Tj/W
Z/9GOzZfhvg3vlTLLQvo6pW5EBd+vT8tfZGRr7rdYOX0zROGS6bwvPu3AXzc
n2n3Ulb0Fo47KhTxsei9UsKGPpsmC/F45bIWJw60UJs4xIsEEjYIr0BXWHpC
vGXujMt7LrRffyrEv7YdeR6wGs12oA7M/fQ/tp28aLetXGCZGE6jz/xoCdE8
eF7PfSQtQRBt8aVgD0WcD1VP6AijjV3twGFSGbsXRNC0ikZlijzg8A/N34Su
5xWE/mpGzFqttqCjaxXAQzWKG9dsZdiQCcx8j9e1ZhvapJMX+tsY9O35eWm0
h5s/WNXqPZukLJpd8jb0b0lyjXq2o9+rvd9NET/hsPQb8mhN8zyIJ8/bTqop
old1hMHzpZ3qyt93M+YrOhXaU8UiV++roPu31EL7H3F/Wo+ponXTN0F73jOd
Gzk10MNseyG+w+CZa7kmOnRJPviIbGyZ2wF0ZH0A9Oe20n3ZJl30/vbHEI/8
ctC4VQ+dIn4CnNsgkXHlMGM8k4eg/duspVOKhuiFpn7w6JVB5XFjdKn0czCb
7aurKcfQqZnd8LyYRkqbvhn6Sd06iGtuvLBpyQl0eVEf2HrxqNvTk+ghFnNo
H9Cz44WdNXpw9CjEU8u42QXs0Cs4BcHliRPGbx0Y63VfEdzt3ZDh58zIr2Ev
8LzxgykZV7TckmXQn8DO4D0D7mhW8Y0QV1htFXbTC71DsFeJIsbTKu1a59DC
r1oh7tUkKPrrPOP36qvB8zG5c245vmjxwBaIPwlvfWFxCe39tAOef+/whJ07
AJ38jQXaT2hdP1oVhHYWDQZzbnG+e+YKmuu6ETwvwXxgWiwMPTFpCD7Qv1ml
MwLtnzQJ/dlXMIVHXEcHZJaBQ1J621Wi0a8T5KC/u75lotOxaE4+fni+0jTB
PeMWOlHYFdr3KZwtN0pk5G/oJvBfXgMOttvoomYcn/D3/0xK7zB+v+cKsHIz
Z6ZzOlqB6SD0Z/p4ZFo4Ez2V+Qfsfb1a5cN99IML16B93OmM8MBsxvyMVEL8
qY4/tTMX3fPYF9xZ0fq75BEjP5/ugXxc3LltvcoTRr7HYj5teeivVlnI+D09
OtBeV6TNRvMZ2mXGG+IeN7ddrS9BW1Xj++LZL+folTHG/1EaXH6prYlWzhgP
uzV4cGbbN+NX6MZAJ3gfu+Nl3o9VjHrwowTiMr1tiieq0RHrw8DGhpLmA7WM
/s57wv71rbvsb9fA2M8PaiCertKeMfYObb1dDvqrLZCscX2PzsvC/T8hHjD6
jcaoT/odEOdJaV/u3You3hQEVlotJTvfjrYfDoD2lqEBhv6djPev3g71KORP
+znmbsbvN6DAOR5SSaG96CCpRXie9jmgnLMfXfk3DeJzZtSnG4OMeIkS1lua
FMuaz4z9VGwBVtcKFE8YQWcHBkB9ti+jdNaNo2fTrOH9kbLSrmkTaH2nz9C+
8F5g9OZpRn+XCbhTsONp1jc0v1IePL94Q7pDapZRjyTpEN/CGjT/eA7t250L
543uhY718r8Z/Y2P4fkxJa1e+gd9b6Udnn82QbYqi4z+ta5CvLyz42ol0zSe
N38jwYOH/svVZEF3LSqB2d8Eva9fitZI74H+ZZQ6v+mxo9VC68DGj/7ja+ZE
Dx6agfPYVzRY6ehK9MxoO7wvLaHT/CM3WpKdF+Lv1UK85zejEy8xw31i9tnH
JH9xdArnQYgLScm+ZN6G3m/hC1ZLD+kPlUK7vSyF892er4tluQxjvA4P4X4R
GSG7NUoOzfTDElz4L0R3zU7GeMX2wX2o82yXa8Iu9LifH3hxTDZmnRK6U6AK
3r/l5JWiNGU0T58bWLetq2PzXvTr0CNwv/LQkfuTpYoW5aqE5+MrrohIa6CJ
Gh/cx8p3dqs/0UQrO3+B9oPZcnbyB9CLveZw32MXCQ0r1WHMj34bxP+72Z2r
ooduHNgN8XgLpufLD6N9jdeBmcTFarsM0Pda+6B/52md1ofGaD2XaHBbqVu/
zzE080W8n5Kgm5MHzBjzt7oD7qfZB0vn+U+gs/ll4P7Lw9e7bPgkWrxa4iCc
Z31L+J5ZoxceWIOHs8RFQ+zQNwprwUc8D8oaOaLTH2nB82XKHiqip9GVhQ7g
zay3dL65olelnYT7dmTTc5NKD7T/lD14Lr7PJuoMOjUrHtpbWbF4Wnqj4we2
Q/ztNgn//y4wxvtlCdzf5b/rXVu4iJbblAHx1HLPxHf+aJEP3vA9wR4afz85
kDGe+A9gr8MvCp1CGM/ftAL3CPS/UrqKdowVge+J/YOsTcsiGPPtaATfJ4Ln
9EfuRzHGc98Evm8cK88eEXnAWK+Pg/B91hKedGIym5EvvI1gFaMK5/JcRj4I
h5nCfUOYfv5aPmM87i/Aq4aXXTErQNvOBh+DfH8sHbutCG198zN8/w35GKT9
KkZzZjRBe30N77y654z9dLQZXLL89vP4cvQTO3743tzY/qrW7hVj/U9q4/dn
6lCr/GtGft6jg2cdOAZYatBTz0rge9Zyu8xUSx3j/TPR8P1bP2/4J+MtI/9P
OMD3847q8+yeTeh8Xn5wyvUUPjUauuibBXyfsx2rEuVuRQ93+IA9Ng7L9rWj
7T8/hu/1rjHOvY86Ge1NPkFc86msrl83Y75va4Ef+RkfO9iHVqF5gvn3X7AV
GkB7fXtuA/cD7lTPMTr6bnu0NUXGO1/7lw4z1s9sky3Ui7sj166OMd6Xddse
7venVySZTDCezxi3g/N31/YHYtNoKyl+iMcuHn06+43xe7qSwQt1vpVvZtH1
s56OUA9i0ppifzLyMTMaTDOr7jo1j45LlHWG83PL2IjcX7T84DjEMydX/vj3
Dx2r43SaIv8DSlRgUg==
       "]]},
     Annotation[#, "Charting`Private`Tag$40900#2"]& ], 
    TagBox[
     {GrayLevel[1], AbsoluteThickness[1.6], Opacity[1.], 
      LineBox[CompressedData["
1:eJwkm3k41VsXx1EhTaakUmkgSWhCqmUoESlJEg0iIZQhkSJFhsqYSkhSODiT
4WSopMIlKQnJEEmmSkgypXfv9f51n8+z9l7Dd63f3vs8uUttTpvaCfDx8WVP
4+Oj/11oK5Vna2OixceX1Fc+xIWyA38tLtjvJyzsf6OOC+67OsZinC0JWx8y
6rwFi3UqE1huRwl3s5TucOHrgoNLbDfbEB7JWH7hMWy+ucv159PjhNuKtZ6m
QNQc7efnte0JVwvLTc2BrtD14sIvHQmLOku9yYCtU1faxug5U/tRy1lciPZb
kCtbfoow35/B3Gw4MxF02TzFlbCJwkqVDLhXwJeZ0OlGuLildmkWvDrr8759
pQdh1V0JYUz4vX5oXMHxDPUXGiDLAdkBlxWnMzwJc832KzPBiN21i/ftLGHt
TStsWHDW6ZjnuJI3Ydd3h0Y5cF+h6a7OqXO03mn3ndjw+qtZWTDHh7Ds3yZt
NvxJftNX1X+e5v/93jkOLLM2mCe5zpfyuGYfC4wXvdCy9PCjer7WL2OBd+Nm
h6Tci4T7pQ8JcKCm0tLgl48/ze+f739MsM+4fejWwku0XtXafSyYCKl13fSE
sutOexUWRNuLXWk+dJnW+zH9KQsUduy+c/EvZe2pQlcy4emKa6xliQHUn8hY
GRNMp5Q/L4VAqv/rtgMs6P48td6hlXKxhND7TPAr1umd4X+F1rNVJycTJO75
TbJlg6h9UC4mExi+j8VNn1N2japqZAIcGpH/fSyYsL/tMxEmvNfcuDlWIITW
ZxZM1jvMd9+z+QFl/zTWu0yY/MO2/bQtlOptIvsoE27Uf/O61EG5+gtvKBMU
eArXV1y5SvP/4bkyE4pu2CX9J3eN1u+01z4TzNyTc0+WUS6u/JOWCT0mreWz
7K9TfX92biT5q8i0cIXCqH3rM69MkJx9cGAfg3L1nfeCmZDx/ea0Pwbh1L+p
ya0M0KqsmR/XQ9n6ibx/BtSmz1HeejWC2l18TmbAxu3yS13nRlL/PtrNGeCf
sz3zuR1lrnWFdga8Wma7UeIR5WJm1sEMmBt96dlxwSg6j1sUPDLAmj9p5yNz
ytrRmoUZkOla9F4ojTI3+8SvdBhubT588A9l1eZrDhmgvWe8K0M/muqrO2ie
AdeK5rtP3KbMXfBGLwPq12hMGHdTbouNZqWD7F3zoHsaNyi/P/kqHZxmeooO
hFCWHR6XzIBH52/E6X6kbHLIuCEd+L9lrYhZFUP9n9tZkQ67LKvZX89Rjszs
6UqHWxV9GuqvKLepnGamw2eNWS9DFtyk83kuITEdYjqz3se7UdZ2zrRJB4MY
8w52OWVrMX1OOozrjA89X3KLsnfM/XRg/7w3re4sZVmnthPpYHN3u1R3FeXq
pnPB6TDXqEd+fMVtmt/ucON0KB8JU599gXLkyCWddLiQus5g6XvK1Q+tbNNB
xeyDxQbFWKp3xzXFdGjnv+Cof4kyd1+tMMmfI+tj2UBZdeX5LgbsPFx61UXl
DrX7abUwYELkZLx/EGWTXV/npQM3fzbzRgvlyCJtuXSwPZHzJHVDHNXHYvu0
dJCStKgquEa5erXHBANePZ9oed1OOen6n18M8D19v691Uzytr7i/lgGqi3b8
G4ykbF03t4oBHa965wh2UzY5caaZAbe9I2TnayVQ1rdIY4Ch/Ia1Srcoy7rt
z2PA5PsGHa0flP25hXcYkHXJ19R0+12qf5ZRBgOOqyyztYunrC23+iEDpFvK
PLwHKXOFbRMZUHnVKfDazkTqf1YzhwF+GqI3E5Moa2+4coEB6zpzU7L+UO7f
GpPCgK83Dj4q2X2P7ncodGdArM5k2YcUyibTta4wYNfP5A+9E5Tbrk74M8D/
zfKhyVVJlLc02jHgoNzZCyH7KasuuudC/F8onyp+Ce1hEicZMPP9grB4JmVX
6+3Ef+cql7lyDWift/Y0A4r9n91lT7lP63/43JoBcR/E5DVU7uN8tpB4HsrH
2c8tKVt71ZD9u648UjMKQo6OdmWAfLPws9osytUPVvkwgG+9lf6RFsqiH5cc
Y0BjKOttl3AyPT/yLh5lQG7bvwNuGyiLCjqbMiBM3bRt7Cjl4traQww4Ef7Q
IfAari/5z4oB2l+H+2flUa7+bbCHAQu27Dx3u51y241eUv9QdDz/0tkPqL7H
F7gx4E3Pj9CMTZStR0uMGZCmrS2+wQ7tKWoHiX63o+OeRiLbmxO27OtYpv+E
cvHOG4Q36KlnVndR9jcNJ/5nJ4Sut5R4SPVgH7dkQPdg0+MvQNk/bxbJ7/lO
5e0uJyknyd23J/ol+b8evkm5+vI/Us+ZPzVm/s/RvmUvqXf3brmW6T8oyyow
9jFAIcXL7oZ0CvVfWkf0F5io+CGznbIse8cpBjSZypxNPU25/80A6ZfyghE7
49gUvO8XkHz8P7/fP1RMWVW3lcR/z+DoxfdQ5p5470j643pto654Ks0nf9CJ
Ad7q9nI9mql4n9jYkHmd1J0baUtZVjuC9NM1bGyoJRfX5zz3ZMALs/qOwBbK
fBWHSP/nymTXrhZMo/Wbrz7PAIcvYSU1ypRVnQS9GVCY4Zh77gDat48Gkflz
13so60+Zz0X8KgOObloa8x8DeWJPMAOy+f4GnHpHubjzAbFPLW/wmDtGWTZK
KIQB5hG5tk+WMSjzYq4xIN08cp+tEWVuikUoOU8WOW8TOUOZ70lBLNH3q/76
rATKxYLXkhlwn7l8uUUpcvqzODIvHv/E//2gbP3bl3zPOzY3CaRKpVN9/8Qx
GHBHIG9wlxblar8KJgO+V0S3/7KnbMJZkskAiDpVExdJWbvFl8eAKAvDFzoF
lEWt6nPIebNEPrv7M+XikX3ZDFDr4k+OEMnAeel5w4BQdkuU2nrK/XNynzOg
2bPgUosV5eqsw8Wkv1tvugUG4voFCh9If6e6HVvNoux6XKSa9Ldy196aOrR3
ijaR/t5Q0Dk3SdnacH0n6a/l1LWyKzPpvJ3a3ErOy6Vtsv/toWzia/mJAYt6
Houe8qZsbfa5h/Sbe5tv7n3KbSNbfpJ+e3n0P66gzJcaNsYASa09bTaDlIsN
5vGlg73g6urpC5l0/ZyEf6TfVYLF3G2UubNOkvN65s12zgFntEfNEUuHo4eK
7k3GUNae3SKVDtnL4yJSnlIWfZQkkw5Tv3le3NVJ2VotaFk6HMjee/rXbBat
V9hROR0yzq05GqdOWdX9qUI6TGhP36NjTTnphc+GdNgj/BW6Q5BfftJMh+S3
xcoRWZSLdRfrp8P37yp9imZsap9+zDodIHfGp3cXKEcGpxGOOt9V5Z1CWTb+
hH06dOi+fLrkDWVr1T8u6aAmco9VNoy85+qZdAh553PXZQmH+uu4eikdmmLN
wyQNkBMUQtJB2Xqd72NXym3JjYT9V852sblD2eRnR0Q6tPZZaWx9TtlaOuYW
yedR+hTpHrQ7hj5IhzdF5+3PCXNpf2/ZZaSDX/KyqhMylNt+bmSnw9a1RbYy
zpRVP5qR90bh7t+RwTOy8L63mJoBuaG23w4bZtN5eilwMQMY/7SSRMpzaX5v
/pH36IKaQ+4XVArpfvsZVSxg5KRtjNd8Rvt98W8RB9q2Zqr2WLyg81m6uYwL
ecnJvi+ESqleg63hWbBoztpt7iH/EZaWuwTZUH5qYIuy1ivCjJlx49nAX2/A
Kf7vNZ2Hxa5pOTANihsit72lLKWnlwvuX9QMLXZTbnuxwSAX2kJYj5ccpGx9
NtEwFwrfxyWyT1HO7zy8JxdOOXoef30H12fEH8yF+hjFfqF+yuXbZ7jkQq3n
qwCt3dXUbhV4Ixeull/Z8mAf5ZG1GjdzQWehzm/Bg8gFj2/nArs478QbW8r9
Pw0TciFkRsrOw+dwv1lbSi5svX9xzvmHlB0+7c3LhdTXG+IfjVGudtZozAVn
4898Rf8oq74835QL696EnSid+o5w9wyJT7nw9G3n2trZlK3fBX4m+dXElg8s
o6wdINaTC/wfJ34rGVFOSl8ykguHvpaYPIinbJJkIcmDZSfcHmUkUa4WHZrL
g+7ORTLZKZT9Tcrm8cCj+2xXMYey9PfXC3hw9ZuC36eXlPkknyzlQd7A9cz5
3ym3bepV5oH4pJlg5JYawiGpfPo8KGp3DJyiS1m6aZEBD07+5yfgpU+Zof1w
Jw+kmDf8e3dR9pfwN+LBy0jG5GFTyq5lg7t4cGb5xPBqB8rciyL7eFBv8KDr
vxuUhXOOHeHB5TX5dpvvUFbwM7TmgbJ41Rd2ImWLlfbHeNA4/PnYsoeUrf0i
bXgQ3DTcejOdMp+esy0PNhTPODKdQ7khQNGOB20PZZsv5FJWlbY4wYProRst
+wsod/8NceCBxinDBttnWI9hrCMP7twYKP/XSzkyWvAMD3Z4C+p79ON+S1fC
g4cWlnb+RvYo9eRBoo7qNstxyhqnnnnxyHtQ73kV33uab8CCczwYy48tiJei
HNJ715cHhz5pZajrUtaYXnKFB8IvzRQy9SlXn0wL5kFummPqYmPK/v+yQ3hg
fd1vRbQpZQPO81AezHK7kTzNgnJxxcmrpB9TuuLeu1DWNvAI54HsqvBrp+9Q
Lr887RYP3hiLXalIpGzyd9ZtHlxwj/Fb/hDtv8YIK96e5+2bTtnhfkMsDz48
jnP7wKYse9XrDg8C2xY5rc2l3FBkGseDddPuH79WgP4+XYwn+q5aceRrEda7
RT6BB+G70w5olWB+ynZ3ebDFQ3HvnQrKfHHJhHtvswx/vUG7UV0iD2KfqG43
rqU8ctT8HtH7c87WtI+UuerCSTwYmqauzt9KuW2v6H0eJCsWqlp1UPae+4Ww
yZ6tirweyvm60ck8+OtRvHzOT/TH3PSABxmx2xY5DlEWhjLCFk/LpF6OYn3t
aQ+J3oJV072m1tL1MV0pPHC+8/Hnp/mU8wMfMXiwoOhQj8YSytVHLqbzoLy9
tT16BWXp/yYJL1fqrNuhgva8Q5k8qDZxfJu0gbLBiWDCfp7fy8c2Ue6vyGLy
QCnu9AszLYynl0O4sWjwMXs7Ze9171g8CPniyRM2pGzt85uwmvAo22YP7g/a
zuZBh9IFxhMzyhpv5Tg8iNr7776UJWXGHB5hOHs53vUo5YZXZlwefI+bdvPV
ccqqC1IIxz0LCV9xEuMtmJXFA4OOGSF+pykrnOkiPCwccanhDOUk/qBsHjxc
I35+nQ/6b0wjbGp688z1i5T5ztjk8IDPS/pUZyD6031CmB0fb699lbKJ0yTh
Q8WLj8VFUA457J7LA5Gv9y2HYigXZ8zhkfNmupzZ7jjK3CRdwseVGcaMe5T9
Y/4SFt+3Wl8gBeu5b/6IB8VebO1DGajHaQfCpxLWaj7iYPyt/wjLPM9dL8pD
/qKcx4NXX9XXnCzE+v/dIewt8li+5Bn2b9MYYXkVkF1civ2wCsnnQe2+5/O9
X2F+F+cTvuy9XaLmLWVZr2eEVe/+N1OpDv1ViBbwoOW5oWBQI2XRiTDCVzur
/rW2Uhb++JSwxoy9o5u+IvP9JtypUjt4oxf1Ox9byIMYswPff/zE+qU2EN6b
Vhn9bYhyt+prwrPHtDb1jKL9mtRjHlTuym3tnET71X5iD7mnENQxpY6eV0nh
xK43mKDULky5XMuasICe2PvWWZQb7pg+4cGz21fOtYhTFm5sIvYLvaNLmuZR
DmlVJ/ZNW0+VNchQlo3VIDwc0e5cv5Qyo+8m4Zx2c4laecralqcJu26sLHi3
mrKop9pTHqwJ0bJ+q0rZVSOd2HsbcwSrNlLWeDNBOHWNAuuVJuW2jt+Ebf0T
9pVrUe43UiL7Zd+LjpVup5xveY5ws9yVpJc70R/XlPAd79Edz3djPc77CZtX
uvwo2keZT9mXsMTi9htPLDC/PZSrXc01Cw9jPftnFfEg7OWrtjwbyt2C6cRu
KKUVzLNH/Zo2E7uQY86aHGfU42QrsZc8XlnLdcP9ZdbEfml2gg/7LGWF2b+J
HY6JLmWex3r4cgiP5wT+l+6P+q+dR9bnC466pF3BeriyhD0PukimXEU9NLwJ
r2N+LkyOoGzR50P2/5zcfywphjK3RYPYmXtfCSXewXx4P4nd8SH5xBIpG2yb
Tezyf7LN7jzA/Jd2EvuXnSvHbzEwntxpwkkJ8fdjWGjXTyJ86Occg+hsyt47
Kc/XDeyLyMN8DjwhXB8zEhP2BOuVX0Q4ust587XnuH+HLOE9mp8/h5RhvSu/
kP7NDNsfElSJehdnEa5orVAOrMb8/BoIB62Dukt12N9dJYS3Xck+f7GRcvFj
M8J8DfLLfFspx251I/xUMb7cpwP10zEi7OM757R3D+bbQ9erVwfMPduH/kQH
yfwOLRt57PEL8xfzJ5zl6WzjNoJ6Rr0jfKq8Tfj0X5x32SOEVy/cz3EWqKfz
Gn+DcLdLxf6TQpQ1lm0mnFK8dcJ+JuXq0D7yfdlIZCfbiaFd/T3hJSfkd9pK
US6/H0i4OT/up/VCtIt3ku/7zow5t47IUnadn0bY/EjAlkNylPunHyQsnvWn
/aAiZVmbRnKevJ3iHHpABe2Rk4TdCw0Mnm9Af1EdhKXc5IRWa1LunmJNuGCl
QFmMFvqPeJJH3xOfAie34/7WS4T5bj7e5mBIuWGtNuEHRrECNXuwnsEScj7u
EPB8vnk/5aQuCcK9+Xv9UywpjyyyIxx+WllrjjVl640W5PxdKz9j0tsO6xXK
Ilzb3PWk/ST6V95E2PtGyfldrpRjg/6S813G8L7mI0/0F7+f8DM+v9El5ymb
6F4n94FNnmV+qD9lrqMaYcFT6l6/rlCOtFUhnLFCUu3wNczvri25b4yb+ofK
IilbXFxJuD+qKkf1FubDm0fuqxiDDPe4ePRvuY3wsuWLTulkYb12C+l92CBg
F9GMdudrGTxoD29dPvoZ7ZcuEL6i96Tdpouy94915D5/ne1prTaI+jaLkvvf
1dF0SdIf3K90IY2cL7Iqn6b/Rb1jClJ58Kh+xl0PgQ/UriVG2DKs26pFiHJS
O31PTG4rXaA/i3Lsmhby3rg/dv8jV5xyw6oAwtuz/GIXSKP962byPum2tzoQ
uAj93TlA+NpiDam+ZZQVrp8g7xvlOsm6AwqU86v8yfvHU/eN6er1lKUzf5D3
E5N5R/u/UMqqM47c4MGRKHtmbThlb/40wmJnN0q336As+0IgmpxvllMCf8ai
XWpuFA/Oar37OXGXsqtlcCQPFFbcsxJ5gPYkEcJNwi7/zWMg3x0m783wH5rr
5VjIr8QIa9cI31uXTbnfr/w6eS8/qhfRzsN8tt0nnBL/8KzxE8oOdV+ukfeY
v3u75XPKfCFD5D0rYqe926EM8/vTR967dX+8/t5tRD39nwWR+65ZzzGz9QOe
7znk/az5XKIuvwP1St4XyIMfKZ+1y3owvtitAHL+XeUw3/dRthj6dZm8X077
Sn/+hXaXlEs8mGZmFNg3QrmtTYdwvsb8/vG/lEOs1vuT3zeLuqymT2mg34PV
1Yukn7rmhWdWU2Z830ze+9yVK+Qvq1Iu36RwltxnMwejIjZSLq7XJ78PyuvC
HDO0KHvf3+VBzlOHUum2fZSlBe+c5sHK8A1eRhdw/ZE19uQ9+1F8w7IqyklL
5u/nQc/SnfnxNZQbrGvI76XLJy9umdtAWTWxyJS8X8e/bRf+QjnfaKYJOc8X
l+7vG0F/HxXI7692Gy+vwhUf6Xl3IFub/P763lRoeoFybMP4Kh7c/vdQJ2B1
I83v285R8ns0ZKfOF1XKjKQFf3LhtWif9jY1ym1Gsr9zwf5OtPaDzZQdLGcO
5YLAMnXtKTqUY9nyg+T37fYKCDBHf/eKvuWCbuiPzQGXKEsPzmrNhR/iamoB
H3D/+NGSXNgm/59iQEAT7ffhW9dy4VH1BpNTJc10/yenBST+mccRR2U/0fNP
YumdHEhPCJuxxa6VnhcWXjI54NnuldW0t432/2Da/Wyw99h4MmGyDe/nENls
2Fom/bzm3me6vvR7ZhZ03BSWu767nc7bqf/WZUGRXfGw5Bhl4XbtUi5c+HP3
hETcF3p/iWee5MKje1HOFQmUI6P8rLnQr3/F/eI9ytzEKhsuKPZ7e29Mpmzd
//4oF+xinf2+PaTMt0jwGBeStK0D76dRDvnlZsmFxu59Vw9kfMH7K+EIFySj
9CNnsSg7AP9hLuzetPnWSw6uLzUi60M+Kyecy6askJxpzoUXocuSVXhotztE
eGKtFONrHmXhiv37uaDeOJ0dX4j5rVcmdvfLf3P2PsV8zGft5QJTcaBAqJiy
7PIVplzorOl49vQF5ZFUh91ckD3fUOpRivGiR3ZywXL568pV5ZRjO6YRjql8
9q71FWXXK9lGXHjjkfPhZhVlxpp/+lyYLpPWYlRN2VtHjfD2krgv/O8xHy5l
P+fwnrw6jCd3eQcX8iUv/3RpoCwtpKLDhcEnnr+XN1HOD07U5kLJpLhcbT/l
YiXORi5MpgquvvqLctt8GcIae8ZUtYcxXmvaOlLvnx9qwyPYL6thFS6w7n3e
whynLPpBeS0XuvXrdG0msf7L5oSX9ZcbSPN30PiLBhW5cCj2ye43UyhzWY5K
XLilzTULFKSsGnqD2B0uGwdukKEcUnN9MRdmCIZ8idGnXJ3wWpgLu/SGnskY
Uo5MUZrJhfBA64SHuygnidwQ5EL1y9feSntw/YknExwQn7Jpf+5eyv0/a4S4
YKabsnaLGeW2F/tHOHDrktjsEnPKDh72U7jQUOzba3QQ949NIfYFfL1l760o
i1aLj3LgkJb5A6sjaN8qNs6BRL8XF79YUza5mzjGgbanyoecbClba7X/5sDS
v3Eav+ywvvdmnRyw2SI097wDZdll6wY58PC8x4CAE2X/2W5/ONBZ2Fp11QXZ
j/8rBxTGjDLEXSlrB08QPrkpPyjOHf1Ne0j2M71X2C7zRPtRu0YO9OVFamV4
IR9kNnBA5c/EwnU+mI/uwnYOuKo5jhRcwPzZm5s5kO1ZV6tzEe3JVfUcGMrV
yaq4hPVIS7dxQG2IFbY3EPv1ubyKA97rF5z8GIT+b3R+5EChe9COY6G43mNd
DQcmsgaX9VzD+j7Vl3Bg68CRf67hqH/4rScc8FOtbBqJRD03n3jOgeLT6vn+
N7B/zLRqDghwHsQI38L+NMu/5MD2vjlukbFY704/LgeC1lwwlo5He0lQNgfK
nbtXJd3FeXgm9IwDIkwzQYUk9KfOzeKA0bfidk4y1lclQvK5rrjmmXoKru/w
KuTAG8c78c/SMP+bgrkcEE2f5q2fgesP/M7ngGm3m9lbJsbzUGZyIGblJ9UD
HMxf+PgjDtSfMJzVmoX7Gz4mckA69VHPiVzKruVdyRw4+HVZWd8jzP+R8W0O
xK2ISD5bQJnvystMDjTbjvtNPsZ8rFlxHFj8wN4qqAj7/2hDDAes29+rz36O
eivnxnIgeam25K2XmM9XyVAOdFgz+xeVof8vj8I4IJ8kXZVSjv6PH73PAfvW
wPQ1lZSLV2ue5wBj8cAVXhX200GT7O89fNhmazXWM7SKxFO6WwGlNVjPxtek
nlPNGxca1yGr2vlxgLsw+U/tB+zn7UPhHBi0nF17qBH1vmt9jgMb4ny4Hc3Y
f4HFPhw4+7HzunMrxk9wusKBfOl9jkOfUR+bB6c5MHbgmd6FDqzvlOVlDmy5
vXrZ1C6svz6N+POtvz15rQf5RQ6JV7zxsbTQd+yP2nRXMi83P6273If1tLsT
f3pD/MZ/+1HPKaVnOBCyT87e+xfO+83ysxx4lW1w6ddv1OfFjRMcmCXuHH9q
BPU74EH2m7hF8HrGMN7uhRYciK7Ofnv8L/KgmB0HalXqe1r/YX1l13dxYF7E
6BQrga+0frXkPRyw7JNZXD+VcnVOJ+EEY22NvUKU26quHeHAJ6at6evplEV3
P9An58PMYGf9mZT5Pr7Zz4HjThlBL2ZT5qbMIvFTX1UlbRWjbB27ZxMHulcN
FOZLUPY/9cGYA6tDJevWS6E9Qfwo6Ve3+k+2NGWTeRnqpF/6VtMVF1Lu/6Wk
xYFfqX7LUxZhfgWzjcj3LZi8VVYW+aUAkO/brvRA/DLKqr8XaXPgcUm3m5Qc
ct9TDQ5MLp95PWolZde6VCUOaAeopM5UxHiS2sR/QLtpcbAS+uO7SvIt0znb
KKCCXJS6hAPC9+8M+a7FfMwebSTfJ9/T2aPrkYOXKnIg/Gibwhk1rH/J0XUc
qC6asu2nBtYrf2MNOc8Xrzx8cjPqGV21gAP7fQ29vm7F/SdXL+ZAbLNLlLU2
6hnTvYgDjZujMpt0KWtXGMtyQCY+t9RcD9cXMYQ4cHTsQ+s7fYx3+NYs8n0d
HB/dZYj2Xnsp8n3lL5Ys34X1/5Ej8eSldZW37UFe2iPHAUcvO4OivejfIkGS
nMf1ITabzDA/tVHir28j80KuOerV/2EeB9befHtL5SDmZyQpwoEzQ4PcDCvs
n89Mwo/2SVXKHcF616nKcGA0e9PXJGuMl+RA8t0ifvjfQluctwbhfjb4ufnP
v21HOdKMOY0Dz6sfrBd3wH6I6bewYarqf8ZhJ7E+j/WjbNgR0Wsv7EK5WGp0
nA2hfbMuB5xG/wJCPWx4bbw2YdIN4y91I/XNZpk9OncG+/daio98HzO9q4fO
ov8Zx/vYcMMpvvf0OcqyWRt/sKH+VdHUb+exvt5jjWyQVmxffMIPWVR0kg2W
odM2ffbHfOYkkPzvdivsOxSA+fsJtbKhTX+Xy4craH/XM8SGZWmng01DUJ9/
wh/YYKHxH2vKtf/b676zIbxicW1uGOZ3nFvBJr+3zo7ZRaLeH00/sWHsW5Xs
vBuY7yn4xgZVXzn98pto1ytrYMOJ2b4u52Jx/6y7ZH/CvdobivFoX+g9wIZ3
qkqFTXdRj/OLyH7BFwFt15NQ/7yQUjZs2dckCA/QPlnRzgb3jnVrfqagnlsL
PrKB4Xl1XxID50H6OI8NnwTbz+3NxHh/TavYIBm7KUmAjXb1qaQew1VRZTlc
nKeihko2+Bd2fz+eg/782t+x4ZGRtoTUI5zPvzNT2fC9+fam//JRP5GdL4he
p34e9X6M/V3PesyGA/92BK0qQn/vGjLYcD0ykdlYjKzz4ykbXiwdrrn2EvvX
Z81iw0i28eiWMqzPYs5PNihvT1nSV476aXVeZMPxugm9e5VY7yUFNhviTpg5
m7zB/uyczmBD9Z/MaP53WF+pfj7RK3RKQfZ7tNdUknhbFli12tYjM71I/u6Z
2dPmfsTzcOftO0SvLSJKZU2YX++tZDa0VB0z9fqE8d8UxbNB/GiBt8Jn1Mv+
x202GPSL3vv4BfP/4RtNvodLDqVXO3He2qcHsSFXvPjb5h7kHPUUNvQ+mCf+
4xvqI/D2PhtkN57WSOzDeeLbQvI3Lys7smcA8+GGJxC9Diy+wjeE8Q3+hRG9
uj0zs4axvg9TfYhe56re2Yxif4p8bhK9ZsiNSExgfbYKRG/bhAuLSycx/u3b
iWyIXVO7/Sx/J93Pvn2WDW+KVjutnEo58oJ+FPleTQKiGgQpa19OvcwGzc+N
eaHTKRfb/LjCBlf3dZ80Z1Lms3zgxYbUKVenfp+N65cbkvqbYz4r3hVD/2+e
nSN6yW/au1sS2fKMG9ErL9LrnxTGm/PwHtHLoPsudz5lWbnZd4leH7VKjsl0
4vl/k8TvOXm7V3wJxpdbfY0Niyf6REuWUhZN83Jng1nYDnXPFZRN/t4n+lxd
nHhYfiXG2xBgxYZizu+AD6swXlNgOBuGtY0zQpQoJ/G3k3qUah5Wb1JB/2f+
hLDBxnZiuHctZX+nvkNEr6F9ixI24Pq5Z8+Q80VmxYIl6hhPwfYBGyT0hqSS
N+H68ThrNpi4lEjIbcF4a+MsyPlwM0aUAZStp3wl+yufHp+1WgfXX9gVwwbh
zg0i7G2Y74sVkeR8nD1NaO0Oyv0nHgMbAtTqpuQaYL17Dx8g9RxJ4VM3wnyt
+8zZMBnk+bfAGNcbBxxmw2aO3tgWE1xfNN+JDd4f5v55Zor2ZMk15Pv99/WX
7n7M/5IM6f+vlY/6Sw9gfPMQ4l/VJOiHgSX2t9ttOxtOeZv3Vh7C9fy1y9nA
TJLv2n2UcptXz0nSn/LhL++OUeY6bCF6yw+UtZkdx3lwtFIj3+v82y0fTmB/
F2iR+Mk69o2WjuhvXYcGG1od1T+0OKFeaivns0EmWqjW+hTaeRLG5Lwu/FD9
xRX9LZ6wJf1oT6s64YH6PdljxoY6Ee9XPZ6ox43pJH/x9Qb/OXuj3rsFSDwT
K+mSnz5YT/nFbWwIC+gudvfF/BcctmPDq8z8p78vYv52faRfwrUhhd6XkV0X
E/31JizyxgNxv2GqAxsur1iV6xeM9rOi3Swo3jXK5b+K8WXtPNjw90wFK/A6
xndwJvpp3r2TIRSB9Yx9VCH9KHVMuxqF8x12kuTH+7Hp4awYnK9zu1XZMDhX
5H7kLfR3wliX9AMa70rcQX3MP8qRfpzIiLsVj/sjjHXYkBnuc3t+InJbsAIb
uh8ZxiQkUXY1qt1N+tG6IGrJA/TvzU/6d1zoW1hyCtqfDm5mw32Vx1flGBgv
MV6E3A8HrgUzMpCP6E0n/fC3ClzN+n+97PWkH4zVl9gcnK+5/fPYcLt63Hdt
Ns7XQZ+dbKgdqfTJzUW9MvhIveJLE7zU89Afu2ApG/bsdD5TWIB61BWS+Nfd
trhtfYL+J81NST/uzDxVXISsWET6I/Si+eS255j/seB/LNjey7Qve4n6rvy3
ivRD3Pf4zjKchyO5c9nwTNP42Oty9H9yXTsLJmwWHdlTifHtL5mQflz7YVlT
hfmrdkiwwSvn6YH91Thf318Jk/OnKcysoQbrebO5jgWDU47star7fzz9GhYs
P2JjKdmA8zytg5+cP/knbKsacf/pBnk2BIo7OQe1IL/kdrKA53zaU6sN46U3
CbKhs8zDb6Qd589IqIcFUku9g7O+on/v1ioW6J+/EHmyG+v5JdDFAu86/zvL
v6EeN7vfsIChciW5+QfOw8mlRN+PoaGZN/v/H3/2KAtEOsJyd//C/M+6SpJ6
Ifqp0DDGZ6rLsMEp9lZZ8QjOywejXyxIGIx7e24c40vOH2HB6133GtZN4nxE
L85gwd/UB5+/8XVRf0m3x1mgzM/ofTiFclK/8lQ2HLFi/josiFzrlM2CCB53
Qmo6ZVVF0wHyfczhTauegfZTKqQ//Y4Fs0NnUzaJ1JzNhqUlT+fpilGOTP7b
xALTxS9kxyUoF7+cmseCy95lq3KlKFvPOPmdBTk1r9a5zKcsq66+gA0dSm83
y8tQbuNeKWCBZPD77a2L0b93zSMW6H3+YBy7lLL2LeNcFpzd3Gy+dwXmtzxk
NwtSb7YdFVmJvPtpAAs+/OxweLmKMt82qw8sEDbscbugRJl7Y+IdCzQe/vDZ
qIJ6fFtC5sVxciCgby2ud9r5lwVxFsPX0zZgPSYiYyzye2/sprU61qNzr40F
4zP/Jc7XxHoSHQXI/WM/hVGzBdm0oZkFh54LZV3Twv0jfmksCFs4s3C7LuZX
2fKeBUWeoi//bkc9o5NXsqHvreTrR/pov1vtx4IlivPrThtSFv3mHMMCk8BF
nxSMKVc7vSf5+X9a2vV5D/pnCQ2xIEtDvj/OFNdvlWaxoD1acXTffsz379tz
LBD/oSwwywLXqz8h67fpr59RZomc/46cj2fuq0tePIx6669rYcHD8c2LNKwx
n+EXbBbU7deWH7DB/jQV/ccCQe52lQy7/+vF18oCNZGdGrYOWL/vEjJf9seN
dWSccH3lsYssiC3aa1jnguvLp6WyoFzafF+4K9Z/dA/hUXfLQ/oeGG+0eyEb
FKuO2PGdxf2WDpEssFxpe6rAG/OrrX3GgmuX7L3cz+P83FDOYcGTJif/1X5o
P1KwmLxnN7qGdvijXjEtxN+iyDPRdwNwfUdBOQvMLw24KQRRdnUIe8qCcPdT
e3NCMP5qPZJPme03VbiG89YuymPBpJmDaEUY6tviQPqhtuPrz32ROD9PXMj3
dUrd5u2naIxXeJKct6kKrWzHm2g3fPOCBZ/mHwofuo3xB748JufFjI8uF+Nw
fed5cr7snthvLHIX9VnOJN9D0I8apZv3cP/MdHLeP/u0Z6ZsMubz5CxZP/L2
9beMh5iPyJ9aFqg+31m5MQ3Xfw0m36dDdllGcTrG6xoxY0HSg21XjZjo3/OW
GgsaYood69mo/xoj0j/RoK07j2XhPPj9cGGBgVehwvcc7GeRtDMLLjmoC3s9
Qn+pnDIWFB7M7eIvQH81wuS8GDRc+9/1x9gv6dK1LFDcwk6dV4R80peczzZr
VgclF+P+cvkQ8n0tZtiteUnZv7eVzGvNHDm9/FLU/4amKTn/+JNXbCvH+NLp
GmReBxdPffMK/T2RkmXDhS/xXyyqMH97mScsyK2VfvnlLfbzbFAvE76X3kw+
VYPzUHqB3Icr8sQvj9bi9++d+IV8n4yIY4EfcD2jgcxDzJ2ZOnMa0b9g2yty
fl4NlY1rxvxyW2+xYNoFQT65Vtxv50zs4BLQyvmM/Quov07OoyN8zzQ7cH9r
wU0WsPf4JpZ2IqccMmRBp/aYr0kP9qdrEYMFi9d5HW76hvFDqsh5aL58aMuJ
PrS7ntIi8yjpJjPQj/WV6jqy4L9pfePnf6E+2VN7mMD352ST4DB+3w53yHxp
dHcVRo2gXmaXSH6uH4/HyYxj/Dca68h98+rzubS/uN+87CUL2h4fObiOr5vO
z44ucj5Ks5o0ngpQdh1eS+bBJNFC2mAa5aSaDRUsCI2o+1MjRLk/Kol8zy/8
TT8cFsH1JfNXsWDM7e2j7pmUTSYmm5mwznbXLY85lLkPP55gwUmzCs9JMcqq
ag42LEjW27E/VBL3J+eT+6FR7eUGyXm4P7eP5C+uoC15bz5lPrON91hgNP/p
r1UyuN7HLoUFgSKa73MXU5bdbTjMhCfjj7K1llIu3jqN8ND39dGvllOuDoog
7xGlT1y3/fLIJ7XIfWL3syP8vQLGs2sj/Urkm8/cuxr1aHjnRO4PMeOKt2sw
3oVj5LwWXX6p01iVsn/lXaL3zg28Ka/X4Xrrg1HkftPrkTXciPXqMKax4LH5
IihXR94c68+CIfu9Vjs0cX9OTjQL1py74l2yBfcXfK9mwYmrBTd1tZDvOpH5
vxf/I7tY5//6f+eQ75W5tBq2Y/5i//azQaxo/48nOzC/HcnkvjR8GyqyeSdl
bWVN8j0EtD1dWWCE+3cOzyHn48DAdvXdyMm7opnwW0DehmeC+wuefiXvAUnL
i+v3oX4BAW1MsJcLT8jaj/2aIkX6naT2okDFAuNLCrmy4KP+cD3LknIbs+w8
6ddBxaHVh9EeHEzuY6OTR8QyjuK8uPYmkn6dj1ZWsEH/5189YcLT62VGqccx
30u/SD+H7445rLDH/JwZXUxQ4SgHJTti/4MK4pjgUGzzQNYZ7Zyz5P6//+5W
ceIpypHXDdzI/LS/apFxQ/8P4sm8SQxNjsV54P6tdoR3TVsvPf8s6v986iEW
XJGy33jbG/Obv4icV0Ur403nnkf9p3TWM+GPxtvTN3zR35ndwUxQNZwSJub/
//4a/2SCo5V6RsRl3H+9luib7Oz036wrqGfEY2Jv8r3XcS0Y9cgzPEDeMxHv
+UWuYv5qsZdZYJwktCTkOuaz9bMgC4KyNm8RjEB7ubo7C569OH0wMAr9TbN4
y4SR9w/OCsRgPS2biH5rv3644X8L47vv2cOGk8MzsiZjMb8pl4g+D4S031yI
R32fZtiyoFn6zLexu7j/099bbJiryBA+l0TZmuuxg9w/m5vl/iRjv51cFrIg
eJfoNs8UjB+wewt5/x3ebv0rDfXh+6pI7utT3r5uGbj/zDjJd50/M+4nE/ux
2vUKC5yi2vJcOLj+bOYs8p5Ilqz7loV6+g6R92pLjsGgYy5+f8KvSb+lSi/M
6X6E+yO+kXr31HOVThQgv9TuYEJIV8fOjsdYj8AbExY8H5G2tylCu3iwODl/
phsHthVjfS8+TGHDhoWX7h95ifEU7ch71EWJV9Rciv348vUCG+JOL+qOLMf8
XfQlyX2ffUVMrxL3L58g5/ng7x+ao1Xov/HLanJebzI/zqrGfGUPSLHB8EJR
2LH3uH/Ta/K+8Homnze3HvVz2Efm/6FARFtFA/obcST3V7Xen+l+TdhftwLy
np8IObp+3Se0T50SyAKF1/8d6mxDvZN6ST/M5qgGxX3BfvLxyHl6yTSWs7sT
99cPkN8L7Jt8HwV6UI/oh+1MaGxwEMj7hvO0fzmJLyjzbrVTH/rT+OJL+nN0
0/4lA6iH1Sh5Xx5Jvu/3/hd+v+5Xgllw9et0RvAwxpv2nrxXHym4v9s8iufr
gwIyr1+cGsd+jqOdX4e8L0Q5uiseTqKeuxrJe3jLYIaxBX8PXa89k+TjsFHC
a+ZU5CULmUyI8T6fVCxIue1BAbl/ih9/qTgznbKq3CTR7/uk0S+Fmbg+8lgW
E6R1c2VaZlO2Lmoh7z29KzI7osQoizZuuMYG9/LA03qSlJNSVpLvJ3HGj9hR
Kcrafmk/ye/P3ftfsOZT5vPOs2LDcNTTb8dkKBcrzCH36bI6ublSSyi7rljg
y4Td0uHwainu/+QyyAQfq2F7vxVoj5vxmQlpiUei1q3EfHqFyHu/9nNZYecq
rGfj41E28MmpdMQpYX6BdbEsUHK4PWuPCtZ3/3s3Cywy/6lNWYfr1Q9Jk9+X
ffbWeRswXtaMaWzIWlsd6qSO9QRsb8qET2c0cpZooh6fb2QwQSQ/qfn9Fsom
fVqbyPtzXFgwRAvzOzaQywQbcFPZoov1WY+S91r4pY8W/duRn587TO6jEp3L
D/UpRy6aIPdrt1BGpoUhxmNlkftQ0ki8bqYxxhPx1mCCdrjPZPEeyv2Z9auZ
4PyufaWnKa5vtisk73lJo72r9qP/4XTy3i49kOPTcgD1kTfdQ76fuIUPoyzR
Hq72jQmLPwVU6R1G+wuLOiYYLv0+PHoU9VmkNI+8n46bybJtcP21V7rkPE17
stPGDtmn34cFb3tXeEg5YL3KYeosmFgTlvDqJO5f/3WCfD9uv0v9XDD/1dN+
k+8n9/DPda6Yr/rNu0zw/1Mq3eVOmRs/Qe6L3Hep0i6eyJ86X2VCd2aw9C8v
1MfxnEwmyAQ5SJ/zQS455c8EE+ud0v8uoL8Zjj9I/zQVpa9cxH4+9yHfY77k
DOkZl7GfBpbFLPje921eVCDOw+bTTzJhScXrefOCsX8h0/zZYPqANe9uKNbn
dlSAnP++4fOWX6fsf+dgPHlfHzg9Lz0c4xW0XmNC31qTeSpRuP7yIXJ+L5u5
dh7vBtrT/faR92On2LzNt9D+T66aCVeLB6Wex6Je88YH2FAU915KPx79N7DC
2TB4Jleq6i7W53U7hgPye25K7UtCf0//OZDfW6vOSn1Mxv7bxg+S369TDkgd
TcH1UU6pTChuUZf6mobflxR3JXnf5ElLOWWgf60WMTYoRI/OHWCiHv2ie5hw
yLlxrhcH7UcqI1gQuePx3L9ZOA9dE3uZUCKbMDcgF/un++c+ue/GLsydnof5
TNtwkAlKdYfnRhTg+tFpf5hgzYG5c59gfi0SdeT9HrpkbnwR1r9vShj5fWnL
N3fpc6xffupRNoxv/SyZ9hL3Kyt6k/eO9AvJNWU4P6tdvcnvk8FkyZxy3M/V
Ir/nbr0OkNxUifOhw7Qg50nqcclnVWi/pEHeh5P+epJ61eivbtMoee9ayUtW
1uA8DC41Iu+5jUKSe+tQn9/teuT3zpxuiQ8fsP91CWmZ8KanXOJwI/oTGljP
AoGSdIkvzTgvrhdnkO878aqEYyvq0eBD7lNHbyeJn59Rz95FymxIMN0l4dmB
8TmyKuR+UVojMd6JevT+IO+XqUKzJS71YP78ryeYoPG5T1zoO8Y/tuMVG5wf
vxUP68N+ekclsyHpJldcYgD1UDT5xILa01Hid35hv3T/8DNB2NBdfMkw7l/u
XkXO+xX7xFNG0P4nKZENrpPrxVeP4/4loxVMeNggKZ71F7kkNSgTPmT/FlPn
66X1rj9Pzl+RsHqxpwKUI0mATAD7PLFt0yi7NrSxOeCuEytWIYS8x1qeBakL
z4ntEaHc5nvQirz3fh8Uq5tJudrgZB0bZldrilnNQbvyGHn/62YsFPssRjnp
5oNKNpwNnBC1l8T4LxzJe/1upNii5fMo8/VfIN9fSYL8qtb5aJ8ZlcaEb4zN
G+NlMD/3XnIfiPNMdA4soSx7axo5Pzc9tzOWWEbZX/TKThZYV/kcfLsC18uc
WsuBkI8RdtdWUuY2fp/OAs7Xh276ipRNNNMuZkL9QIHvlDW4v4RD3juTf9+E
PlPB+LWJjzNBTqTj5vl1aL9SU0Per1Kj99U3Yr37w8h702PZbPYvdaz3SiI5
b+OUlxdyNDE/CyVynz7X1Chz2or+fq4l7/nuHcY1K7Ux/jlNov+cfTafvuhS
7lc6M4sNake9eu/pUbau7iXv4cNO14etDCireou8yYRAr/sC0kaol0sW+T2V
GfBodq0xZdGr9TXpUBNRuSDSBP3rzj9D3mPxbfK79mH/bshJcmAp4/c6YXPc
n/DQgQ0GuSJaJRaoz+HmzRxwLV5i5G+FLHMykw23X284sOUIsqbOGHmfN+y0
HbHGfi6xIufN144jp3NtMb+PXQIcmDngcd71BOqzSoPcH+v/hgQrOWL9G+a+
JefZ9MQb3U6oj3HEGyZsDdeSOvkS60++upgJxwtnWM8vw3wHLch793rnh/Ty
ctS3OLWE/vvfw19elZS1R/nHONAMrltXvsF6pd7ms2Cq05bg+mqMN+/dKXJe
3RZ+d+U96hPnDkwwe1m7YGM95jczMpQNF34mHe9owHyiHYzY8HChC/tGE8ZL
+XCPCa/1N43ofsL6GoNecGDIY5ruYNv/56XRlg0ySe+u3f+C+zVemnFg++u7
dSadmM/x4puZ4DziuISvB/f3eqzKhJgVao6cbxj/xr2VbHhiIpBzpA/zs7gn
zYKOC28mZg2g3tvdzrBhZnrcjqe/0N+KvZ4ZsKHuRKTzMOqTdlc6Ew7xr29c
OEq5nD9fmguBa/4trxxH/7J58WxgHqx08ZlEvR7Ikd8TtVdu563i/0bzt5U3
J+dxli3/xymUvcWFU7iw7JOKUYggZddh4f3k96zIRIz6dMptt7rJ/e+uVv6p
cwZlk9t65P6Ks4lRuDWbcr/efUEuvAi3dtcTQ/9v3sxgQ2+h0pMhCbQP++iy
QbxrZNpDKcrcS+HfWaApUbpn33zKqhob88n7SSvqjoAM5SS1yeFMuOp0+EvW
Yow3K6GEA9m3V605tpSy8PXVK7jQ+PL3WdEVlGVL6P8/L9D/vPiZPOVqqwXp
maAoEy5yehX6j9tIzi9TA0uzxUqUrecYRHLg3Bn5xCplynx6H8l7OilpsOvC
Wly/93NGKpS/LlqrtAH9P1ndwoD+kavnm9QoW/SDNRek5Q6UXt2E618eW8wB
7b3L52huwfUrI4j+Dr4/LXoA6+2L/8KEyPTHybE6lCNTq45zIL8u+Lv+dsra
a0PXp0Mbv5nanx24/5uPJguElWX9U3diPavXnmaDquX3iv27MN8jvwvIezYo
X2LaHuyP46Fa8r7KDjycuxf9Rc27wgHGJ5M0WzPUz/b1Mg5UiywaED+A+R4p
1UqHEbUezRcHv+F5t1GLDbK2vEC3Q7j+67k2LhhEXHojexT96TeT/rk+Npau
Pob5GZm4syG2a77NxeOop3KCSCYUS3RmKtvj/OTYSZHzTiv7d4sj5mfRTt4r
os5+WmHO6E+rXZQL6rGGoVtOYz4zzrVkwAmriPSnbjg/x8yOpsOtxbUVcAbt
seUGHCj9LN377Czmyzr7XyYMPTwsonMOebbiSAascEhWfHEe412+TL6vfau7
DLf5od5nE8n7/nLfaqcSf5yvpSuGsyA7y/WaXgD25/jUUi60n+Flll3BeJtn
8jJBTGOsUj8E/V37IUve4+Pwvfwq5q9ZQr5P16KAmYZhWP/jyF4mJF0qV6qM
wH598Cbn39vts4x3RaO/f8sXMmBSyNSlKobyyNafhlmgXHkrbPdtrHehRHk6
HAlvYr29g/NlpqTHhbC9sm9MElDP9OPk+3siadf3LpGyqIRuVxZ8/5A+e999
zO/3hc3076H6lGsfYH3rtS5wwOjI+j37U3H/MlkxFvgs9T5dz8B4/K0dXMjo
eBJxIBPrCVeekgGNafzcBhbyD/fj2TDdaUf1QS5lDcex3VzQUL7W35iN37M0
vy4XHAbeih7i4bwIHwjiQGyu5NqWPMxndOfGDPjP6+DeI4VYL2vGWi4Maya6
tT7B/DjTV5P37mR7lPUzPH8GXNWywfz5yuzPz3G+r3FNM+FKoHONTQnqm9JE
fj/m6mcNfinD/DvvP+NCh8iwuF0FzuPhZcxMkHyjub6zEutNVnzOhm1RF/fZ
v0G9PNzkyO9VsxKP7mrs9zOHFQxInjc9xvE95fJ7DQZcqGk0zu2tw3gJJ54z
gD8xutapAf2JuZP3huqxD0PfG7He+Q1OWWC9QmbuqRbM96btdw5Edllv/NmK
+k0bIXo/y0jZ79qO85le4JgGfS69ngMdaK+jf2+/eK3KLfcuzIfv3nUu7B7y
ePSrB/U90TTGBN+8/Poz37Fex4dsFjB9/g7/7sN6rKqekvtvq+48rwGMf0rU
gAUz+YPVR379f/7WHWPD5pLKA+eGcb3723VMOBks6j02gvnfHSrnQJzh/tjz
45QN6joCs+HVrLj8ib//18NYkQuj1Z8afPm+E85fvM0uCxRilo9OClBuq9fe
mQMWBxzm+0+jzBdgQ94XwQtYm/iFKftr/ZvHgEctAwcvi1C2nu6ygwWdSWo+
U2ZRLnZdHJcJc4+fjwucQzlSutKVDRoHh8o2i1NueBf/Ihssd7v8GpSkHFuf
f5ELvts6l2TMo8z15D/KgSSNo7uOLaDcv+GNTAa8WNPgLb2IsujE0z42fF22
N+XtEspJF9+OkvNU+tW7oGWUXY3XimSA4qxtk1vlKCskfDnFBWOBJ4q/V6J/
723k94jrnw0HmIqUtXuETNgQ/Z0VYLsG8zVhkvcr77M8d4Eq1vd+exITGurv
Nb9bR1m4tn0GF8YqpaeHbqSsKtjRngmLnkdt1NbAfFjrgQvaj0Rs/mhi/rcT
/zLBNjMgnL0V9VwEU7IgKGmi0E4b16+dKp8JjJueXTLbMP9VByMyoPJqn0St
Hua3JHAjF/ou2mtfM6A84pYglguinm3Oukbob1kO0Xv9yYN3Ro2xP2PJflww
P1pTyjVBfYN2SmXBOTOjQft92G+zV2QeE3aWLF5ijvWE1/RmQRFsNaq3wHhS
jWT+P69/5BVmRbm6cnoL+b2zSuXh9iOUQ9KM2VyQX8yoHrfGfFcs0mXCToml
f7NtKXtX/jvNBWfhuFUnT1A20PAc5kLEX3HzpY6or7GGOReyB69dbnBCfRmd
pN+1XVM5EacoW6itGs2GP82+TTvcKGvsSjDkwoKaYaFJj//roc7lwJb/Tm/g
nUX9hfc9y4SjT7qtnc/h/GpMzGTC5axjYcsvoD53lAcyICW1saDRD+fToz+T
C+Xx+zqjLqH9/YB+NvRGvhbfGYj+lst4Z8OsID0tvmBcP+MwNw1Uzxc55YWi
HlvNWFlg6qoee+o6zuNqkddZ4GnHLZGLwH52NHuQ+9Ny1UBzFPbjT3R7Njze
k7woJgbrmZ/nmAWfti80NLqN+w+Nc5nApxlzViCOMmPavLNcWK4y60FBAurT
s52fATtWBL11vYf5MWyY6eAw/9/4ymTcn8vHzYZrs70VWh9ifwRVb2YDe8qA
2a007McaWJ4F70YcLxlnYH5y5l/YMPSjnTWVhf6Lteu4IPXFqvExB/NrGNrM
hU0NtYIe2ZRl78nc5cChKuP1ijycvxW6Vdng96Ls6Oc83D/TRiYL7udpXY8t
xHlfuWR2LpQw8/P3PMX8pkc4Z0CfRsbjhmeY35kX9bkgXRpfdOwF6v94m3E2
6O4Ne95bQtnENPp0Eri0+JV4/IfzIln9lwuxjq7/TVSgnhkq5D3z4vexV1de
o15qA4qP4PulfVWz32L8aK7zA5CarVd9+x3uH96wJRO049Tey9biPKoY7soG
J3mF+vR6tBuV8WfArez5H9d9RL3qZ5HvoxhmND9uwvx50fNToPfVxKftn3D+
8kXJ71XJA32fq9owXmxBCgPgS2uH+Rf8vgJvknlwPP2uq/Urnnf5b+ZlQcz4
i16Hbjx/XvtMcKAoOPfHQC/6G2AqZUK3RGq/zw/MJzP8M/k9nHT715R+jD+Q
vZ4JW5RCh68P4v4B5UY22Of7jM79jf3KvCHDhejtzhOJfyg77K/VzIEn1Yf/
rRzD8y/m9x4udB7aI5A1Qbl70wwxLoj2aE/T/IfzdG8/qVfTc53wS/4fNJ97
ddIMsONfMWPXVMrcc0/vMyAybO7sOkHKqjunPsiAwvlCYkemU+bzT67MhY6U
EYmuGZTbcgPKH8Dsdb1SrrMpJ+1oIP3VKGqaPypKuX/OPR8u2BhWyVyWoCxr
+a2ZC9fri5bMkKJsve2wbxbk2XCXxUhT9j78uzAL2vvuyy1aSNlf0fZTDsw8
f0MhdRHlkBqdMC6oCV1ZrSJL2STY3ikbrG+cVc5fhvE8DkVnw9UlDmt15DDf
lDHRTMjNPLjh1UrKFkFMoscndSP1fYo/8DwTL+PA9JItms1KaN878/0j2GCi
vNVOBf2xnplkwZHmJdp9a1Efnp8lB0IcxLZ5bcD8xfsfxEL2kMAOPnXKxWlX
3CKh2X/IIHQT6iPbdi8LBGd1GolvQfuki2oWqN75sDseUA9fDfL9W8lV7F2h
g/GazV2zISir0Iy1Desv/OWTBdytzANqO7BeXSXrZGisuGv5zADtT1zOZ8JU
84jDBkaY39bKCzxQbve3fmeM/p5lVWTDwVPutpYmlEVXNkmS35djtie+mOL6
j/43c4AdtN/ReT/m+zsjjNx/4vrOvw9gvhffz0sFgXsap/0sMV77hoD7oLRa
0V3oMOXY1m2jeXAgb6Fn5FHKI1/NVuTAZdsS3kwbnK+CFIkCYM9xGQ45juvn
lodmwcfHc9Wn2WM8+2ehSTDVocjrkiPqecvjWjaoSNrn/3WiLHzx7BsuWBbP
GT13Cufx9FhbFlxxzt807Ir6ySlVpAFX+piPuwfmV3dZOxWaSqY/7vNELsm9
kwaCbtnjJ72x39zWxBxYu8hqS5cP5fylveT3y6GKKb62vljvlJOyiRDsyXza
ehHz61qqfA+yl+6ftLqM+6/f6qB///wXGgLR/52W2Xkg7JN60SwY83urwnsI
6+X3FFeHor+K0nHye6DmD5/xddTnzRdy/4T6JelUhKP/6+7X0iBXcedlvSic
79DXhTnQWj/w4vkNytXBjBAWiATETYFblBVqnP89BjWVbdsLY7F/FRU62XCs
6VugWjzlBnGbeY/genBMafZd7P++9eR7yV+/VVAlCefny7WKh+T4+rojM5ly
5NU22TSYfT08eGUK5jO9rDAVNmmolz9IQ//P9vilwfGOVmHZDMyHtyw7FyIi
Q3YmMNG+b/QTAwq3rL0qzcH8B1U9ufC1++OrmCzUZ2rD+3QQvXl5hlgu6qPf
J5AEm3VW7wp7hP3bv2MtC078eH99egHOy+VVh3Mg6s6FqiuP/z/f0eZn4Yme
3GyBIlzvpprBgq6Bqt1+xZTLj3dOywHxxLMRYy9Q7wSj/5VY9rFQx3Ecp3Jh
hDnycKFRVioTI6YPqZiHGq7lIez+0DpKbt1UOpnV0lVbESMP4Y6T3Y0jx+8e
lsUcW3PSeZg8ZeOGPCVPhVW+n77/vfb9fD8P7+/3+/l+E6VwNsyx764a82ko
2P0fsTe6zVe7CbO9Q3ZUUCDkRKV/wv18xe1pgLbLtq/ne/73ozh1C8xttWtv
fMZ6x7OihUB/l2o5/QX9f6MymyCQaXmFNYD1CA14Urj5V1U4NoT6OmhGKCiS
JA/GfsX79n5+WwIdMabWg6OE6yQZIIPFva1XoyawXrcN7wawaUwq1kyivbLa
TgznE/YPh05hfqLHpk1w27DRpkuH68OD5lVQIouNC5olfObhbNTu+8vSL237
jnpVWwkoWDYRj/gton97jlQIdopoe2oZzwOPHd4MF69vX/P8if1RI3VWAsei
ply6hvrc4fOaoOxDxLjbJuotFdfnQVfK+qG632g/MZQphRWriiSXHez3rpr2
emB0BFdW/cHzdNTAVAZ+Vc4L0fpLJN64Vy4Fcdl6vgb7CH/0WDoih/sJ408o
GmG9eG5JHRT5KbUpRoRjT09RCpDZFDsyTJBpFXPNoN3g3uo9QNh8djlIAD8G
IhU5FuiP0k+oBrPmkzRPOuEce1qkGE7lGzN11oRZvfxsOUSkz1QW22K8B4lW
zyH1UudCKAPty1QHa4DvJvDdccD5kFxJKtQaZec2HCY8KWJrK0E9E9/PciHc
pxjNq4dptY+TpSvhKrtoCwHsqaGnqY8R5qR154jA6dGK4t4JwnIzna4FAli9
tOPumG/6ZGc5JIGEOeZBmB+syJJDFoNf9dIL40e8YFdA6VbyYqDPEu5fPk8J
8uFzfqu+hH9JGt0pGGp1eCryJ+xEvdkUwHrhdn9MAObr6P/sLdC5w07GQahX
XwtTAGG1axmGF9A/jn+Z9O2k
       "]], LineBox[CompressedData["
1:eJw91AlMU2ccAPBaNGlAN5WSVVvJBESh0HYpw4axP4WUOBgEA3hkgDoRottQ
5iaZuPWgpaBB5zWQhKNiscghb4VKpQXKBq7ECFULLaAZdCFSwiitiIGSbv2+
GF/y8vLLd/yv5O08fiY9j0wikQTeF31X6CNv1moX4kjvnpinvne+USBzjgUs
9sDh9lcOxh1kxdrPz2qg6PJA7EgjMj/wBacdbn57+6KkCflkQh6hho4k4Ri3
BZ8/U1fWCdbe5ytdbdgpacJ+8HDDdsQSyLTL64wPIOSekG9QIy/yXYsKSA40
5wo0yLNpgigCCm+ElRm7kKdK/S8QUEkRNad0I39hE5zvBv0v5icmPbLBEu5u
A5srzJnZh/xT/r9vdEA5KaKO9yNv3tCQrQTWS/PenAFc72eDh7ogMz08a/oR
skm9cLQViv8SCfOGkI132d1aUMSO3rY/xvsPyZfV8Oj38MGCYewfcqlamA8V
zzpNOL+lRD8tbK0Z9St6js/HnYvqBN4WJnt1FFn8wf5LpXBELk4XWvH+EVd0
H8jco+fIkzj//ESqHJoLmdXyl7i/qiFuOZhmxHrfKeTDR4xv1bD81djfV2z4
Ppfd/hswTEwf/xnsE/ZTzRCfKAmteoXr0US/fgD53WNJ9Dkcby/Dm38FO6Kg
fh7Ho+pkdaBWSq4GO3C/1mbnvfPaZulQOZH3d21vU4HnSoSFuYTz+X59NQEh
60tW25fx+vH6IAKSz1t2RK0g3yI3ujVQuBARr3Xj+EO1Oa1QmVtyItaD46Xa
g1pAb7WUGUgOtJ598aEWbKmRLQIfZHHWJnorUP4sGTZuQCZFshMvAItndaZQ
kJusNsdDyGyLDHjqi1w4JllWQXGQlHdgE/LHu2mVLVBfZc0a/xCZkhB1ox8G
NrJEOVvxfdfX9tyCOYm0YZqKrHhCp9XC5rfWwbyPkGl/0CZ6Ifo7lt2+Dbm8
jGAQkD0t3Xiagf2PSNoHJQfH2a5A5GPayYwOaHrMyijaicxJy3jdC8N8WdFq
MLah0dkKS5rxamEoMiGaOdsM25nsHnIYzr947n478BWyKTkTmV/eWKGE/IAJ
Hz8W8rwoVTIIFZfYu3/lIBsaYjzeef0nS/bn4nrM13ipYP1xoqDqU9y/Cn+6
Bjx29jU6D/fj1DNlE4QcLe2sj8H1Mm9m6SDZPGEJ/hzXKzV+7Z1XEsetisPx
levU5VDZWxoYkYDru0fepwM9dzKeECAbe7ZwdXD2y/5dn+xzvP9f/A/C5eD8

       "]], LineBox[CompressedData["
1:eJxTTMoPSmViYGBQAmIQ3Rac3XnY9Z09AxQE6E/alecO4h+wb78+2S6PN59d
0QvEn/B2XcBqu57X3iGXfUB8CaY7a7barT6psbDVH8R/UHHtyUq7U8tZ35kH
gfX3yPgvsHvR+sjqVQiILzAh22aBHVvK/vY54WD1Hg66a+1UneZc8YsCm/eS
WWmrnYtCpSJjLIhv8e7G1+12Sf9C8zbHg/gNRcXC0+wa7hjtTk0C8SPeV/Bs
tJu3i59DIhXsPt2L2xfY7ZnxJuRUOtg/JZIme+1ul51cWJMFVh9sxLjV7lfI
snd6uSB+gdGpwDV2EsbN1g/zweYb3jXfZmcmmNAxuQjEVzg9TWqbXch7m6uu
pWDz+lco59gVnZVU+lEO4gdwFJ5fbDdx9be8VVVg8+PPBB+w29B5eXdMLYj/
o1x+4k67c+kbOPgbwOpjNI+ssHvj2ht6sAnEXxAsdHmNHZdK1qLiVjC/+W7Q
BjsNJvf3qh1g92m5Jm21c3+gbHOjCxyeM5gfb7dL28fQ2dULlo+qObndrmXO
3as2E8D+36Z/co3doqpdSu8ngd3v/PnaDrsDEdPzF04Fu/+95+aVdvfMSvYE
zwDxHbpShWbY/RUJ5GSbDTavjdt1kR1f/LbPDHMR6QEADtXhsQ==
       "]], 
      LineBox[{{0.9876620020593082, 0.}, {0.9879995156544557, 
       2.2531469131559234`*^-6}, {0.9883423860532496, 
       1.1690838587208319`*^-6}, {0.9886852564520436, 
       2.7430440959763658`*^-6}, {0.9890281268508376, 
       9.607139842549017*^-7}, {0.9893709972496316, 1.657874854732455*^-6}, {
       0.9897138676484256, 2.8802176631481657`*^-6}, {0.9899950935458742, 
       0.}}], LineBox[{{0.9825822539408582, 0.}, {0.982856459672546, 
       7.284654807149238*^-7}, {0.98319933007134, 1.0925501402470061`*^-6}, {
       0.983542200470134, 2.6057245448019017`*^-6}, {0.983885070868928, 
       1.0623830366540687`*^-6}, {0.984227941267722, 
       2.6860741618728312`*^-6}, {0.9845708116665159, 
       1.274206830825797*^-6}, {0.9849136820653099, 
       1.2611988620125913`*^-7}, {0.9852565524641039, 
       2.0755708665110006`*^-6}, {0.9855994228628979, 
       1.3263594188517303`*^-6}, {0.9859422932616919, 
       2.3384234606460552`*^-6}, {0.9862851636604858, 
       3.4777692333731736`*^-6}, {0.9866260252345572, 0.}}], 
      LineBox[{{0.9931451041507771, 0.}, {0.9934854420351593, 
       3.691610458211869*^-6}, {0.9938283124339533, 1.5231216133893*^-6}, {
       0.9941711828327473, 1.7470679820608126`*^-6}, {0.9945140532315413, 
       9.529779527728266*^-7}, {0.9948569236303353, 
       2.0073037044765485`*^-6}, {0.9951997940291293, 3.13554735520416*^-6}, {
       0.9954424315134393, 0.}}], 
      LineBox[{{0.9780913211500554, 0.}, {0.9783991444882243, 
       5.738276029898515*^-7}, {0.9787420148870183, 9.532398503875328*^-8}, {
       0.9790848852858123, 7.508273636158691*^-7}, {0.9794277556846063, 
       1.4011886806386542`*^-6}, {0.9797706260834003, 
       1.3593110091969507`*^-6}, {0.9801134964821943, 
       2.200168056076812*^-6}, {0.9804563668809883, 4.740600277886031*^-7}, {
       0.9807992372797822, 3.3183492098576295`*^-7}, {0.9810073763962894, 
       0.}}], LineBox[{{0.9956674151941871, 0.}, {0.9958855348267172, 
       2.264734852985839*^-6}, {0.996228405225511, 1.8211339857243658`*^-6}, {
       0.996571275624305, 1.0044208359483164`*^-6}, {0.996914146023099, 
       2.6817193665706895`*^-7}, {0.997257016421893, 
       4.0098911202601784`*^-7}, {0.997599886820687, 
       2.5369447297363124`*^-6}, {0.997942757219481, 
       1.1885858562932228`*^-6}, {0.998285627618275, 
       4.4035049470148024`*^-6}, {0.998628498017069, 3.713740301947155*^-7}, {
       0.998971368415863, 1.4473943514836662`*^-6}, {0.9992654208322195, 
       0.}}], LineBox[{{0.9902767422075148, 0.}, {0.9903996084460136, 
       3.525867690035156*^-7}, {0.9907424788448076, 
       1.0958960676710205`*^-6}, {0.9910853492436016, 
       2.6347041195418086`*^-6}, {0.9912713789604369, 0.}}], 
      LineBox[{{0.9815160247269071, 0.}, {0.9818278484761642, 
       7.663572745286729*^-7}, {0.9821707188749581, 1.152300188045352*^-6}, {
       0.982466728824911, 0.}}], 
      LineBox[{{0.9918654004404444, 0.}, {0.9921139604399833, 
       1.1972425928430397`*^-7}, {0.9924568308387773, 
       6.756205805924509*^-8}, {0.9927997012375713, 
       1.2188320118733387`*^-6}, {0.9931350143788641, 0.}}], 
      LineBox[{{0.9866308402698115, 0.}, {0.9869709044580737, 
       2.483735870861814*^-6}, {0.9873137748568677, 
       1.8074270838885909`*^-6}, {0.9876499930691759, 0.}}], 
      LineBox[{{0.9774469422809252, 0.}, {0.9777491251451815, 
       4.999213397693936*^-7}, {0.9780207734037453, 0.}}], 
      LineBox[{{0.999356844106977, 0.}, {0.999657109213451, 
       1.6934924488287706`*^-6}, {0.999903766552767, 0.}}]},
     Annotation[#, "Charting`Private`Tag$40900#3"]& ]}, {}, {}},
  AspectRatio->NCache[GoldenRatio^(-1), 0.6180339887498948],
  Axes->{True, True},
  AxesLabel->{None, None},
  AxesOrigin->{0, 0},
  BaseStyle->{FontFamily -> "Arial"},
  DisplayFunction->Identity,
  Frame->{{False, False}, {False, False}},
  FrameLabel->{{None, None}, {None, None}},
  FrameTicks->{{Automatic, Automatic}, {Automatic, Automatic}},
  GridLines->{None, None},
  GridLinesStyle->Directive[
    GrayLevel[0.5, 0.4]],
  ImagePadding->All,
  ImageSize->{572., Automatic},
  Method->{
   "DefaultBoundaryStyle" -> Automatic, "DefaultMeshStyle" -> 
    AbsolutePointSize[6], "ScalingFunctions" -> None, 
    "CoordinatesToolOptions" -> {"DisplayFunction" -> ({
        (Part[{{Identity, Identity}, {Identity, Identity}}, 1, 2][#]& )[
         Part[#, 1]], 
        (Part[{{Identity, Identity}, {Identity, Identity}}, 2, 2][#]& )[
         Part[#, 2]]}& ), "CopiedValueFunction" -> ({
        (Part[{{Identity, Identity}, {Identity, Identity}}, 1, 2][#]& )[
         Part[#, 1]], 
        (Part[{{Identity, Identity}, {Identity, Identity}}, 2, 2][#]& )[
         Part[#, 2]]}& )}},
  PlotRange->{{0, 1}, {0, 0.00005}},
  PlotRangeClipping->True,
  PlotRangePadding->{{0, 0}, {0, 0}},
  Ticks->{Automatic, Automatic}]], "Output",
 CellChangeTimes->{{3.74116888300852*^9, 3.741168914991672*^9}, {
   3.7411689537308407`*^9, 3.741168994446384*^9}, {3.74116903409752*^9, 
   3.741169077928515*^9}, 3.741322066004903*^9, {3.741322096379217*^9, 
   3.7413221203500357`*^9}, 3.741336751643519*^9, 3.7414108822843*^9, 
   3.7414122277899323`*^9, 3.7414123134158*^9},
 ExpressionUUID -> "1f117462-8b7a-4067-8657-6ce0edf6bf35"]
}, Open  ]],

Cell[TextData[{
 "It appears that the error between the short-range exchange energy obtained \
through the sum of the separate Coulomb and Breit calculations and the \
short-range exchange energy obtained through the Coulomb-Breit calculation is \
of the order of ",
 Cell[BoxData[
  FormBox[
   SuperscriptBox["10", 
    RowBox[{"-", "6"}]], TraditionalForm]]],
 " for the order 6 of the Pad\[EAcute] approximants, and could go even lower \
with higher orders. \nThe two methods can thus be considered as equivalents \
for Pad\[EAcute] approximants of order 6 or higher."
}], "Text",
 CellChangeTimes->{{3.741408144599476*^9, 3.7414083738714046`*^9}, {
  3.741411465903193*^9, 3.74141149133498*^9}, {3.7414123534852867`*^9, 
  3.741412464474506*^9}}]
}, Closed]]
}, Closed]]
}, Closed]]
}, Open  ]]
}, Open  ]]
},
WindowSize->{1853, 1025},
WindowMargins->{{0, Automatic}, {0, Automatic}},
FrontEndVersion->"11.3 for Linux x86 (64-bit) (March 6, 2018)",
StyleDefinitions->FrontEnd`FileName[{"Report"}, "StandardReport.nb", 
  CharacterEncoding -> "UTF-8"]
]
(* End of Notebook Content *)

(* Internal cache information *)
(*CellTagsOutline
CellTagsIndex->{}
*)
(*CellTagsIndex
CellTagsIndex->{}
*)
(*NotebookFileOutline
Notebook[{
Cell[CellGroupData[{
Cell[580, 22, 542, 9, 165, "Chapter",ExpressionUUID->"3ecf45d0-c07a-46d3-9913-4e3a72c6e449"],
Cell[1125, 33, 669, 14, 166, "Subtitle",ExpressionUUID->"e546b7da-b0f3-4494-8292-4519e1a30d74"],
Cell[1797, 49, 140, 2, 34, "Text",ExpressionUUID->"93278e3d-662c-41eb-9dc8-fe7a8e9c8693"],
Cell[1940, 53, 4813, 97, 285, "Text",ExpressionUUID->"f8dabe74-5bba-4406-82a0-464dc32821f0"],
Cell[CellGroupData[{
Cell[6778, 154, 261, 6, 32, "Subsubtitle",ExpressionUUID->"cd72ad39-209c-4743-a995-1bc6c760601a"],
Cell[CellGroupData[{
Cell[7064, 164, 252, 3, 70, "Section",ExpressionUUID->"a087474c-de1e-4a3b-8d4f-b56f42fdf834"],
Cell[CellGroupData[{
Cell[7341, 171, 316, 7, 33, "Subsection",ExpressionUUID->"26ee7acf-8bbf-4663-9350-f5bca607df08"],
Cell[CellGroupData[{
Cell[7682, 182, 314, 5, 31, "Subsubsection",ExpressionUUID->"3e9422dd-805a-47fd-a931-e419d9c44785"],
Cell[7999, 189, 678, 13, 35, "Text",ExpressionUUID->"d176c33a-af29-4038-8e93-516ff70226b9"],
Cell[8680, 204, 2149, 65, 98, "Input",ExpressionUUID->"df7198f5-4e2f-40cf-bf9f-4110a1ceff4b"],
Cell[10832, 271, 750, 16, 43, "Input",ExpressionUUID->"35c1b665-6c2e-4de3-bf1b-bef9da58994a"],
Cell[11585, 289, 567, 12, 33, "Text",ExpressionUUID->"2dcda777-691d-45b3-a928-bf0b7f19c2e4"],
Cell[12155, 303, 3098, 79, 91, "Input",ExpressionUUID->"1fba1a58-bce7-4b8c-860b-3f978ae9dd71"],
Cell[15256, 384, 918, 18, 43, "Input",ExpressionUUID->"c6a62e0f-eebf-472a-9163-6ce9821d9f70"]
}, Closed]],
Cell[CellGroupData[{
Cell[16211, 407, 191, 3, 31, "Subsubsection",ExpressionUUID->"dee010af-f488-4229-a4f7-c479e36438b1"],
Cell[16405, 412, 711, 11, 55, "Text",ExpressionUUID->"dca759a2-df0c-4b37-85c3-b5a0c0ae26ce"],
Cell[17119, 425, 466, 11, 62, "Input",ExpressionUUID->"91ce8e91-fe0b-4551-88a9-910c0c86af63"],
Cell[17588, 438, 309, 6, 33, "Text",ExpressionUUID->"afe036be-78e9-4936-95bc-0d471b47e76a"],
Cell[17900, 446, 11290, 299, 606, "Input",ExpressionUUID->"76802003-b95a-4ef6-ae4c-f8d335f0dd0e"],
Cell[29193, 747, 416, 8, 33, "Text",ExpressionUUID->"110a2ca1-f0bd-44fb-94ab-79096e15ab6c"],
Cell[29612, 757, 3301, 92, 256, "Input",ExpressionUUID->"ddaff6b5-54ae-4661-b814-00479870b9fa"],
Cell[32916, 851, 362, 7, 33, "Text",ExpressionUUID->"6ad5867f-d940-4dd2-998b-98b1fba56cb9"],
Cell[33281, 860, 19023, 488, 1063, "Input",ExpressionUUID->"2cf9fc88-e0b7-4f81-857d-6fbf1e9a62fd"]
}, Closed]]
}, Closed]],
Cell[CellGroupData[{
Cell[52353, 1354, 317, 6, 33, "Subsection",ExpressionUUID->"36959359-5bc7-4f82-8185-dd8af1290eab"],
Cell[52673, 1362, 321, 6, 33, "Text",ExpressionUUID->"617ba2b1-6cea-4259-ba68-021a4b46b7fc"],
Cell[52997, 1370, 930, 23, 44, "Input",ExpressionUUID->"9b7bd603-bc7d-4ee9-ab7d-17fb0d1be265"],
Cell[53930, 1395, 679, 18, 43, "Input",ExpressionUUID->"3db6b254-60d6-44f1-b994-7d3ebf24672d"],
Cell[54612, 1415, 519, 12, 43, "Input",ExpressionUUID->"21ca6e04-74e2-40c4-8f88-ecbf4e6b77b7"],
Cell[55134, 1429, 1135, 23, 43, "Input",ExpressionUUID->"356db6d4-1b57-4f82-90b8-863e63ddd22b"],
Cell[56272, 1454, 1226, 30, 44, "Input",ExpressionUUID->"4a8f9992-ad40-4cb7-b2fb-9dba2e1c39b2"],
Cell[57501, 1486, 709, 17, 43, "Input",ExpressionUUID->"8d732e60-2df3-49dc-94a5-cb015af7befc"]
}, Closed]]
}, Closed]],
Cell[CellGroupData[{
Cell[58259, 1509, 411, 8, 56, "Section",ExpressionUUID->"42c72d06-0525-46d6-89f8-9b91f3b11cf2"],
Cell[CellGroupData[{
Cell[58695, 1521, 232, 3, 35, "Subsection",ExpressionUUID->"cb4602cb-e1a4-4a24-82d8-495045542c07"],
Cell[58930, 1526, 364, 7, 33, "Text",ExpressionUUID->"603847e3-4d99-4e39-958f-8ae47d19db79"],
Cell[59297, 1535, 1853, 54, 90, "Input",ExpressionUUID->"d066ff25-7a80-4cde-8a5e-38969bf2074d"],
Cell[61153, 1591, 365, 6, 33, "Text",ExpressionUUID->"db68f0dd-d20e-4001-8d31-a6dd9c8c115f"],
Cell[61521, 1599, 6022, 133, 305, "Input",ExpressionUUID->"21882abd-6baa-4090-8008-b4f041acf306"]
}, Closed]],
Cell[CellGroupData[{
Cell[67580, 1737, 290, 5, 35, "Subsection",ExpressionUUID->"4f889624-928f-4ed6-a4d6-4754ad1645ed"],
Cell[CellGroupData[{
Cell[67895, 1746, 286, 4, 33, "Subsubsection",ExpressionUUID->"e1261da4-e649-4ce6-b540-e1b98bee379c"],
Cell[68184, 1752, 424, 8, 33, "Text",ExpressionUUID->"4a008f6f-a0d7-4321-9d1a-8f9df2c0b482"],
Cell[68611, 1762, 1531, 42, 87, "Input",ExpressionUUID->"3f1efe4d-169c-44ad-b4d8-e42a042ee8b6"],
Cell[70145, 1806, 1570, 29, 43, "Input",ExpressionUUID->"8cbed45f-ba72-44c4-b33d-4989da0fe010"],
Cell[71718, 1837, 317, 6, 33, "Text",ExpressionUUID->"b5dbbf07-ec89-4f6f-b50b-b6a0e3c166e0"],
Cell[72038, 1845, 1724, 46, 87, "Input",ExpressionUUID->"443cd855-1bfb-42e1-baca-d9ae999447fc"],
Cell[73765, 1893, 1645, 30, 100, "Input",ExpressionUUID->"f40a0eac-68d9-4fb8-8ff9-182dbc3de4b1"]
}, Closed]],
Cell[CellGroupData[{
Cell[75447, 1928, 216, 3, 33, "Subsubsection",ExpressionUUID->"275360dd-05f5-49d2-ad65-189b5f73105e"],
Cell[75666, 1933, 325, 4, 33, "Text",ExpressionUUID->"1e6da0d2-b144-4f4d-ab85-61e6d308352b"],
Cell[75994, 1939, 9215, 216, 632, "Input",ExpressionUUID->"953b1638-837c-4da1-b80f-f00d2ceb103b"],
Cell[85212, 2157, 295, 7, 33, "Text",ExpressionUUID->"d1dde1df-ad9f-47f3-832c-0b09d333ce03"],
Cell[85510, 2166, 721, 12, 43, "Input",ExpressionUUID->"c454ac8d-aace-4895-865a-6c8a2ddd64a3"],
Cell[86234, 2180, 511, 11, 43, "Input",ExpressionUUID->"3fc885dc-11aa-4c05-bfde-85c94385b409"]
}, Closed]],
Cell[CellGroupData[{
Cell[86782, 2196, 277, 4, 33, "Subsubsection",ExpressionUUID->"4c21d97d-33d1-4287-8364-88baa46d5f2b"],
Cell[87062, 2202, 515, 8, 33, "Text",ExpressionUUID->"d354c4a0-6e81-4a17-ac0a-dbc8991f436d"],
Cell[87580, 2212, 911, 19, 43, "Input",ExpressionUUID->"b91accde-fdf6-47e6-beab-15c035d2c961"],
Cell[88494, 2233, 706, 16, 43, "Input",ExpressionUUID->"9dca9799-0895-4c4d-b973-13f543597d7d"],
Cell[89203, 2251, 874, 18, 43, "Input",ExpressionUUID->"32e6c12d-0a27-45a9-a125-8272de7a4718"],
Cell[90080, 2271, 597, 14, 43, "Input",ExpressionUUID->"1bcea4e1-1599-4772-aee3-1dc941eafb84"],
Cell[90680, 2287, 409, 8, 33, "Text",ExpressionUUID->"ed68fe91-d09a-4821-9424-1ee811e00ed4"],
Cell[91092, 2297, 957, 16, 43, "Input",ExpressionUUID->"7fd1fd44-421b-4e65-bd80-dac484fb4209"],
Cell[92052, 2315, 659, 12, 43, "Input",ExpressionUUID->"cff0cbfc-7ebb-4ddd-88cb-7ede16aecf59"],
Cell[92714, 2329, 928, 16, 43, "Input",ExpressionUUID->"794cf849-6137-431e-b8e3-c809219b4b5e"],
Cell[93645, 2347, 609, 11, 43, "Input",ExpressionUUID->"c324bd60-cb1d-4a75-b809-5b57dd077982"],
Cell[94257, 2360, 329, 7, 33, "Text",ExpressionUUID->"e21ab2f2-20fa-4f20-aaf5-fc936674f5b8"],
Cell[94589, 2369, 1424, 33, 66, "Input",ExpressionUUID->"d07f5ce1-ee2b-42ee-b7a7-a40c5115139c"],
Cell[96016, 2404, 1470, 34, 66, "Input",ExpressionUUID->"ef86f349-f196-4119-8fad-d8ce565b3384"]
}, Closed]]
}, Closed]],
Cell[CellGroupData[{
Cell[97535, 2444, 154, 2, 35, "Subsection",ExpressionUUID->"623a936f-92cc-4236-91b4-25f2f70700c3"],
Cell[CellGroupData[{
Cell[97714, 2450, 269, 3, 33, "Subsubsection",ExpressionUUID->"8d35845f-7f80-46e8-808b-7f7f87394988"],
Cell[CellGroupData[{
Cell[98008, 2457, 203, 4, 42, "Input",ExpressionUUID->"9df73f38-04ca-4221-8f34-4aaa88b382c8"],
Cell[98214, 2463, 592, 15, 67, "Output",ExpressionUUID->"91a4722e-059a-4232-ba24-de99b20b23f0"]
}, Open  ]],
Cell[CellGroupData[{
Cell[98843, 2483, 203, 4, 42, "Input",ExpressionUUID->"8bf298f8-d170-49ad-badc-15fc77cf9e9e"],
Cell[99049, 2489, 769, 20, 73, "Output",ExpressionUUID->"82c14e9d-eabf-4ed8-a218-c5ee6663846f"]
}, Open  ]],
Cell[CellGroupData[{
Cell[99855, 2514, 203, 4, 42, "Input",ExpressionUUID->"784a75bc-a185-4077-83a2-a9566d665d32"],
Cell[100061, 2520, 982, 25, 72, "Output",ExpressionUUID->"8f4b8c47-ea55-45ca-94d9-0e8f09855cb5"]
}, Open  ]],
Cell[101058, 2548, 282, 6, 100, "Input",ExpressionUUID->"0a9a272b-6831-424e-a9d5-8d39d5f035f9"],
Cell[CellGroupData[{
Cell[101365, 2558, 1786, 45, 66, "Input",ExpressionUUID->"1e0f8b01-8f5d-4c64-8ccd-e72accbb6607"],
Cell[103154, 2605, 12179, 226, 385, "Output",ExpressionUUID->"4db752a4-6df7-45f4-9366-382d65ad481a"]
}, Open  ]]
}, Closed]],
Cell[CellGroupData[{
Cell[115382, 2837, 251, 4, 33, "Subsubsection",ExpressionUUID->"0714bd96-a8d1-4935-bf60-0f69d80f8aa2"],
Cell[115636, 2843, 1898, 28, 43, "Input",ExpressionUUID->"43bf6f61-41de-459e-8eb5-ff8543bbf4b3"],
Cell[117537, 2873, 405, 7, 43, "Input",ExpressionUUID->"78adce96-9a1f-4085-b199-5a983cf7bac5"],
Cell[117945, 2882, 452, 8, 43, "Input",ExpressionUUID->"58daf481-4ffb-4628-a597-f38b91d04fa2"],
Cell[CellGroupData[{
Cell[118422, 2894, 2236, 58, 89, "Input",ExpressionUUID->"2ff6e801-2cb4-4b50-aab1-644ae15ab337"],
Cell[120661, 2954, 11929, 221, 370, "Output",ExpressionUUID->"1ab79a62-964a-48f1-a91f-f03ec358c133"]
}, Open  ]],
Cell[CellGroupData[{
Cell[132627, 3180, 1825, 50, 66, "Input",ExpressionUUID->"a7f00134-604b-4d85-bf61-161078ba0a08"],
Cell[134455, 3232, 14427, 260, 990, "Output",ExpressionUUID->"b5aec1ef-70ab-4002-aac4-84c7e1969752"]
}, Open  ]]
}, Closed]]
}, Closed]]
}, Closed]],
Cell[CellGroupData[{
Cell[148955, 3500, 355, 4, 56, "Section",ExpressionUUID->"4df3c283-bc3d-4c0d-9f21-a98fda0e7e36"],
Cell[CellGroupData[{
Cell[149335, 3508, 228, 3, 33, "Subsection",ExpressionUUID->"9d993871-b738-4064-a4e6-be0fadc27ea9"],
Cell[149566, 3513, 410, 7, 33, "Text",ExpressionUUID->"28f5aba9-cac1-4cc0-b399-2905a0a609af"],
Cell[149979, 3522, 2545, 65, 210, "Input",ExpressionUUID->"2b7bd7ad-d9c1-42ac-9c84-d680688716e0"],
Cell[152527, 3589, 387, 6, 33, "Text",ExpressionUUID->"8b10241d-ae19-473a-95fc-bec0cf9f463a"],
Cell[152917, 3597, 5514, 122, 197, "Input",ExpressionUUID->"9f5c3d2a-ddcc-400e-a993-107d8d9f8a45"]
}, Closed]],
Cell[CellGroupData[{
Cell[158468, 3724, 288, 4, 33, "Subsection",ExpressionUUID->"b29f9ed1-b761-4ea7-ae28-b89bb04ea9a4"],
Cell[CellGroupData[{
Cell[158781, 3732, 286, 4, 31, "Subsubsection",ExpressionUUID->"eb10bf5f-1cb0-4c72-a42e-b65d28598421"],
Cell[159070, 3738, 394, 7, 55, "Text",ExpressionUUID->"6008383f-e9bc-4520-8d3b-128dcce1a0a4"],
Cell[159467, 3747, 1601, 41, 87, "Input",ExpressionUUID->"d3872068-9532-4afe-9b56-6b73104e2322"],
Cell[161071, 3790, 1643, 30, 100, "Input",ExpressionUUID->"3c080009-9b80-4d19-a17a-d03a86d4e635"]
}, Closed]],
Cell[CellGroupData[{
Cell[162751, 3825, 218, 3, 31, "Subsubsection",ExpressionUUID->"93cac2d3-8a1d-4271-b795-92d05d8dd75d"],
Cell[162972, 3830, 281, 4, 33, "Text",ExpressionUUID->"42c1ccb4-e0b8-40d3-a98d-b634bc990761"],
Cell[163256, 3836, 4709, 110, 376, "Input",ExpressionUUID->"d34324b3-1e0d-4aa7-952d-0971895d1704"],
Cell[167968, 3948, 295, 7, 33, "Text",ExpressionUUID->"e27e2496-8a48-472d-8bae-3cf9a65ff60e"],
Cell[168266, 3957, 765, 12, 43, "Input",ExpressionUUID->"af9bf1ca-9dcc-4235-bb66-287cf8f15270"],
Cell[169034, 3971, 513, 11, 43, "Input",ExpressionUUID->"9fea1278-6022-4c57-a27c-b41fa2efd5b3"]
}, Closed]],
Cell[CellGroupData[{
Cell[169584, 3987, 275, 4, 31, "Subsubsection",ExpressionUUID->"123b316b-ed0f-4574-b5c1-205047d7080f"],
Cell[169862, 3993, 366, 6, 33, "Text",ExpressionUUID->"2225e913-477c-4f83-945c-5328333edb83"],
Cell[170231, 4001, 963, 20, 43, "Input",ExpressionUUID->"3d635c72-399c-42f3-8adb-3c62e56ba2ba"],
Cell[171197, 4023, 760, 17, 43, "Input",ExpressionUUID->"5024c5e8-a0bf-4ce8-93a1-efa021bea3a9"],
Cell[171960, 4042, 924, 19, 43, "Input",ExpressionUUID->"61d8ce36-e4ea-49d7-ba03-4d9c7e2297a0"],
Cell[172887, 4063, 649, 15, 43, "Input",ExpressionUUID->"3aad7fc3-7d9e-40cf-bb80-a67f89e7e17c"],
Cell[173539, 4080, 359, 7, 33, "Text",ExpressionUUID->"b5d5239f-9214-4a33-8538-0103fdcf61c4"],
Cell[173901, 4089, 1009, 17, 43, "Input",ExpressionUUID->"ae341985-aae0-4b7c-830b-bde1203021b2"],
Cell[174913, 4108, 710, 13, 43, "Input",ExpressionUUID->"db5694fc-fcf3-4859-a534-0ffe3b830d63"],
Cell[175626, 4123, 974, 16, 43, "Input",ExpressionUUID->"b1bd7127-0839-49af-b73d-f39176201107"],
Cell[176603, 4141, 660, 12, 43, "Input",ExpressionUUID->"b24a64d1-eb93-40a0-a273-216c961b63ed"],
Cell[177266, 4155, 328, 7, 33, "Text",ExpressionUUID->"d286bdc9-b671-4dfe-ba35-81be9b6995e2"],
Cell[177597, 4164, 1448, 34, 66, "Input",ExpressionUUID->"958a0192-1e63-4175-a634-3ddf0d0c63df"],
Cell[179048, 4200, 1497, 34, 66, "Input",ExpressionUUID->"10512a55-8f6e-41f9-ba95-6200d0911ec3"]
}, Closed]]
}, Closed]],
Cell[CellGroupData[{
Cell[180594, 4240, 95, 1, 32, "Subsection",ExpressionUUID->"c4365b25-e6e7-47e7-92a2-4d727439ca2d"],
Cell[CellGroupData[{
Cell[180714, 4245, 343, 4, 31, "Subsubsection",ExpressionUUID->"65c00cea-df1c-4d83-82c8-39b8f1730fa1"],
Cell[CellGroupData[{
Cell[181082, 4253, 273, 5, 41, "Input",ExpressionUUID->"eb53f015-5b76-44b8-ad49-af72b009fe24"],
Cell[181358, 4260, 436, 10, 60, "Output",ExpressionUUID->"bc6a7877-f74c-4e51-b3a9-47f2254add0f"]
}, Open  ]],
Cell[CellGroupData[{
Cell[181831, 4275, 269, 5, 41, "Input",ExpressionUUID->"6dbd7b84-c61a-49b9-be74-1e5075184f23"],
Cell[182103, 4282, 684, 17, 72, "Output",ExpressionUUID->"bf52dab6-6c10-4b32-94a1-5fc6b1f37a11"]
}, Open  ]],
Cell[CellGroupData[{
Cell[182824, 4304, 269, 5, 41, "Input",ExpressionUUID->"2a64be8d-fbdc-49e6-aa22-39e8479129c5"],
Cell[183096, 4311, 878, 22, 72, "Output",ExpressionUUID->"0bdab766-3fd2-40a3-ac84-03cd65d3f2ec"]
}, Open  ]],
Cell[183989, 4336, 285, 6, 100, "Input",ExpressionUUID->"c4742cae-c5e1-4f7f-8419-a7e8d9358050"],
Cell[CellGroupData[{
Cell[184299, 4346, 1650, 39, 66, "Input",ExpressionUUID->"eb6282ca-5691-4bed-8352-68c3446c13ff"],
Cell[185952, 4387, 25217, 440, 727, "Output",ExpressionUUID->"b6ab4874-6920-4086-9049-ae4393d6d723"]
}, Open  ]]
}, Closed]],
Cell[CellGroupData[{
Cell[211218, 4833, 299, 4, 31, "Subsubsection",ExpressionUUID->"93cc4676-5aa4-40a5-a789-954166207fe5"],
Cell[211520, 4839, 1944, 28, 43, "Input",ExpressionUUID->"2a6ae5fd-166a-474d-a492-f8765e716839"],
Cell[213467, 4869, 454, 8, 43, "Input",ExpressionUUID->"e1799594-e287-409a-a2be-8d69f1b1fa0b"],
Cell[213924, 4879, 547, 9, 100, "Input",ExpressionUUID->"ee58f054-971a-4cc6-b39c-4a39c108f997"],
Cell[CellGroupData[{
Cell[214496, 4892, 2097, 51, 89, "Input",ExpressionUUID->"3474c70d-65f9-44bf-a95c-787f19de9b17"],
Cell[216596, 4945, 44971, 769, 379, 30014, 521, "CachedBoxData", "BoxData", "Output",ExpressionUUID->"d2847e4e-da53-4cb6-8e44-e52a8ad69290"]
}, Open  ]],
Cell[CellGroupData[{
Cell[261604, 5719, 1946, 51, 66, "Input",ExpressionUUID->"ecabad2a-0f75-4599-a0c6-4b7f94b06a15"],
Cell[263553, 5772, 14918, 268, 902, "Output",ExpressionUUID->"b348bbef-3c65-48dd-9de6-bb7eb4429a91"]
}, Open  ]]
}, Closed]]
}, Closed]]
}, Closed]],
Cell[CellGroupData[{
Cell[278544, 6048, 268, 5, 56, "Section",ExpressionUUID->"7bec3435-db0f-4025-ad34-b96cb848dd5b"],
Cell[CellGroupData[{
Cell[278837, 6057, 229, 3, 33, "Subsection",ExpressionUUID->"c85ba833-7fad-4645-8143-f3c4ec00864f"],
Cell[279069, 6062, 463, 8, 33, "Text",ExpressionUUID->"ff8f201b-c47e-4437-8826-b032106f3338"],
Cell[279535, 6072, 1895, 57, 104, "Input",ExpressionUUID->"1ac67da5-87fd-46ec-a821-6974edbb97d6"],
Cell[281433, 6131, 450, 8, 33, "Text",ExpressionUUID->"5b885f8a-5e64-484d-a061-ba4abedef068"],
Cell[281886, 6141, 6250, 143, 286, "Input",ExpressionUUID->"fe43391d-1337-49c0-82ad-f02fb0ad2044"]
}, Closed]],
Cell[CellGroupData[{
Cell[288173, 6289, 288, 4, 33, "Subsection",ExpressionUUID->"c35a7630-1136-47ea-98c0-eb4783b5f68c"],
Cell[CellGroupData[{
Cell[288486, 6297, 227, 3, 31, "Subsubsection",ExpressionUUID->"bd868d71-8677-45f8-a5ee-814ac258e7ec"],
Cell[288716, 6302, 364, 6, 33, "Text",ExpressionUUID->"22216966-4f10-4d90-9501-d69a5839a506"],
Cell[289083, 6310, 1576, 42, 87, "Input",ExpressionUUID->"420020c9-a28b-47cd-bfa5-430c1bcfee4c"],
Cell[290662, 6354, 1618, 29, 43, "Input",ExpressionUUID->"c1d1307f-5edc-4c95-acd8-f8fd2c1bc644"],
Cell[292283, 6385, 317, 6, 33, "Text",ExpressionUUID->"c971b0ab-09f3-45a2-a9e6-f1557c3256ba"],
Cell[292603, 6393, 1821, 47, 87, "Input",ExpressionUUID->"70505686-197a-4027-92b5-4ea3511e1275"],
Cell[294427, 6442, 1693, 30, 43, "Input",ExpressionUUID->"437d5ca2-88bc-4b73-b20d-818f558307ae"]
}, Closed]],
Cell[CellGroupData[{
Cell[296157, 6477, 267, 4, 31, "Subsubsection",ExpressionUUID->"cef6e36d-e3ff-43ad-83d4-281f2e4358e2"],
Cell[296427, 6483, 281, 4, 33, "Text",ExpressionUUID->"a64d18bd-47a3-46d0-8cfa-c3dc8c86b3f0"],
Cell[296711, 6489, 9086, 214, 632, "Input",ExpressionUUID->"8e950c20-6bf7-4299-8445-bfca950bfe24"],
Cell[305800, 6705, 237, 5, 33, "Text",ExpressionUUID->"d335fbe7-a28f-455d-973c-18138ad85e46"],
Cell[306040, 6712, 812, 14, 43, "Input",ExpressionUUID->"80d0ef69-4639-4f18-8a6c-bd1bbabb43a5"],
Cell[306855, 6728, 561, 11, 43, "Input",ExpressionUUID->"151bac71-df63-4252-8530-908a61e836eb"]
}, Closed]],
Cell[CellGroupData[{
Cell[307453, 6744, 275, 4, 31, "Subsubsection",ExpressionUUID->"9d72997f-bf42-47f8-ac5b-812d5c17317e"],
Cell[307731, 6750, 393, 7, 33, "Text",ExpressionUUID->"ac032bd2-4463-418f-990b-92e91ed32374"],
Cell[308127, 6759, 963, 20, 43, "Input",ExpressionUUID->"a53739ce-2882-47c9-8092-c778a5dab4a8"],
Cell[309093, 6781, 760, 17, 43, "Input",ExpressionUUID->"2bdcef6d-955e-4cac-a841-07b2151879e1"],
Cell[309856, 6800, 926, 19, 43, "Input",ExpressionUUID->"4716d896-a704-47cc-8e6a-7cf0760910c5"],
Cell[310785, 6821, 649, 15, 43, "Input",ExpressionUUID->"794465ad-7908-4516-8926-e96f8457f574"],
Cell[311437, 6838, 359, 7, 33, "Text",ExpressionUUID->"4c8821fb-712e-4a48-abae-6f876f723f6b"],
Cell[311799, 6847, 1011, 17, 43, "Input",ExpressionUUID->"3847635b-25db-48db-8946-bb089b407232"],
Cell[312813, 6866, 709, 13, 43, "Input",ExpressionUUID->"14dc1bd3-4d3b-4cd9-97d4-052be3e44d84"],
Cell[313525, 6881, 976, 16, 43, "Input",ExpressionUUID->"fcc79df5-e5b0-40b3-bab5-5dbb48f255be"],
Cell[314504, 6899, 662, 12, 43, "Input",ExpressionUUID->"6eca558c-c899-489a-a5c4-bc51e8766b80"],
Cell[315169, 6913, 333, 6, 33, "Text",ExpressionUUID->"b94b1e65-db5e-4cfa-b863-fbe2eaae323c"],
Cell[315505, 6921, 1456, 34, 66, "Input",ExpressionUUID->"c85f701e-ff58-4332-84de-1a09457ead83"],
Cell[316964, 6957, 1523, 35, 66, "Input",ExpressionUUID->"6200297b-9c61-4dc7-b7ae-5bacb7ea2939"]
}, Closed]]
}, Closed]],
Cell[CellGroupData[{
Cell[318536, 6998, 95, 1, 32, "Subsection",ExpressionUUID->"9ad52a99-d894-44c8-85f2-4700126626ca"],
Cell[CellGroupData[{
Cell[318656, 7003, 422, 5, 31, "Subsubsection",ExpressionUUID->"9bf4b054-3f29-4193-bc7f-707ea8bb404e"],
Cell[CellGroupData[{
Cell[319103, 7012, 271, 5, 41, "Input",ExpressionUUID->"fc86f042-9644-4f7a-8f0a-68d6ea8ad6a7"],
Cell[319377, 7019, 503, 13, 64, "Output",ExpressionUUID->"3cc1146f-94cb-4f96-9d2b-7efb5a55675a"]
}, Open  ]],
Cell[CellGroupData[{
Cell[319917, 7037, 320, 6, 41, "Input",ExpressionUUID->"5194ecf4-723b-4b5a-bc20-9925e6103a0f"],
Cell[320240, 7045, 813, 22, 72, "Output",ExpressionUUID->"d9664f80-2ffd-437c-9755-c0fa252b83a0"]
}, Open  ]],
Cell[CellGroupData[{
Cell[321090, 7072, 320, 6, 41, "Input",ExpressionUUID->"cead788b-d412-471e-99dd-3d6eea6b8c64"],
Cell[321413, 7080, 975, 25, 72, "Output",ExpressionUUID->"1717aaec-7ce7-4024-a081-eb91640d7c75"]
}, Open  ]],
Cell[322403, 7108, 282, 6, 100, "Input",ExpressionUUID->"9579b6da-1868-447e-921d-e15bf01bfe44"],
Cell[CellGroupData[{
Cell[322710, 7118, 1761, 40, 66, "Input",ExpressionUUID->"6937658b-d562-4d29-bd07-5549353e7b5c"],
Cell[324474, 7160, 25559, 442, 589, "Output",ExpressionUUID->"7c56d23b-e309-4238-912a-d6e2c00b5677"]
}, Open  ]]
}, Closed]],
Cell[CellGroupData[{
Cell[350082, 7608, 255, 3, 31, "Subsubsection",ExpressionUUID->"8f71a35b-235a-4857-ac99-17491838debd"],
Cell[350340, 7613, 2048, 30, 43, "Input",ExpressionUUID->"246b5830-7237-4c26-a048-ee886345576d"],
Cell[352391, 7645, 501, 9, 43, "Input",ExpressionUUID->"f43dad37-d942-4fa2-9f22-33f3ababc2d9"],
Cell[352895, 7656, 506, 9, 100, "Input",ExpressionUUID->"b6711c56-713c-4c19-9b59-12bc0c2eaaac"],
Cell[CellGroupData[{
Cell[353426, 7669, 1804, 49, 66, "Input",ExpressionUUID->"3f33a1f0-97c2-4159-919e-30955519f7dc"],
Cell[355233, 7720, 19653, 347, 367, "Output",ExpressionUUID->"bd8a64a5-da92-4839-b06c-0cd4f990e91f"]
}, Open  ]]
}, Closed]]
}, Closed]],
Cell[CellGroupData[{
Cell[374947, 8074, 241, 3, 33, "Subsection",ExpressionUUID->"c28df2ed-2ca3-42af-9ece-9bea5c8a50ff"],
Cell[375191, 8079, 525, 8, 33, "Text",ExpressionUUID->"b7098de8-f33b-451d-8dd2-3419912c8362"],
Cell[CellGroupData[{
Cell[375741, 8091, 252, 3, 31, "Subsubsection",ExpressionUUID->"4ab73879-9410-47fa-96fb-b2c6c9f52314"],
Cell[375996, 8096, 285, 6, 33, "Text",ExpressionUUID->"64e35584-23db-44aa-8883-bce4e636750f"],
Cell[CellGroupData[{
Cell[376306, 8106, 1466, 31, 43, "Input",ExpressionUUID->"1e339f5a-05d6-4d50-9a74-67795f08b88a"],
Cell[377775, 8139, 14754, 259, 295, "Output",ExpressionUUID->"2bd0df48-3a76-4e0c-83b4-d4d5a07787ae"]
}, Open  ]],
Cell[392544, 8401, 228, 3, 33, "Text",ExpressionUUID->"290c428f-d950-4c3e-92fb-13c3b16e2ad2"],
Cell[CellGroupData[{
Cell[392797, 8408, 1096, 31, 43, "Input",ExpressionUUID->"07fa85bd-61a4-443f-9aab-2be80923c297"],
Cell[393896, 8441, 40523, 681, 468, "Output",ExpressionUUID->"a17d6608-be18-43cc-8a23-55d4ee6ec05f"]
}, Open  ]],
Cell[434434, 9125, 363, 6, 33, "Text",ExpressionUUID->"443387ff-8edf-4e35-b79c-d9ee65d682d3"],
Cell[CellGroupData[{
Cell[434822, 9135, 1752, 47, 66, "Input",ExpressionUUID->"def1f06e-b617-44b0-bcef-02fe16635c25"],
Cell[436577, 9184, 36113, 620, 284, "Output",ExpressionUUID->"c451b0a2-1f65-4c68-9b7a-d724751368fd"]
}, Open  ]],
Cell[472705, 9807, 345, 6, 33, "Text",ExpressionUUID->"d7a3536a-a6ce-426e-9b2c-0f6461f2950c"],
Cell[CellGroupData[{
Cell[473075, 9817, 1679, 46, 66, "Input",ExpressionUUID->"56758a2f-0693-48da-b07a-e8d9a704d695"],
Cell[474757, 9865, 26303, 451, 273, "Output",ExpressionUUID->"04e27018-f2a1-4537-8691-cde893063804"]
}, Open  ]],
Cell[501075, 10319, 686, 14, 55, "Text",ExpressionUUID->"43a9a55d-8908-4056-bbb4-0475eed09d57"]
}, Closed]],
Cell[CellGroupData[{
Cell[501798, 10338, 255, 3, 31, "Subsubsection",ExpressionUUID->"1e60e3fa-b84a-4481-9ab2-661cb52db7e0"],
Cell[502056, 10343, 364, 7, 33, "Text",ExpressionUUID->"1ed531db-5e19-4488-9691-e03dae47fda4"],
Cell[CellGroupData[{
Cell[502445, 10354, 1773, 50, 89, "Input",ExpressionUUID->"241ae2f1-5900-4507-8c71-000265f7fab0"],
Cell[504221, 10406, 39096, 661, 439, "Output",ExpressionUUID->"33f60251-f377-43c0-bc28-e1c104aa23b8"]
}, Open  ]],
Cell[543332, 11070, 265, 5, 33, "Text",ExpressionUUID->"85e4b010-1f1e-4f56-93fd-9ea6b3f17180"],
Cell[CellGroupData[{
Cell[543622, 11079, 2078, 57, 112, "Input",ExpressionUUID->"002aa746-f63f-4172-a35c-d2924a5a85eb"],
Cell[545703, 11138, 52571, 880, 370, "Output",ExpressionUUID->"6d4948f0-aec9-4070-a71f-d2e85420c500"]
}, Open  ]],
Cell[598289, 12021, 751, 15, 99, "Text",ExpressionUUID->"aaadf83d-2ca4-4a93-94a2-291ab761160f"]
}, Closed]]
}, Closed]]
}, Closed]]
}, Open  ]]
}, Open  ]]
}
]
*)
